# Supplementary material for: Location and topology of the fundamental gap in photonic crystals
Source: arXiv:2106.10267 source file (2021-11-20)
Supplement: Supplementary file 1 [file supp.pdf]

# SUPPLEMENTAL MATERIAL

## Location and topology of the fundamental gap in photonic crystals

Thomas Christensen,<sup>1,\*</sup> Hoi Chun Po,<sup>1,2</sup> John D. Joannopoulos,<sup>1</sup> and Marin Soljačić<sup>1</sup>

<sup>1</sup>Research Laboratory of Electronics, Massachusetts Institute of Technology, Cambridge, Massachusetts 02139, USA

<sup>2</sup>Department of Physics, Hong Kong University of Science and Technology, Clear Water Bay, Hong Kong, China

### CONTENTS

|                                                           |    |                                                                 |    |
|-----------------------------------------------------------|----|-----------------------------------------------------------------|----|
| S1. Compatibility-allowed band structures                 | 1  | S5. Higher-order minimum-connectivity solutions                 | 15 |
| S2. Computational details                                 | 7  | S6. $\Gamma$ -enforced bosonic topology of regular bands        | 15 |
| S3. Invariance of singular transverse topological indices | 12 | S7. Dielectric obstructions in space group 230 (Ia $\bar{3}$ d) | 19 |
| S4. Time-reversal broken $\Gamma$ -enforced topology      | 13 | Supplemental References                                         | 21 |
|                                                           |    | S8. Tables                                                      | 23 |

### S1. COMPATIBILITY-ALLOWED BAND STRUCTURES

This section reviews salient features of the relations between the spaces of trivial atomic band structures {AI} and the spaces of all compatibility-allowed (or physically realizable) band structures {BS}, specifically in the context of their symmetry content. Special emphasis is placed on motivating the physical and mathematical background necessary to derive the Hilbert basis for {BS}.

For comprehensive reviews of the ideas underlying topological quantum chemistry and symmetry indicators, see e.g., Refs. S1 and S2 or the publications referenced below.

#### A. Symmetry vectors

As in the main text, we define the symmetry vector of a grouping of  $\mu$  bands by

$$\mathbf{n} \equiv [n_{\mathbf{k}_1}^\alpha, n_{\mathbf{k}_1}^\beta, \dots, n_{\mathbf{k}_i}^{\alpha'}, n_{\mathbf{k}_i}^{\beta'}, \dots, \mu]^T, \quad (\text{S1})$$

where  $n_{\mathbf{k}_i}^\alpha$  denotes the multiplicity of the  $\alpha$ th (small) irreducible representation (irrep) at  $\mathbf{k}_i$ . We denote the number\* of elements in  $\mathbf{n}$  by  $N^{\text{irr}}$  and emphasize that symmetry data must be integral, i.e.,  $\mathbf{n} \in \mathbb{Z}^{N^{\text{irr}}}$  (*physical* symmetry data must additionally be non-negative, so that, more precisely,  $\mathbf{n} \in \mathbb{N}^{N^{\text{irr}}}$ ).

We will often take the perspective that  $\mathbf{n}$  is the concatenation of projections of symmetry data at individual  $\mathbf{k}$ -points, i.e., as

$$\mathbf{n} = [\mathbf{n}_{\mathbf{k}_1}^T, \dots, \mathbf{n}_{\mathbf{k}_i}^T, \dots, \mu]^T, \quad (\text{S2})$$

with  $\mathbf{n}_{\mathbf{k}_i} \equiv [n_{\mathbf{k}_i}^\alpha, n_{\mathbf{k}_i}^\beta, \dots]^T$  denoting the projection of  $\mathbf{n}$  onto the symmetry data at  $\mathbf{k}_i$ .

As an example, plane group 17 (p6mm) has three inequivalent high-symmetry  $\mathbf{k}$ -points  $\Gamma$ ,  $K$ , and  $M$ , with 6, 3 and 4 irreps each, respectively. Its associated symmetry vector has 14 components, namely

---

\* [tchr@mit.edu](mailto:tchr@mit.edu)

\* We abuse notation slightly and define  $N^{\text{irr}} \equiv \tilde{N}^{\text{irr}} + 1$  with  $\tilde{N}^{\text{irr}}$  denoting the actual number of distinct irreps sampled in  $\mathbf{n}$ . The plus one term accounts for our inclusion of the band filling  $\mu$  in  $\mathbf{n}$ .

$\mathbf{n} = [n_{\Gamma_1}, n_{\Gamma_2}, n_{\Gamma_3}, n_{\Gamma_4}, n_{\Gamma_5}, n_{\Gamma_6}, n_{K_1}, n_{K_2}, n_{K_3}, n_{M_1}, n_{M_2}, n_{M_3}, n_{M_4}, \mu]^T$ . In specifying symmetry vectors, we will generally favor the “projected” representation of Eq. (S2) for clarity: thus, we will e.g. write the two-band symmetry vector  $[0, 0, 0, 0, 1, 0, 0, 0, 1, 1, 1, 0, 0, 2]^T$  as  $[\Gamma_5, K_3, M_1 + M_2, 2]^T$ .

We note parenthetically that symmetry *vectors* is a slight misnomer since  $\mathbf{n}$  is not an element of a vector space (it cannot be arbitrarily scaled) but rather of a  $\mathbb{Z}$ -module or a monoid, depending on context. Using vector-terminology for non-vectors is a well-established tradition in physics (e.g., Burgers vector), however, and risks little confusion.

## B. The space of trivial atomic insulators {AI}

The set of elementary band representations (EBRs)  $\{\mathbf{a}_i\}_{i=1}^{N^{\text{EBR}}}$  [S3; S4; S5] defines a non-negative integer coefficient basis for all band structures induced by the stacking of symmetric, localized Wannier orbitals—i.e., for the “space” of atomic insulators {AI}—which we nominally identify with topologically trivial bands [S6; S7; S8]. Concretely, the symmetry vectors  $\mathbf{n}$  of such trivial bands can be expanded as

$$\mathbf{n} = \sum_{i=1}^{N^{\text{EBR}}} c_i \mathbf{a}_i = \mathbf{A} \mathbf{c}, \quad (\text{S3})$$

with  $c_i \in \mathbb{N} \equiv \{0, 1, \dots\}$  and  $\mathbf{a}_i \in \mathbb{N}^{N^{\text{irr}}}$ ; at the second equality sign, we give the equivalent matrix definition, specified in terms of the  $N^{\text{irr}} \times N^{\text{EBR}}$  matrix  $\mathbf{A} \equiv [\mathbf{a}_1, \mathbf{a}_2, \dots, \mathbf{a}_{N^{\text{EBR}}}]$  of column-wise EBR vectors and the coefficient vector  $\mathbf{c} \equiv [c_1, \dots, c_{N^{\text{EBR}}}]^T$ . Note that the expansion coefficients are not unique in general since the EBRs are not necessarily linearly independent.

Tabulated EBRs can be obtained from the Bilbao Crystallographic Database (BCD) [S9; S10] or computed ab initio [S11]. We used BCD’s tabulated EBRs accessed through `Crystalline.jl` [S12].

## C. The space of band structures {BS}

Having identified {AI} with the non-negative integer-coefficient  $\text{span}^*$  of EBRs  $\{\mathbf{a}_i\}$ , we seek a similar construction for the set of all band structures {BS}. To that end, we first define the properties of symmetry vectors belonging to {BS}, namely:

*Compatibility.* Any element of {BS} must fulfill all compatibility relations across the Brillouin zone (BZ).

In practice, this can be cast a set of linear constraints via the matrix equation [S6; S7]:

$$\mathbf{C} \mathbf{n} = \mathbf{0}, \quad (\text{S4})$$

where  $\mathbf{C}$  is a matrix that incorporates all relevant compatibility constraints<sup>†</sup> (as well as “filling” constraints, i.e., the requirement that  $\mathbf{n}$  contains a definite number of bands).

\* We will occasionally abuse terminology slightly by referring to *spaces* and *spans*, since neither {AI} nor {BS} in fact constitute vector spaces (lacking both additive inverses and completeness under multiplication by scalars)—but rather are monoids. When referring to non-negative integer-coefficient spans we implicitly intend a notion of integer conical combinations—in the sense that e.g.,  $\{\text{AI}\} = \mathbb{N}\{\mathbf{a}_i\} \equiv \{\sum_i c_i \mathbf{a}_i \mid c_i \in \mathbb{N}\}$  (in the notation of Ref. S13).

† It is worthwhile to briefly review the construction of  $\mathbf{C}$  in a simplified setting. To that end, we consider space group 16 and restrict our attention to a subset of the applicable compatibility relations: namely to constraints between the  $\mathbf{k}$ -points at  $\Gamma = [0, 0, 0]^T$  and  $X = [1/2, 0, 0]^T$ . These points have identical little groups (with operations  $\{1, 2_{100}, 2_{010}, 2_{001}\}$  and irreps  $(\Gamma_{1,2,3,4} \text{ and } X_{1,2,3,4})$  and are connected by the line  $\Sigma = [\alpha, 0, 0]^T$  (with little group operation  $\{1, 2_{100}\}$  and irreps  $\Sigma_{1,2}$ ). The little groups at  $\Gamma$ ,  $X$ , and  $\Sigma$  all share the  $2_{100}$  operation. This fact implies a compatibility constraint: namely, that the symmetry eigenvalue of the  $2_{100}$  operation remains invariant as we move from  $\Gamma$  to  $\Sigma$  to  $X$  (assuming that we move adiabatically within a single band). Since  $2_{100}$  squares to unity, its symmetry eigenvalues can be either +1 (even) or −1 (odd). The  $\Gamma_{1,3}$ ,  $X_{1,3}$ , and  $\Sigma_1$  irreps all transform evenly under  $2_{100}$  while  $\Gamma_{2,4}$ ,  $X_{2,4}$ , and  $\Sigma_2$  transform oddly. Then, if a band e.g., exhibits the  $\Gamma_1$  irrep at  $\Gamma$ , it must therefore “subduce” into the  $\Sigma_1$  irrep if we move towards  $X$  along  $\Sigma$ . In total, there are 8 such subduction relations:

$$\begin{aligned} \Gamma_1 &\rightarrow \Sigma_1, & \Gamma_3 &\rightarrow \Sigma_1, & X_1 &\rightarrow \Sigma_1, & X_3 &\rightarrow \Sigma_1, \\ \Gamma_2 &\rightarrow \Sigma_2, & \Gamma_4 &\rightarrow \Sigma_2, & X_2 &\rightarrow \Sigma_2, & X_4 &\rightarrow \Sigma_2. \end{aligned}$$

*Physicality.* Any element of  $\{\text{BS}\}$  must refer to a physically realizable and well-defined set of symmetries, i.e., the elements of any associated symmetry vector must be non-negative integers:

$$n_j \in \mathbb{N}, \quad \forall j = 1, \dots, N^{\text{irr}}. \quad (\text{S5})$$

Put differently,  $\{\text{BS}\}$  is the non-negative integral subset of the null space of  $\mathbf{C}$ .

To arrive at a set of generators for  $\{\text{BS}\}$ , it is helpful to initially consider a “quasi-physical” set  $\{\overline{\text{BS}}\}$ , distinguished from  $\{\text{BS}\}$  by relaxing Eq. (S5) to allow negative symmetry data, i.e., allowing  $n_j \in \mathbb{Z}$  (later, in Supplemental Section S1.D, we will extract  $\{\text{BS}\}$  from  $\{\overline{\text{BS}}\}$  via cone intersection). Unlike  $\{\text{BS}\}$ ,  $\{\overline{\text{BS}}\}$  defines a group under addition (or a lattice embedded in  $\mathbb{Z}^{N^{\text{irr}}}$ ), since each element has an additive inverse.\* Analogously, we can define the group “extension” of  $\{\text{AI}\}$  from the integer span of EBRs.

$$\{\overline{\text{AI}}\} \equiv \left\{ \sum_{i=1}^{d^{\text{AI}}} c_i \mathbf{a}_i \mid c_i \in \mathbb{Z} \right\}, \quad (\text{S6})$$

where  $d^{\text{AI}} (\leq N^{\text{EBR}})$  denotes the dimension of the span, i.e., the number of linearly independent vectors in  $\{\mathbf{a}_i\}$ . As a first step, we seek an analogous basis for  $\{\overline{\text{BS}}\}$ , i.e., a basis  $\{\mathbf{b}_i\}$  with  $d^{\text{BS}}$  elements:

$$\{\overline{\text{BS}}\} \equiv \left\{ \sum_{i=1}^{d^{\text{BS}}} c_i \mathbf{b}_i \mid c_i \in \mathbb{Z} \right\}. \quad (\text{S7})$$

To find this basis—without explicitly constructing the compatibility matrix  $\mathbf{C}$ —we first observe that every EBR  $\mathbf{a}_{i'}$  automatically fulfills Eq. (S4), i.e., that  $\mathbf{C}\mathbf{a}_{i'} = \mathbf{0}$ . Accordingly, every linear combination of  $\{\mathbf{a}_{i'}\}$  also automatically respects Eq. (S4) since  $\mathbf{C} \sum_{i'} q_{i'} \mathbf{a}_{i'} = \sum_{i'} q_{i'} (\mathbf{C}\mathbf{a}_{i'})$  [S2; S7]. Crucially, we do not require that the coefficients  $q_{i'}$  are integers—only that their span over  $\{\mathbf{a}_{i'}\}$  is. In practice,  $q_{i'}$  are a subset of the rationals  $\mathbb{Q}$ .

Before discussing a general method for determining this subset, it is instructive to consider a simple example. To that end, consider space group 110 (I4<sub>cd</sub>) without time-reversal symmetry, which has just two EBRs (induced by  $s$ - and  $p$ -orbitals, respectively, at the 8a Wyckoff position):

$$\mathbf{a}_1 = \begin{bmatrix} \Gamma_1 + \Gamma_2 + \Gamma_3 + \Gamma_4 \\ M_1 + M_2 + M_3 + M_4 \\ 2P_1 \\ 2X_1 \\ 2N_1 + 2N_2 \\ 4 \text{ bands} \end{bmatrix}, \quad \mathbf{a}_2 = \begin{bmatrix} 2\Gamma_5 \\ 2M_5 \\ 2P_1 \\ 2X_1 \\ 2N_1 + 2N_2 \\ 4 \text{ bands} \end{bmatrix}. \quad (\text{S8})$$

From inspection, we see that  $\mathbf{a}_1$  and  $\mathbf{a}_2$  are linearly independent and that the greatest common denominator among their elements are  $\text{gcd}(\mathbf{a}_1) = 1$  and  $\text{gcd}(\mathbf{a}_2) = 2$ . This implies that there are two linearly independent sets of  $\{q_{i'}\}$  whose combinations with  $\{\mathbf{a}_{i'}\}$  produce integer symmetry data, namely  $\{q_1 = 1, q_2 = 0\}$  and  $\{q_1 = 0, q_2 = \frac{1}{2}\}$ . As a result, all integer combinations of  $\mathbf{a}_1$  and  $\frac{1}{2}\mathbf{a}_2$  belong to  $\{\overline{\text{BS}}\}$ , and we can identify  $\mathbf{b}_1 = \mathbf{a}_1$  and  $\mathbf{b}_2 = \frac{1}{2}\mathbf{a}_2 = [\Gamma_5, M_5, P_1, X_1, N_1 + N_2, 2]^T$ . On the other hand,  $\mathbf{b}_2$  (and its odd multiples) clearly does not belong to  $\{\overline{\text{AI}}\}$ ; accordingly, it must correspond to a topologically nontrivial state.

At this point, it is of course not clear whether  $\mathbf{b}_1$  and  $\mathbf{b}_2$  span all of  $\{\overline{\text{BS}}\}$  or merely a subset of it. As shown by explicit evaluation of the integer null space of  $\mathbf{C}$  in Ref. S7, however, the dimension  $d^{\text{BS}}$  of  $\{\overline{\text{BS}}\}$  (i.e., the nullity of  $\mathbf{C}$ ) is exactly equal to the dimension  $d^{\text{AI}} \leq N^{\text{EBR}}$  of  $\{\overline{\text{AI}}\}$  (i.e., the dimension of the column space of  $\mathbf{A}$  or the number of linearly independent vectors in  $\{\mathbf{a}_i\}$ ) for all space groups. For our present example  $d^{\text{AI}} = N^{\text{EBR}} = 2$ , implying that  $\{\overline{\text{BS}}\}$  is indeed spanned by just  $\mathbf{b}_1$  and  $\mathbf{b}_2$ .

---

We can cast these relations as linear constraints on the irrep multiplicities  $\mathbf{n}_\Gamma = [n_{\Gamma_1}, n_{\Gamma_2}, n_{\Gamma_3}, n_{\Gamma_4}]^T$  and  $\mathbf{n}_X = [n_{X_1}, n_{X_2}, n_{X_3}, n_{X_4}]^T$  by “summing up” similar constraints, leading to the relations  $n_{\Gamma_1} + n_{\Gamma_3} = n_{X_1} + n_{X_3}$  and  $n_{\Gamma_2} + n_{\Gamma_4} = n_{X_2} + n_{X_4}$ . Finally, defining  $\mathbf{n} = [\mathbf{n}_\Gamma, \mathbf{n}_X]^T$ , the constraints can be cast as the matrix equation  $\mathbf{C}\mathbf{n} = \mathbf{0}$  with  $\mathbf{C} = \begin{bmatrix} 1 & 0 & 1 & 0 & -1 & 0 & -1 & 0 \\ 0 & 1 & 0 & 1 & 0 & -1 & 0 & -1 \end{bmatrix}$ . Additional constraints can be incorporated by appending rows to  $\mathbf{C}$ .

\* More precisely,  $\{\text{BS}\}$  and  $\{\overline{\text{AI}}\}$  are modules over the ring of integers—distinguished from the more familiar notion of vector spaces by having scalars drawn from a ring (here,  $\mathbb{Z}$ ) rather than a field (say,  $\mathbb{R}$  or  $\mathbb{C}$ ).

*Smith normal decomposition.* Extracting the coefficients  $\{q_i\}$  is usually more subtle than in the above example since valid expansions may require superpositions of fractional EBRs (e.g., we might have  $\mathbf{b}_2 = \frac{1}{2}\mathbf{a}_1 + \frac{1}{2}\mathbf{a}_2 \in \mathbb{Z}^{N^{\text{irr}}}$  even if  $\frac{1}{2}\mathbf{a}_1 \notin \mathbb{Z}^{N^{\text{irr}}}$  and  $\frac{1}{2}\mathbf{a}_2 \notin \mathbb{Z}^{N^{\text{irr}}}$ ; i.e., considering only  $\mathbf{b}_i = \mathbf{a}_i / \gcd(\mathbf{a}_i)$  will not lead to the most general base-cases). To overcome this subtlety, we may remind ourselves that  $\{\mathbf{b}_i\}$  are the basis vectors whose integer combinations generate the non-negative integer-valued column space of  $\mathbf{A} = [\mathbf{a}_1, \mathbf{a}_2, \dots, \mathbf{a}_{N^{\text{EBR}}}]$ .

The so-called Smith normal decomposition provides a general approach to extract basis vectors for this kind of column space [S2; S7; S14]. This decomposition is well-defined for any rectangular integer-valued matrix (more generally, for matrices over an ideal principal domain) [S15], i.e., also for our  $N^{\text{irr}} \times N^{\text{EBR}}$  matrix  $\mathbf{A}$ , and takes the form\*

$$\mathbf{A} = \mathbf{S}\mathbf{\Lambda}\mathbf{T}, \quad (\text{S9})$$

where  $\mathbf{S}$  and  $\mathbf{T}$  are  $N^{\text{irr}} \times N^{\text{irr}}$  and  $N^{\text{EBR}} \times N^{\text{EBR}}$  integer-valued and unimodular<sup>†</sup> matrices and  $\mathbf{\Lambda}$  is an  $N^{\text{irr}} \times N^{\text{EBR}}$  integer-valued diagonal matrix (the Smith normal form of  $\mathbf{A}$ ). The diagonal of  $\mathbf{\Lambda}$  contains exactly  $d^{\text{AI}} \leq \min(N^{\text{irr}}, N^{\text{EBR}})$  nonzero elements  $\lambda_i$  (the *elementary divisors* or *invariant factors* of  $\mathbf{A}$ ) such that  $\text{diag}(\mathbf{\Lambda}) \equiv [\lambda_1, \dots, \lambda_{d^{\text{AI}}}, 0, \dots, 0]^T$  with  $\lambda_{i+1}$  divisible by  $\lambda_i$ .<sup>‡</sup>

The relevance of the Smith normal decomposition in our context is that the integer combinations of the first  $d^{\text{AI}}$  columns of  $\mathbf{S}$  spans the integer-valued column space of  $\mathbf{A}$  (the null space of  $\mathbf{A}$ , on the hand, is spanned by the last  $N^{\text{EBR}} - d^{\text{AI}}$  columns of  $\mathbf{T}^{-1}$ , cf. the zero-entries on the lower diagonal of  $\mathbf{\Lambda}$ )—and, so, equivalently, define a basis for  $\{\overline{\text{BS}}\}$  (since  $d^{\text{BS}} = d^{\text{AI}}$ ). Denoting the columns of  $\mathbf{S}$  by  $\mathbf{s}_i$  we then identify  $\mathbf{b}_i = \mathbf{s}_i$  for  $i \in \{1, \dots, d^{\text{AI}}\}$ , or equivalently say that  $\{\overline{\text{BS}}\}$  is spanned by the integer combinations of the columns of

$$\mathbf{B} \equiv [\mathbf{b}_1, \dots, \mathbf{b}_{d^{\text{BS}}}] = [\mathbf{s}_1, \dots, \mathbf{s}_{d^{\text{BS}}}] \quad (\text{S10})$$

The Smith decomposition also gives us the valid rational expansion coefficients  $\{q_i\}$ . To see this, we first define the  $N^{\text{EBR}} \times d^{\text{BS}}$  rational matrix  $\mathbf{Q} = [\mathbf{q}_1, \dots, \mathbf{q}_{d^{\text{BS}}}]$  whose columns  $\mathbf{q}_i = [q_{1,i}, \dots, q_{N^{\text{irr}},i}]^T$  give the expansion coefficients for  $\mathbf{b}_i$  in the basis of  $\{\mathbf{a}_i\}$ , i.e., such that  $\mathbf{B} = \mathbf{A}\mathbf{Q}$ . We then note that Eq. (S9) implies  $\mathbf{S}\mathbf{\Lambda} = \mathbf{A}\mathbf{T}^{-1}$ . Next, since  $\mathbf{\Lambda}$  is diagonal we can project this column-by-column to  $(\mathbf{S}\mathbf{\Lambda})_i = \mathbf{s}_i\lambda_i = (\mathbf{A}\mathbf{T}^{-1})_i = \mathbf{A}\mathbf{t}_i^{-1}$  where  $\mathbf{t}_i^{-1}$  denotes the  $i$ th column of  $\mathbf{T}^{-1}$ . Finally, we recall that  $\mathbf{B}$  is equal to the first  $d^{\text{AI}}$  columns of  $\mathbf{S}$ , i.e., that  $\mathbf{b}_i = \mathbf{s}_i$ , so that  $\mathbf{b}_i = \mathbf{A}\mathbf{t}_i^{-1}/\lambda_i$  which in turn implies  $\mathbf{B} = \mathbf{A}\mathbf{Q}$  with  $\mathbf{q}_i = \mathbf{t}_i^{-1}/\lambda_i$ . Since  $\mathbf{t}_i$  are integer-valued ( $\mathbf{T}$  is a unimodular matrix over  $\mathbb{Z}$ ), we see that fractional expansion coefficients—and associated nontrivial topology—arise exactly when  $\lambda_i \neq 1$ .<sup>§</sup>

## D. Monoids and Hilbert bases

With  $\{\overline{\text{BS}}\}$  in hand, we return to the problem of obtaining a basis for  $\{\text{BS}\}$ . We remind that  $\{\overline{\text{BS}}\}$  differs from  $\{\text{BS}\}$  only by allowing negative symmetry data, i.e., by not enforcing Eq. (S5). We can visualize the

\* We compute the decomposition using a freely available implementation in the Julia programming language [S16].

<sup>†</sup> Unimodular matrices over the integers have determinants of  $\pm 1$ . This implies that the inverse matrices  $\mathbf{S}^{-1}$  and  $\mathbf{T}^{-1}$  are also integer-valued, i.e.,  $(\mathbf{S}^{-1})_{ij}, (\mathbf{T}^{-1})_{ij} \in \mathbb{Z}$  (as can be seen e.g., from Cramer's rule and the fact that  $\det \mathbf{A} = \pm 1$  implies  $\det \mathbf{A}^{-1} = (\det \mathbf{A})^{-1} = \pm 1$ ).  $\mathbf{S}$  and  $\mathbf{T}$  are therefore elements of  $\text{GL}_{N^{\text{irr}}}(\mathbb{Z})$  and  $\text{GL}_{N^{\text{EBR}}}(\mathbb{Z})$ ; the general linear group over the ring of integers. An important consequence of this is that  $\mathbf{z} = \mathbf{S}^{-1}\mathbf{n}$  is necessarily a vector over the integers since  $n_i \in \mathbb{N}$ .

<sup>‡</sup> The decomposition is unique up to signs; we pick a convention of non-negative  $\lambda_i$ , i.e.,  $\lambda_i \in \mathbb{N}$ .

<sup>§</sup> The Smith normal decomposition can also be used to test whether a symmetry vector  $\mathbf{n}$  is in  $\{\overline{\text{BS}}\}$  (i.e., whether it fulfills the compatibility relations). Specifically, denoting by  $\tilde{\mathbf{S}}$  ( $\tilde{\mathbf{S}}^{-1}$ ) the first  $d^{\text{AI}}$  columns (rows) of  $\mathbf{S}$  ( $\mathbf{S}^{-1}$ ),  $\mathbf{n}$  is in  $\{\overline{\text{BS}}\}$  if and only if  $\tilde{\mathbf{S}}\mathbf{S}^{-1}\mathbf{n} - \mathbf{n} = \mathbf{0}$ , which can be derived from the ansatz  $\tilde{\mathbf{S}}\mathbf{c} = \mathbf{n}$  and noting that  $\mathbf{S}^{-1}\tilde{\mathbf{S}} = \mathbf{I}$  (i.e.,  $\mathbf{S}^{-1}$  is a left-inverse of  $\tilde{\mathbf{S}}$ —although not generally a right-inverse).

Similarly, the decomposition can be used to test whether a symmetry vector in  $\{\overline{\text{BS}}\}$  is also in  $\{\overline{\text{AI}}\}$ , i.e., whether it is topologically trivial [S14]. Specifically, if  $\mathbf{n}$  is in  $\{\overline{\text{AI}}\}$  it can be written as  $\mathbf{n} = \tilde{\mathbf{S}}\tilde{\mathbf{\Lambda}}\mathbf{c}$  with  $\mathbf{c} \in \mathbb{Z}^{d^{\text{AI}}}$ . Accordingly,  $\mathbf{n}$  is trivial (or possibly topologically fragile [S17]) if and only if all  $c_i = (\tilde{\mathbf{S}}^{-1}\mathbf{n})_i/\lambda_i \in \mathbb{Z}$ , or, equivalently, if  $(\tilde{\mathbf{S}}^{-1}\mathbf{n})_i \equiv 0 \pmod{\lambda_i}$  for all  $i = 1, \dots, d^{\text{AI}}$ . An equivalent approach involves the generalized inverse  $\mathbf{A}^g = \mathbf{T}^{-1}\mathbf{\Lambda}^g\mathbf{S}^{-1}$  of  $\mathbf{A}$  ( $\mathbf{\Lambda}^g$  is the generalized inverse of the diagonal matrix  $\mathbf{\Lambda}$ , which is itself a diagonal matrix with elements  $\Lambda_{ii}^g = \begin{cases} \lambda_i^{-1} & \text{if } \lambda_i \neq 0 \\ 0 & \text{otherwise} \end{cases}$ ):  $\mathbf{A}\mathbf{c} = \mathbf{n}$  is solvable over  $\mathbb{Z}$  if  $\mathbf{A}^g\mathbf{n}$  is integral [S18].

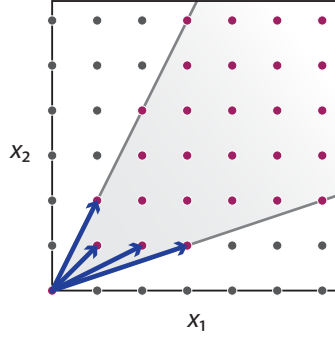

**Supplemental Figure S1. The Hilbert basis of a monoid in two dimensions.** The intersection between a cone  $C = \{\mathbf{x} \in \mathbb{R}^2 \mid 2x_1 \geq x_2 \wedge x_1 \leq 3x_2\}$  (gray area) and the set of integers  $\mathbb{Z}^2$  (markers) defines an affine monoid  $M = C \cap \mathbb{Z}^2$  (purple markers). Every point in  $M$  can be written as a (non-unique) integer conical combination of four Hilbert basis vectors (blue arrows). The set of band structure symmetries  $\{\text{BS}\}$  is a monoid.

difference geometrically by embedding the overall problem in a vector space  $\mathbb{R}^{N^{\text{irr}}}$ : in that case,  $\{\text{BS}\}$  is the intersection of a *lattice*  $\{\overline{\text{BS}}\}$  (meaning, a  $\mathbb{Z}$ -module embedded in a vector space over  $\mathbb{R}$ ) and a rational polyhedral cone\*  $C \equiv \{\mathbf{x} \in \mathbb{R}^{N^{\text{irr}}} \mid x_j \geq 0\}$  defined by the physicality condition in Eq. (S5) (i.e., just the non-negative orthant). Accordingly, we have

$$\{\text{BS}\} = \{\overline{\text{BS}}\} \cap C. \quad (\text{S11})$$

The algebraic structure of Eq. (S11) is that of a positive affine monoid  $M \subset \mathbb{Z}^{N^{\text{irr}}}$ , cf. Gordan’s lemma [S13]. A monoid denotes a set of elements equipped with an additive binary composition operation and an identity element.<sup>†</sup> Here, the operation is vector addition (i.e., “stacking” of bands) with  $\mathbf{0}$  as the associated identity (i.e., zero bands). Conceptually, monoids can be viewed as semi-groups with an identity operation or groups lacking inverses (neither  $\{\text{BS}\}$  nor  $\{\text{AI}\}$  are closed under subtraction of symmetry vectors). The relevance of emphasizing this algebraic structure, is that positive affine monoids are generated by non-negative integer combinations of a unique, minimal (i.e., irreducible) basis: a Hilbert basis [S13], see Supplemental Figure S1. These facts imply Eq. (2) of the main text, which we restate here: i.e., there exists a finite set of non-negative basis vectors  $\{\mathbf{h}_i\}_i$  such that (with  $|\text{BS}|$  denoting the number of Hilbert basis elements)

$$\{\text{BS}\} = \left\{ \sum_{i=1}^{|\text{BS}|} c_i \mathbf{h}_i \mid c_i \in \mathbb{N} \right\}. \quad (\text{S12})$$

The Hilbert basis  $\{\mathbf{h}_i\}$  of  $\{\text{BS}\}$  clearly plays an analogous role for  $\{\text{BS}\}$  as the EBRs  $\{\mathbf{a}_i\}$  do for  $\{\text{AI}\}$ . Unlike the EBR basis, however, the Hilbert basis of  $\{\text{BS}\}$  is guaranteed to be minimal<sup>‡</sup> and its elements  $\mathbf{h}_i$  are irreducible. Because  $\{\text{BS}\}$  is not embedded in a larger physical structure, this implies that  $\mathbf{h}_i$  describe

\* Here, we refer to the concept of cones in the linear algebra sense. We note the following definitions and properties:

1. A (pointed) *cone*  $C$  is a subset of a vector space  $V$  if for each  $\mathbf{x} \in C$  we have  $\alpha \mathbf{x} \in C$  for all non-negative scalars  $\alpha \geq 0$ .
2. A cone is *convex* if all non-negative spans of  $\mathbf{x} \in C$  is also in  $C$ , i.e., if  $x, y \in C$  implies  $\alpha x + \beta y \in C$  for all  $\alpha, \beta \geq 0$ .
3. A *polyhedral* cone is a convex cone in  $\mathbb{R}^d$  defined by a set of linear, homogeneous inequalities  $C = \{\mathbf{x} \in \mathbb{R}^d \mid (\mathbf{A}\mathbf{x})_i \geq 0\}$  for some matrix  $\mathbf{A}$ .
4. Every polyhedral cone can be *generated* by a finite set of *generators*  $\mathbf{v}_i \in \mathbb{R}^d$  through a *conical combination* (i.e., a non-negative coefficient span) such that  $C = \{\alpha_1 \mathbf{v}_1 + \dots + \alpha_n \mathbf{v}_n \mid \alpha_i \geq 0\}$ .
5. A *rational* cone has rational generators  $\mathbf{v}_i \in \mathbb{Q}^d$  (equivalently, there exists generators with solely integer elements).

<sup>†</sup> An *affine* monoid is a commutative monoid that is isomorphic to a submonoid of a  $\mathbb{Z}$ -module (or, equivalently, a free Abelian group; in our case, this is  $\{\overline{\text{BS}}\}$ ). A monoid is additionally *positive* if its only identity element (or unit) is  $\mathbf{0}$ .

<sup>‡</sup> The EBR basis is not a generally a Hilbert basis of  $\{\text{AI}\}$ , however, since it is not always minimal. For instance, several space groups have EBRs with identical symmetry vectors. A few space groups have EBRs that can be nontrivially decomposed: e.g., in space group 222 with time-reversal, the symmetry vector of the EBR induced by the  $E$  irrep at 6b is equal to the sum of the EBRs induced by the  $T_1$  and  $T_2$  irreps at 2a.

connected bands: if they were not, they could be written as a sum of disconnected bands in  $\{\text{BS}\}$ , i.e., they would be reducible.\*

Hilbert bases can be computed by at least two specialized softwares, namely Normaliz [S19; S20; S21] and 4ti2 [S22]; we use the former, accessed via its Python interface PyNormaliz. Computational run times are discussed in Supplemental Section S2.A. In practice, we compute the structure of  $\{\text{BS}\}$  in a manner slightly different from Eq. (S11), by instead computing the Hilbert basis  $\{\mathbf{h}'_i\}$  of the related monoid  $M'$  which governs the allowable coefficients for an expansion of  $\{\text{BS}\}$  in the form  $\{\text{BS}\} = \{\mathbf{B}\mathbf{c} \mid \mathbf{c} \in M'\}$ . This monoid is simply  $M' = \mathbb{Z}^{d^{\text{AI}}} \cap C'$  where  $C'$  is the (rational) polyhedral cone defined by

$$C' \equiv \{\mathbf{x} \in \mathbb{R}^{d^{\text{BS}}} \mid (\mathbf{B}\mathbf{x})_j \geq 0, \forall j = 1, \dots, N^{\text{irr}}\}. \quad (\text{S13})$$

Geometrically,  $C'$  is the intersection of  $N^{\text{irr}}$  half-spaces in  $\mathbb{R}^{d^{\text{BS}}}$ , each defined by a row of  $\mathbf{B}$ . The corresponding Hilbert basis of  $\{\text{BS}\}$  is obtained by multiplying the Hilbert basis of  $M'$  by  $\mathbf{B}$ , i.e.,  $\mathbf{h}_i = \mathbf{B}\mathbf{h}'_i$ . The difference between  $M'$  and the definition of  $\{\text{BS}\}$  in Eq. (S11) are only a matter of representation—but there are two computational advantages to working with  $M'$ : (1)  $M'$  is always embedded in a lower-dimensional space than  $\{\text{BS}\}$  since  $N^{\text{irr}} \geq d^{\text{BS}}$  and (2)  $M'$  involves a simpler lattice, namely  $\mathbb{Z}^{d^{\text{AI}}}$ .

### E. Atopological Hilbert bases: fragile topology

The construction above is analogous to Song *et al.*'s recent development of a Hilbert basis for the monoid of trivial and fragile band structures [S23]. We briefly reiterate their results here as additional context and to facilitate the discussion of fragile phononic  $\Gamma$ -enforced topology in Supplemental Section S8.C.

This “atopological” monoid, denoted here by  $\{\text{AI} + \text{F}\}$ , is the intersection of the integer-combination column space of  $\mathbf{A}$ , i.e.,  $\{\overline{\text{AI}}\}$ , and the “physical cone”  $C \equiv \{\mathbf{x} \in \mathbb{R}^{N^{\text{irr}}} \mid x_j \geq 0\}$  from earlier:

$$\{\text{AI} + \text{F}\} = \{\overline{\text{AI}}\} \cap C. \quad (\text{S14})$$

This monoid is *not* generally equal to  $\{\text{AI}\}$ —rather,  $\{\text{AI}\} \subseteq \{\text{AI} + \text{F}\}$ —since physical elements in  $\{\text{AI} + \text{F}\}$  might originate from subtraction of two or more EBRs in  $\{\text{AI}\}$ . These elements correspond to fragile topology [S7]: states that are neither topologically trivial (since they are not in  $\{\text{AI}\}$ ) nor topologically nontrivial in a stable sense (since they can be trivialized by incorporating certain trivial states; namely the subtracted EBRs). The difference of  $\{\text{AI} + \text{F}\}$  and  $\{\text{AI}\}$  define the set of symmetry-identifiable fragile phases  $\{\text{F}\} \equiv \{\text{AI} + \text{F}\} - \{\text{AI}\}$  (which, in general, is not a monoid; one fragile state may be trivialized by another fragile state, i.e.,  $\{\text{F}\}$  is not closed under addition).

In calculating the Hilbert basis for  $\{\text{AI} + \text{F}\}$  it is again helpful to work in the coefficient representation. We may work directly with the EBR basis—the Smith normal decomposition is not intrinsically necessary.<sup>†</sup> Since  $\{\overline{\text{AI}}\} = \{\sum_i c_i \mathbf{a}_i \mid c_i \in \mathbb{Z}\} = \{\mathbf{A}\mathbf{c} \mid \mathbf{c} \in \mathbb{Z}^{N^{\text{EBR}}}\}$ , cf. Eq. (S6), the relevant “coefficient-space” cone for the EBR vectors is

$$C'' \equiv \{\mathbf{x} \in \mathbb{R}^{N^{\text{EBR}}} \mid (\mathbf{A}\mathbf{x})_j \geq 0, \forall j = 1, \dots, N^{\text{irr}}\}, \quad (\text{S15})$$

which defines an associated affine monoid  $M'' = \mathbb{Z}^{N^{\text{EBR}}} \cap C''$  for the set of allowable coefficients. The corresponding “symmetry-space” monoid  $\{\text{AI} + \text{F}\}$  is then related to  $M''$  by  $\{\text{AI} + \text{F}\} = \{\mathbf{A}\mathbf{c} \mid \mathbf{c} \in M''\}$ ,

\* The same argument does not apply to the EBR basis of  $\{\text{AI}\}$  since it is embedded in  $\{\text{BS}\}$  (i.e.,  $\{\text{AI}\} \subseteq \{\text{BS}\}$ ): some elements of  $\{\mathbf{a}_i\}$  are disconnectible [S11] and expressible as sums of elements in  $\{\text{BS}\}$  [S17] (e.g., as the sum of two nontrivial symmetry vectors).

<sup>†</sup> It is of course also possible to use the Smith normal decomposition (as in Ref. S23). To do so, we may note that the Smith normal decomposition allows expressing  $\{\overline{\text{AI}}\}$  as  $\{\mathbf{B}\tilde{\mathbf{A}}\mathbf{c} \mid \mathbf{c} \in \mathbb{Z}^{d^{\text{AI}}}\}$  (with  $\tilde{\mathbf{A}}$  denoting the first  $d^{\text{AI}}$  rows of  $\mathbf{A}$ ), which then implies the related “coefficient-space” cone  $C''' \equiv \{\mathbf{x} \in \mathbb{R}^{d^{\text{AI}}} \mid (\mathbf{B}\tilde{\mathbf{A}}\mathbf{x})_j \geq 0, \forall j = 1, \dots, N^{\text{irr}}\}$  and the associated monoid  $M''' = \mathbb{Z}^{d^{\text{AI}}} \cap C'''$ . As before, the elements of  $M'''$  then generate  $\{\text{AI} + \text{F}\}$  via  $\{\mathbf{B}\tilde{\mathbf{A}}\mathbf{c} \mid \mathbf{c} \in M'''\}$  and the Hilbert basis of  $\{\text{AI} + \text{F}\}$  can be obtained from that of  $M'''$  by multiplication with  $\mathbf{B}\tilde{\mathbf{A}}$ . Perhaps counterintuitively, despite the dimension of the embedding space of  $M'''$  being smaller than that of  $M''$  (since  $d^{\text{AI}} \leq N^{\text{EBR}}$ ), we find that it is usually computationally superior to work with  $M''$  ( $\sim 25\%$ ). Speculatively, this might be related to the non-negativity of the EBR vectors (which is not guaranteed for the columns of  $\mathbf{B}\tilde{\mathbf{A}}$ ).



in full analogy to our earlier construction of  $\{\text{BS}\}$ . Also as before, the Hilbert basis  $\{\mathbf{h}_i''\}$  of  $M''$  generates the Hilbert basis  $\{\mathbf{f}_i\}$  of  $\{\text{AI} + \text{F}\}$  via  $\mathbf{f}_i = \mathbf{A}\mathbf{h}_i''$ .

Elements of  $\{\mathbf{f}_i\}$  that cannot be written as a combination of EBRs with non-negative coefficients correspond to fragile states [S17]. In the terminology of Ref. S23, we refer to this subset of the Hilbert basis as its fragile roots: any fragile symmetry vector can be written as a non-negative sum of fragile roots (and, possibly, EBRs). Note that a sum of fragile roots may be trivial (i.e., a fragile state can be trivialized not only by trivial states but also by other fragile states).

## F. Symmetry-identifiable topology and bases

We summarize the various bases and sets discussed in the preceding sections in [Supplemental Table I](#) as well as their relation to the topological classification of symmetry vectors in [Supplemental Table II](#).

In practice, we decide solvability in a non-negative integer coefficient space (e.g., to check whether a symmetry vector  $\mathbf{n}$  can be expressed as a sum of EBR vectors) by checking the feasibility of an associated integer programming problem using the JuMP optimization package [S24] and the GLPK solvers [S25].

| Set                        | Symmetry data is ...  | Physical | Basis                                               | Coefficients ( $\mathbf{c} \in R$ )   |
|----------------------------|-----------------------|----------|-----------------------------------------------------|---------------------------------------|
| $\{\text{AI}\}$            | Trivial               | ✓        | $\{\mathbf{a}_i\}$                                  | $\mathbb{N}^{N^{\text{EBR}}}$         |
| $\{\text{AI} + \text{F}\}$ | Not stably nontrivial | ✓        | $\{\mathbf{f}_i\}$                                  | $\mathbb{N}^{ \text{AI} + \text{F} }$ |
| $\{\text{BS}\}$            | Compatible            | ✓        | $\{\mathbf{h}_i\}$                                  | $\mathbb{N}^{ \text{BS} }$            |
| $\{\text{AI}\}$            | Not stably nontrivial |          | $\{\mathbf{a}_i\}$ and $\{\lambda_i \mathbf{b}_i\}$ | $\mathbb{Z}^{d^{\text{AI}}}$          |
| $\{\text{BS}\}$            | Compatible            |          | $\{\mathbf{b}_i\}$                                  | $\mathbb{Z}^{d^{\text{BS}}}$          |

**Supplemental Table I. Symmetry vector sets.** For each set (column 1), we indicate its main symmetry-identifiable implications (column 2), whether the set's elements are necessarily physical (column 3), a canonical basis (column 4), and the algebraic structure of the basis' expansion coefficients (column 5).  $\mathbf{a}_i$  denotes an EBR vector,  $\mathbf{f}_i$  a Hilbert vector of  $\{\text{AI} + \text{F}\}$ ,  $\mathbf{h}_i$  a Hilbert vector of  $\{\text{BS}\}$ ,  $\mathbf{b}_i$  a non-singular column vector of the Smith normal  $\mathbf{S}$ -matrix of  $\mathbf{A}$ , and  $\lambda_i$  the associated elementary divisor. Note that  $d^{\text{AI}} = d^{\text{BS}}$ .

| Topology   | Set                                        | Has $c_i \in \mathbb{N}$ expansion? |                    |                    | $c_i \in \mathbb{Z}$ expansion? |                    | Expansions in EBRs $\{\mathbf{a}_i\}$ ...               |
|------------|--------------------------------------------|-------------------------------------|--------------------|--------------------|---------------------------------|--------------------|---------------------------------------------------------|
|            |                                            | $\{\mathbf{a}_i\}$                  | $\{\mathbf{f}_i\}$ | $\{\mathbf{h}_i\}$ | $\{\lambda_i \mathbf{b}_i\}$    | $\{\mathbf{b}_i\}$ |                                                         |
| Trivial    | $\{\text{AI}\}$                            | ✓                                   | ✓                  | ✓                  | ✓                               | ✓                  | Exist with all $c_i \in \mathbb{N}$                     |
| Fragile    | $\{\text{AI} + \text{F}\} - \{\text{AI}\}$ | ÷                                   | ✓                  | ✓                  | ✓                               | ✓                  | Requires at least one $c_i \in \mathbb{Z} - \mathbb{N}$ |
| Nontrivial | $\{\text{BS}\} - \{\text{AI} + \text{F}\}$ | ÷                                   | ÷                  | ✓                  | ÷                               | ✓                  | Requires at least one $c_i \in \mathbb{Q} - \mathbb{Z}$ |

**Supplemental Table II. Topological classification of symmetry and expandability.** For the symmetry-identifiable classifications of trivial, fragile, and (stably) nontrivial topology (column 1), we indicate the associated symmetry vector set (column 2), whether non-negative integer expansions exists in the  $\{\mathbf{a}_i\}$ ,  $\{\mathbf{f}_i\}$ , or  $\{\mathbf{h}_i\}$  bases (column 3–5), whether integer expansions exist in the Smith column-space  $\{\lambda_i \mathbf{b}_i\}$  and  $\{\mathbf{b}_i\}$  bases (column 6–7), and constraints on the coefficients in an EBR expansion (column 8).

## S2. COMPUTATIONAL DETAILS

### A. Hilbert basis

*Implementation.* The computation of Hilbert basis vectors for  $\{\text{BS}\}$  and  $\{\text{AI} + \text{F}\}$  is implemented in our software package `SymmetryBases.jl` [S26] and can be accessed via the functions `compatibility_basis` and `nontopological_basis`. The computation leverages the Normaliz library [S19; S20; S21], accessed via PyNormaliz, for the computation of Hilbert basis vectors of integer lattices in cones.

*Run time.* The computational run time of Hilbert bases for  $\{\text{BS}\}$  and  $\{\text{AI} + \text{F}\}$  is highly variable and sensitive to space group number, the existence of time-reversal symmetry, and whether particles transform as

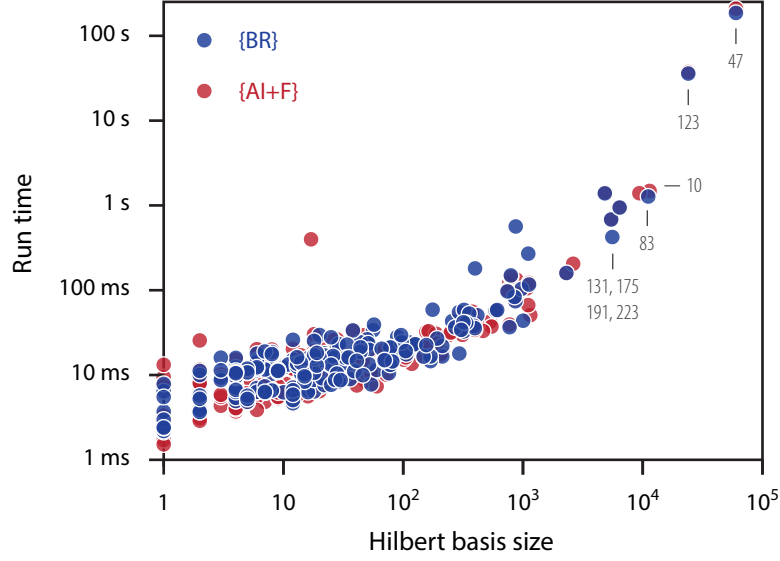

**Supplemental Figure S2. Hilbert basis size versus run time across all space groups.** The run time for calculating Hilbert bases for {BS} and {AI + F} is highly correlated with the number of elements in the basis. A few space groups, annotated by gray labels, have very high run times and basis size. Results are for bosons with time-reversal symmetry, with Hilbert bases calculated via Normaliz (on a 4-core 1.6 GHz CPU).

bosons or fermions. Here, we focus exclusively on the bosonic case (i.e. on single-valued space groups). There is a high degree of correlation between run time and the number Hilbert basis elements as illustrated in Supplemental Figure S2 (in median, the Hilbert bases contain 18 elements but the variability is very large: e.g., space group 47 contains 60.000 elements). While the median run time was on the order of tens of ms, a handful of space groups exhibited run time reaching a few minutes (tested on a 1.6 GHz 4-core i5-8250U CPU).

If time-reversal symmetry is broken, we found that it becomes highly challenging to compute the Hilbert bases for {AI + F} in space groups 83, 174, 175, and 176: Normaliz failed to converge for either of these space groups in 24 h (the Hilbert bases for {BS}, fortunately, do not exhibit similar issues). This is not a significant issue: the practical computational utility of the Hilbert basis of {AI + F} is not large and mainly of conceptual relevance (the basis is not intrinsically necessary in assessing fragility, cf. Supplemental Table II).

## B. Exhaustive computation of connectivity-constrained solutions

In the iterative procedure described in the main text for obtaining the photonic transverse connectivity  $\mu^T$ , we require as an intermediary the exhaustive enumeration of all regular solutions  $\{\mathbf{n}^{L+T}\}$  with connectivity  $\mu^{L+T}$  with  $\Gamma$ -symmetry constrained by Eq. (3). The salient challenge in this computation is the exhaustive enumeration of *all* solutions with a fixed connectivity (the  $\Gamma$ -constraints then feature merely as a filtering step). In fact, this challenge is a key motivation for introducing the Hilbert basis  $\{\mathbf{h}_i\}$  of {BS}.

We now consider this problem in detail: omitting inessential notational detail, we seek all symmetry vector solutions  $\{\mathbf{n}\}$  in {BS} with connectivity  $\mu$ . Any such solution  $\mathbf{n}$  can be expressed as a conical integer combination of  $\{\mathbf{h}_i\}$ , i.e., there exists (possibly non-unique) coefficients  $c'_i \in \mathbb{N}$  such that

$$\mathbf{n} = \sum_i^{|\text{BS}|} c'_i \mathbf{h}_i. \quad (\text{S16})$$



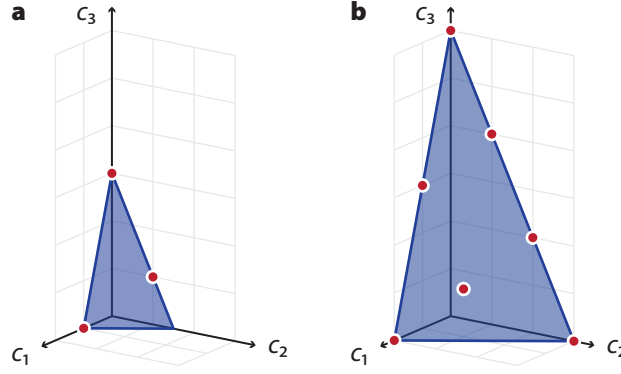

**Supplemental Figure S3. Integer lattice points in simplices.** The solutions to Eq. (S17) are the integer lattice points contained in (or on the boundary of) a  $|\text{BS}|$ -dimensional simplex with vertices  $\{\mathbf{c}^{(1)}, \mathbf{c}^{(2)}, \dots, \mathbf{c}^{(|\text{BS}|)}\}$  with coordinates  $c_i^{(j)} = \delta_{ij}\mu/\mu_i$ . Here, we visualize the solutions to a simple 3-dimensional variant, namely  $c_1\mu_1 + c_2\mu_2 + c_3\mu_3 = \mu$  with  $\mu_1 = 3$ ,  $\mu_2 = 2$ , and  $\mu_3 = 1$  and a target connectivity of  $\mu = 3$  (a) and  $\mu = 6$  (b). Simplices are shown in shaded blue and associated integer solutions in red markers.

If  $\mathbf{n}$  has connectivity  $\mu$ , its coefficients  $\{c_i\}$  must solve the equation:

$$\mu = \sum_i^{|\text{BS}|} c_i \mu_i, \quad (\text{S17})$$

with  $\mu_i$  denoting the band connectivity of the  $i$ th Hilbert basis vector  $\mathbf{h}_i$ . Equation (S17) is a linear Diophantine equation with conical constraints (i.e., requiring  $c_i \geq 0$ ) consisting of only non-negative (integer) terms. Equivalently, the solutions to Eq. (S17) are the integer lattice points of an integral polytope:<sup>\*</sup> as a whole, the problem falls under integer programming. Geometrically, we can visualize the solutions as the integer lattice points in the simplex  $\{\mathbf{c} \in \mathbb{R}_{\geq 0}^{|\text{BS}|} \mid \sum_i c_i \mu_i = \mu\}$  (as illustrated in Supplemental Figure S3), implying that there are only finitely many solutions.

The non-negative structure of Eq. (S17) enables a simple algorithm that very rapidly obtains these solutions exhaustively. We summarize the salient steps and considerations in this algorithm below:<sup>†</sup>

1. We can disregard any Hilbert vectors with connectivity greater than  $\mu$ , i.e., we restrict the summation in Eq. (S17) to a subset  $i \in \{i'\}$  whose Hilbert vectors have connectivities  $\mu_i \leq \mu$ .
2. To not overflow Eq. (S17), valid expansions can at most contain  $I^{\max} \equiv \lfloor \mu / \min \mu_i \rfloor$  additions of Hilbert vectors (i.e.,  $\sum_i c_i \leq I^{\max}$ ).
3. We can therefore exhaustively check every possible solution by iterating through  $I^{\max}$  nested for-loops. Concretely, our algorithm proceeds as (here indicated in pseudocode: **accept** denotes storage of a solution and **continue** denotes progression to the next iteration of the current loop):

```

for  $i_1 \in \{i'\}$ 
  if  $\mu_{i_1} = \mu$ 
     $\mathbf{h}_{i_1}$  solves Eq. (S17): accept & continue
  end
  for  $i_2 \in \{i'\}$ 
    if  $\mu_{i_1} + \mu_{i_2} = \mu$ 
       $\mathbf{h}_{i_1} + \mathbf{h}_{i_2}$  solves Eq. (S17): accept & continue

```

<sup>\*</sup> This identification with an integral polytope implies that there exists a function—the so-called Ehrhart polynomial—which counts (and bounds) the number of solutions. This function can be computed in Normaliz (via `EhrhartSeries` or directly via `NumberLatticePoints`) [S19].

<sup>†</sup> Solutions to Eq. (S17) could also be obtained directly via Normaliz [S19] as the lattice points of an integral polytope. In practice, we found that our algorithm was several orders of magnitude faster (presumably due to exploiting the non-negativity of  $\mu_i$ ).

```

end
[...additional nested for-loops and if-statements...]
for  $i_{j\max} \in \{i'\}$ 
  if  $\mu_{i_1} + \mu_{i_2} + \dots + \mu_{i_{j\max}} = \mu$ 
     $\mathbf{h}_{i_1} + \mathbf{h}_{i_2} + \dots + \mathbf{h}_{i_{j\max}}$  solves Eq. (S17): accept & continue
  end
end
end
end
end

```

Our implementation is available in our software package PhotonicBandConnectivity.jl [S27]. For technical reasons, we adopt a slightly different but equivalent approach in practice: instead of  $I^{\max}$  nested for-loops, we use  $I^{\max}$  levels of recursion. Additionally, we check the  $\Gamma$ -point symmetry constraints concurrently (i.e., at every iteration).

4. Since the Hilbert basis is not orthogonal, the above procedure may generate the same solution multiple times (i.e., there may exist several distinct expansions corresponding to the same symmetry vector). At the procedure's end, we extract the unique set of symmetry vectors.

It is worthwhile emphasizing how significant the advantages of the Hilbert basis' conicity are: without it, enumeration of all solutions to Eq. (S17) would require considering not only the addition of basis vectors but also their *subtraction*, entailing an unbounded number of coefficient sets to explore and significant combinatorial challenges.

### C. Construction and specification of photonic crystal lattices in Supplemental Figures 3 and 4

The photonic crystal unit cells in Supplemental Figures 3 and 4 were constructed as isolevel surfaces of symmetry-constrained Fourier sums. To construct these surfaces, we first consider an arbitrary discrete Fourier sum in the reciprocal lattice vectors  $\{\mathbf{G}\} = \{n_1\mathbf{G}_1 + n_2\mathbf{G}_2 + n_3\mathbf{G}_3 \mid n_i \in \mathbb{Z}\}$  with coefficients  $c_{\mathbf{G}}$ :

$$f(\mathbf{r}) = \sum_{\{\mathbf{G}\}} c_{\mathbf{G}} e^{i\mathbf{G} \cdot \mathbf{r}}, \quad (\text{S18})$$

which is necessarily periodic in the direct basis  $\{\mathbf{R}\}$ , i.e.,  $f(\mathbf{r} + \mathbf{R}) = f(\mathbf{r})$ . Additionally, to ensure symmetry, we require that  $gf(\mathbf{r}) = f(g^{-1}\mathbf{r}) = f(\mathbf{r})$  for every operation  $g = \{\mathbf{W}|\mathbf{w}\}$  in the considered space group  $G$ . Since  $g^{-1} = \{\mathbf{W}^{-1} | -\mathbf{W}^{-1}\mathbf{w}\}$  we then require that:

$$\begin{aligned} f(g^{-1}\mathbf{r}) &= \sum_{\{\mathbf{G}\}} c_{\mathbf{G}} e^{i\mathbf{G} \cdot g^{-1}\mathbf{r}} = \sum_{\{\mathbf{G}\}} c_{\mathbf{G}} e^{i\mathbf{G} \cdot \mathbf{W}^{-1}(\mathbf{r} - \mathbf{w})} = \sum_{\{\mathbf{G}\}} c_{\mathbf{G}} e^{i(\mathbf{W}^{-1})^T \mathbf{G} \cdot (\mathbf{r} - \mathbf{w})} = \sum_{\{\mathbf{G}\}} c_{\mathbf{G}} e^{i(g\mathbf{G}) \cdot (\mathbf{r} - \mathbf{w})} \\ &= f(\mathbf{r}) = \sum_{\{\mathbf{G}\}} c_{\mathbf{G}} e^{i\mathbf{G} \cdot \mathbf{r}}, \end{aligned} \quad (\text{S19})$$

where we have defined the action of a symmetry operation on a  $\mathbf{k}$ -vector by  $g\mathbf{k} \equiv (\mathbf{W}^{-1})^T \mathbf{k}$ . To fulfill Eq. (S19) for all  $\mathbf{r}$ , the series' summands must be equal term-by-term. Accordingly, we require that

$$c_{\mathbf{G}} e^{-i\mathbf{gG} \cdot \mathbf{w}} = c_{g\mathbf{G}} \quad (\text{S20})$$

for all  $\mathbf{G}$  in the sum and for all  $g \in G$ . This defines a set of coupled equations for the coefficients  $c_{\mathbf{G}}$ . In practice, however, only a small subset of coefficients are coupled, namely those within a single star of  $\mathbf{G}$ , i.e., in  $\text{star}(\mathbf{G})$  where  $\text{star}(\mathbf{k}) \equiv \{g\mathbf{k} \mid g \in G\} = \{(\mathbf{W}^{-1})^T \mathbf{k} \mid g \in G\}$ . For each star and each operation  $g$ , the coefficients must then satisfy

$$\underbrace{\begin{bmatrix} e^{-i(g\mathbf{G}_1) \cdot \mathbf{w}} & \delta_{\mathbf{G}_1, g\mathbf{G}_2} & \dots & \delta_{\mathbf{G}_1, g\mathbf{G}_n} \\ \delta_{\mathbf{G}_2, g\mathbf{G}_1} & e^{-i(g\mathbf{G}_2) \cdot \mathbf{w}} & \dots & \delta_{\mathbf{G}_2, g\mathbf{G}_n} \\ \vdots & \vdots & \ddots & \vdots \\ \delta_{\mathbf{G}_n, g\mathbf{G}_1} & \delta_{\mathbf{G}_n, g\mathbf{G}_2} & \dots & e^{-i(g\mathbf{G}_n) \cdot \mathbf{w}} \end{bmatrix}}_{\equiv \mathbf{C}^{g, \text{star}(\mathbf{G})}} \underbrace{\begin{bmatrix} c_{\mathbf{G}_1} \\ c_{\mathbf{G}_2} \\ \vdots \\ c_{\mathbf{G}_n} \end{bmatrix}}_{\equiv \mathbf{c}^{\text{star}(\mathbf{G})}} = \begin{bmatrix} 0 \\ 0 \\ \vdots \\ 0 \end{bmatrix}, \quad (\text{S21})$$

| $\text{star}(\mathbf{G})$                                                                                                                                                                | $\tilde{\mathbf{c}}^{\text{star}(\mathbf{G})}$   | $\mathbf{C}^{\text{star}(\mathbf{G})}$ |
|------------------------------------------------------------------------------------------------------------------------------------------------------------------------------------------|--------------------------------------------------|----------------------------------------|
| $\bar{1}10, \bar{1}10, \bar{1}\bar{1}0, 110$                                                                                                                                             | $1, \bar{1}, \bar{1}, 1$                         | 0.215266                               |
| $\bar{1}0\bar{1}, \bar{1}01, 0\bar{1}\bar{1}, 0\bar{1}1, 01\bar{1}, 011, 10\bar{1}, 101$                                                                                                 | $1, \bar{1}, 1, \bar{1}, \bar{1}, 1, \bar{1}, 1$ | 0.156874                               |
| $\bar{1}\bar{1}\bar{1}, \bar{1}\bar{1}\bar{1}, \bar{1}\bar{1}\bar{1}, \bar{1}\bar{1}\bar{1}, \bar{1}\bar{1}\bar{1}, \bar{1}\bar{1}\bar{1}, \bar{1}\bar{1}\bar{1}, \bar{1}\bar{1}\bar{1}$ | $1, 1, 1, 1, 1, 1, 1, 1$                         | -0.101230                              |
| $\bar{2}00, \bar{0}20, 020, 200$                                                                                                                                                         | $1, 1, 1, 1$                                     | 0.062241                               |
| $00\bar{2}, 002$                                                                                                                                                                         | $1, 1$                                           | 0.024818                               |
| $\bar{2}0\bar{1}, \bar{2}01, 0\bar{2}\bar{1}, 0\bar{2}1, 02\bar{1}, 021, 20\bar{1}, 201$                                                                                                 | $1, 1, \bar{1}, \bar{1}, \bar{1}, \bar{1}, 1, 1$ | 0.068251                               |
| $10\bar{2}, 102, 01\bar{2}, 012, 01\bar{2}, 012, 10\bar{2}, 102$                                                                                                                         | $1, \bar{1}, \bar{1}, 1, 1, \bar{1}, \bar{1}, 1$ | -0.018741                              |
| $\bar{2}1\bar{1}, \bar{2}11, \bar{1}2\bar{1}, \bar{1}21, \bar{1}2\bar{1}, \bar{1}21, 21\bar{1}, 211$                                                                                     | $1, \bar{1}, 1, \bar{1}, \bar{1}, 1, \bar{1}, 1$ | 0.015518                               |
| $\bar{2}\bar{1}\bar{1}, \bar{2}\bar{1}1, \bar{1}2\bar{1}, \bar{1}21, \bar{1}2\bar{1}, \bar{1}21, 2\bar{1}\bar{1}, 2\bar{1}1$                                                             | $1, \bar{1}, \bar{1}, 1, 1, \bar{1}, \bar{1}, 1$ | 0.107742                               |
| $\bar{1}\bar{1}\bar{2}, \bar{1}\bar{1}2, \bar{1}\bar{1}\bar{2}, \bar{1}\bar{1}2, \bar{1}\bar{1}\bar{2}, \bar{1}\bar{1}2, \bar{1}\bar{1}\bar{2}, \bar{1}\bar{1}2$                         | $1, 1, \bar{1}, \bar{1}, \bar{1}, \bar{1}, 1, 1$ | -0.108274                              |
| $\bar{2}\bar{2}0, \bar{2}20, \bar{2}\bar{2}0, \bar{2}20$                                                                                                                                 | $1, 1, 1, 1$                                     | -0.123322                              |
| $\bar{2}0\bar{2}, \bar{2}02, 0\bar{2}\bar{2}, 0\bar{2}2, 02\bar{2}, 022, 20\bar{2}, 202$                                                                                                 | $1, 1, 1, 1, 1, 1, 1, 1$                         | 0.180336                               |
| $\bar{2}\bar{2}\bar{1}, \bar{2}\bar{2}1, \bar{2}\bar{2}\bar{1}, \bar{2}\bar{2}1, \bar{2}\bar{2}\bar{1}, \bar{2}\bar{2}1, \bar{2}\bar{2}\bar{1}, \bar{2}\bar{2}1$                         | $1, 1, \bar{1}, \bar{1}, \bar{1}, \bar{1}, 1, 1$ | -0.104719                              |
| $\bar{2}1\bar{2}, \bar{2}12, \bar{1}2\bar{2}, \bar{1}22, \bar{1}2\bar{2}, \bar{1}22, 21\bar{2}, 212$                                                                                     | $1, \bar{1}, \bar{1}, 1, 1, \bar{1}, \bar{1}, 1$ | -0.094150                              |
| $\bar{2}\bar{1}\bar{2}, \bar{2}\bar{1}2, \bar{1}2\bar{2}, \bar{1}22, \bar{1}2\bar{2}, \bar{1}22, 2\bar{1}\bar{2}, 2\bar{1}2$                                                             | $1, \bar{1}, 1, \bar{1}, \bar{1}, 1, \bar{1}, 1$ | -0.019122                              |
| $\bar{2}\bar{2}\bar{2}, \bar{2}\bar{2}2, \bar{2}\bar{2}\bar{2}, \bar{2}\bar{2}2, \bar{2}\bar{2}\bar{2}, \bar{2}\bar{2}2, \bar{2}\bar{2}\bar{2}, \bar{2}\bar{2}2$                         | $1, 1, 1, 1, 1, 1, 1, 1$                         | 0.046883                               |

**Supplemental Table III. Lattice expansion coefficients for space group 86 PhC in Supplemental Figure 3.** Direct basis vectors  $\mathbf{R}_1 = [1, 0, 0]^T$ ,  $\mathbf{R}_2 = [0, 1, 0]^T$ , and  $\mathbf{R}_3 = [0, 0, 1.25]^T$ ; associated reciprocal basis vectors  $\mathbf{G}_1 = 2\pi[1, 0, 0]^T$ ,  $\mathbf{G}_2 = 2\pi[0, 1, 0]^T$ , and  $\mathbf{G}_3 = 2\pi[0, 0, 0.8]^T$ ; isovalue  $f_0 = -0.350136$ ; and permittivities  $\varepsilon_1 = 16$  and  $\varepsilon_2 = 1$ . Vectors in  $\text{star}(\mathbf{G})$  are given in the reciprocal lattice basis so that e.g.,  $\bar{2}\bar{1}\bar{1} = -2\mathbf{G}_1 + \mathbf{G}_2 - \mathbf{G}_3$ .

where we have denoted the elements of  $\text{star}(\mathbf{G})$  by  $\{\mathbf{G}_1, \mathbf{G}_2, \dots, \mathbf{G}_n\}$  (not to be confused with the reciprocal lattice *basis*). Similarly writing the elements of  $G$  as  $\{g_1, g_2, \dots, g_{|G|}\}$ , we aggregate every equation from  $g \in G$  in a single matrix  $\mathbf{C}^{\text{star}(\mathbf{G})}$ , defined as the vertical concatenation of the  $\mathbf{C}^{g_i, \text{star}(\mathbf{G})}$  matrices:

$$\mathbf{C}^{\text{star}(\mathbf{G})} \equiv \begin{bmatrix} \mathbf{C}^{g_1, \text{star}(\mathbf{G})} \\ \mathbf{C}^{g_2, \text{star}(\mathbf{G})} \\ \vdots \\ \mathbf{C}^{g_{|G|}, \text{star}(\mathbf{G})} \end{bmatrix}. \quad (\text{S22})$$

The coefficients  $\tilde{\mathbf{c}}^{\text{star}(\mathbf{G})}$  are then simply elements in the null space of  $\mathbf{C}^{\text{star}(\mathbf{G})}$ , i.e.,  $\mathbf{C}^{\text{star}(\mathbf{G})} \tilde{\mathbf{c}}^{\text{star}(\mathbf{G})} = \mathbf{0}$ . In practice, it is convenient to pick a fixed and suitably normalized representative element of the null space, say  $\tilde{\mathbf{c}}^{\text{star}(\mathbf{G})}$ , such that any coefficient  $c_{\mathbf{G}'}$  with  $\mathbf{G}' \in \text{star}(\mathbf{G})$  can be expressed as the product of a fixed “intra-star” term  $c_{\mathbf{G}'}^{\text{star}(\mathbf{G})}$  and a free “inter-star” term  $c_{\text{star}(\mathbf{G})}$ , i.e., as  $c_{\mathbf{G}'} = \tilde{c}_{\mathbf{G}'}^{\text{star}(\mathbf{G})} c_{\text{star}(\mathbf{G})}$ .

Revisiting Eq. (S18), we may then restructure the sum as:

$$f(\mathbf{r}) = \sum_{\{\text{star}(\mathbf{G})\}} c_{\text{star}(\mathbf{G})} \sum_{\mathbf{G} \in \text{star}(\mathbf{G})} c_{\mathbf{G}}^{\text{star}(\mathbf{G})} e^{i\mathbf{G} \cdot \mathbf{r}}, \quad (\text{S23})$$

where the first sum runs over distinct reciprocal lattice vector stars. In this sum, only the (complex) “inter-star” coefficients  $c_{\text{star}(\mathbf{G})}$  are free: all other coefficients are fully constrained by symmetry. In a different perspective, the second sum gives a basis for functions transforming like the trivial representation of  $G$ .

A concrete lattice symmetric under  $G$  can then finally be defined as the real isosurface derived from  $f$ . Concretely, a two-material ( $\varepsilon_1$  and  $\varepsilon_2$ ) PhC can then be defined as the permittivity profile:

$$\varepsilon(\mathbf{r}) = \begin{cases} \varepsilon_1 & \text{for } \text{Re } f(\mathbf{r}) \leq f_0 \\ \varepsilon_2 & \text{for } \text{Re } f(\mathbf{r}) > f_0 \end{cases}, \quad (\text{S24})$$

with isosurface value  $f_0$ .

We give our expansions for the photonic crystals considered in Supplemental Figures 3 and 4 in Supplemental Tables III and IV. The expansion coefficients can be chosen entirely real due to inversion symmetry. Analogous lattices in other space groups can be created using Crystalline.jl [S12].

| star( <b>G</b> )                       | $\tilde{\mathbf{c}}^{\text{star}(\mathbf{G})}$ | Cstar( <b>G</b> ) |
|----------------------------------------|------------------------------------------------|-------------------|
| 011, 011, 101, 101, 101, 101, 011, 011 | 1, 1, 1, 1, 1, 1, 1, 1                         | -0.066833         |
| 110, 110                               | 1, 1                                           | 0.119745          |
| 110, 110                               | 1, 1                                           | 0.103475          |
| 002, 002                               | 1, 1                                           | 0.006432          |
| 012, 012, 102, 102, 102, 102, 012, 012 | 1, 1, 1, 1, 1, 1, 1, 1                         | 0.214477          |
| 020, 200, 200, 020                     | 1, 1, 1, 1                                     | -0.044208         |
| 112, 112, 112, 112                     | 1, 1, 1, 1                                     | -0.052412         |
| 112, 112, 112, 112                     | 1, 1, 1, 1                                     | -0.030409         |
| 021, 021, 201, 201, 201, 201, 021, 021 | 1, 1, 1, 1, 1, 1, 1, 1                         | 0.008148          |
| 022, 022, 202, 202, 202, 202, 022, 022 | 1, 1, 1, 1, 1, 1, 1, 1                         | 0.006858          |

**Supplemental Table IV. Lattice expansion coefficients for space group 68 PhC in Supplemental Figure 4.**

Direct (primitive) basis vectors  $\mathbf{R}_1 = [0.4, -0.5, 0]^T$ ,  $\mathbf{R}_2 = [0.4, 0.5, 0]^T$ , and  $\mathbf{R}_3 = [0, 0, 1.2]^T$ ; associated reciprocal basis vectors  $\mathbf{G}_1 = 2\pi[1.25, -1, 0]^T$ ,  $\mathbf{G}_2 = 2\pi[1.25, 1, 0]^T$ , and  $\mathbf{G}_3 = 2\pi[0, 0, 5/6]^T$ ; isovalue  $f_0 = -0.237634$ ; and permittivities  $\varepsilon_1 = 16$  and  $\varepsilon_2 = 1$ . Vectors in star(**G**) are given in the reciprocal lattice basis so that e.g.,  $112 = -\mathbf{G}_1 - \mathbf{G}_2 + 2\mathbf{G}_3$ .

### S3. INVARIANCE OF SINGULAR TRANSVERSE TOPOLOGICAL INDICES

We prove that Eq. (6), i.e.,  $v_i^T = (v_i^{L+T} - v_i^L) \bmod \lambda_i$ , is invariant to the choice of longitudinal and apolar vectors. The proof can be made by explicit construction: we first assume that we have originally calculated  $v_i^T$  by considering a particular choice of longitudinal and apolar vectors  $\mathbf{n}^L$  and  $\mathbf{n}^{L+T}$  with associated indices  $v_i^L$  and  $v_i^{L+T}$ . Next, we consider the implications of adding some bands to our original choice of  $\mathbf{n}^L$  (and, by extension, to  $\mathbf{n}^{L+T}$ ), aiming to show that  $v_i^T$  is invariant to this. In particular, define by  $\tilde{\mathbf{n}}^L = \mathbf{n}^L + \tilde{\mathbf{n}}^L$  the longitudinal symmetry vector obtained by adding a symmetry vector  $\tilde{\mathbf{n}}^L$  to our original choice  $\mathbf{n}^L$ .<sup>\*</sup> The apolar vector is similarly updated to  $\tilde{\mathbf{n}}^{L+T} = \mathbf{n}^{L+T} + \tilde{\mathbf{n}}^L$ . The topological indices of  $\tilde{\mathbf{n}}^L$  and  $\tilde{\mathbf{n}}^{L+T}$  are obtained by addition modulo  $\lambda_i$ , i.e.,:

$$\tilde{v}_i^L = (v_i^L + \tilde{v}_i^L) \bmod \lambda_i, \quad (\text{S25a})$$

$$\tilde{v}_i^{L+T} = (v_i^{L+T} + \tilde{v}_i^L) \bmod \lambda_i, \quad (\text{S25b})$$

with  $\tilde{v}_i^L$  denoting the indices of  $\tilde{\mathbf{n}}^L$ . The transverse indices  $\tilde{v}_i^T$  associated with the decomposition of  $\mathbf{n}^T$  in  $\tilde{\mathbf{n}}^L$  and  $\tilde{\mathbf{n}}^{L+T}$  are then given by Eq. (6):

$$\begin{aligned} \tilde{v}_i^T &= (\tilde{v}_i^{L+T} - \tilde{v}_i^L) \bmod \lambda_i \\ &= \{[(v_i^{L+T} + \tilde{v}_i^L) \bmod \lambda_i] - [(v_i^L + \tilde{v}_i^L) \bmod \lambda_i]\} \bmod \lambda_i \\ &= (v_i^{L+T} + \tilde{v}_i^L - v_i^L - \tilde{v}_i^L) \bmod \lambda_i \\ &= (v_i^{L+T} - v_i^L) \bmod \lambda_i \\ &= v_i^T, \end{aligned} \quad (\text{S26})$$

where we have inserted Eq. (S25) at the second equality and exploited that the modulo operation is distributive [i.e.,  $(a \bmod n) + (b \bmod n) = (a + b) \bmod n$ ] at the third equality. This establishes that Eq. (6) is invariant to the choice of auxiliary modes, and hence that the transverse topological indices  $v_i^T$  are unique (even though the auxiliary indices are not).<sup>†</sup>

We note parenthetically that attempting to define an invariant transverse index by considering only a “coarse-grained” trivial-or-nontrivial classification of the auxiliary modes is unworkable. Concretely,

<sup>\*</sup> We allow  $\tilde{\mathbf{n}}^L$  to be any quasi-regular symmetry vector such that  $\tilde{\mathbf{n}}^L$  still respects the  $\Gamma$ -point constraints in Eq. (3) (i.e.,  $\tilde{\mathbf{n}}^L$  is a subset of  $\{\tilde{\mathbf{B}}\}$  rather than just  $\{\mathbf{B}\}$ ). In particular,  $\tilde{\mathbf{n}}^L$  can be the subtraction of two valid longitudinal symmetry vectors, corresponding to simply making an entirely new choice of longitudinal symmetry vector.

<sup>†</sup> Note that this proof makes no assumption about whether the symmetry vector  $\mathbf{n}^T = \mathbf{n}^{L+T} - \mathbf{n}^L = \tilde{\mathbf{n}}^{L+T} - \tilde{\mathbf{n}}^L$  has minimal connectivity or not: i.e., it applies to all transverse bands connected to  $\omega = 0$ .

suppose we define a coarse-grained  $\mathbb{Z}_2$ -index  $\nu = 1 - \delta_{0,\nu_1} \cdots \delta_{0,\nu_d,BS}$  and then define the transverse index  $\nu^T = (\nu^{L+T} - \nu^L) \bmod 2$  from the coarse-grained apolar and longitudinal indices  $\nu^{L+T}$  and  $\nu^L$ . We can see that this is not invariant by example: suppose we consider a symmetry indicator group  $\mathbb{Z}_2 \times \mathbb{Z}_2$  and initially have choices for the apolar and longitudinal symmetry vectors with indices  $(\nu_1^{L+T}, \nu_2^{L+T}) = (0, 1)$  and  $(\nu_1^L, \nu_2^L) = (1, 0)$ , corresponding to  $\nu^{L+T} = 1$ ,  $\nu^L = 1$ , and  $\nu^T = (1 - 1) \bmod 2 = 0$ . If we then add a longitudinal symmetry vector with indices  $(\tilde{\nu}_1^L, \tilde{\nu}_2^L) = (1, 0)$ , we obtain new indices  $(\tilde{\nu}_1^{L+T}, \tilde{\nu}_2^{L+T}) = (1, 1)$  and  $(\tilde{\nu}_1^L, \tilde{\nu}_2^L) = ((1 + 1) \bmod 2, 0) = (0, 0)$  with corresponding coarse-grained indices  $\tilde{\nu}^{L+T} = 1$ ,  $\tilde{\nu}^L = 0$ , and  $\tilde{\nu}^T = (1 - 0) \bmod 2 = 1$ : i.e., we find that  $\tilde{\nu}^T$  differs from  $\nu^T$  and that the definition is not invariant.

#### S4. TIME-REVERSAL BROKEN $\Gamma$ -ENFORCED TOPOLOGY

As summarized in [Supplemental Figure 2](#) of the main text, 32 space groups exhibit  $\Gamma$ -enforced topology in their minimum-connectivity bands below the fundamental bandgap in a time-reversal (TR) broken setting, namely:

13 (P2/c), 48 (Pnnn), 49 (Pccm), 50 (Pban), 68 (Ccca), 73 (Ibca), 85 (P4/n), 86 (P4<sub>2</sub>/n), 87 (I4/m), 106 (P4<sub>2</sub>bc), 110 (I4<sub>1</sub>cd), 116 (P4<sub>2</sub>c2), 117 (P4<sub>2</sub>b2), 118 (P4<sub>2</sub>n2), 120 (I4<sub>2</sub>c2), 124 (P4/mcc), 126 (P4/nnc), 130 (P4/ncc), 133 (P4<sub>2</sub>/nbc), 142 (I4<sub>1</sub>/acd), 163 (P3<sub>1</sub>c), 165 (P3<sub>2</sub>c1), 167 (R3c), 190 (P6<sub>2</sub>c), 192 (P6/mcc), 201 (Pn3), 206 (Ia3), 218 (P4<sub>2</sub>3n), 219 (F4<sub>2</sub>3c), 222 (Pn3n), 228 (Fd3c), and 230 (Ia3d).

An important question to ask of these space groups, is whether TR can be broken by a uniform magnetic field  $\mathbf{B} = B\hat{\mathbf{n}}$  without simultaneously breaking a spatial symmetry of the space group. In practice, this requires that all rotation axes, roto-inversion axes, and mirror normals are aligned with  $\hat{\mathbf{n}}$  (a uniform magnetic field is invariant under inversion, since the magnetic field is a pseudovector; similarly for mirror planes aligned with  $\hat{\mathbf{n}}$ ). A simple consequence of this is that the existence of two or more mirror planes with distinct normals excludes compatibility with a uniform magnetic field.

Of the above candidates, only space groups 13 (P2/c), 85 (P4/n), 86 (P4<sub>2</sub>/n), and 87 (I4/m) are compatible with this requirement, permitting a uniform magnetic field aligned with the lattice vector  $\mathbf{R}_2$  in space group 13 and aligned with  $\mathbf{R}_3$  (conventional setting) in space groups 85–87. Regrettably, to realize  $\Gamma$ -enforced topology which isn't merely a copy of its TR-invariant counterpart for these space groups, one requires either large TR-breaking amplitudes or a fine-tuned TR-invariant configuration, as we explain below by analyzing each case in detail:

##### A. Space group 13 (P2/c)

The minimum connectivity is  $\mu^T = 2$  with TR and  $\tilde{\mu}^T = 2$  without TR, hosting  $\Gamma$ -enforced topology in either case. TR symmetry does not cause the irreps of space group 13 to stick together and the EBRs are similarly unaffected. The presence of TR-broken  $\Gamma$ -enforced topology is therefore just a direct equivalent of its TR-invariant counterpart.

##### B. Space group 86 (P4<sub>2</sub>/n)

The minimum connectivity is  $\mu^T = 2$  with TR and  $\tilde{\mu}^T = 2$  without TR, hosting  $\Gamma$ -enforced topology in either case. There are 4 TR-broken solutions and 2 TR-invariant solutions. One pair of solutions,  $[(\blacksquare)^{2T}, A_1^\mp + A_2^\pm, M_1, Z_2, R_1, X_1]^T$ , exists in either setting (with TR-invariant index  $1 \in \mathbb{Z}_2$  and TR-broken indices  $(1, 1) \in \mathbb{Z}_2 \times \mathbb{Z}_2$ ), cf. [Supplemental Sections S8.A](#) and [S8.B](#). The remaining pair of TR-broken solutions,  $[(\blacksquare)^{2T}, A_3^\mp + A_4^\pm, M_2, Z_2, R_1, X_1]^T$ , is not related to the TR-invariant solutions and has different topological indices  $(1, 0) \in \mathbb{Z}_2 \times \mathbb{Z}_2$ . This “new” pair of solutions is possible only under TR-breaking,

because TR otherwise causes the 1D complex irreps  $\Gamma_{3,4}^{\pm}$  and  $A_{3,4}^{\pm}$  to stick together as 2D coreps  $\Gamma_3^{\pm}\Gamma_4^{\pm}$  and  $A_3^{\pm}A_4^{\pm}$ .

It is not possible, however, to bring these new solutions into existence by applying a perturbative (i.e., small) TR-breaking term to a (not fine-tuned) TR-invariant  $\mu^T = 4$  configuration. This is because the new TR-broken solutions have zero parity at  $A$  (cf. the  $A_3^{\mp} + A_4^{\pm}$  combination)—but the corep  $A_3^{\pm}A_4^{\pm}$  has parity  $\pm 2$  (which is not changed by splitting the corep, of course). The states could potentially be realized by first splitting the  $A$ -coreps of a  $\mu^T = 4$  state with  $A_3^+A_4^+ + A_3^-A_4^-$  (2 such solutions exist) into  $A_3^+ + A_4^+$  and  $A_3^- + A_4^-$  groupings by a perturbative TR-breaking; and then subsequently driving a band-inversion between these groups. This, however, requires either a large TR-breaking or a fine-tuned initial TR-invariant configuration with near-degenerate  $A_3^+A_4^+$  and  $A_3^-A_4^-$  states.

### C. Space group 87 (I4/m)

The minimum connectivity is  $\mu^T = 3$  with TR and  $\tilde{\mu}^T = 2$  without TR. Interestingly, the  $\tilde{\mu}^T = 2$  solution *cannot* be obtained from a  $\mu^T = 3$  solution by perturbatively breaking TR. To see this, we observe that all TR-respecting solutions corresponding to  $\mu^T = 3$  have the following symmetry content at the M-point (cf. [Supplemental Section S8.A](#)):

$$M_1^- + M_3^-M_4^- \text{ or } M_2^- + M_3^-M_4^- \text{ or } M_1^+ + M_3^+M_4^+ \text{ or } M_2^+ + M_3^+M_4^+ \quad (\text{S27a})$$

while all the  $\tilde{\mu}^T = 2$  TR-broken solutions have M-point symmetry content of the form (cf. [Supplemental Section S8.B](#)):

$$M_3^+ + M_4^- \text{ or } M_3^- + M_4^+. \quad (\text{S27b})$$

The solutions in [Eq. \(S27a\)](#) have total parity  $-3$  or  $+3$  (i.e., sum of inversion eigenvalues, each indicated by the irrep superscript), while the solutions in [Eq. \(S27b\)](#) have total parity 0 (plus an unknown contribution of  $\pm 1$  from the—by assumption—split-off band). Since a TR-breaking perturbation cannot change this parity, the two sets of solutions cannot be connected by a small TR-breaking perturbation (but would require multiple band inversions).

In fact, since all  $\tilde{\mu}^T = 2$  solutions have the  $M_3^{\pm} + M_4^{\mp}$  symmetry and since the  $M_3^{\pm}$  and  $M_4^{\pm}$  irreps are complex and stick together under TR in the combinations  $M_3^+M_4^+$  and  $M_3^-M_4^-$ , realizing a  $\tilde{\mu}^T = 2$  state by breaking TR perturbatively must necessarily start from a grouping of bands with accidentally degenerate  $M_3^+M_4^+$  and  $M_3^-M_4^-$  states, i.e., a symmetry vector containing both of these physical irreps. We have verified by explicit enumeration that such a configuration requires  $\mu^T = 5$ —and that all such states are simple sums of a  $\mu^T = 3$  state and a “detachable”  $\mu = 2$  state (i.e. the sum of a solution to the transverse minimum connectivity problem and a Hilbert basis vector with filling  $\mu = 2$ ).

Summarizing these considerations, we conclude that realizing  $\tilde{\mu}^T = 2$   $\Gamma$ -enforced topology in space group 87 requires either a large TR-breaking amplitude (which drives multiple band inversions) or a perturbative TR breaking applied to a fine-tuned TR-invariant state with accidentally degenerate  $M_3^+M_4^+$  and  $M_3^-M_4^-$  states.

### D. Space group 85 (P4/n)

The minimum connectivity is  $\mu^T = 4$  with TR and  $\tilde{\mu}^T = 2$  without TR. TR causes the 1D irreps  $Z_3^{\pm}$  and  $Z_4^{\pm}$  to stick together as 2D irreps  $Z_3^{\pm}Z_4^{\pm}$  (and similarly so for the  $\Gamma_3^{\pm}$  and  $\Gamma_4^{\pm}$  irreps). With broken TR symmetry, there are four  $\tilde{\mu}^T = 2$  solutions. We focus on their  $Z$ -point symmetry content, which is of the form:

$$Z_3^{\pm} + Z_4^{\mp} = \{Z_3^+ + Z_4^- \text{ or } Z_3^- + Z_4^+\}. \quad (\text{S28a})$$

With TR symmetry, there are 24  $\mu^T = 4$  solutions, which exhibit the following  $Z$ -point variations:

$$Z_1^{\pm} + Z_2^{\pm} + Z_3^{\pm}Z_4^{\pm} \text{ or } 2Z_1^{\pm} + Z_3^{\pm}Z_4^{\pm} \text{ or } 2Z_2^{\pm} + Z_3^{\pm}Z_4^{\pm}. \quad (\text{S28b})$$

The TR-broken solutions in Eq. (S28a) have a total parity of 0, while the TR-invariant solutions in Eq. (S28b) have a parity of  $\pm 4$ . Accordingly, the same reasoning as in Supplemental Section S4.C applies: the TR-broken  $\tilde{\mu}^T = 2$   $\Gamma$ -enforced state cannot be realized by breaking TR perturbatively with a starting point in a  $\mu^T = 4$  a state (unless a fine-tuned accidental degeneracy exists).

## S5. HIGHER-ORDER MINIMUM-CONNECTIVITY SOLUTIONS

Besides minimum-connectivity solutions of the  $\omega = 0$  connected bands, it is interesting to consider what other connectivities are possible for photonic bands that connect to  $\omega = 0$ . To that end, we define a notion of an  $n$ th minimum-connectivity solution as one whose connectivity  $\mu_n^T$  is greater than the  $(n - 1)$ th minimum-connectivity, i.e., such that  $\mu_n^T > \mu_{n-1}^T$ . The solutions associated with  $\mu_1^T$  are simply the minimum-connectivity solutions we have focused on up to this point, i.e.,  $\mu^T \equiv \mu_1^T$ . The “second” minimum-connectivity solutions associated with  $\mu_2^T$  correspond to the next-most-minimal connectivity, and so on.

It is straightforward to adapt our existing approach to search for these “higher-order” solutions by simply increasing the initial guess for total connectivity for  $n$ th minimum-connectivity solution to  $\mu_{n-1}^{L+T} + 1$  and incrementing therefrom. With this small revision, we can readily compute the next-most-minimal connectivities  $\mu_2^T$  and so on.\* The tabulated listings in Supplemental Sections S8.A and S8.B give  $\mu_2^T$  in all space groups.

### A. What is the *realized* minimum connectivity of space groups with $\Gamma$ -enforced topology?

The minimum-connectivity TR-invariant solutions of space groups 13, 48, 49, 50, 68, and 86 are all nontrivial, i.e., manifest  $\Gamma$ -enforced topology. Since all symmetry-indicated stable topological phases of time-reversal invariant bosons are associated with *gapless* topology [S28], this entails that each such minimum-connectivity solution *must* connect to a higher-frequency regular solution which fulfills the compatibility relations on its own (since space groups 13, 48, 49, 50, 68, and 86 are all centrosymmetric, these connections manifest as nodal lines): this underlies the concept of topological non-gaps introduced in the main text. The minimum connectivity of these space groups is therefore larger than what is suggested by compatibility relations alone (i.e., is *not* equal to 2, as suggested by Supplemental Figure 2). An important follow-up question is therefore “what is the *realized* minimum connectivity, when accounting for topological degeneracies?” We can answer this question simply by looking at the second-order minimum-connectivity solutions: if any of these solutions are trivial, they in fact give the actual minimum connectivity. With this approach, we have verified that the *realized* minimum connectivity of these space groups in fact is  $\mu^T = 4$ .

Note that similar conclusions cannot be directly translated to space groups with TR-broken  $\Gamma$ -enforced topology, because the TR-broken setting also includes gapped bosonic topology (e.g., Chern insulators [S29]) and not just nodal degeneracies.

## S6. $\Gamma$ -ENFORCED BOSONIC TOPOLOGY OF REGULAR BANDS

Above the fundamental gap, all photonic bands have “regular” symmetry content. It is natural to ask what the possible connectivities of these regular bands are. To answer this, we turn to the compatibility basis

---

\* In practice, these higher-order solutions need not be completely connected. Specifically, they can be built from a “singular” and a “regular” solution – which are separable – in the following sense: an  $n$ th order solution of connectivity  $\mu_n^T = \mu_m^T + \mu$  may be (but is not always) the sum of a lower-order  $m < n$  “singular” (i.e., zero-frequency connected) solution with connectivity  $\mu_m^T$  and a “regular” (i.e., a Hilbert basis vector, or a span thereof) solution with connectivity  $\mu$ .



$\{\mathbf{h}_i\}$  from [Supplemental Section S1.D](#). Each Hilbert basis vector  $\mathbf{h}_i$  necessarily describes a connected grouping of bands: if it did not, we could write it as the sum of band groupings—i.e., Hilbert basis vectors—in contradiction of the minimal property of Hilbert bases. Thus, the possible connectivities of a given space group  $\{\mu\}$  are just the unique connectivities in the compatibility basis  $\{\mathbf{h}_i\}$ . [Supplemental Table V](#) gives the connectivities of regular photonic (or, bosonic) bands for all space groups with TR.

For each connectivity, we can additionally ask whether *all* possible realizations of that connectivity are topologically nontrivial or not, i.e., whether they exhibit filling-enforced topology. To do so, we simply compute the topology of each Hilbert basis vector (see [Supplemental Section S1.F](#)). Connectivities with filling-enforced topology are highlighted in [Supplemental Table V](#), and color-coded according to three partitions: all-nontrivial, all-fragile, or mixed nontrivial–fragile filling-enforced topology. Only three space groups support all-nontrivial filling-enforced topology with TR, namely space groups 87, 175, and 176. By comparison, all-fragile and mixed nontrivial–fragile filling-enforced topology is much more prevalent. Of note, we observe that the minimum-connectivity bands never hosts filling-enforced topology, regardless of space group type.

[Supplemental Table VI](#) gives the analogous results with broken TR-symmetry: there, the minimum-connectivity bands occasionally do host filling-enforced topology (space groups 106, 110, 220, and 230).

| SG | $\mu$                             | SG  | $\mu$                                | SG  | $\mu$                             | SG  | $\mu$                                                         |
|----|-----------------------------------|-----|--------------------------------------|-----|-----------------------------------|-----|---------------------------------------------------------------|
| 1  | 1                                 | 64  | 2, 4                                 | 126 | 2, 4, 8                           | 186 | 2, 4                                                          |
| 2  | 1                                 | 65  | 1, 2, <b>3, 4, 5, 6, 7, 10</b>       | 127 | 2, 4, <b>6, 8</b>                 | 187 | 1, 2, <b>3, 4</b>                                             |
| 3  | 1                                 | 66  | 2, <b>4</b>                          | 128 | 2, 4, <b>6, 8</b>                 | 188 | 2, 4, <b>6</b>                                                |
| 4  | 2                                 | 67  | 2, <b>4, 6, 8</b>                    | 129 | 2, 4, <b>8</b>                    | 189 | 1, 2, <b>4</b>                                                |
| 5  | 1                                 | 68  | 2, 4                                 | 130 | 4, 8                              | 190 | 2, 4                                                          |
| 6  | 1                                 | 69  | 1, 2, <b>4, 5</b>                    | 131 | 2, <b>4, 6, 8, 10, 12, 14, 16</b> | 191 | 1, 2, <b>3, 4, 5, 6, 7, 8, 10</b>                             |
| 7  | 2                                 | 70  | 2, 4                                 | 132 | 2, 4, <b>6, 8, 10</b>             | 192 | 2, 4, <b>6, 8</b>                                             |
| 8  | 1                                 | 71  | 1, <b>2, 3, 4, 5, 6</b>              | 133 | 4, 8, <b>12</b>                   | 193 | 2, 4, <b>6, 8, 10, 12, 14, 16, 20</b>                         |
| 9  | 2                                 | 72  | 2, 4                                 | 134 | 2, 4, <b>6, 8, 10, 12, 16</b>     | 194 | 2, 4, <b>8</b>                                                |
| 10 | 1, <b>2</b>                       | 73  | 4, <b>12</b>                         | 135 | 4, <b>8</b>                       | 195 | 1, 2, 3                                                       |
| 11 | 2                                 | 74  | 2, <b>4, 6</b>                       | 136 | 2, 4, <b>6, 8</b>                 | 196 | 1, 2, 3                                                       |
| 12 | 1, 2                              | 75  | 1, 2                                 | 137 | 2, 4, 8                           | 197 | 1, 2, 3                                                       |
| 13 | 2                                 | 76  | 4                                    | 138 | 4, <b>8, 12, 16</b>               | 198 | 4, 8                                                          |
| 14 | 2                                 | 77  | 2                                    | 139 | 1, 2, <b>3, 4, 5, 6, 7, 8</b>     | 199 | 4, 6, 8                                                       |
| 15 | 2                                 | 78  | 4                                    | 140 | 2, 4, <b>6, 8, 10, 12, 16</b>     | 200 | 1, 2, 3, <b>4, 5, 6, 7, 8, 9, 10, 11, 12, 14</b>              |
| 16 | 1, <b>2</b>                       | 79  | 1, 2                                 | 141 | 2, 4, <b>6, 8</b>                 | 201 | 2, 4, 6, 8, <b>12</b>                                         |
| 17 | 2                                 | 80  | 2                                    | 142 | 4, 8, <b>12</b>                   | 202 | 1, 2, 3, 4, <b>5, 6, 8</b>                                    |
| 18 | 2                                 | 81  | 1, 2                                 | 143 | 1, 2                              | 203 | 2, 4, 6, 8                                                    |
| 19 | 4                                 | 82  | 1, 2                                 | 144 | 3                                 | 204 | 1, 2, 3, 4, <b>5, 6, 7, 8, 9, 10, 11, 12</b>                  |
| 20 | 2                                 | 83  | 1, 2, <b>3, 4, 5, 6</b>              | 145 | 3                                 | 205 | 4, 8                                                          |
| 21 | 1, 2                              | 84  | 2, <b>4</b>                          | 146 | 1, 2                              | 206 | 4, 8, 12                                                      |
| 22 | 1                                 | 85  | 2, 4                                 | 147 | 1, 2                              | 207 | 1, 2, 3                                                       |
| 23 | 1                                 | 86  | 2, 4                                 | 148 | 1, 2                              | 208 | 2, 4, 6                                                       |
| 24 | 2                                 | 87  | 1, 2, <b>3, 4, 5</b>                 | 149 | 1, 2                              | 209 | 1, 2, 3, 6                                                    |
| 25 | 1, <b>2</b>                       | 88  | 2, 4                                 | 150 | 1, 2                              | 210 | 2, 4, 6                                                       |
| 26 | 2                                 | 89  | 1, 2                                 | 151 | 3                                 | 211 | 1, 2, 3, 4, 6                                                 |
| 27 | 2                                 | 90  | 2, 4                                 | 152 | 3                                 | 212 | 4, 8                                                          |
| 28 | 2                                 | 91  | 4                                    | 153 | 3                                 | 213 | 4, 8                                                          |
| 29 | 4                                 | 92  | 4                                    | 154 | 3                                 | 214 | 4, 6, 8                                                       |
| 30 | 2                                 | 93  | 2, <b>4</b>                          | 155 | 1, 2                              | 215 | 1, 2, 3, <b>4, 6</b>                                          |
| 31 | 2                                 | 94  | 2, 4                                 | 156 | 1, 2                              | 216 | 1, 2, 3                                                       |
| 32 | 2                                 | 95  | 4                                    | 157 | 1, 2                              | 217 | 1, 2, 3, <b>4, 6</b>                                          |
| 33 | 4                                 | 96  | 4                                    | 158 | 2, 4                              | 218 | 2, 4, 6, <b>8, 12</b>                                         |
| 34 | 2                                 | 97  | 1, 2                                 | 159 | 2, 4                              | 219 | 2, 4, 6, <b>8, 12</b>                                         |
| 35 | 1, 2                              | 98  | 2, 4                                 | 160 | 1, 2                              | 220 | 6, 8, 12, 16                                                  |
| 36 | 2                                 | 99  | 1, 2                                 | 161 | 2, 4                              | 221 | 1, 2, 3, <b>4, 5, 6, 7, 8, 9, 10, 11, 12, 13, 14, 15, 16</b>  |
| 37 | 2                                 | 100 | 2, 4                                 | 162 | 1, 2                              | 222 | 2, 4, 6, 8, 12, <b>14, 16, 18, 24</b>                         |
| 38 | 1                                 | 101 | 2, 4                                 | 163 | 2, 4                              | 223 | 2, 4, 6, 8, <b>10, 12, 14, 16, 18, 20</b>                     |
| 39 | 2                                 | 102 | 2, 4                                 | 164 | 1, 2                              | 224 | 2, 4, 6, 8, <b>10, 12, 14, 16, 18, 20, 22, 24, 26, 28, 32</b> |
| 40 | 2                                 | 103 | 2, 4                                 | 165 | 2, 4                              | 225 | 1, 2, 3, 4, <b>5, 6, 7, 8, 9, 10, 11, 12</b>                  |
| 41 | 2                                 | 104 | 2, 4                                 | 166 | 1, 2                              | 226 | 2, 4, 6, <b>8, 10, 12, 14, 16, 18, 20, 22, 26</b>             |
| 42 | 1, 2                              | 105 | 2, <b>4</b>                          | 167 | 2, 4                              | 227 | 2, 4, 6, 8, <b>10, 12</b>                                     |
| 43 | 2                                 | 106 | 4                                    | 168 | 1, 2                              | 228 | 4, 8, 12, 16, <b>20</b>                                       |
| 44 | 1                                 | 107 | 1, 2                                 | 169 | 6                                 | 229 | 1, 2, 3, 4, <b>5, 6, 7, 8, 9, 10, 11, 12, 13, 15, 16</b>      |
| 45 | 2                                 | 108 | 2, 4                                 | 170 | 6                                 | 230 | 8, 12, 16, <b>20, 24</b>                                      |
| 46 | 2                                 | 109 | 2                                    | 171 | 3                                 |     |                                                               |
| 47 | 1, <b>2, 3, 4, 5, 6, 7, 8, 10</b> | 110 | 4                                    | 172 | 3                                 |     |                                                               |
| 48 | 2, 4                              | 111 | 1, 2, <b>3, 4</b>                    | 173 | 2, 4                              |     |                                                               |
| 49 | 2, <b>4</b>                       | 112 | 2, <b>4</b>                          | 174 | 1, 2, <b>3, 4</b>                 |     |                                                               |
| 50 | 2, 4                              | 113 | 2, 4                                 | 175 | 1, 2, <b>3, 4, 5, 6</b>           |     |                                                               |
| 51 | 2, <b>4</b>                       | 114 | 2, 4                                 | 176 | 2, 4, <b>6, 8</b>                 |     |                                                               |
| 52 | 4                                 | 115 | 1, 2                                 | 177 | 1, 2                              |     |                                                               |
| 53 | 2, 4                              | 116 | 2, 4                                 | 178 | 6                                 |     |                                                               |
| 54 | 4                                 | 117 | 2, 4                                 | 179 | 6                                 |     |                                                               |
| 55 | 2, <b>4</b>                       | 118 | 2, 4                                 | 180 | 3, <b>6</b>                       |     |                                                               |
| 56 | 4                                 | 119 | 1, 2                                 | 181 | 3, <b>6</b>                       |     |                                                               |
| 57 | 4                                 | 120 | 2, <b>4</b>                          | 182 | 2, 4                              |     |                                                               |
| 58 | 2                                 | 121 | 1, 2                                 | 183 | 1, 2                              |     |                                                               |
| 59 | 2, 4                              | 122 | 2, 4                                 | 184 | 2, 4                              |     |                                                               |
| 60 | 4                                 | 123 | 1, 2, <b>3, 4, 5, 6, 7, 8, 9, 10</b> | 185 | 2, 4                              |     |                                                               |
| 61 | 4                                 | 124 | 2, 4, <b>6, 8</b>                    |     |                                   |     |                                                               |
| 62 | 4                                 | 125 | 2, 4, <b>6, 8</b>                    |     |                                   |     |                                                               |
| 63 | 2, 4                              |     |                                      |     |                                   |     |                                                               |

**Supplemental Table V. Possible connectivities of regular, connected bosonic bands with TR.** Connectivities with filling-enforced topology are highlighted in bold. The type of filling-enforced topology is color-coded: **all-nontrivial** in red, **all-fragile** in blue, and **mixed nontrivial-fragile** in green. Applicable to bands above the fundamental gap, i.e., *not* connected to  $\omega = 0$ .

| SG | $\mu$                                        | SG  | $\mu$                                           | SG  | $\mu$                                        | SG  | $\mu$                                                                                          |
|----|----------------------------------------------|-----|-------------------------------------------------|-----|----------------------------------------------|-----|------------------------------------------------------------------------------------------------|
| 1  | 1                                            | 64  | 2, 4                                            | 126 | 2, 4                                         | 187 | 1, 2, <b>3, 4</b>                                                                              |
| 2  | 1                                            | 65  | 1, 2, <b>3, 4, 5, 6</b> ,<br><b>7, 10</b>       | 127 | 2, <b>4, 6, 8</b>                            | 188 | 2, <b>4</b>                                                                                    |
| 3  | 1                                            | 66  | 2, <b>4</b>                                     | 128 | 2, 4                                         | 189 | 1, 2, <b>4, 6</b>                                                                              |
| 4  | 2                                            | 67  | 2, <b>4, 6, 8</b>                               | 129 | 2, 4, <b>8</b>                               | 190 | 2                                                                                              |
| 5  | 1                                            | 68  | 2, 4                                            | 130 | 4                                            | 191 | 1, 2, <b>3, 4, 5, 6</b> ,<br><b>7, 8, 10</b>                                                   |
| 6  | 1                                            | 69  | 1, 2, <b>4, 5</b>                               | 131 | 2, <b>4, 6, 8, 10</b> ,<br><b>12, 14, 16</b> | 192 | 2, 4                                                                                           |
| 7  | 2                                            | 70  | 2, 4                                            | 132 | 2, 4, <b>6, 8, 10</b>                        | 193 | 2, 4, <b>6, 8, 10, 12</b>                                                                      |
| 8  | 1                                            | 71  | 1, <b>2, 3, 4, 5, 6</b>                         | 133 | 4, <b>6, 8</b>                               | 194 | 2, 4, <b>8</b>                                                                                 |
| 9  | 2                                            | 72  | 2, 4                                            | 134 | 2, 4, <b>6, 8, 10</b> ,<br><b>12, 16</b>     | 195 | 1, 3                                                                                           |
| 10 | 1, <b>2</b>                                  | 73  | 4, <b>6</b>                                     | 135 | 4, <b>8</b>                                  | 196 | 1, 3                                                                                           |
| 11 | 2                                            | 74  | 2, <b>4, 6</b>                                  | 136 | 2, 4, <b>6, 8</b>                            | 197 | 1, 3                                                                                           |
| 12 | 1, 2                                         | 75  | 1                                               | 137 | 2, 4, 8                                      | 198 | 4                                                                                              |
| 13 | 2                                            | 76  | 4                                               | 138 | 4, <b>8, 12</b>                              | 199 | 4, 6                                                                                           |
| 14 | 2                                            | 77  | 2                                               | 139 | 1, 2, <b>3, 4, 5, 6</b> ,<br><b>7, 8</b>     | 200 | 1, <b>2, 3, 4, 5, 6</b> ,<br><b>7, 9, 10, 12</b>                                               |
| 15 | 2                                            | 78  | 4                                               | 140 | 2, 4, <b>6, 8, 10</b>                        | 201 | 2, 4, 6, <b>12</b>                                                                             |
| 16 | 1, <b>2</b>                                  | 79  | 1                                               | 141 | 2, 4, <b>6, 8</b>                            | 202 | 1, 2, 3, <b>4, 5, 6</b>                                                                        |
| 17 | 2                                            | 80  | 2                                               | 142 | 4, <b>6, 8</b>                               | 203 | 2, 4, 6                                                                                        |
| 18 | 2                                            | 81  | 1                                               | 143 | 1                                            | 204 | 1, <b>2, 3, 4, 5, 6</b> ,<br><b>7, 9, 10, 12</b>                                               |
| 19 | 4                                            | 82  | 1                                               | 144 | 3                                            | 205 | 4                                                                                              |
| 20 | 2                                            | 83  | 1, <b>2</b>                                     | 145 | 3                                            | 206 | 4, <b>6</b>                                                                                    |
| 21 | 1, 2                                         | 84  | 2, <b>4</b>                                     | 146 | 1                                            | 207 | 1, 2, 3                                                                                        |
| 22 | 1                                            | 85  | 2                                               | 147 | 1                                            | 208 | 2, 4, 6                                                                                        |
| 23 | 1                                            | 86  | 2, 4                                            | 148 | 1                                            | 209 | 1, 2, 3, 6                                                                                     |
| 24 | 2                                            | 87  | 1, 2                                            | 149 | 1, 2                                         | 210 | 2, 4, 6                                                                                        |
| 25 | 1, <b>2</b>                                  | 88  | 2, 4                                            | 150 | 1, 2                                         | 211 | 1, 2, 3, 4, 6                                                                                  |
| 26 | 2                                            | 89  | 1, 2                                            | 151 | 3                                            | 212 | 4, 8                                                                                           |
| 27 | 2                                            | 90  | 2                                               | 152 | 3                                            | 213 | 4, 8                                                                                           |
| 28 | 2                                            | 91  | 4                                               | 153 | 3                                            | 214 | 4, 6, 8                                                                                        |
| 29 | 4                                            | 92  | 4                                               | 154 | 3                                            | 215 | 1, 2, 3, <b>4, 6</b>                                                                           |
| 30 | 2                                            | 93  | 2, <b>4</b>                                     | 155 | 1, 2                                         | 216 | 1, 2, 3                                                                                        |
| 31 | 2                                            | 94  | 2, 4                                            | 156 | 1, 2                                         | 217 | 1, 2, 3, <b>4, 6</b>                                                                           |
| 32 | 2                                            | 95  | 4                                               | 157 | 1, 2                                         | 218 | 2, <b>4, 6</b>                                                                                 |
| 33 | 4                                            | 96  | 4                                               | 158 | 2                                            | 219 | 2, <b>4, 6</b>                                                                                 |
| 34 | 2                                            | 97  | 1, 2                                            | 159 | 2                                            | 220 | <b>4, 6, 8</b>                                                                                 |
| 35 | 1, 2                                         | 98  | 2, 4                                            | 160 | 1, 2                                         | 221 | 1, 2, 3, <b>4, 5, 6, 7</b> ,<br><b>8, 9, 10, 11, 12</b> ,<br><b>13, 14, 15, 16</b>             |
| 36 | 2                                            | 99  | 1, 2                                            | 161 | 2                                            | 222 | 2, 4, 6, 8, <b>12</b>                                                                          |
| 37 | 2                                            | 100 | 2                                               | 162 | 1, 2                                         | 223 | 2, 6, 8, <b>10, 12</b> ,<br><b>14, 16, 18, 20</b>                                              |
| 38 | 1                                            | 101 | 2, 4                                            | 163 | 2                                            | 224 | 2, 4, 6, 8, <b>10</b> ,<br><b>12, 14, 16, 18</b> ,<br><b>20, 22, 24, 26</b> ,<br><b>28, 32</b> |
| 39 | 2                                            | 102 | 2, 4                                            | 164 | 1, 2                                         | 225 | 1, 2, 3, 4, <b>5, 6, 7</b> ,<br><b>8, 9, 10, 11, 12</b>                                        |
| 40 | 2                                            | 103 | 2                                               | 165 | 2                                            | 226 | 2, 4, 6, <b>8, 10</b> ,<br><b>12, 14, 16, 18</b>                                               |
| 41 | 2                                            | 104 | 2                                               | 166 | 1, 2                                         | 227 | 2, 4, 6, 8, <b>10, 12</b>                                                                      |
| 42 | 1, 2                                         | 105 | 2, <b>4</b>                                     | 167 | 2                                            | 228 | 4, <b>6, 8, 10, 12</b>                                                                         |
| 43 | 2                                            | 106 | <b>2, 4</b>                                     | 168 | 1                                            | 229 | 1, 2, 3, 4, <b>5, 6, 7</b> ,<br><b>8, 9, 10, 11, 12</b> ,<br><b>13, 15, 16</b>                 |
| 44 | 1                                            | 107 | 1, 2                                            | 169 | 6                                            | 230 | <b>6, 8, 10, 12</b>                                                                            |
| 45 | 2                                            | 108 | 2                                               | 170 | 6                                            |     |                                                                                                |
| 46 | 2                                            | 109 | 2                                               | 171 | 3                                            |     |                                                                                                |
| 47 | 1, <b>2, 3, 4, 5, 6</b> ,<br><b>7, 8, 10</b> | 110 | <b>2, 4</b>                                     | 172 | 3                                            |     |                                                                                                |
| 48 | 2, 4                                         | 111 | 1, 2, <b>3, 4</b>                               | 173 | 2                                            |     |                                                                                                |
| 49 | 2, <b>4</b>                                  | 112 | 2, <b>4</b>                                     | 174 | 1, <b>2</b>                                  |     |                                                                                                |
| 50 | 2, 4                                         | 113 | 2                                               | 175 | 1, <b>2</b>                                  |     |                                                                                                |
| 51 | 2, <b>4</b>                                  | 114 | 2                                               | 176 | 2, <b>4</b>                                  |     |                                                                                                |
| 52 | 4                                            | 115 | 1, 2                                            | 177 | 1, 2                                         |     |                                                                                                |
| 53 | 2, 4                                         | 116 | 2                                               | 178 | 6                                            |     |                                                                                                |
| 54 | 4                                            | 117 | 2                                               | 179 | 6                                            |     |                                                                                                |
| 55 | 2, <b>4</b>                                  | 118 | 2                                               | 180 | 3, <b>6</b>                                  |     |                                                                                                |
| 56 | 4                                            | 119 | 1, 2                                            | 181 | 3, <b>6</b>                                  |     |                                                                                                |
| 57 | 4                                            | 120 | 2                                               | 182 | 2, 4                                         |     |                                                                                                |
| 58 | 2                                            | 121 | 1, 2                                            | 183 | 1, 2                                         |     |                                                                                                |
| 59 | 2, 4                                         | 122 | 2, 4                                            | 184 | 2                                            |     |                                                                                                |
| 60 | 4                                            | 123 | 1, 2, <b>3, 4, 5, 6</b> ,<br><b>7, 8, 9, 10</b> | 185 | 2, 4                                         |     |                                                                                                |
| 61 | 4                                            | 124 | 2, 4                                            | 186 | 2, 4                                         |     |                                                                                                |
| 62 | 4                                            | 125 | 2, 4, <b>6, 8</b>                               |     |                                              |     |                                                                                                |
| 63 | 2, 4                                         |     |                                                 |     |                                              |     |                                                                                                |

**Supplemental Table VI. Possible connectivities of regular, connected bosonic bands without TR.** Connectivities with filling-enforced topology are highlighted in bold. The type of filling-enforced topology is color-coded: **all-nontrivial** in red, **all-fragile** in blue, and **mixed nontrivial-fragile** in green. Applicable to bands above the fundamental gap, i.e., *not* connected to  $\omega = 0$ .

### S7. DIELECTRIC OBSTRUCTIONS IN SPACE GROUP 230 ( $1a\bar{3}d$ )

Here, we elaborate on the difficulty of realizing a  $\mu^T = 8$  solution in space group 230 (referred to as a dielectric obstruction in the main text). There are four distinct  $\mu^T = 8$  solutions in space group 230 (see [Supplemental Section S8.A](#)):

$$[(\blacksquare)^{2T} + \Gamma_1^- + \Gamma_2^+ + \Gamma_2^- + \Gamma_4^-, H_1 + H_4, 2P_3, 3N_1 + N_2]^T, \quad (\text{S29a})$$

$$[(\blacksquare)^{2T} + \Gamma_1^+ + \Gamma_2^+ + \Gamma_2^- + \Gamma_4^+, H_1 + H_4, 2P_3, 3N_1 + N_2]^T, \quad (\text{S29b})$$

$$[(\blacksquare)^{2T} + \Gamma_1^+ + \Gamma_1^- + \Gamma_2^- + \Gamma_5^-, H_1 + H_4, 2P_3, 2N_1 + 2N_2]^T, \quad (\text{S29c})$$

$$[(\blacksquare)^{2T} + \Gamma_1^+ + \Gamma_1^- + \Gamma_2^+ + \Gamma_5^+, H_1 + H_4, 2P_3, 2N_1 + 2N_2]^T. \quad (\text{S29d})$$

Each solution is fully consistent with all compatibility relations across the BZ, as we have verified explicitly by manually checking every relations ([Supplemental Figures S4](#) and [S5](#)). Despite this, it is extremely challenging to realize the required band symmetries in photonic crystals composed of realistic dielectric materials due to the required symmetry content. Concretely, the requirement of a  $\Gamma_1^\pm$  irrep in all  $\mu^T = 8$  solutions is troublesome\*: comparing with the empty-lattice (i.e., constant permittivity) dispersion diagram ([Supplemental Figure S6](#)), we see that these irreps do not occur in the first 38 bands (appearing first in a 48-fold degenerate band grouping in bands 39 to 86). As a result, to bring a  $\Gamma_1^\pm$  irrep into the first 8 bands, at least 30 band inversions must be driven as we interpolate between a concrete PhC and the empty lattice in space group 230. This would require very large dielectric contrasts, likely beyond those that can be realized with conventional dielectric materials. This effectively places a strong dielectric obstruction to realizing the  $\mu^T = 8$  solutions [Eqs. \(S29\)](#) with conventional PhCs (although realizations may be possible with metallic PhCs, since their dispersions can be very far from the empty lattice).

The second-order solutions in space group 230 have connectivity  $\mu_2^T = 12$ . Among these are two solutions

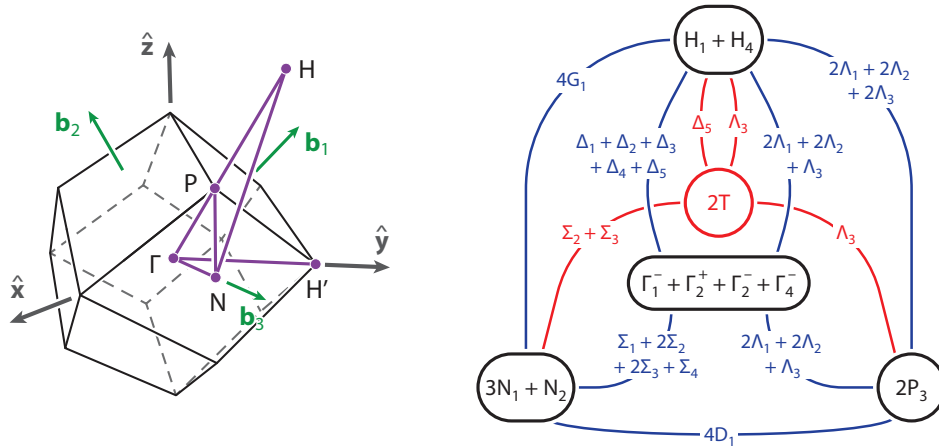

**Supplemental Figure S4.** **Left:** Brillouin zone of space group 230 (Bravais type cl). Directions of the primitive reciprocal lattice vectors,  $\mathbf{b}_1 = (2\pi/a)(\mathbf{y} + \mathbf{z})$ ,  $\mathbf{b}_2 = (2\pi/a)(\mathbf{x} + \mathbf{z})$ , and  $\mathbf{b}_3 = (2\pi/a)(\mathbf{x} + \mathbf{y})$ , are indicated in green. The considered high-symmetry  $\mathbf{k}$ -path and high-symmetry  $\mathbf{k}$ -points are indicated in purple. The high-symmetry  $\mathbf{k}$ -points are  $\Gamma = \mathbf{0}$ ,  $H = \frac{1}{2}(\mathbf{b}_1 + \mathbf{b}_2 + \mathbf{b}_3)$ ,  $P = \frac{1}{4}(\mathbf{b}_1 + \mathbf{b}_2 + \mathbf{b}_3)$ ,  $N = \frac{1}{2}\mathbf{b}_3$ , and  $H' = H - \mathbf{b}_2 = \frac{1}{2}(\mathbf{b}_1 - \mathbf{b}_2 + \mathbf{b}_3)$ . **Right:** Visualization of compatibility relations among the maximal high-symmetry  $\mathbf{k}$ -points of a  $\mu^T = 8$  solution in space group 230 with  $\mathbf{n}^T = [(\blacksquare)^{2T} + \Gamma_1^- + \Gamma_2^+ + \Gamma_2^- + \Gamma_4^-, H_1 + H_4, 2P_3, 3N_1 + N_2]^T$ , i.e., [Eq. \(S29a\)](#). The singular  $\omega = 0$   $\Gamma$ -irreps are indicated by 2T and the directly pinned line-irreps emanating from them are shown in red.

\* Although less severe, the second required  $P_3$  irrep is also located in the high bands of the empty-lattice dispersion ([Supplemental Figure S6](#)) and may be challenging to bring into the bottom 8 bands in realistic PhCs as well.

that do not require a  $\Gamma_1^\pm$  irrep, namely:

$$[(\blacksquare)^{2T} + \Gamma_2^- + \Gamma_4^+ + \Gamma_4^- + \Gamma_5^-, H_1 + H_2H_3 + H_4, P_1P_2 + 2P_3, 4N_1 + 2N_2]^T, \quad (\text{S30a})$$

$$[(\blacksquare)^{2T} + \Gamma_2^+ + \Gamma_4^+ + \Gamma_4^- + \Gamma_5^+, H_1 + H_2H_3 + H_4, P_1P_2 + 2P_3, 4N_1 + 2N_2]^T. \quad (\text{S30b})$$

As a result, these solutions are not subject to a dielectric obstruction. Indeed, by scanning a large number of PhCs in space group 230, we found that a gap was frequently opened at  $\mu^T = 12$ .

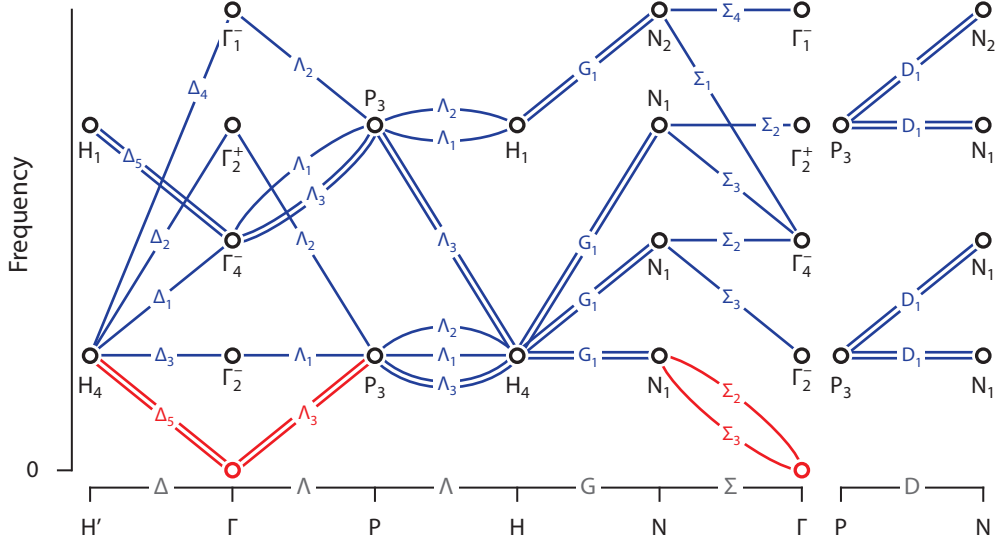

**Supplemental Figure S5.** A possible connectivity graph in frequency-space of a  $\mu^T = 8$  solution in space group 230 with  $\mathbf{n}^T = [(\blacksquare)^{2T} + \Gamma_1^- + \Gamma_2^+ + \Gamma_2^- + \Gamma_4^-, H_1 + H_4, 2P_3, 3N_1 + N_2]^T$ , i.e., Eq. (S29a). The singular  $\omega = 0$   $\Gamma$ -irreps are indicated by red nodes and the directly pinned line-irreps are similarly shown in red. The shown connectivity graph is one among many possibilities: in practice, nodes can be moved freely vertically (except to  $\omega = 0$ ) so long that the overall connectivities remains consistent with compatibility constraints.

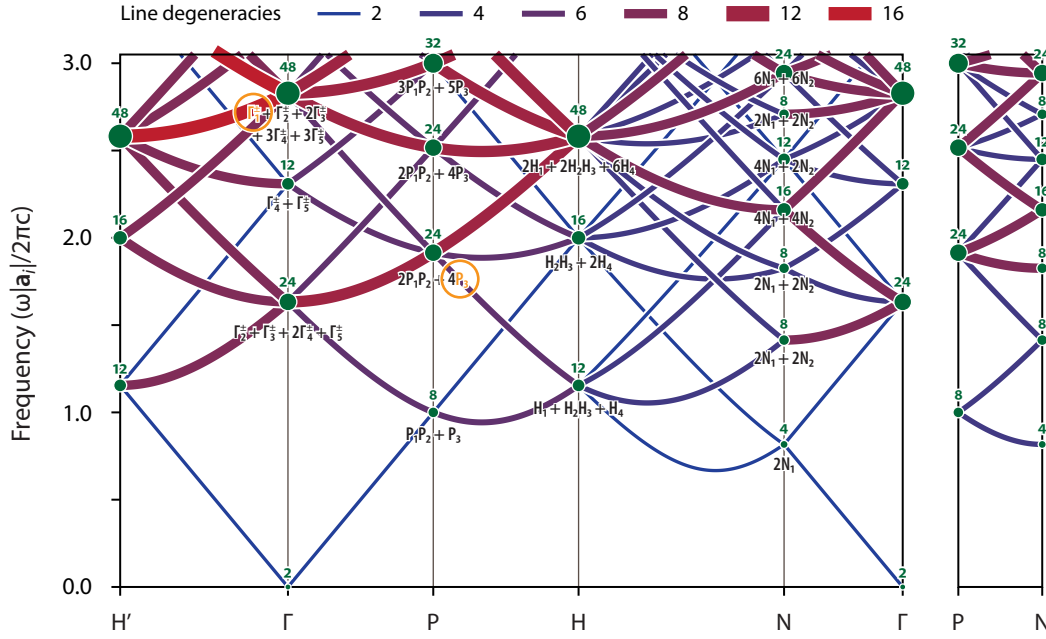

**Supplemental Figure S6. Empty-lattice dispersion and band symmetries of space group 230.** The order of line degeneracies are indicated by color and line width; the order of point degeneracies are indicated in text and by marker size. The band symmetries at high-symmetry  $\mathbf{k}$ -points are indicated by text annotations (the notation  $\Gamma_i^\pm = \sum_{\sigma=\pm} \Gamma_i^\sigma$  is used for brevity). The (first)  $\Gamma_1^\pm$  and (second)  $P_3$  irreps are highlighted in orange; they occur in high-lying bands, making it very difficult to realize the  $\mu^T = 8$  solutions with conventional dielectric materials. Frequencies are scaled by the primitive direct basis vectors  $\mathbf{a}_i$ .

## SUPPLEMENTAL REFERENCES

- [S1] J. Cano and B. Bradlyn, Band representations and topological quantum chemistry, *Annu. Rev. Condens. Matter Phys.* **12**, 225 (2021).
- [S2] H. C. Po, Symmetry indicators of band topology, *J. Phys.: Condens. Matter* **32**, 263001 (2020).
- [S3] H. Bary, L. Michel, and J. Zak, Symmetry and classification of energy bands in crystals, in *Group Theoretical Methods in Physics*, Lecture Notes in Physics (Springer, 1988) pp. 289–308.
- [S4] L. Michel and J. Zak, Connectivity of energy bands in crystals, *Phys. Rev. B* **59**, 5998 (1999).
- [S5] L. Michel and J. Zak, Elementary energy bands in crystals are connected, *Phys. Rep.* **341**, 377 (2001).
- [S6] J. Kruthoff, J. de Boer, J. van Wezel, C. L. Kane, and R.-J. Slager, Topological classification of crystalline insulators through band structure combinatorics, *Phys. Rev. X* **7**, 041069 (2017).
- [S7] H. C. Po, A. Vishwanath, and H. Watanabe, Symmetry-based indicators of band topology in the 230 space groups, *Nature Commun.* **8**, 50 (2017).
- [S8] B. Bradlyn, L. Elcoro, J. Cano, M. G. Vergniory, Z. Wang, C. Felser, M. I. Aroyo, and B. A. Bernevig, Topological quantum chemistry, *Nature* **547**, 298 (2017).
- [S9] Bilbao Crystallographic Server: BANDREP (2017).
- [S10] L. Elcoro, B. Bradlyn, Z. Wang, M. G. Vergniory, J. Cano, C. Felser, B. A. Bernevig, D. Orobengoa, G. Flor, and M. I. Aroyo, Double crystallographic groups and their representations on the Bilbao Crystallographic Server, *J. Appl. Cryst.* **50**, 1457 (2017).
- [S11] J. Cano, B. Bradlyn, Z. Wang, L. Elcoro, M. G. Vergniory, C. Felser, M. I. Aroyo, and B. A. Bernevig, Building blocks of topological quantum chemistry: Elementary band representations, *Phys. Rev. B* **97**, 035139 (2018).
- [S12] Crystalline.jl (v0.4.12), <https://github.com/thchr/Crystalline.jl>.
- [S13] W. Bruns and J. Gubeladze, *Polytopes, Rings, and K-Theory* (Springer, 2009).
- [S14] F. Tang, H. C. Po, A. Vishwanath, and X. Wan, Efficient topological materials discovery using symmetry indicators, *Nature Physics* **15**, 470 (2019).
- [S15] H. J. S. Smith, On systems of linear indeterminate equations and congruences, *Philos. Trans. Royal Soc. London* **151**, 293 (1861).
- [S16] A. Diky, SmithNormalForm.jl, <https://github.com/wildart/SmithNormalForm.jl> (2017).

- [S17] H. C. Po, H. Watanabe, and A. Vishwanath, Fragile topology and Wannier obstructions, *Phys. Rev. Lett.* **121**, 126402 (2018).
- [S18] A. Ben-Israel and T. N. E. Greville, *Generalized Inverses: Theory and Applications*, 2nd ed. (Springer, 2003).
- [S19] W. Bruns, B. Ichim, T. Römer, R. Sieg, and C. Söger, Normaliz. Algorithms for rational cones and affine monoids, <https://www.normaliz.uni-osnabrueck.de>.
- [S20] W. Bruns and B. Ichim, Normaliz: Algorithms for affine monoids and rational cones, *J. Algebra* **324**, 1098 (2010).
- [S21] W. Bruns, B. Ichim, and C. Söger, The power of pyramid decomposition in Normaliz, *J. Symb. Comp.* **74**, 513 (2016).
- [S22] R. Hemmecke, R. Hemmecke, M. Köppe, P. Malkin, and M. Walter, 4ti2—a software package for algebraic, geometric and combinatorial problems on linear spaces, <https://github.com/4ti2/4ti2>.
- [S23] Z.-D. Song, L. Elcoro, Y.-F. Xu, N. Regnault, and B. A. Bernevig, Fragile phases as affine monoids: classification and material examples, *Phys. Rev. X* **10**, 031001 (2020).
- [S24] I. Dunning, J. Huchette, and M. Lubin, JuMP: A modeling language for mathematical optimization, *SIAM Review* **59**, 295 (2017).
- [S25] GNU Linear Programming Kit (GLPK), <https://www.gnu.org/software/glpk>.
- [S26] SymmetryBases.jl (v0.3.4), <https://github.com/thchr/SymmetryBases.jl>.
- [S27] PhotonicBandConnectivity.jl (v0.2.5), <https://github.com/thchr/PhotonicBandConnectivity.jl>.
- [S28] Z. Song, T. Zhang, and C. Fang, Diagnosis for nonmagnetic topological semimetals in the absence of spin-orbital coupling, *Phys. Rev. X* **8**, 031069 (2018).
- [S29] C. Fang, M. J. Gilbert, and B. A. Bernevig, Bulk topological invariants in noninteracting point group symmetric insulators, *Phys. Rev. B* **86**, 115112 (2012).



## S8. TABLES

For each space group, we list the minimum-connectivity solutions  $\mu^T = \mu_1^T$ , as well as their topological indices  $\nu^T$  if the indicator group is nontrivial. For clarity, we indicate trivial indices, i.e.,  $\nu^T = (\nu_1^T, \dots, \nu_n^T) = (0, \dots, 0)$ , simply as “trivial.” The singular  $\Gamma$ -point symmetry content is indicated by  $(\blacksquare)^{2T}$ .

### A. Photonic minimum-connectivity solutions (with time-reversal symmetry)

Space group 1 ( $\mathbb{Z}_1$ )

1st minimal solution:  $\mu_1^T = 2$  (1 symmetry vector)

| $\mathbf{n}^T$                                                                  |
|---------------------------------------------------------------------------------|
| $[(\blacksquare)^{2T}, 2R_1^-, 2T_1^-, 2U_1^-, 2V_1^-, 2X_1^-, 2Y_1^-, 2Z_1^-]$ |

2nd minimal solution:  $\mu_2^T = 3$  (1 symmetry vector)

Space group 2 ( $\mathbb{Z}_2 \times \mathbb{Z}_2 \times \mathbb{Z}_2 \times \mathbb{Z}_4$ )

1st minimal solution:  $\mu_1^T = 2$  (2187 symmetry vectors)

| $\mathbf{n}^T$                                                                                              | $\nu^T \in \mathbb{Z}_2 \times \mathbb{Z}_2 \times \mathbb{Z}_2 \times \mathbb{Z}_4$ |
|-------------------------------------------------------------------------------------------------------------|--------------------------------------------------------------------------------------|
| $[(\blacksquare)^{2T}, 2R_1^-, 2T_1^-, 2U_1^-, 2V_1^-, 2X_1^-, 2Y_1^-, 2Z_1^-]$                             | (1, 0, 0, 1)                                                                         |
| $[(\blacksquare)^{2T}, 2R_1^-, 2T_1^-, 2U_1^-, 2V_1^-, 2X_1^-, 2Y_1^-, Z_1^+ + Z_1^-]$                      | (1, 0, 0, 2)                                                                         |
| $[(\blacksquare)^{2T}, 2R_1^-, 2T_1^-, 2U_1^-, V_1^+ + V_1^-, 2X_1^-, 2Y_1^-, 2Z_1^-]$                      | (1, 0, 1, 0)                                                                         |
| $[(\blacksquare)^{2T}, 2R_1^-, 2T_1^-, 2U_1^-, V_1^+ + V_1^-, 2X_1^-, 2Y_1^-, Z_1^+ + Z_1^-]$               | (1, 0, 1, 1)                                                                         |
| $[(\blacksquare)^{2T}, 2R_1^-, 2T_1^-, 2U_1^-, 2V_1^-, 2X_1^-, Y_1^+ + Y_1^-, 2Z_1^-]$                      | (1, 1, 0, 2)                                                                         |
| $[(\blacksquare)^{2T}, 2R_1^-, 2T_1^-, 2U_1^-, 2V_1^-, 2X_1^-, Y_1^+ + Y_1^-, Z_1^+ + Z_1^-]$               | (1, 1, 0, 3)                                                                         |
| $[(\blacksquare)^{2T}, 2R_1^-, 2T_1^-, 2U_1^-, V_1^+ + V_1^-, 2X_1^-, Y_1^+ + Y_1^-, 2Z_1^-]$               | (1, 1, 1, 1)                                                                         |
| $[(\blacksquare)^{2T}, 2R_1^-, 2T_1^-, 2U_1^-, V_1^+ + V_1^-, 2X_1^-, Y_1^+ + Y_1^-, Z_1^+ + Z_1^-]$        | (1, 1, 1, 2)                                                                         |
| $[(\blacksquare)^{2T}, 2R_1^-, 2T_1^-, 2U_1^-, 2V_1^-, X_1^+ + X_1^-, 2Y_1^-, 2Z_1^-]$                      | (0, 1, 1, 2)                                                                         |
| $[(\blacksquare)^{2T}, 2R_1^-, 2T_1^-, 2U_1^-, 2V_1^-, X_1^+ + X_1^-, 2Y_1^-, Z_1^+ + Z_1^-]$               | (0, 1, 1, 3)                                                                         |
| $[(\blacksquare)^{2T}, 2R_1^-, 2T_1^-, 2U_1^-, V_1^+ + V_1^-, X_1^+ + X_1^-, 2Y_1^-, 2Z_1^-]$               | (0, 1, 0, 1)                                                                         |
| $[(\blacksquare)^{2T}, 2R_1^-, 2T_1^-, 2U_1^-, V_1^+ + V_1^-, X_1^+ + X_1^-, 2Y_1^-, Z_1^+ + Z_1^-]$        | (0, 1, 0, 2)                                                                         |
| $[(\blacksquare)^{2T}, 2R_1^-, 2T_1^-, 2U_1^-, 2V_1^-, X_1^+ + X_1^-, Y_1^+ + Y_1^-, 2Z_1^-]$               | (0, 0, 1, 3)                                                                         |
| $[(\blacksquare)^{2T}, 2R_1^-, 2T_1^-, 2U_1^-, 2V_1^-, X_1^+ + X_1^-, Y_1^+ + Y_1^-, Z_1^+ + Z_1^-]$        | (0, 0, 1, 0)                                                                         |
| $[(\blacksquare)^{2T}, 2R_1^-, 2T_1^-, 2U_1^-, V_1^+ + V_1^-, X_1^+ + X_1^-, Y_1^+ + Y_1^-, 2Z_1^-]$        | (0, 0, 0, 2)                                                                         |
| $[(\blacksquare)^{2T}, 2R_1^-, 2T_1^-, 2U_1^-, V_1^+ + V_1^-, X_1^+ + X_1^-, Y_1^+ + Y_1^-, Z_1^+ + Z_1^-]$ | (0, 0, 0, 3)                                                                         |
| $[(\blacksquare)^{2T}, 2R_1^-, T_1^+ + T_1^-, 2U_1^-, 2V_1^-, 2X_1^-, 2Y_1^-, 2Z_1^-]$                      | (0, 1, 0, 0)                                                                         |
| $[(\blacksquare)^{2T}, 2R_1^-, T_1^+ + T_1^-, 2U_1^-, 2V_1^-, 2X_1^-, 2Y_1^-, Z_1^+ + Z_1^-]$               | (0, 1, 0, 1)                                                                         |
| $[(\blacksquare)^{2T}, 2R_1^-, T_1^+ + T_1^-, 2U_1^-, V_1^+ + V_1^-, 2X_1^-, 2Y_1^-, 2Z_1^-]$               | (0, 1, 1, 3)                                                                         |
| $[(\blacksquare)^{2T}, 2R_1^-, T_1^+ + T_1^-, 2U_1^-, V_1^+ + V_1^-, 2X_1^-, 2Y_1^-, Z_1^+ + Z_1^-]$        | (0, 1, 1, 0)                                                                         |
| $[(\blacksquare)^{2T}, 2R_1^-, T_1^+ + T_1^-, 2U_1^-, 2V_1^-, 2X_1^-, Y_1^+ + Y_1^-, 2Z_1^-]$               | (0, 0, 0, 1)                                                                         |
| $[(\blacksquare)^{2T}, 2R_1^-, T_1^+ + T_1^-, 2U_1^-, 2V_1^-, 2X_1^-, Y_1^+ + Y_1^-, Z_1^+ + Z_1^-]$        | (0, 0, 0, 2)                                                                         |
| $[(\blacksquare)^{2T}, 2R_1^-, T_1^+ + T_1^-, 2U_1^-, V_1^+ + V_1^-, 2X_1^-, Y_1^+ + Y_1^-, 2Z_1^-]$        | (0, 0, 1, 0)                                                                         |
| $[(\blacksquare)^{2T}, 2R_1^-, T_1^+ + T_1^-, 2U_1^-, V_1^+ + V_1^-, 2X_1^-, Y_1^+ + Y_1^-, Z_1^+ + Z_1^-]$ | (0, 0, 1, 1)                                                                         |
| $[(\blacksquare)^{2T}, 2R_1^-, T_1^+ + T_1^-, 2U_1^-, 2V_1^-, X_1^+ + X_1^-, 2Y_1^-, 2Z_1^-]$               | (1, 0, 1, 1)                                                                         |
| $[(\blacksquare)^{2T}, 2R_1^-, T_1^+ + T_1^-, 2U_1^-, 2V_1^-, X_1^+ + X_1^-, 2Y_1^-, Z_1^+ + Z_1^-]$        | (1, 0, 1, 2)                                                                         |
| $[(\blacksquare)^{2T}, 2R_1^-, T_1^+ + T_1^-, 2U_1^-, V_1^+ + V_1^-, X_1^+ + X_1^-, 2Y_1^-, 2Z_1^-]$        | (1, 0, 0, 0)                                                                         |

... continued on next page















... continued on next page

... continued on next page

... continued on next page



... continued on next page

... continued from previous page

|                                                                                                        |              |
|--------------------------------------------------------------------------------------------------------|--------------|
| $[(\bullet)^{2T}, R_1^+ + R_1^-, 2T_1^-, U_1^+ + U_1^-, V_1^+ + V_1^-, 2X_1^+, 2Y_1^+, 2Z_1^+]$        | (0, 1, 1, 2) |
| $[(\bullet)^{2T}, R_1^+ + R_1^-, T_1^+ + T_1^-, U_1^+ + U_1^-, 2V_1^-, 2X_1^+, 2Y_1^+, 2Z_1^+]$        | (1, 0, 0, 2) |
| $[(\bullet)^{2T}, R_1^+ + R_1^-, T_1^+ + T_1^-, U_1^+ + U_1^-, V_1^+ + V_1^-, 2X_1^+, 2Y_1^+, 2Z_1^+]$ | (1, 0, 1, 1) |
| $[(\bullet)^{2T}, 2R_1^-, 2T_1^-, 2U_1^-, 2V_1^+, 2X_1^+, 2Y_1^+, 2Z_1^-]$                             | (1, 0, 0, 3) |
| $[(\bullet)^{2T}, 2R_1^-, 2T_1^-, 2U_1^-, 2V_1^+, 2X_1^+, 2Y_1^+, Z_1^+ + Z_1^-]$                      | (1, 0, 0, 0) |
| $[(\bullet)^{2T}, 2R_1^-, T_1^+ + T_1^-, 2U_1^-, 2V_1^+, 2X_1^+, 2Y_1^+, 2Z_1^-]$                      | (0, 1, 0, 2) |
| $[(\bullet)^{2T}, 2R_1^-, T_1^+ + T_1^-, 2U_1^-, 2V_1^+, 2X_1^+, 2Y_1^+, Z_1^+ + Z_1^-]$               | (0, 1, 0, 3) |
| $[(\bullet)^{2T}, 2R_1^-, 2T_1^-, U_1^+ + U_1^-, 2V_1^+, 2X_1^+, 2Y_1^+, 2Z_1^-]$                      | (1, 1, 1, 2) |
| $[(\bullet)^{2T}, 2R_1^-, 2T_1^-, U_1^+ + U_1^-, 2V_1^+, 2X_1^+, 2Y_1^+, Z_1^+ + Z_1^-]$               | (1, 1, 1, 3) |
| $[(\bullet)^{2T}, 2R_1^-, T_1^+ + T_1^-, U_1^+ + U_1^-, 2V_1^+, 2X_1^+, 2Y_1^+, 2Z_1^-]$               | (0, 0, 1, 1) |
| $[(\bullet)^{2T}, 2R_1^-, T_1^+ + T_1^-, U_1^+ + U_1^-, 2V_1^+, 2X_1^+, 2Y_1^+, Z_1^+ + Z_1^-]$        | (0, 0, 1, 2) |
| $[(\bullet)^{2T}, R_1^+ + R_1^-, 2T_1^-, 2U_1^-, 2V_1^+, 2X_1^+, 2Y_1^+, 2Z_1^-]$                      | (0, 0, 1, 0) |
| $[(\bullet)^{2T}, R_1^+ + R_1^-, 2T_1^-, 2U_1^-, 2V_1^+, 2X_1^+, 2Y_1^+, Z_1^+ + Z_1^-]$               | (0, 0, 1, 1) |
| $[(\bullet)^{2T}, R_1^+ + R_1^-, T_1^+ + T_1^-, 2U_1^-, 2V_1^+, 2X_1^+, 2Y_1^+, 2Z_1^-]$               | (1, 1, 1, 3) |
| $[(\bullet)^{2T}, R_1^+ + R_1^-, T_1^+ + T_1^-, 2U_1^-, 2V_1^+, 2X_1^+, 2Y_1^+, Z_1^+ + Z_1^-]$        | (1, 1, 1, 0) |
| $[(\bullet)^{2T}, R_1^+ + R_1^-, 2T_1^-, U_1^+ + U_1^-, 2V_1^+, 2X_1^+, 2Y_1^+, 2Z_1^-]$               | (0, 1, 0, 3) |
| $[(\bullet)^{2T}, R_1^+ + R_1^-, 2T_1^-, U_1^+ + U_1^-, 2V_1^+, 2X_1^+, 2Y_1^+, Z_1^+ + Z_1^-]$        | (0, 1, 0, 0) |
| $[(\bullet)^{2T}, R_1^+ + R_1^-, T_1^+ + T_1^-, U_1^+ + U_1^-, 2V_1^+, 2X_1^+, 2Y_1^+, 2Z_1^-]$        | (1, 0, 0, 2) |
| $[(\bullet)^{2T}, R_1^+ + R_1^-, T_1^+ + T_1^-, U_1^+ + U_1^-, 2V_1^+, 2X_1^+, 2Y_1^+, Z_1^+ + Z_1^-]$ | (1, 0, 0, 3) |
| $[(\bullet)^{2T}, 2R_1^-, 2T_1^-, 2U_1^-, 2V_1^+, 2X_1^+, 2Y_1^+, 2Z_1^+]$                             | (1, 0, 0, 1) |
| $[(\bullet)^{2T}, 2R_1^-, T_1^+ + T_1^-, 2U_1^-, 2V_1^+, 2X_1^+, 2Y_1^+, 2Z_1^+]$                      | (0, 1, 0, 0) |
| $[(\bullet)^{2T}, 2R_1^-, 2T_1^-, U_1^+ + U_1^-, 2V_1^+, 2X_1^+, 2Y_1^+, 2Z_1^+]$                      | (1, 1, 1, 0) |
| $[(\bullet)^{2T}, 2R_1^-, T_1^+ + T_1^-, U_1^+ + U_1^-, 2V_1^+, 2X_1^+, 2Y_1^+, 2Z_1^+]$               | (0, 0, 1, 3) |
| $[(\bullet)^{2T}, R_1^+ + R_1^-, 2T_1^-, 2U_1^-, 2V_1^+, 2X_1^+, 2Y_1^+, 2Z_1^+]$                      | (0, 0, 1, 2) |
| $[(\bullet)^{2T}, R_1^+ + R_1^-, T_1^+ + T_1^-, 2U_1^-, 2V_1^+, 2X_1^+, 2Y_1^+, 2Z_1^+]$               | (1, 1, 1, 1) |
| $[(\bullet)^{2T}, R_1^+ + R_1^-, 2T_1^-, U_1^+ + U_1^-, 2V_1^+, 2X_1^+, 2Y_1^+, 2Z_1^+]$               | (0, 1, 0, 1) |
| $[(\bullet)^{2T}, R_1^+ + R_1^-, T_1^+ + T_1^-, U_1^+ + U_1^-, 2V_1^+, 2X_1^+, 2Y_1^+, 2Z_1^+]$        | (1, 0, 0, 0) |
| $[(\bullet)^{2T}, 2R_1^-, 2T_1^+, 2U_1^-, 2V_1^-, 2X_1^-, 2Y_1^-, 2Z_1^-]$                             | (1, 0, 0, 3) |
| $[(\bullet)^{2T}, 2R_1^-, 2T_1^+, 2U_1^-, 2V_1^-, 2X_1^-, 2Y_1^-, Z_1^+ + Z_1^-]$                      | (1, 0, 0, 0) |
| $[(\bullet)^{2T}, 2R_1^-, 2T_1^+, 2U_1^-, V_1^+ + V_1^-, 2X_1^-, 2Y_1^-, 2Z_1^-]$                      | (1, 0, 1, 2) |
| $[(\bullet)^{2T}, 2R_1^-, 2T_1^+, 2U_1^-, V_1^+ + V_1^-, 2X_1^-, 2Y_1^-, Z_1^+ + Z_1^-]$               | (1, 0, 1, 3) |
| $[(\bullet)^{2T}, 2R_1^-, 2T_1^+, 2U_1^-, 2V_1^-, 2X_1^-, Y_1^+ + Y_1^-, 2Z_1^-]$                      | (1, 1, 0, 0) |
| $[(\bullet)^{2T}, 2R_1^-, 2T_1^+, 2U_1^-, 2V_1^-, 2X_1^-, Y_1^+ + Y_1^-, Z_1^+ + Z_1^-]$               | (1, 1, 0, 1) |
| $[(\bullet)^{2T}, 2R_1^-, 2T_1^+, 2U_1^-, V_1^+ + V_1^-, 2X_1^-, Y_1^+ + Y_1^-, 2Z_1^-]$               | (1, 1, 1, 3) |
| $[(\bullet)^{2T}, 2R_1^-, 2T_1^+, 2U_1^-, V_1^+ + V_1^-, 2X_1^-, Y_1^+ + Y_1^-, Z_1^+ + Z_1^-]$        | (1, 1, 1, 0) |
| $[(\bullet)^{2T}, 2R_1^-, 2T_1^+, 2U_1^-, 2V_1^-, X_1^+ + X_1^-, 2Y_1^-, 2Z_1^-]$                      | (0, 1, 1, 0) |
| $[(\bullet)^{2T}, 2R_1^-, 2T_1^+, 2U_1^-, 2V_1^-, X_1^+ + X_1^-, 2Y_1^-, Z_1^+ + Z_1^-]$               | (0, 1, 1, 1) |
| $[(\bullet)^{2T}, 2R_1^-, 2T_1^+, 2U_1^-, V_1^+ + V_1^-, X_1^+ + X_1^-, 2Y_1^-, 2Z_1^-]$               | (0, 1, 0, 3) |
| $[(\bullet)^{2T}, 2R_1^-, 2T_1^+, 2U_1^-, V_1^+ + V_1^-, X_1^+ + X_1^-, 2Y_1^-, Z_1^+ + Z_1^-]$        | (0, 1, 0, 0) |
| $[(\bullet)^{2T}, 2R_1^-, 2T_1^+, 2U_1^-, 2V_1^-, X_1^+ + X_1^-, Y_1^+ + Y_1^-, 2Z_1^-]$               | (0, 0, 1, 1) |
| $[(\bullet)^{2T}, 2R_1^-, 2T_1^+, 2U_1^-, 2V_1^-, X_1^+ + X_1^-, Y_1^+ + Y_1^-, Z_1^+ + Z_1^-]$        | (0, 0, 1, 2) |
| $[(\bullet)^{2T}, 2R_1^-, 2T_1^+, 2U_1^-, V_1^+ + V_1^-, X_1^+ + X_1^-, Y_1^+ + Y_1^-, 2Z_1^-]$        | trivial      |
| $[(\bullet)^{2T}, 2R_1^-, 2T_1^+, 2U_1^-, V_1^+ + V_1^-, X_1^+ + X_1^-, Y_1^+ + Y_1^-, Z_1^+ + Z_1^-]$ | (0, 0, 0, 1) |
| $[(\bullet)^{2T}, 2R_1^-, 2T_1^+, U_1^+ + U_1^-, 2V_1^-, 2X_1^-, 2Y_1^-, 2Z_1^-]$                      | (1, 1, 1, 2) |
| $[(\bullet)^{2T}, 2R_1^-, 2T_1^+, U_1^+ + U_1^-, 2V_1^-, 2X_1^-, 2Y_1^-, Z_1^+ + Z_1^-]$               | (1, 1, 1, 3) |
| $[(\bullet)^{2T}, 2R_1^-, 2T_1^+, U_1^+ + U_1^-, V_1^+ + V_1^-, 2X_1^-, 2Y_1^-, 2Z_1^-]$               | (1, 1, 0, 1) |
| $[(\bullet)^{2T}, 2R_1^-, 2T_1^+, U_1^+ + U_1^-, V_1^+ + V_1^-, 2X_1^-, 2Y_1^-, Z_1^+ + Z_1^-]$        | (1, 1, 0, 2) |
| $[(\bullet)^{2T}, 2R_1^-, 2T_1^+, U_1^+ + U_1^-, 2V_1^-, 2X_1^-, Y_1^+ + Y_1^-, 2Z_1^-]$               | (1, 0, 1, 3) |
| $[(\bullet)^{2T}, 2R_1^-, 2T_1^+, U_1^+ + U_1^-, 2V_1^-, 2X_1^-, Y_1^+ + Y_1^-, Z_1^+ + Z_1^-]$        | (1, 0, 1, 0) |
| $[(\bullet)^{2T}, 2R_1^-, 2T_1^+, U_1^+ + U_1^-, V_1^+ + V_1^-, 2X_1^-, Y_1^+ + Y_1^-, 2Z_1^-]$        | (1, 0, 0, 2) |
| $[(\bullet)^{2T}, 2R_1^-, 2T_1^+, U_1^+ + U_1^-, V_1^+ + V_1^-, 2X_1^-, Y_1^+ + Y_1^-, Z_1^+ + Z_1^-]$ | (1, 0, 0, 3) |
| $[(\bullet)^{2T}, 2R_1^-, 2T_1^+, U_1^+ + U_1^-, 2V_1^-, X_1^+ + X_1^-, 2Y_1^-, 2Z_1^-]$               | (0, 0, 0, 3) |
| $[(\bullet)^{2T}, 2R_1^-, 2T_1^+, U_1^+ + U_1^-, 2V_1^-, X_1^+ + X_1^-, 2Y_1^-, Z_1^+ + Z_1^-]$        | trivial      |
| $[(\bullet)^{2T}, 2R_1^-, 2T_1^+, U_1^+ + U_1^-, V_1^+ + V_1^-, X_1^+ + X_1^-, 2Y_1^-, 2Z_1^-]$        | (0, 0, 1, 2) |

... continued on next page

... continued on next page



... continued on next page

... continued on next page

... continued on next page

... continued on next page



... continued on next page



... continued on next page



... continued on next page





... continued on next page

























... continued on next page



... continued on next page

... continued on next page



... continued from previous page

$$[(\blacksquare)^{2T}, 2R_1^+, 2T_1^+, 2U_1^+, 2V_1^+, 2X_1^+, 2Y_1^+, 2Z_1^+] \quad (1, 0, 0, 3)$$

Skipped higher-order solutions...

Space group 3 ( $\mathbb{Z}_2$ )

1st minimal solution:  $\mu_1^T = 2$  (27 symmetry vectors)

| $\mathbf{n}^T$                                                                                  | $\mathbf{v}^T \in \mathbb{Z}_2$ |
|-------------------------------------------------------------------------------------------------|---------------------------------|
| $[(\blacksquare)^{2T}, 2A_2, 2B_1, 2C_2, 2D_1, 2E_2, 2Y_2, 2Z_2]$                               | trivial                         |
| $[(\blacksquare)^{2T}, 2A_2, B_1 + B_2, 2C_2, D_1 + D_2, 2E_2, 2Y_2, 2Z_2]$                     | 1                               |
| $[(\blacksquare)^{2T}, 2A_2, 2B_1, C_1 + C_2, 2D_1, 2E_2, Y_1 + Y_2, 2Z_2]$                     | 1                               |
| $[(\blacksquare)^{2T}, 2A_2, B_1 + B_2, C_1 + C_2, D_1 + D_2, 2E_2, Y_1 + Y_2, 2Z_2]$           | trivial                         |
| $[(\blacksquare)^{2T}, A_1 + A_2, 2B_1, 2C_2, 2D_1, E_1 + E_2, 2Y_2, 2Z_2]$                     | 1                               |
| $[(\blacksquare)^{2T}, A_1 + A_2, B_1 + B_2, 2C_2, D_1 + D_2, E_1 + E_2, 2Y_2, 2Z_2]$           | trivial                         |
| $[(\blacksquare)^{2T}, A_1 + A_2, 2B_1, C_1 + C_2, 2D_1, E_1 + E_2, Y_1 + Y_2, 2Z_2]$           | trivial                         |
| $[(\blacksquare)^{2T}, A_1 + A_2, B_1 + B_2, C_1 + C_2, D_1 + D_2, E_1 + E_2, Y_1 + Y_2, 2Z_2]$ | 1                               |
| $[(\blacksquare)^{2T}, 2A_2, 2B_2, 2C_2, 2D_2, 2E_2, 2Y_2, 2Z_2]$                               | trivial                         |
| $[(\blacksquare)^{2T}, 2A_2, 2B_2, C_1 + C_2, 2D_2, 2E_2, Y_1 + Y_2, 2Z_2]$                     | 1                               |
| $[(\blacksquare)^{2T}, A_1 + A_2, 2B_2, 2C_2, 2D_2, E_1 + E_2, 2Y_2, 2Z_2]$                     | 1                               |
| $[(\blacksquare)^{2T}, A_1 + A_2, 2B_2, C_1 + C_2, 2D_2, E_1 + E_2, Y_1 + Y_2, 2Z_2]$           | trivial                         |
| $[(\blacksquare)^{2T}, 2A_2, 2B_1, 2C_1, 2D_1, 2E_2, 2Y_1, 2Z_2]$                               | trivial                         |
| $[(\blacksquare)^{2T}, 2A_2, B_1 + B_2, 2C_1, D_1 + D_2, 2E_2, 2Y_1, 2Z_2]$                     | 1                               |
| $[(\blacksquare)^{2T}, A_1 + A_2, 2B_1, 2C_1, 2D_1, E_1 + E_2, 2Y_1, 2Z_2]$                     | 1                               |
| $[(\blacksquare)^{2T}, A_1 + A_2, B_1 + B_2, 2C_1, D_1 + D_2, E_1 + E_2, 2Y_1, 2Z_2]$           | trivial                         |
| $[(\blacksquare)^{2T}, 2A_2, 2B_2, 2C_1, 2D_2, 2E_2, 2Y_1, 2Z_2]$                               | trivial                         |
| $[(\blacksquare)^{2T}, A_1 + A_2, 2B_2, 2C_1, 2D_2, E_1 + E_2, 2Y_1, 2Z_2]$                     | 1                               |
| $[(\blacksquare)^{2T}, 2A_1, 2B_1, 2C_2, 2D_1, 2E_1, 2Y_2, 2Z_2]$                               | trivial                         |
| $[(\blacksquare)^{2T}, 2A_1, B_1 + B_2, 2C_2, D_1 + D_2, 2E_1, 2Y_2, 2Z_2]$                     | 1                               |
| $[(\blacksquare)^{2T}, 2A_1, 2B_1, C_1 + C_2, 2D_1, 2E_1, Y_1 + Y_2, 2Z_2]$                     | 1                               |
| $[(\blacksquare)^{2T}, 2A_1, B_1 + B_2, C_1 + C_2, D_1 + D_2, 2E_1, Y_1 + Y_2, 2Z_2]$           | trivial                         |
| $[(\blacksquare)^{2T}, 2A_1, 2B_2, 2C_2, 2D_2, 2E_1, 2Y_2, 2Z_2]$                               | trivial                         |
| $[(\blacksquare)^{2T}, 2A_1, 2B_2, C_1 + C_2, 2D_2, 2E_1, Y_1 + Y_2, 2Z_2]$                     | 1                               |
| $[(\blacksquare)^{2T}, 2A_1, 2B_1, 2C_1, 2D_1, 2E_1, 2Y_1, 2Z_2]$                               | trivial                         |
| $[(\blacksquare)^{2T}, 2A_1, B_1 + B_2, 2C_1, D_1 + D_2, 2E_1, 2Y_1, 2Z_2]$                     | 1                               |
| $[(\blacksquare)^{2T}, 2A_1, 2B_2, 2C_1, 2D_2, 2E_1, 2Y_1, 2Z_2]$                               | trivial                         |

2nd minimal solution:  $\mu_2^T = 3$  (128 symmetry vectors)

Space group 4 ( $\mathbb{Z}_1$ )

1st minimal solution:  $\mu_1^T = 4$  (1 symmetry vector)

| $\mathbf{n}^T$                                                                                                 |
|----------------------------------------------------------------------------------------------------------------|
| $[(\blacksquare)^{2T} + 2\Gamma_1, 2A_1 + 2A_2, 2B_1 + 2B_2, 2C_1C_2, 2D_1D_2, 2E_1E_2, 2Y_1 + 2Y_2, 2Z_1Z_2]$ |

2nd minimal solution:  $\mu_2^T = 6$  (1 symmetry vector)

Space group 5 ( $\mathbb{Z}_1$ )

1st minimal solution:  $\mu_1^T = 2$  (3 symmetry vectors)

| $\mathbf{n}^T$                                                  |
|-----------------------------------------------------------------|
| $[(\blacksquare)^{2T}, 2A_2, 2M_2, 2Y_2, 2L_1, 2V_1]$           |
| $[(\blacksquare)^{2T}, A_1 + A_2, M_1 + M_2, 2Y_2, 2L_1, 2V_1]$ |
| $[(\blacksquare)^{2T}, 2A_1, 2M_1, 2Y_2, 2L_1, 2V_1]$           |

2nd minimal solution:  $\mu_2^T = 3$  (8 symmetry vectors)

Space group 6 ( $\mathbb{Z}_1$ )

1st minimal solution:  $\mu_1^T = 2$  (3 symmetry vectors)

| $\mathbf{n}^T$                                                                                       |
|------------------------------------------------------------------------------------------------------|
| $[(\blacksquare)^{2T}, A_1 + A_2, B_1 + B_2, 2C_2, 2D_2, 2E_2, Y_1 + Y_2, 2Z_2]$                     |
| $[(\blacksquare)^{2T}, A_1 + A_2, B_1 + B_2, C_1 + C_2, D_1 + D_2, E_1 + E_2, Y_1 + Y_2, Z_1 + Z_2]$ |
| $[(\blacksquare)^{2T}, A_1 + A_2, B_1 + B_2, 2C_1, 2D_1, 2E_1, Y_1 + Y_2, 2Z_1]$                     |

2nd minimal solution:  $\mu_2^T = 3$  (8 symmetry vectors)

Space group 7 ( $\mathbb{Z}_1$ )

1st minimal solution:  $\mu_1^T = 2$  (1 symmetry vector)

| $\mathbf{n}^T$                                                                           |
|------------------------------------------------------------------------------------------|
| $[(\blacksquare)^{2T}, A_1A_2, B_1B_2, C_1 + C_2, D_1D_2, E_1E_2, Y_1 + Y_2, Z_1 + Z_2]$ |

2nd minimal solution:  $\mu_2^T = 4$  (1 symmetry vector)

Space group 8 ( $\mathbb{Z}_1$ )

1st minimal solution:  $\mu_1^T = 2$  (1 symmetry vector)

| $\mathbf{n}^T$                                                       |
|----------------------------------------------------------------------|
| $[(\blacksquare)^{2T}, A_1 + A_2, M_1 + M_2, Y_1 + Y_2, 2L_1, 2V_1]$ |

2nd minimal solution:  $\mu_2^T = 3$  (2 symmetry vectors)

Space group 9 ( $\mathbb{Z}_1$ )

1st minimal solution:  $\mu_1^T = 2$  (1 symmetry vector)

| $\mathbf{n}^T$                                              |
|-------------------------------------------------------------|
| $[(\bullet)^{2T}, A_1 A_2, M_1 M_2, Y_1 + Y_2, 2L_1, 2V_1]$ |

2nd minimal solution:  $\mu_2^T = 4$  (1 symmetry vector)

Space group 10 ( $\mathbb{Z}_2 \times \mathbb{Z}_2 \times \mathbb{Z}_2$ )

1st minimal solution:  $\mu_1^T = 2$  (344 symmetry vectors)

| $\mathbf{n}^T$                                                                                                              | $\mathbf{v}^T \in \mathbb{Z}_2 \times \mathbb{Z}_2 \times \mathbb{Z}_2$ |
|-----------------------------------------------------------------------------------------------------------------------------|-------------------------------------------------------------------------|
| $[(\bullet)^{2T}, A_2^+ + A_2^-, B_1^+ + B_1^-, 2C_2^-, 2D_1^+, 2E_2^-, Y_2^+ + Y_2^-, 2Z_2^-]$                             | trivial                                                                 |
| $[(\bullet)^{2T}, A_2^+ + A_2^-, B_1^+ + B_2^-, 2C_2^-, D_1^+ + D_2^-, 2E_2^-, Y_2^+ + Y_2^-, 2Z_2^-]$                      | (0, 1, 1)                                                               |
| $[(\bullet)^{2T}, A_2^+ + A_2^-, B_1^+ + B_1^-, C_1^+ + C_2^-, 2D_1^+, 2E_2^-, Y_1^- + Y_2^-, 2Z_2^-]$                      | (0, 1, 1)                                                               |
| $[(\bullet)^{2T}, A_2^+ + A_2^-, B_1^+ + B_2^-, C_1^+ + C_2^-, D_1^+ + D_2^-, 2E_2^-, Y_1^- + Y_2^-, 2Z_2^-]$               | trivial                                                                 |
| $[(\bullet)^{2T}, A_1^- + A_2^-, B_1^+ + B_1^-, 2C_2^-, 2D_1^+, E_1^+ + E_2^-, Y_2^+ + Y_2^-, 2Z_2^-]$                      | (0, 1, 1)                                                               |
| $[(\bullet)^{2T}, A_1^- + A_2^-, B_1^+ + B_2^-, 2C_2^-, D_1^+ + D_2^-, E_1^+ + E_2^-, Y_2^+ + Y_2^-, 2Z_2^-]$               | trivial                                                                 |
| $[(\bullet)^{2T}, A_1^- + A_2^-, B_1^+ + B_1^-, C_1^+ + C_2^-, 2D_1^+, E_1^+ + E_2^-, Y_1^- + Y_2^-, 2Z_2^-]$               | trivial                                                                 |
| $[(\bullet)^{2T}, A_1^- + A_2^-, B_1^+ + B_2^-, C_1^+ + C_2^-, D_1^+ + D_2^-, E_1^+ + E_2^-, Y_1^- + Y_2^-, 2Z_2^-]$        | (0, 1, 1)                                                               |
| $[(\bullet)^{2T}, A_2^+ + A_2^-, B_1^- + B_2^-, 2C_2^-, D_1^+ + D_2^-, 2E_2^-, Y_2^+ + Y_2^-, 2Z_2^-]$                      | (1, 0, 0)                                                               |
| $[(\bullet)^{2T}, A_2^+ + A_2^-, B_2^+ + B_2^-, 2C_2^-, 2D_2^-, 2E_2^-, Y_2^+ + Y_2^-, 2Z_2^-]$                             | (1, 1, 1)                                                               |
| $[(\bullet)^{2T}, A_2^+ + A_2^-, B_1^- + B_2^-, C_1^+ + C_2^-, D_1^+ + D_2^-, 2E_2^-, Y_1^- + Y_2^-, 2Z_2^-]$               | (1, 1, 1)                                                               |
| $[(\bullet)^{2T}, A_2^+ + A_2^-, B_2^+ + B_2^-, C_1^+ + C_2^-, 2D_2^-, 2E_2^-, Y_1^- + Y_2^-, 2Z_2^-]$                      | (1, 0, 0)                                                               |
| $[(\bullet)^{2T}, A_1^- + A_2^-, B_1^- + B_2^-, 2C_2^-, D_1^+ + D_2^-, E_1^+ + E_2^-, Y_2^+ + Y_2^-, 2Z_2^-]$               | (1, 1, 1)                                                               |
| $[(\bullet)^{2T}, A_1^- + A_2^-, B_2^+ + B_2^-, 2C_2^-, 2D_2^-, E_1^+ + E_2^-, Y_2^+ + Y_2^-, 2Z_2^-]$                      | (1, 0, 0)                                                               |
| $[(\bullet)^{2T}, A_1^- + A_2^-, B_1^- + B_2^-, C_1^+ + C_2^-, D_1^+ + D_2^-, E_1^+ + E_2^-, Y_1^- + Y_2^-, 2Z_2^-]$        | (1, 0, 0)                                                               |
| $[(\bullet)^{2T}, A_1^- + A_2^-, B_2^+ + B_2^-, C_1^+ + C_2^-, 2D_2^-, E_1^+ + E_2^-, Y_1^- + Y_2^-, 2Z_2^-]$               | (1, 1, 1)                                                               |
| $[(\bullet)^{2T}, A_2^+ + A_2^-, B_1^+ + B_1^-, C_1^+ + C_2^-, 2D_1^+, 2E_2^-, Y_1^+ + Y_2^+, 2Z_2^-]$                      | (1, 0, 0)                                                               |
| $[(\bullet)^{2T}, A_2^+ + A_2^-, B_1^+ + B_2^-, C_1^+ + C_2^-, D_1^+ + D_2^-, 2E_2^-, Y_1^+ + Y_2^+, 2Z_2^-]$               | (1, 1, 1)                                                               |
| $[(\bullet)^{2T}, A_2^+ + A_2^-, B_1^+ + B_1^-, 2C_1^+, 2D_1^+, 2E_2^-, Y_1^+ + Y_2^+, 2Z_2^-]$                             | (1, 1, 1)                                                               |
| $[(\bullet)^{2T}, A_2^+ + A_2^-, B_1^+ + B_2^-, 2C_1^+, D_1^+ + D_2^-, 2E_2^-, Y_1^+ + Y_2^+, 2Z_2^-]$                      | (1, 0, 0)                                                               |
| $[(\bullet)^{2T}, A_1^- + A_2^-, B_1^+ + B_1^-, C_1^+ + C_2^-, 2D_1^+, E_1^+ + E_2^-, Y_1^+ + Y_2^+, 2Z_2^-]$               | (1, 1, 1)                                                               |
| $[(\bullet)^{2T}, A_1^- + A_2^-, B_1^+ + B_2^-, C_1^+ + C_2^-, D_1^+ + D_2^-, E_1^+ + E_2^-, Y_1^+ + Y_2^+, 2Z_2^-]$        | (1, 0, 0)                                                               |
| $[(\bullet)^{2T}, A_1^- + A_2^-, B_1^+ + B_1^-, 2C_1^+, 2D_1^+, E_1^+ + E_2^-, Y_1^+ + Y_2^+, 2Z_2^-]$                      | (1, 0, 0)                                                               |
| $[(\bullet)^{2T}, A_1^- + A_2^-, B_1^+ + B_2^-, 2C_1^+, D_1^+ + D_2^-, E_1^+ + E_2^-, Y_1^+ + Y_2^+, 2Z_2^-]$               | (1, 1, 1)                                                               |
| $[(\bullet)^{2T}, A_2^+ + A_2^-, B_1^- + B_2^-, C_1^+ + C_2^-, D_1^+ + D_2^-, 2E_2^-, Y_1^+ + Y_2^+, 2Z_2^-]$               | trivial                                                                 |
| $[(\bullet)^{2T}, A_2^+ + A_2^-, B_2^+ + B_2^-, C_1^+ + C_2^-, 2D_2^-, 2E_2^-, Y_1^+ + Y_2^+, 2Z_2^-]$                      | (0, 1, 1)                                                               |
| $[(\bullet)^{2T}, A_2^+ + A_2^-, B_1^- + B_2^-, 2C_1^+, D_1^+ + D_2^-, 2E_2^-, Y_1^+ + Y_2^+, 2Z_2^-]$                      | (0, 1, 1)                                                               |
| $[(\bullet)^{2T}, A_2^+ + A_2^-, B_2^+ + B_2^-, 2C_1^+, 2D_2^-, 2E_2^-, Y_1^+ + Y_2^+, 2Z_2^-]$                             | trivial                                                                 |
| $[(\bullet)^{2T}, A_1^- + A_2^-, B_1^- + B_2^-, C_1^+ + C_2^-, D_1^+ + D_2^-, E_1^+ + E_2^-, Y_1^+ + Y_2^+, 2Z_2^-]$        | (0, 1, 1)                                                               |
| $[(\bullet)^{2T}, A_1^- + A_2^-, B_2^+ + B_2^-, C_1^+ + C_2^-, 2D_2^-, E_1^+ + E_2^-, Y_1^+ + Y_2^+, 2Z_2^-]$               | trivial                                                                 |
| $[(\bullet)^{2T}, A_1^- + A_2^-, B_1^- + B_2^-, 2C_1^+, D_1^+ + D_2^-, E_1^+ + E_2^-, Y_1^+ + Y_2^+, 2Z_2^-]$               | trivial                                                                 |
| $[(\bullet)^{2T}, A_1^- + A_2^-, B_2^+ + B_2^-, 2C_1^+, 2D_2^-, E_1^+ + E_2^-, Y_1^+ + Y_2^+, 2Z_2^-]$                      | (0, 1, 1)                                                               |
| $[(\bullet)^{2T}, A_2^+ + A_2^-, B_1^+ + B_1^-, C_2^+ + C_2^-, D_1^+ + D_1^-, E_2^+ + E_2^-, Y_2^+ + Y_2^-, Z_2^+ + Z_2^-]$ | (0, 0, 1)                                                               |
| $[(\bullet)^{2T}, A_2^+ + A_2^-, B_1^+ + B_2^-, C_2^+ + C_2^-, D_1^+ + D_2^-, E_2^+ + E_2^-, Y_2^+ + Y_2^-, Z_2^+ + Z_2^-]$ | (0, 1, 0)                                                               |
| $[(\bullet)^{2T}, A_2^+ + A_2^-, B_1^+ + B_1^-, C_1^+ + C_2^-, D_1^+ + D_1^-, E_2^+ + E_2^-, Y_1^- + Y_2^-, Z_2^+ + Z_2^-]$ | (0, 1, 0)                                                               |
| $[(\bullet)^{2T}, A_2^+ + A_2^-, B_1^+ + B_2^-, C_1^+ + C_2^-, D_1^+ + D_2^-, E_2^+ + E_2^-, Y_1^- + Y_2^-, Z_2^+ + Z_2^-]$ | (0, 0, 1)                                                               |
| $[(\bullet)^{2T}, A_1^- + A_2^-, B_1^+ + B_1^-, C_2^+ + C_2^-, D_1^+ + D_1^-, E_1^+ + E_2^+, Y_2^+ + Y_2^-, Z_2^+ + Z_2^-]$ | (0, 1, 0)                                                               |

... continued on next page

... continued on next page





... continued on next page





... continued from previous page

|                                                                                                               |           |
|---------------------------------------------------------------------------------------------------------------|-----------|
| $[(\bullet)^{2T}, A_2^+ + A_2^-, B_2^+ + B_2^-, 2C_2^+, 2D_2^+, 2E_2^+, Y_2^+ + Y_2^-, 2Z_2^+]$               | (1, 1, 1) |
| $[(\bullet)^{2T}, A_2^+ + A_2^-, B_2^+ + B_2^-, C_1^- + C_2^+, 2D_2^+, 2E_2^+, Y_1^- + Y_2^-, 2Z_2^+]$        | (1, 0, 1) |
| $[(\bullet)^{2T}, A_2^+ + A_2^-, B_2^+ + B_2^-, C_1^- + C_2^+, 2D_2^+, 2E_2^+, Y_1^+ + Y_2^+, 2Z_2^+]$        | (0, 1, 0) |
| $[(\bullet)^{2T}, A_1^- + A_2^-, B_2^+ + B_2^-, 2C_2^+, 2D_2^+, E_1^- + E_2^+, Y_2^+ + Y_2^-, 2Z_2^+]$        | (1, 0, 1) |
| $[(\bullet)^{2T}, A_1^- + A_2^-, B_2^+ + B_2^-, C_1^- + C_2^+, 2D_2^+, E_1^- + E_2^+, Y_1^- + Y_2^-, 2Z_2^+]$ | (1, 1, 1) |
| $[(\bullet)^{2T}, A_1^- + A_2^-, B_2^+ + B_2^-, C_1^- + C_2^+, 2D_2^+, E_1^- + E_2^+, Y_1^+ + Y_2^+, 2Z_2^+]$ | trivial   |
| $[(\bullet)^{2T}, A_1^+ + A_2^+, B_2^+ + B_2^-, 2C_2^+, 2D_2^+, E_1^- + E_2^+, Y_2^+ + Y_2^-, 2Z_2^+]$        | (0, 1, 0) |
| $[(\bullet)^{2T}, A_1^+ + A_2^+, B_2^+ + B_2^-, C_1^- + C_2^+, 2D_2^+, E_1^- + E_2^+, Y_1^- + Y_2^-, 2Z_2^+]$ | trivial   |
| $[(\bullet)^{2T}, A_1^+ + A_2^+, B_2^+ + B_2^-, C_1^- + C_2^+, 2D_2^+, E_1^- + E_2^+, Y_1^+ + Y_2^+, 2Z_2^+]$ | (1, 1, 1) |
| $[(\bullet)^{2T}, A_2^+ + A_2^-, B_1^+ + B_1^-, 2C_1^-, 2D_1^-, 2E_2^+, Y_1^+ + Y_1^-, 2Z_2^+]$               | (1, 1, 1) |
| $[(\bullet)^{2T}, A_2^+ + A_2^-, B_1^+ + B_1^-, 2C_1^-, D_1^- + D_2^+, 2E_2^+, Y_1^+ + Y_1^-, 2Z_2^+]$        | (1, 0, 1) |
| $[(\bullet)^{2T}, A_2^+ + A_2^-, B_1^- + B_2^-, 2C_1^-, D_1^- + D_2^+, 2E_2^+, Y_1^+ + Y_1^-, 2Z_2^+]$        | (0, 1, 0) |
| $[(\bullet)^{2T}, A_1^- + A_2^-, B_1^+ + B_1^-, 2C_1^-, 2D_1^-, E_1^- + E_2^+, Y_1^+ + Y_1^-, 2Z_2^+]$        | (1, 0, 1) |
| $[(\bullet)^{2T}, A_1^- + A_2^-, B_1^+ + B_2^-, 2C_1^-, D_1^- + D_2^+, E_1^- + E_2^+, Y_1^+ + Y_1^-, 2Z_2^+]$ | (1, 1, 1) |
| $[(\bullet)^{2T}, A_1^- + A_2^-, B_1^- + B_2^-, 2C_1^-, D_1^- + D_2^+, E_1^- + E_2^+, Y_1^+ + Y_1^-, 2Z_2^+]$ | trivial   |
| $[(\bullet)^{2T}, A_1^+ + A_2^+, B_1^+ + B_1^-, 2C_1^-, 2D_1^-, E_1^- + E_2^+, Y_1^+ + Y_1^-, 2Z_2^+]$        | (0, 1, 0) |
| $[(\bullet)^{2T}, A_1^+ + A_2^+, B_1^+ + B_2^-, 2C_1^-, D_1^- + D_2^+, E_1^- + E_2^+, Y_1^+ + Y_1^-, 2Z_2^+]$ | trivial   |
| $[(\bullet)^{2T}, A_1^+ + A_2^+, B_1^- + B_2^-, 2C_1^-, D_1^- + D_2^+, E_1^- + E_2^+, Y_1^+ + Y_1^-, 2Z_2^+]$ | (1, 1, 1) |
| $[(\bullet)^{2T}, A_2^+ + A_2^-, B_2^+ + B_2^-, 2C_1^-, 2D_2^+, 2E_2^+, Y_1^+ + Y_1^-, 2Z_2^+]$               | trivial   |
| $[(\bullet)^{2T}, A_1^- + A_2^-, B_2^+ + B_2^-, 2C_1^-, 2D_2^+, E_1^- + E_2^+, Y_1^+ + Y_1^-, 2Z_2^+]$        | (0, 1, 0) |
| $[(\bullet)^{2T}, A_1^+ + A_2^+, B_2^+ + B_2^-, 2C_1^-, 2D_2^+, E_1^- + E_2^+, Y_1^+ + Y_1^-, 2Z_2^+]$        | (1, 0, 1) |
| $[(\bullet)^{2T}, A_1^+ + A_1^-, B_1^+ + B_1^-, 2C_2^+, 2D_1^-, 2E_1^-, Y_2^+ + Y_2^-, 2Z_2^+]$               | (1, 1, 1) |
| $[(\bullet)^{2T}, A_1^+ + A_1^-, B_1^- + B_2^-, 2C_2^+, D_1^- + D_2^+, 2E_1^-, Y_2^+ + Y_2^-, 2Z_2^+]$        | (0, 1, 0) |
| $[(\bullet)^{2T}, A_1^+ + A_1^-, B_1^+ + B_1^-, C_1^- + C_2^+, 2D_1^-, 2E_1^-, Y_1^+ + Y_2^+, 2Z_2^+]$        | (0, 1, 0) |
| $[(\bullet)^{2T}, A_1^+ + A_1^-, B_1^- + B_2^-, C_1^- + C_2^+, D_1^- + D_2^+, 2E_1^-, Y_1^+ + Y_2^+, 2Z_2^+]$ | (1, 1, 1) |
| $[(\bullet)^{2T}, A_1^+ + A_1^-, B_1^+ + B_2^-, 2C_2^+, D_1^- + D_2^+, 2E_1^-, Y_2^+ + Y_2^-, 2Z_2^+]$        | (1, 0, 1) |
| $[(\bullet)^{2T}, A_1^+ + A_1^-, B_2^+ + B_2^-, 2C_2^+, 2D_2^+, 2E_1^-, Y_2^+ + Y_2^-, 2Z_2^+]$               | trivial   |
| $[(\bullet)^{2T}, A_1^+ + A_1^-, B_1^+ + B_2^-, C_1^- + C_2^+, D_1^- + D_2^+, 2E_1^-, Y_1^+ + Y_2^+, 2Z_2^+]$ | trivial   |
| $[(\bullet)^{2T}, A_1^+ + A_1^-, B_2^+ + B_2^-, C_1^- + C_2^+, 2D_2^+, 2E_1^-, Y_1^+ + Y_2^+, 2Z_2^+]$        | (1, 0, 1) |
| $[(\bullet)^{2T}, A_1^+ + A_1^-, B_1^+ + B_1^-, C_1^- + C_2^+, 2D_1^-, 2E_1^-, Y_1^- + Y_2^-, 2Z_2^+]$        | (1, 0, 1) |
| $[(\bullet)^{2T}, A_1^+ + A_1^-, B_1^- + B_2^-, C_1^- + C_2^+, D_1^- + D_2^+, 2E_1^-, Y_1^- + Y_2^-, 2Z_2^+]$ | trivial   |
| $[(\bullet)^{2T}, A_1^+ + A_1^-, B_1^+ + B_1^-, 2C_1^-, 2D_1^-, 2E_1^-, Y_1^+ + Y_1^-, 2Z_2^+]$               | trivial   |
| $[(\bullet)^{2T}, A_1^+ + A_1^-, B_1^- + B_2^-, 2C_1^-, D_1^- + D_2^+, 2E_1^-, Y_1^+ + Y_1^-, 2Z_2^+]$        | (1, 0, 1) |
| $[(\bullet)^{2T}, A_1^+ + A_1^-, B_1^+ + B_2^-, C_1^- + C_2^+, D_1^- + D_2^+, 2E_1^-, Y_1^- + Y_2^-, 2Z_2^+]$ | (1, 1, 1) |
| $[(\bullet)^{2T}, A_1^+ + A_1^-, B_2^+ + B_2^-, C_1^- + C_2^+, 2D_2^+, 2E_1^-, Y_1^- + Y_2^-, 2Z_2^+]$        | (0, 1, 0) |
| $[(\bullet)^{2T}, A_1^+ + A_1^-, B_1^+ + B_2^-, 2C_1^-, D_1^- + D_2^+, 2E_1^-, Y_1^+ + Y_1^-, 2Z_2^+]$        | (0, 1, 0) |
| $[(\bullet)^{2T}, A_1^+ + A_1^-, B_2^+ + B_2^-, 2C_1^-, 2D_2^+, 2E_1^-, Y_1^+ + Y_1^-, 2Z_2^+]$               | (1, 1, 1) |

Skipped higher-order solutions...

Space group 11 ( $\mathbb{Z}_2$ )1st minimal solution:  $\mu_1^T = 4$  (43 symmetry vectors)

| $\mathbf{n}^T$                                                                                                                                      | $\mathbf{v}^T \in \mathbb{Z}_2$ |
|-----------------------------------------------------------------------------------------------------------------------------------------------------|---------------------------------|
| $[(\bullet)^{2T} + 2\Gamma_1^-, 2A_1^- + A_2^+ + A_2^-, 2B_1^- + B_2^+ + B_2^-, 2C_1, 2D_1, 2E_1, Y_1^+ + Y_1^- + 2Y_2^+, 2Z_1]$                    | trivial                         |
| $[(\bullet)^{2T} + \Gamma_1^+ + \Gamma_1^-, 2A_1^- + 2A_2^-, 2B_1^- + 2B_2^-, 2C_1, 2D_1, 2E_1, 2Y_1^+ + 2Y_2^+, 2Z_1]$                             | trivial                         |
| $[(\bullet)^{2T} + \Gamma_1^+ + \Gamma_1^-, 2A_1^- + 2A_2^-, 2B_1^- + 2B_2^-, 2C_1, 2D_1, 2E_1, Y_1^+ + Y_1^- + Y_2^+ + Y_2^-, 2Z_1]$               | 1                               |
| $[(\bullet)^{2T} + \Gamma_1^+ + \Gamma_1^-, 2A_1^- + 2A_2^-, B_1^+ + B_1^- + B_2^+ + B_2^-, 2C_1, 2D_1, 2E_1, 2Y_1^+ + 2Y_2^+, 2Z_1]$               | 1                               |
| $[(\bullet)^{2T} + \Gamma_1^+ + \Gamma_1^-, 2A_1^- + 2A_2^-, B_1^+ + B_1^- + B_2^+ + B_2^-, 2C_1, 2D_1, 2E_1, Y_1^+ + Y_1^- + Y_2^+ + Y_2^-, 2Z_1]$ | trivial                         |
| $[(\bullet)^{2T} + \Gamma_1^+ + \Gamma_1^-, A_1^+ + A_1^- + A_2^+ + A_2^-, 2B_1^- + 2B_2^-, 2C_1, 2D_1, 2E_1, 2Y_1^+ + 2Y_2^+, 2Z_1]$               | 1                               |

... continued on next page

... continued from previous page

|                                                                                                                                                                   |         |
|-------------------------------------------------------------------------------------------------------------------------------------------------------------------|---------|
| $[(\bullet)^{2T} + \Gamma_1^+ + \Gamma_1^-, A_1^+ + A_1^- + A_2^+ + A_2^-, 2B_1^- + 2B_2^-, 2C_1, 2D_1, 2E_1, Y_1^+ + Y_1^- + Y_2^+ + Y_2^-, 2Z_1]$               | trivial |
| $[(\bullet)^{2T} + \Gamma_1^+ + \Gamma_1^-, A_1^+ + A_1^- + A_2^+ + A_2^-, B_1^+ + B_1^- + B_2^+ + B_2^-, 2C_1, 2D_1, 2E_1, 2Y_1^+ + 2Y_2^+, 2Z_1]$               | trivial |
| $[(\bullet)^{2T} + \Gamma_1^+ + \Gamma_1^-, A_1^+ + A_1^- + A_2^+ + A_2^-, B_1^+ + B_1^- + B_2^+ + B_2^-, 2C_1, 2D_1, 2E_1, Y_1^+ + Y_1^- + Y_2^+ + Y_2^-, 2Z_1]$ | 1       |
| $[(\bullet)^{2T} + 2\Gamma_1^-, 2A_1^- + A_2^+ + A_2^-, 2B_1^- + B_2^+ + B_2^-, 2C_1, 2D_1, 2E_1, 2Y_1^- + Y_2^+ + Y_2^-, 2Z_1]$                                  | 1       |
| $[(\bullet)^{2T} + \Gamma_1^+ + \Gamma_1^-, 2A_1^- + 2A_2^-, 2B_1^- + 2B_2^-, 2C_1, 2D_1, 2E_1, 2Y_1^- + 2Y_2^-, 2Z_1]$                                           | trivial |
| $[(\bullet)^{2T} + \Gamma_1^+ + \Gamma_1^-, 2A_1^- + 2A_2^-, B_1^+ + B_1^- + B_2^+ + B_2^-, 2C_1, 2D_1, 2E_1, 2Y_1^- + 2Y_2^-, 2Z_1]$                             | 1       |
| $[(\bullet)^{2T} + \Gamma_1^+ + \Gamma_1^-, A_1^+ + A_1^- + A_2^+ + A_2^-, 2B_1^- + 2B_2^-, 2C_1, 2D_1, 2E_1, 2Y_1^- + 2Y_2^-, 2Z_1]$                             | 1       |
| $[(\bullet)^{2T} + \Gamma_1^+ + \Gamma_1^-, A_1^+ + A_1^- + A_2^+ + A_2^-, B_1^+ + B_1^- + B_2^+ + B_2^-, 2C_1, 2D_1, 2E_1, 2Y_1^- + 2Y_2^-, 2Z_1]$               | trivial |
| $[(\bullet)^{2T} + 2\Gamma_1^-, 2A_1^- + A_2^+ + A_2^-, B_1^+ + B_1^- + 2B_2^+, 2C_1, 2D_1, 2E_1, Y_1^+ + Y_1^- + 2Y_2^+, 2Z_1]$                                  | 1       |
| $[(\bullet)^{2T} + 2\Gamma_1^-, 2A_1^- + A_2^+ + A_2^-, B_1^+ + B_1^- + 2B_2^+, 2C_1, 2D_1, 2E_1, 2Y_1^- + Y_2^+ + Y_2^-, 2Z_1]$                                  | trivial |
| $[(\bullet)^{2T} + 2\Gamma_1^-, A_1^+ + A_1^- + 2A_2^+, 2B_1^- + B_2^+ + B_2^-, 2C_1, 2D_1, 2E_1, Y_1^+ + Y_1^- + 2Y_2^+, 2Z_1]$                                  | 1       |
| $[(\bullet)^{2T} + 2\Gamma_1^-, A_1^+ + A_1^- + 2A_2^+, 2B_1^- + B_2^+ + B_2^-, 2C_1, 2D_1, 2E_1, 2Y_1^- + Y_2^+ + Y_2^-, 2Z_1]$                                  | trivial |
| $[(\bullet)^{2T} + 2\Gamma_1^-, A_1^+ + A_1^- + 2A_2^+, B_1^+ + B_1^- + 2B_2^+, 2C_1, 2D_1, 2E_1, Y_1^+ + Y_1^- + 2Y_2^+, 2Z_1]$                                  | trivial |
| $[(\bullet)^{2T} + 2\Gamma_1^-, A_1^+ + A_1^- + 2A_2^+, B_1^+ + B_1^- + 2B_2^+, 2C_1, 2D_1, 2E_1, 2Y_1^- + Y_2^+ + Y_2^-, 2Z_1]$                                  | 1       |
| $[(\bullet)^{2T} + 2\Gamma_1^+, A_1^+ + A_1^- + 2A_2^-, B_1^+ + B_1^- + 2B_2^-, 2C_1, 2D_1, 2E_1, 2Y_1^+ + Y_2^+ + Y_2^-, 2Z_1]$                                  | 1       |
| $[(\bullet)^{2T} + 2\Gamma_1^+, A_1^+ + A_1^- + 2A_2^-, B_1^+ + B_1^- + 2B_2^-, 2C_1, 2D_1, 2E_1, Y_1^+ + Y_1^- + 2Y_2^-, 2Z_1]$                                  | trivial |
| $[(\bullet)^{2T} + \Gamma_1^+ + \Gamma_1^-, 2A_1^- + 2A_2^-, 2B_1^+ + 2B_2^+, 2C_1, 2D_1, 2E_1, 2Y_1^+ + 2Y_2^+, 2Z_1]$                                           | trivial |
| $[(\bullet)^{2T} + \Gamma_1^+ + \Gamma_1^-, 2A_1^- + 2A_2^-, 2B_1^+ + 2B_2^+, 2C_1, 2D_1, 2E_1, Y_1^+ + Y_1^- + Y_2^+ + Y_2^-, 2Z_1]$                             | 1       |
| $[(\bullet)^{2T} + \Gamma_1^+ + \Gamma_1^-, A_1^+ + A_1^- + A_2^+ + A_2^-, 2B_1^+ + 2B_2^+, 2C_1, 2D_1, 2E_1, 2Y_1^+ + 2Y_2^+, 2Z_1]$                             | 1       |
| $[(\bullet)^{2T} + \Gamma_1^+ + \Gamma_1^-, A_1^+ + A_1^- + A_2^+ + A_2^-, 2B_1^+ + 2B_2^+, 2C_1, 2D_1, 2E_1, Y_1^+ + Y_1^- + Y_2^+ + Y_2^-, 2Z_1]$               | trivial |
| $[(\bullet)^{2T} + \Gamma_1^+ + \Gamma_1^-, 2A_1^- + 2A_2^-, 2B_1^+ + 2B_2^+, 2C_1, 2D_1, 2E_1, 2Y_1^- + 2Y_2^-, 2Z_1]$                                           | trivial |
| $[(\bullet)^{2T} + \Gamma_1^+ + \Gamma_1^-, A_1^+ + A_1^- + A_2^+ + A_2^-, 2B_1^+ + 2B_2^+, 2C_1, 2D_1, 2E_1, 2Y_1^- + 2Y_2^-, 2Z_1]$                             | 1       |
| $[(\bullet)^{2T} + 2\Gamma_1^+, A_1^+ + A_1^- + 2A_2^-, 2B_1^+ + B_2^+ + B_2^-, 2C_1, 2D_1, 2E_1, 2Y_1^+ + Y_2^+ + Y_2^-, 2Z_1]$                                  | trivial |
| $[(\bullet)^{2T} + 2\Gamma_1^+, A_1^+ + A_1^- + 2A_2^-, 2B_1^+ + B_2^+ + B_2^-, 2C_1, 2D_1, 2E_1, Y_1^+ + Y_1^- + 2Y_2^-, 2Z_1]$                                  | 1       |
| $[(\bullet)^{2T} + \Gamma_1^+ + \Gamma_1^-, 2A_1^+ + 2A_2^+, 2B_1^- + 2B_2^-, 2C_1, 2D_1, 2E_1, 2Y_1^+ + 2Y_2^+, 2Z_1]$                                           | trivial |
| $[(\bullet)^{2T} + \Gamma_1^+ + \Gamma_1^-, 2A_1^+ + 2A_2^+, 2B_1^- + 2B_2^-, 2C_1, 2D_1, 2E_1, Y_1^+ + Y_1^- + Y_2^+ + Y_2^-, 2Z_1]$                             | 1       |
| $[(\bullet)^{2T} + \Gamma_1^+ + \Gamma_1^-, 2A_1^+ + 2A_2^+, B_1^+ + B_1^- + B_2^+ + B_2^-, 2C_1, 2D_1, 2E_1, 2Y_1^+ + 2Y_2^+, 2Z_1]$                             | 1       |
| $[(\bullet)^{2T} + \Gamma_1^+ + \Gamma_1^-, 2A_1^+ + 2A_2^+, B_1^+ + B_1^- + B_2^+ + B_2^-, 2C_1, 2D_1, 2E_1, Y_1^+ + Y_1^- + Y_2^+ + Y_2^-, 2Z_1]$               | trivial |
| $[(\bullet)^{2T} + \Gamma_1^+ + \Gamma_1^-, 2A_1^+ + 2A_2^+, 2B_1^- + 2B_2^-, 2C_1, 2D_1, 2E_1, 2Y_1^- + 2Y_2^-, 2Z_1]$                                           | trivial |
| $[(\bullet)^{2T} + \Gamma_1^+ + \Gamma_1^-, 2A_1^+ + 2A_2^+, B_1^+ + B_1^- + B_2^+ + B_2^-, 2C_1, 2D_1, 2E_1, 2Y_1^- + 2Y_2^-, 2Z_1]$                             | 1       |
| $[(\bullet)^{2T} + 2\Gamma_1^+, 2A_1^+ + A_2^+ + A_2^-, B_1^+ + B_1^- + 2B_2^-, 2C_1, 2D_1, 2E_1, 2Y_1^+ + Y_2^+ + Y_2^-, 2Z_1]$                                  | trivial |
| $[(\bullet)^{2T} + 2\Gamma_1^+, 2A_1^+ + A_2^+ + A_2^-, B_1^+ + B_1^- + 2B_2^-, 2C_1, 2D_1, 2E_1, Y_1^+ + Y_1^- + 2Y_2^-, 2Z_1]$                                  | 1       |
| $[(\bullet)^{2T} + \Gamma_1^+ + \Gamma_1^-, 2A_1^+ + 2A_2^+, 2B_1^+ + 2B_2^+, 2C_1, 2D_1, 2E_1, 2Y_1^+ + 2Y_2^+, 2Z_1]$                                           | trivial |
| $[(\bullet)^{2T} + \Gamma_1^+ + \Gamma_1^-, 2A_1^+ + 2A_2^+, 2B_1^+ + 2B_2^+, 2C_1, 2D_1, 2E_1, Y_1^+ + Y_1^- + Y_2^+ + Y_2^-, 2Z_1]$                             | 1       |
| $[(\bullet)^{2T} + \Gamma_1^+ + \Gamma_1^-, 2A_1^+ + 2A_2^+, 2B_1^+ + 2B_2^+, 2C_1, 2D_1, 2E_1, 2Y_1^- + 2Y_2^-, 2Z_1]$                                           | trivial |
| $[(\bullet)^{2T} + 2\Gamma_1^+, 2A_1^+ + A_2^+ + A_2^-, 2B_1^+ + B_2^+ + B_2^-, 2C_1, 2D_1, 2E_1, 2Y_1^+ + Y_2^+ + Y_2^-, 2Z_1]$                                  | 1       |
| $[(\bullet)^{2T} + 2\Gamma_1^+, 2A_1^+ + A_2^+ + A_2^-, 2B_1^+ + B_2^+ + B_2^-, 2C_1, 2D_1, 2E_1, Y_1^+ + Y_1^- + 2Y_2^-, 2Z_1]$                                  | trivial |

2nd minimal solution:  $\mu_2^T = 6$  (252 symmetry vectors)

Space group 12 ( $\mathbb{Z}_2 \times \mathbb{Z}_2$ )

1st minimal solution:  $\mu_1^T = 2$  (54 symmetry vectors)

| $\mathbf{n}^T$                                                                                | $\mathbf{v}^T \in \mathbb{Z}_2 \times \mathbb{Z}_2$ |
|-----------------------------------------------------------------------------------------------|-----------------------------------------------------|
| $[(\bullet)^{2T}, A_2^+ + A_2^-, M_2^+ + M_2^-, Y_2^+ + Y_2^-, 2L_1^-, 2V_1^+]$               | (0, 1)                                              |
| $[(\bullet)^{2T}, A_2^+ + A_2^-, M_2^+ + M_2^-, Y_2^+ + Y_2^-, 2L_1^-, V_1^+ + V_1^-]$        | (1, 1)                                              |
| $[(\bullet)^{2T}, A_2^+ + A_2^-, M_2^+ + M_2^-, Y_2^+ + Y_2^-, 2L_1^-, 2V_1^-]$               | (0, 1)                                              |
| $[(\bullet)^{2T}, A_2^+ + A_2^-, M_2^+ + M_2^-, Y_2^+ + Y_2^-, L_1^+ + L_1^-, 2V_1^+]$        | (1, 1)                                              |
| $[(\bullet)^{2T}, A_2^+ + A_2^-, M_2^+ + M_2^-, Y_2^+ + Y_2^-, L_1^+ + L_1^-, V_1^+ + V_1^-]$ | (0, 1)                                              |
| $[(\bullet)^{2T}, A_2^+ + A_2^-, M_2^+ + M_2^-, Y_2^+ + Y_2^-, L_1^+ + L_1^-, 2V_1^-]$        | (1, 1)                                              |

... continued on next page



Space group 13 ( $\mathbb{Z}_2 \times \mathbb{Z}_2$ )

1st minimal solution:  $\mu_1^T = 2$  (6 symmetry vectors & filling-enforced topology)

| $\mathbf{n}^T$                                                                      | $\mathbf{v}^T \in \mathbb{Z}_2 \times \mathbb{Z}_2$ |
|-------------------------------------------------------------------------------------|-----------------------------------------------------|
| $[(\bullet)^{2T}, A_1, B_1, C_1^+ + C_2^+, D_1, E_1, Y_1^- + Y_2^-, Z_2^+ + Z_2^-]$ | (0, 1)                                              |
| $[(\bullet)^{2T}, A_1, B_1, C_1^+ + C_2^+, D_1, E_1, Y_1^+ + Y_2^+, Z_2^+ + Z_2^-]$ | (1, 1)                                              |
| $[(\bullet)^{2T}, A_1, B_1, C_1^+ + C_1^-, D_1, E_1, Y_1^+ + Y_1^-, Z_2^+ + Z_2^-]$ | (1, 0)                                              |
| $[(\bullet)^{2T}, A_1, B_1, C_2^+ + C_2^-, D_1, E_1, Y_2^+ + Y_2^-, Z_2^+ + Z_2^-]$ | (1, 0)                                              |
| $[(\bullet)^{2T}, A_1, B_1, C_1^- + C_2^-, D_1, E_1, Y_1^- + Y_2^-, Z_2^+ + Z_2^-]$ | (1, 1)                                              |
| $[(\bullet)^{2T}, A_1, B_1, C_1^- + C_2^-, D_1, E_1, Y_1^+ + Y_2^+, Z_2^+ + Z_2^-]$ | (0, 1)                                              |

2nd minimal solution:  $\mu_2^T = 4$  (152 symmetry vectors)

Space group 14 ( $\mathbb{Z}_2$ )

1st minimal solution:  $\mu_1^T = 4$  (27 symmetry vectors)

| $\mathbf{n}^T$                                                                                                                                            | $\mathbf{v}^T \in \mathbb{Z}_2$ |
|-----------------------------------------------------------------------------------------------------------------------------------------------------------|---------------------------------|
| $[(\bullet)^{2T} + \Gamma_1^+ + \Gamma_1^-, 2A_1, 2B_1, 2C_1, 2D_1^+ D_2^+, 2E_1^- E_2^-, 2Y_1^- + 2Y_2^-, 2Z_1]$                                         | trivial                         |
| $[(\bullet)^{2T} + \Gamma_1^+ + \Gamma_1^-, 2A_1, 2B_1, 2C_1, 2D_1^+ D_2^+, 2E_1^- E_2^-, Y_1^+ + Y_1^- + Y_2^+ + Y_2^-, 2Z_1]$                           | 1                               |
| $[(\bullet)^{2T} + \Gamma_1^+ + \Gamma_1^-, 2A_1, 2B_1, 2C_1, 2D_1^+ D_2^+, E_1^+ E_2^+ + E_1^- E_2^-, 2Y_1^- + 2Y_2^-, 2Z_1]$                            | 1                               |
| $[(\bullet)^{2T} + \Gamma_1^+ + \Gamma_1^-, 2A_1, 2B_1, 2C_1, 2D_1^+ D_2^+, E_1^+ E_2^+ + E_1^- E_2^-, Y_1^+ + Y_1^- + Y_2^+ + Y_2^-, 2Z_1]$              | trivial                         |
| $[(\bullet)^{2T} + \Gamma_1^+ + \Gamma_1^-, 2A_1, 2B_1, 2C_1, D_1^+ D_2^+ + D_1^- D_2^-, 2E_1^- E_2^-, 2Y_1^- + 2Y_2^-, 2Z_1]$                            | 1                               |
| $[(\bullet)^{2T} + \Gamma_1^+ + \Gamma_1^-, 2A_1, 2B_1, 2C_1, D_1^+ D_2^+ + D_1^- D_2^-, 2E_1^- E_2^-, Y_1^+ + Y_1^- + Y_2^+ + Y_2^-, 2Z_1]$              | trivial                         |
| $[(\bullet)^{2T} + \Gamma_1^+ + \Gamma_1^-, 2A_1, 2B_1, 2C_1, D_1^+ D_2^+ + D_1^- D_2^-, E_1^+ E_2^+ + E_1^- E_2^-, 2Y_1^- + 2Y_2^-, 2Z_1]$               | trivial                         |
| $[(\bullet)^{2T} + \Gamma_1^+ + \Gamma_1^-, 2A_1, 2B_1, 2C_1, D_1^+ D_2^+ + D_1^- D_2^-, E_1^+ E_2^+ + E_1^- E_2^-, Y_1^+ + Y_1^- + Y_2^+ + Y_2^-, 2Z_1]$ | 1                               |
| $[(\bullet)^{2T} + \Gamma_1^+ + \Gamma_1^-, 2A_1, 2B_1, 2C_1, 2D_1^+ D_2^+, 2E_1^- E_2^-, 2Y_1^+ + 2Y_2^+, 2Z_1]$                                         | trivial                         |
| $[(\bullet)^{2T} + \Gamma_1^+ + \Gamma_1^-, 2A_1, 2B_1, 2C_1, 2D_1^+ D_2^+, E_1^+ E_2^+ + E_1^- E_2^-, 2Y_1^+ + 2Y_2^+, 2Z_1]$                            | 1                               |
| $[(\bullet)^{2T} + \Gamma_1^+ + \Gamma_1^-, 2A_1, 2B_1, 2C_1, D_1^+ D_2^+ + D_1^- D_2^-, 2E_1^- E_2^-, 2Y_1^+ + 2Y_2^+, 2Z_1]$                            | 1                               |
| $[(\bullet)^{2T} + \Gamma_1^+ + \Gamma_1^-, 2A_1, 2B_1, 2C_1, D_1^+ D_2^+ + D_1^- D_2^-, E_1^+ E_2^+ + E_1^- E_2^-, 2Y_1^+ + 2Y_2^+, 2Z_1]$               | trivial                         |
| $[(\bullet)^{2T} + \Gamma_1^+ + \Gamma_1^-, 2A_1, 2B_1, 2C_1, 2D_1^+ D_2^+, 2E_1^+ E_2^+, 2Y_1^- + 2Y_2^-, 2Z_1]$                                         | trivial                         |
| $[(\bullet)^{2T} + \Gamma_1^+ + \Gamma_1^-, 2A_1, 2B_1, 2C_1, 2D_1^+ D_2^+, 2E_1^+ E_2^+, Y_1^+ + Y_1^- + Y_2^+ + Y_2^-, 2Z_1]$                           | 1                               |
| $[(\bullet)^{2T} + \Gamma_1^+ + \Gamma_1^-, 2A_1, 2B_1, 2C_1, D_1^+ D_2^+ + D_1^- D_2^-, 2E_1^+ E_2^+, 2Y_1^- + 2Y_2^-, 2Z_1]$                            | 1                               |
| $[(\bullet)^{2T} + \Gamma_1^+ + \Gamma_1^-, 2A_1, 2B_1, 2C_1, D_1^+ D_2^+ + D_1^- D_2^-, 2E_1^+ E_2^+, Y_1^+ + Y_1^- + Y_2^+ + Y_2^-, 2Z_1]$              | trivial                         |
| $[(\bullet)^{2T} + \Gamma_1^+ + \Gamma_1^-, 2A_1, 2B_1, 2C_1, 2D_1^+ D_2^+, 2E_1^+ E_2^+, 2Y_1^+ + 2Y_2^+, 2Z_1]$                                         | trivial                         |
| $[(\bullet)^{2T} + \Gamma_1^+ + \Gamma_1^-, 2A_1, 2B_1, 2C_1, D_1^+ D_2^+ + D_1^- D_2^-, 2E_1^+ E_2^+, 2Y_1^+ + 2Y_2^+, 2Z_1]$                            | 1                               |
| $[(\bullet)^{2T} + \Gamma_1^+ + \Gamma_1^-, 2A_1, 2B_1, 2C_1, 2D_1^- D_2^-, 2E_1^- E_2^-, 2Y_1^- + 2Y_2^-, 2Z_1]$                                         | trivial                         |
| $[(\bullet)^{2T} + \Gamma_1^+ + \Gamma_1^-, 2A_1, 2B_1, 2C_1, 2D_1^- D_2^-, 2E_1^- E_2^-, Y_1^+ + Y_1^- + Y_2^+ + Y_2^-, 2Z_1]$                           | 1                               |
| $[(\bullet)^{2T} + \Gamma_1^+ + \Gamma_1^-, 2A_1, 2B_1, 2C_1, 2D_1^- D_2^-, E_1^+ E_2^+ + E_1^- E_2^-, 2Y_1^- + 2Y_2^-, 2Z_1]$                            | 1                               |
| $[(\bullet)^{2T} + \Gamma_1^+ + \Gamma_1^-, 2A_1, 2B_1, 2C_1, 2D_1^- D_2^-, E_1^+ E_2^+ + E_1^- E_2^-, Y_1^+ + Y_1^- + Y_2^+ + Y_2^-, 2Z_1]$              | trivial                         |
| $[(\bullet)^{2T} + \Gamma_1^+ + \Gamma_1^-, 2A_1, 2B_1, 2C_1, 2D_1^- D_2^-, 2E_1^- E_2^-, 2Y_1^+ + 2Y_2^+, 2Z_1]$                                         | trivial                         |
| $[(\bullet)^{2T} + \Gamma_1^+ + \Gamma_1^-, 2A_1, 2B_1, 2C_1, 2D_1^- D_2^-, E_1^+ E_2^+ + E_1^- E_2^-, 2Y_1^+ + 2Y_2^+, 2Z_1]$                            | 1                               |
| $[(\bullet)^{2T} + \Gamma_1^+ + \Gamma_1^-, 2A_1, 2B_1, 2C_1, 2D_1^- D_2^-, 2E_1^+ E_2^+, 2Y_1^- + 2Y_2^-, 2Z_1]$                                         | trivial                         |
| $[(\bullet)^{2T} + \Gamma_1^+ + \Gamma_1^-, 2A_1, 2B_1, 2C_1, 2D_1^- D_2^-, 2E_1^+ E_2^+, Y_1^+ + Y_1^- + Y_2^+ + Y_2^-, 2Z_1]$                           | 1                               |
| $[(\bullet)^{2T} + \Gamma_1^+ + \Gamma_1^-, 2A_1, 2B_1, 2C_1, 2D_1^- D_2^-, 2E_1^+ E_2^+, 2Y_1^+ + 2Y_2^+, 2Z_1]$                                         | trivial                         |

2nd minimal solution:  $\mu_2^T = 6$  (128 symmetry vectors)

Space group 15 ( $\mathbb{Z}_2 \times \mathbb{Z}_2$ )

1st minimal solution:  $\mu_1^T = 2$  (9 symmetry vectors)

| $\mathbf{n}^T$                                                            | $\mathbf{v}^T \in \mathbb{Z}_2 \times \mathbb{Z}_2$ |
|---------------------------------------------------------------------------|-----------------------------------------------------|
| $[(\bullet)^{2T}, A_1, M_1, Y_2^+ + Y_2^-, 2L_1^-, 2V_1^-]$               | trivial                                             |
| $[(\bullet)^{2T}, A_1, M_1, Y_2^+ + Y_2^-, L_1^+ + L_1^-, 2V_1^-]$        | (1, 0)                                              |
| $[(\bullet)^{2T}, A_1, M_1, Y_2^+ + Y_2^-, 2L_1^+, 2V_1^-]$               | trivial                                             |
| $[(\bullet)^{2T}, A_1, M_1, Y_2^+ + Y_2^-, 2L_1^-, V_1^+ + V_1^-]$        | (1, 1)                                              |
| $[(\bullet)^{2T}, A_1, M_1, Y_2^+ + Y_2^-, L_1^+ + L_1^-, V_1^+ + V_1^-]$ | (0, 1)                                              |
| $[(\bullet)^{2T}, A_1, M_1, Y_2^+ + Y_2^-, 2L_1^+, V_1^+ + V_1^-]$        | (1, 1)                                              |
| $[(\bullet)^{2T}, A_1, M_1, Y_2^+ + Y_2^-, 2L_1^-, 2V_1^+]$               | trivial                                             |
| $[(\bullet)^{2T}, A_1, M_1, Y_2^+ + Y_2^-, L_1^+ + L_1^-, 2V_1^+]$        | (1, 0)                                              |
| $[(\bullet)^{2T}, A_1, M_1, Y_2^+ + Y_2^-, 2L_1^+, 2V_1^+]$               | trivial                                             |

2nd minimal solution:  $\mu_2^T = 4$  (200 symmetry vectors)

Space group 16 ( $\mathbb{Z}_1$ )

1st minimal solution:  $\mu_1^T = 2$  (28 symmetry vectors)

| $\mathbf{n}^T$                                                                             |
|--------------------------------------------------------------------------------------------|
| $[(\bullet)^{2T}, R_3 + R_4, S_3 + S_4, T_1 + T_4, U_2 + U_4, X_2 + X_4, Y_2 + Y_3, 2Z_4]$ |
| $[(\bullet)^{2T}, R_2 + R_3, S_2 + S_3, T_1 + T_4, 2U_2, 2X_2, Y_2 + Y_3, 2Z_4]$           |
| $[(\bullet)^{2T}, 2R_4, S_3 + S_4, T_2 + T_4, U_1 + U_4, X_2 + X_4, Y_2 + Y_3, Z_3 + Z_4]$ |
| $[(\bullet)^{2T}, R_3 + R_4, 2S_3, T_3 + T_4, U_1 + U_2, 2X_2, 2Y_3, Z_3 + Z_4]$           |
| $[(\bullet)^{2T}, R_2 + R_4, S_2 + S_3, T_2 + T_4, U_1 + U_2, 2X_2, Y_2 + Y_3, Z_3 + Z_4]$ |
| $[(\bullet)^{2T}, R_1 + R_4, S_1 + S_3, T_3 + T_4, U_1 + U_4, X_2 + X_4, 2Y_3, Z_3 + Z_4]$ |
| $[(\bullet)^{2T}, R_2 + R_4, S_1 + S_4, T_2 + T_4, U_3 + U_4, 2X_4, Y_2 + Y_3, Z_3 + Z_4]$ |
| $[(\bullet)^{2T}, R_2 + R_3, S_1 + S_3, T_3 + T_4, U_2 + U_3, X_2 + X_4, 2Y_3, Z_3 + Z_4]$ |
| $[(\bullet)^{2T}, 2R_2, S_1 + S_2, T_2 + T_4, U_2 + U_3, X_2 + X_4, Y_2 + Y_3, Z_3 + Z_4]$ |
| $[(\bullet)^{2T}, R_1 + R_2, 2S_1, T_3 + T_4, U_3 + U_4, 2X_4, 2Y_3, Z_3 + Z_4]$           |
| $[(\bullet)^{2T}, R_1 + R_4, S_1 + S_4, T_1 + T_4, 2U_4, 2X_4, Y_2 + Y_3, 2Z_4]$           |
| $[(\bullet)^{2T}, R_1 + R_2, S_1 + S_2, T_1 + T_4, U_2 + U_4, X_2 + X_4, Y_2 + Y_3, 2Z_4]$ |
| $[(\bullet)^{2T}, R_2 + R_4, S_1 + S_3, 2T_4, U_2 + U_4, X_2 + X_4, 2Y_3, 2Z_4]$           |
| $[(\bullet)^{2T}, 2R_3, S_3 + S_4, T_1 + T_3, U_2 + U_3, X_2 + X_4, Y_2 + Y_3, Z_3 + Z_4]$ |
| $[(\bullet)^{2T}, R_3 + R_4, S_3 + S_4, T_2 + T_3, U_1 + U_3, X_2 + X_4, Y_2 + Y_3, 2Z_3]$ |
| $[(\bullet)^{2T}, R_1 + R_3, S_1 + S_3, 2T_3, U_1 + U_3, X_2 + X_4, 2Y_3, 2Z_3]$           |
| $[(\bullet)^{2T}, R_2 + R_3, S_1 + S_4, T_2 + T_3, 2U_3, 2X_4, Y_2 + Y_3, 2Z_3]$           |
| $[(\bullet)^{2T}, R_1 + R_3, S_1 + S_4, T_1 + T_3, U_3 + U_4, 2X_4, Y_2 + Y_3, Z_3 + Z_4]$ |
| $[(\bullet)^{2T}, R_2 + R_3, S_2 + S_4, T_1 + T_2, U_2 + U_3, X_2 + X_4, 2Y_2, Z_3 + Z_4]$ |
| $[(\bullet)^{2T}, R_2 + R_4, S_2 + S_4, 2T_2, U_1 + U_3, X_2 + X_4, 2Y_2, 2Z_3]$           |
| $[(\bullet)^{2T}, R_1 + R_2, S_1 + S_2, T_2 + T_3, U_1 + U_3, X_2 + X_4, Y_2 + Y_3, 2Z_3]$ |
| $[(\bullet)^{2T}, R_1 + R_3, S_2 + S_4, 2T_1, U_2 + U_4, X_2 + X_4, 2Y_2, 2Z_4]$           |
| $[(\bullet)^{2T}, R_1 + R_4, S_2 + S_4, T_1 + T_2, U_1 + U_4, X_2 + X_4, 2Y_2, Z_3 + Z_4]$ |
| $[(\bullet)^{2T}, R_1 + R_3, S_2 + S_3, T_1 + T_3, U_1 + U_2, 2X_2, Y_2 + Y_3, Z_3 + Z_4]$ |
| $[(\bullet)^{2T}, R_1 + R_2, 2S_2, T_1 + T_2, U_1 + U_2, 2X_2, 2Y_2, Z_3 + Z_4]$           |
| $[(\bullet)^{2T}, 2R_1, S_1 + S_2, T_1 + T_3, U_1 + U_4, X_2 + X_4, Y_2 + Y_3, Z_3 + Z_4]$ |
| $[(\bullet)^{2T}, R_1 + R_4, S_2 + S_3, T_2 + T_3, 2U_1, 2X_2, Y_2 + Y_3, 2Z_3]$           |
| $[(\bullet)^{2T}, R_3 + R_4, 2S_4, T_1 + T_2, U_3 + U_4, 2X_4, 2Y_2, Z_3 + Z_4]$           |



2nd minimal solution:  $\mu_2^T = 3$  (920 symmetry vectors)

Space group 17 ( $\mathbb{Z}_1$ )

1st minimal solution:  $\mu_1^T = 4$  (10 symmetry vectors)

| $\mathbf{n}^T$                                                                                                              |
|-----------------------------------------------------------------------------------------------------------------------------|
| $[(\bullet)^{2T} + 2\Gamma_2, 2R_1, S_1 + S_2 + S_3 + S_4, 2T_1, 2U_1, 2X_2 + 2X_4, 2Y_2 + 2Y_3, 2Z_1]$                     |
| $[(\bullet)^{2T} + \Gamma_1 + \Gamma_2, 2R_1, S_1 + S_2 + 2S_4, 2T_1, 2U_1, X_1 + X_2 + 2X_4, 2Y_2 + Y_3 + Y_4, 2Z_1]$      |
| $[(\bullet)^{2T} + \Gamma_1 + \Gamma_2, 2R_1, 2S_1 + S_3 + S_4, 2T_1, 2U_1, X_1 + X_2 + 2X_4, Y_1 + Y_2 + 2Y_3, 2Z_1]$      |
| $[(\bullet)^{2T} + \Gamma_1 + \Gamma_2, 2R_1, 2S_2 + S_3 + S_4, 2T_1, 2U_1, 2X_2 + X_3 + X_4, 2Y_2 + Y_3 + Y_4, 2Z_1]$      |
| $[(\bullet)^{2T} + \Gamma_1 + \Gamma_2, 2R_1, S_1 + S_2 + 2S_3, 2T_1, 2U_1, 2X_2 + X_3 + X_4, Y_1 + Y_2 + 2Y_3, 2Z_1]$      |
| $[(\bullet)^{2T} + 2\Gamma_1, 2R_1, 2S_2 + 2S_4, 2T_1, 2U_1, X_1 + X_2 + X_3 + X_4, 2Y_2 + 2Y_4, 2Z_1]$                     |
| $[(\bullet)^{2T} + 2\Gamma_1, 2R_1, S_1 + S_2 + S_3 + S_4, 2T_1, 2U_1, X_1 + X_2 + X_3 + X_4, Y_1 + Y_2 + Y_3 + Y_4, 2Z_1]$ |
| $[(\bullet)^{2T} + 2\Gamma_1, 2R_1, 2S_1 + 2S_3, 2T_1, 2U_1, X_1 + X_2 + X_3 + X_4, 2Y_1 + 2Y_3, 2Z_1]$                     |
| $[(\bullet)^{2T} + 2\Gamma_1, 2R_1, 2S_1 + 2S_4, 2T_1, 2U_1, 2X_1 + 2X_4, Y_1 + Y_2 + Y_3 + Y_4, 2Z_1]$                     |
| $[(\bullet)^{2T} + 2\Gamma_1, 2R_1, 2S_2 + 2S_3, 2T_1, 2U_1, 2X_2 + 2X_3, Y_1 + Y_2 + Y_3 + Y_4, 2Z_1]$                     |

2nd minimal solution:  $\mu_2^T = 6$  (48 symmetry vectors)

Space group 18 ( $\mathbb{Z}_1$ )

1st minimal solution:  $\mu_1^T = 4$  (3 symmetry vectors)

| $\mathbf{n}^T$                                                                                                  |
|-----------------------------------------------------------------------------------------------------------------|
| $[(\bullet)^{2T} + 2\Gamma_1, 2R_3R_4, 2S_3S_4, 2T_1, 2U_1, 2X_1, 2Y_1, Z_1 + Z_2 + Z_3 + Z_4]$                 |
| $[(\bullet)^{2T} + 2\Gamma_1, R_1R_2 + R_3R_4, S_1S_2 + S_3S_4, 2T_1, 2U_1, 2X_1, 2Y_1, Z_1 + Z_2 + Z_3 + Z_4]$ |
| $[(\bullet)^{2T} + 2\Gamma_1, 2R_1R_2, 2S_1S_2, 2T_1, 2U_1, 2X_1, 2Y_1, Z_1 + Z_2 + Z_3 + Z_4]$                 |

2nd minimal solution:  $\mu_2^T = 6$  (8 symmetry vectors)

Space group 19 ( $\mathbb{Z}_1$ )

1st minimal solution:  $\mu_1^T = 4$  (1 symmetry vector)

| $\mathbf{n}^T$                                                                                              |
|-------------------------------------------------------------------------------------------------------------|
| $[(\bullet)^{2T} + 2\Gamma_1, R_1R_1, S_1S_2 + S_3S_4, T_1T_3 + T_2T_4, U_1U_4 + U_2U_3, 2X_1, 2Y_1, 2Z_1]$ |

2nd minimal solution:  $\mu_2^T = 8$  (1 symmetry vector)

Space group 20 ( $\mathbb{Z}_1$ )

1st minimal solution:  $\mu_1^T = 4$  (2 symmetry vectors)

| $\mathbf{n}^T$                                                                                    |
|---------------------------------------------------------------------------------------------------|
| $[(\blacksquare)^{2T} + \Gamma_1 + \Gamma_2, 2T_1, 2Y_2 + Y_3 + Y_4, 2Z_1, 2R_1R_2, 2S_1 + 2S_2]$ |
| $[(\blacksquare)^{2T} + 2\Gamma_1, 2T_1, Y_1 + Y_2 + Y_3 + Y_4, 2Z_1, 2R_1R_2, 2S_1 + 2S_2]$      |

2nd minimal solution:  $\mu_2^T = 6$  (6 symmetry vectors)

Space group 21 ( $\mathbb{Z}_1$ )

1st minimal solution:  $\mu_1^T = 2$  (3 symmetry vectors)

| $\mathbf{n}^T$                                                            |
|---------------------------------------------------------------------------|
| $[(\blacksquare)^{2T}, T_1 + T_2, 2Y_2, Z_3 + Z_4, 2R_2, 2S_2]$           |
| $[(\blacksquare)^{2T}, T_1 + T_2, 2Y_2, Z_3 + Z_4, R_1 + R_2, S_1 + S_2]$ |
| $[(\blacksquare)^{2T}, T_1 + T_2, 2Y_2, Z_3 + Z_4, 2R_1, 2S_1]$           |

2nd minimal solution:  $\mu_2^T = 3$  (56 symmetry vectors)

Space group 22 ( $\mathbb{Z}_1$ )

1st minimal solution:  $\mu_1^T = 2$  (1 symmetry vector)

| $\mathbf{n}^T$                                                 |
|----------------------------------------------------------------|
| $[(\blacksquare)^{2T}, T_2 + T_4, Y_2 + Y_3, Z_3 + Z_4, 2L_1]$ |

2nd minimal solution:  $\mu_2^T = 3$  (14 symmetry vectors)

Space group 23 ( $\mathbb{Z}_1$ )

1st minimal solution:  $\mu_1^T = 3$  (20 symmetry vectors)

| $\mathbf{n}^T$                                                                                                               |
|------------------------------------------------------------------------------------------------------------------------------|
| $[(\blacksquare)^{2T} + \Gamma_1, 3W_4, 3WA_4, X_2 + X_3 + X_4, 3R_1, 3S_2, 3T_2]$                                           |
| $[(\blacksquare)^{2T} + \Gamma_1, W_3 + 2W_4, WA_3 + 2WA_4, X_2 + X_3 + X_4, 2R_1 + R_2, S_1 + 2S_2, 3T_2]$                  |
| $[(\blacksquare)^{2T} + \Gamma_1, W_2 + 2W_4, WA_2 + 2WA_4, X_2 + X_3 + X_4, 2R_1 + R_2, 3S_2, T_1 + 2T_2]$                  |
| $[(\blacksquare)^{2T} + \Gamma_1, W_1 + 2W_4, WA_1 + 2WA_4, X_2 + X_3 + X_4, 3R_1, S_1 + 2S_2, T_1 + 2T_2]$                  |
| $[(\blacksquare)^{2T} + \Gamma_1, 2W_3 + W_4, 2WA_3 + WA_4, X_2 + X_3 + X_4, R_1 + 2R_2, 2S_1 + S_2, 3T_2]$                  |
| $[(\blacksquare)^{2T} + \Gamma_1, W_2 + W_3 + W_4, WA_2 + WA_3 + WA_4, X_2 + X_3 + X_4, R_1 + 2R_2, S_1 + 2S_2, T_1 + 2T_2]$ |
| $[(\blacksquare)^{2T} + \Gamma_1, W_1 + W_3 + W_4, WA_1 + WA_3 + WA_4, X_2 + X_3 + X_4, 2R_1 + R_2, 2S_1 + S_2, T_1 + 2T_2]$ |
| $[(\blacksquare)^{2T} + \Gamma_1, 2W_2 + W_4, 2WA_2 + WA_4, X_2 + X_3 + X_4, R_1 + 2R_2, 3S_2, 2T_1 + T_2]$                  |
| $[(\blacksquare)^{2T} + \Gamma_1, W_1 + W_2 + W_4, WA_1 + WA_2 + WA_4, X_2 + X_3 + X_4, 2R_1 + R_2, S_1 + 2S_2, 2T_1 + T_2]$ |
| $[(\blacksquare)^{2T} + \Gamma_1, 2W_1 + W_4, 2WA_1 + WA_4, X_2 + X_3 + X_4, 3R_1, 2S_1 + S_2, 2T_1 + T_2]$                  |
| $[(\blacksquare)^{2T} + \Gamma_1, 3W_3, 3WA_3, X_2 + X_3 + X_4, 3R_2, 3S_1, 3T_2]$                                           |
| $[(\blacksquare)^{2T} + \Gamma_1, W_2 + 2W_3, WA_2 + 2WA_3, X_2 + X_3 + X_4, 3R_2, 2S_1 + S_2, T_1 + 2T_2]$                  |
| $[(\blacksquare)^{2T} + \Gamma_1, W_1 + 2W_3, WA_1 + 2WA_3, X_2 + X_3 + X_4, R_1 + 2R_2, 3S_1, T_1 + 2T_2]$                  |
| $[(\blacksquare)^{2T} + \Gamma_1, 2W_2 + W_3, 2WA_2 + WA_3, X_2 + X_3 + X_4, 3R_2, S_1 + 2S_2, 2T_1 + T_2]$                  |

... continued on next page

... continued from previous page

---

|                                                                                                                              |
|------------------------------------------------------------------------------------------------------------------------------|
| $[(\blacksquare)^{2T} + \Gamma_1, W_1 + W_2 + W_3, WA_1 + WA_2 + WA_3, X_2 + X_3 + X_4, R_1 + 2R_2, 2S_1 + S_2, 2T_1 + T_2]$ |
| $[(\blacksquare)^{2T} + \Gamma_1, 2W_1 + W_3, 2WA_1 + WA_3, X_2 + X_3 + X_4, 2R_1 + R_2, 3S_1, 2T_1 + T_2]$                  |
| $[(\blacksquare)^{2T} + \Gamma_1, 3W_2, 3WA_2, X_2 + X_3 + X_4, 3R_2, 3S_2, 3T_1]$                                           |
| $[(\blacksquare)^{2T} + \Gamma_1, W_1 + 2W_2, WA_1 + 2WA_2, X_2 + X_3 + X_4, R_1 + 2R_2, S_1 + 2S_2, 3T_1]$                  |
| $[(\blacksquare)^{2T} + \Gamma_1, 2W_1 + W_2, 2WA_1 + WA_2, X_2 + X_3 + X_4, 2R_1 + R_2, 2S_1 + S_2, 3T_1]$                  |
| $[(\blacksquare)^{2T} + \Gamma_1, 3W_1, 3WA_1, X_2 + X_3 + X_4, 3R_1, 3S_1, 3T_1]$                                           |

---

2nd minimal solution:  $\mu_2^T = 4$  (140 symmetry vectors)

Space group 24 ( $\mathbb{Z}_1$ )

1st minimal solution:  $\mu_1^T = 2$  (1 symmetry vector)

---

|                                                                           |
|---------------------------------------------------------------------------|
| $\mathbf{n}^T$                                                            |
| $[(\blacksquare)^{2T}, W_1, WA_1, 2X_4, R_1 + R_2, S_1 + S_2, T_1 + T_2]$ |

---

2nd minimal solution:  $\mu_2^T = 4$  (7 symmetry vectors)

Space group 25 ( $\mathbb{Z}_1$ )

1st minimal solution:  $\mu_1^T = 2$  (20 symmetry vectors)

---

|                                                                                                      |
|------------------------------------------------------------------------------------------------------|
| $\mathbf{n}^T$                                                                                       |
| $[(\blacksquare)^{2T}, 2R_3, 2S_3, T_2 + T_3, U_1 + U_3, X_1 + X_3, Y_2 + Y_3, Z_3 + Z_4]$           |
| $[(\blacksquare)^{2T}, R_3 + R_4, S_3 + S_4, T_1 + T_2, U_3 + U_4, X_3 + X_4, Y_1 + Y_2, Z_3 + Z_4]$ |
| $[(\blacksquare)^{2T}, R_2 + R_3, S_2 + S_3, T_2 + T_3, U_3 + U_4, X_3 + X_4, Y_2 + Y_3, Z_3 + Z_4]$ |
| $[(\blacksquare)^{2T}, R_1 + R_3, S_1 + S_3, T_1 + T_2, U_1 + U_3, X_1 + X_3, Y_1 + Y_2, Z_3 + Z_4]$ |
| $[(\blacksquare)^{2T}, R_3 + R_4, S_3 + S_4, T_3 + T_4, U_3 + U_4, X_3 + X_4, Y_3 + Y_4, Z_3 + Z_4]$ |
| $[(\blacksquare)^{2T}, R_1 + R_4, S_1 + S_4, T_1 + T_4, U_3 + U_4, X_3 + X_4, Y_1 + Y_4, Z_3 + Z_4]$ |
| $[(\blacksquare)^{2T}, R_1 + R_2, S_1 + S_2, T_1 + T_2, U_3 + U_4, X_3 + X_4, Y_1 + Y_2, Z_3 + Z_4]$ |
| $[(\blacksquare)^{2T}, R_1 + R_3, S_1 + S_3, T_3 + T_4, U_1 + U_3, X_1 + X_3, Y_3 + Y_4, Z_3 + Z_4]$ |
| $[(\blacksquare)^{2T}, R_1 + R_2, S_1 + S_2, T_3 + T_4, U_3 + U_4, X_3 + X_4, Y_3 + Y_4, Z_3 + Z_4]$ |
| $[(\blacksquare)^{2T}, 2R_1, 2S_1, T_1 + T_4, U_1 + U_3, X_1 + X_3, Y_1 + Y_4, Z_3 + Z_4]$           |
| $[(\blacksquare)^{2T}, R_3 + R_4, S_3 + S_4, T_1 + T_2, U_1 + U_2, X_1 + X_2, Y_1 + Y_2, Z_3 + Z_4]$ |
| $[(\blacksquare)^{2T}, R_2 + R_4, S_2 + S_4, T_1 + T_2, U_2 + U_4, X_2 + X_4, Y_1 + Y_2, Z_3 + Z_4]$ |
| $[(\blacksquare)^{2T}, 2R_4, 2S_4, T_1 + T_4, U_2 + U_4, X_2 + X_4, Y_1 + Y_4, Z_3 + Z_4]$           |
| $[(\blacksquare)^{2T}, R_1 + R_4, S_1 + S_4, T_1 + T_4, U_1 + U_2, X_1 + X_2, Y_1 + Y_4, Z_3 + Z_4]$ |
| $[(\blacksquare)^{2T}, R_2 + R_3, S_2 + S_3, T_2 + T_3, U_1 + U_2, X_1 + X_2, Y_2 + Y_3, Z_3 + Z_4]$ |
| $[(\blacksquare)^{2T}, 2R_2, 2S_2, T_2 + T_3, U_2 + U_4, X_2 + X_4, Y_2 + Y_3, Z_3 + Z_4]$           |
| $[(\blacksquare)^{2T}, R_1 + R_2, S_1 + S_2, T_1 + T_2, U_1 + U_2, X_1 + X_2, Y_1 + Y_2, Z_3 + Z_4]$ |
| $[(\blacksquare)^{2T}, R_2 + R_4, S_2 + S_4, T_3 + T_4, U_2 + U_4, X_2 + X_4, Y_3 + Y_4, Z_3 + Z_4]$ |
| $[(\blacksquare)^{2T}, R_1 + R_2, S_1 + S_2, T_3 + T_4, U_1 + U_2, X_1 + X_2, Y_3 + Y_4, Z_3 + Z_4]$ |
| $[(\blacksquare)^{2T}, R_3 + R_4, S_3 + S_4, T_3 + T_4, U_1 + U_2, X_1 + X_2, Y_3 + Y_4, Z_3 + Z_4]$ |

---

2nd minimal solution:  $\mu_2^T = 3$  (208 symmetry vectors)

Space group 26 ( $\mathbb{Z}_1$ )

1st minimal solution:  $\mu_1^T = 4$  (3 symmetry vectors)

| $\mathbf{n}^T$                                                                                                                                                                         |
|----------------------------------------------------------------------------------------------------------------------------------------------------------------------------------------|
| $[(\blacksquare)^{2T} + \Gamma_1 + \Gamma_2, 2R_2R_4, 2S_2 + 2S_4, T_1T_3 + T_2T_4, 2U_2U_4, 2X_2 + 2X_4, Y_1 + Y_2 + Y_3 + Y_4, Z_1Z_3 + Z_2Z_4]$                                     |
| $[(\blacksquare)^{2T} + \Gamma_1 + \Gamma_2, R_1R_3 + R_2R_4, S_1 + S_2 + S_3 + S_4, T_1T_3 + T_2T_4, U_1U_3 + U_2U_4, X_1 + X_2 + X_3 + X_4, Y_1 + Y_2 + Y_3 + Y_4, Z_1Z_3 + Z_2Z_4]$ |
| $[(\blacksquare)^{2T} + \Gamma_1 + \Gamma_2, 2R_1R_3, 2S_1 + 2S_3, T_1T_3 + T_2T_4, 2U_1U_3, 2X_1 + 2X_3, Y_1 + Y_2 + Y_3 + Y_4, Z_1Z_3 + Z_2Z_4]$                                     |

2nd minimal solution:  $\mu_2^T = 6$  (8 symmetry vectors)

Space group 27 ( $\mathbb{Z}_2$ )

1st minimal solution:  $\mu_1^T = 2$  (8 symmetry vectors)

| $\mathbf{n}^T$                                                                           | $\mathbf{v}^T \in \mathbb{Z}_2$ |
|------------------------------------------------------------------------------------------|---------------------------------|
| $[(\blacksquare)^{2T}, R_3R_4, S_3 + S_4, T_3T_4, U_3U_4, X_3 + X_4, Y_3 + Y_4, Z_3Z_4]$ | trivial                         |
| $[(\blacksquare)^{2T}, R_3R_4, S_3 + S_4, T_3T_4, U_1U_2, X_1 + X_2, Y_3 + Y_4, Z_3Z_4]$ | 1                               |
| $[(\blacksquare)^{2T}, R_3R_4, S_3 + S_4, T_1T_2, U_3U_4, X_3 + X_4, Y_1 + Y_2, Z_3Z_4]$ | 1                               |
| $[(\blacksquare)^{2T}, R_3R_4, S_3 + S_4, T_1T_2, U_1U_2, X_1 + X_2, Y_1 + Y_2, Z_3Z_4]$ | trivial                         |
| $[(\blacksquare)^{2T}, R_1R_2, S_1 + S_2, T_3T_4, U_3U_4, X_3 + X_4, Y_3 + Y_4, Z_3Z_4]$ | 1                               |
| $[(\blacksquare)^{2T}, R_1R_2, S_1 + S_2, T_3T_4, U_1U_2, X_1 + X_2, Y_3 + Y_4, Z_3Z_4]$ | trivial                         |
| $[(\blacksquare)^{2T}, R_1R_2, S_1 + S_2, T_1T_2, U_3U_4, X_3 + X_4, Y_1 + Y_2, Z_3Z_4]$ | trivial                         |
| $[(\blacksquare)^{2T}, R_1R_2, S_1 + S_2, T_1T_2, U_1U_2, X_1 + X_2, Y_1 + Y_2, Z_3Z_4]$ | 1                               |

2nd minimal solution:  $\mu_2^T = 4$  (54 symmetry vectors)

Space group 28 ( $\mathbb{Z}_1$ )

1st minimal solution:  $\mu_1^T = 2$  (2 symmetry vectors)

| $\mathbf{n}^T$                                                               |
|------------------------------------------------------------------------------|
| $[(\blacksquare)^{2T}, R_1, S_1, T_1 + T_2, U_1, X_1, Y_1 + Y_2, Z_3 + Z_4]$ |
| $[(\blacksquare)^{2T}, R_1, S_1, T_3 + T_4, U_1, X_1, Y_3 + Y_4, Z_3 + Z_4]$ |

2nd minimal solution:  $\mu_2^T = 4$  (10 symmetry vectors)

Space group 29 ( $\mathbb{Z}_1$ )

1st minimal solution:  $\mu_1^T = 4$  (1 symmetry vector)

| $\mathbf{n}^T$                                                                                                                     |
|------------------------------------------------------------------------------------------------------------------------------------|
| $[(\blacksquare)^{2T} + \Gamma_1 + \Gamma_2, R_1R_1, 2S_1, T_1T_4 + T_2T_3, U_1U_1, 2X_1, Y_1 + Y_2 + Y_3 + Y_4, Z_1Z_4 + Z_2Z_3]$ |

2nd minimal solution:  $\mu_2^T = 8$  (1 symmetry vector)

Space group 30 ( $\mathbb{Z}_1$ )

1st minimal solution:  $\mu_1^T = 2$  (2 symmetry vectors)

|                                                                          |
|--------------------------------------------------------------------------|
| $\mathbf{n}^T$                                                           |
| $[(\blacksquare)^{2T}, R_1, S_1, T_1, U_3 U_4, X_3 + X_4, Y_1, Z_3 Z_4]$ |
| $[(\blacksquare)^{2T}, R_1, S_1, T_1, U_1 U_2, X_1 + X_2, Y_1, Z_3 Z_4]$ |

2nd minimal solution:  $\mu_2^T = 4$  (6 symmetry vectors)

Space group 31 ( $\mathbb{Z}_1$ )

1st minimal solution:  $\mu_1^T = 4$  (1 symmetry vector)

|                                                                                                                                    |
|------------------------------------------------------------------------------------------------------------------------------------|
| $\mathbf{n}^T$                                                                                                                     |
| $[(\blacksquare)^{2T} + \Gamma_1 + \Gamma_2, 2R_1, 2S_1, T_1 T_3 + T_2 T_4, 2U_1, 2X_1, Y_1 + Y_2 + Y_3 + Y_4, Z_1 Z_3 + Z_2 Z_4]$ |

2nd minimal solution:  $\mu_2^T = 6$  (2 symmetry vectors)

Space group 32 ( $\mathbb{Z}_1$ )

1st minimal solution:  $\mu_1^T = 2$  (2 symmetry vectors)

|                                                                          |
|--------------------------------------------------------------------------|
| $\mathbf{n}^T$                                                           |
| $[(\blacksquare)^{2T}, R_3 R_4, S_3 S_4, T_1, U_1, X_1, Y_1, Z_3 + Z_4]$ |
| $[(\blacksquare)^{2T}, R_1 R_2, S_1 S_2, T_1, U_1, X_1, Y_1, Z_3 + Z_4]$ |

2nd minimal solution:  $\mu_2^T = 4$  (6 symmetry vectors)

Space group 33 ( $\mathbb{Z}_1$ )

1st minimal solution:  $\mu_1^T = 4$  (1 symmetry vector)

|                                                                                                                                   |
|-----------------------------------------------------------------------------------------------------------------------------------|
| $\mathbf{n}^T$                                                                                                                    |
| $[(\blacksquare)^{2T} + \Gamma_1 + \Gamma_2, R_1 R_3 + R_2 R_4, S_1 S_2 + S_3 S_4, 2T_1, U_1 U_1, 2X_1, 2Y_1, Z_1 Z_4 + Z_2 Z_3]$ |

2nd minimal solution:  $\mu_2^T = 8$  (1 symmetry vector)

Space group 34 ( $\mathbb{Z}_1$ )

1st minimal solution:  $\mu_1^T = 2$  (2 symmetry vectors)

| $\mathbf{n}^T$                                                           |
|--------------------------------------------------------------------------|
| $[(\blacksquare)^{2T}, R_3 + R_4, S_3 S_4, T_1, U_1, X_1, Y_1, Z_3 Z_4]$ |
| $[(\blacksquare)^{2T}, R_1 + R_2, S_1 S_2, T_1, U_1, X_1, Y_1, Z_3 Z_4]$ |

2nd minimal solution:  $\mu_2^T = 4$  (6 symmetry vectors)

Space group 35 ( $\mathbb{Z}_1$ )

1st minimal solution:  $\mu_1^T = 2$  (6 symmetry vectors)

| $\mathbf{n}^T$                                                                 |
|--------------------------------------------------------------------------------|
| $[(\blacksquare)^{2T}, T_3 + T_4, Y_3 + Y_4, Z_3 + Z_4, 2R_2, 2S_2]$           |
| $[(\blacksquare)^{2T}, T_3 + T_4, Y_3 + Y_4, Z_3 + Z_4, R_1 + R_2, S_1 + S_2]$ |
| $[(\blacksquare)^{2T}, T_3 + T_4, Y_3 + Y_4, Z_3 + Z_4, 2R_1, 2S_1]$           |
| $[(\blacksquare)^{2T}, T_1 + T_2, Y_1 + Y_2, Z_3 + Z_4, 2R_2, 2S_2]$           |
| $[(\blacksquare)^{2T}, T_1 + T_2, Y_1 + Y_2, Z_3 + Z_4, R_1 + R_2, S_1 + S_2]$ |
| $[(\blacksquare)^{2T}, T_1 + T_2, Y_1 + Y_2, Z_3 + Z_4, 2R_1, 2S_1]$           |

2nd minimal solution:  $\mu_2^T = 3$  (32 symmetry vectors)

Space group 36 ( $\mathbb{Z}_1$ )

1st minimal solution:  $\mu_1^T = 4$  (1 symmetry vector)

| $\mathbf{n}^T$                                                                                                                    |
|-----------------------------------------------------------------------------------------------------------------------------------|
| $[(\blacksquare)^{2T} + \Gamma_1 + \Gamma_2, T_1 T_3 + T_2 T_4, Y_1 + Y_2 + Y_3 + Y_4, Z_1 Z_3 + Z_2 Z_4, 2R_1 R_2, 2S_1 + 2S_2]$ |

2nd minimal solution:  $\mu_2^T = 6$  (2 symmetry vectors)

Space group 37 ( $\mathbb{Z}_2$ )

1st minimal solution:  $\mu_1^T = 2$  (6 symmetry vectors)

| $\mathbf{n}^T$                                                             | $\mathbf{v}^T \in \mathbb{Z}_2$ |
|----------------------------------------------------------------------------|---------------------------------|
| $[(\blacksquare)^{2T}, T_1 T_2, Y_1 + Y_2, Z_3 Z_4, 2R_2, 2S_2]$           | 1                               |
| $[(\blacksquare)^{2T}, T_3 T_4, Y_3 + Y_4, Z_3 Z_4, 2R_2, 2S_2]$           | trivial                         |
| $[(\blacksquare)^{2T}, T_1 T_2, Y_1 + Y_2, Z_3 Z_4, R_1 + R_2, S_1 + S_2]$ | trivial                         |
| $[(\blacksquare)^{2T}, T_3 T_4, Y_3 + Y_4, Z_3 Z_4, R_1 + R_2, S_1 + S_2]$ | 1                               |
| $[(\blacksquare)^{2T}, T_1 T_2, Y_1 + Y_2, Z_3 Z_4, 2R_1, 2S_1]$           | 1                               |
| $[(\blacksquare)^{2T}, T_3 T_4, Y_3 + Y_4, Z_3 Z_4, 2R_1, 2S_1]$           | trivial                         |

2nd minimal solution:  $\mu_2^T = 4$  (30 symmetry vectors)

Space group 38 ( $\mathbb{Z}_1$ )

1st minimal solution:  $\mu_1^T = 2$  (4 symmetry vectors)

| $\mathbf{n}^T$                                                                 |
|--------------------------------------------------------------------------------|
| $[(\blacksquare)^{2T}, T_3 + T_4, Y_3 + Y_4, Z_3 + Z_4, R_1 + R_2, S_1 + S_2]$ |
| $[(\blacksquare)^{2T}, T_1 + T_4, Y_3 + Y_4, Z_1 + Z_4, 2R_1, S_1 + S_2]$      |
| $[(\blacksquare)^{2T}, T_2 + T_3, Y_3 + Y_4, Z_2 + Z_3, 2R_2, S_1 + S_2]$      |
| $[(\blacksquare)^{2T}, T_1 + T_2, Y_3 + Y_4, Z_1 + Z_2, R_1 + R_2, S_1 + S_2]$ |

2nd minimal solution:  $\mu_2^T = 3$  (24 symmetry vectors)

Space group 39 ( $\mathbb{Z}_1$ )

1st minimal solution:  $\mu_1^T = 2$  (2 symmetry vectors)

| $\mathbf{n}^T$                                                             |
|----------------------------------------------------------------------------|
| $[(\blacksquare)^{2T}, T_1 + T_2, Y_3 + Y_4, Z_1 + Z_2, R_1 R_2, S_1 S_2]$ |
| $[(\blacksquare)^{2T}, T_3 + T_4, Y_3 + Y_4, Z_3 + Z_4, R_1 R_2, S_1 S_2]$ |

2nd minimal solution:  $\mu_2^T = 4$  (10 symmetry vectors)

Space group 40 ( $\mathbb{Z}_1$ )

1st minimal solution:  $\mu_1^T = 2$  (1 symmetry vector)

| $\mathbf{n}^T$                                                     |
|--------------------------------------------------------------------|
| $[(\blacksquare)^{2T}, T_1, Y_3 + Y_4, Z_1, R_1 + R_2, S_1 + S_2]$ |

2nd minimal solution:  $\mu_2^T = 4$  (4 symmetry vectors)

Space group 41 ( $\mathbb{Z}_1$ )

1st minimal solution:  $\mu_1^T = 2$  (1 symmetry vector)

| $\mathbf{n}^T$                                                 |
|----------------------------------------------------------------|
| $[(\blacksquare)^{2T}, T_1, Y_3 + Y_4, Z_1, R_1 R_2, S_1 S_2]$ |

2nd minimal solution:  $\mu_2^T = 4$  (2 symmetry vectors)

Space group 42 ( $\mathbb{Z}_1$ )

1st minimal solution:  $\mu_1^T = 2$  (2 symmetry vectors)

| $\mathbf{n}^T$                                                 |
|----------------------------------------------------------------|
| $[(\blacksquare)^{2T}, T_3 + T_4, Y_3 + Y_4, Z_3 + Z_4, 2L_1]$ |
| $[(\blacksquare)^{2T}, T_1 + T_2, Y_1 + Y_2, Z_3 + Z_4, 2L_1]$ |

2nd minimal solution:  $\mu_2^T = 3$  (8 symmetry vectors)

Space group 43 ( $\mathbb{Z}_1$ )

1st minimal solution:  $\mu_1^T = 2$  (1 symmetry vector)

| $\mathbf{n}^T$                                   |
|--------------------------------------------------|
| $[(\blacksquare)^{2T}, T_1, Y_1, Z_3 Z_4, 2L_1]$ |

2nd minimal solution:  $\mu_2^T = 4$  (2 symmetry vectors)

Space group 44 ( $\mathbb{Z}_1$ )

1st minimal solution:  $\mu_1^T = 2$  (3 symmetry vectors)

| $\mathbf{n}^T$                                                                 |
|--------------------------------------------------------------------------------|
| $[(\blacksquare)^{2T}, X_3 + X_4, R_1 + R_2, S_1 + S_2, 2T_2, 2W_2]$           |
| $[(\blacksquare)^{2T}, X_3 + X_4, R_1 + R_2, S_1 + S_2, T_1 + T_2, W_1 + W_2]$ |
| $[(\blacksquare)^{2T}, X_3 + X_4, R_1 + R_2, S_1 + S_2, 2T_1, 2W_1]$           |

2nd minimal solution:  $\mu_2^T = 3$  (16 symmetry vectors)

Space group 45 ( $\mathbb{Z}_1$ )

1st minimal solution:  $\mu_1^T = 2$  (2 symmetry vectors)

| $\mathbf{n}^T$                                                      |
|---------------------------------------------------------------------|
| $[(\blacksquare)^{2T}, X_3 + X_4, R_1 R_2, S_1 S_2, 2T_2, W_2 W_2]$ |
| $[(\blacksquare)^{2T}, X_3 + X_4, R_1 R_2, S_1 S_2, 2T_1, W_1 W_1]$ |

2nd minimal solution:  $\mu_2^T = 4$  (6 symmetry vectors)



Space group 46 ( $\mathbb{Z}_1$ )

1st minimal solution:  $\mu_1^T = 2$  (1 symmetry vector)

$$\frac{\mathbf{n}^T}{[(\bullet)^{2T}, X_3 + X_4, R_1 R_2, S_1 + S_2, T_1 + T_2, W_1 W_2]}$$

2nd minimal solution:  $\mu_2^T = 4$  (4 symmetry vectors)

Space group 47 ( $\mathbb{Z}_1$ )

1st minimal solution:  $\mu_1^T = 2$  (56 symmetry vectors)

$$\frac{\mathbf{n}^T}{\begin{aligned} &[(\bullet)^{2T}, R_3^+ + R_4^-, S_3^+ + S_4^-, T_1^- + T_4^-, U_2^- + U_4^-, X_2^- + X_4^-, Y_2^+ + Y_3^+, Z_4^+ + Z_4^-] \\ &[(\bullet)^{2T}, R_1^- + R_4^-, S_1^- + S_4^-, T_1^- + T_4^-, U_4^+ + U_4^-, X_4^+ + X_4^-, Y_2^+ + Y_3^+, Z_4^+ + Z_4^-] \\ &[(\bullet)^{2T}, 2R_3^+, S_3^+ + S_4^-, T_1^- + T_3^+, U_2^- + U_3^+, X_2^- + X_4^-, Y_2^+ + Y_3^+, Z_3^+ + Z_4^+] \\ &[(\bullet)^{2T}, R_3^+ + R_4^-, S_4^+ + S_4^-, T_1^- + T_2^-, U_3^+ + U_4^+, X_4^+ + X_4^-, Y_2^+ + Y_2^-, Z_3^+ + Z_4^+] \\ &[(\bullet)^{2T}, R_2^- + R_3^+, S_2^- + S_4^-, T_1^- + T_2^-, U_2^- + U_3^+, X_2^- + X_4^-, Y_2^+ + Y_2^-, Z_3^+ + Z_4^+] \\ &[(\bullet)^{2T}, R_1^- + R_3^+, S_1^- + S_4^-, T_1^- + T_3^+, U_3^+ + U_4^+, X_4^+ + X_4^-, Y_2^+ + Y_3^+, Z_3^+ + Z_4^+] \\ &[(\bullet)^{2T}, R_2^- + R_3^+, S_2^- + S_3^+, T_1^- + T_4^-, U_2^+ + U_2^-, X_2^+ + X_2^-, Y_2^+ + Y_3^+, Z_4^+ + Z_4^-] \\ &[(\bullet)^{2T}, R_1^- + R_2^+, S_1^- + S_2^+, T_1^- + T_4^-, U_2^+ + U_4^+, X_2^+ + X_4^+, Y_2^+ + Y_3^+, Z_4^+ + Z_4^-] \\ &[(\bullet)^{2T}, R_1^- + R_3^+, S_2^- + S_3^+, T_1^- + T_3^+, U_1^- + U_2^-, X_2^- + X_2^-, Y_2^+ + Y_3^+, Z_3^+ + Z_4^+] \\ &[(\bullet)^{2T}, R_1^- + R_4^+, S_2^- + S_4^+, T_1^- + T_2^-, U_1^- + U_4^+, X_2^- + X_4^+, Y_2^+ + Y_2^-, Z_3^+ + Z_4^+] \\ &[(\bullet)^{2T}, R_1^- + R_2^-, S_2^- + S_2^-, T_1^- + T_2^-, U_1^- + U_2^-, X_2^- + X_2^-, Y_2^+ + Y_2^-, Z_3^+ + Z_4^+] \\ &[(\bullet)^{2T}, 2R_1^-, S_1^- + S_2^-, T_1^- + T_3^+, U_1^- + U_4^+, X_2^- + X_4^+, Y_2^+ + Y_3^+, Z_3^+ + Z_4^+] \\ &[(\bullet)^{2T}, R_1^- + R_3^-, S_2^- + S_4^+, T_1^- + T_1^-, U_2^+ + U_4^+, X_2^+ + X_4^+, Y_2^+ + Y_2^-, Z_4^+ + Z_4^-] \\ &[(\bullet)^{2T}, R_1^- + R_3^+, S_2^- + S_4^-, T_1^- + T_1^-, U_2^- + U_4^-, X_2^- + X_4^-, Y_2^+ + Y_2^-, Z_4^+ + Z_4^-] \\ &[(\bullet)^{2T}, 2R_4^-, S_3^+ + S_4^-, T_2^+ + T_4^-, U_1^+ + U_4^-, X_2^- + X_4^-, Y_2^+ + Y_3^+, Z_3^- + Z_4^-] \\ &[(\bullet)^{2T}, R_3^- + R_4^-, S_3^- + S_4^-, T_2^+ + T_3^+, U_1^+ + U_3^+, X_2^- + X_4^-, Y_2^+ + Y_3^+, Z_3^- + Z_3^-] \\ &[(\bullet)^{2T}, R_2^- + R_4^-, S_2^- + S_4^-, T_2^+ + T_2^-, U_1^+ + U_3^+, X_2^- + X_4^-, Y_2^+ + Y_2^-, Z_3^- + Z_3^-] \\ &[(\bullet)^{2T}, R_2^- + R_4^-, S_2^- + S_3^+, T_2^+ + T_4^-, U_1^+ + U_2^+, X_2^+ + X_2^-, Y_2^+ + Y_3^+, Z_3^- + Z_4^-] \\ &[(\bullet)^{2T}, R_1^- + R_4^-, S_2^- + S_4^-, T_1^+ + T_2^+, U_1^+ + U_4^-, X_2^- + X_4^-, Y_2^+ + Y_2^-, Z_3^- + Z_4^-] \\ &[(\bullet)^{2T}, R_2^- + R_4^-, S_1^+ + S_3^+, T_4^+ + T_4^-, U_2^- + U_4^-, X_2^- + X_4^-, Y_3^+ + Y_3^-, Z_4^+ + Z_4^-] \\ &[(\bullet)^{2T}, R_2^- + R_3^-, S_1^+ + S_3^+, T_3^+ + T_4^+, U_2^- + U_3^+, X_2^- + X_4^-, Y_3^+ + Y_3^-, Z_3^+ + Z_4^+] \\ &[(\bullet)^{2T}, R_2^- + R_4^-, S_1^+ + S_4^+, T_2^- + T_4^+, U_3^+ + U_4^+, X_4^+ + X_4^-, Y_2^- + Y_3^-, Z_3^+ + Z_4^+] \\ &[(\bullet)^{2T}, 2R_2^-, S_1^+ + S_2^-, T_2^- + T_4^+, U_2^- + U_3^+, X_2^- + X_4^-, Y_2^- + Y_3^-, Z_3^+ + Z_4^+] \\ &[(\bullet)^{2T}, R_1^- + R_2^-, S_1^+ + S_1^-, T_3^+ + T_4^+, U_3^+ + U_4^+, X_4^+ + X_4^-, Y_3^+ + Y_3^-, Z_3^+ + Z_4^+] \\ &[(\bullet)^{2T}, R_1^+ + R_2^-, S_1^+ + S_2^-, T_1^+ + T_4^+, U_2^- + U_4^-, X_2^- + X_4^-, Y_2^- + Y_3^-, Z_4^+ + Z_4^-] \\ &[(\bullet)^{2T}, R_1^+ + R_4^-, S_1^+ + S_3^+, T_3^- + T_4^-, U_1^+ + U_4^-, X_2^- + X_4^-, Y_3^+ + Y_3^-, Z_3^- + Z_4^-] \\ &[(\bullet)^{2T}, R_1^+ + R_3^+, S_1^+ + S_3^+, T_3^+ + T_3^-, U_1^+ + U_3^+, X_2^- + X_4^-, Y_3^+ + Y_3^-, Z_3^+ + Z_3^-] \\ &[(\bullet)^{2T}, R_1^+ + R_2^-, S_1^+ + S_2^-, T_2^- + T_3^-, U_1^+ + U_3^+, X_2^- + X_4^-, Y_2^- + Y_3^-, Z_3^+ + Z_3^-] \\ &[(\bullet)^{2T}, 2R_1^+, S_1^+ + S_2^-, T_1^+ + T_3^-, U_1^+ + U_4^-, X_2^- + X_4^-, Y_2^- + Y_3^-, Z_3^- + Z_4^-] \\ &[(\bullet)^{2T}, R_2^- + R_4^-, S_1^- + S_4^-, T_2^+ + T_4^-, U_3^- + U_4^-, X_4^+ + X_4^-, Y_2^+ + Y_3^+, Z_3^- + Z_4^-] \\ &[(\bullet)^{2T}, R_2^- + R_3^-, S_1^+ + S_4^+, T_2^- + T_3^-, U_3^+ + U_3^-, X_4^+ + X_4^-, Y_2^- + Y_3^-, Z_3^+ + Z_3^-] \\ &[(\bullet)^{2T}, R_2^- + R_3^+, S_1^- + S_4^-, T_2^+ + T_3^+, U_3^+ + U_3^-, X_4^+ + X_4^-, Y_2^+ + Y_3^+, Z_3^+ + Z_3^-] \\ &[(\bullet)^{2T}, 2R_2^+, S_1^- + S_2^+, T_2^+ + T_4^-, U_2^+ + U_3^-, X_2^+ + X_4^+, Y_2^+ + Y_3^+, Z_3^- + Z_4^-] \\ &[(\bullet)^{2T}, R_1^- + R_2^+, S_1^- + S_2^+, T_2^+ + T_3^+, U_1^- + U_3^-, X_2^+ + X_4^+, Y_2^+ + Y_3^+, Z_3^+ + Z_3^-] \\ &[(\bullet)^{2T}, R_3^+ + R_4^+, S_3^+ + S_3^-, T_3^+ + T_4^+, U_1^- + U_2^-, X_2^- + X_2^-, Y_3^+ + Y_3^-, Z_3^+ + Z_4^+] \\ &[(\bullet)^{2T}, 2R_4^+, S_3^- + S_4^+, T_2^- + T_4^+, U_1^- + U_4^+, X_2^- + X_4^+, Y_2^- + Y_3^-, Z_3^+ + Z_4^+] \end{aligned}}$$

... continued on next page

... continued from previous page

$$\begin{array}{l}
[(\blacksquare)^{2T}, R_2^- + R_4^+, S_2^- + S_3^-, T_2^- + T_4^+, U_1^- + U_2^-, X_2^+ + X_2^-, Y_2^- + Y_3^-, Z_3^+ + Z_4^-] \\
[(\blacksquare)^{2T}, R_1^- + R_4^+, S_1^- + S_3^-, T_3^+ + T_4^+, U_1^- + U_4^+, X_2^+ + X_4^+, Y_3^+ + Y_3^-, Z_3^+ + Z_4^-] \\
[(\blacksquare)^{2T}, R_3^- + R_4^-, S_3^+ + S_3^-, T_3^- + T_4^-, U_1^+ + U_2^+, X_2^+ + X_2^-, Y_3^+ + Y_3^-, Z_3^- + Z_4^-] \\
[(\blacksquare)^{2T}, R_3^- + R_4^+, S_3^- + S_4^+, T_1^+ + T_4^+, U_2^+ + U_4^+, X_2^+ + X_4^+, Y_2^- + Y_3^-, Z_4^+ + Z_4^-] \\
[(\blacksquare)^{2T}, 2R_3^-, S_3^- + S_4^+, T_1^+ + T_3^-, U_2^+ + U_3^-, X_2^+ + X_4^+, Y_2^- + Y_3^-, Z_3^- + Z_4^-] \\
[(\blacksquare)^{2T}, R_3^- + R_4^-, S_4^+ + S_4^-, T_1^+ + T_2^+, U_3^- + U_4^-, X_4^+ + X_4^-, Y_2^+ + Y_2^-, Z_3^- + Z_4^-] \\
[(\blacksquare)^{2T}, R_3^- + R_4^+, S_3^- + S_4^+, T_2^- + T_3^-, U_1^- + U_3^-, X_2^+ + X_4^+, Y_2^- + Y_3^-, Z_3^+ + Z_3^-] \\
[(\blacksquare)^{2T}, R_2^- + R_3^-, S_2^- + S_3^-, T_1^+ + T_4^+, U_2^+ + U_2^-, X_2^+ + X_2^-, Y_2^- + Y_3^-, Z_4^+ + Z_4^-] \\
[(\blacksquare)^{2T}, R_2^+ + R_3^-, S_2^+ + S_4^+, T_1^+ + T_2^+, U_2^+ + U_3^-, X_2^+ + X_4^+, Y_2^+ + Y_2^-, Z_3^- + Z_4^-] \\
[(\blacksquare)^{2T}, R_2^+ + R_4^+, S_2^+ + S_4^+, T_2^+ + T_2^-, U_1^- + U_3^-, X_2^+ + X_4^+, Y_2^+ + Y_2^-, Z_3^+ + Z_3^-] \\
[(\blacksquare)^{2T}, R_2^+ + R_4^+, S_1^- + S_3^-, T_4^+ + T_4^-, U_2^+ + U_4^+, X_2^+ + X_4^+, Y_3^+ + Y_3^-, Z_4^+ + Z_4^-] \\
[(\blacksquare)^{2T}, R_2^+ + R_3^-, S_1^- + S_3^-, T_3^- + T_4^-, U_2^+ + U_3^-, X_2^+ + X_4^+, Y_3^+ + Y_3^-, Z_3^- + Z_4^-] \\
[(\blacksquare)^{2T}, R_1^- + R_3^-, S_1^- + S_3^-, T_3^+ + T_3^-, U_1^- + U_3^-, X_2^+ + X_4^+, Y_3^+ + Y_3^-, Z_3^+ + Z_3^-] \\
[(\blacksquare)^{2T}, R_1^+ + R_3^-, S_2^- + S_3^-, T_1^+ + T_3^-, U_1^+ + U_2^+, X_2^+ + X_2^-, Y_2^- + Y_3^-, Z_3^- + Z_4^-] \\
[(\blacksquare)^{2T}, R_1^+ + R_4^+, S_2^- + S_3^-, T_2^- + T_3^-, U_1^+ + U_1^-, X_2^+ + X_2^-, Y_2^- + Y_3^-, Z_3^+ + Z_3^-] \\
[(\blacksquare)^{2T}, R_1^+ + R_4^+, S_1^+ + S_4^+, T_1^+ + T_4^+, U_4^+ + U_4^-, X_4^+ + X_4^-, Y_2^- + Y_3^-, Z_4^+ + Z_4^-] \\
[(\blacksquare)^{2T}, R_1^+ + R_3^-, S_1^+ + S_4^+, T_1^+ + T_3^-, U_3^- + U_4^-, X_4^+ + X_4^-, Y_2^- + Y_3^-, Z_3^- + Z_4^-] \\
[(\blacksquare)^{2T}, R_1^+ + R_2^+, S_2^+ + S_2^-, T_1^+ + T_2^+, U_1^+ + U_2^+, X_2^+ + X_2^-, Y_2^+ + Y_2^-, Z_3^- + Z_4^-] \\
[(\blacksquare)^{2T}, R_1^+ + R_2^+, S_1^+ + S_1^-, T_3^- + T_4^-, U_3^- + U_4^-, X_4^+ + X_4^-, Y_3^+ + Y_3^-, Z_3^- + Z_4^-]
\end{array}$$

Skipped higher-order solutions...

Space group 48 ( $\mathbb{Z}_2$ )

1st minimal solution:  $\mu_1^T = 2$  (4 symmetry vectors & filling-enforced topology)

| $\mathbf{n}^T$                                                       | $\mathbf{v}^T \in \mathbb{Z}_2$ |
|----------------------------------------------------------------------|---------------------------------|
| $[(\blacksquare)^{2T}, R_4^+ + R_4^-, S_2, T_2, U_1, X_2, Y_2, Z_2]$ | 1                               |
| $[(\blacksquare)^{2T}, R_3^+ + R_3^-, S_2, T_1, U_2, X_2, Y_2, Z_2]$ | 1                               |
| $[(\blacksquare)^{2T}, R_2^+ + R_2^-, S_1, T_2, U_2, X_2, Y_2, Z_2]$ | 1                               |
| $[(\blacksquare)^{2T}, R_1^+ + R_1^-, S_1, T_1, U_1, X_2, Y_2, Z_2]$ | 1                               |

2nd minimal solution:  $\mu_2^T = 4$  (48 symmetry vectors)

Space group 49 ( $\mathbb{Z}_2$ )

1st minimal solution:  $\mu_1^T = 2$  (4 symmetry vectors & filling-enforced topology)

| $\mathbf{n}^T$                                                                           | $\mathbf{v}^T \in \mathbb{Z}_2$ |
|------------------------------------------------------------------------------------------|---------------------------------|
| $[(\blacksquare)^{2T}, R_2, S_3^+ + S_3^-, T_2, U_1, X_2^+ + X_2^-, Y_3^+ + Y_3^-, Z_2]$ | 1                               |
| $[(\blacksquare)^{2T}, R_2, S_4^+ + S_4^-, T_1, U_2, X_4^+ + X_4^-, Y_2^+ + Y_2^-, Z_2]$ | 1                               |
| $[(\blacksquare)^{2T}, R_1, S_2^+ + S_2^-, T_1, U_1, X_2^+ + X_2^-, Y_2^+ + Y_2^-, Z_2]$ | 1                               |
| $[(\blacksquare)^{2T}, R_1, S_1^+ + S_1^-, T_2, U_2, X_4^+ + X_4^-, Y_3^+ + Y_3^-, Z_2]$ | 1                               |

2nd minimal solution:  $\mu_2^T = 4$  (284 symmetry vectors)

Space group 50 ( $\mathbb{Z}_2$ )

1st minimal solution:  $\mu_1^T = 2$  (4 symmetry vectors & filling-enforced topology)

| $\mathbf{n}^T$                                                       | $\mathbf{v}^T \in \mathbb{Z}_2$ |
|----------------------------------------------------------------------|---------------------------------|
| $[(\blacksquare)^{2T}, R_2, S_2, T_2, U_1, X_2, Y_2, Z_3^+ + Z_3^-]$ | 1                               |
| $[(\blacksquare)^{2T}, R_2, S_2, T_1, U_2, X_2, Y_2, Z_4^+ + Z_4^-]$ | 1                               |
| $[(\blacksquare)^{2T}, R_1, S_1, T_2, U_1, X_2, Y_2, Z_3^+ + Z_3^-]$ | 1                               |
| $[(\blacksquare)^{2T}, R_1, S_1, T_1, U_2, X_2, Y_2, Z_4^+ + Z_4^-]$ | 1                               |

2nd minimal solution:  $\mu_2^T = 4$  (54 symmetry vectors)

Space group 51 ( $\mathbb{Z}_1$ )

1st minimal solution:  $\mu_1^T = 4$  (44 symmetry vectors)

| $\mathbf{n}^T$                                                                                                                                                                                     |
|----------------------------------------------------------------------------------------------------------------------------------------------------------------------------------------------------|
| $[(\blacksquare)^{2T} + \Gamma_3^+ + \Gamma_3^-, R_1 + R_2, S_1 + S_2, T_1^+ + T_2^+ + T_3^+ + T_4^+, U_1 + U_2, X_1 + X_2, Y_2^+ + Y_2^- + Y_3^+ + Y_3^-, Z_3^+ + Z_3^- + Z_4^+ + Z_4^-]$         |
| $[(\blacksquare)^{2T} + \Gamma_3^+ + \Gamma_3^-, 2R_2, 2S_2, T_1^- + T_2^+ + T_3^+ + T_4^-, U_1 + U_2, X_1 + X_2, 2Y_2^+ + 2Y_3^+, Z_3^+ + Z_3^- + Z_4^+ + Z_4^-]$                                 |
| $[(\blacksquare)^{2T} + \Gamma_1^+ + \Gamma_3^-, 2R_2, 2S_2, T_2^+ + 2T_3^+ + T_4^-, U_1 + U_2, X_1 + X_2, Y_2^+ + 2Y_3^+ + Y_4^-, Z_2^- + Z_3^+ + Z_3^- + Z_4^-]$                                 |
| $[(\blacksquare)^{2T} + \Gamma_1^+ + \Gamma_3^-, R_1 + R_2, S_1 + S_2, T_1^+ + T_2^+ + T_2^- + T_3^+, U_1 + U_2, X_1 + X_2, Y_1^+ + Y_2^+ + Y_2^- + Y_3^+, Z_2^- + Z_3^+ + Z_3^- + Z_4^-]$         |
| $[(\blacksquare)^{2T} + \Gamma_1^+ + \Gamma_3^-, R_1 + R_2, S_1 + S_2, T_2^- + T_3^+ + T_3^- + T_4^-, U_1 + U_2, X_1 + X_2, Y_2^- + Y_3^+ + Y_3^- + Y_4^-, Z_2^- + Z_3^+ + Z_3^- + Z_4^-]$         |
| $[(\blacksquare)^{2T} + \Gamma_1^+ + \Gamma_3^-, R_1 + R_2, S_1 + S_2, T_1^+ + T_3^+ + T_4^+ + T_4^-, U_1 + U_2, X_1 + X_2, Y_2^- + Y_3^+ + Y_3^- + Y_4^-, Z_1^+ + Z_3^+ + Z_4^+ + Z_4^-]$         |
| $[(\blacksquare)^{2T} + \Gamma_1^+ + \Gamma_3^-, 2R_2, 2S_2, T_1^- + T_3^+ + 2T_4^-, U_1 + U_2, X_1 + X_2, Y_2^+ + 2Y_3^+ + Y_4^-, Z_1^+ + Z_3^+ + Z_4^+ + Z_4^-]$                                 |
| $[(\blacksquare)^{2T} + \Gamma_1^- + \Gamma_3^-, 2R_1, 2S_1, T_1^+ + T_3^- + 2T_4^+, U_1 + U_2, X_1 + X_2, Y_2^- + 2Y_3^- + Y_4^+, Z_1^- + Z_3^- + Z_4^+ + Z_4^-]$                                 |
| $[(\blacksquare)^{2T} + \Gamma_1^- + \Gamma_3^-, R_1 + R_2, S_1 + S_2, T_1^- + T_3^- + T_4^- + T_4^-, U_1 + U_2, X_1 + X_2, Y_2^- + Y_3^+ + Y_3^- + Y_4^+, Z_1^- + Z_3^- + Z_4^+ + Z_4^-]$         |
| $[(\blacksquare)^{2T} + \Gamma_1^- + \Gamma_3^-, R_1 + R_2, S_1 + S_2, T_2^+ + T_3^+ + T_3^- + T_4^+, U_1 + U_2, X_1 + X_2, Y_2^+ + Y_3^+ + Y_3^- + Y_4^+, Z_2^+ + Z_3^+ + Z_3^- + Z_4^+]$         |
| $[(\blacksquare)^{2T} + \Gamma_1^+ + \Gamma_1^-, R_1 + R_2, S_1 + S_2, T_3^+ + T_3^- + T_4^+ + T_4^-, U_1 + U_2, X_1 + X_2, Y_3^+ + Y_3^- + Y_4^+ + Y_4^-, Z_1^- + Z_2^- + Z_3^- + Z_4^-]$         |
| $[(\blacksquare)^{2T} + \Gamma_1^+ + \Gamma_1^-, 2R_1, 2S_1, T_1^+ + T_2^- + T_3^- + T_4^+, U_1 + U_2, X_1 + X_2, Y_1^+ + Y_2^- + Y_3^- + Y_4^+, Z_1^+ + Z_2^- + Z_3^- + Z_4^+]$                   |
| $[(\blacksquare)^{2T} + \Gamma_1^- + \Gamma_3^-, 2R_1, 2S_1, T_2^- + 2T_3^- + T_4^+, U_1 + U_2, X_1 + X_2, Y_2^- + 2Y_3^- + Y_4^+, Z_2^- + Z_3^- + Z_3^- + Z_4^+]$                                 |
| $[(\blacksquare)^{2T} + \Gamma_3^+ + \Gamma_3^-, 2S_1, 2S_1, T_1^+ + T_2^- + T_3^- + T_4^+, U_1 + U_2, X_1 + X_2, 2Y_2^- + 2Y_3^-, Z_3^+ + Z_3^- + Z_4^+ + Z_4^-]$                                 |
| $[(\blacksquare)^{2T} + \Gamma_3^+ + \Gamma_3^-, R_1 + R_2, S_1 + S_2, T_1^- + T_2^- + T_2^- + T_3^- + T_4^-, U_1 + U_2, X_1 + X_2, Y_2^+ + Y_2^- + Y_3^+ + Y_3^-, Z_3^+ + Z_3^- + Z_4^+ + Z_4^-]$ |
| $[(\blacksquare)^{2T} + \Gamma_1^+ + \Gamma_3^+, 2R_1, 2S_1, T_1^+ + 2T_2^- + T_3^-, U_1 + U_2, X_1 + X_2, Y_1^+ + 2Y_2^- + Y_3^-, Z_2^- + Z_3^+ + Z_3^- + Z_4^-]$                                 |
| $[(\blacksquare)^{2T} + \Gamma_1^- + \Gamma_3^-, R_1 + R_2, S_1 + S_2, T_1^+ + T_1^- + T_2^+ + T_4^+, U_1 + U_2, X_1 + X_2, Y_1^- + Y_2^+ + Y_2^- + Y_3^-, Z_1^- + Z_3^- + Z_4^+ + Z_4^-]$         |
| $[(\blacksquare)^{2T} + \Gamma_1^- + \Gamma_3^-, 2R_2, 2S_2, 2T_1^- + T_2^+ + T_4^-, U_1 + U_2, X_1 + X_2, Y_1^- + 2Y_2^+ + Y_3^+, Z_1^- + Z_3^- + Z_4^+ + Z_4^-]$                                 |
| $[(\blacksquare)^{2T} + \Gamma_1^- + \Gamma_3^-, 2R_2, 2S_2, T_1^- + 2T_2^+ + T_3^+, U_1 + U_2, X_1 + X_2, Y_1^- + 2Y_2^+ + Y_3^+, Z_2^+ + Z_3^+ + Z_3^- + Z_4^+]$                                 |
| $[(\blacksquare)^{2T} + \Gamma_1^+ + \Gamma_1^-, 2R_2, 2S_2, T_1^- + T_2^+ + T_3^+ + T_4^-, U_1 + U_2, X_1 + X_2, Y_1^- + Y_2^+ + Y_3^+ + Y_4^-, Z_1^- + Z_2^- + Z_3^- + Z_4^-]$                   |
| $[(\blacksquare)^{2T} + \Gamma_1^+ + \Gamma_1^-, R_1 + R_2, S_1 + S_2, T_1^+ + T_1^- + T_2^+ + T_2^-, U_1 + U_2, X_1 + X_2, Y_1^+ + Y_1^- + Y_2^+ + Y_2^-, Z_1^- + Z_2^- + Z_3^- + Z_4^-]$         |
| $[(\blacksquare)^{2T} + \Gamma_1^+ + \Gamma_1^-, 2R_2, 2S_2, 2T_2^+ + 2T_3^+, U_1 + U_2, X_1 + X_2, Y_1^- + Y_2^+ + Y_3^+ + Y_4^-, Z_2^+ + Z_2^- + Z_3^+ + Z_3^-]$                                 |
| $[(\blacksquare)^{2T} + \Gamma_1^+ + \Gamma_1^-, R_1 + R_2, S_1 + S_2, T_2^+ + T_2^- + T_3^+ + T_3^-, U_1 + U_2, X_1 + X_2, Y_1^+ + Y_2^+ + Y_3^+ + Y_4^+, Z_2^+ + Z_2^- + Z_3^+ + Z_3^-]$         |
| $[(\blacksquare)^{2T} + \Gamma_1^+ + \Gamma_1^-, R_1 + R_2, S_1 + S_2, T_1^+ + T_2^+ + T_3^+ + T_4^+, U_1 + U_2, X_1 + X_2, Y_1^+ + Y_2^+ + Y_3^+ + Y_4^+, Z_1^- + Z_2^- + Z_3^- + Z_4^-]$         |
| $[(\blacksquare)^{2T} + \Gamma_1^- + \Gamma_3^-, R_1 + R_2, S_1 + S_2, T_1^- + T_2^+ + T_2^- + T_3^-, U_1 + U_2, X_1 + X_2, Y_1^- + Y_2^+ + Y_2^- + Y_3^-, Z_2^+ + Z_3^+ + Z_3^- + Z_4^+]$         |
| $[(\blacksquare)^{2T} + \Gamma_1^+ + \Gamma_3^+, 2R_1, 2S_1, 2T_1^+ + T_2^- + T_4^+, U_1 + U_2, X_1 + X_2, Y_1^+ + 2Y_2^- + Y_3^-, Z_1^+ + Z_3^+ + Z_4^+ + Z_4^-]$                                 |
| $[(\blacksquare)^{2T} + \Gamma_1^+ + \Gamma_3^+, R_1 + R_2, S_1 + S_2, T_1^+ + T_1^- + T_2^- + T_4^-, U_1 + U_2, X_1 + X_2, Y_1^+ + Y_2^+ + Y_2^- + Y_3^+, Z_1^+ + Z_3^+ + Z_4^+ + Z_4^-]$         |
| $[(\blacksquare)^{2T} + \Gamma_1^+ + \Gamma_1^-, R_1 + R_2, S_1 + S_2, T_1^- + T_2^- + T_3^- + T_4^-, U_1 + U_2, X_1 + X_2, Y_1^- + Y_2^- + Y_3^- + Y_4^-, Z_1^- + Z_2^- + Z_3^- + Z_4^-]$         |
| $[(\blacksquare)^{2T} + \Gamma_1^+ + \Gamma_1^-, R_1 + R_2, S_1 + S_2, T_2^+ + T_2^- + T_3^+ + T_3^-, U_1 + U_2, X_1 + X_2, Y_1^- + Y_2^- + Y_3^- + Y_4^-, Z_2^+ + Z_2^- + Z_3^+ + Z_3^-]$         |
| $[(\blacksquare)^{2T} + \Gamma_1^+ + \Gamma_1^-, 2R_1, 2S_1, 2T_2^- + 2T_3^-, U_1 + U_2, X_1 + X_2, Y_1^+ + Y_2^- + Y_3^- + Y_4^+, Z_2^+ + Z_2^- + Z_3^+ + Z_3^-]$                                 |
| $[(\blacksquare)^{2T} + \Gamma_1^+ + \Gamma_1^-, R_1 + R_2, S_1 + S_2, T_1^+ + T_1^- + T_4^+ + T_4^-, U_1 + U_2, X_1 + X_2, Y_1^- + Y_2^- + Y_3^- + Y_4^-, Z_1^+ + Z_1^- + Z_4^+ + Z_4^-]$         |
| $[(\blacksquare)^{2T} + \Gamma_1^+ + \Gamma_1^-, R_1 + R_2, S_1 + S_2, T_1^+ + T_2^+ + T_3^+ + T_4^+, U_1 + U_2, X_1 + X_2, Y_1^- + Y_2^- + Y_3^- + Y_4^-, Z_1^- + Z_2^- + Z_3^- + Z_4^-]$         |
| $[(\blacksquare)^{2T} + \Gamma_1^+ + \Gamma_1^-, 2R_1, 2S_1, 2T_1^+ + 2T_4^+, U_1 + U_2, X_1 + X_2, Y_1^+ + Y_2^- + Y_3^- + Y_4^+, Z_1^+ + Z_1^- + Z_4^+ + Z_4^-]$                                 |
| $[(\blacksquare)^{2T} + \Gamma_1^+ + \Gamma_1^-, R_1 + R_2, S_1 + S_2, T_1^+ + T_2^+ + T_3^+ + T_4^+, U_1 + U_2, X_1 + X_2, Y_1^- + Y_2^- + Y_3^- + Y_4^-, Z_1^+ + Z_2^+ + Z_3^+ + Z_4^+]$         |

... continued on next page

... continued from previous page

---

|                                                                                                                                                                                            |
|--------------------------------------------------------------------------------------------------------------------------------------------------------------------------------------------|
| $[(\blacksquare)^{2T} + \Gamma_1^+ + \Gamma_1^-, 2R_1, 2S_1, T_1^+ + T_2^- + T_3^- + T_4^+, U_1 + U_2, X_1 + X_2, Y_1^+ + Y_2^- + Y_3^- + Y_4^+, Z_1^+ + Z_2^+ + Z_3^+ + Z_4^+]$           |
| $[(\blacksquare)^{2T} + \Gamma_1^+ + \Gamma_1^-, 2R_2, 2S_2, 2T_1^- + 2T_4^-, U_1 + U_2, X_1 + X_2, Y_1^- + Y_2^+ + Y_3^+ + Y_4^-, Z_1^+ + Z_1^- + Z_4^+ + Z_4^-]$                         |
| $[(\blacksquare)^{2T} + \Gamma_1^+ + \Gamma_1^-, R_1 + R_2, S_1 + S_2, T_1^- + T_2^- + T_3^- + T_4^-, U_1 + U_2, X_1 + X_2, Y_1^+ + Y_2^+ + Y_3^+ + Y_4^+, Z_1^- + Z_2^- + Z_3^- + Z_4^-]$ |
| $[(\blacksquare)^{2T} + \Gamma_1^+ + \Gamma_1^-, R_1 + R_2, S_1 + S_2, T_1^+ + T_1^- + T_4^+ + T_4^-, U_1 + U_2, X_1 + X_2, Y_1^+ + Y_2^+ + Y_3^+ + Y_4^+, Z_1^+ + Z_1^- + Z_4^+ + Z_4^-]$ |
| $[(\blacksquare)^{2T} + \Gamma_1^+ + \Gamma_1^-, 2R_2, 2S_2, T_1^- + T_2^+ + T_3^+ + T_4^-, U_1 + U_2, X_1 + X_2, Y_1^- + Y_2^+ + Y_3^+ + Y_4^-, Z_1^+ + Z_2^+ + Z_3^+ + Z_4^+]$           |
| $[(\blacksquare)^{2T} + \Gamma_1^+ + \Gamma_1^-, R_1 + R_2, S_1 + S_2, T_1^+ + T_2^+ + T_3^+ + T_4^+, U_1 + U_2, X_1 + X_2, Y_1^+ + Y_2^+ + Y_3^+ + Y_4^+, Z_1^+ + Z_2^+ + Z_3^+ + Z_4^+]$ |
| $[(\blacksquare)^{2T} + \Gamma_1^+ + \Gamma_1^-, R_1 + R_2, S_1 + S_2, T_1^- + T_2^- + T_3^- + T_4^-, U_1 + U_2, X_1 + X_2, Y_1^+ + Y_2^+ + Y_3^+ + Y_4^+, Z_1^+ + Z_2^+ + Z_3^+ + Z_4^+]$ |
| $[(\blacksquare)^{2T} + \Gamma_1^+ + \Gamma_1^-, R_1 + R_2, S_1 + S_2, T_1^- + T_2^- + T_3^- + T_4^-, U_1 + U_2, X_1 + X_2, Y_1^- + Y_2^- + Y_3^- + Y_4^-, Z_1^+ + Z_2^+ + Z_3^+ + Z_4^+]$ |
| $[(\blacksquare)^{2T} + \Gamma_1^+ + \Gamma_1^-, R_1 + R_2, S_1 + S_2, T_3^+ + T_3^- + T_4^+ + T_4^-, U_1 + U_2, X_1 + X_2, Y_3^+ + Y_3^- + Y_4^+ + Y_4^-, Z_1^+ + Z_2^+ + Z_3^+ + Z_4^+]$ |
| $[(\blacksquare)^{2T} + \Gamma_1^+ + \Gamma_1^-, R_1 + R_2, S_1 + S_2, T_1^+ + T_1^- + T_2^+ + T_2^-, U_1 + U_2, X_1 + X_2, Y_1^+ + Y_1^- + Y_2^+ + Y_2^-, Z_1^+ + Z_2^+ + Z_3^+ + Z_4^+]$ |

---

2nd minimal solution:  $\mu_2^T = 6$  (748 symmetry vectors)

Space group 52 ( $\mathbb{Z}_2$ )

1st minimal solution:  $\mu_1^T = 4$  (6 symmetry vectors)

| $\mathbf{n}^T$                                                                                                                   | $\mathbf{v}^T \in \mathbb{Z}_2$ |
|----------------------------------------------------------------------------------------------------------------------------------|---------------------------------|
| $[(\blacksquare)^{2T} + \Gamma_4^+ + \Gamma_4^-, R_1 + R_2, S_1 S_2, 2T_1^-, U_1 + U_2, 2X_2, Y_1 + Y_2, 2Z_2]$                  | trivial                         |
| $[(\blacksquare)^{2T} + \Gamma_4^+ + \Gamma_4^-, R_1 + R_2, S_1 S_2, T_1^+ + T_1^-, U_1 + U_2, 2X_2, Y_1 + Y_2, 2Z_2]$           | 1                               |
| $[(\blacksquare)^{2T} + \Gamma_4^+ + \Gamma_4^-, R_1 + R_2, S_1 S_2, 2T_1^+, U_1 + U_2, 2X_2, Y_1 + Y_2, 2Z_2]$                  | trivial                         |
| $[(\blacksquare)^{2T} + \Gamma_1^+ + \Gamma_1^-, R_1 + R_2, S_1 S_2, 2T_1^-, U_1 + U_2, X_1 + X_2, Y_1 + Y_2, Z_1 + Z_2]$        | trivial                         |
| $[(\blacksquare)^{2T} + \Gamma_1^+ + \Gamma_1^-, R_1 + R_2, S_1 S_2, T_1^+ + T_1^-, U_1 + U_2, X_1 + X_2, Y_1 + Y_2, Z_1 + Z_2]$ | 1                               |
| $[(\blacksquare)^{2T} + \Gamma_1^+ + \Gamma_1^-, R_1 + R_2, S_1 S_2, 2T_1^+, U_1 + U_2, X_1 + X_2, Y_1 + Y_2, Z_1 + Z_2]$        | trivial                         |

2nd minimal solution:  $\mu_2^T = 8$  (50 symmetry vectors)

Space group 53 ( $\mathbb{Z}_2$ )

1st minimal solution:  $\mu_1^T = 4$  (45 symmetry vectors)

| $\mathbf{n}^T$                                                                                                                                        | $\mathbf{v}^T \in \mathbb{Z}_2$ |
|-------------------------------------------------------------------------------------------------------------------------------------------------------|---------------------------------|
| $[(\blacksquare)^{2T} + \Gamma_2^+ + \Gamma_2^-, 2R_1^-, S_1 + S_2, T_1 + T_2, 2U_1^+, 2X_2, Y_2^+ + Y_2^- + Y_3^+ + Y_3^-, Z_1 + Z_2]$               | 1                               |
| $[(\blacksquare)^{2T} + \Gamma_2^+ + \Gamma_2^-, 2R_1^-, S_1 + S_2, T_1 + T_2, U_1^+ + U_1^-, 2X_2, Y_2^+ + Y_2^- + Y_3^+ + Y_3^-, Z_1 + Z_2]$        | trivial                         |
| $[(\blacksquare)^{2T} + \Gamma_2^+ + \Gamma_2^-, 2R_1^-, S_1 + S_2, T_1 + T_2, 2U_1^-, 2X_2, Y_2^+ + Y_2^- + Y_3^+ + Y_3^-, Z_1 + Z_2]$               | 1                               |
| $[(\blacksquare)^{2T} + \Gamma_2^+ + \Gamma_2^-, R_1^+ + R_1^-, S_1 + S_2, T_1 + T_2, 2U_1^+, 2X_2, Y_2^+ + Y_2^- + Y_3^+ + Y_3^-, Z_1 + Z_2]$        | trivial                         |
| $[(\blacksquare)^{2T} + \Gamma_2^+ + \Gamma_2^-, R_1^+ + R_1^-, S_1 + S_2, T_1 + T_2, U_1^+ + U_1^-, 2X_2, Y_2^+ + Y_2^- + Y_3^+ + Y_3^-, Z_1 + Z_2]$ | 1                               |
| $[(\blacksquare)^{2T} + \Gamma_2^+ + \Gamma_2^-, R_1^+ + R_1^-, S_1 + S_2, T_1 + T_2, 2U_1^-, 2X_2, Y_2^+ + Y_2^- + Y_3^+ + Y_3^-, Z_1 + Z_2]$        | trivial                         |
| $[(\blacksquare)^{2T} + \Gamma_2^+ + \Gamma_2^-, 2R_1^+, S_1 + S_2, T_1 + T_2, 2U_1^+, 2X_2, Y_2^+ + Y_2^- + Y_3^+ + Y_3^-, Z_1 + Z_2]$               | 1                               |
| $[(\blacksquare)^{2T} + \Gamma_2^+ + \Gamma_2^-, 2R_1^+, S_1 + S_2, T_1 + T_2, U_1^+ + U_1^-, 2X_2, Y_2^+ + Y_2^- + Y_3^+ + Y_3^-, Z_1 + Z_2]$        | trivial                         |
| $[(\blacksquare)^{2T} + \Gamma_2^+ + \Gamma_2^-, 2R_1^+, S_1 + S_2, T_1 + T_2, 2U_1^-, 2X_2, Y_2^+ + Y_2^- + Y_3^+ + Y_3^-, Z_1 + Z_2]$               | 1                               |
| $[(\blacksquare)^{2T} + \Gamma_1^+ + \Gamma_1^-, 2R_1^-, 2S_2, T_1 + T_2, 2U_1^+, X_1 + X_2, Y_2^+ + Y_2^- + Y_4^+ + Y_4^-, Z_1 + Z_2]$               | 1                               |
| $[(\blacksquare)^{2T} + \Gamma_1^+ + \Gamma_1^-, 2R_1^-, 2S_2, T_1 + T_2, U_1^+ + U_1^-, X_1 + X_2, Y_2^+ + Y_2^- + Y_4^+ + Y_4^-, Z_1 + Z_2]$        | trivial                         |
| $[(\blacksquare)^{2T} + \Gamma_1^+ + \Gamma_1^-, 2R_1^-, S_1 + S_2, T_1 + T_2, 2U_1^+, X_1 + X_2, Y_1^+ + Y_2^+ + Y_3^+ + Y_4^+, Z_1 + Z_2]$          | trivial                         |
| $[(\blacksquare)^{2T} + \Gamma_1^+ + \Gamma_1^-, 2R_1^-, S_1 + S_2, T_1 + T_2, U_1^+ + U_1^-, X_1 + X_2, Y_1^+ + Y_2^+ + Y_3^+ + Y_4^+, Z_1 + Z_2]$   | 1                               |
| $[(\blacksquare)^{2T} + \Gamma_1^+ + \Gamma_1^-, R_1^+ + R_1^-, 2S_2, T_1 + T_2, 2U_1^+, X_1 + X_2, Y_2^+ + Y_2^- + Y_4^+ + Y_4^-, Z_1 + Z_2]$        | trivial                         |
| $[(\blacksquare)^{2T} + \Gamma_1^+ + \Gamma_1^-, R_1^+ + R_1^-, 2S_2, T_1 + T_2, U_1^+ + U_1^-, X_1 + X_2, Y_2^+ + Y_2^- + Y_4^+ + Y_4^-, Z_1 + Z_2]$ | 1                               |

... continued on next page

... continued from previous page

|                                                                                                                                                            |         |
|------------------------------------------------------------------------------------------------------------------------------------------------------------|---------|
| $[(\blacksquare)^{2T} + \Gamma_1^+ + \Gamma_1^-, R_1^+ + R_1^-, S_1 + S_2, T_1 + T_2, 2U_1^+, X_1 + X_2, Y_1^+ + Y_2^+ + Y_3^+ + Y_4^+, Z_1 + Z_2]$        | 1       |
| $[(\blacksquare)^{2T} + \Gamma_1^+ + \Gamma_1^-, R_1^+ + R_1^-, S_1 + S_2, T_1 + T_2, U_1^+ + U_1^-, X_1 + X_2, Y_1^+ + Y_2^+ + Y_3^+ + Y_4^+, Z_1 + Z_2]$ | trivial |
| $[(\blacksquare)^{2T} + \Gamma_1^+ + \Gamma_1^-, 2R_1^-, 2S_2, T_1 + T_2, 2U_1^-, X_1 + X_2, Y_2^+ + Y_2^- + Y_4^+ + Y_4^-, Z_1 + Z_2]$                    | 1       |
| $[(\blacksquare)^{2T} + \Gamma_1^+ + \Gamma_1^-, 2R_1^-, S_1 + S_2, T_1 + T_2, 2U_1^-, X_1 + X_2, Y_1^+ + Y_2^+ + Y_3^+ + Y_4^+, Z_1 + Z_2]$               | trivial |
| $[(\blacksquare)^{2T} + \Gamma_1^+ + \Gamma_1^-, R_1^+ + R_1^-, 2S_2, T_1 + T_2, 2U_1^-, X_1 + X_2, Y_2^+ + Y_2^- + Y_4^+ + Y_4^-, Z_1 + Z_2]$             | trivial |
| $[(\blacksquare)^{2T} + \Gamma_1^+ + \Gamma_1^-, R_1^+ + R_1^-, S_1 + S_2, T_1 + T_2, 2U_1^-, X_1 + X_2, Y_1^+ + Y_2^+ + Y_3^+ + Y_4^+, Z_1 + Z_2]$        | 1       |
| $[(\blacksquare)^{2T} + \Gamma_1^+ + \Gamma_1^-, 2R_1^-, S_1 + S_2, T_1 + T_2, 2U_1^+, X_1 + X_2, Y_1^- + Y_2^- + Y_3^- + Y_4^-, Z_1 + Z_2]$               | trivial |
| $[(\blacksquare)^{2T} + \Gamma_1^+ + \Gamma_1^-, 2R_1^-, S_1 + S_2, T_1 + T_2, U_1^+ + U_1^-, X_1 + X_2, Y_1^- + Y_2^- + Y_3^- + Y_4^-, Z_1 + Z_2]$        | 1       |
| $[(\blacksquare)^{2T} + \Gamma_1^+ + \Gamma_1^-, 2R_1^-, 2S_1, T_1 + T_2, 2U_1^+, X_1 + X_2, Y_1^+ + Y_1^- + Y_3^+ + Y_3^-, Z_1 + Z_2]$                    | 1       |
| $[(\blacksquare)^{2T} + \Gamma_1^+ + \Gamma_1^-, 2R_1^-, 2S_1, T_1 + T_2, U_1^+ + U_1^-, X_1 + X_2, Y_1^+ + Y_1^- + Y_3^+ + Y_3^-, Z_1 + Z_2]$             | trivial |
| $[(\blacksquare)^{2T} + \Gamma_1^+ + \Gamma_1^-, R_1^+ + R_1^-, S_1 + S_2, T_1 + T_2, 2U_1^+, X_1 + X_2, Y_1^- + Y_2^- + Y_3^- + Y_4^-, Z_1 + Z_2]$        | 1       |
| $[(\blacksquare)^{2T} + \Gamma_1^+ + \Gamma_1^-, R_1^+ + R_1^-, S_1 + S_2, T_1 + T_2, U_1^+ + U_1^-, X_1 + X_2, Y_1^- + Y_2^- + Y_3^- + Y_4^-, Z_1 + Z_2]$ | trivial |
| $[(\blacksquare)^{2T} + \Gamma_1^+ + \Gamma_1^-, R_1^+ + R_1^-, 2S_1, T_1 + T_2, 2U_1^+, X_1 + X_2, Y_1^+ + Y_1^- + Y_3^+ + Y_3^-, Z_1 + Z_2]$             | trivial |
| $[(\blacksquare)^{2T} + \Gamma_1^+ + \Gamma_1^-, R_1^+ + R_1^-, 2S_1, T_1 + T_2, U_1^+ + U_1^-, X_1 + X_2, Y_1^+ + Y_1^- + Y_3^+ + Y_3^-, Z_1 + Z_2]$      | 1       |
| $[(\blacksquare)^{2T} + \Gamma_1^+ + \Gamma_1^-, 2R_1^-, S_1 + S_2, T_1 + T_2, 2U_1^-, X_1 + X_2, Y_1^- + Y_2^- + Y_3^- + Y_4^-, Z_1 + Z_2]$               | trivial |
| $[(\blacksquare)^{2T} + \Gamma_1^+ + \Gamma_1^-, 2R_1^-, 2S_1, T_1 + T_2, 2U_1^-, X_1 + X_2, Y_1^+ + Y_1^- + Y_3^+ + Y_3^-, Z_1 + Z_2]$                    | 1       |
| $[(\blacksquare)^{2T} + \Gamma_1^+ + \Gamma_1^-, R_1^+ + R_1^-, S_1 + S_2, T_1 + T_2, 2U_1^-, X_1 + X_2, Y_1^- + Y_2^- + Y_3^- + Y_4^-, Z_1 + Z_2]$        | 1       |
| $[(\blacksquare)^{2T} + \Gamma_1^+ + \Gamma_1^-, R_1^+ + R_1^-, 2S_1, T_1 + T_2, 2U_1^-, X_1 + X_2, Y_1^+ + Y_1^- + Y_3^+ + Y_3^-, Z_1 + Z_2]$             | trivial |
| $[(\blacksquare)^{2T} + \Gamma_1^+ + \Gamma_1^-, 2R_1^+, 2S_2, T_1 + T_2, 2U_1^+, X_1 + X_2, Y_2^+ + Y_2^- + Y_4^+ + Y_4^-, Z_1 + Z_2]$                    | 1       |
| $[(\blacksquare)^{2T} + \Gamma_1^+ + \Gamma_1^-, 2R_1^+, 2S_2, T_1 + T_2, U_1^+ + U_1^-, X_1 + X_2, Y_2^+ + Y_2^- + Y_4^+ + Y_4^-, Z_1 + Z_2]$             | trivial |
| $[(\blacksquare)^{2T} + \Gamma_1^+ + \Gamma_1^-, 2R_1^+, S_1 + S_2, T_1 + T_2, 2U_1^+, X_1 + X_2, Y_1^+ + Y_2^+ + Y_3^+ + Y_4^+, Z_1 + Z_2]$               | trivial |
| $[(\blacksquare)^{2T} + \Gamma_1^+ + \Gamma_1^-, 2R_1^+, S_1 + S_2, T_1 + T_2, U_1^+ + U_1^-, X_1 + X_2, Y_1^+ + Y_2^+ + Y_3^+ + Y_4^+, Z_1 + Z_2]$        | 1       |
| $[(\blacksquare)^{2T} + \Gamma_1^+ + \Gamma_1^-, 2R_1^+, 2S_2, T_1 + T_2, 2U_1^-, X_1 + X_2, Y_2^+ + Y_2^- + Y_4^+ + Y_4^-, Z_1 + Z_2]$                    | 1       |
| $[(\blacksquare)^{2T} + \Gamma_1^+ + \Gamma_1^-, 2R_1^+, S_1 + S_2, T_1 + T_2, 2U_1^-, X_1 + X_2, Y_1^+ + Y_2^+ + Y_3^+ + Y_4^+, Z_1 + Z_2]$               | trivial |
| $[(\blacksquare)^{2T} + \Gamma_1^+ + \Gamma_1^-, 2R_1^+, S_1 + S_2, T_1 + T_2, 2U_1^+, X_1 + X_2, Y_1^- + Y_2^- + Y_3^- + Y_4^-, Z_1 + Z_2]$               | trivial |
| $[(\blacksquare)^{2T} + \Gamma_1^+ + \Gamma_1^-, 2R_1^+, S_1 + S_2, T_1 + T_2, U_1^+ + U_1^-, X_1 + X_2, Y_1^- + Y_2^- + Y_3^- + Y_4^-, Z_1 + Z_2]$        | 1       |
| $[(\blacksquare)^{2T} + \Gamma_1^+ + \Gamma_1^-, 2R_1^+, 2S_1, T_1 + T_2, 2U_1^+, X_1 + X_2, Y_1^+ + Y_1^- + Y_3^+ + Y_3^-, Z_1 + Z_2]$                    | 1       |
| $[(\blacksquare)^{2T} + \Gamma_1^+ + \Gamma_1^-, 2R_1^+, 2S_1, T_1 + T_2, U_1^+ + U_1^-, X_1 + X_2, Y_1^+ + Y_1^- + Y_3^+ + Y_3^-, Z_1 + Z_2]$             | trivial |
| $[(\blacksquare)^{2T} + \Gamma_1^+ + \Gamma_1^-, 2R_1^+, S_1 + S_2, T_1 + T_2, 2U_1^-, X_1 + X_2, Y_1^- + Y_2^- + Y_3^- + Y_4^-, Z_1 + Z_2]$               | trivial |
| $[(\blacksquare)^{2T} + \Gamma_1^+ + \Gamma_1^-, 2R_1^+, 2S_1, T_1 + T_2, 2U_1^-, X_1 + X_2, Y_1^+ + Y_1^- + Y_3^+ + Y_3^-, Z_1 + Z_2]$                    | 1       |

2nd minimal solution:  $\mu_2^T = 6$  (512 symmetry vectors)

Space group 54 ( $\mathbb{Z}_2$ )

1st minimal solution:  $\mu_1^T = 4$  (5 symmetry vectors)

| $\mathbf{n}^T$                                                                                                                                 | $\mathbf{v}^T \in \mathbb{Z}_2$ |
|------------------------------------------------------------------------------------------------------------------------------------------------|---------------------------------|
| $[(\blacksquare)^{2T} + \Gamma_3^+ + \Gamma_3^-, R_1 R_2, S_1 + S_2, T_1 + T_2, U_1 U_2, X_1 + X_2, Y_2^+ + Y_2^- + Y_3^+ + Y_3^-, 2Z_2]$      | 1                               |
| $[(\blacksquare)^{2T} + \Gamma_1^+ + \Gamma_1^-, R_1 R_2, S_1 + S_2, T_1 + T_2, U_1 U_2, X_1 + X_2, Y_1^- + Y_2^- + Y_3^- + Y_4^-, Z_1 + Z_2]$ | trivial                         |
| $[(\blacksquare)^{2T} + \Gamma_1^+ + \Gamma_1^-, R_1 R_2, S_1 + S_2, 2T_2, U_1 U_2, X_1 + X_2, Y_3^+ + Y_3^- + Y_4^+ + Y_4^-, Z_1 + Z_2]$      | 1                               |
| $[(\blacksquare)^{2T} + \Gamma_1^+ + \Gamma_1^-, R_1 R_2, S_1 + S_2, 2T_1, U_1 U_2, X_1 + X_2, Y_1^+ + Y_1^- + Y_2^+ + Y_2^-, Z_1 + Z_2]$      | 1                               |
| $[(\blacksquare)^{2T} + \Gamma_1^+ + \Gamma_1^-, R_1 R_2, S_1 + S_2, T_1 + T_2, U_1 U_2, X_1 + X_2, Y_1^+ + Y_2^+ + Y_3^+ + Y_4^+, Z_1 + Z_2]$ | trivial                         |

2nd minimal solution:  $\mu_2^T = 8$  (57 symmetry vectors)

Space group 55 ( $\mathbb{Z}_1$ )

1st minimal solution:  $\mu_1^T = 4$  (20 symmetry vectors)

| $\mathbf{n}^T$                                                                                                                                                                |
|-------------------------------------------------------------------------------------------------------------------------------------------------------------------------------|
| $[(\bullet)^{2T} + \Gamma_1^+ + \Gamma_1^-, R_3^+ R_4^+ + R_3^- R_4^-, S_3^+ S_4^+ + S_3^- S_4^-, T_1 + T_2, U_1 + U_2, X_1 + X_2, Y_1 + Y_2, Z_1^- + Z_2^- + Z_3^- + Z_4^-]$ |
| $[(\bullet)^{2T} + \Gamma_1^+ + \Gamma_1^-, R_1^- R_2^- + R_3^- R_4^-, S_1^+ S_2^+ + S_3^+ S_4^+, T_1 + T_2, U_1 + U_2, X_1 + X_2, Y_1 + Y_2, Z_1^- + Z_2^- + Z_3^- + Z_4^-]$ |
| $[(\bullet)^{2T} + \Gamma_1^+ + \Gamma_1^-, 2R_3^- R_4^-, S_3^+ S_4^+ + S_3^- S_4^-, 2T_2, 2U_1, X_1 + X_2, Y_1 + Y_2, Z_1^+ + Z_2^+ + Z_3^- + Z_4^-]$                        |
| $[(\bullet)^{2T} + \Gamma_1^+ + \Gamma_1^-, R_1^+ R_2^+ + R_3^- R_4^-, S_1^+ S_2^+ + S_3^+ S_4^+, 2T_2, 2U_1, X_1 + X_2, Y_1 + Y_2, Z_1^+ + Z_2^+ + Z_3^- + Z_4^-]$           |
| $[(\bullet)^{2T} + \Gamma_1^+ + \Gamma_1^-, R_1^- R_2^- + R_3^- R_4^-, S_1^- S_2^- + S_3^- S_4^-, T_1 + T_2, U_1 + U_2, X_1 + X_2, Y_1 + Y_2, Z_1^- + Z_2^- + Z_3^- + Z_4^-]$ |
| $[(\bullet)^{2T} + \Gamma_1^+ + \Gamma_1^-, R_1^+ R_2^+ + R_3^- R_4^-, S_1^- S_2^- + S_3^- S_4^-, 2T_2, 2U_1, X_1 + X_2, Y_1 + Y_2, Z_1^+ + Z_2^+ + Z_3^- + Z_4^-]$           |
| $[(\bullet)^{2T} + \Gamma_1^+ + \Gamma_1^-, R_1^+ R_2^+ + R_3^+ R_4^+, S_1^+ S_2^+ + S_3^+ S_4^+, T_1 + T_2, U_1 + U_2, X_1 + X_2, Y_1 + Y_2, Z_1^- + Z_2^- + Z_3^- + Z_4^-]$ |
| $[(\bullet)^{2T} + \Gamma_1^+ + \Gamma_1^-, R_1^+ R_2^+ + R_1^- R_2^-, S_1^+ S_2^+ + S_1^- S_2^-, T_1 + T_2, U_1 + U_2, X_1 + X_2, Y_1 + Y_2, Z_1^- + Z_2^- + Z_3^- + Z_4^-]$ |
| $[(\bullet)^{2T} + \Gamma_1^+ + \Gamma_1^-, 2R_1^+ R_2^+, S_1^+ S_2^+ + S_1^- S_2^-, 2T_2, 2U_1, X_1 + X_2, Y_1 + Y_2, Z_1^+ + Z_2^+ + Z_3^- + Z_4^-]$                        |
| $[(\bullet)^{2T} + \Gamma_1^+ + \Gamma_1^-, 2R_3^+ R_4^+, S_3^+ S_4^+ + S_3^- S_4^-, 2T_1, 2U_2, X_1 + X_2, Y_1 + Y_2, Z_1^- + Z_2^- + Z_3^+ + Z_4^+]$                        |
| $[(\bullet)^{2T} + \Gamma_1^+ + \Gamma_1^-, R_1^- R_2^- + R_3^+ R_4^+, S_1^+ S_2^+ + S_3^+ S_4^+, 2T_1, 2U_2, X_1 + X_2, Y_1 + Y_2, Z_1^- + Z_2^- + Z_3^+ + Z_4^+]$           |
| $[(\bullet)^{2T} + \Gamma_1^+ + \Gamma_1^-, R_3^+ R_4^+ + R_3^- R_4^-, S_3^+ S_4^+ + S_3^- S_4^-, T_1 + T_2, U_1 + U_2, X_1 + X_2, Y_1 + Y_2, Z_1^+ + Z_2^+ + Z_3^+ + Z_4^+]$ |
| $[(\bullet)^{2T} + \Gamma_1^+ + \Gamma_1^-, R_1^+ R_2^+ + R_3^+ R_4^+, S_1^+ S_2^+ + S_3^+ S_4^+, T_1 + T_2, U_1 + U_2, X_1 + X_2, Y_1 + Y_2, Z_1^+ + Z_2^+ + Z_3^+ + Z_4^+]$ |
| $[(\bullet)^{2T} + \Gamma_1^+ + \Gamma_1^-, R_1^- R_2^- + R_3^+ R_4^+, S_1^- S_2^- + S_3^- S_4^-, 2T_1, 2U_2, X_1 + X_2, Y_1 + Y_2, Z_1^- + Z_2^- + Z_3^+ + Z_4^+]$           |
| $[(\bullet)^{2T} + \Gamma_1^+ + \Gamma_1^-, 2R_1^- R_2^-, S_1^+ S_2^+ + S_1^- S_2^-, 2T_1, 2U_2, X_1 + X_2, Y_1 + Y_2, Z_1^- + Z_2^- + Z_3^+ + Z_4^+]$                        |
| $[(\bullet)^{2T} + \Gamma_1^+ + \Gamma_1^-, R_1^- R_2^- + R_3^- R_4^-, S_1^- S_2^- + S_3^- S_4^-, T_1 + T_2, U_1 + U_2, X_1 + X_2, Y_1 + Y_2, Z_1^+ + Z_2^+ + Z_3^+ + Z_4^+]$ |
| $[(\bullet)^{2T} + \Gamma_1^+ + \Gamma_1^-, R_1^+ R_2^+ + R_1^- R_2^-, S_1^+ S_2^+ + S_1^- S_2^-, T_1 + T_2, U_1 + U_2, X_1 + X_2, Y_1 + Y_2, Z_1^+ + Z_2^+ + Z_3^+ + Z_4^+]$ |
| $[(\bullet)^{2T} + \Gamma_1^+ + \Gamma_1^-, R_1^- R_2^- + R_3^- R_4^-, S_1^+ S_2^+ + S_3^+ S_4^+, T_1 + T_2, U_1 + U_2, X_1 + X_2, Y_1 + Y_2, Z_1^+ + Z_2^+ + Z_3^+ + Z_4^+]$ |
| $[(\bullet)^{2T} + \Gamma_1^+ + \Gamma_1^-, R_1^+ R_2^+ + R_3^+ R_4^+, S_1^- S_2^- + S_3^- S_4^-, T_1 + T_2, U_1 + U_2, X_1 + X_2, Y_1 + Y_2, Z_1^+ + Z_2^+ + Z_3^+ + Z_4^+]$ |
| $[(\bullet)^{2T} + \Gamma_1^+ + \Gamma_1^-, R_1^+ R_2^+ + R_3^+ R_4^+, S_1^- S_2^- + S_3^- S_4^-, T_1 + T_2, U_1 + U_2, X_1 + X_2, Y_1 + Y_2, Z_1^- + Z_2^- + Z_3^- + Z_4^-]$ |

2nd minimal solution:  $\mu_2^T = 6$  (208 symmetry vectors)

Space group 56 ( $\mathbb{Z}_2$ )

1st minimal solution:  $\mu_1^T = 4$  (4 symmetry vectors)

| $\mathbf{n}^T$                                                                                                                        | $\mathbf{v}^T \in \mathbb{Z}_2$ |
|---------------------------------------------------------------------------------------------------------------------------------------|---------------------------------|
| $[(\bullet)^{2T} + \Gamma_1^+ + \Gamma_1^-, R_1^- R_2^- + R_3^- R_4^-, S_1 + S_2, T_1 T_2, U_1 U_2, X_1 + X_2, Y_1 + Y_2, Z_1 + Z_2]$ | trivial                         |
| $[(\bullet)^{2T} + \Gamma_1^+ + \Gamma_1^-, R_3^+ R_4^+ + R_3^- R_4^-, 2S_2, T_1 T_2, U_1 U_2, X_1 + X_2, Y_1 + Y_2, Z_1 + Z_2]$      | 1                               |
| $[(\bullet)^{2T} + \Gamma_1^+ + \Gamma_1^-, R_1^+ R_2^+ + R_1^- R_2^-, 2S_1, T_1 T_2, U_1 U_2, X_1 + X_2, Y_1 + Y_2, Z_1 + Z_2]$      | 1                               |
| $[(\bullet)^{2T} + \Gamma_1^+ + \Gamma_1^-, R_1^+ R_2^+ + R_3^+ R_4^+, S_1 + S_2, T_1 T_2, U_1 U_2, X_1 + X_2, Y_1 + Y_2, Z_1 + Z_2]$ | trivial                         |

2nd minimal solution:  $\mu_2^T = 8$  (36 symmetry vectors)

Space group 57 ( $\mathbb{Z}_1$ )

1st minimal solution:  $\mu_1^T = 4$  (2 symmetry vectors)

| $\mathbf{n}^T$                                                                                                                            |
|-------------------------------------------------------------------------------------------------------------------------------------------|
| $[(\bullet)^{2T} + \Gamma_1^+ + \Gamma_1^-, R_1 R_2, S_1 + S_2, T_1 T_2, U_1 + U_2, X_1^+ + X_2^+ + X_3^+ + X_4^+, Y_1 + Y_2, Z_1 + Z_2]$ |
| $[(\bullet)^{2T} + \Gamma_1^+ + \Gamma_1^-, R_1 R_2, S_1 + S_2, T_1 T_2, U_1 + U_2, X_1^- + X_2^- + X_3^- + X_4^-, Y_1 + Y_2, Z_1 + Z_2]$ |

2nd minimal solution:  $\mu_2^T = 8$  (16 symmetry vectors)



... continued from previous page

---

|                                                                                                                                                    |
|----------------------------------------------------------------------------------------------------------------------------------------------------|
| $[(\blacksquare)^{2T} + \Gamma_1^+ + \Gamma_1^-, 2R_2, 2S_2, T_1 + T_2, U_1 + U_2, X_1 + X_2, Y_1 + Y_2, Z_1^+ + Z_2^+ + Z_3^+ + Z_4^+]$           |
| $[(\blacksquare)^{2T} + \Gamma_1^+ + \Gamma_1^-, R_1 + R_2, S_1 + S_2, T_1 + T_2, U_1 + U_2, X_1 + X_2, Y_1 + Y_2, Z_1^+ + Z_2^+ + Z_3^+ + Z_4^+]$ |
| $[(\blacksquare)^{2T} + \Gamma_1^+ + \Gamma_1^-, 2R_1, 2S_1, T_1 + T_2, U_1 + U_2, X_1 + X_2, Y_1 + Y_2, Z_1^- + Z_2^- + Z_3^- + Z_4^-]$           |
| $[(\blacksquare)^{2T} + \Gamma_1^+ + \Gamma_1^-, 2R_1, 2S_1, T_1 + T_2, U_1 + U_2, X_1 + X_2, Y_1 + Y_2, Z_1^+ + Z_2^+ + Z_3^+ + Z_4^+]$           |

---

2nd minimal solution:  $\mu_2^T = 6$  (40 symmetry vectors)

Space group 60 ( $\mathbb{Z}_2$ )

1st minimal solution:  $\mu_1^T = 4$  (3 symmetry vectors)

| $\mathbf{n}^T$                                                                                                               | $\mathbf{v}^T \in \mathbb{Z}_2$ |
|------------------------------------------------------------------------------------------------------------------------------|---------------------------------|
| $[(\blacksquare)^{2T} + \Gamma_1^+ + \Gamma_1^-, R_1 R_2, 2S_1^-, T_1 T_2, U_1 U_2, X_1 + X_2, Y_1 + Y_2, Z_1 + Z_2]$        | trivial                         |
| $[(\blacksquare)^{2T} + \Gamma_1^+ + \Gamma_1^-, R_1 R_2, S_1^+ + S_1^-, T_1 T_2, U_1 U_2, X_1 + X_2, Y_1 + Y_2, Z_1 + Z_2]$ | 1                               |
| $[(\blacksquare)^{2T} + \Gamma_1^+ + \Gamma_1^-, R_1 R_2, 2S_1^+, T_1 T_2, U_1 U_2, X_1 + X_2, Y_1 + Y_2, Z_1 + Z_2]$        | trivial                         |

2nd minimal solution:  $\mu_2^T = 8$  (20 symmetry vectors)

Space group 61 ( $\mathbb{Z}_1$ )

1st minimal solution:  $\mu_1^T = 4$  (2 symmetry vectors)

| $\mathbf{n}^T$                                                                                                             |
|----------------------------------------------------------------------------------------------------------------------------|
| $[(\blacksquare)^{2T} + \Gamma_1^+ + \Gamma_1^-, R_1^- R_1^-, S_1 S_2, T_1 T_2, U_1 U_2, X_1 + X_2, Y_1 + Y_2, Z_1 + Z_2]$ |
| $[(\blacksquare)^{2T} + \Gamma_1^+ + \Gamma_1^-, R_1^+ R_1^+, S_1 S_2, T_1 T_2, U_1 U_2, X_1 + X_2, Y_1 + Y_2, Z_1 + Z_2]$ |

2nd minimal solution:  $\mu_2^T = 8$  (6 symmetry vectors)

Space group 62 ( $\mathbb{Z}_1$ )

1st minimal solution:  $\mu_1^T = 4$  (2 symmetry vectors)

| $\mathbf{n}^T$                                                                                                                             |
|--------------------------------------------------------------------------------------------------------------------------------------------|
| $[(\blacksquare)^{2T} + \Gamma_1^+ + \Gamma_1^-, R_1 R_2, S_1 S_2, T_1 + T_2, U_1^+ U_4^+ + U_2^+ U_3^+, X_1 + X_2, Y_1 + Y_2, Z_1 + Z_2]$ |
| $[(\blacksquare)^{2T} + \Gamma_1^+ + \Gamma_1^-, R_1 R_2, S_1 S_2, T_1 + T_2, U_1^- U_4^- + U_2^- U_3^-, X_1 + X_2, Y_1 + Y_2, Z_1 + Z_2]$ |

2nd minimal solution:  $\mu_2^T = 8$  (10 symmetry vectors)

Space group 63 ( $\mathbb{Z}_1$ )

1st minimal solution:  $\mu_1^T = 4$  (10 symmetry vectors)



| $\mathbf{n}^T$                                                                                                                              |
|---------------------------------------------------------------------------------------------------------------------------------------------|
| $[(\blacksquare)^{2T} + \Gamma_1^+ + \Gamma_2^+, T_1 + T_2, Y_2^+ + Y_2^- + Y_3^- + Y_4^-, Z_1 + Z_2, 2R_1, 2S_1^+ + S_2^+ + S_2^-]$        |
| $[(\blacksquare)^{2T} + \Gamma_1^+ + \Gamma_1^-, T_1 + T_2, Y_1^- + Y_2^- + Y_3^- + Y_4^-, Z_1 + Z_2, 2R_1, S_1^+ + S_1^- + S_2^+ + S_2^-]$ |
| $[(\blacksquare)^{2T} + \Gamma_1^+ + \Gamma_1^-, T_1 + T_2, Y_1^- + Y_2^- + Y_3^- + Y_4^-, Z_1 + Z_2, 2R_1, 2S_1^+ + 2S_2^+]$               |
| $[(\blacksquare)^{2T} + \Gamma_1^- + \Gamma_2^-, T_1 + T_2, Y_2^+ + Y_2^- + Y_3^+ + Y_4^+, Z_1 + Z_2, 2R_1, 2S_1^- + S_2^+ + S_2^-]$        |
| $[(\blacksquare)^{2T} + \Gamma_1^- + \Gamma_2^-, T_1 + T_2, Y_2^+ + Y_2^- + Y_3^+ + Y_4^+, Z_1 + Z_2, 2R_1, S_1^+ + S_1^- + 2S_2^+]$        |
| $[(\blacksquare)^{2T} + \Gamma_1^+ + \Gamma_2^+, T_1 + T_2, Y_2^+ + Y_2^- + Y_3^- + Y_4^-, Z_1 + Z_2, 2R_1, S_1^+ + S_1^- + 2S_2^-]$        |
| $[(\blacksquare)^{2T} + \Gamma_1^+ + \Gamma_1^-, T_1 + T_2, Y_1^- + Y_2^- + Y_3^- + Y_4^-, Z_1 + Z_2, 2R_1, 2S_1^- + 2S_2^-]$               |
| $[(\blacksquare)^{2T} + \Gamma_1^+ + \Gamma_1^-, T_1 + T_2, Y_1^- + Y_2^- + Y_3^+ + Y_4^+, Z_1 + Z_2, 2R_1, 2S_1^- + 2S_2^-]$               |
| $[(\blacksquare)^{2T} + \Gamma_1^+ + \Gamma_1^-, T_1 + T_2, Y_1^- + Y_2^- + Y_3^+ + Y_4^+, Z_1 + Z_2, 2R_1, S_1^+ + S_1^- + S_2^+ + S_2^-]$ |
| $[(\blacksquare)^{2T} + \Gamma_1^+ + \Gamma_1^-, T_1 + T_2, Y_1^- + Y_2^- + Y_3^+ + Y_4^+, Z_1 + Z_2, 2R_1, 2S_1^+ + 2S_2^+]$               |

2nd minimal solution:  $\mu_2^T = 6$  (90 symmetry vectors)

Space group 64 ( $\mathbb{Z}_1$ )

1st minimal solution:  $\mu_1^T = 4$  (6 symmetry vectors)

| $\mathbf{n}^T$                                                                                                                          |
|-----------------------------------------------------------------------------------------------------------------------------------------|
| $[(\blacksquare)^{2T} + \Gamma_1^+ + \Gamma_1^-, T_1 + T_2, Y_1^- + Y_2^- + Y_3^- + Y_4^-, Z_1 + Z_2, 2R_1^- R_2^-, 2S_1]$              |
| $[(\blacksquare)^{2T} + \Gamma_1^+ + \Gamma_1^-, T_1 + T_2, Y_1^- + Y_2^- + Y_3^- + Y_4^-, Z_1 + Z_2, R_1^+ R_2^+ + R_1^- R_2^-, 2S_1]$ |
| $[(\blacksquare)^{2T} + \Gamma_1^+ + \Gamma_1^-, T_1 + T_2, Y_1^- + Y_2^- + Y_3^- + Y_4^-, Z_1 + Z_2, 2R_1^+ R_2^+, 2S_1]$              |
| $[(\blacksquare)^{2T} + \Gamma_1^+ + \Gamma_1^-, T_1 + T_2, Y_1^+ + Y_2^+ + Y_3^+ + Y_4^+, Z_1 + Z_2, 2R_1^- R_2^-, 2S_1]$              |
| $[(\blacksquare)^{2T} + \Gamma_1^+ + \Gamma_1^-, T_1 + T_2, Y_1^+ + Y_2^+ + Y_3^+ + Y_4^+, Z_1 + Z_2, R_1^+ R_2^+ + R_1^- R_2^-, 2S_1]$ |
| $[(\blacksquare)^{2T} + \Gamma_1^+ + \Gamma_1^-, T_1 + T_2, Y_1^+ + Y_2^+ + Y_3^+ + Y_4^+, Z_1 + Z_2, 2R_1^+ R_2^+, 2S_1]$              |

2nd minimal solution:  $\mu_2^T = 6$  (40 symmetry vectors)

Space group 65 ( $\mathbb{Z}_1$ )

1st minimal solution:  $\mu_1^T = 2$  (8 symmetry vectors)

| $\mathbf{n}^T$                                                                                     |
|----------------------------------------------------------------------------------------------------|
| $[(\blacksquare)^{2T}, T_1^- + T_2^-, Y_2^+ + Y_2^-, Z_3^+ + Z_4^+, 2R_2^+, S_2^+ + S_2^-]$        |
| $[(\blacksquare)^{2T}, T_1^- + T_2^-, Y_2^+ + Y_2^-, Z_3^+ + Z_4^+, R_1^- + R_2^+, S_1^- + S_2^-]$ |
| $[(\blacksquare)^{2T}, T_1^+ + T_2^+, Y_2^+ + Y_2^-, Z_3^- + Z_4^-, 2R_2^-, S_2^+ + S_2^-]$        |
| $[(\blacksquare)^{2T}, T_1^- + T_2^-, Y_2^+ + Y_2^-, Z_3^+ + Z_4^+, R_1^- + R_2^+, S_1^+ + S_2^+]$ |
| $[(\blacksquare)^{2T}, T_1^- + T_2^-, Y_2^+ + Y_2^-, Z_3^+ + Z_4^+, 2R_1^-, S_1^+ + S_1^-]$        |
| $[(\blacksquare)^{2T}, T_1^+ + T_2^+, Y_2^+ + Y_2^-, Z_3^- + Z_4^-, R_1^+ + R_2^-, S_1^+ + S_2^+]$ |
| $[(\blacksquare)^{2T}, T_1^+ + T_2^+, Y_2^+ + Y_2^-, Z_3^- + Z_4^-, R_1^+ + R_2^-, S_1^- + S_2^-]$ |
| $[(\blacksquare)^{2T}, T_1^+ + T_2^+, Y_2^+ + Y_2^-, Z_3^- + Z_4^-, 2R_1^+, S_1^+ + S_1^-]$        |

2nd minimal solution:  $\mu_2^T = 3$  (400 symmetry vectors)

Space group 66 ( $\mathbb{Z}_2$ )

1st minimal solution:  $\mu_1^T = 2$  (6 symmetry vectors)

| $\mathbf{n}^T$                                                                 | $\mathbf{v}^T \in \mathbb{Z}_2$ |
|--------------------------------------------------------------------------------|---------------------------------|
| $[(\blacksquare)^{2T}, T_1, Y_2^+ + Y_2^-, Z_2, R_2^+ + R_2^-, S_2^+ + S_2^-]$ | 1                               |
| $[(\blacksquare)^{2T}, T_1, Y_2^+ + Y_2^-, Z_2, R_1^+ + R_2^+, S_1^- + S_2^-]$ | trivial                         |
| $[(\blacksquare)^{2T}, T_1, Y_2^+ + Y_2^-, Z_2, R_1^- + R_2^-, S_1^+ + S_2^+]$ | trivial                         |
| $[(\blacksquare)^{2T}, T_1, Y_2^+ + Y_2^-, Z_2, R_1^+ + R_2^+, S_1^+ + S_2^+]$ | trivial                         |
| $[(\blacksquare)^{2T}, T_1, Y_2^+ + Y_2^-, Z_2, R_1^+ + R_1^-, S_1^+ + S_1^-]$ | 1                               |
| $[(\blacksquare)^{2T}, T_1, Y_2^+ + Y_2^-, Z_2, R_1^- + R_2^-, S_1^- + S_2^-]$ | trivial                         |

2nd minimal solution:  $\mu_2^T = 4$  (261 symmetry vectors)

Space group 67 ( $\mathbb{Z}_1$ )

1st minimal solution:  $\mu_1^T = 4$  (70 symmetry vectors)

| $\mathbf{n}^T$                                                                                                                                             |
|------------------------------------------------------------------------------------------------------------------------------------------------------------|
| $[(\blacksquare)^{2T} + \Gamma_1^+ + \Gamma_1^-, T_1^+ + T_2^+ + T_3^+ + T_4^+, Y_1^+ + Y_2^+ + Y_3^+ + Y_4^+, Z_1^- + Z_2^- + Z_3^- + Z_4^-, 2R_1, 2S_1]$ |
| $[(\blacksquare)^{2T} + \Gamma_1^- + \Gamma_3^-, T_2^+ + T_3^+ + T_3^- + T_4^+, Y_2^+ + Y_3^+ + Y_3^- + Y_4^+, Z_2^+ + Z_3^+ + Z_3^- + Z_4^+, 2R_1, 2S_1]$ |
| $[(\blacksquare)^{2T} + \Gamma_3^+ + \Gamma_3^-, T_1^+ + T_2^+ + T_3^+ + T_4^+, Y_2^+ + Y_2^- + Y_3^- + Y_3^-, Z_3^+ + Z_3^- + Z_4^+ + Z_4^-, 2R_1, 2S_1]$ |
| $[(\blacksquare)^{2T} + \Gamma_1^+ + \Gamma_2^-, T_2^+ + T_2^- + T_3^+ + T_4^-, Y_2^+ + Y_2^- + Y_3^- + Y_4^-, 2Z_2^- + Z_3^- + Z_4^-, 2R_1, 2S_1]$        |
| $[(\blacksquare)^{2T} + \Gamma_1^- + \Gamma_3^-, T_1^- + T_3^+ + 2T_3^-, Y_2^+ + Y_3^+ + Y_3^- + Y_4^+, Z_1^- + Z_3^+ + 2Z_3^-, 2R_1, 2S_1]$               |
| $[(\blacksquare)^{2T} + \Gamma_3^- + \Gamma_4^+, T_1^- + T_2^+ + T_3^+ + T_3^-, 2Y_2^+ + Y_3^+ + Y_4^+, Z_3^+ + 2Z_3^- + Z_4^+, 2R_1, 2S_1]$               |
| $[(\blacksquare)^{2T} + \Gamma_1^+ + \Gamma_1^-, T_2^+ + T_2^- + T_3^+ + T_3^-, Y_1^+ + Y_2^+ + Y_3^+ + Y_4^+, Z_2^+ + Z_2^- + Z_3^+ + Z_3^-, 2R_1, 2S_1]$ |
| $[(\blacksquare)^{2T} + \Gamma_1^+ + \Gamma_1^-, T_1^+ + T_1^- + T_3^+ + T_3^-, Y_1^+ + Y_2^+ + Y_3^+ + Y_4^+, Z_1^+ + Z_1^- + Z_3^+ + Z_3^-, 2R_1, 2S_1]$ |
| $[(\blacksquare)^{2T} + \Gamma_1^+ + \Gamma_4^+, T_2^+ + 2T_3^+ + T_3^-, Y_2^+ + Y_3^+ + Y_4^+ + Y_4^-, Z_2^- + Z_3^+ + 2Z_3^-, 2R_1, 2S_1]$               |
| $[(\blacksquare)^{2T} + \Gamma_1^+ + \Gamma_4^+, T_1^- + T_3^+ + T_3^- + T_4^-, Y_2^+ + Y_3^+ + Y_4^+ + Y_4^-, Z_1^+ + Z_3^+ + Z_3^- + Z_4^+, 2R_1, 2S_1]$ |
| $[(\blacksquare)^{2T} + \Gamma_1^+ + \Gamma_2^-, T_1^+ + T_2^+ + 2T_3^+, Y_2^+ + Y_2^- + Y_3^- + Y_4^-, Z_1^+ + Z_2^- + Z_3^+ + Z_3^-, 2R_1, 2S_1]$        |
| $[(\blacksquare)^{2T} + \Gamma_2^- + \Gamma_3^-, T_1^+ + T_1^- + T_2^+ + T_3^+, 2Y_2^+ + Y_2^- + Y_3^-, Z_1^+ + Z_3^+ + Z_3^- + Z_4^+, 2R_1, 2S_1]$        |
| $[(\blacksquare)^{2T} + \Gamma_1^+ + \Gamma_3^+, T_1^+ + T_2^+ + T_2^- + T_3^+, Y_1^+ + Y_2^+ + Y_2^- + Y_3^+, Z_2^- + Z_3^+ + Z_3^- + Z_4^-, 2R_1, 2S_1]$ |
| $[(\blacksquare)^{2T} + \Gamma_1^+ + \Gamma_4^+, T_2^+ + T_3^+ + T_4^+ + T_4^-, Y_2^+ + Y_3^+ + Y_4^+ + Y_4^-, Z_2^- + Z_3^+ + Z_4^+ + Z_4^-, 2R_1, 2S_1]$ |
| $[(\blacksquare)^{2T} + \Gamma_1^- + \Gamma_4^-, T_1^+ + 2T_4^+ + T_4^-, Y_2^- + Y_3^- + Y_4^+ + Y_4^-, Z_1^- + Z_4^+ + 2Z_4^-, 2R_1, 2S_1]$               |
| $[(\blacksquare)^{2T} + \Gamma_1^- + \Gamma_2^+, T_1^+ + T_2^+ + 2T_4^+, Y_2^+ + Y_2^- + Y_3^- + Y_4^+, Z_1^- + Z_2^+ + Z_4^+ + Z_4^-, 2R_1, 2S_1]$        |
| $[(\blacksquare)^{2T} + \Gamma_1^- + \Gamma_2^-, T_1^- + T_1^- + T_3^- + T_4^+, Y_2^+ + Y_2^- + Y_3^- + Y_4^+, 2Z_1^- + Z_3^- + Z_4^-, 2R_1, 2S_1]$        |
| $[(\blacksquare)^{2T} + \Gamma_1^- + \Gamma_4^-, T_1^+ + T_3^+ + T_3^- + T_4^+, Y_2^- + Y_3^- + Y_4^+ + Y_4^-, Z_1^- + Z_3^+ + Z_3^- + Z_4^-, 2R_1, 2S_1]$ |
| $[(\blacksquare)^{2T} + \Gamma_1^+ + \Gamma_1^-, T_1^+ + T_1^- + T_4^+ + T_4^-, Y_1^+ + Y_2^+ + Y_3^+ + Y_4^+, Z_1^+ + Z_1^- + Z_4^+ + Z_4^-, 2R_1, 2S_1]$ |
| $[(\blacksquare)^{2T} + \Gamma_2^+ + \Gamma_4^+, T_1^+ + T_1^- + T_2^+ + T_4^+, 2Y_2^+ + Y_2^- + Y_4^+, Z_1^- + Z_3^- + Z_4^+ + Z_4^-, 2R_1, 2S_1]$        |
| $[(\blacksquare)^{2T} + \Gamma_1^+ + \Gamma_1^-, T_3^+ + T_3^- + T_4^+ + T_4^-, Y_3^+ + Y_3^- + Y_4^+ + Y_4^-, Z_1^- + Z_2^- + Z_3^- + Z_4^-, 2R_1, 2S_1]$ |
| $[(\blacksquare)^{2T} + \Gamma_1^- + \Gamma_3^-, T_2^+ + 2T_4^+ + T_4^-, Y_2^+ + Y_3^+ + Y_3^- + Y_4^+, Z_2^+ + 2Z_4^+ + Z_4^-, 2R_1, 2S_1]$               |
| $[(\blacksquare)^{2T} + \Gamma_1^- + \Gamma_3^-, T_1^- + T_3^- + T_4^+ + T_4^-, Y_2^+ + Y_3^+ + Y_3^- + Y_4^+, Z_1^- + Z_3^- + Z_4^+ + Z_4^-, 2R_1, 2S_1]$ |
| $[(\blacksquare)^{2T} + \Gamma_3^- + \Gamma_4^+, T_1^- + T_2^+ + T_4^+ + T_4^-, 2Y_2^+ + Y_3^+ + Y_4^+, Z_3^- + 2Z_4^+ + Z_4^-, 2R_1, 2S_1]$               |
| $[(\blacksquare)^{2T} + \Gamma_1^+ + \Gamma_1^-, T_2^+ + T_2^- + T_4^+ + T_4^-, Y_1^+ + Y_2^+ + Y_3^+ + Y_4^+, Z_2^+ + Z_2^- + Z_4^+ + Z_4^-, 2R_1, 2S_1]$ |
| $[(\blacksquare)^{2T} + \Gamma_1^+ + \Gamma_4^+, T_1^- + T_4^+ + 2T_4^-, Y_2^+ + Y_3^+ + Y_4^+ + Y_4^-, Z_1^+ + 2Z_4^+ + Z_4^-, 2R_1, 2S_1]$               |
| $[(\blacksquare)^{2T} + \Gamma_1^- + \Gamma_4^-, T_2^- + T_3^- + T_4^+ + T_4^-, Y_2^- + Y_3^- + Y_4^+ + Y_4^-, Z_2^+ + Z_3^+ + Z_4^+ + Z_4^-, 2R_1, 2S_1]$ |
| $[(\blacksquare)^{2T} + \Gamma_3^+ + \Gamma_4^-, T_1^+ + T_2^- + T_4^+ + T_4^-, 2Y_2^- + Y_3^- + Y_4^-, Z_3^+ + Z_4^+ + 2Z_4^-, 2R_1, 2S_1]$               |
| $[(\blacksquare)^{2T} + \Gamma_1^+ + \Gamma_1^-, T_2^+ + T_2^- + T_4^+ + T_4^-, Y_1^- + Y_2^- + Y_3^- + Y_4^-, Z_2^+ + Z_2^- + Z_4^+ + Z_4^-, 2R_1, 2S_1]$ |
| $[(\blacksquare)^{2T} + \Gamma_1^+ + \Gamma_1^-, T_1^+ + T_1^- + T_4^+ + T_4^-, Y_1^- + Y_2^- + Y_3^- + Y_4^-, Z_1^+ + Z_1^- + Z_4^+ + Z_4^-, 2R_1, 2S_1]$ |
| $[(\blacksquare)^{2T} + \Gamma_1^+ + \Gamma_3^+, T_2^- + T_4^+ + 2T_4^-, Y_2^- + Y_3^+ + Y_3^- + Y_4^-, Z_2^- + Z_4^+ + 2Z_4^-, 2R_1, 2S_1]$               |
| $[(\blacksquare)^{2T} + \Gamma_1^+ + \Gamma_3^+, T_1^+ + T_3^+ + T_4^+ + T_4^-, Y_2^- + Y_3^+ + Y_3^- + Y_4^-, Z_1^+ + Z_3^+ + Z_4^+ + Z_4^-, 2R_1, 2S_1]$ |
| $[(\blacksquare)^{2T} + \Gamma_1^- + \Gamma_3^-, T_1^+ + T_1^- + T_2^+ + T_4^+, Y_1^- + Y_2^+ + Y_2^- + Y_3^-, Z_1^- + Z_3^- + Z_4^+ + Z_4^-, 2R_1, 2S_1]$ |
| $[(\blacksquare)^{2T} + \Gamma_1^- + \Gamma_2^+, T_2^+ + T_2^- + T_3^- + T_4^+, Y_2^+ + Y_2^- + Y_3^- + Y_4^+, 2Z_2^+ + Z_3^+ + Z_4^+, 2R_1, 2S_1]$        |
| $[(\blacksquare)^{2T} + \Gamma_1^+ + \Gamma_1^-, T_3^+ + T_3^- + T_4^+ + T_4^-, Y_3^+ + Y_3^- + Y_4^+ + Y_4^-, Z_1^+ + Z_2^+ + Z_3^+ + Z_4^+, 2R_1, 2S_1]$ |
| $[(\blacksquare)^{2T} + \Gamma_1^+ + \Gamma_1^-, T_1^+ + T_2^+ + T_3^+ + T_4^+, Y_1^- + Y_2^- + Y_3^- + Y_4^-, Z_1^+ + Z_2^+ + Z_3^+ + Z_4^+, 2R_1, 2S_1]$ |

... continued on next page

... continued from previous page

$$\begin{aligned}
&[(\blacksquare)^{2T} + \Gamma_2^+ + \Gamma_3^+, T_1^+ + T_2^+ + T_2^- + T_4^+, Y_2^+ + 2Y_2^- + Y_3^-, Z_2^+ + Z_3^+ + Z_4^+ + Z_4^-, 2R_1, 2S_1] \\
&[(\blacksquare)^{2T} + \Gamma_1^+ + \Gamma_1^-, T_1^- + T_2^- + T_3^- + T_4^-, Y_1^- + Y_2^- + Y_3^- + Y_4^-, Z_1^- + Z_2^- + Z_3^- + Z_4^-, 2R_1, 2S_1] \\
&[(\blacksquare)^{2T} + \Gamma_4^+ + \Gamma_4^-, T_1^- + T_2^- + T_3^- + T_4^-, Y_2^+ + Y_2^- + Y_4^+ + Y_4^-, Z_3^+ + Z_3^- + Z_4^+ + Z_4^-, 2R_1, 2S_1] \\
&[(\blacksquare)^{2T} + \Gamma_1^+ + \Gamma_2^-, T_1^- + T_2^- + 2T_4^-, Y_2^+ + Y_2^- + Y_3^+ + Y_4^-, Z_1^+ + Z_2^- + Z_4^+ + Z_4^-, 2R_1, 2S_1] \\
&[(\blacksquare)^{2T} + \Gamma_2^- + \Gamma_4^-, T_1^+ + T_1^- + T_2^- + T_4^-, Y_2^+ + 2Y_2^- + Y_4^-, Z_1^+ + Z_3^+ + Z_4^+ + Z_4^-, 2R_1, 2S_1] \\
&[(\blacksquare)^{2T} + \Gamma_1^+ + \Gamma_3^+, T_2^- + T_3^+ + T_3^- + T_4^-, Y_2^- + Y_3^+ + Y_3^- + Y_4^-, Z_2^- + Z_3^+ + Z_3^- + Z_4^-, 2R_1, 2S_1] \\
&[(\blacksquare)^{2T} + \Gamma_1^+ + \Gamma_4^+, T_1^- + T_2^+ + T_2^- + T_4^-, Y_1^- + Y_2^+ + Y_2^- + Y_4^-, Z_2^- + Z_3^- + Z_4^+ + Z_4^-, 2R_1, 2S_1] \\
&[(\blacksquare)^{2T} + \Gamma_1^+ + \Gamma_1^-, T_1^+ + T_2^+ + T_3^+ + T_4^-, Y_1^- + Y_2^- + Y_3^- + Y_4^-, Z_1^- + Z_2^- + Z_3^- + Z_4^-, 2R_1, 2S_1] \\
&[(\blacksquare)^{2T} + \Gamma_1^+ + \Gamma_1^-, T_1^- + T_2^- + T_3^- + T_4^-, Y_1^+ + Y_2^+ + Y_3^+ + Y_4^+, Z_1^- + Z_2^- + Z_3^- + Z_4^-, 2R_1, 2S_1] \\
&[(\blacksquare)^{2T} + \Gamma_1^- + \Gamma_2^-, T_1^- + T_2^- + 2T_3^-, Y_2^+ + Y_2^- + Y_3^- + Y_4^+, Z_1^- + Z_2^+ + Z_3^+ + Z_3^-, 2R_1, 2S_1] \\
&[(\blacksquare)^{2T} + \Gamma_1^+ + \Gamma_1^-, T_1^+ + T_1^- + T_3^+ + T_3^-, Y_1^- + Y_2^- + Y_3^- + Y_4^-, Z_1^+ + Z_1^- + Z_3^+ + Z_3^-, 2R_1, 2S_1] \\
&[(\blacksquare)^{2T} + \Gamma_2^+ + \Gamma_3^+, T_1^+ + T_1^- + T_2^- + T_3^-, Y_2^+ + 2Y_2^- + Y_3^-, Z_1^- + Z_3^+ + Z_3^- + Z_4^-, 2R_1, 2S_1] \\
&[(\blacksquare)^{2T} + \Gamma_1^- + \Gamma_4^-, T_1^+ + T_1^- + T_2^- + T_3^-, Y_1^+ + Y_2^+ + Y_2^- + Y_4^+, Z_1^- + Z_3^+ + Z_3^- + Z_4^-, 2R_1, 2S_1] \\
&[(\blacksquare)^{2T} + \Gamma_2^+ + \Gamma_2^-, T_1^+ + T_1^- + T_2^+ + T_2^-, 2Y_2^+ + 2Y_2^-, Z_1^- + Z_2^- + Z_3^- + Z_4^-, 2R_1, 2S_1] \\
&[(\blacksquare)^{2T} + \Gamma_1^+ + \Gamma_1^-, T_1^+ + T_1^- + T_2^+ + T_2^-, Y_1^+ + Y_1^- + Y_2^+ + Y_2^-, Z_1^- + Z_2^- + Z_3^- + Z_4^-, 2R_1, 2S_1] \\
&[(\blacksquare)^{2T} + \Gamma_2^- + \Gamma_3^-, T_1^- + T_2^+ + T_2^- + T_4^-, 2Y_2^+ + Y_2^- + Y_3^+, Z_2^- + Z_3^- + Z_4^+ + Z_4^-, 2R_1, 2S_1] \\
&[(\blacksquare)^{2T} + \Gamma_1^- + \Gamma_4^-, T_2^- + T_3^+ + 2T_3^-, Y_2^- + Y_3^- + Y_4^+ + Y_4^-, Z_2^+ + 2Z_3^+ + Z_3^-, 2R_1, 2S_1] \\
&[(\blacksquare)^{2T} + \Gamma_1^+ + \Gamma_1^-, T_1^- + T_2^- + T_3^- + T_4^-, Y_1^+ + Y_2^+ + Y_3^+ + Y_4^+, Z_1^+ + Z_2^+ + Z_3^+ + Z_4^+, 2R_1, 2S_1] \\
&[(\blacksquare)^{2T} + \Gamma_2^+ + \Gamma_4^+, T_1^- + T_2^+ + T_2^- + T_3^-, 2Y_2^+ + Y_2^- + Y_4^+, Z_2^+ + Z_3^+ + Z_3^- + Z_4^+, 2R_1, 2S_1] \\
&[(\blacksquare)^{2T} + \Gamma_3^+ + \Gamma_4^-, T_1^+ + T_2^- + T_3^+ + T_3^-, 2Y_2^- + Y_3^- + Y_4^-, 2Z_3^+ + Z_3^- + Z_4^-, 2R_1, 2S_1] \\
&[(\blacksquare)^{2T} + \Gamma_1^+ + \Gamma_1^-, T_2^+ + T_2^- + T_3^+ + T_3^-, Y_1^- + Y_2^- + Y_3^- + Y_4^-, Z_2^+ + Z_2^- + Z_3^+ + Z_3^-, 2R_1, 2S_1] \\
&[(\blacksquare)^{2T} + \Gamma_1^+ + \Gamma_3^+, T_1^+ + 2T_3^+ + T_3^-, Y_2^- + Y_3^+ + Y_3^- + Y_4^-, Z_1^+ + 2Z_3^+ + Z_3^-, 2R_1, 2S_1] \\
&[(\blacksquare)^{2T} + \Gamma_1^- + \Gamma_4^-, T_1^+ + T_2^+ + T_2^- + T_4^+, Y_1^+ + Y_2^+ + Y_2^- + Y_4^+, Z_2^+ + Z_3^+ + Z_4^+ + Z_4^-, 2R_1, 2S_1] \\
&[(\blacksquare)^{2T} + \Gamma_2^- + \Gamma_4^-, T_1^+ + T_2^+ + T_2^- + T_3^-, Y_2^+ + 2Y_2^- + Y_4^-, Z_2^- + Z_3^+ + Z_3^- + Z_4^-, 2R_1, 2S_1] \\
&[(\blacksquare)^{2T} + \Gamma_1^- + \Gamma_3^-, T_1^- + T_2^+ + T_2^- + T_3^-, Y_1^- + Y_2^+ + Y_2^- + Y_3^-, Z_2^+ + Z_3^+ + Z_3^- + Z_4^+, 2R_1, 2S_1] \\
&[(\blacksquare)^{2T} + \Gamma_1^+ + \Gamma_2^-, T_1^+ + T_1^- + T_3^+ + T_4^-, Y_2^+ + Y_2^- + Y_3^+ + Y_4^-, 2Z_1^+ + Z_3^+ + Z_4^+, 2R_1, 2S_1] \\
&[(\blacksquare)^{2T} + \Gamma_1^+ + \Gamma_3^+, T_1^+ + T_1^- + T_2^- + T_4^-, Y_1^+ + Y_2^+ + Y_2^- + Y_3^+, Z_1^+ + Z_3^+ + Z_4^+ + Z_4^-, 2R_1, 2S_1] \\
&[(\blacksquare)^{2T} + \Gamma_1^+ + \Gamma_1^-, T_1^+ + T_2^+ + T_3^+ + T_4^-, Y_1^+ + Y_2^+ + Y_3^+ + Y_4^+, Z_1^+ + Z_2^+ + Z_3^+ + Z_4^+, 2R_1, 2S_1] \\
&[(\blacksquare)^{2T} + \Gamma_1^+ + \Gamma_4^+, T_1^+ + T_1^- + T_2^+ + T_3^-, Y_1^- + Y_2^+ + Y_2^- + Y_4^-, Z_1^+ + Z_3^+ + Z_3^- + Z_4^+, 2R_1, 2S_1] \\
&[(\blacksquare)^{2T} + \Gamma_1^+ + \Gamma_1^-, T_1^- + T_2^- + T_3^- + T_4^-, Y_1^- + Y_2^- + Y_3^- + Y_4^-, Z_1^- + Z_2^- + Z_3^- + Z_4^+, 2R_1, 2S_1] \\
&[(\blacksquare)^{2T} + \Gamma_2^+ + \Gamma_2^-, T_1^+ + T_1^- + T_2^+ + T_2^-, 2Y_2^+ + 2Y_2^-, Z_1^+ + Z_2^+ + Z_3^+ + Z_4^+, 2R_1, 2S_1] \\
&[(\blacksquare)^{2T} + \Gamma_1^+ + \Gamma_1^-, T_1^+ + T_1^- + T_2^+ + T_2^-, Y_1^+ + Y_1^- + Y_2^+ + Y_2^-, Z_1^+ + Z_2^+ + Z_3^+ + Z_4^+, 2R_1, 2S_1] \\
&[(\blacksquare)^{2T} + \Gamma_3^+ + \Gamma_3^-, T_1^- + T_2^- + T_3^- + T_4^-, Y_2^+ + Y_2^- + Y_3^+ + Y_3^-, Z_3^+ + Z_3^- + Z_4^+ + Z_4^-, 2R_1, 2S_1] \\
&[(\blacksquare)^{2T} + \Gamma_4^+ + \Gamma_4^-, T_1^+ + T_2^+ + T_3^+ + T_4^+, Y_2^+ + Y_2^- + Y_4^+ + Y_4^-, Z_3^+ + Z_3^- + Z_4^+ + Z_4^-, 2R_1, 2S_1]
\end{aligned}$$

2nd minimal solution:  $\mu_2^T = 6$  (1422 symmetry vectors)

Space group 68 ( $\mathbb{Z}_2$ )

1st minimal solution:  $\mu_1^T = 2$  (1 symmetry vector & filling-enforced topology)

|                                                            |                                 |
|------------------------------------------------------------|---------------------------------|
| $\mathbf{n}^T$                                             | $\mathbf{v}^T \in \mathbb{Z}_2$ |
| $[(\blacksquare)^{2T}, T_1, Y_2^+ + Y_2^-, Z_2, R_1, S_1]$ | 1                               |

2nd minimal solution:  $\mu_2^T = 4$  (7 symmetry vectors)

Space group 69 ( $\mathbb{Z}_1$ )

1st minimal solution:  $\mu_1^T = 3$  (56 symmetry vectors)



... continued from previous page

---

|                                                                                                              |
|--------------------------------------------------------------------------------------------------------------|
| $[(\bullet)^{2T} + \Gamma_1^-, T_2^+ + T_3^+ + T_4^-, Y_2^+ + Y_3^+ + Y_4^-, Z_2^+ + Z_3^+ + Z_4^-, 3L_1^+]$ |
| $[(\bullet)^{2T} + \Gamma_1^-, T_2^+ + T_3^+ + T_4^-, Y_1^- + Y_3^+ + Y_3^-, Z_1^- + Z_3^+ + Z_3^-, 3L_1^+]$ |
| $[(\bullet)^{2T} + \Gamma_1^-, T_1^- + T_2^+ + T_2^-, Y_1^- + Y_2^+ + Y_2^-, Z_2^+ + Z_3^+ + Z_4^-, 3L_1^+]$ |

---

2nd minimal solution:  $\mu_2^T = 4$  (650 symmetry vectors)

Space group 70 ( $\mathbb{Z}_2$ )

1st minimal solution:  $\mu_1^T = 2$  (3 symmetry vectors)

---

| $\mathbf{n}^T$                                   | $\mathbf{v}^T \in \mathbb{Z}_2$ |
|--------------------------------------------------|---------------------------------|
| $[(\bullet)^{2T}, T_2, Y_2, Z_2, 2L_1^-]$        | trivial                         |
| $[(\bullet)^{2T}, T_2, Y_2, Z_2, L_1^+ + L_1^-]$ | 1                               |
| $[(\bullet)^{2T}, T_2, Y_2, Z_2, 2L_1^+]$        | trivial                         |

---

2nd minimal solution:  $\mu_2^T = 4$  (20 symmetry vectors)

Space group 71 ( $\mathbb{Z}_1$ )

1st minimal solution:  $\mu_1^T = 3$  (168 symmetry vectors)

---

| $\mathbf{n}^T$                                                                                                                               |
|----------------------------------------------------------------------------------------------------------------------------------------------|
| $[(\bullet)^{2T} + \Gamma_1^+, X_2^- + X_3^- + X_4^-, R_2^+ + 2R_2^-, 2S_1^+ + S_1^-, T_2^+ + 2T_2^-, 3W_3]$                                 |
| $[(\bullet)^{2T} + \Gamma_1^+, X_2^- + X_3^- + X_4^-, R_2^+ + 2R_2^-, S_1^+ + S_1^- + S_2^-, T_1^+ + T_2^+ + T_2^-, W_2 + 2W_3]$             |
| $[(\bullet)^{2T} + \Gamma_1^+, X_2^- + X_3^- + X_4^-, R_1^+ + R_2^+ + R_2^-, S_1^+ + S_1^- + S_2^-, T_2^+ + 2T_2^-, 2W_3 + W_4]$             |
| $[(\bullet)^{2T} + \Gamma_1^+, X_2^- + X_3^- + X_4^-, R_1^+ + R_2^+ + R_2^-, 2S_1^+ + S_1^-, T_1^+ + T_2^+ + T_2^-, W_1 + 2W_3]$             |
| $[(\bullet)^{2T} + \Gamma_1^+, X_2^- + X_3^- + X_4^-, R_2^+ + 2R_2^-, S_1^+ + S_1^- + S_2^-, T_1^+ + 2T_2^-, W_2 + 2W_3]$                    |
| $[(\bullet)^{2T} + \Gamma_1^+, X_2^- + X_3^- + X_4^-, R_2^+ + 2R_2^-, S_1^- + 2S_2^-, T_1^+ + T_1^- + T_2^-, 2W_2 + W_3]$                    |
| $[(\bullet)^{2T} + \Gamma_1^+, X_2^- + X_3^- + X_4^-, R_1^+ + R_2^+ + R_2^-, S_1^- + 2S_2^-, T_1^+ + 2T_2^-, W_2 + W_3 + W_4]$               |
| $[(\bullet)^{2T} + \Gamma_1^+, X_2^- + X_3^- + X_4^-, R_1^+ + R_2^+ + R_2^-, S_1^+ + S_1^- + S_2^-, T_1^+ + T_1^- + T_2^-, W_1 + W_2 + W_3]$ |
| $[(\bullet)^{2T} + \Gamma_1^+, X_2^- + X_3^- + X_4^-, R_1^+ + R_2^+ + R_2^-, S_1^- + 2S_2^-, T_1^+ + T_2^+ + T_2^-, W_2 + W_3 + W_4]$        |
| $[(\bullet)^{2T} + \Gamma_1^+, X_2^- + X_3^- + X_4^-, 2R_1^+ + R_2^+, S_1^- + 2S_2^-, T_2^+ + 2T_2^-, W_3 + 2W_4]$                           |
| $[(\bullet)^{2T} + \Gamma_1^+, X_2^- + X_3^- + X_4^-, 2R_1^+ + R_2^+, S_1^+ + S_1^- + S_2^-, T_1^+ + T_2^+ + T_2^-, W_1 + W_3 + W_4]$        |
| $[(\bullet)^{2T} + \Gamma_1^+, X_2^- + X_3^- + X_4^-, R_1^+ + R_2^+ + R_2^-, 2S_1^+ + S_1^-, T_1^- + 2T_2^-, W_1 + 2W_3]$                    |
| $[(\bullet)^{2T} + \Gamma_1^+, X_2^- + X_3^- + X_4^-, 2R_1^+ + R_2^+, S_1^+ + S_1^- + S_2^-, T_1^- + 2T_2^-, W_1 + W_3 + W_4]$               |
| $[(\bullet)^{2T} + \Gamma_1^+, X_2^- + X_3^- + X_4^-, 2R_1^+ + R_2^+, 2S_1^+ + S_1^-, T_1^+ + T_1^- + T_2^-, 2W_1 + W_3]$                    |
| $[(\bullet)^{2T} + \Gamma_1^+, X_2^- + X_3^- + X_4^-, R_2^+ + 2R_2^-, S_1^- + 2S_2^-, 2T_1^+ + T_2^+, 2W_2 + W_3]$                           |
| $[(\bullet)^{2T} + \Gamma_1^+, X_2^- + X_3^- + X_4^-, R_1^+ + R_2^+ + R_2^-, S_1^+ + S_1^- + S_2^-, 2T_1^+ + T_2^+, W_1 + W_2 + W_3]$        |
| $[(\bullet)^{2T} + \Gamma_1^+, X_2^- + X_3^- + X_4^-, R_1^+ + R_2^+ + R_2^-, S_1^- + 2S_2^-, 2T_1^+ + T_1^-, W_1 + 2W_2]$                    |
| $[(\bullet)^{2T} + \Gamma_1^+, X_2^- + X_3^- + X_4^-, 2R_1^+ + R_2^+, S_1^- + 2S_2^-, 2T_1^+ + T_2^+, W_1 + W_2 + W_4]$                      |
| $[(\bullet)^{2T} + \Gamma_1^+, X_2^- + X_3^- + X_4^-, 2R_1^+ + R_2^+, S_1^- + 2S_2^-, T_1^+ + T_1^- + T_2^-, W_1 + W_2 + W_4]$               |
| $[(\bullet)^{2T} + \Gamma_1^+, X_2^- + X_3^- + X_4^-, 2R_1^+ + R_2^+, S_1^+ + S_1^- + S_2^-, 2T_1^+ + T_1^-, 2W_1 + W_2]$                    |
| $[(\bullet)^{2T} + \Gamma_1^+, X_2^- + X_3^- + X_4^-, R_1^- + 2R_2^-, S_1^+ + S_1^- + S_2^-, T_2^+ + 2T_2^-, 2W_3 + W_4]$                    |
| $[(\bullet)^{2T} + \Gamma_1^+, X_2^- + X_3^- + X_4^-, R_1^- + 2R_2^-, S_1^- + 2S_2^-, T_1^+ + T_2^+ + T_2^-, W_2 + W_3 + W_4]$               |
| $[(\bullet)^{2T} + \Gamma_1^+, X_2^- + X_3^- + X_4^-, R_1^+ + R_1^- + R_2^-, S_1^- + 2S_2^-, T_2^+ + 2T_2^-, W_3 + 2W_4]$                    |
| $[(\bullet)^{2T} + \Gamma_1^+, X_2^- + X_3^- + X_4^-, R_1^+ + R_1^- + R_2^-, S_1^+ + S_1^- + S_2^-, T_1^+ + T_2^+ + T_2^-, W_1 + W_3 + W_4]$ |
| $[(\bullet)^{2T} + \Gamma_1^+, X_2^- + X_3^- + X_4^-, R_1^- + 2R_2^-, S_1^- + 2S_2^-, T_1^- + 2T_2^-, W_2 + W_3 + W_4]$                      |

---

... continued on next page



... continued on next page

... continued from previous page

---

|                                                                                                                                                   |
|---------------------------------------------------------------------------------------------------------------------------------------------------|
| $[(\blacksquare)^{2T} + \Gamma_1^-, X_2^+ + X_3^+ + X_4^+, R_1^+ + 2R_2^+, S_1^+ + S_1^- + S_2^+, 2T_1^- + T_2^-, W_1 + W_2 + W_3]$               |
| $[(\blacksquare)^{2T} + \Gamma_1^-, X_2^+ + X_3^+ + X_4^+, R_1^+ + 2R_2^+, S_1^- + S_2^+ + S_2^-, T_1^+ + 2T_2^+, W_2 + W_3 + W_4]$               |
| $[(\blacksquare)^{2T} + \Gamma_1^-, X_2^+ + X_3^+ + X_4^+, R_1^+ + 2R_2^+, S_1^+ + 2S_2^+, T_1^+ + 2T_2^+, W_2 + W_3 + W_4]$                      |
| $[(\blacksquare)^{2T} + \Gamma_1^-, X_2^+ + X_3^+ + X_4^+, R_1^+ + 2R_2^+, 2S_2^+ + S_2^-, T_1^+ + T_1^- + T_2^+, 2W_2 + W_4]$                    |
| $[(\blacksquare)^{2T} + \Gamma_1^-, X_2^+ + X_3^+ + X_4^+, R_1^+ + 2R_2^+, S_1^+ + 2S_1^-, T_1^+ + 2T_2^+, W_1 + 2W_3]$                           |
| $[(\blacksquare)^{2T} + \Gamma_1^-, X_2^+ + X_3^+ + X_4^+, R_1^+ + 2R_2^+, 2S_1^- + S_2^-, T_1^+ + T_1^- + T_2^+, W_1 + W_2 + W_3]$               |
| $[(\blacksquare)^{2T} + \Gamma_1^-, X_2^+ + X_3^+ + X_4^+, R_1^+ + 2R_2^+, S_1^+ + S_1^- + S_2^+, T_1^+ + T_1^- + T_2^+, W_1 + W_2 + W_3]$        |
| $[(\blacksquare)^{2T} + \Gamma_1^-, X_2^+ + X_3^+ + X_4^+, R_1^+ + 2R_2^+, S_1^- + S_2^+ + S_2^-, T_1^+ + 2T_1^-, W_1 + 2W_2]$                    |
| $[(\blacksquare)^{2T} + \Gamma_1^-, X_2^+ + X_3^+ + X_4^+, R_1^+ + 2R_2^+, S_1^+ + 2S_2^+, T_1^+ + 2T_1^-, W_1 + 2W_2]$                           |
| $[(\blacksquare)^{2T} + \Gamma_1^-, X_2^+ + X_3^+ + X_4^+, R_1^+ + R_1^- + R_2^+, S_1^- + S_2^+ + S_2^-, 2T_2^+ + T_2^-, W_3 + 2W_4]$             |
| $[(\blacksquare)^{2T} + \Gamma_1^-, X_2^+ + X_3^+ + X_4^+, R_1^+ + R_1^- + R_2^+, S_1^+ + 2S_2^+, 2T_2^+ + T_2^-, W_3 + 2W_4]$                    |
| $[(\blacksquare)^{2T} + \Gamma_1^-, X_2^+ + X_3^+ + X_4^+, R_1^+ + R_1^- + R_2^+, 2S_2^+ + S_2^-, T_1^- + T_2^+ + T_2^-, W_2 + 2W_4]$             |
| $[(\blacksquare)^{2T} + \Gamma_1^-, X_2^+ + X_3^+ + X_4^+, R_1^+ + R_1^- + R_2^+, 2S_1^- + S_2^-, T_1^- + T_2^+ + T_2^-, W_1 + W_3 + W_4]$        |
| $[(\blacksquare)^{2T} + \Gamma_1^-, X_2^+ + X_3^+ + X_4^+, R_1^+ + R_1^- + R_2^+, S_1^+ + S_1^- + S_2^+, T_1^- + T_2^+ + T_2^-, W_1 + W_3 + W_4]$ |
| $[(\blacksquare)^{2T} + \Gamma_1^-, X_2^+ + X_3^+ + X_4^+, R_1^+ + R_1^- + R_2^+, S_1^- + S_2^+ + S_2^-, 2T_1^- + T_2^-, W_1 + W_2 + W_4]$        |
| $[(\blacksquare)^{2T} + \Gamma_1^-, X_2^+ + X_3^+ + X_4^+, R_1^+ + R_1^- + R_2^+, S_1^+ + 2S_2^+, 2T_1^- + T_2^-, W_1 + W_2 + W_4]$               |
| $[(\blacksquare)^{2T} + \Gamma_1^-, X_2^+ + X_3^+ + X_4^+, R_1^+ + R_1^- + R_2^+, S_1^+ + 2S_1^-, 2T_1^- + T_2^-, 2W_1 + W_3]$                    |
| $[(\blacksquare)^{2T} + \Gamma_1^-, X_2^+ + X_3^+ + X_4^+, R_1^+ + R_1^- + R_2^+, 2S_2^+ + S_2^-, T_1^+ + 2T_2^+, W_2 + 2W_4]$                    |
| $[(\blacksquare)^{2T} + \Gamma_1^-, X_2^+ + X_3^+ + X_4^+, R_1^+ + R_1^- + R_2^+, 2S_1^- + S_2^-, T_1^+ + 2T_2^+, W_1 + W_3 + W_4]$               |
| $[(\blacksquare)^{2T} + \Gamma_1^-, X_2^+ + X_3^+ + X_4^+, R_1^+ + R_1^- + R_2^+, S_1^+ + S_1^- + S_2^+, T_1^+ + 2T_2^+, W_1 + W_3 + W_4]$        |
| $[(\blacksquare)^{2T} + \Gamma_1^-, X_2^+ + X_3^+ + X_4^+, R_1^+ + R_1^- + R_2^+, S_1^- + S_2^+ + S_2^-, T_1^+ + T_1^- + T_2^+, W_1 + W_2 + W_4]$ |
| $[(\blacksquare)^{2T} + \Gamma_1^-, X_2^+ + X_3^+ + X_4^+, R_1^+ + R_1^- + R_2^+, S_1^+ + 2S_2^+, T_1^+ + T_1^- + T_2^+, W_1 + W_2 + W_4]$        |
| $[(\blacksquare)^{2T} + \Gamma_1^-, X_2^+ + X_3^+ + X_4^+, R_1^+ + R_1^- + R_2^+, S_1^+ + 2S_1^-, T_1^+ + T_1^- + T_2^+, 2W_1 + W_3]$             |
| $[(\blacksquare)^{2T} + \Gamma_1^-, X_2^+ + X_3^+ + X_4^+, R_1^+ + R_1^- + R_2^+, 2S_1^- + S_2^-, T_1^+ + 2T_1^-, 2W_1 + W_2]$                    |
| $[(\blacksquare)^{2T} + \Gamma_1^-, X_2^+ + X_3^+ + X_4^+, R_1^+ + R_1^- + R_2^+, S_1^+ + S_1^- + S_2^+, T_1^+ + 2T_1^-, 2W_1 + W_2]$             |
| $[(\blacksquare)^{2T} + \Gamma_1^-, X_2^+ + X_3^+ + X_4^+, R_1^+ + 2R_1^-, 2S_2^+ + S_2^-, 2T_2^+ + T_2^-, 3W_4]$                                 |
| $[(\blacksquare)^{2T} + \Gamma_1^-, X_2^+ + X_3^+ + X_4^+, R_1^+ + 2R_1^-, S_1^- + S_2^+ + S_2^-, T_1^- + T_2^+ + T_2^-, W_1 + 2W_4]$             |
| $[(\blacksquare)^{2T} + \Gamma_1^-, X_2^+ + X_3^+ + X_4^+, R_1^+ + 2R_1^-, S_1^+ + 2S_2^+, T_1^- + T_2^+ + T_2^-, W_1 + 2W_4]$                    |
| $[(\blacksquare)^{2T} + \Gamma_1^-, X_2^+ + X_3^+ + X_4^+, R_1^+ + 2R_1^-, 2S_1^- + S_2^-, 2T_1^- + T_2^-, 2W_1 + W_4]$                           |
| $[(\blacksquare)^{2T} + \Gamma_1^-, X_2^+ + X_3^+ + X_4^+, R_1^+ + 2R_1^-, S_1^+ + S_1^- + S_2^+, 2T_1^- + T_2^-, 2W_1 + W_4]$                    |
| $[(\blacksquare)^{2T} + \Gamma_1^-, X_2^+ + X_3^+ + X_4^+, R_1^+ + 2R_1^-, S_1^- + S_2^+ + S_2^-, T_1^+ + 2T_2^+, W_1 + 2W_4]$                    |
| $[(\blacksquare)^{2T} + \Gamma_1^-, X_2^+ + X_3^+ + X_4^+, R_1^+ + 2R_1^-, S_1^+ + 2S_2^+, T_1^+ + 2T_2^+, W_1 + 2W_4]$                           |
| $[(\blacksquare)^{2T} + \Gamma_1^-, X_2^+ + X_3^+ + X_4^+, R_1^+ + 2R_1^-, 2S_1^- + S_2^-, T_1^+ + T_1^- + T_2^+, 2W_1 + W_4]$                    |
| $[(\blacksquare)^{2T} + \Gamma_1^-, X_2^+ + X_3^+ + X_4^+, R_1^+ + 2R_1^-, S_1^+ + S_1^- + S_2^+, T_1^+ + T_1^- + T_2^+, 2W_1 + W_4]$             |
| $[(\blacksquare)^{2T} + \Gamma_1^-, X_2^+ + X_3^+ + X_4^+, R_1^+ + 2R_1^-, S_1^+ + 2S_1^-, T_1^+ + 2T_1^-, 3W_1]$                                 |

---

2nd minimal solution:  $\mu_2^T = 4$  (3602 symmetry vectors)

Space group 72 ( $\mathbb{Z}_4$ )

1st minimal solution:  $\mu_1^T = 4$  (18 symmetry vectors)

---

| $\mathbf{n}^T$                                                                                                                               |
|----------------------------------------------------------------------------------------------------------------------------------------------|
| $[(\blacksquare)^{2T} + \Gamma_1^- + \Gamma_2^-, X_2^+ + X_2^- + X_3^+ + X_4^+, 2R_1, 2S_1, 3T_2^+ + T_2^-, 2W_3W_4]$                        |
| $[(\blacksquare)^{2T} + \Gamma_1^- + \Gamma_2^-, X_2^+ + X_2^- + X_3^+ + X_4^+, 2R_1, 2S_1, 2T_1^- + T_2^+ + T_2^-, W_1W_2 + W_3W_4]$        |
| $[(\blacksquare)^{2T} + \Gamma_1^+ + \Gamma_1^-, X_1^+ + X_2^+ + X_3^+ + X_4^+, 2R_1, 2S_1, 2T_2^+ + 2T_2^-, 2W_3W_4]$                       |
| $[(\blacksquare)^{2T} + \Gamma_1^+ + \Gamma_1^-, X_1^+ + X_2^+ + X_3^+ + X_4^+, 2R_1, 2S_1, T_1^+ + T_1^- + T_2^+ + T_2^-, W_1W_2 + W_3W_4]$ |
| $[(\blacksquare)^{2T} + \Gamma_1^+ + \Gamma_1^-, X_1^+ + X_2^+ + X_3^+ + X_4^+, 2R_1, 2S_1, 2T_1^- + 2T_2^-, W_1W_2 + W_3W_4]$               |
| $[(\blacksquare)^{2T} + \Gamma_1^+ + \Gamma_1^-, X_1^- + X_2^- + X_3^- + X_4^-, 2R_1, 2S_1, 2T_2^+ + 2T_2^-, 2W_3W_4]$                       |
| $[(\blacksquare)^{2T} + \Gamma_1^+ + \Gamma_1^-, X_1^- + X_2^- + X_3^- + X_4^-, 2R_1, 2S_1, T_1^+ + T_1^- + T_2^+ + T_2^-, W_1W_2 + W_3W_4]$ |
| $[(\blacksquare)^{2T} + \Gamma_1^+ + \Gamma_2^-, X_2^+ + X_2^- + X_3^- + X_4^-, 2R_1, 2S_1, T_2^+ + 3T_2^-, 2W_3W_4]$                        |

---

... continued on next page



... continued from previous page

---

|                                                                                                                                       |
|---------------------------------------------------------------------------------------------------------------------------------------|
| $[(\blacksquare)^{2T} + \Gamma_1^+ + \Gamma_2^+, X_2^+ + X_2^- + X_3^- + X_4^-, 2R_1, 2S_1, 2T_1^+ + T_2^- + T_2^-, W_1W_2 + W_3W_4]$ |
| $[(\blacksquare)^{2T} + \Gamma_1^+ + \Gamma_1^-, X_1^- + X_2^- + X_3^- + X_4^-, 2R_1, 2S_1, 2T_1^- + 2T_2^-, W_1W_2 + W_3W_4]$        |
| $[(\blacksquare)^{2T} + \Gamma_1^+ + \Gamma_2^+, X_2^+ + X_2^- + X_3^- + X_4^-, 2R_1, 2S_1, T_1^+ + T_1^- + 2T_2^-, W_1W_2 + W_3W_4]$ |
| $[(\blacksquare)^{2T} + \Gamma_1^- + \Gamma_2^-, X_2^+ + X_2^- + X_3^+ + X_4^+, 2R_1, 2S_1, T_1^+ + T_1^- + 2T_2^+, W_1W_2 + W_3W_4]$ |
| $[(\blacksquare)^{2T} + \Gamma_1^+ + \Gamma_1^-, X_1^- + X_2^- + X_3^- + X_4^-, 2R_1, 2S_1, 2T_1^+ + 2T_2^+, W_1W_2 + W_3W_4]$        |
| $[(\blacksquare)^{2T} + \Gamma_1^- + \Gamma_2^-, X_2^+ + X_2^- + X_3^+ + X_4^+, 2R_1, 2S_1, T_1^+ + 3T_1^-, 2W_1W_2]$                 |
| $[(\blacksquare)^{2T} + \Gamma_1^+ + \Gamma_1^-, X_1^- + X_2^- + X_3^- + X_4^-, 2R_1, 2S_1, 2T_1^+ + 2T_1^-, 2W_1W_2]$                |
| $[(\blacksquare)^{2T} + \Gamma_1^+ + \Gamma_1^-, X_1^+ + X_2^+ + X_3^+ + X_4^+, 2R_1, 2S_1, 2T_1^+ + 2T_1^-, 2W_1W_2]$                |
| $[(\blacksquare)^{2T} + \Gamma_1^+ + \Gamma_2^+, X_2^+ + X_2^- + X_3^- + X_4^-, 2R_1, 2S_1, 3T_1^+ + T_1^-, 2W_1W_2]$                 |
| $[(\blacksquare)^{2T} + \Gamma_1^+ + \Gamma_1^-, X_1^+ + X_2^+ + X_3^+ + X_4^+, 2R_1, 2S_1, 2T_1^+ + 2T_2^+, W_1W_2 + W_3W_4]$        |

---

2nd minimal solution:  $\mu_2^T = 6$  (216 symmetry vectors)

Space group 73 ( $\mathbb{Z}_1$ )

1st minimal solution:  $\mu_1^T = 4$  (2 symmetry vectors)

---

| $\mathbf{n}^T$                                                                                             |
|------------------------------------------------------------------------------------------------------------|
| $[(\blacksquare)^{2T} + \Gamma_1^+ + \Gamma_1^-, X_1^+ + X_2^+ + X_3^+ + X_4^+, 2R_1, 2S_1, 2T_1, W_1W_1]$ |
| $[(\blacksquare)^{2T} + \Gamma_1^+ + \Gamma_1^-, X_1^- + X_2^- + X_3^- + X_4^-, 2R_1, 2S_1, 2T_1, W_1W_1]$ |

---

2nd minimal solution:  $\mu_2^T = 8$  (26 symmetry vectors)

Space group 74 ( $\mathbb{Z}_1$ )

1st minimal solution:  $\mu_1^T = 2$  (4 symmetry vectors)

---

| $\mathbf{n}^T$                                                                 |
|--------------------------------------------------------------------------------|
| $[(\blacksquare)^{2T}, X_4^+ + X_4^-, R_1^+ + R_2^+, S_1^- + S_2^-, T_1, W_1]$ |
| $[(\blacksquare)^{2T}, X_4^+ + X_4^-, R_1^+ + R_2^+, S_1^+ + S_2^+, T_1, W_1]$ |
| $[(\blacksquare)^{2T}, X_4^+ + X_4^-, R_1^- + R_2^-, S_1^- + S_2^-, T_1, W_1]$ |
| $[(\blacksquare)^{2T}, X_4^+ + X_4^-, R_1^- + R_2^-, S_1^+ + S_2^+, T_1, W_1]$ |

---

2nd minimal solution:  $\mu_2^T = 4$  (82 symmetry vectors)

Space group 75 ( $\mathbb{Z}_2$ )

1st minimal solution:  $\mu_1^T = 2$  (12 symmetry vectors)

---

| $\mathbf{n}^T$                                                        | $\mathbf{v}^T \in \mathbb{Z}_2$ |
|-----------------------------------------------------------------------|---------------------------------|
| $[(\blacksquare)^{2T}, A_3A_4, M_3M_4, Z_3Z_4, 2R_1, 2X_1]$           | trivial                         |
| $[(\blacksquare)^{2T}, A_3A_4, M_3M_4, Z_3Z_4, R_1 + R_2, X_1 + X_2]$ | 1                               |
| $[(\blacksquare)^{2T}, A_3A_4, M_3M_4, Z_3Z_4, 2R_2, 2X_2]$           | trivial                         |
| $[(\blacksquare)^{2T}, 2A_2, 2M_2, Z_3Z_4, 2R_1, 2X_1]$               | trivial                         |

---

... continued on next page

... continued from previous page

|                                                                             |         |
|-----------------------------------------------------------------------------|---------|
| $[(\blacksquare)^{2T}, 2A_2, 2M_2, Z_3Z_4, R_1 + R_2, X_1 + X_2]$           | 1       |
| $[(\blacksquare)^{2T}, 2A_2, 2M_2, Z_3Z_4, 2R_2, 2X_2]$                     | trivial |
| $[(\blacksquare)^{2T}, A_1 + A_2, M_1 + M_2, Z_3Z_4, 2R_1, 2X_1]$           | 1       |
| $[(\blacksquare)^{2T}, A_1 + A_2, M_1 + M_2, Z_3Z_4, R_1 + R_2, X_1 + X_2]$ | trivial |
| $[(\blacksquare)^{2T}, A_1 + A_2, M_1 + M_2, Z_3Z_4, 2R_2, 2X_2]$           | 1       |
| $[(\blacksquare)^{2T}, 2A_1, 2M_1, Z_3Z_4, 2R_1, 2X_1]$                     | trivial |
| $[(\blacksquare)^{2T}, 2A_1, 2M_1, Z_3Z_4, R_1 + R_2, X_1 + X_2]$           | 1       |
| $[(\blacksquare)^{2T}, 2A_1, 2M_1, Z_3Z_4, 2R_2, 2X_2]$                     | trivial |

2nd minimal solution:  $\mu_2^T = 3$  (48 symmetry vectors)

Space group 76 ( $\mathbb{Z}_1$ )

1st minimal solution:  $\mu_1^T = 4$  (1 symmetry vector)

| $\mathbf{n}^T$                                                                                                            |
|---------------------------------------------------------------------------------------------------------------------------|
| $[(\blacksquare)^{2T} + \Gamma_1 + \Gamma_2, A_1A_3 + A_2A_4, M_1 + M_2 + M_3M_4, Z_1Z_3 + Z_2Z_4, 2R_1R_2, 2X_1 + 2X_2]$ |

2nd minimal solution:  $\mu_2^T = 8$  (1 symmetry vector)

Space group 77 ( $\mathbb{Z}_2$ )

1st minimal solution:  $\mu_1^T = 2$  (6 symmetry vectors)

| $\mathbf{n}^T$                                                              | $\mathbf{v}^T \in \mathbb{Z}_2$ |
|-----------------------------------------------------------------------------|---------------------------------|
| $[(\blacksquare)^{2T}, A_3 + A_4, M_3M_4, Z_3 + Z_4, 2R_2, 2X_2]$           | trivial                         |
| $[(\blacksquare)^{2T}, A_3 + A_4, M_3M_4, Z_3 + Z_4, R_1 + R_2, X_1 + X_2]$ | 1                               |
| $[(\blacksquare)^{2T}, A_3 + A_4, M_3M_4, Z_3 + Z_4, 2R_1, 2X_1]$           | trivial                         |
| $[(\blacksquare)^{2T}, A_1A_2, M_1 + M_2, Z_3 + Z_4, 2R_2, 2X_2]$           | 1                               |
| $[(\blacksquare)^{2T}, A_1A_2, M_1 + M_2, Z_3 + Z_4, R_1 + R_2, X_1 + X_2]$ | trivial                         |
| $[(\blacksquare)^{2T}, A_1A_2, M_1 + M_2, Z_3 + Z_4, 2R_1, 2X_1]$           | 1                               |

2nd minimal solution:  $\mu_2^T = 4$  (30 symmetry vectors)

Space group 78 ( $\mathbb{Z}_1$ )

1st minimal solution:  $\mu_1^T = 4$  (1 symmetry vector)

| $\mathbf{n}^T$                                                                                                            |
|---------------------------------------------------------------------------------------------------------------------------|
| $[(\blacksquare)^{2T} + \Gamma_1 + \Gamma_2, A_1A_3 + A_2A_4, M_1 + M_2 + M_3M_4, Z_1Z_3 + Z_2Z_4, 2R_1R_2, 2X_1 + 2X_2]$ |

2nd minimal solution:  $\mu_2^T = 8$  (1 symmetry vector)

Space group 79 ( $\mathbb{Z}_1$ )

1st minimal solution:  $\mu_1^T = 2$  (2 symmetry vectors)

| $\mathbf{n}^T$                                      |
|-----------------------------------------------------|
| $[(\blacksquare)^{2T}, M_3M_4, 2P_1, 2X_1, 2N_1]$   |
| $[(\blacksquare)^{2T}, M_3M_4, P_2P_2, 2X_2, 2N_1]$ |

2nd minimal solution:  $\mu_2^T = 3$  (4 symmetry vectors)

Space group 80 ( $\mathbb{Z}_1$ )

1st minimal solution:  $\mu_1^T = 2$  (1 symmetry vector)

| $\mathbf{n}^T$                                              |
|-------------------------------------------------------------|
| $[(\blacksquare)^{2T}, M_3 + M_4, P_1P_2, X_1 + X_2, 2N_1]$ |

2nd minimal solution:  $\mu_2^T = 4$  (2 symmetry vectors)

Space group 81 ( $\mathbb{Z}_2 \times \mathbb{Z}_2$ )

1st minimal solution:  $\mu_1^T = 2$  (30 symmetry vectors)

| $\mathbf{n}^T$                                                              | $\mathbf{v}^T \in \mathbb{Z}_2 \times \mathbb{Z}_2$ |
|-----------------------------------------------------------------------------|-----------------------------------------------------|
| $[(\blacksquare)^{2T}, A_3A_4, M_3M_4, Z_3Z_4, 2R_1, 2X_1]$                 | (1, 1)                                              |
| $[(\blacksquare)^{2T}, A_3A_4, M_3M_4, Z_3Z_4, R_1 + R_2, X_1 + X_2]$       | (0, 1)                                              |
| $[(\blacksquare)^{2T}, A_3A_4, M_3M_4, Z_3Z_4, 2R_2, 2X_2]$                 | (1, 1)                                              |
| $[(\blacksquare)^{2T}, 2A_2, 2M_2, Z_3Z_4, 2R_1, 2X_1]$                     | (1, 1)                                              |
| $[(\blacksquare)^{2T}, 2A_2, 2M_2, Z_3Z_4, R_1 + R_2, X_1 + X_2]$           | (0, 1)                                              |
| $[(\blacksquare)^{2T}, 2A_2, 2M_2, Z_3Z_4, 2R_2, 2X_2]$                     | (1, 1)                                              |
| $[(\blacksquare)^{2T}, 2A_2, M_1 + M_2, Z_3Z_4, 2R_1, 2X_1]$                | trivial                                             |
| $[(\blacksquare)^{2T}, 2A_2, M_1 + M_2, Z_3Z_4, R_1 + R_2, X_1 + X_2]$      | (1, 0)                                              |
| $[(\blacksquare)^{2T}, 2A_2, M_1 + M_2, Z_3Z_4, 2R_2, 2X_2]$                | trivial                                             |
| $[(\blacksquare)^{2T}, 2A_2, 2M_1, Z_3Z_4, 2R_1, 2X_1]$                     | (1, 1)                                              |
| $[(\blacksquare)^{2T}, 2A_2, 2M_1, Z_3Z_4, R_1 + R_2, X_1 + X_2]$           | (0, 1)                                              |
| $[(\blacksquare)^{2T}, 2A_2, 2M_1, Z_3Z_4, 2R_2, 2X_2]$                     | (1, 1)                                              |
| $[(\blacksquare)^{2T}, A_1 + A_2, 2M_2, Z_3Z_4, 2R_1, 2X_1]$                | (1, 0)                                              |
| $[(\blacksquare)^{2T}, A_1 + A_2, 2M_2, Z_3Z_4, R_1 + R_2, X_1 + X_2]$      | trivial                                             |
| $[(\blacksquare)^{2T}, A_1 + A_2, 2M_2, Z_3Z_4, 2R_2, 2X_2]$                | (1, 0)                                              |
| $[(\blacksquare)^{2T}, A_1 + A_2, M_1 + M_2, Z_3Z_4, 2R_1, 2X_1]$           | (0, 1)                                              |
| $[(\blacksquare)^{2T}, A_1 + A_2, M_1 + M_2, Z_3Z_4, R_1 + R_2, X_1 + X_2]$ | (1, 1)                                              |
| $[(\blacksquare)^{2T}, A_1 + A_2, M_1 + M_2, Z_3Z_4, 2R_2, 2X_2]$           | (0, 1)                                              |
| $[(\blacksquare)^{2T}, A_1 + A_2, 2M_1, Z_3Z_4, 2R_1, 2X_1]$                | (1, 0)                                              |
| $[(\blacksquare)^{2T}, A_1 + A_2, 2M_1, Z_3Z_4, R_1 + R_2, X_1 + X_2]$      | trivial                                             |
| $[(\blacksquare)^{2T}, A_1 + A_2, 2M_1, Z_3Z_4, 2R_2, 2X_2]$                | (1, 0)                                              |
| $[(\blacksquare)^{2T}, 2A_1, 2M_2, Z_3Z_4, 2R_1, 2X_1]$                     | (1, 1)                                              |
| $[(\blacksquare)^{2T}, 2A_1, 2M_2, Z_3Z_4, R_1 + R_2, X_1 + X_2]$           | (0, 1)                                              |

... continued on next page

... continued from previous page

|                                                                        |         |
|------------------------------------------------------------------------|---------|
| $[(\blacksquare)^{2T}, 2A_1, 2M_2, Z_3Z_4, 2R_2, 2X_2]$                | (1, 1)  |
| $[(\blacksquare)^{2T}, 2A_1, M_1 + M_2, Z_3Z_4, 2R_1, 2X_1]$           | trivial |
| $[(\blacksquare)^{2T}, 2A_1, M_1 + M_2, Z_3Z_4, R_1 + R_2, X_1 + X_2]$ | (1, 0)  |
| $[(\blacksquare)^{2T}, 2A_1, M_1 + M_2, Z_3Z_4, 2R_2, 2X_2]$           | trivial |
| $[(\blacksquare)^{2T}, 2A_1, 2M_1, Z_3Z_4, 2R_1, 2X_1]$                | (1, 1)  |
| $[(\blacksquare)^{2T}, 2A_1, 2M_1, Z_3Z_4, R_1 + R_2, X_1 + X_2]$      | (0, 1)  |
| $[(\blacksquare)^{2T}, 2A_1, 2M_1, Z_3Z_4, 2R_2, 2X_2]$                | (1, 1)  |

2nd minimal solution:  $\mu_2^T = 3$  (320 symmetry vectors)

Space group 82 ( $\mathbb{Z}_2$ )

1st minimal solution:  $\mu_1^T = 2$  (10 symmetry vectors)

| $\mathbf{n}^T$                                                           | $\mathbf{v}^T \in \mathbb{Z}_2$ |
|--------------------------------------------------------------------------|---------------------------------|
| $[(\blacksquare)^{2T}, M_3M_4, 2P_2, 2PA_2, 2X_1, 2N_1]$                 | 1                               |
| $[(\blacksquare)^{2T}, M_3M_4, P_2 + P_3, PA_2 + PA_3, X_1 + X_2, 2N_1]$ | trivial                         |
| $[(\blacksquare)^{2T}, M_3M_4, P_2 + P_4, PA_2 + PA_4, X_1 + X_2, 2N_1]$ | trivial                         |
| $[(\blacksquare)^{2T}, M_3M_4, P_1 + P_2, PA_1 + PA_2, 2X_1, 2N_1]$      | 1                               |
| $[(\blacksquare)^{2T}, M_3M_4, 2P_3, 2PA_3, 2X_2, 2N_1]$                 | 1                               |
| $[(\blacksquare)^{2T}, M_3M_4, P_3 + P_4, PA_3 + PA_4, 2X_2, 2N_1]$      | 1                               |
| $[(\blacksquare)^{2T}, M_3M_4, P_1 + P_3, PA_1 + PA_3, X_1 + X_2, 2N_1]$ | trivial                         |
| $[(\blacksquare)^{2T}, M_3M_4, 2P_4, 2PA_4, 2X_2, 2N_1]$                 | 1                               |
| $[(\blacksquare)^{2T}, M_3M_4, P_1 + P_4, PA_1 + PA_4, X_1 + X_2, 2N_1]$ | trivial                         |
| $[(\blacksquare)^{2T}, M_3M_4, 2P_1, 2PA_1, 2X_1, 2N_1]$                 | 1                               |

2nd minimal solution:  $\mu_2^T = 3$  (80 symmetry vectors)

Space group 83 ( $\mathbb{Z}_2 \times \mathbb{Z}_2 \times \mathbb{Z}_2$ )

1st minimal solution:  $\mu_1^T = 2$  (32 symmetry vectors)

| $\mathbf{n}^T$                                                                                  | $\mathbf{v}^T \in \mathbb{Z}_2 \times \mathbb{Z}_2 \times \mathbb{Z}_2$ |
|-------------------------------------------------------------------------------------------------|-------------------------------------------------------------------------|
| $[(\blacksquare)^{2T}, 2A_2^-, M_2^+ + M_2^-, Z_3^+Z_4^+, 2R_2^+, X_2^+ + X_2^-]$               | trivial                                                                 |
| $[(\blacksquare)^{2T}, 2A_2^-, M_2^+ + M_2^-, Z_3^+Z_4^+, R_1^- + R_2^+, X_1^+ + X_2^+]$        | (1, 1, 1)                                                               |
| $[(\blacksquare)^{2T}, 2A_2^+, M_2^+ + M_2^-, Z_3^-Z_4^-, 2R_2^-, X_2^+ + X_2^-]$               | trivial                                                                 |
| $[(\blacksquare)^{2T}, 2A_2^+, M_2^+ + M_2^-, Z_3^-Z_4^-, R_1^+ + R_2^-, X_1^+ + X_2^+]$        | (1, 0, 0)                                                               |
| $[(\blacksquare)^{2T}, A_1^- + A_2^-, M_1^+ + M_2^-, Z_3^+Z_4^+, 2R_2^+, X_2^+ + X_2^-]$        | (1, 1, 1)                                                               |
| $[(\blacksquare)^{2T}, A_1^- + A_2^-, M_1^+ + M_2^-, Z_3^+Z_4^+, R_1^- + R_2^+, X_1^+ + X_2^+]$ | trivial                                                                 |
| $[(\blacksquare)^{2T}, A_1^+ + A_2^+, M_1^+ + M_2^-, Z_3^-Z_4^-, 2R_2^-, X_2^+ + X_2^-]$        | (1, 0, 0)                                                               |
| $[(\blacksquare)^{2T}, A_1^+ + A_2^+, M_1^+ + M_2^-, Z_3^-Z_4^-, R_1^+ + R_2^-, X_1^+ + X_2^+]$ | trivial                                                                 |
| $[(\blacksquare)^{2T}, 2A_2^-, M_2^+ + M_2^-, Z_3^+Z_4^+, R_1^- + R_2^+, X_1^- + X_2^-]$        | (0, 1, 0)                                                               |
| $[(\blacksquare)^{2T}, 2A_2^-, M_2^+ + M_2^-, Z_3^+Z_4^+, 2R_1^-, X_1^+ + X_1^-]$               | (1, 0, 1)                                                               |
| $[(\blacksquare)^{2T}, A_1^- + A_2^-, M_1^+ + M_2^-, Z_3^+Z_4^+, R_1^- + R_2^+, X_1^- + X_2^-]$ | (1, 0, 1)                                                               |
| $[(\blacksquare)^{2T}, A_1^- + A_2^-, M_1^+ + M_2^-, Z_3^+Z_4^+, 2R_1^-, X_1^+ + X_1^-]$        | (0, 1, 0)                                                               |
| $[(\blacksquare)^{2T}, A_1^- + A_2^-, M_1^- + M_2^+, Z_3^+Z_4^+, 2R_2^+, X_2^+ + X_2^-]$        | (0, 1, 0)                                                               |
| $[(\blacksquare)^{2T}, A_1^- + A_2^-, M_1^- + M_2^+, Z_3^+Z_4^+, R_1^- + R_2^+, X_1^- + X_2^-]$ | trivial                                                                 |

... continued on next page

... continued from previous page

|                                                                                                  |           |
|--------------------------------------------------------------------------------------------------|-----------|
| $[(\blacksquare)^{2T}, A_1^- + A_2^-, M_1^- + M_2^+, Z_3^+ Z_4^+, R_1^- + R_2^+, X_1^+ + X_2^+]$ | (1, 0, 1) |
| $[(\blacksquare)^{2T}, A_1^- + A_2^-, M_1^- + M_2^+, Z_3^+ Z_4^+, 2R_1^-, X_1^+ + X_1^-]$        | (1, 1, 1) |
| $[(\blacksquare)^{2T}, 2A_2^+, M_2^+ + M_2^-, Z_3^- Z_4^-, R_1^+ + R_2^-, X_1^- + X_2^-]$        | (0, 0, 1) |
| $[(\blacksquare)^{2T}, 2A_2^+, M_2^+ + M_2^-, Z_3^- Z_4^-, 2R_1^+, X_1^+ + X_1^-]$               | (1, 0, 1) |
| $[(\blacksquare)^{2T}, 2A_1^-, M_1^+ + M_1^-, Z_3^+ Z_4^+, 2R_2^+, X_2^+ + X_2^-]$               | (1, 0, 1) |
| $[(\blacksquare)^{2T}, 2A_1^-, M_1^+ + M_1^-, Z_3^+ Z_4^+, R_1^- + R_2^+, X_1^+ + X_2^+]$        | (0, 1, 0) |
| $[(\blacksquare)^{2T}, 2A_1^-, M_1^+ + M_1^-, Z_3^+ Z_4^+, R_1^- + R_2^+, X_1^- + X_2^-]$        | (1, 1, 1) |
| $[(\blacksquare)^{2T}, 2A_1^-, M_1^+ + M_1^-, Z_3^+ Z_4^+, 2R_1^-, X_1^+ + X_1^-]$               | trivial   |
| $[(\blacksquare)^{2T}, A_1^+ + A_2^+, M_1^+ + M_2^-, Z_3^- Z_4^-, R_1^+ + R_2^-, X_1^- + X_2^-]$ | (1, 0, 1) |
| $[(\blacksquare)^{2T}, A_1^+ + A_2^+, M_1^+ + M_2^-, Z_3^- Z_4^-, 2R_1^+, X_1^+ + X_1^-]$        | (0, 0, 1) |
| $[(\blacksquare)^{2T}, A_1^+ + A_2^+, M_1^- + M_2^+, Z_3^- Z_4^-, 2R_2^-, X_2^+ + X_2^-]$        | (0, 0, 1) |
| $[(\blacksquare)^{2T}, A_1^+ + A_2^+, M_1^- + M_2^+, Z_3^- Z_4^-, R_1^+ + R_2^-, X_1^- + X_2^-]$ | trivial   |
| $[(\blacksquare)^{2T}, A_1^+ + A_2^+, M_1^- + M_2^+, Z_3^- Z_4^-, R_1^+ + R_2^-, X_1^+ + X_2^+]$ | (1, 0, 1) |
| $[(\blacksquare)^{2T}, A_1^+ + A_2^+, M_1^- + M_2^+, Z_3^- Z_4^-, 2R_1^+, X_1^+ + X_1^-]$        | (1, 0, 0) |
| $[(\blacksquare)^{2T}, 2A_1^+, M_1^+ + M_1^-, Z_3^- Z_4^-, 2R_2^-, X_2^+ + X_2^-]$               | (1, 0, 1) |
| $[(\blacksquare)^{2T}, 2A_1^+, M_1^+ + M_1^-, Z_3^- Z_4^-, R_1^+ + R_2^-, X_1^- + X_2^-]$        | (1, 0, 0) |
| $[(\blacksquare)^{2T}, 2A_1^+, M_1^+ + M_1^-, Z_3^- Z_4^-, R_1^+ + R_2^-, X_1^+ + X_2^+]$        | (0, 0, 1) |
| $[(\blacksquare)^{2T}, 2A_1^+, M_1^+ + M_1^-, Z_3^- Z_4^-, 2R_1^+, X_1^+ + X_1^-]$               | trivial   |

2nd minimal solution:  $\mu_2^T = 3$  (1344 symmetry vectors)

Space group 84 ( $\mathbb{Z}_2 \times \mathbb{Z}_2$ )

1st minimal solution:  $\mu_1^T = 2$  (12 symmetry vectors)

| $\mathbf{n}^T$                                                                 | $\mathbf{v}^T \in \mathbb{Z}_2 \times \mathbb{Z}_2$ |
|--------------------------------------------------------------------------------|-----------------------------------------------------|
| $[(\blacksquare)^{2T}, A_1, M_1^+ + M_2^-, Z_2, R_1^- + R_2^-, X_1^- + X_2^-]$ | (1, 0)                                              |
| $[(\blacksquare)^{2T}, A_1, M_1^- + M_2^+, Z_2, R_1^- + R_2^-, X_1^- + X_2^-]$ | trivial                                             |
| $[(\blacksquare)^{2T}, A_1, M_1^+ + M_2^-, Z_2, R_1^- + R_2^-, X_1^+ + X_2^+]$ | trivial                                             |
| $[(\blacksquare)^{2T}, A_1, M_1^+ + M_2^-, Z_2, R_2^+ + R_2^-, X_2^+ + X_2^-]$ | (0, 1)                                              |
| $[(\blacksquare)^{2T}, A_1, M_1^- + M_2^+, Z_2, R_1^- + R_2^-, X_1^+ + X_2^+]$ | (1, 0)                                              |
| $[(\blacksquare)^{2T}, A_1, M_1^- + M_2^+, Z_2, R_2^+ + R_2^-, X_2^+ + X_2^-]$ | (1, 1)                                              |
| $[(\blacksquare)^{2T}, A_1, M_1^+ + M_2^-, Z_2, R_1^+ + R_1^-, X_1^+ + X_1^-]$ | (1, 1)                                              |
| $[(\blacksquare)^{2T}, A_1, M_1^+ + M_2^-, Z_2, R_1^+ + R_2^+, X_1^- + X_2^-]$ | (1, 0)                                              |
| $[(\blacksquare)^{2T}, A_1, M_1^- + M_2^+, Z_2, R_1^+ + R_1^-, X_1^+ + X_1^-]$ | (0, 1)                                              |
| $[(\blacksquare)^{2T}, A_1, M_1^- + M_2^+, Z_2, R_1^+ + R_2^+, X_1^- + X_2^-]$ | trivial                                             |
| $[(\blacksquare)^{2T}, A_1, M_1^+ + M_2^-, Z_2, R_1^+ + R_2^+, X_1^+ + X_2^+]$ | trivial                                             |
| $[(\blacksquare)^{2T}, A_1, M_1^- + M_2^+, Z_2, R_1^+ + R_2^+, X_1^+ + X_2^+]$ | (1, 0)                                              |

2nd minimal solution:  $\mu_2^T = 4$  (484 symmetry vectors)

Space group 85 ( $\mathbb{Z}_2$ )

1st minimal solution:  $\mu_1^T = 4$  (24 symmetry vectors)

| $\mathbf{n}^T$                                                                                         | $\mathbf{v}^T \in \mathbb{Z}_2$ |
|--------------------------------------------------------------------------------------------------------|---------------------------------|
| $[(\blacksquare)^{2T} + \Gamma_1^+ + \Gamma_2^-, 2A_2, 2M_2, Z_1^+ + Z_2^+ + Z_3^+ Z_4^+, 2R_1, 2X_1]$ | 1                               |

... continued on next page

... continued from previous page

|                                                                                                                  |         |
|------------------------------------------------------------------------------------------------------------------|---------|
| $[(\blacksquare)^{2T} + \Gamma_1^+ + \Gamma_2^-, 2A_2, 2M_2, Z_1^- + Z_2^- + Z_3^- Z_4^-, 2R_1, 2X_1]$           | 1       |
| $[(\blacksquare)^{2T} + \Gamma_1^+ + \Gamma_1^-, 2A_2, 2M_2, 2Z_1^+ + Z_3^+ Z_4^+, 2R_1, 2X_1]$                  | trivial |
| $[(\blacksquare)^{2T} + \Gamma_1^+ + \Gamma_1^-, 2A_2, 2M_2, 2Z_1^- + Z_3^- Z_4^-, 2R_1, 2X_1]$                  | trivial |
| $[(\blacksquare)^{2T} + \Gamma_1^+ + \Gamma_2^-, A_1 + A_2, M_1 + M_2, Z_1^+ + Z_2^+ + Z_3^+ Z_4^+, 2R_1, 2X_1]$ | trivial |
| $[(\blacksquare)^{2T} + \Gamma_1^+ + \Gamma_2^-, A_1 + A_2, M_1 + M_2, Z_1^- + Z_2^- + Z_3^- Z_4^-, 2R_1, 2X_1]$ | trivial |
| $[(\blacksquare)^{2T} + \Gamma_1^+ + \Gamma_1^-, A_1 + A_2, M_1 + M_2, 2Z_1^+ + Z_3^+ Z_4^+, 2R_1, 2X_1]$        | 1       |
| $[(\blacksquare)^{2T} + \Gamma_1^+ + \Gamma_1^-, A_1 + A_2, M_1 + M_2, 2Z_1^- + Z_3^- Z_4^-, 2R_1, 2X_1]$        | 1       |
| $[(\blacksquare)^{2T} + \Gamma_1^+ + \Gamma_2^-, 2A_1, 2M_1, Z_1^+ + Z_2^+ + Z_3^+ Z_4^+, 2R_1, 2X_1]$           | 1       |
| $[(\blacksquare)^{2T} + \Gamma_1^+ + \Gamma_2^-, 2A_1, 2M_1, Z_1^- + Z_2^- + Z_3^- Z_4^-, 2R_1, 2X_1]$           | 1       |
| $[(\blacksquare)^{2T} + \Gamma_1^+ + \Gamma_1^-, 2A_1, 2M_1, 2Z_1^+ + Z_3^+ Z_4^+, 2R_1, 2X_1]$                  | trivial |
| $[(\blacksquare)^{2T} + \Gamma_1^+ + \Gamma_1^-, 2A_1, 2M_1, 2Z_1^- + Z_3^- Z_4^-, 2R_1, 2X_1]$                  | trivial |
| $[(\blacksquare)^{2T} + \Gamma_2^+ + \Gamma_2^-, 2A_2, 2M_2, 2Z_2^+ + Z_3^+ Z_4^+, 2R_1, 2X_1]$                  | trivial |
| $[(\blacksquare)^{2T} + \Gamma_1^- + \Gamma_2^+, 2A_2, 2M_2, Z_1^+ + Z_2^+ + Z_3^+ Z_4^+, 2R_1, 2X_1]$           | 1       |
| $[(\blacksquare)^{2T} + \Gamma_2^+ + \Gamma_2^-, A_1 + A_2, M_1 + M_2, 2Z_2^+ + Z_3^+ Z_4^+, 2R_1, 2X_1]$        | 1       |
| $[(\blacksquare)^{2T} + \Gamma_1^- + \Gamma_2^+, A_1 + A_2, M_1 + M_2, Z_1^+ + Z_2^+ + Z_3^+ Z_4^+, 2R_1, 2X_1]$ | trivial |
| $[(\blacksquare)^{2T} + \Gamma_2^+ + \Gamma_2^-, 2A_1, 2M_1, 2Z_2^+ + Z_3^+ Z_4^+, 2R_1, 2X_1]$                  | trivial |
| $[(\blacksquare)^{2T} + \Gamma_1^- + \Gamma_2^+, 2A_1, 2M_1, Z_1^+ + Z_2^+ + Z_3^+ Z_4^+, 2R_1, 2X_1]$           | 1       |
| $[(\blacksquare)^{2T} + \Gamma_2^+ + \Gamma_2^-, 2A_2, 2M_2, 2Z_2^- + Z_3^- Z_4^-, 2R_1, 2X_1]$                  | trivial |
| $[(\blacksquare)^{2T} + \Gamma_2^+ + \Gamma_2^-, A_1 + A_2, M_1 + M_2, 2Z_2^- + Z_3^- Z_4^-, 2R_1, 2X_1]$        | 1       |
| $[(\blacksquare)^{2T} + \Gamma_1^- + \Gamma_2^+, 2A_2, 2M_2, Z_1^- + Z_2^- + Z_3^- Z_4^-, 2R_1, 2X_1]$           | 1       |
| $[(\blacksquare)^{2T} + \Gamma_1^- + \Gamma_2^+, A_1 + A_2, M_1 + M_2, Z_1^- + Z_2^- + Z_3^- Z_4^-, 2R_1, 2X_1]$ | trivial |
| $[(\blacksquare)^{2T} + \Gamma_2^+ + \Gamma_2^-, 2A_1, 2M_1, 2Z_2^- + Z_3^- Z_4^-, 2R_1, 2X_1]$                  | trivial |
| $[(\blacksquare)^{2T} + \Gamma_1^- + \Gamma_2^+, 2A_1, 2M_1, Z_1^- + Z_2^- + Z_3^- Z_4^-, 2R_1, 2X_1]$           | 1       |

2nd minimal solution:  $\mu_2^T = 6$  (160 symmetry vectors)

Space group 86 ( $\mathbb{Z}_2$ )

1st minimal solution:  $\mu_1^T = 2$  (2 symmetry vectors & filling-enforced topology)

| $\mathbf{n}^T$                                             | $\mathbf{v}^T \in \mathbb{Z}_2$ |
|------------------------------------------------------------|---------------------------------|
| $[(\blacksquare)^{2T}, A_1^- + A_2^+, M_1, Z_2, R_1, X_1]$ | 1                               |
| $[(\blacksquare)^{2T}, A_1^+ + A_2^-, M_1, Z_2, R_1, X_1]$ | 1                               |

2nd minimal solution:  $\mu_2^T = 4$  (12 symmetry vectors)

Space group 87 ( $\mathbb{Z}_2 \times \mathbb{Z}_2$ )

1st minimal solution:  $\mu_1^T = 3$  (128 symmetry vectors)

| $\mathbf{n}^T$                                                                                        | $\mathbf{v}^T \in \mathbb{Z}_2 \times \mathbb{Z}_2$ |
|-------------------------------------------------------------------------------------------------------|-----------------------------------------------------|
| $[(\blacksquare)^{2T} + \Gamma_1^+, M_1^- + M_3^- M_4^-, 3P_2, 2X_1^+ + X_1^-, 3N_1^+]$               | (1, 0)                                              |
| $[(\blacksquare)^{2T} + \Gamma_1^+, M_1^- + M_3^- M_4^-, 3P_2, 2X_1^+ + X_1^-, 2N_1^+ + N_1^-]$       | trivial                                             |
| $[(\blacksquare)^{2T} + \Gamma_1^+, M_1^- + M_3^- M_4^-, P_1 + 2P_2, 2X_1^+ + X_1^-, 3N_1^+]$         | trivial                                             |
| $[(\blacksquare)^{2T} + \Gamma_1^+, M_1^- + M_3^- M_4^-, P_1 + 2P_2, 2X_1^+ + X_1^-, 2N_1^+ + N_1^-]$ | (1, 0)                                              |
| $[(\blacksquare)^{2T} + \Gamma_1^+, M_1^- + M_3^- M_4^-, 3P_2, 2X_1^+ + X_1^-, N_1^+ + 2N_1^-]$       | (1, 0)                                              |
| $[(\blacksquare)^{2T} + \Gamma_1^+, M_1^- + M_3^- M_4^-, P_1 + 2P_2, 2X_1^+ + X_1^-, N_1^+ + 2N_1^-]$ | trivial                                             |

... continued on next page



... continued on next page



... continued from previous page

|                                                                                                                 |         |
|-----------------------------------------------------------------------------------------------------------------|---------|
| $[(\blacksquare)^{2T} + \Gamma_1^-, M_1^+ + M_3^+ M_4^+, P_1 + P_3 P_4, X_1^- + X_2^+ + X_2^-, N_1^+ + 2N_1^-]$ | (0, 1)  |
| $[(\blacksquare)^{2T} + \Gamma_1^-, M_1^+ + M_3^+ M_4^+, P_1 + P_3 P_4, X_1^- + X_2^+ + X_2^-, 3N_1^-]$         | (1, 1)  |
| $[(\blacksquare)^{2T} + \Gamma_1^-, M_1^+ + M_3^+ M_4^+, P_1 + P_3 P_4, X_1^+ + 2X_2^+, 3N_1^+]$                | trivial |
| $[(\blacksquare)^{2T} + \Gamma_1^-, M_1^+ + M_3^+ M_4^+, P_1 + P_3 P_4, X_1^+ + 2X_2^+, 2N_1^+ + N_1^-]$        | (1, 0)  |
| $[(\blacksquare)^{2T} + \Gamma_1^-, M_1^+ + M_3^+ M_4^+, P_1 + P_3 P_4, X_1^+ + 2X_2^+, N_1^+ + 2N_1^-]$        | trivial |
| $[(\blacksquare)^{2T} + \Gamma_1^-, M_1^+ + M_3^+ M_4^+, P_1 + P_3 P_4, X_1^+ + 2X_2^+, 3N_1^-]$                | (1, 0)  |
| $[(\blacksquare)^{2T} + \Gamma_1^-, M_1^+ + M_3^+ M_4^+, 2P_1 + P_2, X_1^+ + 2X_1^-, 3N_1^+]$                   | (1, 0)  |
| $[(\blacksquare)^{2T} + \Gamma_1^-, M_1^+ + M_3^+ M_4^+, 2P_1 + P_2, X_1^+ + 2X_1^-, 2N_1^+ + N_1^-]$           | trivial |
| $[(\blacksquare)^{2T} + \Gamma_1^-, M_1^+ + M_3^+ M_4^+, 2P_1 + P_2, X_1^+ + 2X_1^-, N_1^+ + 2N_1^-]$           | (1, 0)  |
| $[(\blacksquare)^{2T} + \Gamma_1^-, M_1^+ + M_3^+ M_4^+, 2P_1 + P_2, X_1^+ + 2X_1^-, 3N_1^-]$                   | trivial |
| $[(\blacksquare)^{2T} + \Gamma_1^-, M_1^+ + M_3^+ M_4^+, 3P_1, X_1^+ + 2X_1^-, 3N_1^+]$                         | trivial |
| $[(\blacksquare)^{2T} + \Gamma_1^-, M_1^+ + M_3^+ M_4^+, 3P_1, X_1^+ + 2X_1^-, 2N_1^+ + N_1^-]$                 | (1, 0)  |
| $[(\blacksquare)^{2T} + \Gamma_1^-, M_1^+ + M_3^+ M_4^+, 3P_1, X_1^+ + 2X_1^-, N_1^+ + 2N_1^-]$                 | trivial |
| $[(\blacksquare)^{2T} + \Gamma_1^-, M_1^+ + M_3^+ M_4^+, 3P_1, X_1^+ + 2X_1^-, 3N_1^-]$                         | (1, 0)  |

2nd minimal solution:  $\mu_2^T = 4$  (1080 symmetry vectors)

Space group 88 ( $\mathbb{Z}_2$ )

1st minimal solution:  $\mu_1^T = 2$  (6 symmetry vectors)

| $\mathbf{n}^T$                                            | $\mathbf{v}^T \in \mathbb{Z}_2$ |
|-----------------------------------------------------------|---------------------------------|
| $[(\blacksquare)^{2T}, M_2, P_1 P_4, X_1, 2N_1^-]$        | trivial                         |
| $[(\blacksquare)^{2T}, M_2, P_1 P_4, X_1, N_1^+ + N_1^-]$ | 1                               |
| $[(\blacksquare)^{2T}, M_2, P_1 P_4, X_1, 2N_1^+]$        | trivial                         |
| $[(\blacksquare)^{2T}, M_2, P_2 P_3, X_1, 2N_1^-]$        | trivial                         |
| $[(\blacksquare)^{2T}, M_2, P_2 P_3, X_1, N_1^+ + N_1^-]$ | 1                               |
| $[(\blacksquare)^{2T}, M_2, P_2 P_3, X_1, 2N_1^+]$        | trivial                         |

2nd minimal solution:  $\mu_2^T = 4$  (30 symmetry vectors)

Space group 89 ( $\mathbb{Z}_1$ )

1st minimal solution:  $\mu_1^T = 2$  (4 symmetry vectors)

| $\mathbf{n}^T$                                                           |
|--------------------------------------------------------------------------|
| $[(\blacksquare)^{2T}, A_2 + A_4, 2M_2, Z_5, R_3 + R_4, 2X_3]$           |
| $[(\blacksquare)^{2T}, A_3 + A_4, M_2 + M_3, Z_5, R_2 + R_4, X_2 + X_3]$ |
| $[(\blacksquare)^{2T}, A_1 + A_2, M_2 + M_3, Z_5, R_1 + R_3, X_2 + X_3]$ |
| $[(\blacksquare)^{2T}, A_1 + A_3, 2M_3, Z_5, R_1 + R_2, 2X_2]$           |

2nd minimal solution:  $\mu_2^T = 3$  (84 symmetry vectors)

Space group 90 ( $\mathbb{Z}_1$ )

1st minimal solution:  $\mu_1^T = 4$  (5 symmetry vectors)

| $\mathbf{n}^T$                                                                                         |
|--------------------------------------------------------------------------------------------------------|
| $[(\blacksquare)^{2T} + 2\Gamma_1, 2A_5, 2M_5, Z_1 + Z_3 + Z_5, 2R_1, 2X_1]$                           |
| $[(\blacksquare)^{2T} + \Gamma_1 + \Gamma_2, A_2A_3 + A_5, M_2M_3 + M_5, Z_2 + Z_3 + Z_5, 2R_1, 2X_1]$ |
| $[(\blacksquare)^{2T} + \Gamma_1 + \Gamma_2, A_1A_4 + A_5, M_2M_3 + M_5, Z_1 + Z_4 + Z_5, 2R_1, 2X_1]$ |
| $[(\blacksquare)^{2T} + 2\Gamma_2, A_1A_4 + A_2A_3, 2M_2M_3, Z_2 + Z_4 + Z_5, 2R_1, 2X_1]$             |
| $[(\blacksquare)^{2T} + 2\Gamma_1, A_1A_4 + A_2A_3, M_1M_4 + M_2M_3, Z_1 + Z_3 + Z_5, 2R_1, 2X_1]$     |

2nd minimal solution:  $\mu_2^T = 6$  (31 symmetry vectors)

Space group 91 ( $\mathbb{Z}_1$ )

1st minimal solution:  $\mu_1^T = 4$  (4 symmetry vectors)

| $\mathbf{n}^T$                                                                                                    |
|-------------------------------------------------------------------------------------------------------------------|
| $[(\blacksquare)^{2T} + \Gamma_1 + \Gamma_4, A_1 + A_2, M_3 + M_4 + M_5, Z_1 + Z_2, 2R_1, 2X_2 + X_3 + X_4]$      |
| $[(\blacksquare)^{2T} + \Gamma_1 + \Gamma_2, A_1 + A_2, M_2 + M_3 + M_5, Z_1 + Z_2, 2R_1, X_1 + X_2 + X_3 + X_4]$ |
| $[(\blacksquare)^{2T} + \Gamma_1 + \Gamma_4, A_1 + A_2, M_1 + M_2 + M_5, Z_1 + Z_2, 2R_1, X_1 + X_2 + 2X_3]$      |
| $[(\blacksquare)^{2T} + \Gamma_3 + \Gamma_4, A_1 + A_2, M_2 + M_3 + M_5, Z_1 + Z_2, 2R_1, 2X_2 + 2X_3]$           |

2nd minimal solution:  $\mu_2^T = 8$  (16 symmetry vectors)

Space group 92 ( $\mathbb{Z}_1$ )

1st minimal solution:  $\mu_1^T = 4$  (1 symmetry vector)

| $\mathbf{n}^T$                                                                                        |
|-------------------------------------------------------------------------------------------------------|
| $[(\blacksquare)^{2T} + \Gamma_1 + \Gamma_2, A_1A_2, M_2M_3 + M_5, Z_1 + Z_2, R_1R_3 + R_2R_4, 2X_1]$ |

2nd minimal solution:  $\mu_2^T = 8$  (2 symmetry vectors)

Space group 93 ( $\mathbb{Z}_1$ )

1st minimal solution:  $\mu_1^T = 2$  (2 symmetry vectors)

| $\mathbf{n}^T$                                                           |
|--------------------------------------------------------------------------|
| $[(\blacksquare)^{2T}, A_5, M_2 + M_3, Z_1 + Z_2, R_2 + R_3, X_2 + X_3]$ |
| $[(\blacksquare)^{2T}, A_5, M_2 + M_3, Z_3 + Z_4, R_1 + R_4, X_2 + X_3]$ |

2nd minimal solution:  $\mu_2^T = 4$  (104 symmetry vectors)

Space group 94 ( $\mathbb{Z}_1$ )

1st minimal solution:  $\mu_1^T = 4$  (2 symmetry vectors)

| $\mathbf{n}^T$                                                                                         |
|--------------------------------------------------------------------------------------------------------|
| $[(\blacksquare)^{2T} + \Gamma_1 + \Gamma_2, A_2A_3 + A_5, M_2M_3 + M_5, Z_2 + Z_3 + Z_5, 2R_1, 2X_1]$ |
| $[(\blacksquare)^{2T} + \Gamma_1 + \Gamma_2, A_1A_4 + A_5, M_2M_3 + M_5, Z_1 + Z_4 + Z_5, 2R_1, 2X_1]$ |

2nd minimal solution:  $\mu_2^T = 6$  (10 symmetry vectors)

Space group 95 ( $\mathbb{Z}_1$ )

1st minimal solution:  $\mu_1^T = 4$  (4 symmetry vectors)

| $\mathbf{n}^T$                                                                                                    |
|-------------------------------------------------------------------------------------------------------------------|
| $[(\blacksquare)^{2T} + \Gamma_1 + \Gamma_4, A_1 + A_2, M_3 + M_4 + M_5, Z_1 + Z_2, 2R_1, 2X_2 + X_3 + X_4]$      |
| $[(\blacksquare)^{2T} + \Gamma_1 + \Gamma_2, A_1 + A_2, M_2 + M_3 + M_5, Z_1 + Z_2, 2R_1, X_1 + X_2 + X_3 + X_4]$ |
| $[(\blacksquare)^{2T} + \Gamma_1 + \Gamma_4, A_1 + A_2, M_1 + M_2 + M_5, Z_1 + Z_2, 2R_1, X_1 + X_2 + 2X_3]$      |
| $[(\blacksquare)^{2T} + \Gamma_3 + \Gamma_4, A_1 + A_2, M_2 + M_3 + M_5, Z_1 + Z_2, 2R_1, 2X_2 + 2X_3]$           |

2nd minimal solution:  $\mu_2^T = 8$  (16 symmetry vectors)

Space group 96 ( $\mathbb{Z}_1$ )

1st minimal solution:  $\mu_1^T = 4$  (1 symmetry vector)

| $\mathbf{n}^T$                                                                                        |
|-------------------------------------------------------------------------------------------------------|
| $[(\blacksquare)^{2T} + \Gamma_1 + \Gamma_2, A_1A_2, M_2M_3 + M_5, Z_1 + Z_2, R_1R_3 + R_2R_4, 2X_1]$ |

2nd minimal solution:  $\mu_2^T = 8$  (2 symmetry vectors)

Space group 97 ( $\mathbb{Z}_1$ )

1st minimal solution:  $\mu_1^T = 3$  (8 symmetry vectors)

| $\mathbf{n}^T$                                                                           |
|------------------------------------------------------------------------------------------|
| $[(\blacksquare)^{2T} + \Gamma_1, M_3 + M_5, 3P_2, X_1 + 2X_2, 3N_2]$                    |
| $[(\blacksquare)^{2T} + \Gamma_1, M_3 + M_5, P_1 + 2P_2, X_1 + 2X_2, N_1 + 2N_2]$        |
| $[(\blacksquare)^{2T} + \Gamma_1, M_3 + M_5, 2P_1 + P_2, X_1 + 2X_2, 2N_1 + N_2]$        |
| $[(\blacksquare)^{2T} + \Gamma_2, M_4 + M_5, P_2 + P_3P_4, X_2 + 2X_4, N_1 + 2N_2]$      |
| $[(\blacksquare)^{2T} + \Gamma_1, M_3 + M_5, P_2 + P_3P_4, X_2 + X_3 + X_4, N_1 + 2N_2]$ |
| $[(\blacksquare)^{2T} + \Gamma_1, M_3 + M_5, P_1 + P_3P_4, X_2 + X_3 + X_4, 2N_1 + N_2]$ |
| $[(\blacksquare)^{2T} + \Gamma_1, M_3 + M_5, 3P_1, X_1 + 2X_2, 3N_1]$                    |
| $[(\blacksquare)^{2T} + \Gamma_2, M_4 + M_5, P_1 + P_3P_4, X_2 + 2X_4, 2N_1 + N_2]$      |

2nd minimal solution:  $\mu_2^T = 4$  (48 symmetry vectors)

Space group 98 ( $\mathbb{Z}_1$ )

1st minimal solution:  $\mu_1^T = 2$  (1 symmetry vector)

|                                                               |
|---------------------------------------------------------------|
| $\mathbf{n}^T$                                                |
| $[(\blacksquare)^{2T}, M_3 + M_4, P_1, X_2 + X_4, N_1 + N_2]$ |

2nd minimal solution:  $\mu_2^T = 4$  (6 symmetry vectors)

Space group 99 ( $\mathbb{Z}_1$ )

1st minimal solution:  $\mu_1^T = 2$  (8 symmetry vectors)

|                                                                          |
|--------------------------------------------------------------------------|
| $\mathbf{n}^T$                                                           |
| $[(\blacksquare)^{2T}, A_5, M_5, Z_5, R_3 + R_4, X_3 + X_4]$             |
| $[(\blacksquare)^{2T}, A_5, M_5, Z_5, R_1 + R_2, X_1 + X_2]$             |
| $[(\blacksquare)^{2T}, A_2 + A_3, M_2 + M_3, Z_5, R_3 + R_4, X_3 + X_4]$ |
| $[(\blacksquare)^{2T}, A_2 + A_3, M_2 + M_3, Z_5, R_1 + R_2, X_1 + X_2]$ |
| $[(\blacksquare)^{2T}, A_3 + A_4, M_3 + M_4, Z_5, R_2 + R_3, X_2 + X_3]$ |
| $[(\blacksquare)^{2T}, A_1 + A_2, M_1 + M_2, Z_5, R_1 + R_4, X_1 + X_4]$ |
| $[(\blacksquare)^{2T}, A_1 + A_4, M_1 + M_4, Z_5, R_3 + R_4, X_3 + X_4]$ |
| $[(\blacksquare)^{2T}, A_1 + A_4, M_1 + M_4, Z_5, R_1 + R_2, X_1 + X_2]$ |

2nd minimal solution:  $\mu_2^T = 3$  (56 symmetry vectors)

Space group 100 ( $\mathbb{Z}_1$ )

1st minimal solution:  $\mu_1^T = 2$  (1 symmetry vector)

|                                                  |
|--------------------------------------------------|
| $\mathbf{n}^T$                                   |
| $[(\blacksquare)^{2T}, A_5, M_5, Z_5, R_1, X_1]$ |

2nd minimal solution:  $\mu_2^T = 4$  (8 symmetry vectors)

Space group 101 ( $\mathbb{Z}_1$ )

1st minimal solution:  $\mu_1^T = 2$  (2 symmetry vectors)

|                                                            |
|------------------------------------------------------------|
| $\mathbf{n}^T$                                             |
| $[(\blacksquare)^{2T}, A_5, M_5, Z_5, R_3 R_4, X_3 + X_4]$ |
| $[(\blacksquare)^{2T}, A_5, M_5, Z_5, R_1 R_2, X_1 + X_2]$ |

2nd minimal solution:  $\mu_2^T = 4$  (12 symmetry vectors)

Space group 102 ( $\mathbb{Z}_1$ )

1st minimal solution:  $\mu_1^T = 2$  (1 symmetry vector)

| $\mathbf{n}^T$                                   |
|--------------------------------------------------|
| $[(\blacksquare)^{2T}, A_5, M_5, Z_5, R_1, X_1]$ |

2nd minimal solution:  $\mu_2^T = 4$  (4 symmetry vectors)

Space group 103 ( $\mathbb{Z}_2$ )

1st minimal solution:  $\mu_1^T = 4$  (12 symmetry vectors)

| $\mathbf{n}^T$                                                                                                                  | $\mathbf{v}^T \in \mathbb{Z}_2$ |
|---------------------------------------------------------------------------------------------------------------------------------|---------------------------------|
| $[(\blacksquare)^{2T} + \Gamma_5, A_5 A_5, 2M_5, Z_5 Z_5, 2R_1 R_2, 2X_1 + 2X_2]$                                               | trivial                         |
| $[(\blacksquare)^{2T} + \Gamma_5, A_5 A_5, 2M_5, Z_5 Z_5, R_1 R_2 + R_3 R_4, X_1 + X_2 + X_3 + X_4]$                            | 1                               |
| $[(\blacksquare)^{2T} + \Gamma_5, A_5 A_5, 2M_5, Z_5 Z_5, 2R_3 R_4, 2X_3 + 2X_4]$                                               | trivial                         |
| $[(\blacksquare)^{2T} + \Gamma_5, 2A_2 A_3, 2M_2 + 2M_3, Z_5 Z_5, 2R_1 R_2, 2X_1 + 2X_2]$                                       | trivial                         |
| $[(\blacksquare)^{2T} + \Gamma_5, 2A_2 A_3, 2M_2 + 2M_3, Z_5 Z_5, R_1 R_2 + R_3 R_4, X_1 + X_2 + X_3 + X_4]$                    | 1                               |
| $[(\blacksquare)^{2T} + \Gamma_5, 2A_2 A_3, 2M_2 + 2M_3, Z_5 Z_5, 2R_3 R_4, 2X_3 + 2X_4]$                                       | trivial                         |
| $[(\blacksquare)^{2T} + \Gamma_5, A_1 A_4 + A_2 A_3, M_1 + M_2 + M_3 + M_4, Z_5 Z_5, 2R_1 R_2, 2X_1 + 2X_2]$                    | 1                               |
| $[(\blacksquare)^{2T} + \Gamma_5, A_1 A_4 + A_2 A_3, M_1 + M_2 + M_3 + M_4, Z_5 Z_5, R_1 R_2 + R_3 R_4, X_1 + X_2 + X_3 + X_4]$ | trivial                         |
| $[(\blacksquare)^{2T} + \Gamma_5, A_1 A_4 + A_2 A_3, M_1 + M_2 + M_3 + M_4, Z_5 Z_5, 2R_3 R_4, 2X_3 + 2X_4]$                    | 1                               |
| $[(\blacksquare)^{2T} + \Gamma_5, 2A_1 A_4, 2M_1 + 2M_4, Z_5 Z_5, 2R_1 R_2, 2X_1 + 2X_2]$                                       | trivial                         |
| $[(\blacksquare)^{2T} + \Gamma_5, 2A_1 A_4, 2M_1 + 2M_4, Z_5 Z_5, R_1 R_2 + R_3 R_4, X_1 + X_2 + X_3 + X_4]$                    | 1                               |
| $[(\blacksquare)^{2T} + \Gamma_5, 2A_1 A_4, 2M_1 + 2M_4, Z_5 Z_5, 2R_3 R_4, 2X_3 + 2X_4]$                                       | trivial                         |

2nd minimal solution:  $\mu_2^T = 6$  (48 symmetry vectors)

Space group 104 ( $\mathbb{Z}_1$ )

1st minimal solution:  $\mu_1^T = 4$  (2 symmetry vectors)

| $\mathbf{n}^T$                                                                                |
|-----------------------------------------------------------------------------------------------|
| $[(\blacksquare)^{2T} + \Gamma_5, 2A_5, 2M_5, Z_5 Z_5, 2R_1, 2X_1]$                           |
| $[(\blacksquare)^{2T} + \Gamma_5, A_1 A_2 + A_3 A_4, M_1 M_3 + M_2 M_4, Z_5 Z_5, 2R_1, 2X_1]$ |

2nd minimal solution:  $\mu_2^T = 6$  (4 symmetry vectors)

Space group 105 ( $\mathbb{Z}_1$ )

1st minimal solution:  $\mu_1^T = 2$  (4 symmetry vectors)

| $\mathbf{n}^T$                                                         |
|------------------------------------------------------------------------|
| $[(\blacksquare)^{2T}, A_5, M_5, Z_5, R_3 + R_4, X_3 + X_4]$           |
| $[(\blacksquare)^{2T}, A_1 A_2, M_1 + M_2, Z_5, R_1 + R_4, X_1 + X_4]$ |
| $[(\blacksquare)^{2T}, A_5, M_5, Z_5, R_1 + R_2, X_1 + X_2]$           |
| $[(\blacksquare)^{2T}, A_3 A_4, M_3 + M_4, Z_5, R_2 + R_3, X_2 + X_3]$ |

2nd minimal solution:  $\mu_2^T = 4$  (32 symmetry vectors)

Space group 106 ( $\mathbb{Z}_1$ )

1st minimal solution:  $\mu_1^T = 4$  (2 symmetry vectors)

| $\mathbf{n}^T$                                                                             |
|--------------------------------------------------------------------------------------------|
| $[(\blacksquare)^{2T} + \Gamma_5, A_1 A_4 + A_2 A_3, M_1 M_3 + M_2 M_4, 2Z_5, 2R_1, 2X_1]$ |
| $[(\blacksquare)^{2T} + \Gamma_5, A_5 A_5, 2M_5, 2Z_5, 2R_1, 2X_1]$                        |

2nd minimal solution:  $\mu_2^T = 8$  (6 symmetry vectors)

Space group 107 ( $\mathbb{Z}_1$ )

1st minimal solution:  $\mu_1^T = 2$  (2 symmetry vectors)

| $\mathbf{n}^T$                                                |
|---------------------------------------------------------------|
| $[(\blacksquare)^{2T}, M_5, P_3 P_4, X_3 + X_4, N_1 + N_2]$   |
| $[(\blacksquare)^{2T}, M_5, P_1 + P_2, X_1 + X_2, N_1 + N_2]$ |

2nd minimal solution:  $\mu_2^T = 3$  (8 symmetry vectors)

Space group 108 ( $\mathbb{Z}_1$ )

1st minimal solution:  $\mu_1^T = 2$  (1 symmetry vector)

| $\mathbf{n}^T$                                            |
|-----------------------------------------------------------|
| $[(\blacksquare)^{2T}, M_5, P_1 P_2, X_1 + X_2, N_1 N_2]$ |

2nd minimal solution:  $\mu_2^T = 4$  (8 symmetry vectors)

Space group 109 ( $\mathbb{Z}_1$ )

1st minimal solution:  $\mu_1^T = 2$  (1 symmetry vector)

| $\mathbf{n}^T$                                    |
|---------------------------------------------------|
| $[(\blacksquare)^{2T}, M_5, P_1, X_1, N_1 + N_2]$ |

2nd minimal solution:  $\mu_2^T = 4$  (3 symmetry vectors)

Space group 110 ( $\mathbb{Z}_1$ )

1st minimal solution:  $\mu_1^T = 4$  (1 symmetry vector)

|                                                                 |
|-----------------------------------------------------------------|
| $\mathbf{n}^T$                                                  |
| $[(\blacksquare)^{2T} + \Gamma_5, 2M_5, P_1P_1, 2X_1, 2N_1N_2]$ |

2nd minimal solution:  $\mu_2^T = 8$  (2 symmetry vectors)

Space group 111 ( $\mathbb{Z}_1$ )

1st minimal solution:  $\mu_1^T = 2$  (8 symmetry vectors)

|                                                                          |
|--------------------------------------------------------------------------|
| $\mathbf{n}^T$                                                           |
| $[(\blacksquare)^{2T}, A_2 + A_3, M_1 + M_2, Z_5, R_3 + R_4, 2X_3]$      |
| $[(\blacksquare)^{2T}, A_3 + A_4, M_1 + M_4, Z_5, R_2 + R_4, X_2 + X_3]$ |
| $[(\blacksquare)^{2T}, A_1 + A_2, M_1 + M_4, Z_5, R_1 + R_3, X_2 + X_3]$ |
| $[(\blacksquare)^{2T}, A_1 + A_4, M_1 + M_2, Z_5, R_3 + R_4, 2X_3]$      |
| $[(\blacksquare)^{2T}, A_1 + A_2, M_2 + M_3, Z_5, R_1 + R_3, X_2 + X_3]$ |
| $[(\blacksquare)^{2T}, A_2 + A_3, M_3 + M_4, Z_5, R_1 + R_2, 2X_2]$      |
| $[(\blacksquare)^{2T}, A_1 + A_4, M_3 + M_4, Z_5, R_1 + R_2, 2X_2]$      |
| $[(\blacksquare)^{2T}, A_3 + A_4, M_2 + M_3, Z_5, R_2 + R_4, X_2 + X_3]$ |

2nd minimal solution:  $\mu_2^T = 3$  (192 symmetry vectors)

Space group 112 ( $\mathbb{Z}_1$ )

1st minimal solution:  $\mu_1^T = 2$  (4 symmetry vectors)

|                                                                       |
|-----------------------------------------------------------------------|
| $\mathbf{n}^T$                                                        |
| $[(\blacksquare)^{2T}, A_5, M_2 + M_3, Z_3Z_4, R_1 + R_4, X_2 + X_3]$ |
| $[(\blacksquare)^{2T}, A_5, M_1 + M_4, Z_3Z_4, R_1 + R_4, X_2 + X_3]$ |
| $[(\blacksquare)^{2T}, A_5, M_2 + M_3, Z_1Z_2, R_2 + R_3, X_2 + X_3]$ |
| $[(\blacksquare)^{2T}, A_5, M_1 + M_4, Z_1Z_2, R_2 + R_3, X_2 + X_3]$ |

2nd minimal solution:  $\mu_2^T = 4$  (152 symmetry vectors)

Space group 113 ( $\mathbb{Z}_1$ )

1st minimal solution:  $\mu_1^T = 4$  (6 symmetry vectors)

| $\mathbf{n}^T$                                                                                               |
|--------------------------------------------------------------------------------------------------------------|
| $[(\blacksquare)^{2T} + 2\Gamma_2, A_2A_4 + A_5, M_2M_4 + M_5, Z_2 + Z_4 + Z_5, 2R_1, 2X_1]$                 |
| $[(\blacksquare)^{2T} + \Gamma_1 + \Gamma_2, 2A_5, 2M_5, Z_2 + Z_3 + Z_5, 2R_1, 2X_1]$                       |
| $[(\blacksquare)^{2T} + \Gamma_1 + \Gamma_2, 2A_5, 2M_5, Z_1 + Z_4 + Z_5, 2R_1, 2X_1]$                       |
| $[(\blacksquare)^{2T} + \Gamma_1 + \Gamma_2, A_1A_3 + A_2A_4, M_1M_3 + M_2M_4, Z_1 + Z_4 + Z_5, 2R_1, 2X_1]$ |
| $[(\blacksquare)^{2T} + 2\Gamma_1, A_1A_3 + A_5, M_1M_3 + M_5, Z_1 + Z_3 + Z_5, 2R_1, 2X_1]$                 |
| $[(\blacksquare)^{2T} + \Gamma_1 + \Gamma_2, A_1A_3 + A_2A_4, M_1M_3 + M_2M_4, Z_2 + Z_3 + Z_5, 2R_1, 2X_1]$ |

2nd minimal solution:  $\mu_2^T = 6$  (38 symmetry vectors)

Space group 114 ( $\mathbb{Z}_1$ )

1st minimal solution:  $\mu_1^T = 6$  (6 symmetry vectors)

| $\mathbf{n}^T$                                                                                                                      |
|-------------------------------------------------------------------------------------------------------------------------------------|
| $[(\blacksquare)^{2T} + \Gamma_1 + \Gamma_2 + \Gamma_5, A_2A_3 + A_5A_5, M_1M_3 + M_2M_4 + M_5, Z_1Z_2 + Z_3Z_4 + Z_5, 3R_1, 3X_1]$ |
| $[(\blacksquare)^{2T} + \Gamma_1 + \Gamma_2 + \Gamma_5, A_1A_4 + A_5A_5, M_1M_3 + M_2M_4 + M_5, Z_1Z_2 + Z_3Z_4 + Z_5, 3R_1, 3X_1]$ |
| $[(\blacksquare)^{2T} + \Gamma_1 + \Gamma_2 + \Gamma_5, 3A_2A_3, 3M_5, Z_1Z_2 + Z_3Z_4 + Z_5, 3R_1, 3X_1]$                          |
| $[(\blacksquare)^{2T} + \Gamma_1 + \Gamma_2 + \Gamma_5, A_1A_4 + 2A_2A_3, 3M_5, Z_1Z_2 + Z_3Z_4 + Z_5, 3R_1, 3X_1]$                 |
| $[(\blacksquare)^{2T} + \Gamma_1 + \Gamma_2 + \Gamma_5, 2A_1A_4 + A_2A_3, 3M_5, Z_1Z_2 + Z_3Z_4 + Z_5, 3R_1, 3X_1]$                 |
| $[(\blacksquare)^{2T} + \Gamma_1 + \Gamma_2 + \Gamma_5, 3A_1A_4, 3M_5, Z_1Z_2 + Z_3Z_4 + Z_5, 3R_1, 3X_1]$                          |

2nd minimal solution:  $\mu_2^T = 8$  (18 symmetry vectors)

Space group 115 ( $\mathbb{Z}_1$ )

1st minimal solution:  $\mu_1^T = 2$  (6 symmetry vectors)

| $\mathbf{n}^T$                                                           |
|--------------------------------------------------------------------------|
| $[(\blacksquare)^{2T}, A_3 + A_4, 2M_3, Z_5, R_2 + R_3, X_2 + X_3]$      |
| $[(\blacksquare)^{2T}, A_2 + A_4, M_2 + M_3, Z_5, R_3 + R_4, X_3 + X_4]$ |
| $[(\blacksquare)^{2T}, A_2 + A_4, M_2 + M_3, Z_5, R_1 + R_2, X_1 + X_2]$ |
| $[(\blacksquare)^{2T}, A_1 + A_3, M_2 + M_3, Z_5, R_3 + R_4, X_3 + X_4]$ |
| $[(\blacksquare)^{2T}, A_1 + A_3, M_2 + M_3, Z_5, R_1 + R_2, X_1 + X_2]$ |
| $[(\blacksquare)^{2T}, A_1 + A_2, 2M_2, Z_5, R_1 + R_4, X_1 + X_4]$      |

2nd minimal solution:  $\mu_2^T = 3$  (128 symmetry vectors)

Space group 116 ( $\mathbb{Z}_1$ )

1st minimal solution:  $\mu_1^T = 4$  (30 symmetry vectors)

| $\mathbf{n}^T$                                                                                                      |
|---------------------------------------------------------------------------------------------------------------------|
| $[(\blacksquare)^{2T} + \Gamma_5, 2A_5, 2M_2 + M_3 + M_4, Z_1Z_4 + Z_2Z_3, 2R_3R_4, 2X_3 + 2X_4]$                   |
| $[(\blacksquare)^{2T} + \Gamma_5, 2A_5, 2M_2 + M_3 + M_4, Z_1Z_4 + Z_2Z_3, R_1R_2 + R_3R_4, X_1 + X_2 + X_3 + X_4]$ |

... continued on next page



... continued from previous page

---

|                                                                                                                                        |
|----------------------------------------------------------------------------------------------------------------------------------------|
| $[(\blacksquare)^{2T} + \Gamma_5, 2A_5, M_1 + M_2 + 2M_3, Z_1 Z_4 + Z_2 Z_3, 2R_3 R_4, 2X_3 + 2X_4]$                                   |
| $[(\blacksquare)^{2T} + \Gamma_5, 2A_5, M_1 + M_2 + 2M_3, Z_1 Z_4 + Z_2 Z_3, R_1 R_2 + R_3 R_4, X_1 + X_2 + X_3 + X_4]$                |
| $[(\blacksquare)^{2T} + \Gamma_5, 2A_5, 2M_2 + M_3 + M_4, Z_1 Z_4 + Z_2 Z_3, 2R_1 R_2, 2X_1 + 2X_2]$                                   |
| $[(\blacksquare)^{2T} + \Gamma_5, 2A_5, M_1 + M_2 + 2M_3, Z_1 Z_4 + Z_2 Z_3, 2R_1 R_2, 2X_1 + 2X_2]$                                   |
| $[(\blacksquare)^{2T} + \Gamma_2 + \Gamma_4, A_1 A_4 + A_5, M_2 + M_3 + M_5, Z_1 Z_4 + Z_5, 2R_3 R_4, 2X_3 + 2X_4]$                    |
| $[(\blacksquare)^{2T} + \Gamma_2 + \Gamma_4, A_1 A_4 + A_5, M_2 + M_3 + M_5, Z_1 Z_4 + Z_5, R_1 R_2 + R_3 R_4, X_1 + X_2 + X_3 + X_4]$ |
| $[(\blacksquare)^{2T} + \Gamma_1 + \Gamma_4, A_1 A_4 + A_5, M_2 + M_4 + M_5, Z_1 Z_4 + Z_5, 2R_3 R_4, 2X_3 + 2X_4]$                    |
| $[(\blacksquare)^{2T} + \Gamma_1 + \Gamma_3, A_1 A_4 + A_5, M_2 + M_3 + M_5, Z_1 Z_4 + Z_5, 2R_3 R_4, 2X_3 + 2X_4]$                    |
| $[(\blacksquare)^{2T} + \Gamma_1 + \Gamma_4, A_1 A_4 + A_5, M_2 + M_4 + M_5, Z_1 Z_4 + Z_5, R_1 R_2 + R_3 R_4, X_1 + X_2 + X_3 + X_4]$ |
| $[(\blacksquare)^{2T} + \Gamma_1 + \Gamma_3, A_1 A_4 + A_5, M_2 + M_3 + M_5, Z_1 Z_4 + Z_5, R_1 R_2 + R_3 R_4, X_1 + X_2 + X_3 + X_4]$ |
| $[(\blacksquare)^{2T} + \Gamma_1 + \Gamma_4, A_1 A_4 + A_5, M_1 + M_3 + M_5, Z_1 Z_4 + Z_5, 2R_3 R_4, 2X_3 + 2X_4]$                    |
| $[(\blacksquare)^{2T} + \Gamma_1 + \Gamma_4, A_1 A_4 + A_5, M_1 + M_3 + M_5, Z_1 Z_4 + Z_5, R_1 R_2 + R_3 R_4, X_1 + X_2 + X_3 + X_4]$ |
| $[(\blacksquare)^{2T} + \Gamma_2 + \Gamma_4, A_1 A_4 + A_5, M_2 + M_3 + M_5, Z_1 Z_4 + Z_5, 2R_1 R_2, 2X_1 + 2X_2]$                    |
| $[(\blacksquare)^{2T} + \Gamma_1 + \Gamma_4, A_1 A_4 + A_5, M_2 + M_4 + M_5, Z_1 Z_4 + Z_5, 2R_1 R_2, 2X_1 + 2X_2]$                    |
| $[(\blacksquare)^{2T} + \Gamma_1 + \Gamma_3, A_1 A_4 + A_5, M_2 + M_3 + M_5, Z_1 Z_4 + Z_5, 2R_1 R_2, 2X_1 + 2X_2]$                    |
| $[(\blacksquare)^{2T} + \Gamma_1 + \Gamma_4, A_1 A_4 + A_5, M_1 + M_3 + M_5, Z_1 Z_4 + Z_5, 2R_1 R_2, 2X_1 + 2X_2]$                    |
| $[(\blacksquare)^{2T} + \Gamma_2 + \Gamma_4, A_2 A_3 + A_5, M_2 + M_3 + M_5, Z_2 Z_3 + Z_5, 2R_3 R_4, 2X_3 + 2X_4]$                    |
| $[(\blacksquare)^{2T} + \Gamma_2 + \Gamma_4, A_2 A_3 + A_5, M_2 + M_3 + M_5, Z_2 Z_3 + Z_5, R_1 R_2 + R_3 R_4, X_1 + X_2 + X_3 + X_4]$ |
| $[(\blacksquare)^{2T} + \Gamma_1 + \Gamma_4, A_2 A_3 + A_5, M_2 + M_4 + M_5, Z_2 Z_3 + Z_5, 2R_3 R_4, 2X_3 + 2X_4]$                    |
| $[(\blacksquare)^{2T} + \Gamma_1 + \Gamma_3, A_2 A_3 + A_5, M_2 + M_3 + M_5, Z_2 Z_3 + Z_5, 2R_3 R_4, 2X_3 + 2X_4]$                    |
| $[(\blacksquare)^{2T} + \Gamma_1 + \Gamma_4, A_2 A_3 + A_5, M_2 + M_4 + M_5, Z_2 Z_3 + Z_5, R_1 R_2 + R_3 R_4, X_1 + X_2 + X_3 + X_4]$ |
| $[(\blacksquare)^{2T} + \Gamma_1 + \Gamma_3, A_2 A_3 + A_5, M_2 + M_3 + M_5, Z_2 Z_3 + Z_5, R_1 R_2 + R_3 R_4, X_1 + X_2 + X_3 + X_4]$ |
| $[(\blacksquare)^{2T} + \Gamma_1 + \Gamma_4, A_2 A_3 + A_5, M_1 + M_3 + M_5, Z_2 Z_3 + Z_5, 2R_3 R_4, 2X_3 + 2X_4]$                    |
| $[(\blacksquare)^{2T} + \Gamma_1 + \Gamma_4, A_2 A_3 + A_5, M_1 + M_3 + M_5, Z_2 Z_3 + Z_5, R_1 R_2 + R_3 R_4, X_1 + X_2 + X_3 + X_4]$ |
| $[(\blacksquare)^{2T} + \Gamma_2 + \Gamma_4, A_2 A_3 + A_5, M_2 + M_3 + M_5, Z_2 Z_3 + Z_5, 2R_1 R_2, 2X_1 + 2X_2]$                    |
| $[(\blacksquare)^{2T} + \Gamma_1 + \Gamma_4, A_2 A_3 + A_5, M_2 + M_4 + M_5, Z_2 Z_3 + Z_5, 2R_1 R_2, 2X_1 + 2X_2]$                    |
| $[(\blacksquare)^{2T} + \Gamma_1 + \Gamma_3, A_2 A_3 + A_5, M_2 + M_3 + M_5, Z_2 Z_3 + Z_5, 2R_1 R_2, 2X_1 + 2X_2]$                    |
| $[(\blacksquare)^{2T} + \Gamma_1 + \Gamma_4, A_2 A_3 + A_5, M_1 + M_3 + M_5, Z_2 Z_3 + Z_5, 2R_1 R_2, 2X_1 + 2X_2]$                    |

---

2nd minimal solution:  $\mu_2^T = 6$  (256 symmetry vectors)

Space group 117 ( $Z_1$ )

1st minimal solution:  $\mu_1^T = 4$  (10 symmetry vectors)

---

| $n^T$                                                                                                            |
|------------------------------------------------------------------------------------------------------------------|
| $[(\blacksquare)^{2T} + \Gamma_2 + \Gamma_4, A_2 A_3 + A_5, M_1 M_4 + M_5, Z_1 + Z_4 + Z_5, 2R_1, 2X_1]$         |
| $[(\blacksquare)^{2T} + \Gamma_2 + \Gamma_4, A_1 A_4 + A_5, M_1 M_4 + M_5, Z_2 + Z_3 + Z_5, 2R_1, 2X_1]$         |
| $[(\blacksquare)^{2T} + \Gamma_1 + \Gamma_4, 2A_5, 2M_5, Z_2 + Z_4 + Z_5, 2R_1, 2X_1]$                           |
| $[(\blacksquare)^{2T} + \Gamma_1 + \Gamma_4, 2A_5, 2M_5, Z_1 + Z_3 + Z_5, 2R_1, 2X_1]$                           |
| $[(\blacksquare)^{2T} + \Gamma_2 + \Gamma_3, A_1 A_4 + A_2 A_3, 2M_1 M_4, Z_1 + Z_3 + Z_5, 2R_1, 2X_1]$          |
| $[(\blacksquare)^{2T} + \Gamma_1 + \Gamma_3, A_2 A_3 + A_5, M_1 M_4 + M_5, Z_1 + Z_4 + Z_5, 2R_1, 2X_1]$         |
| $[(\blacksquare)^{2T} + \Gamma_1 + \Gamma_4, A_1 A_4 + A_2 A_3, M_1 M_4 + M_2 M_3, Z_1 + Z_3 + Z_5, 2R_1, 2X_1]$ |
| $[(\blacksquare)^{2T} + \Gamma_1 + \Gamma_3, A_1 A_4 + A_5, M_1 M_4 + M_5, Z_2 + Z_3 + Z_5, 2R_1, 2X_1]$         |
| $[(\blacksquare)^{2T} + \Gamma_2 + \Gamma_3, A_1 A_4 + A_2 A_3, 2M_1 M_4, Z_2 + Z_4 + Z_5, 2R_1, 2X_1]$          |
| $[(\blacksquare)^{2T} + \Gamma_1 + \Gamma_4, A_1 A_4 + A_2 A_3, M_1 M_4 + M_2 M_3, Z_2 + Z_4 + Z_5, 2R_1, 2X_1]$ |

---

2nd minimal solution:  $\mu_2^T = 6$  (76 symmetry vectors)

Space group 118 ( $\mathbb{Z}_1$ )

1st minimal solution:  $\mu_1^T = 4$  (10 symmetry vectors)

| $\mathbf{n}^T$                                                                                         |
|--------------------------------------------------------------------------------------------------------|
| $[(\blacksquare)^{2T} + \Gamma_1 + \Gamma_3, A_2 + A_3 + A_5, M_1M_4 + M_5, Z_1Z_4 + Z_5, 2R_1, 2X_1]$ |
| $[(\blacksquare)^{2T} + \Gamma_1 + \Gamma_3, A_1 + A_4 + A_5, M_1M_4 + M_5, Z_2Z_3 + Z_5, 2R_1, 2X_1]$ |
| $[(\blacksquare)^{2T} + \Gamma_1 + \Gamma_4, 2A_2 + A_3 + A_4, 2M_5, Z_1Z_4 + Z_5, 2R_1, 2X_1]$        |
| $[(\blacksquare)^{2T} + \Gamma_1 + \Gamma_4, A_1 + A_2 + 2A_4, 2M_5, Z_2Z_3 + Z_5, 2R_1, 2X_1]$        |
| $[(\blacksquare)^{2T} + \Gamma_1 + \Gamma_4, A_1 + A_2 + 2A_3, 2M_5, Z_1Z_4 + Z_5, 2R_1, 2X_1]$        |
| $[(\blacksquare)^{2T} + \Gamma_1 + \Gamma_4, 2A_1 + A_3 + A_4, 2M_5, Z_2Z_3 + Z_5, 2R_1, 2X_1]$        |
| $[(\blacksquare)^{2T} + \Gamma_2 + \Gamma_4, A_2 + A_3 + A_5, M_1M_4 + M_5, Z_1Z_4 + Z_5, 2R_1, 2X_1]$ |
| $[(\blacksquare)^{2T} + \Gamma_2 + \Gamma_4, A_1 + A_4 + A_5, M_1M_4 + M_5, Z_2Z_3 + Z_5, 2R_1, 2X_1]$ |
| $[(\blacksquare)^{2T} + \Gamma_5, A_2 + A_4 + A_5, M_1M_4 + M_5, Z_1Z_4 + Z_2Z_3, 2R_1, 2X_1]$         |
| $[(\blacksquare)^{2T} + \Gamma_5, A_1 + A_3 + A_5, M_1M_4 + M_5, Z_1Z_4 + Z_2Z_3, 2R_1, 2X_1]$         |

2nd minimal solution:  $\mu_2^T = 6$  (64 symmetry vectors)

Space group 119 ( $\mathbb{Z}_1$ )

1st minimal solution:  $\mu_1^T = 2$  (4 symmetry vectors)

| $\mathbf{n}^T$                                                |
|---------------------------------------------------------------|
| $[(\blacksquare)^{2T}, M_5, P_2 + P_4, X_2 + X_4, N_1 + N_2]$ |
| $[(\blacksquare)^{2T}, M_5, P_2 + P_3, X_2 + X_4, N_1 + N_2]$ |
| $[(\blacksquare)^{2T}, M_5, P_1 + P_4, X_2 + X_4, N_1 + N_2]$ |
| $[(\blacksquare)^{2T}, M_5, P_1 + P_3, X_2 + X_4, N_1 + N_2]$ |

2nd minimal solution:  $\mu_2^T = 3$  (64 symmetry vectors)

Space group 120 ( $\mathbb{Z}_1$ )

1st minimal solution:  $\mu_1^T = 4$  (16 symmetry vectors)

| $\mathbf{n}^T$                                                                                             |
|------------------------------------------------------------------------------------------------------------|
| $[(\blacksquare)^{2T} + \Gamma_2 + \Gamma_3, M_1 + M_3 + M_5, P_1P_2 + P_3P_4, 2X_2 + 2X_4, 2N_1N_2]$      |
| $[(\blacksquare)^{2T} + \Gamma_2 + \Gamma_4, M_2 + M_3 + M_5, P_1P_2 + P_3P_4, 2X_2 + X_3 + X_4, 2N_1N_2]$ |
| $[(\blacksquare)^{2T} + \Gamma_2 + \Gamma_4, M_2 + M_3 + M_5, 2P_1P_2, X_1 + 3X_2, 2N_1N_2]$               |
| $[(\blacksquare)^{2T} + \Gamma_1 + \Gamma_3, M_2 + M_3 + M_5, P_1P_2 + P_3P_4, 2X_2 + X_3 + X_4, 2N_1N_2]$ |
| $[(\blacksquare)^{2T} + \Gamma_1 + \Gamma_3, M_2 + M_3 + M_5, 2P_1P_2, X_1 + 3X_2, 2N_1N_2]$               |
| $[(\blacksquare)^{2T} + \Gamma_1 + \Gamma_4, M_1 + M_3 + M_5, 2P_1P_2, 2X_1 + 2X_2, 2N_1N_2]$              |
| $[(\blacksquare)^{2T} + \Gamma_2 + \Gamma_4, M_1 + M_4 + M_5, 2P_3P_4, X_3 + 3X_4, 2N_1N_2]$               |
| $[(\blacksquare)^{2T} + \Gamma_2 + \Gamma_4, M_1 + M_4 + M_5, P_1P_2 + P_3P_4, X_1 + X_2 + 2X_4, 2N_1N_2]$ |
| $[(\blacksquare)^{2T} + \Gamma_1 + \Gamma_3, M_1 + M_4 + M_5, 2P_3P_4, X_3 + 3X_4, 2N_1N_2]$               |
| $[(\blacksquare)^{2T} + \Gamma_1 + \Gamma_3, M_1 + M_4 + M_5, P_1P_2 + P_3P_4, X_1 + X_2 + 2X_4, 2N_1N_2]$ |
| $[(\blacksquare)^{2T} + \Gamma_1 + \Gamma_4, M_1 + M_3 + M_5, 2P_3P_4, 2X_3 + 2X_4, 2N_1N_2]$              |
| $[(\blacksquare)^{2T} + \Gamma_1 + \Gamma_4, M_2 + M_4 + M_5, 2P_3P_4, 2X_3 + 2X_4, 2N_1N_2]$              |

... continued on next page

... continued from previous page

---

|                                                                                                                 |
|-----------------------------------------------------------------------------------------------------------------|
| $[(\blacksquare)^{2T} + \Gamma_1 + \Gamma_4, M_2 + M_4 + M_5, P_1P_2 + P_3P_4, X_1 + X_2 + X_3 + X_4, 2N_1N_2]$ |
| $[(\blacksquare)^{2T} + \Gamma_1 + \Gamma_4, M_1 + M_3 + M_5, P_1P_2 + P_3P_4, X_1 + X_2 + X_3 + X_4, 2N_1N_2]$ |
| $[(\blacksquare)^{2T} + \Gamma_1 + \Gamma_4, M_2 + M_4 + M_5, 2P_1P_2, 2X_1 + 2X_2, 2N_1N_2]$                   |
| $[(\blacksquare)^{2T} + \Gamma_2 + \Gamma_3, M_2 + M_4 + M_5, P_1P_2 + P_3P_4, 2X_2 + 2X_4, 2N_1N_2]$           |

---

2nd minimal solution:  $\mu_2^T = 6$  (128 symmetry vectors)

Space group 121 ( $\mathbb{Z}_1$ )

1st minimal solution:  $\mu_1^T = 3$  (16 symmetry vectors)

---

| $\mathbf{n}^T$                                                                                             |
|------------------------------------------------------------------------------------------------------------|
| $[(\blacksquare)^{2T} + \Gamma_2, M_4 + M_5, P_2 + P_5, PA_2 + PA_5, X_2 + X_3 + X_4, 2N_1 + N_2]$         |
| $[(\blacksquare)^{2T} + \Gamma_2, M_4 + M_5, P_4 + P_5, PA_4 + PA_5, X_2 + X_3 + X_4, N_1 + 2N_2]$         |
| $[(\blacksquare)^{2T} + \Gamma_1, M_3 + M_5, P_1 + P_5, PA_1 + PA_5, X_1 + X_3 + X_4, 2N_1 + N_2]$         |
| $[(\blacksquare)^{2T} + \Gamma_1, M_3 + M_5, P_3 + P_5, PA_3 + PA_5, X_1 + X_3 + X_4, N_1 + 2N_2]$         |
| $[(\blacksquare)^{2T} + \Gamma_1, M_3 + M_5, 2P_1 + P_2, 2PA_1 + PA_2, 2X_1 + X_2, 3N_1]$                  |
| $[(\blacksquare)^{2T} + \Gamma_1, M_3 + M_5, P_1 + P_2 + P_3, PA_1 + PA_2 + PA_3, 2X_1 + X_2, 2N_1 + N_2]$ |
| $[(\blacksquare)^{2T} + \Gamma_1, M_3 + M_5, P_2 + 2P_3, PA_2 + 2PA_3, 2X_1 + X_2, N_1 + 2N_2]$            |
| $[(\blacksquare)^{2T} + \Gamma_1, M_3 + M_5, 2P_1 + P_4, 2PA_1 + PA_4, 2X_1 + X_2, 2N_1 + N_2]$            |
| $[(\blacksquare)^{2T} + \Gamma_1, M_3 + M_5, P_1 + P_3 + P_4, PA_1 + PA_3 + PA_4, 2X_1 + X_2, N_1 + 2N_2]$ |
| $[(\blacksquare)^{2T} + \Gamma_1, M_3 + M_5, 2P_3 + P_4, 2PA_3 + PA_4, 2X_1 + X_2, 3N_2]$                  |
| $[(\blacksquare)^{2T} + \Gamma_2, M_4 + M_5, P_1 + 2P_2, PA_1 + 2PA_2, X_1 + 2X_2, 3N_1]$                  |
| $[(\blacksquare)^{2T} + \Gamma_2, M_4 + M_5, 2P_2 + P_3, 2PA_2 + PA_3, X_1 + 2X_2, 2N_1 + N_2]$            |
| $[(\blacksquare)^{2T} + \Gamma_2, M_4 + M_5, P_1 + P_2 + P_4, PA_1 + PA_2 + PA_4, X_1 + 2X_2, 2N_1 + N_2]$ |
| $[(\blacksquare)^{2T} + \Gamma_2, M_4 + M_5, P_2 + P_3 + P_4, PA_2 + PA_3 + PA_4, X_1 + 2X_2, N_1 + 2N_2]$ |
| $[(\blacksquare)^{2T} + \Gamma_2, M_4 + M_5, P_1 + 2P_4, PA_1 + 2PA_4, X_1 + 2X_2, N_1 + 2N_2]$            |
| $[(\blacksquare)^{2T} + \Gamma_2, M_4 + M_5, P_3 + 2P_4, PA_3 + 2PA_4, X_1 + 2X_2, 3N_2]$                  |

---

2nd minimal solution:  $\mu_2^T = 4$  (100 symmetry vectors)

Space group 122 ( $\mathbb{Z}_1$ )

1st minimal solution:  $\mu_1^T = 2$  (2 symmetry vectors)

---

| $\mathbf{n}^T$                                             |
|------------------------------------------------------------|
| $[(\blacksquare)^{2T}, M_3M_4, P_2, PA_2, X_1, N_1 + N_2]$ |
| $[(\blacksquare)^{2T}, M_3M_4, P_1, PA_1, X_1, N_1 + N_2]$ |

---

2nd minimal solution:  $\mu_2^T = 4$  (6 symmetry vectors)

Space group 123 ( $\mathbb{Z}_1$ )

1st minimal solution:  $\mu_1^T = 2$  (8 symmetry vectors)

| $\mathbf{n}^T$                                                                             |
|--------------------------------------------------------------------------------------------|
| $[(\blacksquare)^{2T}, A_2^-, A_4^-, M_2^+ + M_2^-, Z_5^+, R_3^+ + R_4^+, X_3^+ + X_3^-]$  |
| $[(\blacksquare)^{2T}, A_2^+ + A_4^+, M_2^+ + M_2^-, Z_5^-, R_3^- + R_4^-, X_3^+ + X_3^-]$ |
| $[(\blacksquare)^{2T}, A_3^+ + A_4^+, M_2^- + M_3^-, Z_5^-, R_2^+ + R_4^-, X_2^+ + X_3^+]$ |
| $[(\blacksquare)^{2T}, A_1^- + A_2^-, M_2^- + M_3^+, Z_5^+, R_1^- + R_3^+, X_2^+ + X_3^+]$ |
| $[(\blacksquare)^{2T}, A_1^+ + A_2^+, M_2^+ + M_3^-, Z_5^-, R_1^+ + R_3^-, X_2^- + X_3^-]$ |
| $[(\blacksquare)^{2T}, A_3^- + A_4^-, M_2^+ + M_3^-, Z_5^+, R_2^- + R_4^+, X_2^- + X_3^-]$ |
| $[(\blacksquare)^{2T}, A_1^+ + A_3^+, M_3^+ + M_3^-, Z_5^-, R_1^+ + R_2^+, X_2^+ + X_2^-]$ |
| $[(\blacksquare)^{2T}, A_1^- + A_3^-, M_3^+ + M_3^-, Z_5^+, R_1^- + R_2^-, X_2^+ + X_2^-]$ |

2nd minimal solution:  $\mu_2^T = 3$  (360 symmetry vectors)

Space group 124 ( $\mathbb{Z}_2$ )

1st minimal solution:  $\mu_1^T = 4$  (16 symmetry vectors)

| $\mathbf{n}^T$                                                                                                                   | $\mathbf{v}^T \in \mathbb{Z}_2$ |
|----------------------------------------------------------------------------------------------------------------------------------|---------------------------------|
| $[(\blacksquare)^{2T} + \Gamma_5^-, 2A_1, 2M_2^+ + M_2^- + M_4^+, Z_3Z_4, 2R_2, X_3^+ + 2X_3^- + X_4^-]$                         | trivial                         |
| $[(\blacksquare)^{2T} + \Gamma_5^-, 2A_1, 2M_2^+ + M_2^- + M_4^+, Z_3Z_4, R_1 + R_2, X_1^+ + X_2^+ + X_3^+ + X_3^-]$             | 1                               |
| $[(\blacksquare)^{2T} + \Gamma_5^+, 2A_1, M_2^+ + 2M_2^- + M_4^-, Z_3Z_4, R_1 + R_2, X_1^- + X_2^- + X_3^+ + X_3^-]$             | 1                               |
| $[(\blacksquare)^{2T} + \Gamma_5^+, 2A_1, M_2^+ + 2M_2^- + M_4^-, Z_3Z_4, 2R_2, 2X_3^+ + X_3^- + X_4^+]$                         | trivial                         |
| $[(\blacksquare)^{2T} + \Gamma_5^-, A_1 + A_2, M_1^+ + M_2^+ + M_2^- + M_3^+, Z_3Z_4, 2R_2, X_3^+ + 2X_3^- + X_4^-]$             | 1                               |
| $[(\blacksquare)^{2T} + \Gamma_5^-, A_1 + A_2, M_1^+ + M_2^+ + M_2^- + M_3^+, Z_3Z_4, R_1 + R_2, X_1^+ + X_2^+ + X_3^+ + X_3^-]$ | trivial                         |
| $[(\blacksquare)^{2T} + \Gamma_5^+, A_1 + A_2, M_2^- + M_3^+ + M_3^- + M_4^-, Z_3Z_4, R_1 + R_2, X_2^+ + X_2^- + X_3^+ + X_4^+]$ | trivial                         |
| $[(\blacksquare)^{2T} + \Gamma_5^+, A_1 + A_2, M_1^- + M_2^+ + M_2^- + M_3^-, Z_3Z_4, R_1 + R_2, X_1^- + X_2^- + X_3^+ + X_3^-]$ | trivial                         |
| $[(\blacksquare)^{2T} + \Gamma_5^+, A_1 + A_2, M_1^- + M_2^+ + M_2^- + M_3^-, Z_3Z_4, 2R_2, 2X_3^+ + X_3^- + X_4^+]$             | 1                               |
| $[(\blacksquare)^{2T} + \Gamma_5^-, A_1 + A_2, M_2^+ + M_3^+ + M_3^- + M_4^+, Z_3Z_4, R_1 + R_2, X_2^+ + X_2^- + X_3^- + X_4^-]$ | trivial                         |
| $[(\blacksquare)^{2T} + \Gamma_5^+, A_1 + A_2, M_2^+ + M_3^+ + M_3^- + M_4^+, Z_3Z_4, 2R_1, X_1^+ + 2X_2^+ + X_2^-]$             | 1                               |
| $[(\blacksquare)^{2T} + \Gamma_5^+, A_1 + A_2, M_2^- + M_3^+ + M_3^- + M_4^-, Z_3Z_4, 2R_1, X_1^- + X_2^+ + 2X_2^-]$             | 1                               |
| $[(\blacksquare)^{2T} + \Gamma_5^-, 2A_2, M_1^+ + 2M_3^+ + M_3^-, Z_3Z_4, R_1 + R_2, X_2^+ + X_2^- + X_3^- + X_4^-]$             | 1                               |
| $[(\blacksquare)^{2T} + \Gamma_5^-, 2A_2, M_1^+ + 2M_3^+ + M_3^-, Z_3Z_4, 2R_1, X_1^+ + 2X_2^+ + X_2^-]$                         | trivial                         |
| $[(\blacksquare)^{2T} + \Gamma_5^+, 2A_2, M_1^- + M_3^+ + 2M_3^-, Z_3Z_4, 2R_1, X_1^- + X_2^+ + 2X_2^-]$                         | trivial                         |
| $[(\blacksquare)^{2T} + \Gamma_5^+, 2A_2, M_1^- + M_3^+ + 2M_3^-, Z_3Z_4, R_1 + R_2, X_2^+ + X_2^- + X_3^+ + X_4^+]$             | 1                               |

2nd minimal solution:  $\mu_2^T = 6$  (520 symmetry vectors)

Space group 125 ( $\mathbb{Z}_1$ )

1st minimal solution:  $\mu_1^T = 4$  (20 symmetry vectors)

| $\mathbf{n}^T$                                                                                                       |
|----------------------------------------------------------------------------------------------------------------------|
| $[(\blacksquare)^{2T} + \Gamma_1^+ + \Gamma_1^-, A_3 + A_4, M_3 + M_4, Z_1^- + Z_3^- + Z_5^-, R_1 + R_2, X_1 + X_2]$ |
| $[(\blacksquare)^{2T} + \Gamma_1^+ + \Gamma_1^-, A_3 + A_4, M_3 + M_4, Z_1^+ + Z_3^+ + Z_5^+, R_1 + R_2, X_1 + X_2]$ |
| $[(\blacksquare)^{2T} + \Gamma_1^+ + \Gamma_2^-, A_2 + A_3, M_2 + M_3, Z_2^- + Z_3^- + Z_5^-, R_1 + R_2, X_1 + X_2]$ |
| $[(\blacksquare)^{2T} + \Gamma_1^+ + \Gamma_2^-, A_1 + A_3, M_2 + M_3, Z_1^+ + Z_4^+ + Z_5^+, R_1 + R_2, X_1 + X_2]$ |
| $[(\blacksquare)^{2T} + \Gamma_1^+ + \Gamma_1^-, A_1 + A_2, M_1 + M_2, Z_1^- + Z_3^- + Z_5^-, R_1 + R_2, X_1 + X_2]$ |
| $[(\blacksquare)^{2T} + \Gamma_1^+ + \Gamma_1^-, A_1 + A_2, M_1 + M_2, Z_1^+ + Z_3^+ + Z_5^+, R_1 + R_2, X_1 + X_2]$ |
| $[(\blacksquare)^{2T} + \Gamma_4^+ + \Gamma_4^-, A_3 + A_4, M_3 + M_4, Z_2^- + Z_4^- + Z_5^-, R_1 + R_2, 2X_2]$      |

... continued on next page

... continued from previous page

---

|                                                                                                                 |
|-----------------------------------------------------------------------------------------------------------------|
| $[(\bullet)^{2T} + \Gamma_3^+ + \Gamma_4^-, A_1 + A_4, M_2 + M_4, Z_1^- + Z_4^- + Z_5^-, R_1 + R_2, 2X_2]$      |
| $[(\bullet)^{2T} + \Gamma_4^+ + \Gamma_4^-, A_3 + A_4, M_3 + M_4, Z_2^+ + Z_4^+ + Z_5^+, R_1 + R_2, 2X_2]$      |
| $[(\bullet)^{2T} + \Gamma_1^- + \Gamma_2^+, A_2 + A_4, M_2 + M_4, Z_2^+ + Z_3^+ + Z_5^+, R_1 + R_2, X_1 + X_2]$ |
| $[(\bullet)^{2T} + \Gamma_3^- + \Gamma_4^+, A_2 + A_3, M_2 + M_3, Z_2^- + Z_3^- + Z_5^-, R_1 + R_2, 2X_2]$      |
| $[(\bullet)^{2T} + \Gamma_3^- + \Gamma_4^+, A_1 + A_3, M_2 + M_3, Z_1^+ + Z_4^+ + Z_5^+, R_1 + R_2, 2X_2]$      |
| $[(\bullet)^{2T} + \Gamma_4^+ + \Gamma_4^-, A_1 + A_2, M_1 + M_2, Z_2^- + Z_4^- + Z_5^-, R_1 + R_2, 2X_2]$      |
| $[(\bullet)^{2T} + \Gamma_4^+ + \Gamma_4^-, A_1 + A_2, M_1 + M_2, Z_2^+ + Z_4^+ + Z_5^+, R_1 + R_2, 2X_2]$      |
| $[(\bullet)^{2T} + \Gamma_3^+ + \Gamma_3^-, A_1 + A_2, 2M_2, Z_1^- + Z_3^- + Z_5^-, R_1 + R_2, 2X_2]$           |
| $[(\bullet)^{2T} + \Gamma_3^+ + \Gamma_4^-, A_2 + A_4, M_2 + M_4, Z_2^+ + Z_3^+ + Z_5^+, R_1 + R_2, 2X_2]$      |
| $[(\bullet)^{2T} + \Gamma_2^+ + \Gamma_2^-, A_1 + A_2, 2M_2, Z_2^+ + Z_4^+ + Z_5^+, R_1 + R_2, X_1 + X_2]$      |
| $[(\bullet)^{2T} + \Gamma_1^- + \Gamma_2^+, A_1 + A_4, M_2 + M_4, Z_1^- + Z_4^- + Z_5^-, R_1 + R_2, X_1 + X_2]$ |
| $[(\bullet)^{2T} + \Gamma_3^+ + \Gamma_3^-, A_1 + A_2, 2M_2, Z_1^+ + Z_3^+ + Z_5^+, R_1 + R_2, 2X_2]$           |
| $[(\bullet)^{2T} + \Gamma_2^+ + \Gamma_2^-, A_1 + A_2, 2M_2, Z_2^- + Z_4^- + Z_5^-, R_1 + R_2, X_1 + X_2]$      |

---

2nd minimal solution:  $\mu_2^T = 6$  (308 symmetry vectors)

Space group 126 ( $\mathbb{Z}_1$ )

1st minimal solution:  $\mu_1^T = 6$  (24 symmetry vectors)

---

| $n^T$                                                                                                                             |
|-----------------------------------------------------------------------------------------------------------------------------------|
| $[(\bullet)^{2T} + \Gamma_1^+ + \Gamma_3^+ + \Gamma_5^+, A_2 + A_3 + A_4, M_2 + M_3 + M_4, Z_2 + Z_3Z_4, R_1 + 2R_2, X_1 + 2X_2]$ |
| $[(\bullet)^{2T} + \Gamma_1^+ + \Gamma_3^+ + \Gamma_5^+, A_1 + A_3 + A_4, M_2 + M_3 + M_4, Z_2 + Z_3Z_4, 2R_1 + R_2, X_1 + 2X_2]$ |
| $[(\bullet)^{2T} + \Gamma_2^+ + \Gamma_4^+ + \Gamma_5^+, A_2 + A_3 + A_4, M_2 + M_3 + M_4, Z_1 + Z_3Z_4, R_1 + 2R_2, X_1 + 2X_2]$ |
| $[(\bullet)^{2T} + \Gamma_2^+ + \Gamma_4^+ + \Gamma_5^+, A_1 + A_3 + A_4, M_2 + M_3 + M_4, Z_1 + Z_3Z_4, 2R_1 + R_2, X_1 + 2X_2]$ |
| $[(\bullet)^{2T} + \Gamma_1^+ + \Gamma_3^+ + \Gamma_5^+, 3A_2, M_1 + 2M_2, Z_2 + Z_3Z_4, 3R_2, X_1 + 2X_2]$                       |
| $[(\bullet)^{2T} + \Gamma_1^+ + \Gamma_3^+ + \Gamma_5^+, A_1 + 2A_2, M_1 + 2M_2, Z_2 + Z_3Z_4, R_1 + 2R_2, X_1 + 2X_2]$           |
| $[(\bullet)^{2T} + \Gamma_1^+ + \Gamma_3^+ + \Gamma_5^+, 2A_1 + A_2, M_1 + 2M_2, Z_2 + Z_3Z_4, 2R_1 + R_2, X_1 + 2X_2]$           |
| $[(\bullet)^{2T} + \Gamma_1^+ + \Gamma_3^+ + \Gamma_5^+, 3A_1, M_1 + 2M_2, Z_2 + Z_3Z_4, 3R_1, X_1 + 2X_2]$                       |
| $[(\bullet)^{2T} + \Gamma_2^- + \Gamma_4^- + \Gamma_5^-, A_2 + A_3 + A_4, M_2 + M_3 + M_4, Z_1 + Z_3Z_4, R_1 + 2R_2, X_1 + 2X_2]$ |
| $[(\bullet)^{2T} + \Gamma_2^- + \Gamma_4^- + \Gamma_5^-, A_2 + A_3 + A_4, M_2 + M_3 + M_4, Z_2 + Z_3Z_4, R_1 + 2R_2, X_1 + 2X_2]$ |
| $[(\bullet)^{2T} + \Gamma_2^- + \Gamma_4^- + \Gamma_5^-, 3A_2, M_1 + 2M_2, Z_1 + Z_3Z_4, 3R_2, X_1 + 2X_2]$                       |
| $[(\bullet)^{2T} + \Gamma_2^- + \Gamma_4^- + \Gamma_5^-, A_1 + 2A_2, M_1 + 2M_2, Z_1 + Z_3Z_4, R_1 + 2R_2, X_1 + 2X_2]$           |
| $[(\bullet)^{2T} + \Gamma_2^- + \Gamma_4^- + \Gamma_5^-, 2A_1 + A_2, M_1 + 2M_2, Z_1 + Z_3Z_4, 2R_1 + R_2, X_1 + 2X_2]$           |
| $[(\bullet)^{2T} + \Gamma_2^- + \Gamma_4^- + \Gamma_5^-, 3A_2, M_1 + 2M_2, Z_1 + Z_3Z_4, 3R_2, X_1 + 2X_2]$                       |
| $[(\bullet)^{2T} + \Gamma_1^- + \Gamma_3^- + \Gamma_5^-, 3A_2, M_1 + 2M_2, Z_2 + Z_3Z_4, 3R_2, X_1 + 2X_2]$                       |
| $[(\bullet)^{2T} + \Gamma_2^- + \Gamma_4^- + \Gamma_5^-, A_1 + A_3 + A_4, M_2 + M_3 + M_4, Z_1 + Z_3Z_4, 2R_1 + R_2, X_1 + 2X_2]$ |
| $[(\bullet)^{2T} + \Gamma_1^- + \Gamma_3^- + \Gamma_5^-, A_1 + A_3 + A_4, M_2 + M_3 + M_4, Z_2 + Z_3Z_4, 2R_1 + R_2, X_1 + 2X_2]$ |
| $[(\bullet)^{2T} + \Gamma_2^- + \Gamma_4^- + \Gamma_5^-, 3A_1, M_1 + 2M_2, Z_1 + Z_3Z_4, 3R_1, X_1 + 2X_2]$                       |
| $[(\bullet)^{2T} + \Gamma_2^- + \Gamma_4^- + \Gamma_5^-, A_1 + 2A_2, M_1 + 2M_2, Z_1 + Z_3Z_4, R_1 + 2R_2, X_1 + 2X_2]$           |
| $[(\bullet)^{2T} + \Gamma_1^- + \Gamma_3^- + \Gamma_5^-, A_1 + 2A_2, M_1 + 2M_2, Z_2 + Z_3Z_4, R_1 + 2R_2, X_1 + 2X_2]$           |
| $[(\bullet)^{2T} + \Gamma_2^- + \Gamma_4^- + \Gamma_5^-, 2A_1 + A_2, M_1 + 2M_2, Z_1 + Z_3Z_4, 2R_1 + R_2, X_1 + 2X_2]$           |
| $[(\bullet)^{2T} + \Gamma_1^- + \Gamma_3^- + \Gamma_5^-, 2A_1 + A_2, M_1 + 2M_2, Z_2 + Z_3Z_4, 2R_1 + R_2, X_1 + 2X_2]$           |
| $[(\bullet)^{2T} + \Gamma_2^- + \Gamma_4^- + \Gamma_5^-, 3A_1, M_1 + 2M_2, Z_1 + Z_3Z_4, 3R_1, X_1 + 2X_2]$                       |
| $[(\bullet)^{2T} + \Gamma_1^- + \Gamma_3^- + \Gamma_5^-, 3A_1, M_1 + 2M_2, Z_2 + Z_3Z_4, 3R_1, X_1 + 2X_2]$                       |

---

2nd minimal solution:  $\mu_2^T = 8$  (136 symmetry vectors)

Space group 127 ( $\mathbb{Z}_1$ )

1st minimal solution:  $\mu_1^T = 4$  (14 symmetry vectors)

| $\mathbf{n}^T$                                                                                                                             |
|--------------------------------------------------------------------------------------------------------------------------------------------|
| $[(\bullet)^{2T} + \Gamma_1^+ + \Gamma_2^-, A_2^- A_3^- + A_5^-, M_1^+ M_4^+ + M_5^+, Z_1^+ + Z_4^+ + Z_5^+, R_1 + R_2, X_1 + X_2]$        |
| $[(\bullet)^{2T} + \Gamma_1^+ + \Gamma_2^-, A_1^+ A_4^+ + A_5^-, M_1^+ M_4^+ + M_5^+, Z_2^- + Z_3^- + Z_5^+, 2R_1, X_1 + X_2]$             |
| $[(\bullet)^{2T} + \Gamma_1^+ + \Gamma_1^-, 2A_5^+, M_5^+ + M_5^-, Z_1^- + Z_3^- + Z_5^+, 2R_1, X_1 + X_2]$                                |
| $[(\bullet)^{2T} + \Gamma_1^+ + \Gamma_1^-, A_5^+ + A_5^-, M_5^+ + M_5^-, Z_1^+ + Z_3^+ + Z_5^+, R_1 + R_2, X_1 + X_2]$                    |
| $[(\bullet)^{2T} + \Gamma_1^+ + \Gamma_2^-, A_2^- A_3^- + A_5^+, M_1^+ M_4^+ + M_5^+, Z_1^+ + Z_4^+ + Z_5^-, 2R_2, X_1 + X_2]$             |
| $[(\bullet)^{2T} + \Gamma_1^+ + \Gamma_2^-, A_1^+ A_4^+ + A_5^+, M_1^+ M_4^+ + M_5^+, Z_2^- + Z_3^- + Z_5^-, R_1 + R_2, X_1 + X_2]$        |
| $[(\bullet)^{2T} + \Gamma_1^+ + \Gamma_1^-, A_5^+ + A_5^-, M_5^+ + M_5^-, Z_1^- + Z_3^- + Z_5^-, R_1 + R_2, X_1 + X_2]$                    |
| $[(\bullet)^{2T} + \Gamma_1^+ + \Gamma_1^-, 2A_5^+, M_5^+ + M_5^-, Z_1^+ + Z_3^+ + Z_5^-, 2R_2, X_1 + X_2]$                                |
| $[(\bullet)^{2T} + \Gamma_2^+ + \Gamma_2^-, A_1^- A_4^- + A_2^- A_3^-, M_1^+ M_4^+ + M_1^- M_4^-, Z_2^+ + Z_4^+ + Z_5^-, 2R_2, X_1 + X_2]$ |
| $[(\bullet)^{2T} + \Gamma_2^+ + \Gamma_2^-, A_1^+ A_4^+ + A_2^+ A_3^+, M_1^+ M_4^+ + M_1^- M_4^-, Z_2^- + Z_4^- + Z_5^+, 2R_1, X_1 + X_2]$ |
| $[(\bullet)^{2T} + \Gamma_1^- + \Gamma_2^+, A_1^- A_4^- + A_5^-, M_1^- M_4^- + M_5^-, Z_2^+ + Z_3^+ + Z_5^-, 2R_2, X_1 + X_2]$             |
| $[(\bullet)^{2T} + \Gamma_1^- + \Gamma_2^+, A_2^+ A_3^+ + A_5^-, M_1^- M_4^- + M_5^-, Z_1^- + Z_4^- + Z_5^+, 2R_1, X_1 + X_2]$             |
| $[(\bullet)^{2T} + \Gamma_1^- + \Gamma_2^+, A_2^+ A_3^+ + A_5^-, M_1^- M_4^- + M_5^-, Z_1^- + Z_4^- + Z_5^-, R_1 + R_2, X_1 + X_2]$        |
| $[(\bullet)^{2T} + \Gamma_1^- + \Gamma_2^+, A_1^- A_4^- + A_5^-, M_1^- M_4^- + M_5^-, Z_2^+ + Z_3^+ + Z_5^+, R_1 + R_2, X_1 + X_2]$        |

2nd minimal solution:  $\mu_2^T = 6$  (296 symmetry vectors)

Space group 128 ( $\mathbb{Z}_2$ )

1st minimal solution:  $\mu_1^T = 6$  (64 symmetry vectors)

| $\mathbf{n}^T$                                                                                                                                         | $\mathbf{v}^T \in \mathbb{Z}_2$ |
|--------------------------------------------------------------------------------------------------------------------------------------------------------|---------------------------------|
| $[(\bullet)^{2T} + \Gamma_1^+ + \Gamma_1^- + \Gamma_5^-, A_2 + A_3 A_4, M_1^- M_4^- + M_2^- M_3^- + M_5^-, Z_2 + Z_3 Z_4, 3R_1^+, X_1 + 2X_2]$         | 1                               |
| $[(\bullet)^{2T} + \Gamma_1^+ + \Gamma_1^- + \Gamma_5^-, A_2 + A_3 A_4, M_1^- M_4^- + M_2^- M_3^- + M_5^-, Z_2 + Z_3 Z_4, 2R_1^+ + R_1^-, X_1 + 2X_2]$ | trivial                         |
| $[(\bullet)^{2T} + \Gamma_1^+ + \Gamma_1^- + \Gamma_5^-, A_1 + A_3 A_4, M_1^- M_4^- + M_2^- M_3^- + M_5^-, Z_2 + Z_3 Z_4, 3R_1^+, X_1 + 2X_2]$         | trivial                         |
| $[(\bullet)^{2T} + \Gamma_1^+ + \Gamma_1^- + \Gamma_5^-, A_1 + A_3 A_4, M_1^- M_4^- + M_2^- M_3^- + M_5^-, Z_2 + Z_3 Z_4, 2R_1^+ + R_1^-, X_1 + 2X_2]$ | 1                               |
| $[(\bullet)^{2T} + \Gamma_1^+ + \Gamma_1^- + \Gamma_5^-, A_2 + A_3 A_4, M_1^- M_4^- + M_2^- M_3^- + M_5^-, Z_2 + Z_3 Z_4, R_1^+ + 2R_1^-, X_1 + 2X_2]$ | 1                               |
| $[(\bullet)^{2T} + \Gamma_1^+ + \Gamma_1^- + \Gamma_5^-, A_1 + A_3 A_4, M_1^- M_4^- + M_2^- M_3^- + M_5^-, Z_2 + Z_3 Z_4, R_1^+ + 2R_1^-, X_1 + 2X_2]$ | trivial                         |
| $[(\bullet)^{2T} + \Gamma_1^+ + \Gamma_1^- + \Gamma_5^-, A_2 + A_3 A_4, M_1^- M_4^- + M_2^- M_3^- + M_5^-, Z_2 + Z_3 Z_4, 3R_1^-, X_1 + 2X_2]$         | trivial                         |
| $[(\bullet)^{2T} + \Gamma_1^+ + \Gamma_1^- + \Gamma_5^-, A_1 + A_3 A_4, M_1^- M_4^- + M_2^- M_3^- + M_5^-, Z_2 + Z_3 Z_4, 3R_1^-, X_1 + 2X_2]$         | 1                               |
| $[(\bullet)^{2T} + \Gamma_2^+ + \Gamma_2^- + \Gamma_5^+, A_2 + A_3 A_4, M_1^+ M_4^+ + M_1^- M_4^- + M_5^-, Z_1 + Z_3 Z_4, 3R_1^+, 2X_1 + X_2]$         | trivial                         |
| $[(\bullet)^{2T} + \Gamma_2^+ + \Gamma_2^- + \Gamma_5^+, A_2 + A_3 A_4, M_1^+ M_4^+ + M_1^- M_4^- + M_5^-, Z_1 + Z_3 Z_4, 3R_1^+, X_1 + 2X_2]$         | trivial                         |
| $[(\bullet)^{2T} + \Gamma_2^+ + \Gamma_2^- + \Gamma_5^+, A_2 + A_3 A_4, M_1^+ M_4^+ + M_1^- M_4^- + M_5^-, Z_1 + Z_3 Z_4, 2R_1^+ + R_1^-, 2X_1 + X_2]$ | 1                               |
| $[(\bullet)^{2T} + \Gamma_2^+ + \Gamma_2^- + \Gamma_5^+, A_2 + A_3 A_4, M_1^+ M_4^+ + M_1^- M_4^- + M_5^-, Z_1 + Z_3 Z_4, 2R_1^+ + R_1^-, X_1 + 2X_2]$ | 1                               |
| $[(\bullet)^{2T} + \Gamma_2^+ + \Gamma_2^- + \Gamma_5^+, A_2 + A_3 A_4, M_1^+ M_4^+ + M_1^- M_4^- + M_5^-, Z_1 + Z_3 Z_4, R_1^+ + 2R_1^-, 2X_1 + X_2]$ | trivial                         |
| $[(\bullet)^{2T} + \Gamma_2^+ + \Gamma_2^- + \Gamma_5^+, A_2 + A_3 A_4, M_1^+ M_4^+ + M_1^- M_4^- + M_5^-, Z_1 + Z_3 Z_4, R_1^+ + 2R_1^-, X_1 + 2X_2]$ | trivial                         |
| $[(\bullet)^{2T} + \Gamma_2^+ + \Gamma_2^- + \Gamma_5^+, A_1 + A_3 A_4, M_1^+ M_4^+ + M_1^- M_4^- + M_5^-, Z_1 + Z_3 Z_4, 3R_1^+, 2X_1 + X_2]$         | 1                               |
| $[(\bullet)^{2T} + \Gamma_2^+ + \Gamma_2^- + \Gamma_5^+, A_1 + A_3 A_4, M_1^+ M_4^+ + M_1^- M_4^- + M_5^-, Z_1 + Z_3 Z_4, 3R_1^+, X_1 + 2X_2]$         | 1                               |
| $[(\bullet)^{2T} + \Gamma_2^+ + \Gamma_2^- + \Gamma_5^+, A_1 + A_3 A_4, M_1^+ M_4^+ + M_1^- M_4^- + M_5^-, Z_1 + Z_3 Z_4, 2R_1^+ + R_1^-, 2X_1 + X_2]$ | trivial                         |
| $[(\bullet)^{2T} + \Gamma_2^+ + \Gamma_2^- + \Gamma_5^+, A_1 + A_3 A_4, M_1^+ M_4^+ + M_1^- M_4^- + M_5^-, Z_1 + Z_3 Z_4, 2R_1^+ + R_1^-, X_1 + 2X_2]$ | trivial                         |
| $[(\bullet)^{2T} + \Gamma_2^+ + \Gamma_2^- + \Gamma_5^+, A_1 + A_3 A_4, M_1^+ M_4^+ + M_1^- M_4^- + M_5^-, Z_1 + Z_3 Z_4, R_1^+ + 2R_1^-, 2X_1 + X_2]$ | 1                               |
| $[(\bullet)^{2T} + \Gamma_2^+ + \Gamma_2^- + \Gamma_5^+, A_1 + A_3 A_4, M_1^+ M_4^+ + M_1^- M_4^- + M_5^-, Z_1 + Z_3 Z_4, R_1^+ + 2R_1^-, X_1 + 2X_2]$ | 1                               |
| $[(\bullet)^{2T} + \Gamma_2^+ + \Gamma_2^- + \Gamma_5^+, A_2 + A_3 A_4, M_1^+ M_4^+ + M_1^- M_4^- + M_5^-, Z_1 + Z_3 Z_4, 3R_1^-, 2X_1 + X_2]$         | 1                               |
| $[(\bullet)^{2T} + \Gamma_2^+ + \Gamma_2^- + \Gamma_5^+, A_2 + A_3 A_4, M_1^+ M_4^+ + M_1^- M_4^- + M_5^-, Z_1 + Z_3 Z_4, 3R_1^-, X_1 + 2X_2]$         | 1                               |
| $[(\bullet)^{2T} + \Gamma_2^+ + \Gamma_2^- + \Gamma_5^+, A_1 + A_3 A_4, M_1^+ M_4^+ + M_1^- M_4^- + M_5^-, Z_1 + Z_3 Z_4, 3R_1^-, 2X_1 + X_2]$         | trivial                         |
| $[(\bullet)^{2T} + \Gamma_2^+ + \Gamma_2^- + \Gamma_5^+, A_1 + A_3 A_4, M_1^+ M_4^+ + M_1^- M_4^- + M_5^-, Z_1 + Z_3 Z_4, 3R_1^-, X_1 + 2X_2]$         | trivial                         |

... continued on next page

... continued from previous page

|                                                                                                                                                    |         |
|----------------------------------------------------------------------------------------------------------------------------------------------------|---------|
| $[(\bullet)^{2T} + \Gamma_1^+ + \Gamma_1^- + \Gamma_5^+, 3A_2, M_5^+ + 2M_5^-, Z_2 + Z_3Z_4, 3R_1^+, 2X_1 + X_2]$                                  | 1       |
| $[(\bullet)^{2T} + \Gamma_1^+ + \Gamma_1^- + \Gamma_5^-, 3A_2, 2M_5^+ + M_5^-, Z_2 + Z_3Z_4, 3R_1^+, X_1 + 2X_2]$                                  | 1       |
| $[(\bullet)^{2T} + \Gamma_1^+ + \Gamma_1^- + \Gamma_5^+, 3A_2, M_5^+ + 2M_5^-, Z_2 + Z_3Z_4, 2R_1^+ + R_1^-, 2X_1 + X_2]$                          | trivial |
| $[(\bullet)^{2T} + \Gamma_1^+ + \Gamma_1^- + \Gamma_5^-, 3A_2, 2M_5^+ + M_5^-, Z_2 + Z_3Z_4, 2R_1^+ + R_1^-, X_1 + 2X_2]$                          | trivial |
| $[(\bullet)^{2T} + \Gamma_1^+ + \Gamma_1^- + \Gamma_5^+, 3A_2, M_5^+ + 2M_5^-, Z_2 + Z_3Z_4, R_1^+ + 2R_1^-, 2X_1 + X_2]$                          | 1       |
| $[(\bullet)^{2T} + \Gamma_1^+ + \Gamma_1^- + \Gamma_5^-, 3A_2, 2M_5^+ + M_5^-, Z_2 + Z_3Z_4, R_1^+ + 2R_1^-, X_1 + 2X_2]$                          | 1       |
| $[(\bullet)^{2T} + \Gamma_1^+ + \Gamma_1^- + \Gamma_5^+, A_1 + 2A_2, M_5^+ + 2M_5^-, Z_2 + Z_3Z_4, 3R_1^+, 2X_1 + X_2]$                            | trivial |
| $[(\bullet)^{2T} + \Gamma_1^+ + \Gamma_1^- + \Gamma_5^-, A_1 + 2A_2, 2M_5^+ + M_5^-, Z_2 + Z_3Z_4, 3R_1^+, X_1 + 2X_2]$                            | trivial |
| $[(\bullet)^{2T} + \Gamma_1^+ + \Gamma_1^- + \Gamma_5^+, A_1 + 2A_2, M_5^+ + 2M_5^-, Z_2 + Z_3Z_4, 2R_1^+ + R_1^-, 2X_1 + X_2]$                    | 1       |
| $[(\bullet)^{2T} + \Gamma_1^+ + \Gamma_1^- + \Gamma_5^-, A_1 + 2A_2, 2M_5^+ + M_5^-, Z_2 + Z_3Z_4, 2R_1^+ + R_1^-, X_1 + 2X_2]$                    | 1       |
| $[(\bullet)^{2T} + \Gamma_1^+ + \Gamma_1^- + \Gamma_5^+, A_1 + 2A_2, M_5^+ + 2M_5^-, Z_2 + Z_3Z_4, R_1^+ + 2R_1^-, 2X_1 + X_2]$                    | trivial |
| $[(\bullet)^{2T} + \Gamma_1^+ + \Gamma_1^- + \Gamma_5^-, A_1 + 2A_2, 2M_5^+ + M_5^-, Z_2 + Z_3Z_4, R_1^+ + 2R_1^-, X_1 + 2X_2]$                    | trivial |
| $[(\bullet)^{2T} + \Gamma_1^+ + \Gamma_1^- + \Gamma_5^+, 2A_1 + A_2, M_5^+ + 2M_5^-, Z_2 + Z_3Z_4, 3R_1^+, 2X_1 + X_2]$                            | 1       |
| $[(\bullet)^{2T} + \Gamma_1^+ + \Gamma_1^- + \Gamma_5^-, 2A_1 + A_2, 2M_5^+ + M_5^-, Z_2 + Z_3Z_4, 3R_1^+, X_1 + 2X_2]$                            | 1       |
| $[(\bullet)^{2T} + \Gamma_1^+ + \Gamma_1^- + \Gamma_5^+, 2A_1 + A_2, M_5^+ + 2M_5^-, Z_2 + Z_3Z_4, 2R_1^+ + R_1^-, 2X_1 + X_2]$                    | trivial |
| $[(\bullet)^{2T} + \Gamma_1^+ + \Gamma_1^- + \Gamma_5^-, 2A_1 + A_2, 2M_5^+ + M_5^-, Z_2 + Z_3Z_4, 2R_1^+ + R_1^-, X_1 + 2X_2]$                    | trivial |
| $[(\bullet)^{2T} + \Gamma_1^+ + \Gamma_1^- + \Gamma_5^+, 2A_1 + A_2, M_5^+ + 2M_5^-, Z_2 + Z_3Z_4, R_1^+ + 2R_1^-, 2X_1 + X_2]$                    | 1       |
| $[(\bullet)^{2T} + \Gamma_1^+ + \Gamma_1^- + \Gamma_5^-, 2A_1 + A_2, 2M_5^+ + M_5^-, Z_2 + Z_3Z_4, R_1^+ + 2R_1^-, X_1 + 2X_2]$                    | 1       |
| $[(\bullet)^{2T} + \Gamma_1^+ + \Gamma_1^- + \Gamma_5^+, 3A_2, M_5^+ + 2M_5^-, Z_2 + Z_3Z_4, 3R_1^-, 2X_1 + X_2]$                                  | trivial |
| $[(\bullet)^{2T} + \Gamma_1^+ + \Gamma_1^- + \Gamma_5^-, 3A_2, 2M_5^+ + M_5^-, Z_2 + Z_3Z_4, 3R_1^-, X_1 + 2X_2]$                                  | trivial |
| $[(\bullet)^{2T} + \Gamma_1^+ + \Gamma_1^- + \Gamma_5^+, A_1 + 2A_2, M_5^+ + 2M_5^-, Z_2 + Z_3Z_4, 3R_1^-, 2X_1 + X_2]$                            | 1       |
| $[(\bullet)^{2T} + \Gamma_1^+ + \Gamma_1^- + \Gamma_5^-, A_1 + 2A_2, 2M_5^+ + M_5^-, Z_2 + Z_3Z_4, 3R_1^-, X_1 + 2X_2]$                            | 1       |
| $[(\bullet)^{2T} + \Gamma_1^+ + \Gamma_1^- + \Gamma_5^+, 2A_1 + A_2, M_5^+ + 2M_5^-, Z_2 + Z_3Z_4, 3R_1^-, 2X_1 + X_2]$                            | trivial |
| $[(\bullet)^{2T} + \Gamma_1^+ + \Gamma_1^- + \Gamma_5^-, 2A_1 + A_2, 2M_5^+ + M_5^-, Z_2 + Z_3Z_4, 3R_1^-, X_1 + 2X_2]$                            | trivial |
| $[(\bullet)^{2T} + \Gamma_1^+ + \Gamma_1^- + \Gamma_5^+, 3A_1, M_5^+ + 2M_5^-, Z_2 + Z_3Z_4, 3R_1^+, 2X_1 + X_2]$                                  | trivial |
| $[(\bullet)^{2T} + \Gamma_1^+ + \Gamma_1^- + \Gamma_5^-, 3A_1, 2M_5^+ + M_5^-, Z_2 + Z_3Z_4, 3R_1^+, X_1 + 2X_2]$                                  | trivial |
| $[(\bullet)^{2T} + \Gamma_1^+ + \Gamma_1^- + \Gamma_5^+, 3A_1, M_5^+ + 2M_5^-, Z_2 + Z_3Z_4, 2R_1^+ + R_1^-, 2X_1 + X_2]$                          | 1       |
| $[(\bullet)^{2T} + \Gamma_1^+ + \Gamma_1^- + \Gamma_5^-, 3A_1, 2M_5^+ + M_5^-, Z_2 + Z_3Z_4, 2R_1^+ + R_1^-, X_1 + 2X_2]$                          | 1       |
| $[(\bullet)^{2T} + \Gamma_1^+ + \Gamma_1^- + \Gamma_5^+, 3A_1, M_5^+ + 2M_5^-, Z_2 + Z_3Z_4, R_1^+ + 2R_1^-, 2X_1 + X_2]$                          | trivial |
| $[(\bullet)^{2T} + \Gamma_1^+ + \Gamma_1^- + \Gamma_5^-, 3A_1, 2M_5^+ + M_5^-, Z_2 + Z_3Z_4, R_1^+ + 2R_1^-, X_1 + 2X_2]$                          | trivial |
| $[(\bullet)^{2T} + \Gamma_1^+ + \Gamma_1^- + \Gamma_5^+, 3A_1, M_5^+ + 2M_5^-, Z_2 + Z_3Z_4, 3R_1^-, 2X_1 + X_2]$                                  | 1       |
| $[(\bullet)^{2T} + \Gamma_1^+ + \Gamma_1^- + \Gamma_5^-, 3A_1, 2M_5^+ + M_5^-, Z_2 + Z_3Z_4, 3R_1^-, X_1 + 2X_2]$                                  | 1       |
| $[(\bullet)^{2T} + \Gamma_1^+ + \Gamma_1^- + \Gamma_5^+, A_2 + A_3A_4, M_1^+M_4^+ + M_2^+M_3^+ + M_5^+, Z_2 + Z_3Z_4, 3R_1^+, 2X_1 + X_2]$         | 1       |
| $[(\bullet)^{2T} + \Gamma_1^+ + \Gamma_1^- + \Gamma_5^-, A_2 + A_3A_4, M_1^+M_4^+ + M_2^+M_3^+ + M_5^+, Z_2 + Z_3Z_4, 2R_1^+ + R_1^-, 2X_1 + X_2]$ | trivial |
| $[(\bullet)^{2T} + \Gamma_1^+ + \Gamma_1^- + \Gamma_5^+, A_1 + A_3A_4, M_1^+M_4^+ + M_2^+M_3^+ + M_5^+, Z_2 + Z_3Z_4, 3R_1^+, 2X_1 + X_2]$         | trivial |
| $[(\bullet)^{2T} + \Gamma_1^+ + \Gamma_1^- + \Gamma_5^-, A_1 + A_3A_4, M_1^+M_4^+ + M_2^+M_3^+ + M_5^+, Z_2 + Z_3Z_4, 2R_1^+ + R_1^-, 2X_1 + X_2]$ | 1       |
| $[(\bullet)^{2T} + \Gamma_1^+ + \Gamma_1^- + \Gamma_5^+, A_2 + A_3A_4, M_1^+M_4^+ + M_2^+M_3^+ + M_5^+, Z_2 + Z_3Z_4, R_1^+ + 2R_1^-, 2X_1 + X_2]$ | 1       |
| $[(\bullet)^{2T} + \Gamma_1^+ + \Gamma_1^- + \Gamma_5^-, A_1 + A_3A_4, M_1^+M_4^+ + M_2^+M_3^+ + M_5^+, Z_2 + Z_3Z_4, R_1^+ + 2R_1^-, 2X_1 + X_2]$ | trivial |
| $[(\bullet)^{2T} + \Gamma_1^+ + \Gamma_1^- + \Gamma_5^+, A_2 + A_3A_4, M_1^+M_4^+ + M_2^+M_3^+ + M_5^+, Z_2 + Z_3Z_4, 3R_1^-, 2X_1 + X_2]$         | trivial |
| $[(\bullet)^{2T} + \Gamma_1^+ + \Gamma_1^- + \Gamma_5^-, A_1 + A_3A_4, M_1^+M_4^+ + M_2^+M_3^+ + M_5^+, Z_2 + Z_3Z_4, 3R_1^-, 2X_1 + X_2]$         | 1       |

2nd minimal solution:  $\mu_2^T = 8$  (540 symmetry vectors)

Space group 129 ( $Z_1$ )

1st minimal solution:  $\mu_1^T = 4$  (10 symmetry vectors)

| $n^T$                                                                                                           |
|-----------------------------------------------------------------------------------------------------------------|
| $[(\bullet)^{2T} + \Gamma_1^- + \Gamma_2^+, A_1 + A_4, M_1 + M_4, Z_2^+ + Z_3^+ + Z_5^+, R_1 + R_2, X_1 + X_2]$ |
| $[(\bullet)^{2T} + \Gamma_1^+ + \Gamma_1^-, A_3 + A_4, M_3 + M_4, Z_1^+ + Z_3^+ + Z_5^+, R_1 + R_2, X_1 + X_2]$ |
| $[(\bullet)^{2T} + \Gamma_1^- + \Gamma_2^+, A_2 + A_4, M_1 + M_4, Z_1^- + Z_4^- + Z_5^-, R_1 + R_2, X_1 + X_2]$ |

... continued on next page

... continued from previous page

---

|                                                                                                                      |
|----------------------------------------------------------------------------------------------------------------------|
| $[(\blacksquare)^{2T} + \Gamma_1^+ + \Gamma_1^-, A_3 + A_4, M_3 + M_4, Z_1^- + Z_3^- + Z_5^-, R_1 + R_2, X_1 + X_2]$ |
| $[(\blacksquare)^{2T} + \Gamma_2^+ + \Gamma_2^-, A_1 + A_2, 2M_1, Z_2^- + Z_4^- + Z_5^-, R_1 + R_2, X_1 + X_2]$      |
| $[(\blacksquare)^{2T} + \Gamma_1^+ + \Gamma_2^-, A_1 + A_3, M_1 + M_3, Z_2^- + Z_3^- + Z_5^-, R_1 + R_2, X_1 + X_2]$ |
| $[(\blacksquare)^{2T} + \Gamma_2^+ + \Gamma_2^-, A_1 + A_2, 2M_1, Z_2^+ + Z_4^+ + Z_5^+, R_1 + R_2, X_1 + X_2]$      |
| $[(\blacksquare)^{2T} + \Gamma_1^+ + \Gamma_1^-, A_1 + A_2, M_1 + M_2, Z_1^+ + Z_3^+ + Z_5^+, R_1 + R_2, X_1 + X_2]$ |
| $[(\blacksquare)^{2T} + \Gamma_1^+ + \Gamma_1^-, A_1 + A_2, M_1 + M_2, Z_1^- + Z_3^- + Z_5^-, R_1 + R_2, X_1 + X_2]$ |
| $[(\blacksquare)^{2T} + \Gamma_1^+ + \Gamma_2^-, A_2 + A_3, M_1 + M_3, Z_1^+ + Z_4^+ + Z_5^+, R_1 + R_2, X_1 + X_2]$ |

---

2nd minimal solution:  $\mu_2^T = 6$  (130 symmetry vectors)

Space group 130 ( $\mathbb{Z}_2$ )

1st minimal solution:  $\mu_1^T = 8$  (20 symmetry vectors)

| $\mathbf{n}^T$                                                                                                                                                             | $\mathbf{v}^T \in \mathbb{Z}_2$ |
|----------------------------------------------------------------------------------------------------------------------------------------------------------------------------|---------------------------------|
| $[(\blacksquare)^{2T} + 2\Gamma_1^+ + \Gamma_1^- + \Gamma_3^+ + \Gamma_5^-, 2A_3A_4, 2M_3 + 2M_4, 2Z_2 + Z_3Z_4, 2R_1R_2, 2X_1 + 2X_2]$                                    | trivial                         |
| $[(\blacksquare)^{2T} + 2\Gamma_1^+ + \Gamma_1^- + \Gamma_3^+ + \Gamma_5^-, A_1A_2 + A_3A_4, M_1 + M_2 + M_3 + M_4, 2Z_2 + Z_3Z_4, 2R_1R_2, 2X_1 + 2X_2]$                  | 1                               |
| $[(\blacksquare)^{2T} + \Gamma_1^+ + 2\Gamma_1^- + \Gamma_3^- + \Gamma_5^-, 2A_3A_4, 2M_3 + 2M_4, 2Z_2 + Z_3Z_4, 2R_1R_2, 2X_1 + 2X_2]$                                    | trivial                         |
| $[(\blacksquare)^{2T} + \Gamma_1^+ + \Gamma_1^- + \Gamma_2^- + \Gamma_4^- + \Gamma_5^-, 2A_3A_4, 2M_3 + 2M_4, Z_1 + Z_2 + Z_3Z_4, 2R_1R_2, 2X_1 + 2X_2]$                   | 1                               |
| $[(\blacksquare)^{2T} + \Gamma_1^+ + \Gamma_1^- + \Gamma_2^+ + \Gamma_4^+ + \Gamma_5^+, 2A_3A_4, 2M_3 + 2M_4, Z_1 + Z_2 + Z_3Z_4, 2R_1R_2, 2X_1 + 2X_2]$                   | 1                               |
| $[(\blacksquare)^{2T} + \Gamma_1^+ + \Gamma_1^- + \Gamma_2^+ + \Gamma_4^+ + \Gamma_5^+, A_1A_2 + A_3A_4, M_1 + M_2 + M_3 + M_4, Z_1 + Z_2 + Z_3Z_4, 2R_1R_2, 2X_1 + 2X_2]$ | trivial                         |
| $[(\blacksquare)^{2T} + \Gamma_1^+ + \Gamma_2^+ + \Gamma_2^- + \Gamma_3^+ + \Gamma_5^+, A_1A_2 + A_3A_4, 2M_1 + M_3 + M_4, Z_1 + Z_2 + Z_3Z_4, 2R_1R_2, 2X_1 + 2X_2]$      | trivial                         |
| $[(\blacksquare)^{2T} + 2\Gamma_1^+ + \Gamma_1^- + \Gamma_3^+ + \Gamma_5^-, 2A_1A_2, 2M_1 + 2M_2, 2Z_2 + Z_3Z_4, 2R_1R_2, 2X_1 + 2X_2]$                                    | trivial                         |
| $[(\blacksquare)^{2T} + \Gamma_1^+ + 2\Gamma_1^- + \Gamma_3^- + \Gamma_5^-, A_1A_2 + A_3A_4, M_1 + M_2 + M_3 + M_4, 2Z_2 + Z_3Z_4, 2R_1R_2, 2X_1 + 2X_2]$                  | 1                               |
| $[(\blacksquare)^{2T} + \Gamma_1^+ + \Gamma_1^- + \Gamma_2^- + \Gamma_4^- + \Gamma_5^-, A_1A_2 + A_3A_4, M_1 + M_2 + M_3 + M_4, Z_1 + Z_2 + Z_3Z_4, 2R_1R_2, 2X_1 + 2X_2]$ | trivial                         |
| $[(\blacksquare)^{2T} + \Gamma_1^+ + \Gamma_1^- + \Gamma_2^+ + \Gamma_4^+ + \Gamma_5^+, 2A_1A_2, 2M_1 + 2M_2, Z_1 + Z_2 + Z_3Z_4, 2R_1R_2, 2X_1 + 2X_2]$                   | 1                               |
| $[(\blacksquare)^{2T} + \Gamma_1^+ + \Gamma_2^+ + \Gamma_2^- + \Gamma_3^+ + \Gamma_5^+, 2A_1A_2, 3M_1 + M_2, Z_1 + Z_2 + Z_3Z_4, 2R_1R_2, 2X_1 + 2X_2]$                    | 1                               |
| $[(\blacksquare)^{2T} + \Gamma_1^+ + 2\Gamma_1^- + \Gamma_3^- + \Gamma_5^-, 2A_1A_2, 2M_1 + 2M_2, 2Z_2 + Z_3Z_4, 2R_1R_2, 2X_1 + 2X_2]$                                    | trivial                         |
| $[(\blacksquare)^{2T} + \Gamma_1^+ + \Gamma_1^- + \Gamma_2^- + \Gamma_4^- + \Gamma_5^-, 2A_1A_2, 2M_1 + 2M_2, Z_1 + Z_2 + Z_3Z_4, 2R_1R_2, 2X_1 + 2X_2]$                   | 1                               |
| $[(\blacksquare)^{2T} + \Gamma_1^- + \Gamma_2^+ + \Gamma_2^- + \Gamma_3^- + \Gamma_5^-, A_1A_2 + A_3A_4, 2M_1 + M_3 + M_4, Z_1 + Z_2 + Z_3Z_4, 2R_1R_2, 2X_1 + 2X_2]$      | trivial                         |
| $[(\blacksquare)^{2T} + \Gamma_2^+ + 2\Gamma_2^- + \Gamma_4^- + \Gamma_5^-, A_1A_2 + A_3A_4, 2M_1 + M_3 + M_4, 2Z_1 + Z_3Z_4, 2R_1R_2, 2X_1 + 2X_2]$                       | 1                               |
| $[(\blacksquare)^{2T} + 2\Gamma_2^+ + \Gamma_2^- + \Gamma_4^+ + \Gamma_5^+, A_1A_2 + A_3A_4, 2M_1 + M_3 + M_4, 2Z_1 + Z_3Z_4, 2R_1R_2, 2X_1 + 2X_2]$                       | 1                               |
| $[(\blacksquare)^{2T} + 2\Gamma_2^+ + \Gamma_2^- + \Gamma_4^+ + \Gamma_5^+, 2A_1A_2, 3M_1 + M_2, 2Z_1 + Z_3Z_4, 2R_1R_2, 2X_1 + 2X_2]$                                     | trivial                         |
| $[(\blacksquare)^{2T} + \Gamma_1^- + \Gamma_2^+ + \Gamma_2^- + \Gamma_3^- + \Gamma_5^-, 2A_1A_2, 3M_1 + M_2, Z_1 + Z_2 + Z_3Z_4, 2R_1R_2, 2X_1 + 2X_2]$                    | 1                               |
| $[(\blacksquare)^{2T} + \Gamma_2^+ + 2\Gamma_2^- + \Gamma_4^- + \Gamma_5^-, 2A_1A_2, 3M_1 + M_2, 2Z_1 + Z_3Z_4, 2R_1R_2, 2X_1 + 2X_2]$                                     | trivial                         |

---

2nd minimal solution:  $\mu_2^T = 12$  (132 symmetry vectors)

Space group 131 ( $\mathbb{Z}_1$ )

1st minimal solution:  $\mu_1^T = 2$  (4 symmetry vectors)

---

| $\mathbf{n}^T$                                                                 |
|--------------------------------------------------------------------------------|
| $[(\blacksquare)^{2T}, A_2, M_2^- + M_3^+, Z_4, R_1^- + R_4^-, X_2^+ + X_3^+]$ |
| $[(\blacksquare)^{2T}, A_1, M_2^+ + M_3^-, Z_3, R_2^- + R_3^-, X_2^- + X_3^-]$ |
| $[(\blacksquare)^{2T}, A_2, M_2^- + M_3^+, Z_3, R_2^+ + R_3^+, X_2^+ + X_3^+]$ |
| $[(\blacksquare)^{2T}, A_1, M_2^+ + M_3^-, Z_4, R_1^+ + R_4^+, X_2^- + X_3^-]$ |

---





1st minimal solution:  $\mu_1^T = 8$  (60 symmetry vectors)

[illegible]

... continued on next page

... continued from previous page

$$\begin{aligned}
&[(\blacksquare)^{2T} + \Gamma_1^+ + \Gamma_1^- + \Gamma_2^- + \Gamma_4^- + \Gamma_5^-, 2A_1 + 2A_2, 2M_1 + 2M_2, Z_1 + Z_2 + Z_3 + Z_4, 2R_1 + 2R_2, 2X_1 + 2X_2] \\
&[(\blacksquare)^{2T} + \Gamma_1^- + \Gamma_2^+ + \Gamma_2^- + \Gamma_3^- + \Gamma_5^-, A_1 + A_2 + A_3A_4, M_1 + M_2 + 2M_3, Z_1 + Z_2 + Z_3 + Z_4, 2R_1 + 2R_2, 2X_1 + 2X_2] \\
&[(\blacksquare)^{2T} + \Gamma_1^+ + \Gamma_2^+ + \Gamma_2^- + \Gamma_3^+ + \Gamma_5^+, 2A_3A_4, 3M_3 + M_4, Z_1 + Z_2 + 2Z_4, 3R_1 + R_2, 2X_1 + 2X_2] \\
&[(\blacksquare)^{2T} + \Gamma_1^+ + \Gamma_2^+ + \Gamma_2^- + \Gamma_3^+ + \Gamma_5^+, A_1 + A_2 + A_3A_4, M_1 + M_2 + 2M_3, Z_1 + Z_2 + 2Z_4, 3R_1 + R_2, 2X_1 + 2X_2] \\
&[(\blacksquare)^{2T} + \Gamma_2^- + \Gamma_3^+ + \Gamma_3^- + \Gamma_4^- + \Gamma_5^-, 2A_3A_4, 3M_3 + M_4, Z_1 + Z_2 + 2Z_4, 3R_1 + R_2, X_1 + 3X_2] \\
&[(\blacksquare)^{2T} + \Gamma_1^+ + \Gamma_1^- + \Gamma_2^- + \Gamma_4^- + \Gamma_5^-, 2A_3A_4, 2M_3 + 2M_4, Z_1 + Z_2 + 2Z_4, 3R_1 + R_2, 2X_1 + 2X_2] \\
&[(\blacksquare)^{2T} + \Gamma_1^+ + \Gamma_1^- + \Gamma_2^- + \Gamma_4^- + \Gamma_5^-, A_1 + A_2 + A_3A_4, M_1 + M_2 + M_3 + M_4, Z_1 + Z_2 + 2Z_4, 3R_1 + R_2, 2X_1 + 2X_2] \\
&[(\blacksquare)^{2T} + \Gamma_1^- + \Gamma_2^+ + \Gamma_2^- + \Gamma_3^- + \Gamma_5^-, 2A_3A_4, 3M_3 + M_4, Z_1 + Z_2 + 2Z_4, 3R_1 + R_2, 2X_1 + 2X_2] \\
&[(\blacksquare)^{2T} + \Gamma_2^- + \Gamma_3^+ + \Gamma_3^- + \Gamma_4^- + \Gamma_5^-, A_1 + A_2 + A_3A_4, M_1 + M_2 + 2M_3, Z_1 + Z_2 + 2Z_4, 3R_1 + R_2, X_1 + 3X_2] \\
&[(\blacksquare)^{2T} + \Gamma_1^+ + \Gamma_1^- + \Gamma_2^- + \Gamma_4^- + \Gamma_5^-, 2A_1 + 2A_2, 2M_1 + 2M_2, Z_1 + Z_2 + 2Z_4, 3R_1 + R_2, 2X_1 + 2X_2] \\
&[(\blacksquare)^{2T} + \Gamma_1^- + \Gamma_2^+ + \Gamma_2^- + \Gamma_3^- + \Gamma_5^-, A_1 + A_2 + A_3A_4, M_1 + M_2 + 2M_3, Z_1 + Z_2 + 2Z_4, 3R_1 + R_2, 2X_1 + 2X_2]
\end{aligned}$$

2nd minimal solution:  $\mu_2^T = 12$  (452 symmetry vectors)

Space group 134 ( $\mathbb{Z}_1$ )

1st minimal solution:  $\mu_1^T = 4$  (8 symmetry vectors)

$$\begin{aligned}
&\mathbf{n}^T \\
&[(\blacksquare)^{2T} + \Gamma_3^- + \Gamma_4^+, A_2^- + A_3^- + A_5^-, M_1 + M_3, Z_1 + Z_3, R_1 + R_2, 2X_2] \\
&[(\blacksquare)^{2T} + \Gamma_3^- + \Gamma_4^+, A_1^+ + A_4^+ + A_5^+, M_1 + M_3, Z_1 + Z_4, R_1 + R_2, 2X_2] \\
&[(\blacksquare)^{2T} + \Gamma_1^+ + \Gamma_2^-, A_2^- + A_3^- + A_5^-, M_1 + M_3, Z_1 + Z_3, R_1 + R_2, X_1 + X_2] \\
&[(\blacksquare)^{2T} + \Gamma_1^+ + \Gamma_2^-, A_1^+ + A_4^+ + A_5^+, M_1 + M_3, Z_1 + Z_4, R_1 + R_2, X_1 + X_2] \\
&[(\blacksquare)^{2T} + \Gamma_3^+ + \Gamma_4^-, A_1^- + A_4^- + A_5^-, M_2 + M_3, Z_2 + Z_4, R_1 + R_2, 2X_2] \\
&[(\blacksquare)^{2T} + \Gamma_1^- + \Gamma_2^+, A_1^- + A_4^- + A_5^-, M_2 + M_3, Z_2 + Z_4, R_1 + R_2, X_1 + X_2] \\
&[(\blacksquare)^{2T} + \Gamma_3^+ + \Gamma_4^-, A_2^+ + A_3^+ + A_5^+, M_2 + M_3, Z_2 + Z_3, R_1 + R_2, 2X_2] \\
&[(\blacksquare)^{2T} + \Gamma_1^- + \Gamma_2^+, A_2^+ + A_3^+ + A_5^+, M_2 + M_3, Z_2 + Z_3, R_1 + R_2, X_1 + X_2]
\end{aligned}$$

2nd minimal solution:  $\mu_2^T = 6$  (100 symmetry vectors)

Space group 135 ( $\mathbb{Z}_1$ )

1st minimal solution:  $\mu_1^T = 8$  (18 symmetry vectors)

$$\begin{aligned}
&\mathbf{n}^T \\
&[(\blacksquare)^{2T} + \Gamma_1^+ + \Gamma_2^+ + \Gamma_2^- + \Gamma_3^+ + \Gamma_5^-, 2A_3A_4, M_1^+M_4^+ + 2M_1^-M_4^- + M_2^-M_3^-, Z_1 + Z_2 + Z_3 + Z_4, 2R_1 + 2R_2, X_1 + 3X_2] \\
&[(\blacksquare)^{2T} + \Gamma_1^+ + \Gamma_1^- + \Gamma_2^- + \Gamma_4^- + \Gamma_5^-, 2A_3A_4, M_1^+M_4^+ + M_1^-M_4^- + M_2^+M_3^+ + M_2^-M_3^-, Z_1 + Z_2 + Z_3 + Z_4, 2R_1 + 2R_2, 2X_1 + 2X_2] \\
&[(\blacksquare)^{2T} + \Gamma_1^+ + \Gamma_1^- + \Gamma_2^- + \Gamma_4^- + \Gamma_5^-, A_1A_2 + A_3A_4, M_1^-M_4^- + M_2^-M_3^- + 2M_5^-, Z_1 + Z_2 + Z_3 + Z_4, 2R_1 + 2R_2, 2X_1 + 2X_2] \\
&[(\blacksquare)^{2T} + \Gamma_1^+ + \Gamma_1^- + \Gamma_2^+ + \Gamma_4^+ + \Gamma_5^-, A_1A_2 + A_3A_4, M_1^-M_4^- + M_2^-M_3^- + M_5^+ + M_5^-, Z_1 + Z_2 + Z_3 + Z_4, 2R_1 + 2R_2, X_1 + 3X_2] \\
&[(\blacksquare)^{2T} + \Gamma_1^+ + \Gamma_2^+ + \Gamma_2^- + \Gamma_3^+ + \Gamma_5^-, A_1A_2 + A_3A_4, M_1^+M_4^+ + M_1^-M_4^- + 2M_5^+, Z_1 + Z_2 + Z_3 + Z_4, 2R_1 + 2R_2, X_1 + 3X_2] \\
&[(\blacksquare)^{2T} + \Gamma_1^- + \Gamma_2^+ + \Gamma_2^- + \Gamma_3^- + \Gamma_5^-, A_1A_2 + A_3A_4, M_1^+M_4^+ + M_1^-M_4^- + M_5^+ + M_5^-, Z_1 + Z_2 + Z_3 + Z_4, 2R_1 + 2R_2, 2X_1 + 2X_2] \\
&[(\blacksquare)^{2T} + \Gamma_1^+ + \Gamma_1^- + \Gamma_2^- + \Gamma_4^- + \Gamma_5^-, A_1A_2 + A_3A_4, M_1^+M_4^+ + M_2^+M_3^+ + 2M_5^+, Z_1 + Z_2 + Z_3 + Z_4, 2R_1 + 2R_2, 2X_1 + 2X_2] \\
&[(\blacksquare)^{2T} + \Gamma_1^+ + \Gamma_1^- + \Gamma_2^- + \Gamma_4^- + \Gamma_5^-, 2A_1A_2, 2M_5^+ + 2M_5^-, Z_1 + Z_2 + Z_3 + Z_4, 2R_1 + 2R_2, 2X_1 + 2X_2] \\
&[(\blacksquare)^{2T} + \Gamma_1^+ + \Gamma_1^- + \Gamma_2^+ + \Gamma_4^+ + \Gamma_5^-, 2A_1A_2, 3M_5^+ + M_5^-, Z_1 + Z_2 + Z_3 + Z_4, 2R_1 + 2R_2, X_1 + 3X_2] \\
&[(\blacksquare)^{2T} + \Gamma_1^+ + \Gamma_2^+ + \Gamma_2^- + \Gamma_3^+ + \Gamma_5^+, A_1A_2 + A_3A_4, M_1^+M_4^+ + M_1^-M_4^- + M_5^+ + M_5^-, Z_1 + Z_2 + Z_3 + Z_4, 2R_1 + 2R_2, 2X_1 + 2X_2] \\
&[(\blacksquare)^{2T} + \Gamma_1^+ + \Gamma_1^- + \Gamma_2^- + \Gamma_4^- + \Gamma_5^+, A_1A_2 + A_3A_4, M_1^+M_4^+ + M_2^+M_3^+ + M_5^+ + M_5^-, Z_1 + Z_2 + Z_3 + Z_4, 2R_1 + 2R_2, 3X_1 + X_2] \\
&[(\blacksquare)^{2T} + \Gamma_1^+ + \Gamma_1^- + \Gamma_2^+ + \Gamma_4^+ + \Gamma_5^+, 2A_3A_4, M_1^+M_4^+ + M_1^-M_4^- + M_2^+M_3^+ + M_2^-M_3^-, Z_1 + Z_2 + Z_3 + Z_4, 2R_1 + 2R_2, 2X_1 + 2X_2]
\end{aligned}$$

... continued on next page

... continued from previous page

$$\begin{aligned}
&[(\blacksquare)^{2T} + \Gamma_1^+ + \Gamma_1^- + \Gamma_2^- + \Gamma_4^- + \Gamma_5^+, 2A_1A_2, M_5^+ + 3M_5^-, Z_1 + Z_2 + Z_3 + Z_4, 2R_1 + 2R_2, 3X_1 + X_2] \\
&[(\blacksquare)^{2T} + \Gamma_1^+ + \Gamma_1^- + \Gamma_2^+ + \Gamma_4^+ + \Gamma_5^+, 2A_1A_2, 2M_5^+ + 2M_5^-, Z_1 + Z_2 + Z_3 + Z_4, 2R_1 + 2R_2, 2X_1 + 2X_2] \\
&[(\blacksquare)^{2T} + \Gamma_1^+ + \Gamma_1^- + \Gamma_2^+ + \Gamma_4^+ + \Gamma_5^+, A_1A_2 + A_3A_4, M_1^-M_4^- + M_2^-M_3^- + 2M_5^-, Z_1 + Z_2 + Z_3 + Z_4, 2R_1 + 2R_2, 2X_1 + 2X_2] \\
&[(\blacksquare)^{2T} + \Gamma_1^+ + \Gamma_1^- + \Gamma_2^+ + \Gamma_4^+ + \Gamma_5^+, A_1A_2 + A_3A_4, M_1^+M_4^+ + M_2^+M_3^+ + 2M_5^+, Z_1 + Z_2 + Z_3 + Z_4, 2R_1 + 2R_2, 2X_1 + 2X_2] \\
&[(\blacksquare)^{2T} + \Gamma_1^- + \Gamma_2^+ + \Gamma_2^- + \Gamma_3^- + \Gamma_5^+, 2A_3A_4, 2M_1^+M_4^+ + M_1^-M_4^- + M_2^+M_3^+, Z_1 + Z_2 + Z_3 + Z_4, 2R_1 + 2R_2, 3X_1 + X_2] \\
&[(\blacksquare)^{2T} + \Gamma_1^- + \Gamma_2^+ + \Gamma_2^- + \Gamma_3^- + \Gamma_5^+, A_1A_2 + A_3A_4, M_1^+M_4^+ + M_1^-M_4^- + 2M_5^-, Z_1 + Z_2 + Z_3 + Z_4, 2R_1 + 2R_2, 3X_1 + X_2]
\end{aligned}$$

2nd minimal solution:  $\mu_2^T = 12$  (170 symmetry vectors)

Space group 136 ( $\mathbb{Z}_1$ )

1st minimal solution:  $\mu_1^T = 4$  (12 symmetry vectors)

| $n^T$                                                                                                                 |
|-----------------------------------------------------------------------------------------------------------------------|
| $[(\blacksquare)^{2T} + \Gamma_1^+ + \Gamma_2^-, A_1 + A_3, M_2^-M_3^- + M_5^-, Z_1 + Z_3, 2R_1^-, X_1 + X_2]$        |
| $[(\blacksquare)^{2T} + \Gamma_1^+ + \Gamma_2^-, A_1 + A_3, M_2^-M_3^- + M_5^-, Z_1 + Z_3, R_1^+ + R_1^-, X_1 + X_2]$ |
| $[(\blacksquare)^{2T} + \Gamma_1^+ + \Gamma_2^-, A_1 + A_3, M_2^-M_3^- + M_5^-, Z_1 + Z_3, 2R_1^+, X_1 + X_2]$        |
| $[(\blacksquare)^{2T} + \Gamma_1^+ + \Gamma_2^-, A_1 + A_4, M_2^-M_3^- + M_5^-, Z_1 + Z_4, 2R_1^-, X_1 + X_2]$        |
| $[(\blacksquare)^{2T} + \Gamma_1^+ + \Gamma_2^-, A_1 + A_4, M_2^-M_3^- + M_5^-, Z_1 + Z_4, R_1^+ + R_1^-, X_1 + X_2]$ |
| $[(\blacksquare)^{2T} + \Gamma_1^+ + \Gamma_2^-, A_1 + A_4, M_2^-M_3^- + M_5^-, Z_1 + Z_4, 2R_1^+, X_1 + X_2]$        |
| $[(\blacksquare)^{2T} + \Gamma_1^- + \Gamma_2^+, A_2 + A_3, M_2^+M_3^+ + M_5^+, Z_2 + Z_3, 2R_1^-, X_1 + X_2]$        |
| $[(\blacksquare)^{2T} + \Gamma_1^- + \Gamma_2^+, A_2 + A_3, M_2^+M_3^+ + M_5^+, Z_2 + Z_3, R_1^+ + R_1^-, X_1 + X_2]$ |
| $[(\blacksquare)^{2T} + \Gamma_1^- + \Gamma_2^+, A_2 + A_3, M_2^+M_3^+ + M_5^+, Z_2 + Z_3, 2R_1^+, X_1 + X_2]$        |
| $[(\blacksquare)^{2T} + \Gamma_1^- + \Gamma_2^+, A_2 + A_4, M_2^+M_3^+ + M_5^+, Z_2 + Z_4, 2R_1^-, X_1 + X_2]$        |
| $[(\blacksquare)^{2T} + \Gamma_1^- + \Gamma_2^+, A_2 + A_4, M_2^+M_3^+ + M_5^+, Z_2 + Z_4, R_1^+ + R_1^-, X_1 + X_2]$ |
| $[(\blacksquare)^{2T} + \Gamma_1^- + \Gamma_2^+, A_2 + A_4, M_2^+M_3^+ + M_5^+, Z_2 + Z_4, 2R_1^+, X_1 + X_2]$        |

2nd minimal solution:  $\mu_2^T = 6$  (136 symmetry vectors)

Space group 137 ( $\mathbb{Z}_1$ )

1st minimal solution:  $\mu_1^T = 6$  (12 symmetry vectors)

| $n^T$                                                                                                                                  |
|----------------------------------------------------------------------------------------------------------------------------------------|
| $[(\blacksquare)^{2T} + \Gamma_1^+ + \Gamma_2^+ + \Gamma_5^+, A_2 + A_3A_4, M_1 + M_3 + M_4, Z_1 + Z_3 + Z_4, 2R_1 + R_2, 2X_1 + X_2]$ |
| $[(\blacksquare)^{2T} + \Gamma_1^+ + \Gamma_2^+ + \Gamma_5^+, A_1 + A_3A_4, M_1 + M_3 + M_4, Z_1 + Z_3 + Z_4, 2R_1 + R_2, 2X_1 + X_2]$ |
| $[(\blacksquare)^{2T} + \Gamma_1^+ + \Gamma_2^+ + \Gamma_5^+, 3A_2, 2M_1 + M_2, Z_1 + Z_3 + Z_4, 2R_1 + R_2, 2X_1 + X_2]$              |
| $[(\blacksquare)^{2T} + \Gamma_1^+ + \Gamma_2^+ + \Gamma_5^+, A_1 + 2A_2, 2M_1 + M_2, Z_1 + Z_3 + Z_4, 2R_1 + R_2, 2X_1 + X_2]$        |
| $[(\blacksquare)^{2T} + \Gamma_1^+ + \Gamma_2^+ + \Gamma_5^+, 2A_1 + A_2, 2M_1 + M_2, Z_1 + Z_3 + Z_4, 2R_1 + R_2, 2X_1 + X_2]$        |
| $[(\blacksquare)^{2T} + \Gamma_1^+ + \Gamma_2^+ + \Gamma_5^+, 3A_1, 2M_1 + M_2, Z_1 + Z_3 + Z_4, 2R_1 + R_2, 2X_1 + X_2]$              |
| $[(\blacksquare)^{2T} + \Gamma_1^- + \Gamma_2^- + \Gamma_5^-, A_2 + A_3A_4, M_1 + M_3 + M_4, Z_2 + Z_3 + Z_4, R_1 + 2R_2, X_1 + 2X_2]$ |
| $[(\blacksquare)^{2T} + \Gamma_1^- + \Gamma_2^- + \Gamma_5^-, 3A_2, 2M_1 + M_2, Z_2 + Z_3 + Z_4, R_1 + 2R_2, X_1 + 2X_2]$              |
| $[(\blacksquare)^{2T} + \Gamma_1^- + \Gamma_2^- + \Gamma_5^-, A_1 + A_3A_4, M_1 + M_3 + M_4, Z_2 + Z_3 + Z_4, R_1 + 2R_2, X_1 + 2X_2]$ |
| $[(\blacksquare)^{2T} + \Gamma_1^- + \Gamma_2^- + \Gamma_5^-, A_1 + 2A_2, 2M_1 + M_2, Z_2 + Z_3 + Z_4, R_1 + 2R_2, X_1 + 2X_2]$        |
| $[(\blacksquare)^{2T} + \Gamma_1^- + \Gamma_2^- + \Gamma_5^-, 2A_1 + A_2, 2M_1 + M_2, Z_2 + Z_3 + Z_4, R_1 + 2R_2, X_1 + 2X_2]$        |
| $[(\blacksquare)^{2T} + \Gamma_1^- + \Gamma_2^- + \Gamma_5^-, 3A_1, 2M_1 + M_2, Z_2 + Z_3 + Z_4, R_1 + 2R_2, X_1 + 2X_2]$              |

2nd minimal solution:  $\mu_2^T = 8$  (68 symmetry vectors)

Space group 138 ( $\mathbb{Z}_1$ )

1st minimal solution:  $\mu_1^T = 4$  (4 symmetry vectors)

| $\mathbf{n}^T$                                                                                                   |
|------------------------------------------------------------------------------------------------------------------|
| $[(\blacksquare)^{2T} + \Gamma_1^+ + \Gamma_2^-, A_1^+ A_4^+ + A_5^+, M_1 + M_3, Z_1 + Z_3, R_1 R_2, X_1 + X_2]$ |
| $[(\blacksquare)^{2T} + \Gamma_1^+ + \Gamma_2^-, A_2^- A_3^- + A_5^-, M_1 + M_3, Z_1 + Z_4, R_1 R_2, X_1 + X_2]$ |
| $[(\blacksquare)^{2T} + \Gamma_1^- + \Gamma_2^+, A_2^+ A_3^+ + A_5^+, M_1 + M_4, Z_2 + Z_4, R_1 R_2, X_1 + X_2]$ |
| $[(\blacksquare)^{2T} + \Gamma_1^- + \Gamma_2^+, A_1^- A_4^- + A_5^-, M_1 + M_4, Z_2 + Z_3, R_1 R_2, X_1 + X_2]$ |

2nd minimal solution:  $\mu_2^T = 8$  (82 symmetry vectors)

Space group 139 ( $\mathbb{Z}_1$ )

1st minimal solution:  $\mu_1^T = 3$  (36 symmetry vectors)

| $\mathbf{n}^T$                                                                                                     |
|--------------------------------------------------------------------------------------------------------------------|
| $[(\blacksquare)^{2T} + \Gamma_1^+, M_3^- + M_5^-, P_3 + P_5, X_2^- + X_3^- + X_4^-, N_1^- + 2N_2^-]$              |
| $[(\blacksquare)^{2T} + \Gamma_1^+, M_3^- + M_5^-, P_1 + P_5, X_2^- + X_3^- + X_4^-, N_1^+ + N_1^- + N_2^-]$       |
| $[(\blacksquare)^{2T} + \Gamma_1^+, M_3^- + M_5^-, 2P_3 + P_4, X_1^+ + X_2^+ + X_2^-, N_2^+ + 2N_2^-]$             |
| $[(\blacksquare)^{2T} + \Gamma_1^+, M_3^- + M_5^-, P_1 + P_3 + P_4, X_1^+ + X_2^+ + X_2^-, N_1^+ + N_2^+ + N_2^-]$ |
| $[(\blacksquare)^{2T} + \Gamma_1^+, M_3^- + M_5^-, 2P_1 + P_4, X_1^+ + X_2^+ + X_2^-, 2N_1^+ + N_2^+]$             |
| $[(\blacksquare)^{2T} + \Gamma_2^+, M_4^- + M_5^-, P_4 + P_5, X_2^+ + X_3^+ + X_3^-, N_1^+ + N_2^+ + N_2^-]$       |
| $[(\blacksquare)^{2T} + \Gamma_1^+, M_3^- + M_5^-, P_3 + P_5, X_2^- + X_3^- + X_4^-, N_1^+ + N_2^+ + N_2^-]$       |
| $[(\blacksquare)^{2T} + \Gamma_1^+, M_3^- + M_5^-, P_1 + P_5, X_2^- + X_3^- + X_4^-, 2N_1^+ + N_2^+]$              |
| $[(\blacksquare)^{2T} + \Gamma_1^+, M_3^- + M_5^-, P_2 + 2P_3, X_1^+ + X_2^+ + X_2^-, N_1^- + 2N_2^-]$             |
| $[(\blacksquare)^{2T} + \Gamma_1^+, M_3^- + M_5^-, P_1 + P_2 + P_3, X_1^+ + X_2^+ + X_2^-, N_1^+ + N_1^- + N_2^-]$ |
| $[(\blacksquare)^{2T} + \Gamma_1^+, M_3^- + M_5^-, 2P_1 + P_2, X_1^+ + X_2^+ + X_2^-, 2N_1^+ + N_1^-]$             |
| $[(\blacksquare)^{2T} + \Gamma_2^+, M_4^- + M_5^-, P_2 + P_5, X_2^+ + X_3^+ + X_3^-, N_1^+ + N_1^- + N_2^-]$       |
| $[(\blacksquare)^{2T} + \Gamma_1^+, M_3^- + M_5^-, P_2 + 2P_3, X_1^+ + X_2^+ + X_2^-, N_1^+ + N_2^+ + N_2^-]$      |
| $[(\blacksquare)^{2T} + \Gamma_1^+, M_3^- + M_5^-, P_1 + P_2 + P_3, X_1^+ + X_2^+ + X_2^-, 2N_1^+ + N_2^+]$        |
| $[(\blacksquare)^{2T} + \Gamma_2^+, M_4^- + M_5^-, P_2 + P_5, X_2^+ + X_3^+ + X_3^-, 2N_1^+ + N_2^+]$              |
| $[(\blacksquare)^{2T} + \Gamma_1^+, M_3^- + M_5^-, P_1 + P_3 + P_4, X_1^+ + X_2^+ + X_2^-, N_1^- + 2N_2^-]$        |
| $[(\blacksquare)^{2T} + \Gamma_1^+, M_3^- + M_5^-, 2P_1 + P_4, X_1^+ + X_2^+ + X_2^-, N_1^+ + N_1^- + N_2^-]$      |
| $[(\blacksquare)^{2T} + \Gamma_2^-, M_4^+ + M_5^+, P_3 + P_5, X_2^- + X_3^- + X_3^-, N_1^- + N_2^- + N_2^-]$       |
| $[(\blacksquare)^{2T} + \Gamma_2^-, M_4^+ + M_5^+, P_3 + P_5, X_2^- + X_3^- + X_3^-, N_1^+ + 2N_2^+]$              |
| $[(\blacksquare)^{2T} + \Gamma_2^-, M_4^+ + M_5^+, P_1 + P_5, X_2^- + X_3^- + X_3^-, 2N_1^- + N_2^-]$              |
| $[(\blacksquare)^{2T} + \Gamma_2^-, M_4^+ + M_5^+, P_1 + P_5, X_2^- + X_3^- + X_3^-, N_1^+ + N_1^- + N_2^+]$       |
| $[(\blacksquare)^{2T} + \Gamma_2^+, M_4^- + M_5^-, P_4 + P_5, X_2^+ + X_3^+ + X_3^-, N_1^- + 2N_2^-]$              |
| $[(\blacksquare)^{2T} + \Gamma_1^-, M_3^+ + M_5^+, P_4 + P_5, X_2^+ + X_3^+ + X_4^+, N_1^- + N_2^+ + N_2^-]$       |
| $[(\blacksquare)^{2T} + \Gamma_1^-, M_3^+ + M_5^+, P_3 + 2P_4, X_1^- + X_2^+ + X_2^-, 2N_2^+ + N_2^-]$             |
| $[(\blacksquare)^{2T} + \Gamma_1^-, M_3^+ + M_5^+, P_4 + P_5, X_2^+ + X_3^+ + X_4^+, N_1^+ + 2N_2^+]$              |
| $[(\blacksquare)^{2T} + \Gamma_1^-, M_3^+ + M_5^+, P_2 + P_5, X_2^+ + X_3^+ + X_4^+, 2N_1^- + N_2^-]$              |
| $[(\blacksquare)^{2T} + \Gamma_1^-, M_3^+ + M_5^+, P_2 + P_3 + P_4, X_1^- + X_2^+ + X_2^-, N_1^- + N_2^+ + N_2^-]$ |
| $[(\blacksquare)^{2T} + \Gamma_1^-, M_3^+ + M_5^+, P_2 + P_5, X_2^+ + X_3^+ + X_4^+, N_1^+ + N_1^- + N_2^+]$       |
| $[(\blacksquare)^{2T} + \Gamma_1^-, M_3^+ + M_5^+, P_2 + P_3 + P_4, X_1^- + X_2^+ + X_2^-, N_1^+ + 2N_2^+]$        |
| $[(\blacksquare)^{2T} + \Gamma_1^-, M_3^+ + M_5^+, 2P_2 + P_3, X_1^- + X_2^+ + X_2^-, 2N_1^- + N_2^-]$             |
| $[(\blacksquare)^{2T} + \Gamma_1^-, M_3^+ + M_5^+, 2P_2 + P_3, X_1^- + X_2^+ + X_2^-, N_1^+ + N_1^- + N_2^+]$      |
| $[(\blacksquare)^{2T} + \Gamma_1^-, M_3^+ + M_5^+, P_1 + 2P_4, X_1^- + X_2^+ + X_2^-, N_1^- + N_2^+ + N_2^-]$      |
| $[(\blacksquare)^{2T} + \Gamma_1^-, M_3^+ + M_5^+, P_1 + 2P_4, X_1^- + X_2^+ + X_2^-, N_1^+ + 2N_2^+]$             |
| $[(\blacksquare)^{2T} + \Gamma_1^-, M_3^+ + M_5^+, P_1 + P_2 + P_4, X_1^- + X_2^+ + X_2^-, 2N_1^- + N_2^-]$        |

... continued on next page

... continued from previous page

$$\begin{aligned} &[(\bullet)^{2T} + \Gamma_1^-, M_3^+ + M_5^+, P_1 + P_2 + P_4, X_1^- + X_2^+ + X_2^-, N_1^+ + N_1^- + N_2^+] \\ &[(\bullet)^{2T} + \Gamma_1^-, M_3^+ + M_5^+, P_1 + 2P_2, X_1^- + X_2^+ + X_2^-, N_1^+ + 2N_1^-] \end{aligned}$$

2nd minimal solution:  $\mu_2^T = 4$  (564 symmetry vectors)

Space group 140 ( $\mathbb{Z}_1$ )

1st minimal solution:  $\mu_1^T = 4$  (16 symmetry vectors)

| $\mathbf{n}^T$                                                                                                            |
|---------------------------------------------------------------------------------------------------------------------------|
| $[(\bullet)^{2T} + \Gamma_2^- + \Gamma_4^-, M_4^+ + M_4^- + M_5^+, P_1P_3 + P_2P_4, 2X_3^+ + X_3^- + X_4^+, 2N_1]$        |
| $[(\bullet)^{2T} + \Gamma_1^- + \Gamma_4^-, M_3^- + M_4^+ + M_5^+, P_1P_3 + P_5, X_1^- + X_2^- + X_3^- + X_4^+, 2N_1]$    |
| $[(\bullet)^{2T} + \Gamma_1^+ + \Gamma_2^-, M_1^- + M_4^- + M_5^-, P_2P_4 + P_5, X_1^+ + X_2^+ + 2X_3^+, 2N_1]$           |
| $[(\bullet)^{2T} + \Gamma_1^+ + \Gamma_4^+, M_3^+ + M_4^- + M_5^-, P_2P_4 + P_5, X_1^+ + X_2^+ + X_3^+ + X_4^-, 2N_1]$    |
| $[(\bullet)^{2T} + \Gamma_2^- + \Gamma_3^-, M_3^+ + M_4^- + M_5^+, P_2P_4 + P_5, X_2^+ + X_2^- + 2X_3^+, 2N_1]$           |
| $[(\bullet)^{2T} + \Gamma_2^+ + \Gamma_4^+, M_4^+ + M_4^- + M_5^-, P_1P_3 + P_2P_4, X_3^+ + 2X_3^- + X_4^-, 2N_1]$        |
| $[(\bullet)^{2T} + \Gamma_1^+ + \Gamma_1^-, M_1^- + M_3^- + M_5^-, 2P_5, X_1^+ + X_1^- + X_2^+ + X_2^-, 2N_1]$            |
| $[(\bullet)^{2T} + \Gamma_1^- + \Gamma_3^-, M_3^+ + M_3^- + M_5^+, 2P_5, X_1^- + X_2^+ + 2X_2^-, 2N_1]$                   |
| $[(\bullet)^{2T} + \Gamma_1^- + \Gamma_2^+, M_2^- + M_3^- + M_5^-, P_1P_3 + P_5, X_2^+ + X_2^- + X_3^- + X_4^+, 2N_1]$    |
| $[(\bullet)^{2T} + \Gamma_1^+ + \Gamma_1^-, M_1^- + M_3^- + M_5^-, P_1P_3 + P_2P_4, X_3^+ + X_3^- + X_4^+ + X_4^-, 2N_1]$ |
| $[(\bullet)^{2T} + \Gamma_1^+ + \Gamma_3^+, M_3^+ + M_3^- + M_5^-, 2P_5, X_1^+ + 2X_2^+ + X_2^-, 2N_1]$                   |
| $[(\bullet)^{2T} + \Gamma_1^+ + \Gamma_2^-, M_2^+ + M_3^+ + M_5^-, P_2P_4 + P_5, X_2^+ + X_2^- + X_3^+ + X_4^-, 2N_1]$    |
| $[(\bullet)^{2T} + \Gamma_1^+ + \Gamma_1^-, M_1^+ + M_3^+ + M_5^+, 2P_5, X_1^+ + X_1^- + X_2^+ + X_2^-, 2N_1]$            |
| $[(\bullet)^{2T} + \Gamma_1^+ + \Gamma_1^-, M_1^+ + M_3^+ + M_5^+, P_1P_3 + P_2P_4, X_3^+ + X_3^- + X_4^+ + X_4^-, 2N_1]$ |
| $[(\bullet)^{2T} + \Gamma_1^- + \Gamma_2^+, M_1^+ + M_4^+ + M_5^+, P_1P_3 + P_5, X_1^- + X_2^- + 2X_3^-, 2N_1]$           |
| $[(\bullet)^{2T} + \Gamma_2^+ + \Gamma_3^+, M_3^- + M_4^+ + M_5^-, P_1P_3 + P_5, X_2^+ + X_2^- + 2X_3^-, 2N_1]$           |

2nd minimal solution:  $\mu_2^T = 6$  (324 symmetry vectors)

Space group 141 ( $\mathbb{Z}_1$ )

1st minimal solution:  $\mu_1^T = 2$  (4 symmetry vectors)

| $\mathbf{n}^T$                                   |
|--------------------------------------------------|
| $[(\bullet)^{2T}, M_4, P_2, X_2, N_1^- + N_2^-]$ |
| $[(\bullet)^{2T}, M_4, P_2, X_2, N_1^+ + N_2^+]$ |
| $[(\bullet)^{2T}, M_4, P_1, X_2, N_1^- + N_2^-]$ |
| $[(\bullet)^{2T}, M_4, P_1, X_2, N_1^+ + N_2^+]$ |

2nd minimal solution:  $\mu_2^T = 4$  (24 symmetry vectors)

Space group 142 ( $\mathbb{Z}_1$ )

1st minimal solution:  $\mu_1^T = 8$  (8 symmetry vectors)

| $\mathbf{n}^T$                                                                                                                              |
|---------------------------------------------------------------------------------------------------------------------------------------------|
| $[(\blacksquare)^{2T} + \Gamma_1^+ + \Gamma_2^+ + \Gamma_2^- + \Gamma_3^+ + \Gamma_5^+, M_1 + M_2 + M_3 + M_4, 2P_1P_2, X_1 + 3X_2, 4N_1]$  |
| $[(\blacksquare)^{2T} + \Gamma_1^+ + \Gamma_1^- + \Gamma_2^+ + \Gamma_4^+ + \Gamma_5^+, M_1 + M_2 + M_3 + M_4, 2P_1P_2, 2X_1 + 2X_2, 4N_1]$ |
| $[(\blacksquare)^{2T} + \Gamma_2^+ + \Gamma_3^+ + \Gamma_3^- + \Gamma_4^+ + \Gamma_5^+, M_1 + M_2 + 2M_3, 2P_1P_2, X_1 + 3X_2, 4N_1]$       |
| $[(\blacksquare)^{2T} + \Gamma_1^+ + \Gamma_3^+ + \Gamma_4^+ + \Gamma_4^- + \Gamma_5^+, M_1 + M_2 + 2M_3, 2P_1P_2, 2X_1 + 2X_2, 4N_1]$      |
| $[(\blacksquare)^{2T} + \Gamma_2^- + \Gamma_3^+ + \Gamma_3^- + \Gamma_4^- + \Gamma_5^-, M_1 + M_2 + 2M_3, 2P_1P_2, X_1 + 3X_2, 4N_1]$       |
| $[(\blacksquare)^{2T} + \Gamma_1^- + \Gamma_2^+ + \Gamma_2^- + \Gamma_3^- + \Gamma_5^-, M_1 + M_2 + M_3 + M_4, 2P_1P_2, X_1 + 3X_2, 4N_1]$  |
| $[(\blacksquare)^{2T} + \Gamma_1^+ + \Gamma_1^- + \Gamma_2^- + \Gamma_4^- + \Gamma_5^-, M_1 + M_2 + M_3 + M_4, 2P_1P_2, 2X_1 + 2X_2, 4N_1]$ |
| $[(\blacksquare)^{2T} + \Gamma_1^- + \Gamma_3^- + \Gamma_4^+ + \Gamma_4^- + \Gamma_5^-, M_1 + M_2 + 2M_3, 2P_1P_2, 2X_1 + 2X_2, 4N_1]$      |

2nd minimal solution:  $\mu_2^T = 12$  (36 symmetry vectors)

Space group 143 ( $\mathbb{Z}_1$ )

1st minimal solution:  $\mu_1^T = 2$  (6 symmetry vectors)

| $\mathbf{n}^T$                                                                              |
|---------------------------------------------------------------------------------------------|
| $[(\blacksquare)^{2T}, A_2A_3, 2H_3, 2HA_3, 2K_3, 2KA_3, 2L_1, 2M_1]$                       |
| $[(\blacksquare)^{2T}, A_2A_3, H_1 + H_3, HA_1 + HA_3, K_1 + K_3, KA_1 + KA_3, 2L_1, 2M_1]$ |
| $[(\blacksquare)^{2T}, A_2A_3, H_2 + H_3, HA_2 + HA_3, K_2 + K_3, KA_2 + KA_3, 2L_1, 2M_1]$ |
| $[(\blacksquare)^{2T}, A_2A_3, 2H_1, 2HA_1, 2K_1, 2KA_1, 2L_1, 2M_1]$                       |
| $[(\blacksquare)^{2T}, A_2A_3, H_1 + H_2, HA_1 + HA_2, K_1 + K_2, KA_1 + KA_2, 2L_1, 2M_1]$ |
| $[(\blacksquare)^{2T}, A_2A_3, 2H_2, 2HA_2, 2K_2, 2KA_2, 2L_1, 2M_1]$                       |

2nd minimal solution:  $\mu_2^T = 3$  (10 symmetry vectors)

Space group 144 ( $\mathbb{Z}_1$ )

1st minimal solution:  $\mu_1^T = 3$  (1 symmetry vector)

| $\mathbf{n}^T$                                                                                                                         |
|----------------------------------------------------------------------------------------------------------------------------------------|
| $[(\blacksquare)^{2T} + \Gamma_1, A_1A_3 + A_2, H_1 + H_2 + H_3, HA_1 + HA_2 + HA_3, K_1 + K_2 + K_3, KA_1 + KA_2 + KA_3, 3L_1, 3M_1]$ |

2nd minimal solution:  $\mu_2^T = 6$  (1 symmetry vector)

Space group 145 ( $\mathbb{Z}_1$ )

1st minimal solution:  $\mu_1^T = 3$  (1 symmetry vector)

| $\mathbf{n}^T$                                                                                                                         |
|----------------------------------------------------------------------------------------------------------------------------------------|
| $[(\blacksquare)^{2T} + \Gamma_1, A_1 + A_2A_3, H_1 + H_2 + H_3, HA_1 + HA_2 + HA_3, K_1 + K_2 + K_3, KA_1 + KA_2 + KA_3, 3L_1, 3M_1]$ |

2nd minimal solution:  $\mu_2^T = 6$  (1 symmetry vector)

Space group 146 ( $\mathbb{Z}_1$ )

1st minimal solution:  $\mu_1^T = 2$  (1 symmetry vector)

| $\mathbf{n}^T$                          |
|-----------------------------------------|
| $[(\bullet)^{2T}, T_2 T_3, 2F_1, 2L_1]$ |

2nd minimal solution:  $\mu_2^T = 3$  (1 symmetry vector)

Space group 147 ( $\mathbb{Z}_2 \times \mathbb{Z}_4$ )

1st minimal solution:  $\mu_1^T = 2$  (36 symmetry vectors)

| $\mathbf{n}^T$                                                                  | $\mathbf{v}^T \in \mathbb{Z}_2 \times \mathbb{Z}_4$ |
|---------------------------------------------------------------------------------|-----------------------------------------------------|
| $[(\bullet)^{2T}, A_2^- A_3^-, 2H_1, 2K_1, 2L_1^-, 2M_1^-]$                     | (0, 1)                                              |
| $[(\bullet)^{2T}, A_2^- A_3^-, 2H_1, 2K_1, 2L_1^-, M_1^+ + M_1^-]$              | (0, 2)                                              |
| $[(\bullet)^{2T}, A_2^- A_3^-, 2H_1, 2K_1, L_1^+ + L_1^-, 2M_1^-]$              | (1, 0)                                              |
| $[(\bullet)^{2T}, A_2^- A_3^-, 2H_1, 2K_1, L_1^+ + L_1^-, M_1^+ + M_1^-]$       | (1, 1)                                              |
| $[(\bullet)^{2T}, A_2^- A_3^-, 2H_1, 2K_1, 2L_1^-, 2M_1^+]$                     | (0, 3)                                              |
| $[(\bullet)^{2T}, A_2^- A_3^-, 2H_1, 2K_1, L_1^+ + L_1^-, 2M_1^+]$              | (1, 2)                                              |
| $[(\bullet)^{2T}, A_2^- A_3^-, 2H_1, 2K_1, 2L_1^+, 2M_1^-]$                     | (0, 3)                                              |
| $[(\bullet)^{2T}, A_2^- A_3^-, 2H_1, 2K_1, 2L_1^+, M_1^+ + M_1^-]$              | trivial                                             |
| $[(\bullet)^{2T}, A_2^- A_3^-, 2H_1, 2K_1, 2L_1^+, 2M_1^+]$                     | (0, 1)                                              |
| $[(\bullet)^{2T}, A_2^- A_3^-, H_2 H_3, K_2 K_3, 2L_1^-, 2M_1^-]$               | (0, 1)                                              |
| $[(\bullet)^{2T}, A_2^- A_3^-, H_2 H_3, K_2 K_3, 2L_1^-, M_1^+ + M_1^-]$        | (0, 2)                                              |
| $[(\bullet)^{2T}, A_2^- A_3^-, H_2 H_3, K_2 K_3, L_1^+ + L_1^-, 2M_1^-]$        | (1, 0)                                              |
| $[(\bullet)^{2T}, A_2^- A_3^-, H_2 H_3, K_2 K_3, L_1^+ + L_1^-, M_1^+ + M_1^-]$ | (1, 1)                                              |
| $[(\bullet)^{2T}, A_2^- A_3^-, H_2 H_3, K_2 K_3, 2L_1^-, 2M_1^+]$               | (0, 3)                                              |
| $[(\bullet)^{2T}, A_2^- A_3^-, H_2 H_3, K_2 K_3, L_1^+ + L_1^-, 2M_1^+]$        | (1, 2)                                              |
| $[(\bullet)^{2T}, A_2^- A_3^-, H_2 H_3, K_2 K_3, 2L_1^+, 2M_1^-]$               | (0, 3)                                              |
| $[(\bullet)^{2T}, A_2^- A_3^-, H_2 H_3, K_2 K_3, 2L_1^+, M_1^+ + M_1^-]$        | trivial                                             |
| $[(\bullet)^{2T}, A_2^- A_3^-, H_2 H_3, K_2 K_3, 2L_1^+, 2M_1^+]$               | (0, 1)                                              |
| $[(\bullet)^{2T}, A_2^+ A_3^+, 2H_1, 2K_1, 2L_1^-, 2M_1^-]$                     | (0, 3)                                              |
| $[(\bullet)^{2T}, A_2^+ A_3^+, 2H_1, 2K_1, 2L_1^-, M_1^+ + M_1^-]$              | trivial                                             |
| $[(\bullet)^{2T}, A_2^+ A_3^+, 2H_1, 2K_1, L_1^+ + L_1^-, 2M_1^-]$              | (1, 2)                                              |
| $[(\bullet)^{2T}, A_2^+ A_3^+, 2H_1, 2K_1, L_1^+ + L_1^-, M_1^+ + M_1^-]$       | (1, 3)                                              |
| $[(\bullet)^{2T}, A_2^+ A_3^+, 2H_1, 2K_1, 2L_1^-, 2M_1^+]$                     | (0, 1)                                              |
| $[(\bullet)^{2T}, A_2^+ A_3^+, 2H_1, 2K_1, L_1^+ + L_1^-, 2M_1^+]$              | (1, 0)                                              |
| $[(\bullet)^{2T}, A_2^+ A_3^+, 2H_1, 2K_1, 2L_1^+, 2M_1^-]$                     | (0, 1)                                              |
| $[(\bullet)^{2T}, A_2^+ A_3^+, 2H_1, 2K_1, 2L_1^+, M_1^+ + M_1^-]$              | (0, 2)                                              |
| $[(\bullet)^{2T}, A_2^+ A_3^+, 2H_1, 2K_1, 2L_1^+, 2M_1^+]$                     | (0, 3)                                              |
| $[(\bullet)^{2T}, A_2^+ A_3^+, H_2 H_3, K_2 K_3, 2L_1^-, 2M_1^-]$               | (0, 3)                                              |
| $[(\bullet)^{2T}, A_2^+ A_3^+, H_2 H_3, K_2 K_3, 2L_1^-, M_1^+ + M_1^-]$        | trivial                                             |
| $[(\bullet)^{2T}, A_2^+ A_3^+, H_2 H_3, K_2 K_3, L_1^+ + L_1^-, 2M_1^-]$        | (1, 2)                                              |
| $[(\bullet)^{2T}, A_2^+ A_3^+, H_2 H_3, K_2 K_3, L_1^+ + L_1^-, M_1^+ + M_1^-]$ | (1, 3)                                              |
| $[(\bullet)^{2T}, A_2^+ A_3^+, H_2 H_3, K_2 K_3, 2L_1^-, 2M_1^+]$               | (0, 1)                                              |
| $[(\bullet)^{2T}, A_2^+ A_3^+, H_2 H_3, K_2 K_3, L_1^+ + L_1^-, 2M_1^+]$        | (1, 0)                                              |
| $[(\bullet)^{2T}, A_2^+ A_3^+, H_2 H_3, K_2 K_3, 2L_1^+, 2M_1^-]$               | (0, 1)                                              |
| $[(\bullet)^{2T}, A_2^+ A_3^+, H_2 H_3, K_2 K_3, 2L_1^+, M_1^+ + M_1^-]$        | (0, 2)                                              |
| $[(\bullet)^{2T}, A_2^+ A_3^+, H_2 H_3, K_2 K_3, 2L_1^+, 2M_1^+]$               | (0, 3)                                              |



2nd minimal solution:  $\mu_2^T = 3$  (256 symmetry vectors)

Space group 148 ( $\mathbb{Z}_2 \times \mathbb{Z}_4$ )

1st minimal solution:  $\mu_1^T = 2$  (18 symmetry vectors)

| $\mathbf{n}^T$                                                     | $\mathbf{v}^T \in \mathbb{Z}_2 \times \mathbb{Z}_4$ |
|--------------------------------------------------------------------|-----------------------------------------------------|
| $[(\blacksquare)^{2T}, T_2^- T_3^-, 2F_1^-, 2L_1^+]$               | (1, 1)                                              |
| $[(\blacksquare)^{2T}, T_2^- T_3^-, 2F_1^-, L_1^+ + L_1^-]$        | (1, 2)                                              |
| $[(\blacksquare)^{2T}, T_2^- T_3^-, F_1^+ + F_1^-, 2L_1^+]$        | trivial                                             |
| $[(\blacksquare)^{2T}, T_2^- T_3^-, F_1^+ + F_1^-, L_1^+ + L_1^-]$ | (0, 1)                                              |
| $[(\blacksquare)^{2T}, T_2^- T_3^-, 2F_1^-, 2L_1^-]$               | (1, 3)                                              |
| $[(\blacksquare)^{2T}, T_2^- T_3^-, F_1^+ + F_1^-, 2L_1^-]$        | (0, 2)                                              |
| $[(\blacksquare)^{2T}, T_2^- T_3^-, 2F_1^+, 2L_1^+]$               | (1, 3)                                              |
| $[(\blacksquare)^{2T}, T_2^- T_3^-, 2F_1^+, L_1^+ + L_1^-]$        | (1, 0)                                              |
| $[(\blacksquare)^{2T}, T_2^- T_3^-, 2F_1^+, 2L_1^-]$               | (1, 1)                                              |
| $[(\blacksquare)^{2T}, T_2^- T_3^-, 2F_1^-, 2L_1^+]$               | (1, 3)                                              |
| $[(\blacksquare)^{2T}, T_2^- T_3^-, 2F_1^-, L_1^+ + L_1^-]$        | (1, 0)                                              |
| $[(\blacksquare)^{2T}, T_2^- T_3^-, F_1^+ + F_1^-, 2L_1^+]$        | (0, 2)                                              |
| $[(\blacksquare)^{2T}, T_2^- T_3^-, F_1^+ + F_1^-, L_1^+ + L_1^-]$ | (0, 3)                                              |
| $[(\blacksquare)^{2T}, T_2^- T_3^-, 2F_1^-, 2L_1^-]$               | (1, 1)                                              |
| $[(\blacksquare)^{2T}, T_2^- T_3^-, F_1^+ + F_1^-, 2L_1^-]$        | trivial                                             |
| $[(\blacksquare)^{2T}, T_2^- T_3^-, 2F_1^+, 2L_1^+]$               | (1, 1)                                              |
| $[(\blacksquare)^{2T}, T_2^- T_3^-, 2F_1^+, L_1^+ + L_1^-]$        | (1, 2)                                              |
| $[(\blacksquare)^{2T}, T_2^- T_3^-, 2F_1^+, 2L_1^-]$               | (1, 3)                                              |

2nd minimal solution:  $\mu_2^T = 3$  (128 symmetry vectors)

Space group 149 ( $\mathbb{Z}_1$ )

1st minimal solution:  $\mu_1^T = 2$  (6 symmetry vectors)

| $\mathbf{n}^T$                                                      |
|---------------------------------------------------------------------|
| $[(\blacksquare)^{2T}, A_3, 2H_3, 2K_3, L_1 + L_2, 2M_2]$           |
| $[(\blacksquare)^{2T}, A_3, H_1 + H_3, K_1 + K_3, L_1 + L_2, 2M_2]$ |
| $[(\blacksquare)^{2T}, A_3, H_2 + H_3, K_2 + K_3, L_1 + L_2, 2M_2]$ |
| $[(\blacksquare)^{2T}, A_3, 2H_1, 2K_1, L_1 + L_2, 2M_2]$           |
| $[(\blacksquare)^{2T}, A_3, H_1 + H_2, K_1 + K_2, L_1 + L_2, 2M_2]$ |
| $[(\blacksquare)^{2T}, A_3, 2H_2, 2K_2, L_1 + L_2, 2M_2]$           |

2nd minimal solution:  $\mu_2^T = 3$  (40 symmetry vectors)

Space group 150 ( $\mathbb{Z}_1$ )

1st minimal solution:  $\mu_1^T = 2$  (1 symmetry vector)

| $\mathbf{n}^T$                                                                     |
|------------------------------------------------------------------------------------|
| $[(\blacksquare)^{2T}, A_3, H_1 + H_2, HA_1 + HA_2, 2K_2, 2KA_2, L_1 + L_2, 2M_2]$ |

2nd minimal solution:  $\mu_2^T = 3$  (6 symmetry vectors)

Space group 151 ( $\mathbb{Z}_1$ )

1st minimal solution:  $\mu_1^T = 3$  (4 symmetry vectors)

| $\mathbf{n}^T$                                                                                          |
|---------------------------------------------------------------------------------------------------------|
| $[(\blacksquare)^{2T} + \Gamma_2, A_1 + A_3, H_1 + H_2 + H_3, K_1 + K_2 + K_3, 2L_1 + L_2, 3M_2]$       |
| $[(\blacksquare)^{2T} + \Gamma_1, A_1 + A_3, H_1 + H_2 + H_3, K_1 + K_2 + K_3, 2L_1 + L_2, M_1 + 2M_2]$ |
| $[(\blacksquare)^{2T} + \Gamma_2, A_2 + A_3, H_1 + H_2 + H_3, K_1 + K_2 + K_3, L_1 + 2L_2, 3M_2]$       |
| $[(\blacksquare)^{2T} + \Gamma_1, A_2 + A_3, H_1 + H_2 + H_3, K_1 + K_2 + K_3, L_1 + 2L_2, M_1 + 2M_2]$ |

2nd minimal solution:  $\mu_2^T = 6$  (9 symmetry vectors)

Space group 152 ( $\mathbb{Z}_1$ )

1st minimal solution:  $\mu_1^T = 3$  (2 symmetry vectors)

| $\mathbf{n}^T$                                                                                                        |
|-----------------------------------------------------------------------------------------------------------------------|
| $[(\blacksquare)^{2T} + \Gamma_1, A_2 + A_3, H_2 + H_3, HA_2 + HA_3, K_2 + K_3, KA_2 + KA_3, 2L_1 + L_2, M_1 + 2M_2]$ |
| $[(\blacksquare)^{2T} + \Gamma_1, A_1 + A_3, H_1 + H_3, HA_1 + HA_3, K_2 + K_3, KA_2 + KA_3, L_1 + 2L_2, M_1 + 2M_2]$ |

2nd minimal solution:  $\mu_2^T = 6$  (6 symmetry vectors)

Space group 153 ( $\mathbb{Z}_1$ )

1st minimal solution:  $\mu_1^T = 3$  (4 symmetry vectors)

| $\mathbf{n}^T$                                                                                          |
|---------------------------------------------------------------------------------------------------------|
| $[(\blacksquare)^{2T} + \Gamma_2, A_1 + A_3, H_1 + H_2 + H_3, K_1 + K_2 + K_3, L_1 + 2L_2, 3M_2]$       |
| $[(\blacksquare)^{2T} + \Gamma_1, A_1 + A_3, H_1 + H_2 + H_3, K_1 + K_2 + K_3, L_1 + 2L_2, M_1 + 2M_2]$ |
| $[(\blacksquare)^{2T} + \Gamma_2, A_2 + A_3, H_1 + H_2 + H_3, K_1 + K_2 + K_3, 2L_1 + L_2, 3M_2]$       |
| $[(\blacksquare)^{2T} + \Gamma_1, A_2 + A_3, H_1 + H_2 + H_3, K_1 + K_2 + K_3, 2L_1 + L_2, M_1 + 2M_2]$ |

2nd minimal solution:  $\mu_2^T = 6$  (9 symmetry vectors)

Space group 154 ( $\mathbb{Z}_1$ )

1st minimal solution:  $\mu_1^T = 3$  (2 symmetry vectors)

| $\mathbf{n}^T$                                                                                                        |
|-----------------------------------------------------------------------------------------------------------------------|
| $[(\blacksquare)^{2T} + \Gamma_1, A_1 + A_3, H_1 + H_3, HA_1 + HA_3, K_2 + K_3, KA_2 + KA_3, L_1 + 2L_2, M_1 + 2M_2]$ |
| $[(\blacksquare)^{2T} + \Gamma_1, A_2 + A_3, H_2 + H_3, HA_2 + HA_3, K_2 + K_3, KA_2 + KA_3, 2L_1 + L_2, M_1 + 2M_2]$ |

2nd minimal solution:  $\mu_2^T = 6$  (6 symmetry vectors)

Space group 155 ( $\mathbb{Z}_1$ )

1st minimal solution:  $\mu_1^T = 2$  (1 symmetry vector)

| $\mathbf{n}^T$                                |
|-----------------------------------------------|
| $[(\blacksquare)^{2T}, T_3, 2F_2, L_1 + L_2]$ |

2nd minimal solution:  $\mu_2^T = 3$  (4 symmetry vectors)

Space group 156 ( $\mathbb{Z}_1$ )

1st minimal solution:  $\mu_1^T = 2$  (6 symmetry vectors)

| $\mathbf{n}^T$                                                           |
|--------------------------------------------------------------------------|
| $[(\blacksquare)^{2T}, A_3, 2H_3, 2K_3, L_1 + L_2, M_1 + M_2]$           |
| $[(\blacksquare)^{2T}, A_3, H_1 + H_3, K_1 + K_3, L_1 + L_2, M_1 + M_2]$ |
| $[(\blacksquare)^{2T}, A_3, H_2 + H_3, K_2 + K_3, L_1 + L_2, M_1 + M_2]$ |
| $[(\blacksquare)^{2T}, A_3, 2H_1, 2K_1, L_1 + L_2, M_1 + M_2]$           |
| $[(\blacksquare)^{2T}, A_3, H_1 + H_2, K_1 + K_2, L_1 + L_2, M_1 + M_2]$ |
| $[(\blacksquare)^{2T}, A_3, 2H_2, 2K_2, L_1 + L_2, M_1 + M_2]$           |

2nd minimal solution:  $\mu_2^T = 3$  (20 symmetry vectors)

Space group 157 ( $\mathbb{Z}_1$ )

1st minimal solution:  $\mu_1^T = 2$  (2 symmetry vectors)

| $\mathbf{n}^T$                                                                                     |
|----------------------------------------------------------------------------------------------------|
| $[(\blacksquare)^{2T}, A_3, H_3, HA_3, K_3, KA_3, L_1 + L_2, M_1 + M_2]$                           |
| $[(\blacksquare)^{2T}, A_3, H_1 + H_2, HA_1 + HA_2, K_1 + K_2, KA_1 + KA_2, L_1 + L_2, M_1 + M_2]$ |

2nd minimal solution:  $\mu_2^T = 3$  (4 symmetry vectors)

Space group 158 ( $\mathbb{Z}_1$ )

1st minimal solution:  $\mu_1^T = 4$  (6 symmetry vectors)

| $\mathbf{n}^T$                                                                                 |
|------------------------------------------------------------------------------------------------|
| $[(\blacksquare)^{2T} + \Gamma_3, A_3A_3, 2H_3H_3, 4K_3, 2L_1L_2, 2M_1 + 2M_2]$                |
| $[(\blacksquare)^{2T} + \Gamma_3, A_3A_3, H_1H_1 + H_3H_3, 2K_1 + 2K_3, 2L_1L_2, 2M_1 + 2M_2]$ |
| $[(\blacksquare)^{2T} + \Gamma_3, A_3A_3, H_2H_2 + H_3H_3, 2K_2 + 2K_3, 2L_1L_2, 2M_1 + 2M_2]$ |

... continued on next page

... continued from previous page

---


$$\begin{aligned} &[(\blacksquare)^{2T} + \Gamma_3, A_3 A_3, 2H_1 H_1, 4K_1, 2L_1 L_2, 2M_1 + 2M_2] \\ &[(\blacksquare)^{2T} + \Gamma_3, A_3 A_3, H_1 H_1 + H_2 H_2, 2K_1 + 2K_2, 2L_1 L_2, 2M_1 + 2M_2] \\ &[(\blacksquare)^{2T} + \Gamma_3, A_3 A_3, 2H_2 H_2, 4K_2, 2L_1 L_2, 2M_1 + 2M_2] \end{aligned}$$


---

2nd minimal solution:  $\mu_2^T = 6$  (10 symmetry vectors)

Space group 159 ( $\mathbb{Z}_1$ )

1st minimal solution:  $\mu_1^T = 4$  (3 symmetry vectors)

---


$$\begin{aligned} &\mathbf{n}^T \\ &[(\blacksquare)^{2T} + \Gamma_3, A_3 A_3, 2H_3, 2HA_3, 2K_3, 2KA_3, 2L_1 L_2, 2M_1 + 2M_2] \\ &[(\blacksquare)^{2T} + \Gamma_3, A_3 A_3, H_1 + H_2 + H_3, HA_1 + HA_2 + HA_3, K_1 + K_2 + K_3, KA_1 + KA_2 + KA_3, 2L_1 L_2, 2M_1 + 2M_2] \\ &[(\blacksquare)^{2T} + \Gamma_3, A_3 A_3, 2H_1 + 2H_2, 2HA_1 + 2HA_2, 2K_1 + 2K_2, 2KA_1 + 2KA_2, 2L_1 L_2, 2M_1 + 2M_2] \end{aligned}$$


---

2nd minimal solution:  $\mu_2^T = 6$  (4 symmetry vectors)

Space group 160 ( $\mathbb{Z}_1$ )

1st minimal solution:  $\mu_1^T = 2$  (1 symmetry vector)

---


$$\begin{aligned} &\mathbf{n}^T \\ &[(\blacksquare)^{2T}, T_3, F_1 + F_2, L_1 + L_2] \end{aligned}$$


---

2nd minimal solution:  $\mu_2^T = 3$  (2 symmetry vectors)

Space group 161 ( $\mathbb{Z}_1$ )

1st minimal solution:  $\mu_1^T = 4$  (1 symmetry vector)

---


$$\begin{aligned} &\mathbf{n}^T \\ &[(\blacksquare)^{2T} + \Gamma_3, T_3 T_3, 2F_1 + 2F_2, 2L_1 L_2] \end{aligned}$$


---

2nd minimal solution:  $\mu_2^T = 6$  (1 symmetry vector)

Space group 162 ( $\mathbb{Z}_2$ )

1st minimal solution:  $\mu_1^T = 2$  (8 symmetry vectors)

| $\mathbf{n}^T$                                                                     | $\mathbf{v}^T \in \mathbb{Z}_2$ |
|------------------------------------------------------------------------------------|---------------------------------|
| $[(\blacksquare)^{2T}, A_3^-, H_3, K_3, L_1^- + L_2^-, M_2^+ + M_2^-]$             | 1                               |
| $[(\blacksquare)^{2T}, A_3^-, H_3, K_3, L_1^+ + L_2^+, M_2^+ + M_2^-]$             | trivial                         |
| $[(\blacksquare)^{2T}, A_3^-, H_1 + H_2, K_1 + K_2, L_1^- + L_2^-, M_2^+ + M_2^-]$ | 1                               |
| $[(\blacksquare)^{2T}, A_3^-, H_1 + H_2, K_1 + K_2, L_1^+ + L_2^+, M_2^+ + M_2^-]$ | trivial                         |
| $[(\blacksquare)^{2T}, A_3^+, H_3, K_3, L_1^- + L_2^-, M_2^+ + M_2^-]$             | trivial                         |
| $[(\blacksquare)^{2T}, A_3^+, H_3, K_3, L_1^+ + L_2^+, M_2^+ + M_2^-]$             | 1                               |
| $[(\blacksquare)^{2T}, A_3^+, H_1 + H_2, K_1 + K_2, L_1^- + L_2^-, M_2^+ + M_2^-]$ | trivial                         |
| $[(\blacksquare)^{2T}, A_3^+, H_1 + H_2, K_1 + K_2, L_1^+ + L_2^+, M_2^+ + M_2^-]$ | 1                               |

2nd minimal solution:  $\mu_2^T = 3$  (96 symmetry vectors)

Space group 163 ( $\mathbb{Z}_2$ )

1st minimal solution:  $\mu_1^T = 4$  (12 symmetry vectors)

| $\mathbf{n}^T$                                                                                                | $\mathbf{v}^T \in \mathbb{Z}_2$ |
|---------------------------------------------------------------------------------------------------------------|---------------------------------|
| $[(\blacksquare)^{2T} + \Gamma_3^-, A_1 A_2, 2H_3, 2K_3, 2L_1, M_1^+ + 2M_2^+ + M_2^-]$                       | trivial                         |
| $[(\blacksquare)^{2T} + \Gamma_3^-, A_1 A_2, H_1 + H_2 + H_3, K_1 + K_2 + K_3, 2L_1, M_1^+ + 2M_2^+ + M_2^-]$ | trivial                         |
| $[(\blacksquare)^{2T} + \Gamma_3^-, A_1 A_2, 2H_3, 2K_3, 2L_1, M_1^- + M_2^+ + 2M_2^-]$                       | 1                               |
| $[(\blacksquare)^{2T} + \Gamma_3^-, A_1 A_2, H_1 + H_2 + H_3, K_1 + K_2 + K_3, 2L_1, M_1^- + M_2^+ + 2M_2^-]$ | 1                               |
| $[(\blacksquare)^{2T} + \Gamma_3^-, A_1 A_2, 2H_1 + 2H_2, 2K_1 + 2K_2, 2L_1, M_1^+ + 2M_2^+ + M_2^-]$         | trivial                         |
| $[(\blacksquare)^{2T} + \Gamma_3^-, A_1 A_2, 2H_1 + 2H_2, 2K_1 + 2K_2, 2L_1, M_1^- + M_2^+ + 2M_2^-]$         | 1                               |
| $[(\blacksquare)^{2T} + \Gamma_3^+, A_1 A_2, 2H_3, 2K_3, 2L_1, M_1^+ + 2M_2^+ + M_2^-]$                       | 1                               |
| $[(\blacksquare)^{2T} + \Gamma_3^+, A_1 A_2, H_1 + H_2 + H_3, K_1 + K_2 + K_3, 2L_1, M_1^+ + 2M_2^+ + M_2^-]$ | 1                               |
| $[(\blacksquare)^{2T} + \Gamma_3^+, A_1 A_2, 2H_3, 2K_3, 2L_1, M_1^- + M_2^+ + 2M_2^-]$                       | trivial                         |
| $[(\blacksquare)^{2T} + \Gamma_3^+, A_1 A_2, H_1 + H_2 + H_3, K_1 + K_2 + K_3, 2L_1, M_1^- + M_2^+ + 2M_2^-]$ | trivial                         |
| $[(\blacksquare)^{2T} + \Gamma_3^+, A_1 A_2, 2H_1 + 2H_2, 2K_1 + 2K_2, 2L_1, M_1^+ + 2M_2^+ + M_2^-]$         | 1                               |
| $[(\blacksquare)^{2T} + \Gamma_3^+, A_1 A_2, 2H_1 + 2H_2, 2K_1 + 2K_2, 2L_1, M_1^- + M_2^+ + 2M_2^-]$         | trivial                         |

2nd minimal solution:  $\mu_2^T = 6$  (96 symmetry vectors)

Space group 164 ( $\mathbb{Z}_2$ )

1st minimal solution:  $\mu_1^T = 2$  (4 symmetry vectors)

| $\mathbf{n}^T$                                                                | $\mathbf{v}^T \in \mathbb{Z}_2$ |
|-------------------------------------------------------------------------------|---------------------------------|
| $[(\blacksquare)^{2T}, A_3^-, H_1 + H_2, 2K_2, L_1^- + L_2^-, M_2^+ + M_2^-]$ | 1                               |
| $[(\blacksquare)^{2T}, A_3^-, H_1 + H_2, 2K_2, L_1^+ + L_2^+, M_2^+ + M_2^-]$ | trivial                         |
| $[(\blacksquare)^{2T}, A_3^+, H_1 + H_2, 2K_2, L_1^- + L_2^-, M_2^+ + M_2^-]$ | trivial                         |
| $[(\blacksquare)^{2T}, A_3^+, H_1 + H_2, 2K_2, L_1^+ + L_2^+, M_2^+ + M_2^-]$ | 1                               |

2nd minimal solution:  $\mu_2^T = 3$  (80 symmetry vectors)

Space group 165 ( $\mathbb{Z}_2$ )

1st minimal solution:  $\mu_1^T = 4$  (4 symmetry vectors)

| $\mathbf{n}^T$                                                                                    | $\mathbf{v}^T \in \mathbb{Z}_2$ |
|---------------------------------------------------------------------------------------------------|---------------------------------|
| $[(\blacksquare)^{2T} + \Gamma_3^-, A_1 A_2, 2H_1 H_2, K_1 + 3K_2, 2L_1, M_1^+ + 2M_2^+ + M_2^-]$ | trivial                         |
| $[(\blacksquare)^{2T} + \Gamma_3^-, A_1 A_2, 2H_1 H_2, K_1 + 3K_2, 2L_1, M_1^- + M_2^+ + 2M_2^-]$ | 1                               |
| $[(\blacksquare)^{2T} + \Gamma_3^+, A_1 A_2, 2H_1 H_2, K_1 + 3K_2, 2L_1, M_1^+ + 2M_2^+ + M_2^-]$ | 1                               |
| $[(\blacksquare)^{2T} + \Gamma_3^+, A_1 A_2, 2H_1 H_2, K_1 + 3K_2, 2L_1, M_1^- + M_2^+ + 2M_2^-]$ | trivial                         |

2nd minimal solution:  $\mu_2^T = 6$  (44 symmetry vectors)

Space group 166 ( $\mathbb{Z}_2$ )

1st minimal solution:  $\mu_1^T = 2$  (4 symmetry vectors)

| $\mathbf{n}^T$                                               | $\mathbf{v}^T \in \mathbb{Z}_2$ |
|--------------------------------------------------------------|---------------------------------|
| $[(\blacksquare)^{2T}, T_3^-, F_2^+ + F_2^-, L_1^- + L_2^-]$ | 1                               |
| $[(\blacksquare)^{2T}, T_3^-, F_2^+ + F_2^-, L_1^+ + L_2^+]$ | trivial                         |
| $[(\blacksquare)^{2T}, T_3^+, F_2^+ + F_2^-, L_1^- + L_2^-]$ | trivial                         |
| $[(\blacksquare)^{2T}, T_3^+, F_2^+ + F_2^-, L_1^+ + L_2^+]$ | 1                               |

2nd minimal solution:  $\mu_2^T = 3$  (48 symmetry vectors)

Space group 167 ( $\mathbb{Z}_2$ )

1st minimal solution:  $\mu_1^T = 4$  (4 symmetry vectors)

| $\mathbf{n}^T$                                                              | $\mathbf{v}^T \in \mathbb{Z}_2$ |
|-----------------------------------------------------------------------------|---------------------------------|
| $[(\blacksquare)^{2T} + \Gamma_3^-, T_1 T_2, F_1^- + F_2^+ + 2F_2^-, 2L_1]$ | 1                               |
| $[(\blacksquare)^{2T} + \Gamma_3^-, T_1 T_2, F_1^+ + 2F_2^+ + F_2^-, 2L_1]$ | trivial                         |
| $[(\blacksquare)^{2T} + \Gamma_3^+, T_1 T_2, F_1^- + F_2^+ + 2F_2^-, 2L_1]$ | trivial                         |
| $[(\blacksquare)^{2T} + \Gamma_3^+, T_1 T_2, F_1^+ + 2F_2^+ + F_2^-, 2L_1]$ | 1                               |

2nd minimal solution:  $\mu_2^T = 6$  (24 symmetry vectors)

Space group 168 ( $\mathbb{Z}_2$ )

1st minimal solution:  $\mu_1^T = 2$  (6 symmetry vectors)

| $\mathbf{n}^T$                                                           | $\mathbf{v}^T \in \mathbb{Z}_2$ |
|--------------------------------------------------------------------------|---------------------------------|
| $[(\blacksquare)^{2T}, A_4 A_6, 2H_1, 2K_1, 2L_2, 2M_2]$                 | trivial                         |
| $[(\blacksquare)^{2T}, A_4 A_6, 2H_1, 2K_1, L_1 + L_2, M_1 + M_2]$       | 1                               |
| $[(\blacksquare)^{2T}, A_4 A_6, 2H_1, 2K_1, 2L_1, 2M_1]$                 | trivial                         |
| $[(\blacksquare)^{2T}, A_4 A_6, H_2 H_3, K_2 K_3, 2L_2, 2M_2]$           | trivial                         |
| $[(\blacksquare)^{2T}, A_4 A_6, H_2 H_3, K_2 K_3, L_1 + L_2, M_1 + M_2]$ | 1                               |
| $[(\blacksquare)^{2T}, A_4 A_6, H_2 H_3, K_2 K_3, 2L_1, 2M_1]$           | trivial                         |

2nd minimal solution:  $\mu_2^T = 3$  (16 symmetry vectors)

Space group 169 ( $\mathbb{Z}_1$ )

1st minimal solution:  $\mu_1^T = 6$  (1 symmetry vector)

| $\mathbf{n}^T$                                                                                                                                     |
|----------------------------------------------------------------------------------------------------------------------------------------------------|
| $[(\blacksquare)^{2T} + \Gamma_1 + \Gamma_2 + \Gamma_3\Gamma_5, A_1A_6 + A_2A_5 + A_3A_4, 2H_1H_3 + H_2H_2, 2K_1 + 2K_2K_3, 3L_1L_2, 3M_1 + 3M_2]$ |

2nd minimal solution:  $\mu_2^T = 12$  (1 symmetry vector)

Space group 170 ( $\mathbb{Z}_1$ )

1st minimal solution:  $\mu_1^T = 6$  (1 symmetry vector)

| $\mathbf{n}^T$                                                                                                                                     |
|----------------------------------------------------------------------------------------------------------------------------------------------------|
| $[(\blacksquare)^{2T} + \Gamma_1 + \Gamma_2 + \Gamma_3\Gamma_5, A_1A_2 + A_3A_6 + A_4A_5, H_1H_1 + 2H_2H_3, 2K_1 + 2K_2K_3, 3L_1L_2, 3M_1 + 3M_2]$ |

2nd minimal solution:  $\mu_2^T = 12$  (1 symmetry vector)

Space group 171 ( $\mathbb{Z}_2$ )

1st minimal solution:  $\mu_1^T = 3$  (4 symmetry vectors)

| $\mathbf{n}^T$                                                                                       | $\mathbf{v}^T \in \mathbb{Z}_2$ |
|------------------------------------------------------------------------------------------------------|---------------------------------|
| $[(\blacksquare)^{2T} + \Gamma_2, A_2 + A_4A_6, H_1 + H_2H_3, K_1 + K_2K_3, 3L_2, 3M_2]$             | trivial                         |
| $[(\blacksquare)^{2T} + \Gamma_2, A_2 + A_4A_6, H_1 + H_2H_3, K_1 + K_2K_3, L_1 + 2L_2, M_1 + 2M_2]$ | 1                               |
| $[(\blacksquare)^{2T} + \Gamma_2, A_2 + A_4A_6, H_1 + H_2H_3, K_1 + K_2K_3, 2L_1 + L_2, 2M_1 + M_2]$ | trivial                         |
| $[(\blacksquare)^{2T} + \Gamma_2, A_2 + A_4A_6, H_1 + H_2H_3, K_1 + K_2K_3, 3L_1, 3M_1]$             | 1                               |

2nd minimal solution:  $\mu_2^T = 6$  (14 symmetry vectors)

Space group 172 ( $\mathbb{Z}_2$ )

1st minimal solution:  $\mu_1^T = 3$  (4 symmetry vectors)

| $\mathbf{n}^T$                                                                                       | $\mathbf{v}^T \in \mathbb{Z}_2$ |
|------------------------------------------------------------------------------------------------------|---------------------------------|
| $[(\blacksquare)^{2T} + \Gamma_2, A_2A_6 + A_4, H_1H_3 + H_2, K_1 + K_2K_3, 3L_2, 3M_2]$             | trivial                         |
| $[(\blacksquare)^{2T} + \Gamma_2, A_2A_6 + A_4, H_1H_3 + H_2, K_1 + K_2K_3, L_1 + 2L_2, M_1 + 2M_2]$ | 1                               |
| $[(\blacksquare)^{2T} + \Gamma_2, A_2A_6 + A_4, H_1H_3 + H_2, K_1 + K_2K_3, 2L_1 + L_2, 2M_1 + M_2]$ | trivial                         |
| $[(\blacksquare)^{2T} + \Gamma_2, A_2A_6 + A_4, H_1H_3 + H_2, K_1 + K_2K_3, 3L_1, 3M_1]$             | 1                               |

2nd minimal solution:  $\mu_2^T = 6$  (14 symmetry vectors)

Space group 173 ( $\mathbb{Z}_1$ )

1st minimal solution:  $\mu_1^T = 4$  (3 symmetry vectors)

| $\mathbf{n}^T$                                                                                                   |
|------------------------------------------------------------------------------------------------------------------|
| $[(\blacksquare)^{2T}, \Gamma_3\Gamma_5, A_3A_6 + A_4A_5, 2H_2H_3, 2K_2K_3, 2L_1L_2, 2M_1 + 2M_2]$               |
| $[(\blacksquare)^{2T}, \Gamma_3\Gamma_5, A_3A_6 + A_4A_5, H_1H_1 + H_2H_3, 2K_1 + K_2K_3, 2L_1L_2, 2M_1 + 2M_2]$ |
| $[(\blacksquare)^{2T}, \Gamma_3\Gamma_5, A_3A_6 + A_4A_5, 2H_1H_1, 4K_1, 2L_1L_2, 2M_1 + 2M_2]$                  |

2nd minimal solution:  $\mu_2^T = 6$  (4 symmetry vectors)

Space group 174 ( $\mathbb{Z}_1$ )

1st minimal solution:  $\mu_1^T = 2$  (18 symmetry vectors)

| $\mathbf{n}^T$                                                                                   |
|--------------------------------------------------------------------------------------------------|
| $[(\blacksquare)^{2T}, A_3A_5, H_1 + H_5, HA_1 + HA_5, K_1 + K_6, KA_1 + KA_6, 2L_1, M_1 + M_2]$ |
| $[(\blacksquare)^{2T}, A_3A_5, 2H_5, 2HA_5, K_5 + K_6, KA_5 + KA_6, 2L_1, M_1 + M_2]$            |
| $[(\blacksquare)^{2T}, A_3A_5, H_3 + H_5, HA_3 + HA_5, K_3 + K_6, KA_3 + KA_6, 2L_1, M_1 + M_2]$ |
| $[(\blacksquare)^{2T}, A_4A_6, 2H_6, 2HA_6, K_5 + K_6, KA_5 + KA_6, 2L_2, M_1 + M_2]$            |
| $[(\blacksquare)^{2T}, A_4A_6, H_2 + H_6, HA_2 + HA_6, K_2 + K_5, KA_2 + KA_5, 2L_2, M_1 + M_2]$ |
| $[(\blacksquare)^{2T}, A_4A_6, H_4 + H_6, HA_4 + HA_6, K_4 + K_5, KA_4 + KA_5, 2L_2, M_1 + M_2]$ |
| $[(\blacksquare)^{2T}, A_4A_6, H_2 + H_6, HA_2 + HA_6, K_1 + K_6, KA_1 + KA_6, 2L_2, M_1 + M_2]$ |
| $[(\blacksquare)^{2T}, A_4A_6, 2H_2, 2HA_2, K_1 + K_2, KA_1 + KA_2, 2L_2, M_1 + M_2]$            |
| $[(\blacksquare)^{2T}, A_4A_6, H_2 + H_4, HA_2 + HA_4, K_1 + K_4, KA_1 + KA_4, 2L_2, M_1 + M_2]$ |
| $[(\blacksquare)^{2T}, A_4A_6, H_4 + H_6, HA_4 + HA_6, K_3 + K_6, KA_3 + KA_6, 2L_2, M_1 + M_2]$ |
| $[(\blacksquare)^{2T}, A_4A_6, H_2 + H_4, HA_2 + HA_4, K_2 + K_3, KA_2 + KA_3, 2L_2, M_1 + M_2]$ |
| $[(\blacksquare)^{2T}, A_4A_6, 2H_4, 2HA_4, K_3 + K_4, KA_3 + KA_4, 2L_2, M_1 + M_2]$            |
| $[(\blacksquare)^{2T}, A_3A_5, 2H_1, 2HA_1, K_1 + K_2, KA_1 + KA_2, 2L_1, M_1 + M_2]$            |
| $[(\blacksquare)^{2T}, A_3A_5, H_1 + H_5, HA_1 + HA_5, K_2 + K_5, KA_2 + KA_5, 2L_1, M_1 + M_2]$ |
| $[(\blacksquare)^{2T}, A_3A_5, H_1 + H_3, HA_1 + HA_3, K_1 + K_4, KA_1 + KA_4, 2L_1, M_1 + M_2]$ |
| $[(\blacksquare)^{2T}, A_3A_5, H_3 + H_5, HA_3 + HA_5, K_4 + K_5, KA_4 + KA_5, 2L_1, M_1 + M_2]$ |
| $[(\blacksquare)^{2T}, A_3A_5, H_1 + H_3, HA_1 + HA_3, K_2 + K_3, KA_2 + KA_3, 2L_1, M_1 + M_2]$ |
| $[(\blacksquare)^{2T}, A_3A_5, 2H_3, 2HA_3, K_3 + K_4, KA_3 + KA_4, 2L_1, M_1 + M_2]$            |

2nd minimal solution:  $\mu_2^T = 3$  (216 symmetry vectors)

Space group 175 ( $\mathbb{Z}_2 \times \mathbb{Z}_2 \times \mathbb{Z}_2$ )

1st minimal solution:  $\mu_1^T = 2$  (8 symmetry vectors)

| $\mathbf{n}^T$                                                                     | $\mathbf{v}^T \in \mathbb{Z}_2 \times \mathbb{Z}_2 \times \mathbb{Z}_2$ |
|------------------------------------------------------------------------------------|-------------------------------------------------------------------------|
| $[(\blacksquare)^{2T}, A_4^-A_6^-, 2H_1, K_1 + K_2, 2L_2^-, M_2^+ + M_2^-]$        | (0, 0, 1)                                                               |
| $[(\blacksquare)^{2T}, A_4^-A_6^-, 2H_1, K_1 + K_2, L_1^+ + L_2^-, M_1^+ + M_2^+]$ | (1, 0, 1)                                                               |
| $[(\blacksquare)^{2T}, A_4^+A_6^+, 2H_2, K_1 + K_2, 2L_2^+, M_2^+ + M_2^-]$        | (0, 0, 1)                                                               |
| $[(\blacksquare)^{2T}, A_4^+A_6^+, 2H_2, K_1 + K_2, L_1^- + L_2^+, M_1^- + M_2^-]$ | (0, 1, 1)                                                               |
| $[(\blacksquare)^{2T}, A_4^+A_6^+, 2H_2, K_1 + K_2, L_1^- + L_2^+, M_1^+ + M_2^+]$ | (0, 1, 0)                                                               |

... continued on next page



... continued from previous page

|                                                                                |           |
|--------------------------------------------------------------------------------|-----------|
| $[(\bullet)^{2T}, A_4^+ A_6^+, 2H_2, K_1 + K_2, 2L_1^-, M_1^+ + M_1^-]$        | trivial   |
| $[(\bullet)^{2T}, A_4^- A_6^-, 2H_1, K_1 + K_2, L_1^+ + L_2^-, M_1^- + M_2^-]$ | (1, 0, 0) |
| $[(\bullet)^{2T}, A_4^- A_6^-, 2H_1, K_1 + K_2, 2L_1^+, M_1^+ + M_1^-]$        | trivial   |

2nd minimal solution:  $\mu_2^T = 3$  (256 symmetry vectors)

Space group 176 ( $\mathbb{Z}_2$ )

1st minimal solution:  $\mu_1^T = 4$  (12 symmetry vectors)

| $\mathbf{n}^T$                                                                                                            | $\mathbf{v}^T \in \mathbb{Z}_2$ |
|---------------------------------------------------------------------------------------------------------------------------|---------------------------------|
| $[(\bullet)^{2T} + \Gamma_3^- \Gamma_5^-, A_2 A_3, H_1 H_2 + H_4 H_5, K_1 + K_2 + K_4 K_6, 2L_1, 2M_1^- + M_2^+ + M_2^-]$ | 1                               |
| $[(\bullet)^{2T} + \Gamma_3^- \Gamma_5^-, A_2 A_3, H_1 H_2 + H_4 H_5, K_1 + K_2 + K_4 K_6, 2L_1, M_1^+ + M_1^- + 2M_2^+]$ | trivial                         |
| $[(\bullet)^{2T} + \Gamma_3^- \Gamma_5^-, A_2 A_3, H_1 H_2 + H_3 H_6, K_1 + K_2 + K_4 K_6, 2L_1, 2M_1^- + M_2^+ + M_2^-]$ | 1                               |
| $[(\bullet)^{2T} + \Gamma_3^- \Gamma_5^-, A_2 A_3, H_1 H_2 + H_3 H_6, K_1 + K_2 + K_4 K_6, 2L_1, M_1^+ + M_1^- + 2M_2^+]$ | trivial                         |
| $[(\bullet)^{2T} + \Gamma_3^- \Gamma_5^-, A_2 A_3, 2H_1 H_2, K_1 + 3K_2, 2L_1, 2M_1^- + M_2^+ + M_2^-]$                   | 1                               |
| $[(\bullet)^{2T} + \Gamma_3^- \Gamma_5^-, A_2 A_3, 2H_1 H_2, K_1 + 3K_2, 2L_1, M_1^+ + M_1^- + 2M_2^+]$                   | trivial                         |
| $[(\bullet)^{2T} + \Gamma_3^+ \Gamma_5^+, A_2 A_3, H_1 H_2 + H_4 H_5, K_1 + K_2 + K_3 K_5, 2L_1, M_1^+ + M_1^- + 2M_2^-]$ | trivial                         |
| $[(\bullet)^{2T} + \Gamma_3^+ \Gamma_5^+, A_2 A_3, H_1 H_2 + H_4 H_5, K_1 + K_2 + K_3 K_5, 2L_1, 2M_1^+ + M_2^+ + M_2^-]$ | 1                               |
| $[(\bullet)^{2T} + \Gamma_3^+ \Gamma_5^+, A_2 A_3, 2H_1 H_2, 3K_1 + K_2, 2L_1, M_1^+ + M_1^- + 2M_2^-]$                   | trivial                         |
| $[(\bullet)^{2T} + \Gamma_3^+ \Gamma_5^+, A_2 A_3, 2H_1 H_2, 3K_1 + K_2, 2L_1, 2M_1^+ + M_2^+ + M_2^-]$                   | 1                               |
| $[(\bullet)^{2T} + \Gamma_3^+ \Gamma_5^+, A_2 A_3, H_1 H_2 + H_3 H_6, K_1 + K_2 + K_3 K_5, 2L_1, M_1^+ + M_1^- + 2M_2^-]$ | trivial                         |
| $[(\bullet)^{2T} + \Gamma_3^+ \Gamma_5^+, A_2 A_3, H_1 H_2 + H_3 H_6, K_1 + K_2 + K_3 K_5, 2L_1, 2M_1^+ + M_2^+ + M_2^-]$ | 1                               |

2nd minimal solution:  $\mu_2^T = 6$  (268 symmetry vectors)

Space group 177 ( $\mathbb{Z}_1$ )

1st minimal solution:  $\mu_1^T = 2$  (1 symmetry vector)

| $\mathbf{n}^T$                                            |
|-----------------------------------------------------------|
| $[(\bullet)^{2T}, A_6, H_1 + H_2, 2K_2, L_1 + L_2, 2M_2]$ |

2nd minimal solution:  $\mu_2^T = 3$  (16 symmetry vectors)

Space group 178 ( $\mathbb{Z}_1$ )

1st minimal solution:  $\mu_1^T = 6$  (3 symmetry vectors)

| $\mathbf{n}^T$                                                                                                                        |
|---------------------------------------------------------------------------------------------------------------------------------------|
| $[(\bullet)^{2T} + \Gamma_1 + \Gamma_4 + \Gamma_5, A_1 + A_2 + A_3, H_1 H_2 + 2H_3, 2K_2 + 2K_3, 3L_1, M_1 + 2M_2 + M_3 + 2M_4]$      |
| $[(\bullet)^{2T} + \Gamma_1 + \Gamma_3 + \Gamma_5, A_1 + A_2 + A_3, H_1 H_2 + 2H_3, K_1 + K_2 + 2K_3, 3L_1, M_1 + 2M_2 + 2M_3 + M_4]$ |
| $[(\bullet)^{2T} + \Gamma_2 + \Gamma_3 + \Gamma_5, A_1 + A_2 + A_3, H_1 H_2 + 2H_3, 2K_2 + 2K_3, 3L_1, 3M_2 + 2M_3 + M_4]$            |

2nd minimal solution:  $\mu_2^T = 12$  (8 symmetry vectors)

Space group 179 ( $\mathbb{Z}_1$ )

1st minimal solution:  $\mu_1^T = 6$  (3 symmetry vectors)

| $\mathbf{n}^T$                                                                                                                            |
|-------------------------------------------------------------------------------------------------------------------------------------------|
| $[(\blacksquare)^{2T} + \Gamma_1 + \Gamma_4 + \Gamma_5, A_1 + A_2 + A_3, H_1H_2 + 2H_3, 2K_2 + 2K_3, 3L_1, M_1 + 2M_2 + M_3 + 2M_4]$      |
| $[(\blacksquare)^{2T} + \Gamma_1 + \Gamma_3 + \Gamma_5, A_1 + A_2 + A_3, H_1H_2 + 2H_3, K_1 + K_2 + 2K_3, 3L_1, M_1 + 2M_2 + 2M_3 + M_4]$ |
| $[(\blacksquare)^{2T} + \Gamma_2 + \Gamma_3 + \Gamma_5, A_1 + A_2 + A_3, H_1H_2 + 2H_3, 2K_2 + 2K_3, 3L_1, 3M_2 + 2M_3 + M_4]$            |

2nd minimal solution:  $\mu_2^T = 12$  (8 symmetry vectors)

Space group 180 ( $\mathbb{Z}_1$ )

1st minimal solution:  $\mu_1^T = 3$  (2 symmetry vectors)

| $\mathbf{n}^T$                                                                                   |
|--------------------------------------------------------------------------------------------------|
| $[(\blacksquare)^{2T} + \Gamma_3, A_3 + A_6, H_1 + H_3, K_2 + K_3, L_1 + L_2 + L_4, 2M_2 + M_3]$ |
| $[(\blacksquare)^{2T} + \Gamma_3, A_4 + A_6, H_2 + H_3, K_2 + K_3, L_1 + L_2 + L_3, 2M_2 + M_3]$ |

2nd minimal solution:  $\mu_2^T = 6$  (45 symmetry vectors)

Space group 181 ( $\mathbb{Z}_1$ )

1st minimal solution:  $\mu_1^T = 3$  (2 symmetry vectors)

| $\mathbf{n}^T$                                                                                   |
|--------------------------------------------------------------------------------------------------|
| $[(\blacksquare)^{2T} + \Gamma_3, A_3 + A_6, H_1 + H_3, K_2 + K_3, L_1 + L_2 + L_3, 2M_2 + M_3]$ |
| $[(\blacksquare)^{2T} + \Gamma_3, A_4 + A_6, H_2 + H_3, K_2 + K_3, L_1 + L_2 + L_4, 2M_2 + M_3]$ |

2nd minimal solution:  $\mu_2^T = 6$  (45 symmetry vectors)

Space group 182 ( $\mathbb{Z}_1$ )

1st minimal solution:  $\mu_1^T = 4$  (2 symmetry vectors)

| $\mathbf{n}^T$                                                                                  |
|-------------------------------------------------------------------------------------------------|
| $[(\blacksquare)^{2T} + \Gamma_5, A_2 + A_3, H_1H_2 + H_3, 2K_2 + K_3, 2L_1, 2M_2 + M_3 + M_4]$ |
| $[(\blacksquare)^{2T} + \Gamma_5, A_2 + A_3, 2H_1H_2, K_1 + 3K_2, 2L_1, 2M_2 + M_3 + M_4]$      |

2nd minimal solution:  $\mu_2^T = 6$  (12 symmetry vectors)

Space group 183 ( $\mathbb{Z}_1$ )

1st minimal solution:  $\mu_1^T = 2$  (4 symmetry vectors)

| $\mathbf{n}^T$                                                           |
|--------------------------------------------------------------------------|
| $[(\blacksquare)^{2T}, A_6, H_3, K_3, L_3 + L_4, M_3 + M_4]$             |
| $[(\blacksquare)^{2T}, A_6, H_3, K_3, L_1 + L_2, M_1 + M_2]$             |
| $[(\blacksquare)^{2T}, A_6, H_1 + H_2, K_1 + K_2, L_3 + L_4, M_3 + M_4]$ |
| $[(\blacksquare)^{2T}, A_6, H_1 + H_2, K_1 + K_2, L_1 + L_2, M_1 + M_2]$ |

2nd minimal solution:  $\mu_2^T = 3$  (16 symmetry vectors)

Space group 184 ( $\mathbb{Z}_2$ )

1st minimal solution:  $\mu_1^T = 4$  (6 symmetry vectors)

| $\mathbf{n}^T$                                                                                               | $\mathbf{v}^T \in \mathbb{Z}_2$ |
|--------------------------------------------------------------------------------------------------------------|---------------------------------|
| $[(\blacksquare)^{2T} + \Gamma_6, A_6 A_6, 2H_1 H_2, 2K_1 + 2K_2, 2L_3 L_4, 2M_3 + 2M_4]$                    | trivial                         |
| $[(\blacksquare)^{2T} + \Gamma_6, A_6 A_6, 2H_1 H_2, 2K_1 + 2K_2, L_1 L_2 + L_3 L_4, M_1 + M_2 + M_3 + M_4]$ | 1                               |
| $[(\blacksquare)^{2T} + \Gamma_6, A_6 A_6, 2H_1 H_2, 2K_1 + 2K_2, 2L_1 L_2, 2M_1 + 2M_2]$                    | trivial                         |
| $[(\blacksquare)^{2T} + \Gamma_6, A_6 A_6, H_3 H_3, 2K_3, 2L_3 L_4, 2M_3 + 2M_4]$                            | trivial                         |
| $[(\blacksquare)^{2T} + \Gamma_6, A_6 A_6, H_3 H_3, 2K_3, L_1 L_2 + L_3 L_4, M_1 + M_2 + M_3 + M_4]$         | 1                               |
| $[(\blacksquare)^{2T} + \Gamma_6, A_6 A_6, H_3 H_3, 2K_3, 2L_1 L_2, 2M_1 + 2M_2]$                            | trivial                         |

2nd minimal solution:  $\mu_2^T = 6$  (16 symmetry vectors)

Space group 185 ( $\mathbb{Z}_1$ )

1st minimal solution:  $\mu_1^T = 4$  (2 symmetry vectors)

| $\mathbf{n}^T$                                                                                                        |
|-----------------------------------------------------------------------------------------------------------------------|
| $[(\blacksquare)^{2T} + \Gamma_5, A_5 A_6, H_3 H_3, 2K_3, L_1 L_3 + L_2 L_4, M_1 + M_2 + M_3 + M_4]$                  |
| $[(\blacksquare)^{2T} + \Gamma_5, A_5 A_6, H_1 H_1 + H_2 H_2, 2K_1 + 2K_2, L_1 L_3 + L_2 L_4, M_1 + M_2 + M_3 + M_4]$ |

2nd minimal solution:  $\mu_2^T = 6$  (4 symmetry vectors)

Space group 186 ( $\mathbb{Z}_1$ )

1st minimal solution:  $\mu_1^T = 4$  (3 symmetry vectors)

| $\mathbf{n}^T$                                                                                                        |
|-----------------------------------------------------------------------------------------------------------------------|
| $[(\blacksquare)^{2T} + \Gamma_5, A_5 A_6, 2H_3, 2K_3, L_1 L_4 + L_2 L_3, M_1 + M_2 + M_3 + M_4]$                     |
| $[(\blacksquare)^{2T} + \Gamma_5, A_5 A_6, H_1 H_2 + H_3, K_1 + K_2 + K_3, L_1 L_4 + L_2 L_3, M_1 + M_2 + M_3 + M_4]$ |
| $[(\blacksquare)^{2T} + \Gamma_5, A_5 A_6, 2H_1 H_2, 2K_1 + 2K_2, L_1 L_4 + L_2 L_3, M_1 + M_2 + M_3 + M_4]$          |

2nd minimal solution:  $\mu_2^T = 6$  (8 symmetry vectors)

Space group 187 ( $\mathbb{Z}_1$ )

1st minimal solution:  $\mu_1^T = 2$  (18 symmetry vectors)

| $\mathbf{n}^T$                                                           |
|--------------------------------------------------------------------------|
| $[(\blacksquare)^{2T}, A_6, 2H_6, K_5 + K_6, L_3 + L_4, M_2 + M_3]$      |
| $[(\blacksquare)^{2T}, A_6, H_2 + H_6, K_2 + K_5, L_3 + L_4, M_2 + M_3]$ |
| $[(\blacksquare)^{2T}, A_6, H_4 + H_6, K_4 + K_5, L_3 + L_4, M_2 + M_3]$ |
| $[(\blacksquare)^{2T}, A_6, H_2 + H_6, K_1 + K_6, L_3 + L_4, M_2 + M_3]$ |
| $[(\blacksquare)^{2T}, A_6, 2H_2, K_1 + K_2, L_3 + L_4, M_2 + M_3]$      |
| $[(\blacksquare)^{2T}, A_6, H_2 + H_4, K_1 + K_4, L_3 + L_4, M_2 + M_3]$ |
| $[(\blacksquare)^{2T}, A_6, H_4 + H_6, K_3 + K_6, L_3 + L_4, M_2 + M_3]$ |
| $[(\blacksquare)^{2T}, A_6, H_2 + H_4, K_2 + K_3, L_3 + L_4, M_2 + M_3]$ |
| $[(\blacksquare)^{2T}, A_6, 2H_4, K_3 + K_4, L_3 + L_4, M_2 + M_3]$      |
| $[(\blacksquare)^{2T}, A_5, 2H_5, K_5 + K_6, L_1 + L_2, M_2 + M_3]$      |
| $[(\blacksquare)^{2T}, A_5, H_1 + H_5, K_1 + K_6, L_1 + L_2, M_2 + M_3]$ |
| $[(\blacksquare)^{2T}, A_5, H_3 + H_5, K_3 + K_6, L_1 + L_2, M_2 + M_3]$ |
| $[(\blacksquare)^{2T}, A_5, H_1 + H_5, K_2 + K_5, L_1 + L_2, M_2 + M_3]$ |
| $[(\blacksquare)^{2T}, A_5, 2H_1, K_1 + K_2, L_1 + L_2, M_2 + M_3]$      |
| $[(\blacksquare)^{2T}, A_5, H_3 + H_5, K_4 + K_5, L_1 + L_2, M_2 + M_3]$ |
| $[(\blacksquare)^{2T}, A_5, H_1 + H_3, K_1 + K_4, L_1 + L_2, M_2 + M_3]$ |
| $[(\blacksquare)^{2T}, A_5, H_1 + H_3, K_2 + K_3, L_1 + L_2, M_2 + M_3]$ |
| $[(\blacksquare)^{2T}, A_5, 2H_3, K_3 + K_4, L_1 + L_2, M_2 + M_3]$      |

2nd minimal solution:  $\mu_2^T = 3$  (432 symmetry vectors)

Space group 188 ( $\mathbb{Z}_1$ )

1st minimal solution:  $\mu_1^T = 4$  (18 symmetry vectors)

| $\mathbf{n}^T$                                                                                        |
|-------------------------------------------------------------------------------------------------------|
| $[(\blacksquare)^{2T} + \Gamma_6, A_2A_3, 2H_5H_6, K_5 + 3K_6, 2L_1, M_2 + 2M_3 + M_4]$               |
| $[(\blacksquare)^{2T} + \Gamma_6, A_2A_3, H_1H_2 + H_5H_6, 2K_2 + K_5 + K_6, 2L_1, M_2 + 2M_3 + M_4]$ |
| $[(\blacksquare)^{2T} + \Gamma_6, A_2A_3, H_3H_4 + H_5H_6, 2K_4 + K_5 + K_6, 2L_1, M_2 + 2M_3 + M_4]$ |
| $[(\blacksquare)^{2T} + \Gamma_6, A_2A_3, H_1H_2 + H_5H_6, K_1 + K_2 + 2K_6, 2L_1, M_2 + 2M_3 + M_4]$ |
| $[(\blacksquare)^{2T} + \Gamma_6, A_2A_3, 2H_1H_2, K_1 + 3K_2, 2L_1, M_2 + 2M_3 + M_4]$               |
| $[(\blacksquare)^{2T} + \Gamma_6, A_2A_3, H_1H_2 + H_3H_4, K_1 + K_2 + 2K_4, 2L_1, M_2 + 2M_3 + M_4]$ |
| $[(\blacksquare)^{2T} + \Gamma_6, A_2A_3, H_3H_4 + H_5H_6, K_3 + K_4 + 2K_6, 2L_1, M_2 + 2M_3 + M_4]$ |
| $[(\blacksquare)^{2T} + \Gamma_6, A_2A_3, H_1H_2 + H_3H_4, 2K_2 + K_3 + K_4, 2L_1, M_2 + 2M_3 + M_4]$ |
| $[(\blacksquare)^{2T} + \Gamma_6, A_2A_3, 2H_3H_4, K_3 + 3K_4, 2L_1, M_2 + 2M_3 + M_4]$               |
| $[(\blacksquare)^{2T} + \Gamma_5, A_2A_3, 2H_5H_6, 3K_5 + K_6, 2L_1, M_1 + 2M_2 + M_3]$               |
| $[(\blacksquare)^{2T} + \Gamma_5, A_2A_3, H_1H_2 + H_5H_6, 2K_1 + K_5 + K_6, 2L_1, M_1 + 2M_2 + M_3]$ |
| $[(\blacksquare)^{2T} + \Gamma_5, A_2A_3, H_3H_4 + H_5H_6, 2K_3 + K_5 + K_6, 2L_1, M_1 + 2M_2 + M_3]$ |
| $[(\blacksquare)^{2T} + \Gamma_5, A_2A_3, H_1H_2 + H_5H_6, K_1 + K_2 + 2K_5, 2L_1, M_1 + 2M_2 + M_3]$ |
| $[(\blacksquare)^{2T} + \Gamma_5, A_2A_3, 2H_1H_2, 3K_1 + K_2, 2L_1, M_1 + 2M_2 + M_3]$               |
| $[(\blacksquare)^{2T} + \Gamma_5, A_2A_3, H_3H_4 + H_5H_6, K_3 + K_4 + 2K_5, 2L_1, M_1 + 2M_2 + M_3]$ |
| $[(\blacksquare)^{2T} + \Gamma_5, A_2A_3, H_1H_2 + H_3H_4, 2K_1 + K_3 + K_4, 2L_1, M_1 + 2M_2 + M_3]$ |

... continued on next page

... continued from previous page

---


$$[(\blacksquare)^{2T} + \Gamma_5, A_2 A_3, H_1 H_2 + H_3 H_4, K_1 + K_2 + 2K_3, 2L_1, M_1 + 2M_2 + M_3]$$

$$[(\blacksquare)^{2T} + \Gamma_5, A_2 A_3, 2H_3 H_4, 3K_3 + K_4, 2L_1, M_1 + 2M_2 + M_3]$$


---

2nd minimal solution:  $\mu_2^T = 6$  (200 symmetry vectors)

Space group 189 ( $\mathbb{Z}_1$ )

1st minimal solution:  $\mu_1^T = 2$  (2 symmetry vectors)

---


$$\mathbf{n}^T$$


---


$$[(\blacksquare)^{2T}, A_6, H_2 + H_3, HA_2 + HA_3, K_3 + K_4, KA_3 + KA_4, L_2 + L_3, M_3 + M_4]$$

$$[(\blacksquare)^{2T}, A_5, H_1 + H_4, HA_1 + HA_4, K_3 + K_4, KA_3 + KA_4, L_1 + L_4, M_3 + M_4]$$


---

2nd minimal solution:  $\mu_2^T = 3$  (24 symmetry vectors)

Space group 190 ( $\mathbb{Z}_1$ )

1st minimal solution:  $\mu_1^T = 4$  (6 symmetry vectors)

---


$$\mathbf{n}^T$$


---


$$[(\blacksquare)^{2T} + \Gamma_6, A_1 A_2, 2H_3, 2HA_3, K_2 + 2K_3 + K_4, KA_2 + 2KA_3 + KA_4, 2L_1, M_2 + 2M_3 + M_4]$$

$$[(\blacksquare)^{2T} + \Gamma_6, A_1 A_2, H_2 + H_3, HA_2 + HA_3, K_3 + K_4 + K_6, KA_3 + KA_4 + KA_6, 2L_1, M_2 + 2M_3 + M_4]$$

$$[(\blacksquare)^{2T} + \Gamma_6, A_1 A_2, H_1 + H_3, HA_1 + HA_3, K_3 + K_4 + K_6, KA_3 + KA_4 + KA_6, 2L_1, M_2 + 2M_3 + M_4]$$

$$[(\blacksquare)^{2T} + \Gamma_5, A_1 A_2, 2H_3, 2HA_3, K_1 + K_3 + 2K_4, KA_1 + KA_3 + 2KA_4, 2L_1, M_1 + M_3 + 2M_4]$$

$$[(\blacksquare)^{2T} + \Gamma_5, A_1 A_2, H_2 + H_3, HA_2 + HA_3, K_3 + K_4 + K_5, KA_3 + KA_4 + KA_5, 2L_1, M_1 + M_3 + 2M_4]$$

$$[(\blacksquare)^{2T} + \Gamma_5, A_1 A_2, H_1 + H_3, HA_1 + HA_3, K_3 + K_4 + K_5, KA_3 + KA_4 + KA_5, 2L_1, M_1 + M_3 + 2M_4]$$


---

2nd minimal solution:  $\mu_2^T = 6$  (64 symmetry vectors)

Space group 191 ( $\mathbb{Z}_1$ )

1st minimal solution:  $\mu_1^T = 2$  (2 symmetry vectors)

---


$$\mathbf{n}^T$$


---


$$[(\blacksquare)^{2T}, A_6^-, H_1 + H_4, K_3 + K_4, L_1^+ + L_2^+, M_2^+ + M_2^-]$$

$$[(\blacksquare)^{2T}, A_6^+, H_2 + H_3, K_3 + K_4, L_1^- + L_2^-, M_2^+ + M_2^-]$$


---

2nd minimal solution:  $\mu_2^T = 3$  (64 symmetry vectors)

Space group 192 ( $\mathbb{Z}_2$ )

1st minimal solution:  $\mu_1^T = 4$  (4 symmetry vectors)

| $\mathbf{n}^T$                                                                                                  | $\mathbf{v}^T \in \mathbb{Z}_2$ |
|-----------------------------------------------------------------------------------------------------------------|---------------------------------|
| $[(\blacksquare)^{2T} + \Gamma_6^-, A_3 A_4, 2H_3, K_1 + K_3 + 2K_4, L_1 + L_2, M_2^+ + M_2^- + M_3^- + M_4^-]$ | 1                               |
| $[(\blacksquare)^{2T} + \Gamma_6^-, A_3 A_4, 2H_3, K_1 + K_3 + 2K_4, 2L_1, M_1^+ + 2M_2^+ + M_2^-]$             | trivial                         |
| $[(\blacksquare)^{2T} + \Gamma_6^+, A_3 A_4, 2H_3, K_2 + 2K_3 + K_4, L_1 + L_2, M_2^+ + M_2^- + M_3^+ + M_4^+]$ | 1                               |
| $[(\blacksquare)^{2T} + \Gamma_6^+, A_3 A_4, 2H_3, K_2 + 2K_3 + K_4, 2L_1, M_1^- + M_2^+ + 2M_2^-]$             | trivial                         |

2nd minimal solution:  $\mu_2^T = 6$  (112 symmetry vectors)

Space group 193 ( $\mathbb{Z}_1$ )

1st minimal solution:  $\mu_1^T = 4$  (2 symmetry vectors)

| $\mathbf{n}^T$                                                                                                           |
|--------------------------------------------------------------------------------------------------------------------------|
| $[(\blacksquare)^{2T} + \Gamma_5^+, A_3, H_1 H_3 + H_2 H_4, K_1 + K_3 + 2K_4, L_1 + L_2, M_2^+ + M_2^- + M_3^- + M_4^-]$ |
| $[(\blacksquare)^{2T} + \Gamma_5^-, A_3, H_1 H_3 + H_2 H_4, K_2 + 2K_3 + K_4, L_1 + L_2, M_2^+ + M_2^- + M_3^+ + M_4^+]$ |

2nd minimal solution:  $\mu_2^T = 6$  (36 symmetry vectors)

Space group 194 ( $\mathbb{Z}_1$ )

1st minimal solution:  $\mu_1^T = 4$  (6 symmetry vectors)

| $\mathbf{n}^T$                                                                                                  |
|-----------------------------------------------------------------------------------------------------------------|
| $[(\blacksquare)^{2T} + \Gamma_5^+, A_3, 2H_3, K_1 + K_3 + 2K_4, L_1 + L_2, M_2^+ + M_2^- + M_3^- + M_4^-]$     |
| $[(\blacksquare)^{2T} + \Gamma_5^+, A_3, H_2 + H_3, K_3 + K_4 + K_5, L_1 + L_2, M_2^+ + M_2^- + M_3^- + M_4^-]$ |
| $[(\blacksquare)^{2T} + \Gamma_5^+, A_3, H_1 + H_3, K_3 + K_4 + K_5, L_1 + L_2, M_2^+ + M_2^- + M_3^- + M_4^-]$ |
| $[(\blacksquare)^{2T} + \Gamma_5^-, A_3, 2H_3, K_2 + 2K_3 + K_4, L_1 + L_2, M_2^+ + M_2^- + M_3^+ + M_4^+]$     |
| $[(\blacksquare)^{2T} + \Gamma_5^-, A_3, H_2 + H_3, K_3 + K_4 + K_6, L_1 + L_2, M_2^+ + M_2^- + M_3^+ + M_4^+]$ |
| $[(\blacksquare)^{2T} + \Gamma_5^-, A_3, H_1 + H_3, K_3 + K_4 + K_6, L_1 + L_2, M_2^+ + M_2^- + M_3^+ + M_4^+]$ |

2nd minimal solution:  $\mu_2^T = 6$  (174 symmetry vectors)

Space group 195 ( $\mathbb{Z}_1$ )

1st minimal solution:  $\mu_1^T = 2$  (1 symmetry vector)

| $\mathbf{n}^T$                                         |
|--------------------------------------------------------|
| $[(\blacksquare)^{2T}, R_2 R_3, M_1 + M_2, X_2 + X_3]$ |

2nd minimal solution:  $\mu_2^T = 3$  (8 symmetry vectors)

Space group 196 ( $\mathbb{Z}_1$ )

1st minimal solution:  $\mu_1^T = 2$  (1 symmetry vector)

$$\frac{\mathbf{n}^T}{[(\blacksquare)^{2T}, X_2 + X_3, L_2 L_3, W_1 + W_2]}$$

2nd minimal solution:  $\mu_2^T = 3$  (2 symmetry vectors)

Space group 197 ( $\mathbb{Z}_1$ )

1st minimal solution:  $\mu_1^T = 3$  (2 symmetry vectors)

$$\frac{\mathbf{n}^T}{[(\blacksquare)^{2T} + \Gamma_1, H_4, P_4, PA_4, N_1 + 2N_2] \\ [(\blacksquare)^{2T} + \Gamma_1, H_4, P_1 + P_2 + P_3, PA_1 + PA_2 + PA_3, 3N_1]}$$

2nd minimal solution:  $\mu_2^T = 4$  (2 symmetry vectors)

Space group 198 ( $\mathbb{Z}_1$ )

1st minimal solution:  $\mu_1^T = 4$  (2 symmetry vectors)

$$\frac{\mathbf{n}^T}{[(\blacksquare)^{2T} + \Gamma_2 \Gamma_3, R_2 R_2, M_1 M_2 + M_3 M_4, 2X_1] \\ [(\blacksquare)^{2T} + 2\Gamma_1, R_1 R_3, M_1 M_2 + M_3 M_4, 2X_1]}$$

2nd minimal solution:  $\mu_2^T = 8$  (2 symmetry vectors)

Space group 199 ( $\mathbb{Z}_1$ )

1st minimal solution:  $\mu_1^T = 2$  (1 symmetry vector)

$$\frac{\mathbf{n}^T}{[(\blacksquare)^{2T}, H_2 H_3, P_2, PA_2, N_1 + N_2]}$$

2nd minimal solution:  $\mu_2^T = 4$  (1 symmetry vector)

Space group 200 ( $\mathbb{Z}_1$ )

1st minimal solution:  $\mu_1^T = 2$  (2 symmetry vectors)

| $\mathbf{n}^T$                                                     |
|--------------------------------------------------------------------|
| $[(\blacksquare)^{2T}, R_2^- R_3^-, M_1^- + M_2^+, X_2^+ + X_3^+]$ |
| $[(\blacksquare)^{2T}, R_2^+ R_3^+, M_1^+ + M_2^-, X_2^- + X_3^-]$ |

2nd minimal solution:  $\mu_2^T = 3$  (20 symmetry vectors)

Space group 201 ( $\mathbb{Z}_2$ )

1st minimal solution:  $\mu_1^T = 4$  (4 symmetry vectors)

| $\mathbf{n}^T$                                                                           | $\mathbf{v}^T \in \mathbb{Z}_2$ |
|------------------------------------------------------------------------------------------|---------------------------------|
| $[(\blacksquare)^{2T} + \Gamma_1^+ + \Gamma_1^-, 2R_1^- + R_2^+ R_3^+, 2M_1, X_1 + X_2]$ | 1                               |
| $[(\blacksquare)^{2T} + \Gamma_1^+ + \Gamma_1^-, R_1^- + R_4^-, M_1 + M_2, X_1 + X_2]$   | trivial                         |
| $[(\blacksquare)^{2T} + \Gamma_1^+ + \Gamma_1^-, R_1^+ + R_4^+, M_1 + M_2, X_1 + X_2]$   | trivial                         |
| $[(\blacksquare)^{2T} + \Gamma_1^+ + \Gamma_1^-, 2R_1^+ + R_2^- R_3^-, 2M_1, X_1 + X_2]$ | 1                               |

2nd minimal solution:  $\mu_2^T = 6$  (20 symmetry vectors)

Space group 202 ( $\mathbb{Z}_1$ )

1st minimal solution:  $\mu_1^T = 3$  (8 symmetry vectors)

| $\mathbf{n}^T$                                                                                    |
|---------------------------------------------------------------------------------------------------|
| $[(\blacksquare)^{2T} + \Gamma_1^+, X_2^- + X_3^- + X_4^-, L_1^- + L_2^- L_3^-, W_1 + W_3 + W_4]$ |
| $[(\blacksquare)^{2T} + \Gamma_1^+, X_2^- + X_3^- + X_4^-, L_1^+ + L_2^- L_3^-, W_1 + W_3 + W_4]$ |
| $[(\blacksquare)^{2T} + \Gamma_1^+, X_2^- + X_3^- + X_4^-, L_1^- + L_2^+ L_3^+, W_1 + W_3 + W_4]$ |
| $[(\blacksquare)^{2T} + \Gamma_1^+, X_2^- + X_3^- + X_4^-, L_1^+ + L_2^+ L_3^+, W_1 + W_3 + W_4]$ |
| $[(\blacksquare)^{2T} + \Gamma_1^-, X_2^+ + X_3^+ + X_4^+, L_1^- + L_2^- L_3^-, W_2 + W_3 + W_4]$ |
| $[(\blacksquare)^{2T} + \Gamma_1^-, X_2^+ + X_3^+ + X_4^+, L_1^- + L_2^+ L_3^+, W_2 + W_3 + W_4]$ |
| $[(\blacksquare)^{2T} + \Gamma_1^-, X_2^+ + X_3^+ + X_4^+, L_1^+ + L_2^- L_3^-, W_2 + W_3 + W_4]$ |
| $[(\blacksquare)^{2T} + \Gamma_1^-, X_2^+ + X_3^+ + X_4^+, L_1^+ + L_2^+ L_3^+, W_2 + W_3 + W_4]$ |

2nd minimal solution:  $\mu_2^T = 4$  (30 symmetry vectors)

Space group 203 ( $\mathbb{Z}_2$ )

1st minimal solution:  $\mu_1^T = 2$  (2 symmetry vectors)

| $\mathbf{n}^T$                                 | $\mathbf{v}^T \in \mathbb{Z}_2$ |
|------------------------------------------------|---------------------------------|
| $[(\blacksquare)^{2T}, X_2, L_2^+ L_3^+, W_1]$ | trivial                         |
| $[(\blacksquare)^{2T}, X_2, L_2^- L_3^-, W_1]$ | trivial                         |

2nd minimal solution:  $\mu_2^T = 4$  (6 symmetry vectors)



Space group 204 ( $\mathbb{Z}_1$ )

1st minimal solution:  $\mu_1^T = 3$  (6 symmetry vectors)

| $\mathbf{n}^T$                                                            |
|---------------------------------------------------------------------------|
| $[(\blacksquare)^{2T} + \Gamma_1^+, H_4^-, P_4, N_1^- + 2N_2^-]$          |
| $[(\blacksquare)^{2T} + \Gamma_1^+, H_4^-, P_4, N_1^+ + N_2^+ + N_2^-]$   |
| $[(\blacksquare)^{2T} + \Gamma_1^+, H_4^-, P_1 + P_2P_3, 2N_1^+ + N_1^-]$ |
| $[(\blacksquare)^{2T} + \Gamma_1^-, H_4^+, P_4, N_1^- + N_2^+ + N_2^-]$   |
| $[(\blacksquare)^{2T} + \Gamma_1^-, H_4^+, P_4, N_1^+ + 2N_2^+]$          |
| $[(\blacksquare)^{2T} + \Gamma_1^-, H_4^+, P_1 + P_2P_3, N_1^+ + 2N_1^-]$ |

2nd minimal solution:  $\mu_2^T = 4$  (14 symmetry vectors)

Space group 205 ( $\mathbb{Z}_1$ )

1st minimal solution:  $\mu_1^T = 4$  (2 symmetry vectors)

| $\mathbf{n}^T$                                                                     |
|------------------------------------------------------------------------------------|
| $[(\blacksquare)^{2T} + \Gamma_1^+ + \Gamma_1^-, R_1^- R_3^-, M_1 M_2, X_1 + X_2]$ |
| $[(\blacksquare)^{2T} + \Gamma_1^+ + \Gamma_1^-, R_1^+ R_3^+, M_1 M_2, X_1 + X_2]$ |

2nd minimal solution:  $\mu_2^T = 8$  (14 symmetry vectors)

Space group 206 ( $\mathbb{Z}_1$ )

1st minimal solution:  $\mu_1^T = 4$  (2 symmetry vectors)

| $\mathbf{n}^T$                                                                  |
|---------------------------------------------------------------------------------|
| $[(\blacksquare)^{2T} + \Gamma_1^+ + \Gamma_1^-, H_1^- + H_4^-, P_1 P_3, 2N_1]$ |
| $[(\blacksquare)^{2T} + \Gamma_1^+ + \Gamma_1^-, H_1^+ + H_4^+, P_1 P_3, 2N_1]$ |

2nd minimal solution:  $\mu_2^T = 8$  (12 symmetry vectors)

Space group 207 ( $\mathbb{Z}_1$ )

1st minimal solution:  $\mu_1^T = 2$  (1 symmetry vector)

| $\mathbf{n}^T$                               |
|----------------------------------------------|
| $[(\blacksquare)^{2T}, R_3, M_2 + M_3, X_5]$ |

2nd minimal solution:  $\mu_2^T = 3$  (6 symmetry vectors)

Space group 208 ( $\mathbb{Z}_1$ )

1st minimal solution:  $\mu_1^T = 4$  (2 symmetry vectors)

| $\mathbf{n}^T$                                                                             |
|--------------------------------------------------------------------------------------------|
| $[(\blacksquare)^{2T} + \Gamma_1 + \Gamma_2, R_1 + R_5, M_1 + M_4 + M_5, X_2 + X_3 + X_5]$ |
| $[(\blacksquare)^{2T} + \Gamma_1 + \Gamma_2, R_2 + R_4, M_1 + M_4 + M_5, X_1 + X_4 + X_5]$ |

2nd minimal solution:  $\mu_2^T = 6$  (15 symmetry vectors)

Space group 209 ( $\mathbb{Z}_1$ )

1st minimal solution:  $\mu_1^T = 3$  (2 symmetry vectors)

| $\mathbf{n}^T$                                                         |
|------------------------------------------------------------------------|
| $[(\blacksquare)^{2T} + \Gamma_1, X_3 + X_5, L_2 + L_3, W_2 + W_3W_4]$ |
| $[(\blacksquare)^{2T} + \Gamma_1, X_3 + X_5, L_1 + L_3, W_1 + W_3W_4]$ |

2nd minimal solution:  $\mu_2^T = 4$  (7 symmetry vectors)

Space group 210 ( $\mathbb{Z}_1$ )

1st minimal solution:  $\mu_1^T = 2$  (1 symmetry vector)

| $\mathbf{n}^T$                               |
|----------------------------------------------|
| $[(\blacksquare)^{2T}, X_1 + X_4, L_3, W_1]$ |

2nd minimal solution:  $\mu_2^T = 4$  (2 symmetry vectors)

Space group 211 ( $\mathbb{Z}_1$ )

1st minimal solution:  $\mu_1^T = 3$  (3 symmetry vectors)

| $\mathbf{n}^T$                                                       |
|----------------------------------------------------------------------|
| $[(\blacksquare)^{2T} + \Gamma_1, H_4, P_4, N_2 + N_3 + N_4]$        |
| $[(\blacksquare)^{2T} + \Gamma_1, H_4, P_1 + P_2 + P_3, N_1 + 2N_2]$ |
| $[(\blacksquare)^{2T} + \Gamma_2, H_5, P_4, N_2 + 2N_4]$             |

2nd minimal solution:  $\mu_2^T = 4$  (6 symmetry vectors)

Space group 212 ( $\mathbb{Z}_1$ )

1st minimal solution:  $\mu_1^T = 4$  (2 symmetry vectors)

|                                                                              |
|------------------------------------------------------------------------------|
| $\mathbf{n}^T$                                                               |
| $[(\blacksquare)^{2T} + \Gamma_3, R_1 R_2, M_2 M_3 + M_5, X_1 + X_2]$        |
| $[(\blacksquare)^{2T} + \Gamma_1 + \Gamma_2, R_3, M_2 M_3 + M_5, X_1 + X_2]$ |

2nd minimal solution:  $\mu_2^T = 8$  (4 symmetry vectors)

Space group 213 ( $\mathbb{Z}_1$ )

1st minimal solution:  $\mu_1^T = 4$  (2 symmetry vectors)

|                                                                              |
|------------------------------------------------------------------------------|
| $\mathbf{n}^T$                                                               |
| $[(\blacksquare)^{2T} + \Gamma_3, R_1 R_2, M_2 M_3 + M_5, X_1 + X_2]$        |
| $[(\blacksquare)^{2T} + \Gamma_1 + \Gamma_2, R_3, M_2 M_3 + M_5, X_1 + X_2]$ |

2nd minimal solution:  $\mu_2^T = 8$  (4 symmetry vectors)

Space group 214 ( $\mathbb{Z}_1$ )

1st minimal solution:  $\mu_1^T = 2$  (1 symmetry vector)

|                                              |
|----------------------------------------------|
| $\mathbf{n}^T$                               |
| $[(\blacksquare)^{2T}, H_3, P_2, N_2 + N_4]$ |

2nd minimal solution:  $\mu_2^T = 4$  (2 symmetry vectors)

Space group 215 ( $\mathbb{Z}_1$ )

1st minimal solution:  $\mu_1^T = 2$  (2 symmetry vectors)

|                                              |
|----------------------------------------------|
| $\mathbf{n}^T$                               |
| $[(\blacksquare)^{2T}, R_3, M_1 + M_4, X_5]$ |
| $[(\blacksquare)^{2T}, R_3, M_2 + M_3, X_5]$ |

2nd minimal solution:  $\mu_2^T = 3$  (12 symmetry vectors)

Space group 216 ( $\mathbb{Z}_1$ )

1st minimal solution:  $\mu_1^T = 2$  (4 symmetry vectors)

| $\mathbf{n}^T$                               |
|----------------------------------------------|
| $[(\blacksquare)^{2T}, X_5, L_3, W_2 + W_4]$ |
| $[(\blacksquare)^{2T}, X_5, L_3, W_2 + W_3]$ |
| $[(\blacksquare)^{2T}, X_5, L_3, W_1 + W_4]$ |
| $[(\blacksquare)^{2T}, X_5, L_3, W_1 + W_3]$ |

2nd minimal solution:  $\mu_2^T = 3$  (24 symmetry vectors)

Space group 217 ( $\mathbb{Z}_1$ )

1st minimal solution:  $\mu_1^T = 3$  (4 symmetry vectors)

| $\mathbf{n}^T$                                                              |
|-----------------------------------------------------------------------------|
| $[(\blacksquare)^{2T} + \Gamma_1, H_4, P_4, PA_4, N_1 + N_3 + N_4]$         |
| $[(\blacksquare)^{2T} + \Gamma_1, H_4, P_1 + P_3, PA_1 + PA_3, 2N_1 + N_2]$ |
| $[(\blacksquare)^{2T} + \Gamma_2, H_5, P_5, PA_5, N_2 + N_3 + N_4]$         |
| $[(\blacksquare)^{2T} + \Gamma_2, H_5, P_2 + P_3, PA_2 + PA_3, N_1 + 2N_2]$ |

2nd minimal solution:  $\mu_2^T = 4$  (10 symmetry vectors)

Space group 218 ( $\mathbb{Z}_1$ )

1st minimal solution:  $\mu_1^T = 6$  (16 symmetry vectors)

| $\mathbf{n}^T$                                                                                               |
|--------------------------------------------------------------------------------------------------------------|
| $[(\blacksquare)^{2T} + \Gamma_1 + \Gamma_2 + \Gamma_3, R_4 R_5, M_1 + 2M_2 + M_3 + M_5, X_3 X_4 + 2X_5]$    |
| $[(\blacksquare)^{2T} + \Gamma_1 + \Gamma_2 + \Gamma_3, R_4 R_5, 2M_1 + M_2 + M_4 + M_5, X_3 X_4 + 2X_5]$    |
| $[(\blacksquare)^{2T} + \Gamma_1 + \Gamma_5, R_4 R_5, 2M_1 + 2M_2 + M_5, 2X_3 X_4 + X_5]$                    |
| $[(\blacksquare)^{2T} + \Gamma_2 + \Gamma_4, R_4 R_5, 2M_1 + 2M_2 + M_5, 2X_3 X_4 + X_5]$                    |
| $[(\blacksquare)^{2T} + \Gamma_1 + \Gamma_2 + \Gamma_3, R_4 R_5, M_2 + 2M_3 + M_4 + M_5, X_1 X_2 + 2X_5]$    |
| $[(\blacksquare)^{2T} + \Gamma_1 + \Gamma_2 + \Gamma_3, R_4 R_5, M_1 + M_3 + 2M_4 + M_5, X_1 X_2 + 2X_5]$    |
| $[(\blacksquare)^{2T} + \Gamma_1 + \Gamma_5, R_4 R_5, 2M_2 + 2M_3 + M_5, X_1 X_2 + X_3 X_4 + X_5]$           |
| $[(\blacksquare)^{2T} + \Gamma_1 + \Gamma_5, R_4 R_5, M_1 + M_2 + M_3 + M_4 + M_5, X_1 X_2 + X_3 X_4 + X_5]$ |
| $[(\blacksquare)^{2T} + \Gamma_1 + \Gamma_5, R_4 R_5, 2M_1 + 2M_4 + M_5, X_1 X_2 + X_3 X_4 + X_5]$           |
| $[(\blacksquare)^{2T} + \Gamma_2 + \Gamma_4, R_4 R_5, 2M_2 + 2M_3 + M_5, X_1 X_2 + X_3 X_4 + X_5]$           |
| $[(\blacksquare)^{2T} + \Gamma_2 + \Gamma_4, R_4 R_5, M_1 + M_2 + M_3 + M_4 + M_5, X_1 X_2 + X_3 X_4 + X_5]$ |
| $[(\blacksquare)^{2T} + \Gamma_2 + \Gamma_4, R_4 R_5, 2M_1 + 2M_4 + M_5, X_1 X_2 + X_3 X_4 + X_5]$           |
| $[(\blacksquare)^{2T} + \Gamma_1 + \Gamma_5, R_4 R_5, 2M_3 + 2M_4 + M_5, 2X_1 X_2 + X_5]$                    |
| $[(\blacksquare)^{2T} + \Gamma_2 + \Gamma_4, R_4 R_5, 2M_3 + 2M_4 + M_5, 2X_1 X_2 + X_5]$                    |
| $[(\blacksquare)^{2T} + \Gamma_1 + \Gamma_5, R_1 R_2 + R_3 R_3, 3M_5, X_1 X_2 + X_3 X_4 + X_5]$              |
| $[(\blacksquare)^{2T} + \Gamma_2 + \Gamma_4, R_1 R_2 + R_3 R_3, 3M_5, X_1 X_2 + X_3 X_4 + X_5]$              |

2nd minimal solution:  $\mu_2^T = 8$  (16 symmetry vectors)

Space group 219 ( $\mathbb{Z}_1$ )

1st minimal solution:  $\mu_1^T = 4$  (2 symmetry vectors)

| $\mathbf{n}^T$                                                                  |
|---------------------------------------------------------------------------------|
| $[(\blacksquare)^{2T} + \Gamma_3, X_1 + X_4 + X_5, L_3 L_3, W_1 W_2 + W_3 W_4]$ |
| $[(\blacksquare)^{2T} + \Gamma_3, X_2 + X_3 + X_5, L_3 L_3, W_1 W_2 + W_3 W_4]$ |

2nd minimal solution:  $\mu_2^T = 6$  (8 symmetry vectors)

Space group 220 ( $\mathbb{Z}_1$ )

1st minimal solution:  $\mu_1^T = 6$  (2 symmetry vectors)

| $\mathbf{n}^T$                                                                                  |
|-------------------------------------------------------------------------------------------------|
| $[(\blacksquare)^{2T} + \Gamma_1 + \Gamma_2 + \Gamma_3, H_4 H_5, P_1 + P_3, PA_1 + PA_3, 3N_1]$ |
| $[(\blacksquare)^{2T} + \Gamma_1 + \Gamma_2 + \Gamma_3, H_4 H_5, P_2 + P_3, PA_2 + PA_3, 3N_1]$ |

2nd minimal solution:  $\mu_2^T = 8$  (2 symmetry vectors)

Space group 221 ( $\mathbb{Z}_1$ )

1st minimal solution:  $\mu_1^T = 2$  (2 symmetry vectors)

| $\mathbf{n}^T$                                       |
|------------------------------------------------------|
| $[(\blacksquare)^{2T}, R_3^-, M_2^- + M_3^+, X_5^+]$ |
| $[(\blacksquare)^{2T}, R_3^+, M_2^+ + M_3^-, X_5^-]$ |

2nd minimal solution:  $\mu_2^T = 3$  (20 symmetry vectors)

Space group 222 ( $\mathbb{Z}_1$ )

1st minimal solution:  $\mu_1^T = 6$  (8 symmetry vectors)

| $\mathbf{n}^T$                                                                              |
|---------------------------------------------------------------------------------------------|
| $[(\blacksquare)^{2T} + \Gamma_1^- + \Gamma_4^-, R_4, M_2 + M_3 + M_4, X_2 + X_3 X_4]$      |
| $[(\blacksquare)^{2T} + \Gamma_2^- + \Gamma_5^-, R_4, M_2 + M_3 + M_4, X_1 + X_3 X_4]$      |
| $[(\blacksquare)^{2T} + \Gamma_1^+ + \Gamma_4^+, R_4, M_2 + M_3 + M_4, X_2 + X_3 X_4]$      |
| $[(\blacksquare)^{2T} + \Gamma_1^- + \Gamma_4^-, R_1 + R_2 R_3, M_1 + 2M_2, X_2 + X_3 X_4]$ |
| $[(\blacksquare)^{2T} + \Gamma_2^- + \Gamma_5^-, R_1 + R_2 R_3, M_1 + 2M_2, X_1 + X_3 X_4]$ |
| $[(\blacksquare)^{2T} + \Gamma_1^+ + \Gamma_4^+, R_1 + R_2 R_3, M_1 + 2M_2, X_2 + X_3 X_4]$ |
| $[(\blacksquare)^{2T} + \Gamma_2^+ + \Gamma_5^+, R_4, M_2 + M_3 + M_4, X_1 + X_3 X_4]$      |
| $[(\blacksquare)^{2T} + \Gamma_2^+ + \Gamma_5^+, R_1 + R_2 R_3, M_1 + 2M_2, X_1 + X_3 X_4]$ |

2nd minimal solution:  $\mu_2^T = 8$  (16 symmetry vectors)

Space group 223 ( $\mathbb{Z}_1$ )

1st minimal solution:  $\mu_1^T = 6$  (26 symmetry vectors)

| $\mathbf{n}^T$                                                                                                              |
|-----------------------------------------------------------------------------------------------------------------------------|
| $[(\blacksquare)^{2T} + \Gamma_1^+ + \Gamma_2^+ + \Gamma_3^+, R_4, M_2^- + M_3^+ + M_3^- + M_4^- + M_5^+, 2X_1 + X_3]$      |
| $[(\blacksquare)^{2T} + \Gamma_1^- + \Gamma_2^- + \Gamma_3^+, R_4, M_2^- + M_3^+ + M_3^- + M_4^- + M_5^-, X_1 + X_2 + X_3]$ |
| $[(\blacksquare)^{2T} + \Gamma_1^+ + \Gamma_2^+ + \Gamma_3^+, R_4, M_1^- + M_2^+ + M_2^- + M_3^- + M_5^+, 2X_1 + X_4]$      |
| $[(\blacksquare)^{2T} + \Gamma_1^- + \Gamma_2^- + \Gamma_3^+, R_4, M_1^- + M_2^+ + M_2^- + M_3^- + M_5^-, X_1 + X_2 + X_4]$ |
| $[(\blacksquare)^{2T} + \Gamma_1^+ + \Gamma_5^-, R_4, M_3^+ + M_3^- + M_4^+ + M_4^- + M_5^+, X_1 + 2X_3]$                   |
| $[(\blacksquare)^{2T} + \Gamma_1^+ + \Gamma_5^-, R_4, M_1^- + M_2^+ + M_3^- + M_4^+ + M_5^+, X_1 + X_3 + X_4]$              |
| $[(\blacksquare)^{2T} + \Gamma_2^+ + \Gamma_4^-, R_4, M_2^+ + M_2^- + M_3^+ + M_3^- + M_5^+, X_1 + X_3 + X_4]$              |
| $[(\blacksquare)^{2T} + \Gamma_1^+ + \Gamma_5^-, R_4, M_1^- + M_2^- + M_3^- + M_4^- + M_5^-, X_1 + X_3 + X_4]$              |
| $[(\blacksquare)^{2T} + \Gamma_2^- + \Gamma_4^+, R_4, M_2^+ + M_2^- + M_3^+ + M_3^- + M_5^-, X_2 + X_3 + X_4]$              |
| $[(\blacksquare)^{2T} + \Gamma_1^+ + \Gamma_5^-, R_4, M_1^+ + M_2^- + M_3^+ + M_4^- + M_5^+, X_1 + X_3 + X_4]$              |
| $[(\blacksquare)^{2T} + \Gamma_1^+ + \Gamma_5^-, R_4, M_1^+ + M_1^- + M_2^+ + M_2^- + M_5^+, X_1 + 2X_4]$                   |
| $[(\blacksquare)^{2T} + \Gamma_1^+ + \Gamma_2^+ + \Gamma_3^-, R_4, M_2^+ + M_3^+ + M_3^- + M_4^+ + M_5^+, X_1 + X_2 + X_3]$ |
| $[(\blacksquare)^{2T} + \Gamma_1^- + \Gamma_2^- + \Gamma_3^-, R_4, M_2^+ + M_3^+ + M_3^- + M_4^+ + M_5^-, 2X_2 + X_3]$      |
| $[(\blacksquare)^{2T} + \Gamma_1^+ + \Gamma_2^+ + \Gamma_3^-, R_4, M_2^- + M_3^+ + M_3^- + M_4^- + M_5^-, X_1 + X_2 + X_3]$ |
| $[(\blacksquare)^{2T} + \Gamma_1^+ + \Gamma_2^+ + \Gamma_3^-, R_4, M_1^- + M_2^+ + M_2^- + M_3^- + M_5^-, X_1 + X_2 + X_4]$ |
| $[(\blacksquare)^{2T} + \Gamma_1^+ + \Gamma_2^+ + \Gamma_3^-, R_4, M_1^+ + M_2^+ + M_2^- + M_3^+ + M_5^+, X_1 + X_2 + X_4]$ |
| $[(\blacksquare)^{2T} + \Gamma_1^- + \Gamma_2^- + \Gamma_3^-, R_4, M_1^+ + M_2^+ + M_2^- + M_3^+ + M_5^-, 2X_2 + X_4]$      |
| $[(\blacksquare)^{2T} + \Gamma_1^+ + \Gamma_5^-, R_1 + R_2R_3, 2M_5^+ + M_5^-, X_1 + X_3 + X_4]$                            |
| $[(\blacksquare)^{2T} + \Gamma_1^- + \Gamma_2^- + \Gamma_3^+, R_4, M_2^+ + M_3^+ + M_3^- + M_4^+ + M_5^+, X_1 + X_2 + X_3]$ |
| $[(\blacksquare)^{2T} + \Gamma_1^- + \Gamma_5^+, R_4, M_3^+ + M_3^- + M_4^+ + M_4^- + M_5^-, X_2 + 2X_3]$                   |
| $[(\blacksquare)^{2T} + \Gamma_1^- + \Gamma_5^+, R_4, M_1^- + M_2^+ + M_3^- + M_4^+ + M_5^-, X_2 + X_3 + X_4]$              |
| $[(\blacksquare)^{2T} + \Gamma_1^- + \Gamma_2^- + \Gamma_3^+, R_4, M_1^+ + M_2^+ + M_2^- + M_3^+ + M_5^+, X_1 + X_2 + X_4]$ |
| $[(\blacksquare)^{2T} + \Gamma_1^- + \Gamma_5^+, R_4, M_1^+ + M_2^+ + M_3^+ + M_4^+ + M_5^+, X_2 + X_3 + X_4]$              |
| $[(\blacksquare)^{2T} + \Gamma_1^- + \Gamma_5^+, R_4, M_1^+ + M_2^- + M_3^+ + M_4^- + M_5^-, X_2 + X_3 + X_4]$              |
| $[(\blacksquare)^{2T} + \Gamma_1^- + \Gamma_5^+, R_4, M_1^+ + M_1^- + M_2^+ + M_2^- + M_5^-, X_2 + 2X_4]$                   |
| $[(\blacksquare)^{2T} + \Gamma_1^- + \Gamma_5^+, R_1 + R_2R_3, M_5^+ + 2M_5^-, X_2 + X_3 + X_4]$                            |

2nd minimal solution:  $\mu_2^T = 8$  (50 symmetry vectors)

Space group 224 ( $\mathbb{Z}_1$ )

1st minimal solution:  $\mu_1^T = 4$  (4 symmetry vectors)

| $\mathbf{n}^T$                                                                         |
|----------------------------------------------------------------------------------------|
| $[(\blacksquare)^{2T} + \Gamma_1^+ + \Gamma_2^-, R_2^- + R_4^-, M_1 + M_4, X_1 + X_3]$ |
| $[(\blacksquare)^{2T} + \Gamma_1^+ + \Gamma_2^-, R_1^+ + R_5^+, M_1 + M_4, X_1 + X_4]$ |
| $[(\blacksquare)^{2T} + \Gamma_1^- + \Gamma_2^+, R_2^+ + R_4^+, M_2 + M_4, X_2 + X_3]$ |
| $[(\blacksquare)^{2T} + \Gamma_1^- + \Gamma_2^+, R_1^- + R_5^-, M_2 + M_4, X_2 + X_4]$ |

2nd minimal solution:  $\mu_2^T = 6$  (22 symmetry vectors)

Space group 225 ( $\mathbb{Z}_1$ )

1st minimal solution:  $\mu_1^T = 3$  (8 symmetry vectors)

| $\mathbf{n}^T$                                                                |
|-------------------------------------------------------------------------------|
| $[(\blacksquare)^{2T} + \Gamma_1^+, X_3^- + X_5^-, L_2^- + L_3^-, W_2 + W_5]$ |
| $[(\blacksquare)^{2T} + \Gamma_1^+, X_3^- + X_5^-, L_1^+ + L_3^-, W_1 + W_5]$ |
| $[(\blacksquare)^{2T} + \Gamma_1^+, X_3^- + X_5^-, L_2^- + L_3^+, W_2 + W_5]$ |
| $[(\blacksquare)^{2T} + \Gamma_1^+, X_3^- + X_5^-, L_1^+ + L_3^+, W_1 + W_5]$ |
| $[(\blacksquare)^{2T} + \Gamma_1^-, X_3^+ + X_5^+, L_2^+ + L_3^-, W_3 + W_5]$ |
| $[(\blacksquare)^{2T} + \Gamma_1^-, X_3^+ + X_5^+, L_2^+ + L_3^+, W_3 + W_5]$ |
| $[(\blacksquare)^{2T} + \Gamma_1^-, X_3^+ + X_5^+, L_1^- + L_3^-, W_4 + W_5]$ |
| $[(\blacksquare)^{2T} + \Gamma_1^-, X_3^+ + X_5^+, L_1^- + L_3^+, W_4 + W_5]$ |

2nd minimal solution:  $\mu_2^T = 4$  (74 symmetry vectors)

Space group 226 ( $\mathbb{Z}_1$ )

1st minimal solution:  $\mu_1^T = 4$  (2 symmetry vectors)

| $\mathbf{n}^T$                                                                      |
|-------------------------------------------------------------------------------------|
| $[(\blacksquare)^{2T} + \Gamma_3^-, X_2^- + X_3^+ + X_5^+, L_1 L_2, W_3 W_4 + W_5]$ |
| $[(\blacksquare)^{2T} + \Gamma_3^+, X_2^+ + X_3^- + X_5^-, L_1 L_2, W_1 W_2 + W_5]$ |

2nd minimal solution:  $\mu_2^T = 6$  (14 symmetry vectors)

Space group 227 ( $\mathbb{Z}_1$ )

1st minimal solution:  $\mu_1^T = 2$  (4 symmetry vectors)

| $\mathbf{n}^T$                           |
|------------------------------------------|
| $[(\blacksquare)^{2T}, X_4, L_3^-, W_1]$ |
| $[(\blacksquare)^{2T}, X_4, L_3^+, W_1]$ |
| $[(\blacksquare)^{2T}, X_4, L_3^-, W_2]$ |
| $[(\blacksquare)^{2T}, X_4, L_3^+, W_2]$ |

2nd minimal solution:  $\mu_2^T = 4$  (12 symmetry vectors)

Space group 228 ( $\mathbb{Z}_1$ )

1st minimal solution:  $\mu_1^T = 8$  (4 symmetry vectors)

| $\mathbf{n}^T$                                                                                                               |
|------------------------------------------------------------------------------------------------------------------------------|
| $[(\blacksquare)^{2T} + \Gamma_1^+ + \Gamma_1^- + \Gamma_2^- + \Gamma_5^-, X_1 + X_2 + X_3 + X_4, L_1 L_2 + 2L_3, 2W_1 W_2]$ |
| $[(\blacksquare)^{2T} + \Gamma_1^+ + \Gamma_2^+ + \Gamma_2^- + \Gamma_4^+, X_1 + X_2 + 2X_4, L_1 L_2 + 2L_3, 2W_1 W_2]$      |
| $[(\blacksquare)^{2T} + \Gamma_1^- + \Gamma_2^+ + \Gamma_2^- + \Gamma_4^-, X_1 + X_2 + 2X_4, L_1 L_2 + 2L_3, 2W_1 W_2]$      |
| $[(\blacksquare)^{2T} + \Gamma_1^+ + \Gamma_1^- + \Gamma_2^+ + \Gamma_5^+, X_1 + X_2 + X_3 + X_4, L_1 L_2 + 2L_3, 2W_1 W_2]$ |

2nd minimal solution:  $\mu_2^T = 12$  (16 symmetry vectors)

Space group 229 ( $\mathbb{Z}_1$ )

1st minimal solution:  $\mu_1^T = 3$  (6 symmetry vectors)

| $\mathbf{n}^T$                                                                |
|-------------------------------------------------------------------------------|
| $[(\blacksquare)^{2T} + \Gamma_1^+, H_4^-, P_4, N_2^- + N_3^- + N_4^-]$       |
| $[(\blacksquare)^{2T} + \Gamma_1^+, H_4^-, P_1 + P_3, N_1^+ + N_2^+ + N_2^-]$ |
| $[(\blacksquare)^{2T} + \Gamma_2^-, H_5^+, P_4, N_2^- + N_4^+ + N_4^-]$       |
| $[(\blacksquare)^{2T} + \Gamma_2^+, H_5^-, P_5, N_2^+ + N_4^+ + N_4^-]$       |
| $[(\blacksquare)^{2T} + \Gamma_1^-, H_4^+, P_5, N_2^+ + N_3^+ + N_4^+]$       |
| $[(\blacksquare)^{2T} + \Gamma_1^-, H_4^+, P_2 + P_3, N_1^- + N_2^+ + N_2^-]$ |

2nd minimal solution:  $\mu_2^T = 4$  (36 symmetry vectors)

Space group 230 ( $\mathbb{Z}_1$ )

1st minimal solution:  $\mu_1^T = 8$  (4 symmetry vectors)

| $\mathbf{n}^T$                                                                                            |
|-----------------------------------------------------------------------------------------------------------|
| $[(\blacksquare)^{2T} + \Gamma_1^- + \Gamma_2^+ + \Gamma_2^- + \Gamma_4^-, H_1 + H_4, 2P_3, 3N_1 + N_2]$  |
| $[(\blacksquare)^{2T} + \Gamma_1^+ + \Gamma_2^+ + \Gamma_2^- + \Gamma_4^+, H_1 + H_4, 2P_3, 3N_1 + N_2]$  |
| $[(\blacksquare)^{2T} + \Gamma_1^+ + \Gamma_1^- + \Gamma_2^- + \Gamma_5^-, H_1 + H_4, 2P_3, 2N_1 + 2N_2]$ |
| $[(\blacksquare)^{2T} + \Gamma_1^+ + \Gamma_1^- + \Gamma_2^+ + \Gamma_5^+, H_1 + H_4, 2P_3, 2N_1 + 2N_2]$ |

2nd minimal solution:  $\mu_2^T = 12$  (12 symmetry vectors)

## B. Photonic minimum-connectivity solutions (without time-reversal symmetry)

Space group 1 ( $\mathbb{Z}_1$ )

1st minimal solution:  $\mu_1^T = 2$  (1 symmetry vector)

| $\mathbf{n}^T$                                                    |
|-------------------------------------------------------------------|
| $[(\blacksquare)^{2T}, 2R_1, 2T_1, 2U_1, 2V_1, 2X_1, 2Y_1, 2Z_1]$ |

2nd minimal solution:  $\mu_2^T = 3$  (1 symmetry vector)

Space group 2 ( $\mathbb{Z}_2 \times \mathbb{Z}_2 \times \mathbb{Z}_2 \times \mathbb{Z}_4$ )

1st minimal solution:  $\mu_1^T = 2$  (2187 symmetry vectors)

| $\mathbf{n}^T$                                                                         | $\mathbf{v}^T \in \mathbb{Z}_2 \times \mathbb{Z}_2 \times \mathbb{Z}_2 \times \mathbb{Z}_4$ |
|----------------------------------------------------------------------------------------|---------------------------------------------------------------------------------------------|
| $[(\blacksquare)^{2T}, 2R_1^-, 2T_1^-, 2U_1^-, 2V_1^-, 2X_1^-, 2Y_1^-, 2Z_1^-]$        | (1, 0, 0, 1)                                                                                |
| $[(\blacksquare)^{2T}, 2R_1^-, 2T_1^-, 2U_1^-, 2V_1^-, 2X_1^-, 2Y_1^-, Z_1^+ + Z_1^-]$ | (1, 0, 0, 2)                                                                                |

... continued on next page



... continued on next page

... continued on next page

... continued on next page

... continued on next page

... continued on next page

... continued on next page

... continued on next page

... continued on next page



... continued on next page

... continued on next page

... continued on next page



... continued on next page

... continued on next page

... continued on next page

... continued on next page



... continued on next page

... continued on next page

... continued on next page

... continued on next page

... continued on next page



... continued on next page

... continued on next page



... continued on next page

... continued on next page

... continued on next page

... continued on next page

... continued on next page

... continued on next page

... continued on next page





... continued on next page

... continued on next page

... continued on next page

... continued on next page

... continued on next page

... continued on next page

... continued on next page

... continued on next page



... continued from previous page

|                                                                                                      |              |
|------------------------------------------------------------------------------------------------------|--------------|
| $[(\blacksquare)^{2T}, 2R_1^+, 2T_1^+, 2U_1^+, V_1^+ + V_1^-, 2X_1^+, 2Y_1^-, 2Z_1^-]$               | (1, 0, 1, 0) |
| $[(\blacksquare)^{2T}, 2R_1^+, 2T_1^+, 2U_1^+, V_1^+ + V_1^-, 2X_1^+, 2Y_1^-, Z_1^+ + Z_1^-]$        | (1, 0, 1, 1) |
| $[(\blacksquare)^{2T}, 2R_1^+, 2T_1^+, 2U_1^+, 2V_1^-, 2X_1^+, Y_1^+ + Y_1^-, 2Z_1^-]$               | (1, 1, 0, 2) |
| $[(\blacksquare)^{2T}, 2R_1^+, 2T_1^+, 2U_1^+, 2V_1^-, 2X_1^+, Y_1^+ + Y_1^-, Z_1^+ + Z_1^-]$        | (1, 1, 0, 3) |
| $[(\blacksquare)^{2T}, 2R_1^+, 2T_1^+, 2U_1^+, V_1^+ + V_1^-, 2X_1^+, Y_1^+ + Y_1^-, 2Z_1^-]$        | (1, 1, 1, 1) |
| $[(\blacksquare)^{2T}, 2R_1^+, 2T_1^+, 2U_1^+, V_1^+ + V_1^-, 2X_1^+, Y_1^+ + Y_1^-, Z_1^+ + Z_1^-]$ | (1, 1, 1, 2) |
| $[(\blacksquare)^{2T}, 2R_1^+, 2T_1^+, 2U_1^+, 2V_1^-, 2X_1^+, 2Y_1^-, 2Z_1^+]$                      | (1, 0, 0, 3) |
| $[(\blacksquare)^{2T}, 2R_1^+, 2T_1^+, 2U_1^+, V_1^+ + V_1^-, 2X_1^+, 2Y_1^-, 2Z_1^+]$               | (1, 0, 1, 2) |
| $[(\blacksquare)^{2T}, 2R_1^+, 2T_1^+, 2U_1^+, 2V_1^-, 2X_1^+, Y_1^+ + Y_1^-, 2Z_1^+]$               | (1, 1, 0, 0) |
| $[(\blacksquare)^{2T}, 2R_1^+, 2T_1^+, 2U_1^+, V_1^+ + V_1^-, 2X_1^+, Y_1^+ + Y_1^-, 2Z_1^+]$        | (1, 1, 1, 3) |
| $[(\blacksquare)^{2T}, 2R_1^+, 2T_1^+, 2U_1^+, 2V_1^+, 2X_1^+, 2Y_1^-, 2Z_1^-]$                      | (1, 0, 0, 3) |
| $[(\blacksquare)^{2T}, 2R_1^+, 2T_1^+, 2U_1^+, 2V_1^+, 2X_1^+, 2Y_1^-, Z_1^+ + Z_1^-]$               | (1, 0, 0, 0) |
| $[(\blacksquare)^{2T}, 2R_1^+, 2T_1^+, 2U_1^+, 2V_1^+, 2X_1^+, Y_1^+ + Y_1^-, 2Z_1^-]$               | (1, 1, 0, 0) |
| $[(\blacksquare)^{2T}, 2R_1^+, 2T_1^+, 2U_1^+, 2V_1^+, 2X_1^+, Y_1^+ + Y_1^-, Z_1^+ + Z_1^-]$        | (1, 1, 0, 1) |
| $[(\blacksquare)^{2T}, 2R_1^+, 2T_1^+, 2U_1^+, 2V_1^+, 2X_1^+, 2Y_1^-, 2Z_1^+]$                      | (1, 0, 0, 1) |
| $[(\blacksquare)^{2T}, 2R_1^+, 2T_1^+, 2U_1^+, 2V_1^+, 2X_1^+, Y_1^+ + Y_1^-, 2Z_1^+]$               | (1, 1, 0, 2) |
| $[(\blacksquare)^{2T}, 2R_1^+, 2T_1^+, 2U_1^+, 2V_1^-, 2X_1^+, 2Y_1^+, 2Z_1^-]$                      | (1, 0, 0, 3) |
| $[(\blacksquare)^{2T}, 2R_1^+, 2T_1^+, 2U_1^+, 2V_1^-, 2X_1^+, 2Y_1^+, Z_1^+ + Z_1^-]$               | (1, 0, 0, 0) |
| $[(\blacksquare)^{2T}, 2R_1^+, 2T_1^+, 2U_1^+, V_1^+ + V_1^-, 2X_1^+, 2Y_1^+, 2Z_1^-]$               | (1, 0, 1, 2) |
| $[(\blacksquare)^{2T}, 2R_1^+, 2T_1^+, 2U_1^+, V_1^+ + V_1^-, 2X_1^+, 2Y_1^+, Z_1^+ + Z_1^-]$        | (1, 0, 1, 3) |
| $[(\blacksquare)^{2T}, 2R_1^+, 2T_1^+, 2U_1^+, 2V_1^-, 2X_1^+, 2Y_1^+, 2Z_1^+]$                      | (1, 0, 0, 1) |
| $[(\blacksquare)^{2T}, 2R_1^+, 2T_1^+, 2U_1^+, V_1^+ + V_1^-, 2X_1^+, 2Y_1^+, 2Z_1^+]$               | (1, 0, 1, 0) |
| $[(\blacksquare)^{2T}, 2R_1^+, 2T_1^+, 2U_1^+, 2V_1^+, 2X_1^+, 2Y_1^+, 2Z_1^-]$                      | (1, 0, 0, 1) |
| $[(\blacksquare)^{2T}, 2R_1^+, 2T_1^+, 2U_1^+, 2V_1^+, 2X_1^+, 2Y_1^+, Z_1^+ + Z_1^-]$               | (1, 0, 0, 2) |
| $[(\blacksquare)^{2T}, 2R_1^+, 2T_1^+, 2U_1^+, 2V_1^+, 2X_1^+, 2Y_1^+, 2Z_1^+]$                      | (1, 0, 0, 3) |

Skipped higher-order solutions...

Space group 3 ( $\mathbb{Z}_2$ )1st minimal solution:  $\mu_1^T = 2$  (27 symmetry vectors)

| $\mathbf{n}^T$                                                                                  | $\mathbf{v}^T \in \mathbb{Z}_2$ |
|-------------------------------------------------------------------------------------------------|---------------------------------|
| $[(\blacksquare)^{2T}, 2A_2, 2B_1, 2C_2, 2D_1, 2E_2, 2Y_2, 2Z_2]$                               | trivial                         |
| $[(\blacksquare)^{2T}, 2A_2, B_1 + B_2, 2C_2, D_1 + D_2, 2E_2, 2Y_2, 2Z_2]$                     | 1                               |
| $[(\blacksquare)^{2T}, 2A_2, 2B_1, C_1 + C_2, 2D_1, 2E_2, Y_1 + Y_2, 2Z_2]$                     | 1                               |
| $[(\blacksquare)^{2T}, 2A_2, B_1 + B_2, C_1 + C_2, D_1 + D_2, 2E_2, Y_1 + Y_2, 2Z_2]$           | trivial                         |
| $[(\blacksquare)^{2T}, A_1 + A_2, 2B_1, 2C_2, 2D_1, E_1 + E_2, 2Y_2, 2Z_2]$                     | 1                               |
| $[(\blacksquare)^{2T}, A_1 + A_2, B_1 + B_2, 2C_2, D_1 + D_2, E_1 + E_2, 2Y_2, 2Z_2]$           | trivial                         |
| $[(\blacksquare)^{2T}, A_1 + A_2, 2B_1, C_1 + C_2, 2D_1, E_1 + E_2, Y_1 + Y_2, 2Z_2]$           | trivial                         |
| $[(\blacksquare)^{2T}, A_1 + A_2, B_1 + B_2, C_1 + C_2, D_1 + D_2, E_1 + E_2, Y_1 + Y_2, 2Z_2]$ | 1                               |
| $[(\blacksquare)^{2T}, 2A_2, 2B_2, 2C_2, 2D_2, 2E_2, 2Y_2, 2Z_2]$                               | trivial                         |
| $[(\blacksquare)^{2T}, 2A_2, 2B_2, C_1 + C_2, 2D_2, 2E_2, Y_1 + Y_2, 2Z_2]$                     | 1                               |
| $[(\blacksquare)^{2T}, A_1 + A_2, 2B_2, 2C_2, 2D_2, E_1 + E_2, 2Y_2, 2Z_2]$                     | 1                               |
| $[(\blacksquare)^{2T}, A_1 + A_2, 2B_2, C_1 + C_2, 2D_2, E_1 + E_2, Y_1 + Y_2, 2Z_2]$           | trivial                         |
| $[(\blacksquare)^{2T}, 2A_2, 2B_1, 2C_1, 2D_1, 2E_2, 2Y_1, 2Z_2]$                               | trivial                         |
| $[(\blacksquare)^{2T}, 2A_2, B_1 + B_2, 2C_1, D_1 + D_2, 2E_2, 2Y_1, 2Z_2]$                     | 1                               |
| $[(\blacksquare)^{2T}, A_1 + A_2, 2B_1, 2C_1, 2D_1, E_1 + E_2, 2Y_1, 2Z_2]$                     | 1                               |
| $[(\blacksquare)^{2T}, A_1 + A_2, B_1 + B_2, 2C_1, D_1 + D_2, E_1 + E_2, 2Y_1, 2Z_2]$           | trivial                         |
| $[(\blacksquare)^{2T}, 2A_2, 2B_2, 2C_1, 2D_2, 2E_2, 2Y_1, 2Z_2]$                               | trivial                         |
| $[(\blacksquare)^{2T}, A_1 + A_2, 2B_2, 2C_1, 2D_2, E_1 + E_2, 2Y_1, 2Z_2]$                     | 1                               |

... continued on next page

... continued from previous page

|                                                                                       |         |
|---------------------------------------------------------------------------------------|---------|
| $[(\blacksquare)^{2T}, 2A_1, 2B_1, 2C_2, 2D_1, 2E_1, 2Y_2, 2Z_2]$                     | trivial |
| $[(\blacksquare)^{2T}, 2A_1, B_1 + B_2, 2C_2, D_1 + D_2, 2E_1, 2Y_2, 2Z_2]$           | 1       |
| $[(\blacksquare)^{2T}, 2A_1, 2B_1, C_1 + C_2, 2D_1, 2E_1, Y_1 + Y_2, 2Z_2]$           | 1       |
| $[(\blacksquare)^{2T}, 2A_1, B_1 + B_2, C_1 + C_2, D_1 + D_2, 2E_1, Y_1 + Y_2, 2Z_2]$ | trivial |
| $[(\blacksquare)^{2T}, 2A_1, 2B_2, 2C_2, 2D_2, 2E_1, 2Y_2, 2Z_2]$                     | trivial |
| $[(\blacksquare)^{2T}, 2A_1, 2B_2, C_1 + C_2, 2D_2, 2E_1, Y_1 + Y_2, 2Z_2]$           | 1       |
| $[(\blacksquare)^{2T}, 2A_1, 2B_1, 2C_1, 2D_1, 2E_1, 2Y_1, 2Z_2]$                     | trivial |
| $[(\blacksquare)^{2T}, 2A_1, B_1 + B_2, 2C_1, D_1 + D_2, 2E_1, 2Y_1, 2Z_2]$           | 1       |
| $[(\blacksquare)^{2T}, 2A_1, 2B_2, 2C_1, 2D_2, 2E_1, 2Y_1, 2Z_2]$                     | trivial |

2nd minimal solution:  $\mu_2^T = 3$  (128 symmetry vectors)

Space group 4 ( $\mathbb{Z}_1$ )

1st minimal solution:  $\mu_1^T = 4$  (1 symmetry vector)

| $\mathbf{n}^T$                                                                                                                 |
|--------------------------------------------------------------------------------------------------------------------------------|
| $[(\blacksquare)^{2T} + 2\Gamma_1, 2A_1 + 2A_2, 2B_1 + 2B_2, 2C_1 + 2C_2, 2D_1 + 2D_2, 2E_1 + 2E_2, 2Y_1 + 2Y_2, 2Z_1 + 2Z_2]$ |

2nd minimal solution:  $\mu_2^T = 6$  (1 symmetry vector)

Space group 5 ( $\mathbb{Z}_1$ )

1st minimal solution:  $\mu_1^T = 2$  (3 symmetry vectors)

| $\mathbf{n}^T$                                                  |
|-----------------------------------------------------------------|
| $[(\blacksquare)^{2T}, 2A_2, 2M_2, 2Y_2, 2L_1, 2V_1]$           |
| $[(\blacksquare)^{2T}, A_1 + A_2, M_1 + M_2, 2Y_2, 2L_1, 2V_1]$ |
| $[(\blacksquare)^{2T}, 2A_1, 2M_1, 2Y_2, 2L_1, 2V_1]$           |

2nd minimal solution:  $\mu_2^T = 3$  (8 symmetry vectors)

Space group 6 ( $\mathbb{Z}_1$ )

1st minimal solution:  $\mu_1^T = 2$  (3 symmetry vectors)

| $\mathbf{n}^T$                                                                                       |
|------------------------------------------------------------------------------------------------------|
| $[(\blacksquare)^{2T}, A_1 + A_2, B_1 + B_2, 2C_2, 2D_2, 2E_2, Y_1 + Y_2, 2Z_2]$                     |
| $[(\blacksquare)^{2T}, A_1 + A_2, B_1 + B_2, C_1 + C_2, D_1 + D_2, E_1 + E_2, Y_1 + Y_2, Z_1 + Z_2]$ |
| $[(\blacksquare)^{2T}, A_1 + A_2, B_1 + B_2, 2C_1, 2D_1, 2E_1, Y_1 + Y_2, 2Z_1]$                     |

2nd minimal solution:  $\mu_2^T = 3$  (8 symmetry vectors)

Space group 7 ( $\mathbb{Z}_1$ )

1st minimal solution:  $\mu_1^T = 2$  (1 symmetry vector)

$$\frac{\mathbf{n}^T}{[(\blacksquare)^{2T}, A_1 + A_2, B_1 + B_2, C_1 + C_2, D_1 + D_2, E_1 + E_2, Y_1 + Y_2, Z_1 + Z_2]}$$

2nd minimal solution:  $\mu_2^T = 4$  (1 symmetry vector)

Space group 8 ( $\mathbb{Z}_1$ )

1st minimal solution:  $\mu_1^T = 2$  (1 symmetry vector)

$$\frac{\mathbf{n}^T}{[(\blacksquare)^{2T}, A_1 + A_2, M_1 + M_2, Y_1 + Y_2, 2L_1, 2V_1]}$$

2nd minimal solution:  $\mu_2^T = 3$  (2 symmetry vectors)

Space group 9 ( $\mathbb{Z}_1$ )

1st minimal solution:  $\mu_1^T = 2$  (1 symmetry vector)

$$\frac{\mathbf{n}^T}{[(\blacksquare)^{2T}, A_1 + A_2, M_1 + M_2, Y_1 + Y_2, 2L_1, 2V_1]}$$

2nd minimal solution:  $\mu_2^T = 4$  (1 symmetry vector)

Space group 10 ( $\mathbb{Z}_2 \times \mathbb{Z}_2 \times \mathbb{Z}_2$ )

1st minimal solution:  $\mu_1^T = 2$  (344 symmetry vectors)

| $\mathbf{n}^T$                                                                                                            | $\mathbf{v}^T \in \mathbb{Z}_2 \times \mathbb{Z}_2 \times \mathbb{Z}_2$ |
|---------------------------------------------------------------------------------------------------------------------------|-------------------------------------------------------------------------|
| $[(\blacksquare)^{2T}, A_2^+ + A_2^-, B_1^+ + B_1^-, 2C_2^-, 2D_1^+, 2E_2^-, Y_2^+ + Y_2^-, 2Z_2^-]$                      | trivial                                                                 |
| $[(\blacksquare)^{2T}, A_2^+ + A_2^-, B_1^+ + B_2^+, 2C_2^-, D_1^+ + D_2^-, 2E_2^-, Y_2^+ + Y_2^-, 2Z_2^-]$               | (0, 1, 1)                                                               |
| $[(\blacksquare)^{2T}, A_2^+ + A_2^-, B_1^+ + B_1^-, C_1^+ + C_2^-, 2D_1^+, 2E_2^-, Y_1^- + Y_2^-, 2Z_2^-]$               | (0, 1, 1)                                                               |
| $[(\blacksquare)^{2T}, A_2^+ + A_2^-, B_1^+ + B_2^+, C_1^+ + C_2^-, D_1^+ + D_2^-, 2E_2^-, Y_1^- + Y_2^-, 2Z_2^-]$        | trivial                                                                 |
| $[(\blacksquare)^{2T}, A_1^- + A_2^-, B_1^+ + B_1^-, 2C_2^-, 2D_1^+, E_1^+ + E_2^-, Y_2^+ + Y_2^-, 2Z_2^-]$               | (0, 1, 1)                                                               |
| $[(\blacksquare)^{2T}, A_1^- + A_2^-, B_1^+ + B_2^+, 2C_2^-, D_1^+ + D_2^-, E_1^+ + E_2^-, Y_2^+ + Y_2^-, 2Z_2^-]$        | trivial                                                                 |
| $[(\blacksquare)^{2T}, A_1^- + A_2^-, B_1^+ + B_1^-, C_1^+ + C_2^-, 2D_1^+, E_1^+ + E_2^-, Y_1^- + Y_2^-, 2Z_2^-]$        | trivial                                                                 |
| $[(\blacksquare)^{2T}, A_1^- + A_2^-, B_1^+ + B_2^+, C_1^+ + C_2^-, D_1^+ + D_2^-, E_1^+ + E_2^-, Y_1^- + Y_2^-, 2Z_2^-]$ | (0, 1, 1)                                                               |
| $[(\blacksquare)^{2T}, A_2^+ + A_2^-, B_1^- + B_2^-, 2C_2^-, D_1^+ + D_2^-, 2E_2^-, Y_2^+ + Y_2^-, 2Z_2^-]$               | (1, 0, 0)                                                               |
| $[(\blacksquare)^{2T}, A_2^+ + A_2^-, B_2^+ + B_2^-, 2C_2^-, 2D_2^-, 2E_2^-, Y_2^+ + Y_2^-, 2Z_2^-]$                      | (1, 1, 1)                                                               |
| $[(\blacksquare)^{2T}, A_2^+ + A_2^-, B_1^- + B_2^-, C_1^+ + C_2^-, D_1^+ + D_2^-, 2E_2^-, Y_1^- + Y_2^-, 2Z_2^-]$        | (1, 1, 1)                                                               |
| $[(\blacksquare)^{2T}, A_2^+ + A_2^-, B_2^+ + B_2^-, C_1^+ + C_2^-, 2D_2^-, 2E_2^-, Y_1^- + Y_2^-, 2Z_2^-]$               | (1, 0, 0)                                                               |

... continued on next page



... continued on next page



... continued on next page

... continued on next page



... continued on next page

... continued from previous page

|                                                                                                               |           |
|---------------------------------------------------------------------------------------------------------------|-----------|
| $[(\bullet)^{2T}, A_1^+ + A_1^-, B_1^+ + B_1^-, C_1^- + C_2^+, 2D_1^-, 2E_1^-, Y_1^- + Y_2^-, 2Z_2^+]$        | (1, 0, 1) |
| $[(\bullet)^{2T}, A_1^+ + A_1^-, B_1^- + B_2^-, C_1^- + C_2^+, D_1^- + D_2^+, 2E_1^-, Y_1^- + Y_2^-, 2Z_2^+]$ | trivial   |
| $[(\bullet)^{2T}, A_1^+ + A_1^-, B_1^+ + B_1^-, 2C_1^-, 2D_1^-, 2E_1^-, Y_1^+ + Y_1^-, 2Z_2^+]$               | trivial   |
| $[(\bullet)^{2T}, A_1^+ + A_1^-, B_1^- + B_2^-, 2C_1^-, D_1^- + D_2^+, 2E_1^-, Y_1^+ + Y_1^-, 2Z_2^+]$        | (1, 0, 1) |
| $[(\bullet)^{2T}, A_1^+ + A_1^-, B_1^+ + B_2^+, C_1^- + C_2^+, D_1^- + D_2^+, 2E_1^-, Y_1^- + Y_2^-, 2Z_2^+]$ | (1, 1, 1) |
| $[(\bullet)^{2T}, A_1^+ + A_1^-, B_2^+ + B_2^-, C_1^- + C_2^+, 2D_2^+, 2E_1^-, Y_1^- + Y_2^-, 2Z_2^+]$        | (0, 1, 0) |
| $[(\bullet)^{2T}, A_1^+ + A_1^-, B_1^+ + B_2^+, 2C_1^-, D_1^- + D_2^+, 2E_1^-, Y_1^+ + Y_1^-, 2Z_2^+]$        | (0, 1, 0) |
| $[(\bullet)^{2T}, A_1^+ + A_1^-, B_2^+ + B_2^-, 2C_1^-, 2D_2^+, 2E_1^-, Y_1^+ + Y_1^-, 2Z_2^+]$               | (1, 1, 1) |

Skipped higher-order solutions...

Space group 11 ( $\mathbb{Z}_2$ )1st minimal solution:  $\mu_1^T = 4$  (43 symmetry vectors)

| $\mathbf{n}^T$                                                                                                                                                    | $\mathbf{v}^T \in \mathbb{Z}_2$ |
|-------------------------------------------------------------------------------------------------------------------------------------------------------------------|---------------------------------|
| $[(\bullet)^{2T} + 2\Gamma_1^-, 2A_1^- + A_2^+ + A_2^-, 2B_1^- + B_2^+ + B_2^-, 2C_1, 2D_1, 2E_1, Y_1^+ + Y_1^- + 2Y_2^+, 2Z_1]$                                  | trivial                         |
| $[(\bullet)^{2T} + \Gamma_1^+ + \Gamma_1^-, 2A_1^- + 2A_2^-, 2B_1^- + 2B_2^-, 2C_1, 2D_1, 2E_1, 2Y_1^+ + 2Y_2^+, 2Z_1]$                                           | trivial                         |
| $[(\bullet)^{2T} + \Gamma_1^+ + \Gamma_1^-, 2A_1^- + 2A_2^-, 2B_1^- + 2B_2^-, 2C_1, 2D_1, 2E_1, Y_1^+ + Y_1^- + Y_2^+ + Y_2^-, 2Z_1]$                             | 1                               |
| $[(\bullet)^{2T} + \Gamma_1^+ + \Gamma_1^-, 2A_1^- + 2A_2^-, B_1^+ + B_1^- + B_2^+ + B_2^-, 2C_1, 2D_1, 2E_1, 2Y_1^+ + 2Y_2^+, 2Z_1]$                             | 1                               |
| $[(\bullet)^{2T} + \Gamma_1^+ + \Gamma_1^-, 2A_1^- + 2A_2^-, B_1^+ + B_1^- + B_2^+ + B_2^-, 2C_1, 2D_1, 2E_1, Y_1^+ + Y_1^- + Y_2^+ + Y_2^-, 2Z_1]$               | trivial                         |
| $[(\bullet)^{2T} + \Gamma_1^+ + \Gamma_1^-, A_1^+ + A_1^- + A_2^+ + A_2^-, 2B_1^- + 2B_2^-, 2C_1, 2D_1, 2E_1, 2Y_1^+ + 2Y_2^+, 2Z_1]$                             | 1                               |
| $[(\bullet)^{2T} + \Gamma_1^+ + \Gamma_1^-, A_1^+ + A_1^- + A_2^+ + A_2^-, 2B_1^- + 2B_2^-, 2C_1, 2D_1, 2E_1, Y_1^+ + Y_1^- + Y_2^+ + Y_2^-, 2Z_1]$               | trivial                         |
| $[(\bullet)^{2T} + \Gamma_1^+ + \Gamma_1^-, A_1^+ + A_1^- + A_2^+ + A_2^-, B_1^+ + B_1^- + B_2^+ + B_2^-, 2C_1, 2D_1, 2E_1, 2Y_1^+ + 2Y_2^+, 2Z_1]$               | trivial                         |
| $[(\bullet)^{2T} + \Gamma_1^+ + \Gamma_1^-, A_1^+ + A_1^- + A_2^+ + A_2^-, B_1^+ + B_1^- + B_2^+ + B_2^-, 2C_1, 2D_1, 2E_1, Y_1^+ + Y_1^- + Y_2^+ + Y_2^-, 2Z_1]$ | 1                               |
| $[(\bullet)^{2T} + 2\Gamma_1^-, 2A_1^- + A_2^+ + A_2^-, 2B_1^- + B_2^+ + B_2^-, 2C_1, 2D_1, 2E_1, 2Y_1^- + Y_2^+ + Y_2^-, 2Z_1]$                                  | 1                               |
| $[(\bullet)^{2T} + \Gamma_1^+ + \Gamma_1^-, 2A_1^- + 2A_2^-, 2B_1^- + 2B_2^-, 2C_1, 2D_1, 2E_1, 2Y_1^- + 2Y_2^-, 2Z_1]$                                           | trivial                         |
| $[(\bullet)^{2T} + \Gamma_1^+ + \Gamma_1^-, 2A_1^- + 2A_2^-, B_1^+ + B_1^- + B_2^+ + B_2^-, 2C_1, 2D_1, 2E_1, 2Y_1^- + 2Y_2^-, 2Z_1]$                             | 1                               |
| $[(\bullet)^{2T} + \Gamma_1^+ + \Gamma_1^-, A_1^+ + A_1^- + A_2^+ + A_2^-, 2B_1^- + 2B_2^-, 2C_1, 2D_1, 2E_1, 2Y_1^- + 2Y_2^-, 2Z_1]$                             | 1                               |
| $[(\bullet)^{2T} + \Gamma_1^+ + \Gamma_1^-, A_1^+ + A_1^- + A_2^+ + A_2^-, B_1^+ + B_1^- + B_2^+ + B_2^-, 2C_1, 2D_1, 2E_1, 2Y_1^- + 2Y_2^-, 2Z_1]$               | trivial                         |
| $[(\bullet)^{2T} + 2\Gamma_1^-, 2A_1^- + A_2^+ + A_2^-, B_1^+ + B_1^- + B_2^+ + B_2^-, 2C_1, 2D_1, 2E_1, Y_1^+ + Y_1^- + 2Y_2^+, 2Z_1]$                           | 1                               |
| $[(\bullet)^{2T} + 2\Gamma_1^-, 2A_1^- + A_2^+ + A_2^-, B_1^+ + B_1^- + B_2^+ + B_2^-, 2C_1, 2D_1, 2E_1, 2Y_1^- + Y_2^+ + Y_2^-, 2Z_1]$                           | trivial                         |
| $[(\bullet)^{2T} + 2\Gamma_1^-, A_1^+ + A_1^- + 2A_2^+, 2B_1^- + B_2^+ + B_2^-, 2C_1, 2D_1, 2E_1, Y_1^+ + Y_1^- + 2Y_2^+, 2Z_1]$                                  | 1                               |
| $[(\bullet)^{2T} + 2\Gamma_1^-, A_1^+ + A_1^- + 2A_2^+, 2B_1^- + B_2^+ + B_2^-, 2C_1, 2D_1, 2E_1, 2Y_1^- + Y_2^+ + Y_2^-, 2Z_1]$                                  | trivial                         |
| $[(\bullet)^{2T} + 2\Gamma_1^-, A_1^+ + A_1^- + 2A_2^+, B_1^+ + B_1^- + 2B_2^-, 2C_1, 2D_1, 2E_1, Y_1^+ + Y_1^- + 2Y_2^+, 2Z_1]$                                  | trivial                         |
| $[(\bullet)^{2T} + 2\Gamma_1^-, A_1^+ + A_1^- + 2A_2^+, B_1^+ + B_1^- + 2B_2^-, 2C_1, 2D_1, 2E_1, 2Y_1^- + Y_2^+ + Y_2^-, 2Z_1]$                                  | 1                               |
| $[(\bullet)^{2T} + 2\Gamma_1^-, A_1^+ + A_1^- + 2A_2^-, B_1^+ + B_1^- + 2B_2^-, 2C_1, 2D_1, 2E_1, 2Y_1^+ + Y_2^+ + Y_2^-, 2Z_1]$                                  | 1                               |
| $[(\bullet)^{2T} + 2\Gamma_1^-, A_1^+ + A_1^- + 2A_2^-, B_1^+ + B_1^- + 2B_2^-, 2C_1, 2D_1, 2E_1, Y_1^+ + Y_1^- + 2Y_2^-, 2Z_1]$                                  | trivial                         |
| $[(\bullet)^{2T} + \Gamma_1^+ + \Gamma_1^-, 2A_1^- + 2A_2^-, 2B_1^+ + 2B_2^+, 2C_1, 2D_1, 2E_1, 2Y_1^+ + 2Y_2^+, 2Z_1]$                                           | trivial                         |
| $[(\bullet)^{2T} + \Gamma_1^+ + \Gamma_1^-, 2A_1^- + 2A_2^-, 2B_1^+ + 2B_2^+, 2C_1, 2D_1, 2E_1, Y_1^+ + Y_1^- + Y_2^+ + Y_2^-, 2Z_1]$                             | 1                               |
| $[(\bullet)^{2T} + \Gamma_1^+ + \Gamma_1^-, A_1^+ + A_1^- + A_2^+ + A_2^-, 2B_1^+ + 2B_2^+, 2C_1, 2D_1, 2E_1, 2Y_1^+ + 2Y_2^+, 2Z_1]$                             | 1                               |
| $[(\bullet)^{2T} + \Gamma_1^+ + \Gamma_1^-, A_1^+ + A_1^- + A_2^+ + A_2^-, 2B_1^+ + 2B_2^+, 2C_1, 2D_1, 2E_1, Y_1^+ + Y_1^- + Y_2^+ + Y_2^-, 2Z_1]$               | trivial                         |
| $[(\bullet)^{2T} + \Gamma_1^+ + \Gamma_1^-, 2A_1^- + 2A_2^-, 2B_1^+ + 2B_2^+, 2C_1, 2D_1, 2E_1, 2Y_1^- + 2Y_2^-, 2Z_1]$                                           | trivial                         |
| $[(\bullet)^{2T} + \Gamma_1^+ + \Gamma_1^-, A_1^+ + A_1^- + A_2^+ + A_2^-, 2B_1^+ + 2B_2^+, 2C_1, 2D_1, 2E_1, 2Y_1^- + 2Y_2^-, 2Z_1]$                             | 1                               |
| $[(\bullet)^{2T} + 2\Gamma_1^+, A_1^+ + A_1^- + 2A_2^-, 2B_1^+ + B_2^+ + B_2^-, 2C_1, 2D_1, 2E_1, 2Y_1^+ + Y_2^+ + Y_2^-, 2Z_1]$                                  | trivial                         |
| $[(\bullet)^{2T} + 2\Gamma_1^+, A_1^+ + A_1^- + 2A_2^-, 2B_1^+ + B_2^+ + B_2^-, 2C_1, 2D_1, 2E_1, Y_1^+ + Y_1^- + 2Y_2^-, 2Z_1]$                                  | 1                               |
| $[(\bullet)^{2T} + \Gamma_1^+ + \Gamma_1^-, 2A_1^+ + 2A_2^+, 2B_1^- + 2B_2^-, 2C_1, 2D_1, 2E_1, 2Y_1^+ + 2Y_2^+, 2Z_1]$                                           | trivial                         |
| $[(\bullet)^{2T} + \Gamma_1^+ + \Gamma_1^-, 2A_1^+ + 2A_2^+, B_1^+ + B_1^- + B_2^+ + B_2^-, 2C_1, 2D_1, 2E_1, 2Y_1^+ + Y_2^+ + Y_2^-, 2Z_1]$                      | 1                               |
| $[(\bullet)^{2T} + \Gamma_1^+ + \Gamma_1^-, 2A_1^+ + 2A_2^+, B_1^+ + B_1^- + B_2^+ + B_2^-, 2C_1, 2D_1, 2E_1, Y_1^+ + Y_1^- + Y_2^+ + Y_2^-, 2Z_1]$               | trivial                         |
| $[(\bullet)^{2T} + \Gamma_1^+ + \Gamma_1^-, 2A_1^+ + 2A_2^+, 2B_1^- + 2B_2^-, 2C_1, 2D_1, 2E_1, 2Y_1^+ + 2Y_2^+, 2Z_1]$                                           | 1                               |
| $[(\bullet)^{2T} + \Gamma_1^+ + \Gamma_1^-, 2A_1^+ + 2A_2^+, B_1^+ + B_1^- + B_2^+ + B_2^-, 2C_1, 2D_1, 2E_1, 2Y_1^+ + Y_2^+ + Y_2^-, 2Z_1]$                      | trivial                         |
| $[(\bullet)^{2T} + \Gamma_1^+ + \Gamma_1^-, 2A_1^+ + 2A_2^+, B_1^+ + B_1^- + B_2^+ + B_2^-, 2C_1, 2D_1, 2E_1, Y_1^+ + Y_1^- + Y_2^+ + Y_2^-, 2Z_1]$               | 1                               |
| $[(\bullet)^{2T} + \Gamma_1^+ + \Gamma_1^-, 2A_1^+ + 2A_2^+, 2B_1^- + 2B_2^-, 2C_1, 2D_1, 2E_1, 2Y_1^+ + 2Y_2^+, 2Z_1]$                                           | trivial                         |
| $[(\bullet)^{2T} + \Gamma_1^+ + \Gamma_1^-, 2A_1^+ + 2A_2^+, B_1^+ + B_1^- + B_2^+ + B_2^-, 2C_1, 2D_1, 2E_1, 2Y_1^+ + Y_2^+ + Y_2^-, 2Z_1]$                      | 1                               |
| $[(\bullet)^{2T} + \Gamma_1^+ + \Gamma_1^-, 2A_1^+ + 2A_2^+, B_1^+ + B_1^- + B_2^+ + B_2^-, 2C_1, 2D_1, 2E_1, Y_1^+ + Y_1^- + Y_2^+ + Y_2^-, 2Z_1]$               | trivial                         |
| $[(\bullet)^{2T} + \Gamma_1^+ + \Gamma_1^-, 2A_1^+ + 2A_2^+, 2B_1^- + 2B_2^-, 2C_1, 2D_1, 2E_1, 2Y_1^+ + 2Y_2^+, 2Z_1]$                                           | 1                               |

... continued on next page

... continued from previous page

|                                                                                                                                            |         |
|--------------------------------------------------------------------------------------------------------------------------------------------|---------|
| $[(\blacksquare)^{2T} + \Gamma_1^+ + \Gamma_1^-, 2A_1^+ + 2A_2^+, B_1^+ + B_1^- + B_2^+ + B_2^-, 2C_1, 2D_1, 2E_1, 2Y_1^- + 2Y_2^-, 2Z_1]$ | 1       |
| $[(\blacksquare)^{2T} + 2\Gamma_1^+, 2A_1^+ + A_2^+ + A_2^-, B_1^+ + B_1^- + 2B_2^-, 2C_1, 2D_1, 2E_1, 2Y_1^+ + Y_2^+ + Y_2^-, 2Z_1]$      | trivial |
| $[(\blacksquare)^{2T} + 2\Gamma_1^+, 2A_1^+ + A_2^+ + A_2^-, B_1^+ + B_1^- + 2B_2^-, 2C_1, 2D_1, 2E_1, Y_1^+ + Y_1^- + 2Y_2^-, 2Z_1]$      | 1       |
| $[(\blacksquare)^{2T} + \Gamma_1^+ + \Gamma_1^-, 2A_1^+ + 2A_2^+, 2B_1^+ + 2B_2^+, 2C_1, 2D_1, 2E_1, 2Y_1^+ + 2Y_2^+, 2Z_1]$               | trivial |
| $[(\blacksquare)^{2T} + \Gamma_1^+ + \Gamma_1^-, 2A_1^+ + 2A_2^+, 2B_1^+ + 2B_2^+, 2C_1, 2D_1, 2E_1, Y_1^+ + Y_1^- + Y_2^+ + Y_2^-, 2Z_1]$ | 1       |
| $[(\blacksquare)^{2T} + \Gamma_1^+ + \Gamma_1^-, 2A_1^+ + 2A_2^+, 2B_1^+ + 2B_2^+, 2C_1, 2D_1, 2E_1, 2Y_1^- + 2Y_2^-, 2Z_1]$               | trivial |
| $[(\blacksquare)^{2T} + 2\Gamma_1^+, 2A_1^+ + A_2^+ + A_2^-, 2B_1^+ + B_2^+ + B_2^-, 2C_1, 2D_1, 2E_1, 2Y_1^+ + Y_2^+ + Y_2^-, 2Z_1]$      | 1       |
| $[(\blacksquare)^{2T} + 2\Gamma_1^+, 2A_1^+ + A_2^+ + A_2^-, 2B_1^+ + B_2^+ + B_2^-, 2C_1, 2D_1, 2E_1, Y_1^+ + Y_1^- + 2Y_2^-, 2Z_1]$      | trivial |

2nd minimal solution:  $\mu_2^T = 6$  (252 symmetry vectors)

Space group 12 ( $\mathbb{Z}_2 \times \mathbb{Z}_2$ )

1st minimal solution:  $\mu_1^T = 2$  (54 symmetry vectors)

| $n^T$                                                                                              | $v^T \in \mathbb{Z}_2 \times \mathbb{Z}_2$ |
|----------------------------------------------------------------------------------------------------|--------------------------------------------|
| $[(\blacksquare)^{2T}, A_2^+ + A_2^-, M_2^+ + M_2^-, Y_2^+ + Y_2^-, 2L_1^-, 2V_1^+]$               | (0, 1)                                     |
| $[(\blacksquare)^{2T}, A_2^+ + A_2^-, M_2^+ + M_2^-, Y_2^+ + Y_2^-, 2L_1^-, V_1^+ + V_1^-]$        | (1, 1)                                     |
| $[(\blacksquare)^{2T}, A_2^+ + A_2^-, M_2^+ + M_2^-, Y_2^+ + Y_2^-, 2L_1^-, 2V_1^-]$               | (0, 1)                                     |
| $[(\blacksquare)^{2T}, A_2^+ + A_2^-, M_2^+ + M_2^-, Y_2^+ + Y_2^-, L_1^+ + L_1^-, 2V_1^+]$        | (1, 1)                                     |
| $[(\blacksquare)^{2T}, A_2^+ + A_2^-, M_2^+ + M_2^-, Y_2^+ + Y_2^-, L_1^+ + L_1^-, V_1^+ + V_1^-]$ | (0, 1)                                     |
| $[(\blacksquare)^{2T}, A_2^+ + A_2^-, M_2^+ + M_2^-, Y_2^+ + Y_2^-, L_1^+ + L_1^-, 2V_1^-]$        | (1, 1)                                     |
| $[(\blacksquare)^{2T}, A_2^+ + A_2^-, M_2^+ + M_2^-, Y_2^+ + Y_2^-, 2L_1^+, 2V_1^+]$               | (0, 1)                                     |
| $[(\blacksquare)^{2T}, A_2^+ + A_2^-, M_2^+ + M_2^-, Y_2^+ + Y_2^-, 2L_1^+, V_1^+ + V_1^-]$        | (1, 1)                                     |
| $[(\blacksquare)^{2T}, A_2^+ + A_2^-, M_2^+ + M_2^-, Y_2^+ + Y_2^-, 2L_1^+, 2V_1^-]$               | (0, 1)                                     |
| $[(\blacksquare)^{2T}, A_1^- + A_2^-, M_1^- + M_2^-, Y_2^+ + Y_2^-, 2L_1^-, 2V_1^+]$               | (1, 1)                                     |
| $[(\blacksquare)^{2T}, A_1^- + A_2^-, M_1^- + M_2^-, Y_2^+ + Y_2^-, 2L_1^-, V_1^+ + V_1^-]$        | (0, 1)                                     |
| $[(\blacksquare)^{2T}, A_1^- + A_2^-, M_1^- + M_2^-, Y_2^+ + Y_2^-, 2L_1^-, 2V_1^-]$               | (1, 1)                                     |
| $[(\blacksquare)^{2T}, A_1^- + A_2^-, M_1^+ + M_2^+, Y_2^+ + Y_2^-, 2L_1^-, 2V_1^+]$               | (1, 0)                                     |
| $[(\blacksquare)^{2T}, A_1^- + A_2^-, M_1^+ + M_2^+, Y_2^+ + Y_2^-, 2L_1^-, V_1^+ + V_1^-]$        | trivial                                    |
| $[(\blacksquare)^{2T}, A_1^- + A_2^-, M_1^+ + M_2^+, Y_2^+ + Y_2^-, 2L_1^-, 2V_1^-]$               | (1, 0)                                     |
| $[(\blacksquare)^{2T}, A_1^- + A_2^-, M_1^- + M_2^-, Y_2^+ + Y_2^-, L_1^+ + L_1^-, 2V_1^+]$        | (0, 1)                                     |
| $[(\blacksquare)^{2T}, A_1^- + A_2^-, M_1^- + M_2^-, Y_2^+ + Y_2^-, L_1^+ + L_1^-, V_1^+ + V_1^-]$ | (1, 1)                                     |
| $[(\blacksquare)^{2T}, A_1^- + A_2^-, M_1^- + M_2^-, Y_2^+ + Y_2^-, L_1^+ + L_1^-, 2V_1^-]$        | (0, 1)                                     |
| $[(\blacksquare)^{2T}, A_1^- + A_2^-, M_1^+ + M_2^+, Y_2^+ + Y_2^-, L_1^+ + L_1^-, 2V_1^+]$        | trivial                                    |
| $[(\blacksquare)^{2T}, A_1^- + A_2^-, M_1^+ + M_2^+, Y_2^+ + Y_2^-, L_1^+ + L_1^-, V_1^+ + V_1^-]$ | (1, 0)                                     |
| $[(\blacksquare)^{2T}, A_1^- + A_2^-, M_1^+ + M_2^+, Y_2^+ + Y_2^-, L_1^+ + L_1^-, 2V_1^-]$        | trivial                                    |
| $[(\blacksquare)^{2T}, A_1^- + A_2^-, M_1^- + M_2^-, Y_2^+ + Y_2^-, 2L_1^+, 2V_1^+]$               | (1, 1)                                     |
| $[(\blacksquare)^{2T}, A_1^- + A_2^-, M_1^- + M_2^-, Y_2^+ + Y_2^-, 2L_1^+, V_1^+ + V_1^-]$        | (0, 1)                                     |
| $[(\blacksquare)^{2T}, A_1^- + A_2^-, M_1^- + M_2^-, Y_2^+ + Y_2^-, 2L_1^+, 2V_1^-]$               | (1, 1)                                     |
| $[(\blacksquare)^{2T}, A_1^- + A_2^-, M_1^+ + M_2^+, Y_2^+ + Y_2^-, 2L_1^+, 2V_1^+]$               | (1, 0)                                     |
| $[(\blacksquare)^{2T}, A_1^- + A_2^-, M_1^+ + M_2^+, Y_2^+ + Y_2^-, 2L_1^+, V_1^+ + V_1^-]$        | trivial                                    |
| $[(\blacksquare)^{2T}, A_1^- + A_2^-, M_1^+ + M_2^+, Y_2^+ + Y_2^-, 2L_1^+, 2V_1^-]$               | (1, 0)                                     |
| $[(\blacksquare)^{2T}, A_1^+ + A_2^+, M_1^- + M_2^-, Y_2^+ + Y_2^-, 2L_1^-, 2V_1^+]$               | (1, 0)                                     |
| $[(\blacksquare)^{2T}, A_1^+ + A_2^+, M_1^- + M_2^-, Y_2^+ + Y_2^-, 2L_1^-, V_1^+ + V_1^-]$        | trivial                                    |
| $[(\blacksquare)^{2T}, A_1^+ + A_2^+, M_1^- + M_2^-, Y_2^+ + Y_2^-, 2L_1^-, 2V_1^-]$               | (1, 0)                                     |
| $[(\blacksquare)^{2T}, A_1^+ + A_2^+, M_1^+ + M_2^+, Y_2^+ + Y_2^-, 2L_1^-, 2V_1^+]$               | (1, 1)                                     |
| $[(\blacksquare)^{2T}, A_1^+ + A_2^+, M_1^+ + M_2^+, Y_2^+ + Y_2^-, 2L_1^-, V_1^+ + V_1^-]$        | (0, 1)                                     |
| $[(\blacksquare)^{2T}, A_1^+ + A_2^+, M_1^+ + M_2^+, Y_2^+ + Y_2^-, 2L_1^-, 2V_1^-]$               | (1, 1)                                     |
| $[(\blacksquare)^{2T}, A_1^+ + A_2^+, M_1^- + M_2^-, Y_2^+ + Y_2^-, L_1^+ + L_1^-, 2V_1^+]$        | trivial                                    |
| $[(\blacksquare)^{2T}, A_1^+ + A_2^+, M_1^- + M_2^-, Y_2^+ + Y_2^-, L_1^+ + L_1^-, V_1^+ + V_1^-]$ | (1, 0)                                     |

... continued on next page

... continued from previous page

|                                                                                               |         |
|-----------------------------------------------------------------------------------------------|---------|
| $[(\bullet)^{2T}, A_1^+ + A_2^+, M_1^- + M_2^-, Y_2^+ + Y_2^-, L_1^+ + L_1^-, 2V_1^-]$        | trivial |
| $[(\bullet)^{2T}, A_1^+ + A_2^+, M_1^+ + M_2^+, Y_2^+ + Y_2^-, L_1^+ + L_1^-, 2V_1^+]$        | (0, 1)  |
| $[(\bullet)^{2T}, A_1^+ + A_2^+, M_1^+ + M_2^+, Y_2^+ + Y_2^-, L_1^+ + L_1^-, V_1^+ + V_1^-]$ | (1, 1)  |
| $[(\bullet)^{2T}, A_1^+ + A_2^+, M_1^+ + M_2^+, Y_2^+ + Y_2^-, L_1^+ + L_1^-, 2V_1^-]$        | (0, 1)  |
| $[(\bullet)^{2T}, A_1^+ + A_2^+, M_1^- + M_2^-, Y_2^+ + Y_2^-, 2L_1^+, 2V_1^+]$               | (1, 0)  |
| $[(\bullet)^{2T}, A_1^+ + A_2^+, M_1^- + M_2^-, Y_2^+ + Y_2^-, 2L_1^+, V_1^+ + V_1^-]$        | trivial |
| $[(\bullet)^{2T}, A_1^+ + A_2^+, M_1^- + M_2^-, Y_2^+ + Y_2^-, 2L_1^+, 2V_1^-]$               | (1, 0)  |
| $[(\bullet)^{2T}, A_1^+ + A_2^+, M_1^+ + M_2^+, Y_2^+ + Y_2^-, 2L_1^+, 2V_1^+]$               | (1, 1)  |
| $[(\bullet)^{2T}, A_1^+ + A_2^+, M_1^+ + M_2^+, Y_2^+ + Y_2^-, 2L_1^+, V_1^+ + V_1^-]$        | (0, 1)  |
| $[(\bullet)^{2T}, A_1^+ + A_2^+, M_1^+ + M_2^+, Y_2^+ + Y_2^-, 2L_1^+, 2V_1^-]$               | (1, 1)  |
| $[(\bullet)^{2T}, A_1^+ + A_1^-, M_1^+ + M_1^-, Y_2^+ + Y_2^-, 2L_1^-, 2V_1^+]$               | (0, 1)  |
| $[(\bullet)^{2T}, A_1^+ + A_1^-, M_1^+ + M_1^-, Y_2^+ + Y_2^-, 2L_1^-, V_1^+ + V_1^-]$        | (1, 1)  |
| $[(\bullet)^{2T}, A_1^+ + A_1^-, M_1^+ + M_1^-, Y_2^+ + Y_2^-, 2L_1^-, 2V_1^-]$               | (0, 1)  |
| $[(\bullet)^{2T}, A_1^+ + A_1^-, M_1^+ + M_1^-, Y_2^+ + Y_2^-, L_1^+ + L_1^-, 2V_1^+]$        | (1, 1)  |
| $[(\bullet)^{2T}, A_1^+ + A_1^-, M_1^+ + M_1^-, Y_2^+ + Y_2^-, L_1^+ + L_1^-, V_1^+ + V_1^-]$ | (0, 1)  |
| $[(\bullet)^{2T}, A_1^+ + A_1^-, M_1^+ + M_1^-, Y_2^+ + Y_2^-, L_1^+ + L_1^-, 2V_1^-]$        | (1, 1)  |
| $[(\bullet)^{2T}, A_1^+ + A_1^-, M_1^+ + M_1^-, Y_2^+ + Y_2^-, 2L_1^+, 2V_1^+]$               | (0, 1)  |
| $[(\bullet)^{2T}, A_1^+ + A_1^-, M_1^+ + M_1^-, Y_2^+ + Y_2^-, 2L_1^+, V_1^+ + V_1^-]$        | (1, 1)  |
| $[(\bullet)^{2T}, A_1^+ + A_1^-, M_1^+ + M_1^-, Y_2^+ + Y_2^-, 2L_1^+, 2V_1^-]$               | (0, 1)  |

2nd minimal solution:  $\mu_2^T = 3$  (960 symmetry vectors)Space group 13 ( $\mathbb{Z}_2 \times \mathbb{Z}_2$ )1st minimal solution:  $\mu_1^T = 2$  (6 symmetry vectors & filling-enforced topology)

| $\mathbf{n}^T$                                                                      | $\mathbf{v}^T \in \mathbb{Z}_2 \times \mathbb{Z}_2$ |
|-------------------------------------------------------------------------------------|-----------------------------------------------------|
| $[(\bullet)^{2T}, A_1, B_1, C_1^+ + C_2^+, D_1, E_1, Y_1^- + Y_2^-, Z_2^+ + Z_2^-]$ | (0, 1)                                              |
| $[(\bullet)^{2T}, A_1, B_1, C_1^+ + C_2^+, D_1, E_1, Y_1^+ + Y_2^+, Z_2^+ + Z_2^-]$ | (1, 1)                                              |
| $[(\bullet)^{2T}, A_1, B_1, C_1^+ + C_1^-, D_1, E_1, Y_1^+ + Y_1^-, Z_2^+ + Z_2^-]$ | (1, 0)                                              |
| $[(\bullet)^{2T}, A_1, B_1, C_2^+ + C_2^-, D_1, E_1, Y_2^+ + Y_2^-, Z_2^+ + Z_2^-]$ | (1, 0)                                              |
| $[(\bullet)^{2T}, A_1, B_1, C_1^- + C_2^-, D_1, E_1, Y_1^- + Y_2^-, Z_2^+ + Z_2^-]$ | (1, 1)                                              |
| $[(\bullet)^{2T}, A_1, B_1, C_1^- + C_2^-, D_1, E_1, Y_1^+ + Y_2^+, Z_2^+ + Z_2^-]$ | (0, 1)                                              |

2nd minimal solution:  $\mu_2^T = 4$  (152 symmetry vectors)Space group 14 ( $\mathbb{Z}_2$ )1st minimal solution:  $\mu_1^T = 4$  (27 symmetry vectors)

| $\mathbf{n}^T$                                                                                                                                      | $\mathbf{v}^T \in \mathbb{Z}_2$ |
|-----------------------------------------------------------------------------------------------------------------------------------------------------|---------------------------------|
| $[(\bullet)^{2T} + \Gamma_1^+ + \Gamma_1^-, 2A_1, 2B_1, 2C_1, 2D_1^+ + 2D_2^+, 2E_1^- + 2E_2^-, 2Y_1^- + 2Y_2^-, 2Z_1]$                             | trivial                         |
| $[(\bullet)^{2T} + \Gamma_1^+ + \Gamma_1^-, 2A_1, 2B_1, 2C_1, 2D_1^+ + 2D_2^+, 2E_1^- + 2E_2^-, Y_1^+ + Y_1^- + Y_2^+ + Y_2^-, 2Z_1]$               | 1                               |
| $[(\bullet)^{2T} + \Gamma_1^+ + \Gamma_1^-, 2A_1, 2B_1, 2C_1, 2D_1^+ + 2D_2^+, E_1^+ + E_1^- + E_2^+ + E_2^-, 2Y_1^- + 2Y_2^-, 2Z_1]$               | 1                               |
| $[(\bullet)^{2T} + \Gamma_1^+ + \Gamma_1^-, 2A_1, 2B_1, 2C_1, 2D_1^+ + 2D_2^+, E_1^+ + E_1^- + E_2^+ + E_2^-, Y_1^+ + Y_1^- + Y_2^+ + Y_2^-, 2Z_1]$ | trivial                         |
| $[(\bullet)^{2T} + \Gamma_1^+ + \Gamma_1^-, 2A_1, 2B_1, 2C_1, D_1^+ + D_1^- + D_2^+ + D_2^-, 2E_1^- + 2E_2^-, 2Y_1^- + 2Y_2^-, 2Z_1]$               | 1                               |
| $[(\bullet)^{2T} + \Gamma_1^+ + \Gamma_1^-, 2A_1, 2B_1, 2C_1, D_1^+ + D_1^- + D_2^+ + D_2^-, 2E_1^- + 2E_2^-, Y_1^+ + Y_1^- + Y_2^+ + Y_2^-, 2Z_1]$ | trivial                         |

... continued on next page

... continued from previous page

|                                                                                                                                                                   |         |
|-------------------------------------------------------------------------------------------------------------------------------------------------------------------|---------|
| $[(\bullet)^{2T} + \Gamma_1^+ + \Gamma_1^-, 2A_1, 2B_1, 2C_1, D_1^+ + D_1^- + D_2^+ + D_2^-, E_1^+ + E_1^- + E_2^+ + E_2^-, 2Y_1^- + 2Y_2^-, 2Z_1]$               | trivial |
| $[(\bullet)^{2T} + \Gamma_1^+ + \Gamma_1^-, 2A_1, 2B_1, 2C_1, D_1^+ + D_1^- + D_2^+ + D_2^-, E_1^+ + E_1^- + E_2^+ + E_2^-, Y_1^+ + Y_1^- + Y_2^+ + Y_2^-, 2Z_1]$ | 1       |
| $[(\bullet)^{2T} + \Gamma_1^+ + \Gamma_1^-, 2A_1, 2B_1, 2C_1, 2D_1^+ + 2D_2^+, 2E_1^- + 2E_2^-, 2Y_1^+ + 2Y_2^+, 2Z_1]$                                           | trivial |
| $[(\bullet)^{2T} + \Gamma_1^+ + \Gamma_1^-, 2A_1, 2B_1, 2C_1, 2D_1^+ + 2D_2^+, E_1^+ + E_1^- + E_2^+ + E_2^-, 2Y_1^+ + 2Y_2^+, 2Z_1]$                             | 1       |
| $[(\bullet)^{2T} + \Gamma_1^+ + \Gamma_1^-, 2A_1, 2B_1, 2C_1, D_1^+ + D_1^- + D_2^+ + D_2^-, 2E_1^- + 2E_2^-, 2Y_1^+ + 2Y_2^+, 2Z_1]$                             | 1       |
| $[(\bullet)^{2T} + \Gamma_1^+ + \Gamma_1^-, 2A_1, 2B_1, 2C_1, D_1^+ + D_1^- + D_2^+ + D_2^-, E_1^+ + E_1^- + E_2^+ + E_2^-, 2Y_1^+ + 2Y_2^+, 2Z_1]$               | trivial |
| $[(\bullet)^{2T} + \Gamma_1^+ + \Gamma_1^-, 2A_1, 2B_1, 2C_1, 2D_1^+ + 2D_2^+, 2E_1^+ + 2E_2^+, 2Y_1^- + 2Y_2^-, 2Z_1]$                                           | trivial |
| $[(\bullet)^{2T} + \Gamma_1^+ + \Gamma_1^-, 2A_1, 2B_1, 2C_1, 2D_1^+ + 2D_2^+, 2E_1^+ + 2E_2^+, Y_1^+ + Y_1^- + Y_2^+ + Y_2^-, 2Z_1]$                             | 1       |
| $[(\bullet)^{2T} + \Gamma_1^+ + \Gamma_1^-, 2A_1, 2B_1, 2C_1, D_1^+ + D_1^- + D_2^+ + D_2^-, 2E_1^+ + 2E_2^+, 2Y_1^- + 2Y_2^-, 2Z_1]$                             | 1       |
| $[(\bullet)^{2T} + \Gamma_1^+ + \Gamma_1^-, 2A_1, 2B_1, 2C_1, D_1^+ + D_1^- + D_2^+ + D_2^-, 2E_1^+ + 2E_2^+, Y_1^+ + Y_1^- + Y_2^+ + Y_2^-, 2Z_1]$               | trivial |
| $[(\bullet)^{2T} + \Gamma_1^+ + \Gamma_1^-, 2A_1, 2B_1, 2C_1, 2D_1^+ + 2D_2^+, 2E_1^+ + 2E_2^+, 2Y_1^+ + 2Y_2^+, 2Z_1]$                                           | trivial |
| $[(\bullet)^{2T} + \Gamma_1^+ + \Gamma_1^-, 2A_1, 2B_1, 2C_1, D_1^+ + D_1^- + D_2^+ + D_2^-, 2E_1^+ + 2E_2^+, 2Y_1^+ + 2Y_2^+, 2Z_1]$                             | 1       |
| $[(\bullet)^{2T} + \Gamma_1^+ + \Gamma_1^-, 2A_1, 2B_1, 2C_1, 2D_1^- + 2D_2^-, 2E_1^- + 2E_2^-, 2Y_1^- + 2Y_2^-, 2Z_1]$                                           | trivial |
| $[(\bullet)^{2T} + \Gamma_1^+ + \Gamma_1^-, 2A_1, 2B_1, 2C_1, 2D_1^- + 2D_2^-, 2E_1^- + 2E_2^-, Y_1^+ + Y_1^- + Y_2^+ + Y_2^-, 2Z_1]$                             | 1       |
| $[(\bullet)^{2T} + \Gamma_1^+ + \Gamma_1^-, 2A_1, 2B_1, 2C_1, 2D_1^- + 2D_2^-, E_1^+ + E_1^- + E_2^+ + E_2^-, 2Y_1^- + 2Y_2^-, 2Z_1]$                             | 1       |
| $[(\bullet)^{2T} + \Gamma_1^+ + \Gamma_1^-, 2A_1, 2B_1, 2C_1, 2D_1^- + 2D_2^-, E_1^+ + E_1^- + E_2^+ + E_2^-, Y_1^+ + Y_1^- + Y_2^+ + Y_2^-, 2Z_1]$               | trivial |
| $[(\bullet)^{2T} + \Gamma_1^+ + \Gamma_1^-, 2A_1, 2B_1, 2C_1, 2D_1^- + 2D_2^-, 2E_1^- + 2E_2^-, 2Y_1^+ + 2Y_2^+, 2Z_1]$                                           | trivial |
| $[(\bullet)^{2T} + \Gamma_1^+ + \Gamma_1^-, 2A_1, 2B_1, 2C_1, 2D_1^- + 2D_2^-, E_1^+ + E_1^- + E_2^+ + E_2^-, 2Y_1^+ + 2Y_2^+, 2Z_1]$                             | 1       |
| $[(\bullet)^{2T} + \Gamma_1^+ + \Gamma_1^-, 2A_1, 2B_1, 2C_1, 2D_1^- + 2D_2^-, 2E_1^+ + 2E_2^+, 2Y_1^- + 2Y_2^-, 2Z_1]$                                           | trivial |
| $[(\bullet)^{2T} + \Gamma_1^+ + \Gamma_1^-, 2A_1, 2B_1, 2C_1, 2D_1^- + 2D_2^-, 2E_1^+ + 2E_2^+, Y_1^+ + Y_1^- + Y_2^+ + Y_2^-, 2Z_1]$                             | 1       |
| $[(\bullet)^{2T} + \Gamma_1^+ + \Gamma_1^-, 2A_1, 2B_1, 2C_1, 2D_1^- + 2D_2^-, 2E_1^+ + 2E_2^+, 2Y_1^+ + 2Y_2^+, 2Z_1]$                                           | trivial |

2nd minimal solution:  $\mu_2^T = 6$  (128 symmetry vectors)

Space group 15 ( $\mathbb{Z}_2 \times \mathbb{Z}_2$ )

1st minimal solution:  $\mu_1^T = 2$  (9 symmetry vectors)

| $\mathbf{n}^T$                                                            | $\mathbf{v}^T \in \mathbb{Z}_2 \times \mathbb{Z}_2$ |
|---------------------------------------------------------------------------|-----------------------------------------------------|
| $[(\bullet)^{2T}, A_1, M_1, Y_2^+ + Y_2^-, 2L_1^-, 2V_1^-]$               | trivial                                             |
| $[(\bullet)^{2T}, A_1, M_1, Y_2^+ + Y_2^-, L_1^+ + L_1^-, 2V_1^-]$        | (1, 0)                                              |
| $[(\bullet)^{2T}, A_1, M_1, Y_2^+ + Y_2^-, 2L_1^+, 2V_1^-]$               | trivial                                             |
| $[(\bullet)^{2T}, A_1, M_1, Y_2^+ + Y_2^-, 2L_1^-, V_1^+ + V_1^-]$        | (1, 1)                                              |
| $[(\bullet)^{2T}, A_1, M_1, Y_2^+ + Y_2^-, L_1^+ + L_1^-, V_1^+ + V_1^-]$ | (0, 1)                                              |
| $[(\bullet)^{2T}, A_1, M_1, Y_2^+ + Y_2^-, 2L_1^+, V_1^+ + V_1^-]$        | (1, 1)                                              |
| $[(\bullet)^{2T}, A_1, M_1, Y_2^+ + Y_2^-, 2L_1^-, 2V_1^+]$               | trivial                                             |
| $[(\bullet)^{2T}, A_1, M_1, Y_2^+ + Y_2^-, L_1^+ + L_1^-, 2V_1^+]$        | (1, 0)                                              |
| $[(\bullet)^{2T}, A_1, M_1, Y_2^+ + Y_2^-, 2L_1^+, 2V_1^+]$               | trivial                                             |

2nd minimal solution:  $\mu_2^T = 4$  (200 symmetry vectors)

Space group 16 ( $\mathbb{Z}_1$ )

1st minimal solution:  $\mu_1^T = 2$  (28 symmetry vectors)

| $\mathbf{n}^T$                                                                             |
|--------------------------------------------------------------------------------------------|
| $[(\bullet)^{2T}, R_3 + R_4, S_3 + S_4, T_1 + T_4, U_2 + U_4, X_2 + X_4, Y_2 + Y_3, 2Z_4]$ |

... continued on next page

... continued from previous page

---

|                                                                                                 |
|-------------------------------------------------------------------------------------------------|
| $[(\blacksquare)^{2T}, R_2 + R_3, S_2 + S_3, T_1 + T_4, 2U_2, 2X_2, Y_2 + Y_3, 2Z_4]$           |
| $[(\blacksquare)^{2T}, 2R_4, S_3 + S_4, T_2 + T_4, U_1 + U_4, X_2 + X_4, Y_2 + Y_3, Z_3 + Z_4]$ |
| $[(\blacksquare)^{2T}, R_3 + R_4, 2S_3, T_3 + T_4, U_1 + U_2, 2X_2, 2Y_3, Z_3 + Z_4]$           |
| $[(\blacksquare)^{2T}, R_2 + R_4, S_2 + S_3, T_2 + T_4, U_1 + U_2, 2X_2, Y_2 + Y_3, Z_3 + Z_4]$ |
| $[(\blacksquare)^{2T}, R_1 + R_4, S_1 + S_3, T_3 + T_4, U_1 + U_4, X_2 + X_4, 2Y_3, Z_3 + Z_4]$ |
| $[(\blacksquare)^{2T}, R_2 + R_4, S_1 + S_4, T_2 + T_4, U_3 + U_4, 2X_4, Y_2 + Y_3, Z_3 + Z_4]$ |
| $[(\blacksquare)^{2T}, R_2 + R_3, S_1 + S_3, T_3 + T_4, U_2 + U_3, X_2 + X_4, 2Y_3, Z_3 + Z_4]$ |
| $[(\blacksquare)^{2T}, 2R_2, S_1 + S_2, T_2 + T_4, U_2 + U_3, X_2 + X_4, Y_2 + Y_3, Z_3 + Z_4]$ |
| $[(\blacksquare)^{2T}, R_1 + R_2, 2S_1, T_3 + T_4, U_3 + U_4, 2X_4, 2Y_3, Z_3 + Z_4]$           |
| $[(\blacksquare)^{2T}, R_1 + R_4, S_1 + S_4, T_1 + T_4, 2U_4, 2X_4, Y_2 + Y_3, 2Z_4]$           |
| $[(\blacksquare)^{2T}, R_1 + R_2, S_1 + S_2, T_1 + T_4, U_2 + U_4, X_2 + X_4, Y_2 + Y_3, 2Z_4]$ |
| $[(\blacksquare)^{2T}, R_2 + R_4, S_1 + S_3, 2T_4, U_2 + U_4, X_2 + X_4, 2Y_3, 2Z_4]$           |
| $[(\blacksquare)^{2T}, 2R_3, S_3 + S_4, T_1 + T_3, U_2 + U_3, X_2 + X_4, Y_2 + Y_3, Z_3 + Z_4]$ |
| $[(\blacksquare)^{2T}, R_3 + R_4, S_3 + S_4, T_2 + T_3, U_1 + U_3, X_2 + X_4, Y_2 + Y_3, 2Z_3]$ |
| $[(\blacksquare)^{2T}, R_1 + R_3, S_1 + S_3, 2T_3, U_1 + U_3, X_2 + X_4, 2Y_3, 2Z_3]$           |
| $[(\blacksquare)^{2T}, R_2 + R_3, S_1 + S_4, T_2 + T_3, 2U_3, 2X_4, Y_2 + Y_3, 2Z_3]$           |
| $[(\blacksquare)^{2T}, R_1 + R_3, S_1 + S_4, T_1 + T_3, U_3 + U_4, 2X_4, Y_2 + Y_3, Z_3 + Z_4]$ |
| $[(\blacksquare)^{2T}, R_2 + R_3, S_2 + S_4, T_1 + T_2, U_2 + U_3, X_2 + X_4, 2Y_2, Z_3 + Z_4]$ |
| $[(\blacksquare)^{2T}, R_2 + R_4, S_2 + S_4, 2T_2, U_1 + U_3, X_2 + X_4, 2Y_2, 2Z_3]$           |
| $[(\blacksquare)^{2T}, R_1 + R_2, S_1 + S_2, T_2 + T_3, U_1 + U_3, X_2 + X_4, Y_2 + Y_3, 2Z_3]$ |
| $[(\blacksquare)^{2T}, R_1 + R_3, S_2 + S_4, 2T_1, U_2 + U_4, X_2 + X_4, 2Y_2, 2Z_4]$           |
| $[(\blacksquare)^{2T}, R_1 + R_4, S_2 + S_4, T_1 + T_2, U_1 + U_4, X_2 + X_4, 2Y_2, Z_3 + Z_4]$ |
| $[(\blacksquare)^{2T}, R_1 + R_3, S_2 + S_3, T_1 + T_3, U_1 + U_2, 2X_2, Y_2 + Y_3, Z_3 + Z_4]$ |
| $[(\blacksquare)^{2T}, R_1 + R_2, 2S_2, T_1 + T_2, U_1 + U_2, 2X_2, 2Y_2, Z_3 + Z_4]$           |
| $[(\blacksquare)^{2T}, 2R_1, S_1 + S_2, T_1 + T_3, U_1 + U_4, X_2 + X_4, Y_2 + Y_3, Z_3 + Z_4]$ |
| $[(\blacksquare)^{2T}, R_1 + R_4, S_2 + S_3, T_2 + T_3, 2U_1, 2X_2, Y_2 + Y_3, 2Z_3]$           |
| $[(\blacksquare)^{2T}, R_3 + R_4, 2S_4, T_1 + T_2, U_3 + U_4, 2X_4, 2Y_2, Z_3 + Z_4]$           |

---

2nd minimal solution:  $\mu_2^T = 3$  (920 symmetry vectors)

Space group 17 ( $\mathbb{Z}_1$ )

1st minimal solution:  $\mu_1^T = 4$  (10 symmetry vectors)

---

|                                                                                                                                  |
|----------------------------------------------------------------------------------------------------------------------------------|
| $\mathbf{n}^T$                                                                                                                   |
| $[(\blacksquare)^{2T} + 2\Gamma_2, 2R_1, S_1 + S_2 + S_3 + S_4, 2T_1, 2U_1, 2X_2 + 2X_4, 2Y_2 + 2Y_3, 2Z_1]$                     |
| $[(\blacksquare)^{2T} + \Gamma_1 + \Gamma_2, 2R_1, S_1 + S_2 + 2S_4, 2T_1, 2U_1, X_1 + X_2 + 2X_4, 2Y_2 + Y_3 + Y_4, 2Z_1]$      |
| $[(\blacksquare)^{2T} + \Gamma_1 + \Gamma_2, 2R_1, 2S_1 + S_3 + S_4, 2T_1, 2U_1, X_1 + X_2 + 2X_4, Y_1 + Y_2 + 2Y_3, 2Z_1]$      |
| $[(\blacksquare)^{2T} + \Gamma_1 + \Gamma_2, 2R_1, 2S_2 + S_3 + S_4, 2T_1, 2U_1, 2X_2 + X_3 + X_4, 2Y_2 + Y_3 + Y_4, 2Z_1]$      |
| $[(\blacksquare)^{2T} + \Gamma_1 + \Gamma_2, 2R_1, S_1 + S_2 + 2S_3, 2T_1, 2U_1, 2X_2 + X_3 + X_4, Y_1 + Y_2 + 2Y_3, 2Z_1]$      |
| $[(\blacksquare)^{2T} + 2\Gamma_1, 2R_1, 2S_2 + 2S_4, 2T_1, 2U_1, X_1 + X_2 + X_3 + X_4, 2Y_2 + 2Y_4, 2Z_1]$                     |
| $[(\blacksquare)^{2T} + 2\Gamma_1, 2R_1, S_1 + S_2 + S_3 + S_4, 2T_1, 2U_1, X_1 + X_2 + X_3 + X_4, Y_1 + Y_2 + Y_3 + Y_4, 2Z_1]$ |
| $[(\blacksquare)^{2T} + 2\Gamma_1, 2R_1, 2S_1 + 2S_3, 2T_1, 2U_1, X_1 + X_2 + X_3 + X_4, 2Y_1 + 2Y_3, 2Z_1]$                     |
| $[(\blacksquare)^{2T} + 2\Gamma_1, 2R_1, 2S_1 + 2S_4, 2T_1, 2U_1, 2X_1 + 2X_4, Y_1 + Y_2 + Y_3 + Y_4, 2Z_1]$                     |
| $[(\blacksquare)^{2T} + 2\Gamma_1, 2R_1, 2S_2 + 2S_3, 2T_1, 2U_1, 2X_2 + 2X_3, Y_1 + Y_2 + Y_3 + Y_4, 2Z_1]$                     |

---

2nd minimal solution:  $\mu_2^T = 6$  (48 symmetry vectors)

Space group 18 ( $\mathbb{Z}_1$ )

1st minimal solution:  $\mu_1^T = 4$  (3 symmetry vectors)

| $\mathbf{n}^T$                                                                                                                   |
|----------------------------------------------------------------------------------------------------------------------------------|
| $[(\blacksquare)^{2T} + 2\Gamma_1, 2R_3 + 2R_4, 2S_3 + 2S_4, 2T_1, 2U_1, 2X_1, 2Y_1, Z_1 + Z_2 + Z_3 + Z_4]$                     |
| $[(\blacksquare)^{2T} + 2\Gamma_1, R_1 + R_2 + R_3 + R_4, S_1 + S_2 + S_3 + S_4, 2T_1, 2U_1, 2X_1, 2Y_1, Z_1 + Z_2 + Z_3 + Z_4]$ |
| $[(\blacksquare)^{2T} + 2\Gamma_1, 2R_1 + 2R_2, 2S_1 + 2S_2, 2T_1, 2U_1, 2X_1, 2Y_1, Z_1 + Z_2 + Z_3 + Z_4]$                     |

2nd minimal solution:  $\mu_2^T = 6$  (8 symmetry vectors)

Space group 19 ( $\mathbb{Z}_1$ )

1st minimal solution:  $\mu_1^T = 4$  (1 symmetry vector)

| $\mathbf{n}^T$                                                                                                                   |
|----------------------------------------------------------------------------------------------------------------------------------|
| $[(\blacksquare)^{2T} + 2\Gamma_1, 2R_1, S_1 + S_2 + S_3 + S_4, T_1 + T_2 + T_3 + T_4, U_1 + U_2 + U_3 + U_4, 2X_1, 2Y_1, 2Z_1]$ |

2nd minimal solution:  $\mu_2^T = 8$  (1 symmetry vector)

Space group 20 ( $\mathbb{Z}_1$ )

1st minimal solution:  $\mu_1^T = 4$  (2 symmetry vectors)

| $\mathbf{n}^T$                                                                                        |
|-------------------------------------------------------------------------------------------------------|
| $[(\blacksquare)^{2T} + \Gamma_1 + \Gamma_2, 2T_1, 2Y_2 + Y_3 + Y_4, 2Z_1, 2R_1 + 2R_2, 2S_1 + 2S_2]$ |
| $[(\blacksquare)^{2T} + 2\Gamma_1, 2T_1, Y_1 + Y_2 + Y_3 + Y_4, 2Z_1, 2R_1 + 2R_2, 2S_1 + 2S_2]$      |

2nd minimal solution:  $\mu_2^T = 6$  (6 symmetry vectors)

Space group 21 ( $\mathbb{Z}_1$ )

1st minimal solution:  $\mu_1^T = 2$  (3 symmetry vectors)

| $\mathbf{n}^T$                                                            |
|---------------------------------------------------------------------------|
| $[(\blacksquare)^{2T}, T_1 + T_2, 2Y_2, Z_3 + Z_4, 2R_2, 2S_2]$           |
| $[(\blacksquare)^{2T}, T_1 + T_2, 2Y_2, Z_3 + Z_4, R_1 + R_2, S_1 + S_2]$ |
| $[(\blacksquare)^{2T}, T_1 + T_2, 2Y_2, Z_3 + Z_4, 2R_1, 2S_1]$           |

2nd minimal solution:  $\mu_2^T = 3$  (56 symmetry vectors)

Space group 22 ( $\mathbb{Z}_1$ )

1st minimal solution:  $\mu_1^T = 2$  (1 symmetry vector)

|                                                           |
|-----------------------------------------------------------|
| $\mathbf{n}^T$                                            |
| $[(\bullet)^{2T}, T_2 + T_4, Y_2 + Y_3, Z_3 + Z_4, 2L_1]$ |

2nd minimal solution:  $\mu_2^T = 3$  (14 symmetry vectors)

Space group 23 ( $\mathbb{Z}_1$ )

1st minimal solution:  $\mu_1^T = 3$  (20 symmetry vectors)

|                                                                                                                         |
|-------------------------------------------------------------------------------------------------------------------------|
| $\mathbf{n}^T$                                                                                                          |
| $[(\bullet)^{2T} + \Gamma_1, 3W_4, 3WA_4, X_2 + X_3 + X_4, 3R_1, 3S_2, 3T_2]$                                           |
| $[(\bullet)^{2T} + \Gamma_1, W_3 + 2W_4, WA_3 + 2WA_4, X_2 + X_3 + X_4, 2R_1 + R_2, S_1 + 2S_2, 3T_2]$                  |
| $[(\bullet)^{2T} + \Gamma_1, W_2 + 2W_4, WA_2 + 2WA_4, X_2 + X_3 + X_4, 2R_1 + R_2, 3S_2, T_1 + 2T_2]$                  |
| $[(\bullet)^{2T} + \Gamma_1, W_1 + 2W_4, WA_1 + 2WA_4, X_2 + X_3 + X_4, 3R_1, S_1 + 2S_2, T_1 + 2T_2]$                  |
| $[(\bullet)^{2T} + \Gamma_1, 2W_3 + W_4, 2WA_3 + WA_4, X_2 + X_3 + X_4, R_1 + 2R_2, 2S_1 + S_2, 3T_2]$                  |
| $[(\bullet)^{2T} + \Gamma_1, W_2 + W_3 + W_4, WA_2 + WA_3 + WA_4, X_2 + X_3 + X_4, R_1 + 2R_2, S_1 + 2S_2, T_1 + 2T_2]$ |
| $[(\bullet)^{2T} + \Gamma_1, W_1 + W_3 + W_4, WA_1 + WA_3 + WA_4, X_2 + X_3 + X_4, 2R_1 + R_2, 2S_1 + S_2, T_1 + 2T_2]$ |
| $[(\bullet)^{2T} + \Gamma_1, 2W_2 + W_4, 2WA_2 + WA_4, X_2 + X_3 + X_4, R_1 + 2R_2, 3S_2, 2T_1 + T_2]$                  |
| $[(\bullet)^{2T} + \Gamma_1, W_1 + W_2 + W_4, WA_1 + WA_2 + WA_4, X_2 + X_3 + X_4, 2R_1 + R_2, S_1 + 2S_2, 2T_1 + T_2]$ |
| $[(\bullet)^{2T} + \Gamma_1, 2W_1 + W_4, 2WA_1 + WA_4, X_2 + X_3 + X_4, 3R_1, 2S_1 + S_2, 2T_1 + T_2]$                  |
| $[(\bullet)^{2T} + \Gamma_1, 3W_3, 3WA_3, X_2 + X_3 + X_4, 3R_2, 3S_1, 3T_2]$                                           |
| $[(\bullet)^{2T} + \Gamma_1, W_2 + 2W_3, WA_2 + 2WA_3, X_2 + X_3 + X_4, 3R_2, 2S_1 + S_2, T_1 + 2T_2]$                  |
| $[(\bullet)^{2T} + \Gamma_1, W_1 + 2W_3, WA_1 + 2WA_3, X_2 + X_3 + X_4, R_1 + 2R_2, 3S_1, T_1 + 2T_2]$                  |
| $[(\bullet)^{2T} + \Gamma_1, 2W_2 + W_3, 2WA_2 + WA_3, X_2 + X_3 + X_4, 3R_2, S_1 + 2S_2, 2T_1 + T_2]$                  |
| $[(\bullet)^{2T} + \Gamma_1, W_1 + W_2 + W_3, WA_1 + WA_2 + WA_3, X_2 + X_3 + X_4, R_1 + 2R_2, 2S_1 + S_2, 2T_1 + T_2]$ |
| $[(\bullet)^{2T} + \Gamma_1, 2W_1 + W_3, 2WA_1 + WA_3, X_2 + X_3 + X_4, 2R_1 + R_2, 3S_1, 2T_1 + T_2]$                  |
| $[(\bullet)^{2T} + \Gamma_1, 3W_2, 3WA_2, X_2 + X_3 + X_4, 3R_2, 3S_2, 3T_1]$                                           |
| $[(\bullet)^{2T} + \Gamma_1, W_1 + 2W_2, WA_1 + 2WA_2, X_2 + X_3 + X_4, R_1 + 2R_2, S_1 + 2S_2, 3T_1]$                  |
| $[(\bullet)^{2T} + \Gamma_1, 2W_1 + W_2, 2WA_1 + WA_2, X_2 + X_3 + X_4, 2R_1 + R_2, 2S_1 + S_2, 3T_1]$                  |
| $[(\bullet)^{2T} + \Gamma_1, 3W_1, 3WA_1, X_2 + X_3 + X_4, 3R_1, 3S_1, 3T_1]$                                           |

2nd minimal solution:  $\mu_2^T = 4$  (140 symmetry vectors)

Space group 24 ( $\mathbb{Z}_1$ )

1st minimal solution:  $\mu_1^T = 2$  (1 symmetry vector)

|                                                                      |
|----------------------------------------------------------------------|
| $\mathbf{n}^T$                                                       |
| $[(\bullet)^{2T}, W_1, WA_1, 2X_4, R_1 + R_2, S_1 + S_2, T_1 + T_2]$ |

2nd minimal solution:  $\mu_2^T = 4$  (7 symmetry vectors)



Space group 25 ( $\mathbb{Z}_1$ )

1st minimal solution:  $\mu_1^T = 2$  (20 symmetry vectors)

| $\mathbf{n}^T$                                                                                       |
|------------------------------------------------------------------------------------------------------|
| $[(\blacksquare)^{2T}, 2R_3, 2S_3, T_2 + T_3, U_1 + U_3, X_1 + X_3, Y_2 + Y_3, Z_3 + Z_4]$           |
| $[(\blacksquare)^{2T}, R_3 + R_4, S_3 + S_4, T_1 + T_2, U_3 + U_4, X_3 + X_4, Y_1 + Y_2, Z_3 + Z_4]$ |
| $[(\blacksquare)^{2T}, R_2 + R_3, S_2 + S_3, T_2 + T_3, U_3 + U_4, X_3 + X_4, Y_2 + Y_3, Z_3 + Z_4]$ |
| $[(\blacksquare)^{2T}, R_1 + R_3, S_1 + S_3, T_1 + T_2, U_1 + U_3, X_1 + X_3, Y_1 + Y_2, Z_3 + Z_4]$ |
| $[(\blacksquare)^{2T}, R_3 + R_4, S_3 + S_4, T_3 + T_4, U_3 + U_4, X_3 + X_4, Y_3 + Y_4, Z_3 + Z_4]$ |
| $[(\blacksquare)^{2T}, R_1 + R_4, S_1 + S_4, T_1 + T_4, U_3 + U_4, X_3 + X_4, Y_1 + Y_4, Z_3 + Z_4]$ |
| $[(\blacksquare)^{2T}, R_1 + R_2, S_1 + S_2, T_1 + T_2, U_3 + U_4, X_3 + X_4, Y_1 + Y_2, Z_3 + Z_4]$ |
| $[(\blacksquare)^{2T}, R_1 + R_3, S_1 + S_3, T_3 + T_4, U_1 + U_3, X_1 + X_3, Y_3 + Y_4, Z_3 + Z_4]$ |
| $[(\blacksquare)^{2T}, R_1 + R_2, S_1 + S_2, T_3 + T_4, U_3 + U_4, X_3 + X_4, Y_3 + Y_4, Z_3 + Z_4]$ |
| $[(\blacksquare)^{2T}, 2R_1, 2S_1, T_1 + T_4, U_1 + U_3, X_1 + X_3, Y_1 + Y_4, Z_3 + Z_4]$           |
| $[(\blacksquare)^{2T}, R_3 + R_4, S_3 + S_4, T_1 + T_2, U_1 + U_2, X_1 + X_2, Y_1 + Y_2, Z_3 + Z_4]$ |
| $[(\blacksquare)^{2T}, R_2 + R_4, S_2 + S_4, T_1 + T_2, U_2 + U_4, X_2 + X_4, Y_1 + Y_2, Z_3 + Z_4]$ |
| $[(\blacksquare)^{2T}, 2R_4, 2S_4, T_1 + T_4, U_2 + U_4, X_2 + X_4, Y_1 + Y_4, Z_3 + Z_4]$           |
| $[(\blacksquare)^{2T}, R_1 + R_4, S_1 + S_4, T_1 + T_4, U_1 + U_2, X_1 + X_2, Y_1 + Y_4, Z_3 + Z_4]$ |
| $[(\blacksquare)^{2T}, R_2 + R_3, S_2 + S_3, T_2 + T_3, U_1 + U_2, X_1 + X_2, Y_2 + Y_3, Z_3 + Z_4]$ |
| $[(\blacksquare)^{2T}, 2R_2, 2S_2, T_2 + T_3, U_2 + U_4, X_2 + X_4, Y_2 + Y_3, Z_3 + Z_4]$           |
| $[(\blacksquare)^{2T}, R_1 + R_2, S_1 + S_2, T_1 + T_2, U_1 + U_2, X_1 + X_2, Y_1 + Y_2, Z_3 + Z_4]$ |
| $[(\blacksquare)^{2T}, R_2 + R_4, S_2 + S_4, T_3 + T_4, U_2 + U_4, X_2 + X_4, Y_3 + Y_4, Z_3 + Z_4]$ |
| $[(\blacksquare)^{2T}, R_1 + R_2, S_1 + S_2, T_3 + T_4, U_1 + U_2, X_1 + X_2, Y_3 + Y_4, Z_3 + Z_4]$ |
| $[(\blacksquare)^{2T}, R_3 + R_4, S_3 + S_4, T_3 + T_4, U_1 + U_2, X_1 + X_2, Y_3 + Y_4, Z_3 + Z_4]$ |

2nd minimal solution:  $\mu_2^T = 3$  (208 symmetry vectors)

Space group 26 ( $\mathbb{Z}_1$ )

1st minimal solution:  $\mu_1^T = 4$  (3 symmetry vectors)

| $\mathbf{n}^T$                                                                                                                                                                                                 |
|----------------------------------------------------------------------------------------------------------------------------------------------------------------------------------------------------------------|
| $[(\blacksquare)^{2T} + \Gamma_1 + \Gamma_2, 2R_2 + 2R_4, 2S_2 + 2S_4, T_1 + T_2 + T_3 + T_4, 2U_2 + 2U_4, 2X_2 + 2X_4, Y_1 + Y_2 + Y_3 + Y_4, Z_1 + Z_2 + Z_3 + Z_4]$                                         |
| $[(\blacksquare)^{2T} + \Gamma_1 + \Gamma_2, R_1 + R_2 + R_3 + R_4, S_1 + S_2 + S_3 + S_4, T_1 + T_2 + T_3 + T_4, U_1 + U_2 + U_3 + U_4, X_1 + X_2 + X_3 + X_4, Y_1 + Y_2 + Y_3 + Y_4, Z_1 + Z_2 + Z_3 + Z_4]$ |
| $[(\blacksquare)^{2T} + \Gamma_1 + \Gamma_2, 2R_1 + 2R_3, 2S_1 + 2S_3, T_1 + T_2 + T_3 + T_4, 2U_1 + 2U_3, 2X_1 + 2X_3, Y_1 + Y_2 + Y_3 + Y_4, Z_1 + Z_2 + Z_3 + Z_4]$                                         |

2nd minimal solution:  $\mu_2^T = 6$  (8 symmetry vectors)

Space group 27 ( $\mathbb{Z}_2$ )

1st minimal solution:  $\mu_1^T = 2$  (8 symmetry vectors)

| $\mathbf{n}^T$                                                                                       | $\mathbf{v}^T \in \mathbb{Z}_2$ |
|------------------------------------------------------------------------------------------------------|---------------------------------|
| $[(\blacksquare)^{2T}, R_3 + R_4, S_3 + S_4, T_3 + T_4, U_3 + U_4, X_3 + X_4, Y_3 + Y_4, Z_3 + Z_4]$ | trivial                         |
| $[(\blacksquare)^{2T}, R_3 + R_4, S_3 + S_4, T_3 + T_4, U_1 + U_2, X_1 + X_2, Y_3 + Y_4, Z_3 + Z_4]$ | 1                               |
| $[(\blacksquare)^{2T}, R_3 + R_4, S_3 + S_4, T_1 + T_2, U_3 + U_4, X_3 + X_4, Y_1 + Y_2, Z_3 + Z_4]$ | 1                               |

... continued on next page

... continued from previous page

|                                                                                                      |         |
|------------------------------------------------------------------------------------------------------|---------|
| $[(\blacksquare)^{2T}, R_3 + R_4, S_3 + S_4, T_1 + T_2, U_1 + U_2, X_1 + X_2, Y_1 + Y_2, Z_3 + Z_4]$ | trivial |
| $[(\blacksquare)^{2T}, R_1 + R_2, S_1 + S_2, T_3 + T_4, U_3 + U_4, X_3 + X_4, Y_3 + Y_4, Z_3 + Z_4]$ | 1       |
| $[(\blacksquare)^{2T}, R_1 + R_2, S_1 + S_2, T_3 + T_4, U_1 + U_2, X_1 + X_2, Y_3 + Y_4, Z_3 + Z_4]$ | trivial |
| $[(\blacksquare)^{2T}, R_1 + R_2, S_1 + S_2, T_1 + T_2, U_3 + U_4, X_3 + X_4, Y_1 + Y_2, Z_3 + Z_4]$ | trivial |
| $[(\blacksquare)^{2T}, R_1 + R_2, S_1 + S_2, T_1 + T_2, U_1 + U_2, X_1 + X_2, Y_1 + Y_2, Z_3 + Z_4]$ | 1       |

2nd minimal solution:  $\mu_2^T = 4$  (54 symmetry vectors)

Space group 28 ( $\mathbb{Z}_4$ )

1st minimal solution:  $\mu_1^T = 2$  (2 symmetry vectors)

| $\mathbf{n}^T$                                                               |
|------------------------------------------------------------------------------|
| $[(\blacksquare)^{2T}, R_1, S_1, T_1 + T_2, U_1, X_1, Y_1 + Y_2, Z_3 + Z_4]$ |
| $[(\blacksquare)^{2T}, R_1, S_1, T_3 + T_4, U_1, X_1, Y_3 + Y_4, Z_3 + Z_4]$ |

2nd minimal solution:  $\mu_2^T = 4$  (10 symmetry vectors)

Space group 29 ( $\mathbb{Z}_4$ )

1st minimal solution:  $\mu_1^T = 4$  (1 symmetry vector)

| $\mathbf{n}^T$                                                                                                                             |
|--------------------------------------------------------------------------------------------------------------------------------------------|
| $[(\blacksquare)^{2T} + \Gamma_1 + \Gamma_2, 2R_1, 2S_1, T_1 + T_2 + T_3 + T_4, 2U_1, 2X_1, Y_1 + Y_2 + Y_3 + Y_4, Z_1 + Z_2 + Z_3 + Z_4]$ |

2nd minimal solution:  $\mu_2^T = 8$  (1 symmetry vector)

Space group 30 ( $\mathbb{Z}_4$ )

1st minimal solution:  $\mu_1^T = 2$  (2 symmetry vectors)

| $\mathbf{n}^T$                                                               |
|------------------------------------------------------------------------------|
| $[(\blacksquare)^{2T}, R_1, S_1, T_1, U_3 + U_4, X_3 + X_4, Y_1, Z_3 + Z_4]$ |
| $[(\blacksquare)^{2T}, R_1, S_1, T_1, U_1 + U_2, X_1 + X_2, Y_1, Z_3 + Z_4]$ |

2nd minimal solution:  $\mu_2^T = 4$  (6 symmetry vectors)

Space group 31 ( $\mathbb{Z}_4$ )

1st minimal solution:  $\mu_1^T = 4$  (1 symmetry vector)

| $\mathbf{n}^T$                                                                                                                             |
|--------------------------------------------------------------------------------------------------------------------------------------------|
| $[(\blacksquare)^{2T} + \Gamma_1 + \Gamma_2, 2R_1, 2S_1, T_1 + T_2 + T_3 + T_4, 2U_1, 2X_1, Y_1 + Y_2 + Y_3 + Y_4, Z_1 + Z_2 + Z_3 + Z_4]$ |

2nd minimal solution:  $\mu_2^T = 6$  (2 symmetry vectors)

Space group 32 ( $\mathbb{Z}_1$ )

1st minimal solution:  $\mu_1^T = 2$  (2 symmetry vectors)

| $\mathbf{n}^T$                                                               |
|------------------------------------------------------------------------------|
| $[(\blacksquare)^{2T}, R_3 + R_4, S_3 + S_4, T_1, U_1, X_1, Y_1, Z_3 + Z_4]$ |
| $[(\blacksquare)^{2T}, R_1 + R_2, S_1 + S_2, T_1, U_1, X_1, Y_1, Z_3 + Z_4]$ |

2nd minimal solution:  $\mu_2^T = 4$  (6 symmetry vectors)

Space group 33 ( $\mathbb{Z}_1$ )

1st minimal solution:  $\mu_1^T = 4$  (1 symmetry vector)

| $\mathbf{n}^T$                                                                                                                             |
|--------------------------------------------------------------------------------------------------------------------------------------------|
| $[(\blacksquare)^{2T} + \Gamma_1 + \Gamma_2, R_1 + R_2 + R_3 + R_4, S_1 + S_2 + S_3 + S_4, 2T_1, 2U_1, 2X_1, 2Y_1, Z_1 + Z_2 + Z_3 + Z_4]$ |

2nd minimal solution:  $\mu_2^T = 8$  (1 symmetry vector)

Space group 34 ( $\mathbb{Z}_1$ )

1st minimal solution:  $\mu_1^T = 2$  (2 symmetry vectors)

| $\mathbf{n}^T$                                                               |
|------------------------------------------------------------------------------|
| $[(\blacksquare)^{2T}, R_3 + R_4, S_3 + S_4, T_1, U_1, X_1, Y_1, Z_3 + Z_4]$ |
| $[(\blacksquare)^{2T}, R_1 + R_2, S_1 + S_2, T_1, U_1, X_1, Y_1, Z_3 + Z_4]$ |

2nd minimal solution:  $\mu_2^T = 4$  (6 symmetry vectors)

Space group 35 ( $\mathbb{Z}_1$ )

1st minimal solution:  $\mu_1^T = 2$  (6 symmetry vectors)

| $\mathbf{n}^T$                                                                 |
|--------------------------------------------------------------------------------|
| $[(\blacksquare)^{2T}, T_3 + T_4, Y_3 + Y_4, Z_3 + Z_4, 2R_2, 2S_2]$           |
| $[(\blacksquare)^{2T}, T_3 + T_4, Y_3 + Y_4, Z_3 + Z_4, R_1 + R_2, S_1 + S_2]$ |
| $[(\blacksquare)^{2T}, T_3 + T_4, Y_3 + Y_4, Z_3 + Z_4, 2R_1, 2S_1]$           |
| $[(\blacksquare)^{2T}, T_1 + T_2, Y_1 + Y_2, Z_3 + Z_4, 2R_2, 2S_2]$           |
| $[(\blacksquare)^{2T}, T_1 + T_2, Y_1 + Y_2, Z_3 + Z_4, R_1 + R_2, S_1 + S_2]$ |
| $[(\blacksquare)^{2T}, T_1 + T_2, Y_1 + Y_2, Z_3 + Z_4, 2R_1, 2S_1]$           |

2nd minimal solution:  $\mu_2^T = 3$  (32 symmetry vectors)

Space group 36 ( $\mathbb{Z}_1$ )

1st minimal solution:  $\mu_1^T = 4$  (1 symmetry vector)

| $\mathbf{n}^T$                                                                                                                         |
|----------------------------------------------------------------------------------------------------------------------------------------|
| $[(\bullet)^{2T}, \Gamma_1 + \Gamma_2, T_1 + T_2 + T_3 + T_4, Y_1 + Y_2 + Y_3 + Y_4, Z_1 + Z_2 + Z_3 + Z_4, 2R_1 + 2R_2, 2S_1 + 2S_2]$ |

2nd minimal solution:  $\mu_2^T = 6$  (2 symmetry vectors)

Space group 37 ( $\mathbb{Z}_2$ )

1st minimal solution:  $\mu_1^T = 2$  (6 symmetry vectors)

| $\mathbf{n}^T$                                                            | $\mathbf{v}^T \in \mathbb{Z}_2$ |
|---------------------------------------------------------------------------|---------------------------------|
| $[(\bullet)^{2T}, T_1 + T_2, Y_1 + Y_2, Z_3 + Z_4, 2R_2, 2S_2]$           | 1                               |
| $[(\bullet)^{2T}, T_3 + T_4, Y_3 + Y_4, Z_3 + Z_4, 2R_2, 2S_2]$           | trivial                         |
| $[(\bullet)^{2T}, T_1 + T_2, Y_1 + Y_2, Z_3 + Z_4, R_1 + R_2, S_1 + S_2]$ | trivial                         |
| $[(\bullet)^{2T}, T_3 + T_4, Y_3 + Y_4, Z_3 + Z_4, R_1 + R_2, S_1 + S_2]$ | 1                               |
| $[(\bullet)^{2T}, T_1 + T_2, Y_1 + Y_2, Z_3 + Z_4, 2R_1, 2S_1]$           | 1                               |
| $[(\bullet)^{2T}, T_3 + T_4, Y_3 + Y_4, Z_3 + Z_4, 2R_1, 2S_1]$           | trivial                         |

2nd minimal solution:  $\mu_2^T = 4$  (30 symmetry vectors)

Space group 38 ( $\mathbb{Z}_1$ )

1st minimal solution:  $\mu_1^T = 2$  (4 symmetry vectors)

| $\mathbf{n}^T$                                                            |
|---------------------------------------------------------------------------|
| $[(\bullet)^{2T}, T_3 + T_4, Y_3 + Y_4, Z_3 + Z_4, R_1 + R_2, S_1 + S_2]$ |
| $[(\bullet)^{2T}, T_1 + T_4, Y_3 + Y_4, Z_1 + Z_4, 2R_1, S_1 + S_2]$      |
| $[(\bullet)^{2T}, T_2 + T_3, Y_3 + Y_4, Z_2 + Z_3, 2R_2, S_1 + S_2]$      |
| $[(\bullet)^{2T}, T_1 + T_2, Y_3 + Y_4, Z_1 + Z_2, R_1 + R_2, S_1 + S_2]$ |

2nd minimal solution:  $\mu_2^T = 3$  (24 symmetry vectors)

Space group 39 ( $\mathbb{Z}_1$ )

1st minimal solution:  $\mu_1^T = 2$  (2 symmetry vectors)

| $\mathbf{n}^T$                                                            |
|---------------------------------------------------------------------------|
| $[(\bullet)^{2T}, T_1 + T_2, Y_3 + Y_4, Z_1 + Z_2, R_1 + R_2, S_1 + S_2]$ |
| $[(\bullet)^{2T}, T_3 + T_4, Y_3 + Y_4, Z_3 + Z_4, R_1 + R_2, S_1 + S_2]$ |

2nd minimal solution:  $\mu_2^T = 4$  (10 symmetry vectors)

Space group 40 ( $\mathbb{Z}_1$ )

1st minimal solution:  $\mu_1^T = 2$  (1 symmetry vector)

$$\frac{\mathbf{n}^T}{[(\blacksquare)^{2T}, T_1, Y_3 + Y_4, Z_1, R_1 + R_2, S_1 + S_2]}$$

2nd minimal solution:  $\mu_2^T = 4$  (4 symmetry vectors)

Space group 41 ( $\mathbb{Z}_1$ )

1st minimal solution:  $\mu_1^T = 2$  (1 symmetry vector)

$$\frac{\mathbf{n}^T}{[(\blacksquare)^{2T}, T_1, Y_3 + Y_4, Z_1, R_1 + R_2, S_1 + S_2]}$$

2nd minimal solution:  $\mu_2^T = 4$  (2 symmetry vectors)

Space group 42 ( $\mathbb{Z}_1$ )

1st minimal solution:  $\mu_1^T = 2$  (2 symmetry vectors)

$$\frac{\mathbf{n}^T}{\begin{array}{l} [(\blacksquare)^{2T}, T_3 + T_4, Y_3 + Y_4, Z_3 + Z_4, 2L_1] \\ [(\blacksquare)^{2T}, T_1 + T_2, Y_1 + Y_2, Z_3 + Z_4, 2L_1] \end{array}}$$

2nd minimal solution:  $\mu_2^T = 3$  (8 symmetry vectors)

Space group 43 ( $\mathbb{Z}_1$ )

1st minimal solution:  $\mu_1^T = 2$  (1 symmetry vector)

$$\frac{\mathbf{n}^T}{[(\blacksquare)^{2T}, T_1, Y_1, Z_3 + Z_4, 2L_1]}$$

2nd minimal solution:  $\mu_2^T = 4$  (2 symmetry vectors)

Space group 44 ( $\mathbb{Z}_1$ )

1st minimal solution:  $\mu_1^T = 2$  (3 symmetry vectors)

| $\mathbf{n}^T$                                                            |
|---------------------------------------------------------------------------|
| $[(\bullet)^{2T}, X_3 + X_4, R_1 + R_2, S_1 + S_2, 2T_2, 2W_2]$           |
| $[(\bullet)^{2T}, X_3 + X_4, R_1 + R_2, S_1 + S_2, T_1 + T_2, W_1 + W_2]$ |
| $[(\bullet)^{2T}, X_3 + X_4, R_1 + R_2, S_1 + S_2, 2T_1, 2W_1]$           |

2nd minimal solution:  $\mu_2^T = 3$  (16 symmetry vectors)

Space group 45 ( $\mathbb{Z}_2$ )

1st minimal solution:  $\mu_1^T = 2$  (3 symmetry vectors)

| $\mathbf{n}^T$                                                            | $\mathbf{v}^T \in \mathbb{Z}_2$ |
|---------------------------------------------------------------------------|---------------------------------|
| $[(\bullet)^{2T}, X_3 + X_4, R_1 + R_2, S_1 + S_2, 2T_2, 2W_2]$           | trivial                         |
| $[(\bullet)^{2T}, X_3 + X_4, R_1 + R_2, S_1 + S_2, T_1 + T_2, W_1 + W_2]$ | 1                               |
| $[(\bullet)^{2T}, X_3 + X_4, R_1 + R_2, S_1 + S_2, 2T_1, 2W_1]$           | trivial                         |

2nd minimal solution:  $\mu_2^T = 4$  (10 symmetry vectors)

Space group 46 ( $\mathbb{Z}_1$ )

1st minimal solution:  $\mu_1^T = 2$  (1 symmetry vector)

| $\mathbf{n}^T$                                                            |
|---------------------------------------------------------------------------|
| $[(\bullet)^{2T}, X_3 + X_4, R_1 + R_2, S_1 + S_2, T_1 + T_2, W_1 + W_2]$ |

2nd minimal solution:  $\mu_2^T = 4$  (4 symmetry vectors)

Space group 47 ( $\mathbb{Z}_1$ )

1st minimal solution:  $\mu_1^T = 2$  (56 symmetry vectors)

| $\mathbf{n}^T$                                                                                                              |
|-----------------------------------------------------------------------------------------------------------------------------|
| $[(\bullet)^{2T}, R_3^+ + R_4^-, S_3^+ + S_4^-, T_1^- + T_4^-, U_2^- + U_4^-, X_2^- + X_4^-, Y_2^+ + Y_3^+, Z_4^+ + Z_4^-]$ |
| $[(\bullet)^{2T}, R_1^- + R_4^-, S_1^- + S_4^-, T_1^- + T_4^-, U_4^+ + U_4^-, X_4^+ + X_4^-, Y_2^+ + Y_3^+, Z_4^+ + Z_4^-]$ |
| $[(\bullet)^{2T}, 2R_3^+, S_3^+ + S_4^-, T_1^- + T_3^+, U_2^- + U_3^+, X_2^- + X_4^-, Y_2^+ + Y_3^+, Z_3^+ + Z_4^+]$        |
| $[(\bullet)^{2T}, R_3^+ + R_4^-, S_4^+ + S_4^-, T_1^- + T_2^-, U_3^+ + U_4^+, X_4^+ + X_4^-, Y_2^+ + Y_2^-, Z_3^+ + Z_4^+]$ |
| $[(\bullet)^{2T}, R_2^- + R_3^+, S_2^- + S_4^-, T_1^- + T_2^-, U_2^- + U_3^+, X_2^- + X_4^-, Y_2^+ + Y_2^-, Z_3^+ + Z_4^+]$ |
| $[(\bullet)^{2T}, R_1^- + R_3^+, S_1^- + S_4^-, T_1^- + T_3^+, U_3^+ + U_4^+, X_4^+ + X_4^-, Y_2^+ + Y_3^+, Z_3^+ + Z_4^+]$ |
| $[(\bullet)^{2T}, R_2^+ + R_3^+, S_2^+ + S_3^+, T_1^- + T_4^-, U_2^- + U_2^-, X_2^- + X_2^-, Y_2^+ + Y_3^+, Z_4^+ + Z_4^-]$ |
| $[(\bullet)^{2T}, R_1^- + R_2^-, S_1^- + S_2^+, T_1^- + T_4^-, U_2^- + U_4^+, X_2^- + X_4^+, Y_2^+ + Y_3^+, Z_4^+ + Z_4^-]$ |

... continued on next page

... continued from previous page

$$\begin{aligned}
& [(\bullet)^{2T}, R_1^- + R_3^+, S_2^+ + S_3^+, T_1^- + T_3^+, U_1^- + U_2^-, X_2^+ + X_2^-, Y_2^+ + Y_3^+, Z_3^+ + Z_4^-] \\
& [(\bullet)^{2T}, R_1^- + R_4^+, S_2^+ + S_4^+, T_1^- + T_2^-, U_1^- + U_4^-, X_2^+ + X_4^+, Y_2^+ + Y_2^-, Z_3^+ + Z_4^-] \\
& [(\bullet)^{2T}, R_1^- + R_2^-, S_2^+ + S_2^-, T_1^- + T_2^-, U_1^- + U_2^-, X_2^+ + X_2^-, Y_2^+ + Y_2^-, Z_3^+ + Z_4^-] \\
& [(\bullet)^{2T}, 2R_1^-, S_1^- + S_2^+, T_1^- + T_3^+, U_1^- + U_4^-, X_2^+ + X_4^+, Y_2^+ + Y_3^+, Z_3^+ + Z_4^-] \\
& [(\bullet)^{2T}, R_1^- + R_3^-, S_2^+ + S_4^+, T_1^+ + T_1^-, U_2^+ + U_4^-, X_2^+ + X_4^+, Y_2^+ + Y_2^-, Z_4^+ + Z_4^-] \\
& [(\bullet)^{2T}, R_1^+ + R_3^-, S_2^- + S_4^-, T_1^+ + T_1^-, U_2^- + U_4^-, X_2^- + X_4^-, Y_2^+ + Y_2^-, Z_4^+ + Z_4^-] \\
& [(\bullet)^{2T}, 2R_4^-, S_3^+ + S_4^-, T_2^+ + T_4^-, U_1^+ + U_4^-, X_2^- + X_4^-, Y_2^+ + Y_3^+, Z_3^- + Z_4^-] \\
& [(\bullet)^{2T}, R_3^+ + R_4^-, S_3^+ + S_4^-, T_2^+ + T_3^+, U_1^+ + U_3^+, X_2^- + X_4^-, Y_2^+ + Y_3^+, Z_3^+ + Z_3^-] \\
& [(\bullet)^{2T}, R_2^- + R_4^-, S_2^- + S_4^-, T_2^+ + T_2^-, U_1^+ + U_3^+, X_2^- + X_4^-, Y_2^+ + Y_2^-, Z_3^+ + Z_3^-] \\
& [(\bullet)^{2T}, R_2^+ + R_4^-, S_2^+ + S_3^+, T_2^+ + T_4^-, U_1^+ + U_2^+, X_2^+ + X_2^-, Y_2^+ + Y_3^+, Z_3^- + Z_4^-] \\
& [(\bullet)^{2T}, R_1^- + R_4^-, S_2^+ + S_3^+, T_2^+ + T_3^+, U_1^+ + U_1^-, X_2^+ + X_2^-, Y_2^+ + Y_3^+, Z_3^+ + Z_3^-] \\
& [(\bullet)^{2T}, R_1^+ + R_4^-, S_2^- + S_4^-, T_1^+ + T_2^+, U_1^+ + U_4^-, X_2^- + X_4^-, Y_2^+ + Y_2^-, Z_3^- + Z_4^-] \\
& [(\bullet)^{2T}, R_2^- + R_4^-, S_1^+ + S_3^+, T_4^+ + T_4^-, U_2^- + U_4^-, X_2^- + X_4^-, Y_3^+ + Y_3^-, Z_4^+ + Z_4^-] \\
& [(\bullet)^{2T}, R_2^- + R_3^+, S_1^+ + S_3^+, T_3^+ + T_4^+, U_2^- + U_3^+, X_2^- + X_4^-, Y_3^+ + Y_3^-, Z_3^+ + Z_4^-] \\
& [(\bullet)^{2T}, R_2^- + R_4^+, S_1^+ + S_4^+, T_2^- + T_4^+, U_3^+ + U_4^+, X_4^+ + X_4^-, Y_2^- + Y_3^-, Z_3^+ + Z_4^-] \\
& [(\bullet)^{2T}, 2R_2^-, S_1^+ + S_2^-, T_2^- + T_4^+, U_2^- + U_3^+, X_2^- + X_4^-, Y_2^- + Y_3^-, Z_3^+ + Z_4^-] \\
& [(\bullet)^{2T}, R_1^- + R_2^-, S_1^+ + S_1^-, T_3^+ + T_4^+, U_3^+ + U_4^+, X_4^+ + X_4^-, Y_3^+ + Y_3^-, Z_3^+ + Z_4^-] \\
& [(\bullet)^{2T}, R_1^+ + R_2^-, S_1^+ + S_2^-, T_1^+ + T_4^+, U_2^- + U_4^-, X_2^- + X_4^-, Y_2^- + Y_3^-, Z_4^+ + Z_4^-] \\
& [(\bullet)^{2T}, R_1^+ + R_4^-, S_1^+ + S_3^+, T_3^- + T_4^-, U_1^+ + U_4^-, X_2^- + X_4^-, Y_3^+ + Y_3^-, Z_3^- + Z_4^-] \\
& [(\bullet)^{2T}, R_1^+ + R_3^+, S_1^+ + S_3^+, T_3^+ + T_3^-, U_1^+ + U_3^+, X_2^- + X_4^-, Y_3^+ + Y_3^-, Z_3^+ + Z_3^-] \\
& [(\bullet)^{2T}, R_1^+ + R_2^-, S_1^+ + S_2^-, T_2^- + T_3^-, U_1^+ + U_3^+, X_2^- + X_4^-, Y_2^- + Y_3^-, Z_3^+ + Z_3^-] \\
& [(\bullet)^{2T}, 2R_1^+, S_1^+ + S_2^-, T_1^+ + T_3^-, U_1^+ + U_4^-, X_2^- + X_4^-, Y_2^- + Y_3^-, Z_3^- + Z_4^-] \\
& [(\bullet)^{2T}, R_2^+ + R_4^-, S_1^+ + S_4^-, T_2^+ + T_4^-, U_3^- + U_4^-, X_4^+ + X_4^-, Y_2^+ + Y_3^+, Z_3^- + Z_4^-] \\
& [(\bullet)^{2T}, R_2^- + R_3^-, S_1^+ + S_4^-, T_2^- + T_3^-, U_3^+ + U_3^-, X_4^+ + X_4^-, Y_2^- + Y_3^-, Z_3^+ + Z_3^-] \\
& [(\bullet)^{2T}, R_2^+ + R_3^+, S_1^- + S_4^-, T_2^+ + T_3^+, U_3^+ + U_3^-, X_4^+ + X_4^-, Y_2^+ + Y_3^+, Z_3^+ + Z_3^-] \\
& [(\bullet)^{2T}, 2R_2^+, S_1^- + S_2^+, T_2^+ + T_4^-, U_2^+ + U_3^-, X_2^+ + X_4^+, Y_2^+ + Y_3^+, Z_3^- + Z_4^-] \\
& [(\bullet)^{2T}, R_1^- + R_2^+, S_1^- + S_2^+, T_2^+ + T_3^+, U_1^- + U_3^-, X_2^+ + X_4^+, Y_2^+ + Y_3^+, Z_3^+ + Z_3^-] \\
& [(\bullet)^{2T}, R_3^+ + R_4^+, S_3^+ + S_3^-, T_3^+ + T_4^+, U_1^- + U_2^-, X_2^+ + X_2^-, Y_3^+ + Y_3^-, Z_3^+ + Z_4^-] \\
& [(\bullet)^{2T}, 2R_4^+, S_3^- + S_4^+, T_2^- + T_4^+, U_1^- + U_4^+, X_2^+ + X_4^+, Y_2^- + Y_3^-, Z_3^+ + Z_4^-] \\
& [(\bullet)^{2T}, R_2^- + R_4^+, S_2^- + S_3^-, T_2^- + T_4^+, U_1^- + U_2^-, X_2^+ + X_2^-, Y_2^- + Y_3^-, Z_3^+ + Z_4^-] \\
& [(\bullet)^{2T}, R_1^- + R_4^+, S_1^- + S_3^-, T_3^+ + T_4^+, U_1^- + U_4^+, X_2^+ + X_4^+, Y_3^+ + Y_3^-, Z_3^+ + Z_4^-] \\
& [(\bullet)^{2T}, R_3^- + R_4^-, S_3^+ + S_3^-, T_3^- + T_4^-, U_1^+ + U_2^+, X_2^+ + X_2^-, Y_3^+ + Y_3^-, Z_3^- + Z_4^-] \\
& [(\bullet)^{2T}, R_3^- + R_4^+, S_3^- + S_4^+, T_1^+ + T_4^+, U_2^+ + U_4^+, X_2^+ + X_4^+, Y_2^- + Y_3^-, Z_4^+ + Z_4^-] \\
& [(\bullet)^{2T}, 2R_3^-, S_3^- + S_4^+, T_1^+ + T_3^-, U_2^+ + U_3^-, X_2^+ + X_4^+, Y_2^- + Y_3^-, Z_3^- + Z_4^-] \\
& [(\bullet)^{2T}, R_3^- + R_4^-, S_4^+ + S_4^-, T_1^+ + T_2^+, U_3^- + U_4^-, X_4^+ + X_4^-, Y_2^+ + Y_2^-, Z_3^- + Z_4^-] \\
& [(\bullet)^{2T}, R_3^- + R_4^+, S_3^- + S_4^+, T_2^- + T_3^-, U_1^- + U_3^-, X_2^+ + X_4^+, Y_2^- + Y_3^-, Z_3^+ + Z_3^-] \\
& [(\bullet)^{2T}, R_2^- + R_3^-, S_2^- + S_3^-, T_1^+ + T_4^+, U_2^+ + U_2^-, X_2^+ + X_2^-, Y_2^- + Y_3^-, Z_4^+ + Z_4^-] \\
& [(\bullet)^{2T}, R_2^+ + R_3^-, S_2^+ + S_4^+, T_1^+ + T_2^+, U_2^+ + U_3^-, X_2^+ + X_4^+, Y_2^+ + Y_2^-, Z_3^- + Z_4^-] \\
& [(\bullet)^{2T}, R_2^+ + R_4^+, S_2^+ + S_4^+, T_2^+ + T_2^-, U_1^- + U_3^-, X_2^+ + X_4^+, Y_2^+ + Y_2^-, Z_3^+ + Z_3^-] \\
& [(\bullet)^{2T}, R_2^+ + R_4^-, S_1^- + S_3^-, T_4^+ + T_4^-, U_2^+ + U_4^+, X_2^+ + X_4^+, Y_3^+ + Y_3^-, Z_4^+ + Z_4^-] \\
& [(\bullet)^{2T}, R_2^+ + R_3^-, S_1^- + S_3^-, T_3^- + T_4^-, U_2^+ + U_3^-, X_2^+ + X_4^+, Y_3^+ + Y_3^-, Z_3^- + Z_4^-] \\
& [(\bullet)^{2T}, R_1^- + R_3^-, S_1^- + S_3^-, T_3^+ + T_3^-, U_1^- + U_3^-, X_2^+ + X_4^+, Y_3^+ + Y_3^-, Z_3^+ + Z_3^-] \\
& [(\bullet)^{2T}, R_1^+ + R_3^-, S_2^- + S_3^-, T_1^+ + T_3^-, U_1^+ + U_2^+, X_2^+ + X_2^-, Y_2^- + Y_3^-, Z_3^- + Z_4^-] \\
& [(\bullet)^{2T}, R_1^+ + R_4^+, S_2^- + S_3^-, T_2^- + T_3^-, U_1^+ + U_1^-, X_2^+ + X_2^-, Y_2^- + Y_3^-, Z_3^+ + Z_4^-] \\
& [(\bullet)^{2T}, R_1^+ + R_4^-, S_1^+ + S_4^+, T_1^+ + T_4^+, U_4^+ + U_4^-, X_4^+ + X_4^-, Y_2^- + Y_3^-, Z_4^+ + Z_4^-] \\
& [(\bullet)^{2T}, R_1^+ + R_3^-, S_1^+ + S_4^+, T_1^+ + T_3^-, U_3^- + U_4^-, X_4^+ + X_4^-, Y_2^- + Y_3^-, Z_3^- + Z_4^-] \\
& [(\bullet)^{2T}, R_1^+ + R_2^+, S_2^+ + S_2^-, T_1^+ + T_2^+, U_1^+ + U_2^+, X_2^+ + X_2^-, Y_2^+ + Y_2^-, Z_3^- + Z_4^-] \\
& [(\bullet)^{2T}, R_1^+ + R_2^-, S_1^+ + S_1^-, T_3^- + T_4^-, U_3^- + U_4^-, X_4^+ + X_4^-, Y_3^+ + Y_3^-, Z_3^- + Z_4^-]
\end{aligned}$$

Skipped higher-order solutions...

Space group 48 ( $\mathbb{Z}_2$ )

1st minimal solution:  $\mu_1^T = 2$  (4 symmetry vectors & filling-enforced topology)

| $\mathbf{n}^T$                                                       | $\mathbf{v}^T \in \mathbb{Z}_2$ |
|----------------------------------------------------------------------|---------------------------------|
| $[(\blacksquare)^{2T}, R_4^+ + R_4^-, S_2, T_2, U_1, X_2, Y_2, Z_2]$ | 1                               |
| $[(\blacksquare)^{2T}, R_3^+ + R_3^-, S_2, T_1, U_2, X_2, Y_2, Z_2]$ | 1                               |
| $[(\blacksquare)^{2T}, R_2^+ + R_2^-, S_1, T_2, U_2, X_2, Y_2, Z_2]$ | 1                               |
| $[(\blacksquare)^{2T}, R_1^+ + R_1^-, S_1, T_1, U_1, X_2, Y_2, Z_2]$ | 1                               |

2nd minimal solution:  $\mu_2^T = 4$  (48 symmetry vectors)

Space group 49 ( $\mathbb{Z}_2$ )

1st minimal solution:  $\mu_1^T = 2$  (4 symmetry vectors & filling-enforced topology)

| $\mathbf{n}^T$                                                                           | $\mathbf{v}^T \in \mathbb{Z}_2$ |
|------------------------------------------------------------------------------------------|---------------------------------|
| $[(\blacksquare)^{2T}, R_2, S_3^+ + S_3^-, T_2, U_1, X_2^+ + X_2^-, Y_3^+ + Y_3^-, Z_2]$ | 1                               |
| $[(\blacksquare)^{2T}, R_2, S_4^+ + S_4^-, T_1, U_2, X_4^+ + X_4^-, Y_2^+ + Y_2^-, Z_2]$ | 1                               |
| $[(\blacksquare)^{2T}, R_1, S_2^+ + S_2^-, T_1, U_1, X_2^+ + X_2^-, Y_2^+ + Y_2^-, Z_2]$ | 1                               |
| $[(\blacksquare)^{2T}, R_1, S_1^+ + S_1^-, T_2, U_2, X_4^+ + X_4^-, Y_3^+ + Y_3^-, Z_2]$ | 1                               |

2nd minimal solution:  $\mu_2^T = 4$  (284 symmetry vectors)

Space group 50 ( $\mathbb{Z}_2$ )

1st minimal solution:  $\mu_1^T = 2$  (4 symmetry vectors & filling-enforced topology)

| $\mathbf{n}^T$                                                       | $\mathbf{v}^T \in \mathbb{Z}_2$ |
|----------------------------------------------------------------------|---------------------------------|
| $[(\blacksquare)^{2T}, R_2, S_2, T_2, U_1, X_2, Y_2, Z_3^+ + Z_3^-]$ | 1                               |
| $[(\blacksquare)^{2T}, R_2, S_2, T_1, U_2, X_2, Y_2, Z_4^+ + Z_4^-]$ | 1                               |
| $[(\blacksquare)^{2T}, R_1, S_1, T_2, U_1, X_2, Y_2, Z_3^+ + Z_3^-]$ | 1                               |
| $[(\blacksquare)^{2T}, R_1, S_1, T_1, U_2, X_2, Y_2, Z_4^+ + Z_4^-]$ | 1                               |

2nd minimal solution:  $\mu_2^T = 4$  (54 symmetry vectors)

Space group 51 ( $\mathbb{Z}_1$ )

1st minimal solution:  $\mu_1^T = 4$  (44 symmetry vectors)

| $\mathbf{n}^T$                                                                                                                                                                             |
|--------------------------------------------------------------------------------------------------------------------------------------------------------------------------------------------|
| $[(\blacksquare)^{2T} + \Gamma_3^+ + \Gamma_3^-, R_1 + R_2, S_1 + S_2, T_1^+ + T_2^+ + T_3^+ + T_4^+, U_1 + U_2, X_1 + X_2, Y_2^+ + Y_2^- + Y_3^+ + Y_3^-, Z_3^+ + Z_3^- + Z_4^+ + Z_4^-]$ |
| $[(\blacksquare)^{2T} + \Gamma_3^+ + \Gamma_3^-, 2R_2, 2S_2, T_1^- + T_2^+ + T_3^+ + T_4^-, U_1 + U_2, X_1 + X_2, 2Y_2^+ + 2Y_3^+, Z_3^+ + Z_3^- + Z_4^+ + Z_4^-]$                         |
| $[(\blacksquare)^{2T} + \Gamma_1^+ + \Gamma_3^+, 2R_2, 2S_2, T_2^+ + 2T_3^+ + T_4^-, U_1 + U_2, X_1 + X_2, Y_2^+ + 2Y_3^+ + Y_4^-, Z_2^- + Z_3^+ + Z_3^- + Z_4^-]$                         |

... continued on next page



2nd minimal solution:  $\mu_2^T = 6$  (748 symmetry vectors)

Space group 52 ( $\mathbb{Z}_2$ )

1st minimal solution:  $\mu_1^T = 4$  (6 symmetry vectors)

| $\mathbf{n}^\top$                                                                                                           | $\mathbf{v}^\top \in \mathbb{Z}_2$ |
|-----------------------------------------------------------------------------------------------------------------------------|------------------------------------|
| $[(\blacksquare)^{2\top} + \Gamma_4^+ + \Gamma_4^-, R_1 + R_2, S_1 + S_2, 2T_1^-, U_1 + U_2, 2X_2, Y_1 + Y_2, 2Z_2]$        | trivial                            |
| $[(\blacksquare)^{2\top} + \Gamma_4^+ + \Gamma_4^-, R_1 + R_2, S_1 + S_2, T_1^+ + T_1^-, U_1 + U_2, 2X_2, Y_1 + Y_2, 2Z_2]$ | 1                                  |

... continued on next page



... continued from previous page

|                                                                                                                                                     |         |
|-----------------------------------------------------------------------------------------------------------------------------------------------------|---------|
| $[(\blacksquare)^{2T} + \Gamma_1^+ + \Gamma_1^-, 2R_1^+, S_1 + S_2, T_1 + T_2, 2U_1^+, X_1 + X_2, Y_1^- + Y_2^- + Y_3^- + Y_4^-, Z_1 + Z_2]$        | trivial |
| $[(\blacksquare)^{2T} + \Gamma_1^+ + \Gamma_1^-, 2R_1^+, S_1 + S_2, T_1 + T_2, U_1^+ + U_1^-, X_1 + X_2, Y_1^- + Y_2^- + Y_3^- + Y_4^-, Z_1 + Z_2]$ | 1       |
| $[(\blacksquare)^{2T} + \Gamma_1^+ + \Gamma_1^-, 2R_1^+, 2S_1, T_1 + T_2, 2U_1^+, X_1 + X_2, Y_1^+ + Y_1^- + Y_3^+ + Y_3^-, Z_1 + Z_2]$             | 1       |
| $[(\blacksquare)^{2T} + \Gamma_1^+ + \Gamma_1^-, 2R_1^+, 2S_1, T_1 + T_2, U_1^+ + U_1^-, X_1 + X_2, Y_1^+ + Y_1^- + Y_3^+ + Y_3^-, Z_1 + Z_2]$      | trivial |
| $[(\blacksquare)^{2T} + \Gamma_1^+ + \Gamma_1^-, 2R_1^+, S_1 + S_2, T_1 + T_2, 2U_1^-, X_1 + X_2, Y_1^- + Y_2^- + Y_3^- + Y_4^-, Z_1 + Z_2]$        | trivial |
| $[(\blacksquare)^{2T} + \Gamma_1^+ + \Gamma_1^-, 2R_1^+, 2S_1, T_1 + T_2, 2U_1^-, X_1 + X_2, Y_1^+ + Y_1^- + Y_3^+ + Y_3^-, Z_1 + Z_2]$             | 1       |

2nd minimal solution:  $\mu_2^T = 6$  (512 symmetry vectors)

Space group 54 ( $\mathbb{Z}_2$ )

1st minimal solution:  $\mu_1^T = 4$  (5 symmetry vectors)

| $\mathbf{n}^T$                                                                                                                                     | $\mathbf{v}^T \in \mathbb{Z}_2$ |
|----------------------------------------------------------------------------------------------------------------------------------------------------|---------------------------------|
| $[(\blacksquare)^{2T} + \Gamma_3^+ + \Gamma_3^-, R_1 + R_2, S_1 + S_2, T_1 + T_2, U_1 + U_2, X_1 + X_2, Y_2^+ + Y_2^- + Y_3^+ + Y_3^-, 2Z_2]$      | 1                               |
| $[(\blacksquare)^{2T} + \Gamma_1^+ + \Gamma_1^-, R_1 + R_2, S_1 + S_2, T_1 + T_2, U_1 + U_2, X_1 + X_2, Y_1^- + Y_2^- + Y_3^- + Y_4^-, Z_1 + Z_2]$ | trivial                         |
| $[(\blacksquare)^{2T} + \Gamma_1^+ + \Gamma_1^-, R_1 + R_2, S_1 + S_2, 2T_2, U_1 + U_2, X_1 + X_2, Y_3^+ + Y_3^- + Y_4^+ + Y_4^-, Z_1 + Z_2]$      | 1                               |
| $[(\blacksquare)^{2T} + \Gamma_1^+ + \Gamma_1^-, R_1 + R_2, S_1 + S_2, 2T_1, U_1 + U_2, X_1 + X_2, Y_1^+ + Y_1^- + Y_2^+ + Y_2^-, Z_1 + Z_2]$      | 1                               |
| $[(\blacksquare)^{2T} + \Gamma_1^+ + \Gamma_1^-, R_1 + R_2, S_1 + S_2, T_1 + T_2, U_1 + U_2, X_1 + X_2, Y_1^+ + Y_2^+ + Y_3^+ + Y_4^+, Z_1 + Z_2]$ | trivial                         |

2nd minimal solution:  $\mu_2^T = 8$  (57 symmetry vectors)

Space group 55 ( $\mathbb{Z}_1$ )

1st minimal solution:  $\mu_1^T = 4$  (20 symmetry vectors)

| $\mathbf{n}^T$                                                                                                                                                                             |
|--------------------------------------------------------------------------------------------------------------------------------------------------------------------------------------------|
| $[(\blacksquare)^{2T} + \Gamma_1^+ + \Gamma_1^-, R_3^+ + R_3^- + R_4^+ + R_4^-, S_3^+ + S_3^- + S_4^+ + S_4^-, T_1 + T_2, U_1 + U_2, X_1 + X_2, Y_1 + Y_2, Z_1^- + Z_2^- + Z_3^- + Z_4^-]$ |
| $[(\blacksquare)^{2T} + \Gamma_1^+ + \Gamma_1^-, R_1^- + R_2^- + R_3^- + R_4^-, S_1^+ + S_2^+ + S_3^+ + S_4^+, T_1 + T_2, U_1 + U_2, X_1 + X_2, Y_1 + Y_2, Z_1^- + Z_2^- + Z_3^- + Z_4^-]$ |
| $[(\blacksquare)^{2T} + \Gamma_1^+ + \Gamma_1^-, 2R_3^- + 2R_4^-, S_3^+ + S_3^- + S_4^+ + S_4^-, 2T_2, 2U_1, X_1 + X_2, Y_1 + Y_2, Z_1^+ + Z_2^+ + Z_3^- + Z_4^-]$                         |
| $[(\blacksquare)^{2T} + \Gamma_1^+ + \Gamma_1^-, R_1^+ + R_2^+ + R_3^- + R_4^-, S_1^+ + S_2^+ + S_3^+ + S_4^+, 2T_2, 2U_1, X_1 + X_2, Y_1 + Y_2, Z_1^+ + Z_2^+ + Z_3^- + Z_4^-]$           |
| $[(\blacksquare)^{2T} + \Gamma_1^+ + \Gamma_1^-, R_1^- + R_2^- + R_3^- + R_4^-, S_1^- + S_2^- + S_3^- + S_4^-, T_1 + T_2, U_1 + U_2, X_1 + X_2, Y_1 + Y_2, Z_1^- + Z_2^- + Z_3^- + Z_4^-]$ |
| $[(\blacksquare)^{2T} + \Gamma_1^+ + \Gamma_1^-, R_1^+ + R_2^+ + R_3^- + R_4^-, S_1^- + S_2^- + S_3^- + S_4^-, 2T_2, 2U_1, X_1 + X_2, Y_1 + Y_2, Z_1^+ + Z_2^+ + Z_3^- + Z_4^-]$           |
| $[(\blacksquare)^{2T} + \Gamma_1^+ + \Gamma_1^-, R_1^+ + R_2^+ + R_3^+ + R_4^+, S_1^+ + S_2^+ + S_3^+ + S_4^+, T_1 + T_2, U_1 + U_2, X_1 + X_2, Y_1 + Y_2, Z_1^- + Z_2^- + Z_3^- + Z_4^-]$ |
| $[(\blacksquare)^{2T} + \Gamma_1^+ + \Gamma_1^-, R_1^+ + R_1^- + R_2^+ + R_2^-, S_1^+ + S_1^- + S_2^+ + S_2^-, T_1 + T_2, U_1 + U_2, X_1 + X_2, Y_1 + Y_2, Z_1^- + Z_2^- + Z_3^- + Z_4^-]$ |
| $[(\blacksquare)^{2T} + \Gamma_1^+ + \Gamma_1^-, 2R_1^+ + 2R_2^-, S_1^+ + S_1^- + S_2^+ + S_2^-, 2T_2, 2U_1, X_1 + X_2, Y_1 + Y_2, Z_1^+ + Z_2^+ + Z_3^- + Z_4^-]$                         |
| $[(\blacksquare)^{2T} + \Gamma_1^+ + \Gamma_1^-, 2R_3^+ + 2R_4^+, S_3^+ + S_3^- + S_4^+ + S_4^-, 2T_1, 2U_2, X_1 + X_2, Y_1 + Y_2, Z_1^- + Z_2^- + Z_3^+ + Z_4^+]$                         |
| $[(\blacksquare)^{2T} + \Gamma_1^+ + \Gamma_1^-, R_1^- + R_2^- + R_3^+ + R_4^+, S_1^+ + S_2^+ + S_3^+ + S_4^+, 2T_1, 2U_2, X_1 + X_2, Y_1 + Y_2, Z_1^- + Z_2^- + Z_3^+ + Z_4^+]$           |
| $[(\blacksquare)^{2T} + \Gamma_1^+ + \Gamma_1^-, R_3^+ + R_3^- + R_4^+ + R_4^-, S_3^+ + S_3^- + S_4^+ + S_4^-, T_1 + T_2, U_1 + U_2, X_1 + X_2, Y_1 + Y_2, Z_1^+ + Z_2^+ + Z_3^+ + Z_4^+]$ |
| $[(\blacksquare)^{2T} + \Gamma_1^+ + \Gamma_1^-, R_1^+ + R_2^+ + R_3^+ + R_4^+, S_1^+ + S_2^+ + S_3^+ + S_4^+, T_1 + T_2, U_1 + U_2, X_1 + X_2, Y_1 + Y_2, Z_1^+ + Z_2^+ + Z_3^+ + Z_4^+]$ |
| $[(\blacksquare)^{2T} + \Gamma_1^+ + \Gamma_1^-, R_1^- + R_2^- + R_3^+ + R_4^+, S_1^- + S_2^- + S_3^- + S_4^-, 2T_1, 2U_2, X_1 + X_2, Y_1 + Y_2, Z_1^- + Z_2^- + Z_3^+ + Z_4^+]$           |
| $[(\blacksquare)^{2T} + \Gamma_1^+ + \Gamma_1^-, 2R_1^- + 2R_2^-, S_1^+ + S_1^- + S_2^+ + S_2^-, 2T_1, 2U_2, X_1 + X_2, Y_1 + Y_2, Z_1^- + Z_2^- + Z_3^+ + Z_4^+]$                         |
| $[(\blacksquare)^{2T} + \Gamma_1^+ + \Gamma_1^-, R_1^- + R_2^- + R_3^- + R_4^-, S_1^- + S_2^- + S_3^- + S_4^-, T_1 + T_2, U_1 + U_2, X_1 + X_2, Y_1 + Y_2, Z_1^+ + Z_2^+ + Z_3^+ + Z_4^+]$ |
| $[(\blacksquare)^{2T} + \Gamma_1^+ + \Gamma_1^-, R_1^+ + R_1^- + R_2^+ + R_2^-, S_1^+ + S_1^- + S_2^+ + S_2^-, T_1 + T_2, U_1 + U_2, X_1 + X_2, Y_1 + Y_2, Z_1^+ + Z_2^+ + Z_3^+ + Z_4^+]$ |
| $[(\blacksquare)^{2T} + \Gamma_1^+ + \Gamma_1^-, R_1^- + R_2^- + R_3^- + R_4^-, S_1^+ + S_2^+ + S_3^+ + S_4^+, T_1 + T_2, U_1 + U_2, X_1 + X_2, Y_1 + Y_2, Z_1^+ + Z_2^+ + Z_3^+ + Z_4^+]$ |
| $[(\blacksquare)^{2T} + \Gamma_1^+ + \Gamma_1^-, R_1^+ + R_2^+ + R_3^+ + R_4^+, S_1^- + S_2^- + S_3^- + S_4^-, T_1 + T_2, U_1 + U_2, X_1 + X_2, Y_1 + Y_2, Z_1^+ + Z_2^+ + Z_3^+ + Z_4^+]$ |
| $[(\blacksquare)^{2T} + \Gamma_1^+ + \Gamma_1^-, R_1^+ + R_2^+ + R_3^+ + R_4^+, S_1^- + S_2^- + S_3^- + S_4^-, T_1 + T_2, U_1 + U_2, X_1 + X_2, Y_1 + Y_2, Z_1^- + Z_2^- + Z_3^- + Z_4^-]$ |

2nd minimal solution:  $\mu_2^T = 6$  (208 symmetry vectors)

Space group 56 ( $\mathbb{Z}_2$ )

1st minimal solution:  $\mu_1^T = 4$  (4 symmetry vectors)

| $\mathbf{n}^T$                                                                                                                                | $\mathbf{v}^T \in \mathbb{Z}_2$ |
|-----------------------------------------------------------------------------------------------------------------------------------------------|---------------------------------|
| $[(\bullet)^{2T} + \Gamma_1^+ + \Gamma_1^-, R_1^- + R_2^- + R_3^- + R_4^-, S_1 + S_2, T_1 + T_2, U_1 + U_2, X_1 + X_2, Y_1 + Y_2, Z_1 + Z_2]$ | trivial                         |
| $[(\bullet)^{2T} + \Gamma_1^+ + \Gamma_1^-, R_3^+ + R_3^- + R_4^+ + R_4^-, 2S_2, T_1 + T_2, U_1 + U_2, X_1 + X_2, Y_1 + Y_2, Z_1 + Z_2]$      | 1                               |
| $[(\bullet)^{2T} + \Gamma_1^+ + \Gamma_1^-, R_1^+ + R_1^- + R_2^+ + R_2^-, 2S_1, T_1 + T_2, U_1 + U_2, X_1 + X_2, Y_1 + Y_2, Z_1 + Z_2]$      | 1                               |
| $[(\bullet)^{2T} + \Gamma_1^+ + \Gamma_1^-, R_1^+ + R_2^+ + R_3^+ + R_4^+, S_1 + S_2, T_1 + T_2, U_1 + U_2, X_1 + X_2, Y_1 + Y_2, Z_1 + Z_2]$ | trivial                         |

2nd minimal solution:  $\mu_2^T = 8$  (36 symmetry vectors)

Space group 57 ( $\mathbb{Z}_1$ )

1st minimal solution:  $\mu_1^T = 4$  (2 symmetry vectors)

| $\mathbf{n}^T$                                                                                                                                |
|-----------------------------------------------------------------------------------------------------------------------------------------------|
| $[(\bullet)^{2T} + \Gamma_1^+ + \Gamma_1^-, R_1 + R_2, S_1 + S_2, T_1 + T_2, U_1 + U_2, X_1^+ + X_2^+ + X_3^+ + X_4^+, Y_1 + Y_2, Z_1 + Z_2]$ |
| $[(\bullet)^{2T} + \Gamma_1^+ + \Gamma_1^-, R_1 + R_2, S_1 + S_2, T_1 + T_2, U_1 + U_2, X_1^- + X_2^- + X_3^- + X_4^-, Y_1 + Y_2, Z_1 + Z_2]$ |

2nd minimal solution:  $\mu_2^T = 8$  (16 symmetry vectors)

Space group 58 ( $\mathbb{Z}_2$ )

1st minimal solution:  $\mu_1^T = 4$  (36 symmetry vectors)

| $\mathbf{n}^T$                                                                                                                                        | $\mathbf{v}^T \in \mathbb{Z}_2$ |
|-------------------------------------------------------------------------------------------------------------------------------------------------------|---------------------------------|
| $[(\bullet)^{2T} + \Gamma_1^+ + \Gamma_1^-, 2R_2, S_3^+ + S_3^- + S_4^+ + S_4^-, 2T_1^-, 2U_1^-, X_1 + X_2, Y_1 + Y_2, Z_1 + Z_2]$                    | 1                               |
| $[(\bullet)^{2T} + \Gamma_1^+ + \Gamma_1^-, 2R_2, S_3^+ + S_3^- + S_4^+ + S_4^-, 2T_1^-, U_1^+ + U_1^-, X_1 + X_2, Y_1 + Y_2, Z_1 + Z_2]$             | trivial                         |
| $[(\bullet)^{2T} + \Gamma_1^+ + \Gamma_1^-, R_1 + R_2, S_1^+ + S_2^+ + S_3^+ + S_4^+, 2T_1^-, 2U_1^-, X_1 + X_2, Y_1 + Y_2, Z_1 + Z_2]$               | trivial                         |
| $[(\bullet)^{2T} + \Gamma_1^+ + \Gamma_1^-, R_1 + R_2, S_1^+ + S_2^+ + S_3^+ + S_4^+, 2T_1^-, U_1^+ + U_1^-, X_1 + X_2, Y_1 + Y_2, Z_1 + Z_2]$        | 1                               |
| $[(\bullet)^{2T} + \Gamma_1^+ + \Gamma_1^-, 2R_2, S_3^+ + S_3^- + S_4^+ + S_4^-, T_1^+ + T_1^-, 2U_1^-, X_1 + X_2, Y_1 + Y_2, Z_1 + Z_2]$             | trivial                         |
| $[(\bullet)^{2T} + \Gamma_1^+ + \Gamma_1^-, 2R_2, S_3^+ + S_3^- + S_4^+ + S_4^-, T_1^+ + T_1^-, U_1^+ + U_1^-, X_1 + X_2, Y_1 + Y_2, Z_1 + Z_2]$      | 1                               |
| $[(\bullet)^{2T} + \Gamma_1^+ + \Gamma_1^-, R_1 + R_2, S_1^+ + S_2^+ + S_3^+ + S_4^+, T_1^+ + T_1^-, 2U_1^-, X_1 + X_2, Y_1 + Y_2, Z_1 + Z_2]$        | 1                               |
| $[(\bullet)^{2T} + \Gamma_1^+ + \Gamma_1^-, R_1 + R_2, S_1^+ + S_2^+ + S_3^+ + S_4^+, T_1^+ + T_1^-, U_1^+ + U_1^-, X_1 + X_2, Y_1 + Y_2, Z_1 + Z_2]$ | trivial                         |
| $[(\bullet)^{2T} + \Gamma_1^+ + \Gamma_1^-, 2R_2, S_3^+ + S_3^- + S_4^+ + S_4^-, 2T_1^-, 2U_1^+, X_1 + X_2, Y_1 + Y_2, Z_1 + Z_2]$                    | 1                               |
| $[(\bullet)^{2T} + \Gamma_1^+ + \Gamma_1^-, R_1 + R_2, S_1^+ + S_2^+ + S_3^+ + S_4^+, 2T_1^-, 2U_1^+, X_1 + X_2, Y_1 + Y_2, Z_1 + Z_2]$               | trivial                         |
| $[(\bullet)^{2T} + \Gamma_1^+ + \Gamma_1^-, 2R_2, S_3^+ + S_3^- + S_4^+ + S_4^-, T_1^+ + T_1^-, 2U_1^+, X_1 + X_2, Y_1 + Y_2, Z_1 + Z_2]$             | trivial                         |
| $[(\bullet)^{2T} + \Gamma_1^+ + \Gamma_1^-, R_1 + R_2, S_1^+ + S_2^+ + S_3^+ + S_4^+, T_1^+ + T_1^-, 2U_1^+, X_1 + X_2, Y_1 + Y_2, Z_1 + Z_2]$        | 1                               |
| $[(\bullet)^{2T} + \Gamma_1^+ + \Gamma_1^-, R_1 + R_2, S_1^- + S_2^- + S_3^- + S_4^-, 2T_1^-, 2U_1^-, X_1 + X_2, Y_1 + Y_2, Z_1 + Z_2]$               | trivial                         |
| $[(\bullet)^{2T} + \Gamma_1^+ + \Gamma_1^-, R_1 + R_2, S_1^- + S_2^- + S_3^- + S_4^-, 2T_1^-, U_1^+ + U_1^-, X_1 + X_2, Y_1 + Y_2, Z_1 + Z_2]$        | 1                               |
| $[(\bullet)^{2T} + \Gamma_1^+ + \Gamma_1^-, 2R_1, S_1^+ + S_1^- + S_2^+ + S_2^-, 2T_1^-, 2U_1^-, X_1 + X_2, Y_1 + Y_2, Z_1 + Z_2]$                    | 1                               |
| $[(\bullet)^{2T} + \Gamma_1^+ + \Gamma_1^-, 2R_1, S_1^+ + S_1^- + S_2^+ + S_2^-, 2T_1^-, U_1^+ + U_1^-, X_1 + X_2, Y_1 + Y_2, Z_1 + Z_2]$             | trivial                         |
| $[(\bullet)^{2T} + \Gamma_1^+ + \Gamma_1^-, R_1 + R_2, S_1^- + S_2^- + S_3^- + S_4^-, T_1^+ + T_1^-, 2U_1^-, X_1 + X_2, Y_1 + Y_2, Z_1 + Z_2]$        | 1                               |

... continued on next page

... continued from previous page

|                                                                                                                                                       |         |
|-------------------------------------------------------------------------------------------------------------------------------------------------------|---------|
| $[(\bullet)^{2T} + \Gamma_1^+ + \Gamma_1^-, R_1 + R_2, S_1^- + S_2^- + S_3^- + S_4^-, T_1^+ + T_1^-, U_1^+ + U_1^-, X_1 + X_2, Y_1 + Y_2, Z_1 + Z_2]$ | trivial |
| $[(\bullet)^{2T} + \Gamma_1^+ + \Gamma_1^-, 2R_1, S_1^+ + S_1^- + S_2^+ + S_2^-, T_1^+ + T_1^-, 2U_1^-, X_1 + X_2, Y_1 + Y_2, Z_1 + Z_2]$             | trivial |
| $[(\bullet)^{2T} + \Gamma_1^+ + \Gamma_1^-, 2R_1, S_1^+ + S_1^- + S_2^+ + S_2^-, T_1^+ + T_1^-, U_1^+ + U_1^-, X_1 + X_2, Y_1 + Y_2, Z_1 + Z_2]$      | 1       |
| $[(\bullet)^{2T} + \Gamma_1^+ + \Gamma_1^-, R_1 + R_2, S_1^- + S_2^- + S_3^- + S_4^-, 2T_1^-, 2U_1^+, X_1 + X_2, Y_1 + Y_2, Z_1 + Z_2]$               | trivial |
| $[(\bullet)^{2T} + \Gamma_1^+ + \Gamma_1^-, 2R_1, S_1^+ + S_1^- + S_2^+ + S_2^-, 2T_1^-, 2U_1^+, X_1 + X_2, Y_1 + Y_2, Z_1 + Z_2]$                    | 1       |
| $[(\bullet)^{2T} + \Gamma_1^+ + \Gamma_1^-, R_1 + R_2, S_1^- + S_2^- + S_3^- + S_4^-, T_1^+ + T_1^-, 2U_1^+, X_1 + X_2, Y_1 + Y_2, Z_1 + Z_2]$        | 1       |
| $[(\bullet)^{2T} + \Gamma_1^+ + \Gamma_1^-, 2R_1, S_1^+ + S_1^- + S_2^+ + S_2^-, T_1^+ + T_1^-, 2U_1^+, X_1 + X_2, Y_1 + Y_2, Z_1 + Z_2]$             | trivial |
| $[(\bullet)^{2T} + \Gamma_1^+ + \Gamma_1^-, 2R_2, S_3^+ + S_3^- + S_4^+ + S_4^-, 2T_1^+, 2U_1^-, X_1 + X_2, Y_1 + Y_2, Z_1 + Z_2]$                    | 1       |
| $[(\bullet)^{2T} + \Gamma_1^+ + \Gamma_1^-, 2R_2, S_3^+ + S_3^- + S_4^+ + S_4^-, 2T_1^+, U_1^+ + U_1^-, X_1 + X_2, Y_1 + Y_2, Z_1 + Z_2]$             | trivial |
| $[(\bullet)^{2T} + \Gamma_1^+ + \Gamma_1^-, R_1 + R_2, S_1^+ + S_2^+ + S_3^+ + S_4^+, 2T_1^+, 2U_1^-, X_1 + X_2, Y_1 + Y_2, Z_1 + Z_2]$               | trivial |
| $[(\bullet)^{2T} + \Gamma_1^+ + \Gamma_1^-, R_1 + R_2, S_1^+ + S_2^+ + S_3^+ + S_4^+, 2T_1^+, U_1^+ + U_1^-, X_1 + X_2, Y_1 + Y_2, Z_1 + Z_2]$        | 1       |
| $[(\bullet)^{2T} + \Gamma_1^+ + \Gamma_1^-, 2R_2, S_3^+ + S_3^- + S_4^+ + S_4^-, 2T_1^+, 2U_1^+, X_1 + X_2, Y_1 + Y_2, Z_1 + Z_2]$                    | 1       |
| $[(\bullet)^{2T} + \Gamma_1^+ + \Gamma_1^-, R_1 + R_2, S_1^+ + S_2^+ + S_3^+ + S_4^+, 2T_1^+, 2U_1^+, X_1 + X_2, Y_1 + Y_2, Z_1 + Z_2]$               | trivial |
| $[(\bullet)^{2T} + \Gamma_1^+ + \Gamma_1^-, R_1 + R_2, S_1^- + S_2^- + S_3^- + S_4^-, 2T_1^+, 2U_1^-, X_1 + X_2, Y_1 + Y_2, Z_1 + Z_2]$               | trivial |
| $[(\bullet)^{2T} + \Gamma_1^+ + \Gamma_1^-, R_1 + R_2, S_1^- + S_2^- + S_3^- + S_4^-, 2T_1^+, U_1^+ + U_1^-, X_1 + X_2, Y_1 + Y_2, Z_1 + Z_2]$        | 1       |
| $[(\bullet)^{2T} + \Gamma_1^+ + \Gamma_1^-, 2R_1, S_1^+ + S_1^- + S_2^+ + S_2^-, 2T_1^+, 2U_1^-, X_1 + X_2, Y_1 + Y_2, Z_1 + Z_2]$                    | 1       |
| $[(\bullet)^{2T} + \Gamma_1^+ + \Gamma_1^-, 2R_1, S_1^+ + S_1^- + S_2^+ + S_2^-, 2T_1^+, U_1^+ + U_1^-, X_1 + X_2, Y_1 + Y_2, Z_1 + Z_2]$             | trivial |
| $[(\bullet)^{2T} + \Gamma_1^+ + \Gamma_1^-, R_1 + R_2, S_1^- + S_2^- + S_3^- + S_4^-, 2T_1^+, 2U_1^+, X_1 + X_2, Y_1 + Y_2, Z_1 + Z_2]$               | trivial |
| $[(\bullet)^{2T} + \Gamma_1^+ + \Gamma_1^-, 2R_1, S_1^+ + S_1^- + S_2^+ + S_2^-, 2T_1^+, 2U_1^+, X_1 + X_2, Y_1 + Y_2, Z_1 + Z_2]$                    | 1       |

2nd minimal solution:  $\mu_2^T = 6$  (384 symmetry vectors)

Space group 59 ( $\mathbb{Z}_1$ )

1st minimal solution:  $\mu_1^T = 4$  (6 symmetry vectors)

| $\mathbf{n}^T$                                                                                                                                |
|-----------------------------------------------------------------------------------------------------------------------------------------------|
| $[(\bullet)^{2T} + \Gamma_1^+ + \Gamma_1^-, 2R_2, 2S_2, T_1 + T_2, U_1 + U_2, X_1 + X_2, Y_1 + Y_2, Z_1^- + Z_2^- + Z_3^- + Z_4^-]$           |
| $[(\bullet)^{2T} + \Gamma_1^+ + \Gamma_1^-, R_1 + R_2, S_1 + S_2, T_1 + T_2, U_1 + U_2, X_1 + X_2, Y_1 + Y_2, Z_1^- + Z_2^- + Z_3^- + Z_4^-]$ |
| $[(\bullet)^{2T} + \Gamma_1^+ + \Gamma_1^-, 2R_2, 2S_2, T_1 + T_2, U_1 + U_2, X_1 + X_2, Y_1 + Y_2, Z_1^+ + Z_2^+ + Z_3^+ + Z_4^+]$           |
| $[(\bullet)^{2T} + \Gamma_1^+ + \Gamma_1^-, R_1 + R_2, S_1 + S_2, T_1 + T_2, U_1 + U_2, X_1 + X_2, Y_1 + Y_2, Z_1^+ + Z_2^+ + Z_3^+ + Z_4^+]$ |
| $[(\bullet)^{2T} + \Gamma_1^+ + \Gamma_1^-, 2R_1, 2S_1, T_1 + T_2, U_1 + U_2, X_1 + X_2, Y_1 + Y_2, Z_1^- + Z_2^- + Z_3^- + Z_4^-]$           |
| $[(\bullet)^{2T} + \Gamma_1^+ + \Gamma_1^-, 2R_1, 2S_1, T_1 + T_2, U_1 + U_2, X_1 + X_2, Y_1 + Y_2, Z_1^+ + Z_2^+ + Z_3^+ + Z_4^+]$           |

2nd minimal solution:  $\mu_2^T = 6$  (40 symmetry vectors)

Space group 60 ( $\mathbb{Z}_2$ )

1st minimal solution:  $\mu_1^T = 4$  (3 symmetry vectors)

| $\mathbf{n}^T$                                                                                                                | $\mathbf{v}^T \in \mathbb{Z}_2$ |
|-------------------------------------------------------------------------------------------------------------------------------|---------------------------------|
| $[(\bullet)^{2T} + \Gamma_1^+ + \Gamma_1^-, R_1 + R_2, 2S_1^-, T_1 + T_2, U_1 + U_2, X_1 + X_2, Y_1 + Y_2, Z_1 + Z_2]$        | trivial                         |
| $[(\bullet)^{2T} + \Gamma_1^+ + \Gamma_1^-, R_1 + R_2, S_1^+ + S_1^-, T_1 + T_2, U_1 + U_2, X_1 + X_2, Y_1 + Y_2, Z_1 + Z_2]$ | 1                               |
| $[(\bullet)^{2T} + \Gamma_1^+ + \Gamma_1^-, R_1 + R_2, 2S_1^+, T_1 + T_2, U_1 + U_2, X_1 + X_2, Y_1 + Y_2, Z_1 + Z_2]$        | trivial                         |

2nd minimal solution:  $\mu_2^T = 8$  (20 symmetry vectors)

Space group 61 ( $\mathbb{Z}_2$ )

1st minimal solution:  $\mu_1^T = 4$  (3 symmetry vectors)

| $\mathbf{n}^T$                                                                                                                     | $\mathbf{v}^T \in \mathbb{Z}_2$ |
|------------------------------------------------------------------------------------------------------------------------------------|---------------------------------|
| $[(\blacksquare)^{2T} + \Gamma_1^+ + \Gamma_1^-, 2R_1^-, S_1 + S_2, T_1 + T_2, U_1 + U_2, X_1 + X_2, Y_1 + Y_2, Z_1 + Z_2]$        | trivial                         |
| $[(\blacksquare)^{2T} + \Gamma_1^+ + \Gamma_1^-, R_1^+ + R_1^-, S_1 + S_2, T_1 + T_2, U_1 + U_2, X_1 + X_2, Y_1 + Y_2, Z_1 + Z_2]$ | 1                               |
| $[(\blacksquare)^{2T} + \Gamma_1^+ + \Gamma_1^-, 2R_1^+, S_1 + S_2, T_1 + T_2, U_1 + U_2, X_1 + X_2, Y_1 + Y_2, Z_1 + Z_2]$        | trivial                         |

2nd minimal solution:  $\mu_2^T = 8$  (10 symmetry vectors)

Space group 62 ( $\mathbb{Z}_1$ )

1st minimal solution:  $\mu_1^T = 4$  (2 symmetry vectors)

| $\mathbf{n}^T$                                                                                                                                     |
|----------------------------------------------------------------------------------------------------------------------------------------------------|
| $[(\blacksquare)^{2T} + \Gamma_1^+ + \Gamma_1^-, R_1 + R_2, S_1 + S_2, T_1 + T_2, U_1^+ + U_2^+ + U_3^+ + U_4^+, X_1 + X_2, Y_1 + Y_2, Z_1 + Z_2]$ |
| $[(\blacksquare)^{2T} + \Gamma_1^+ + \Gamma_1^-, R_1 + R_2, S_1 + S_2, T_1 + T_2, U_1^- + U_2^- + U_3^- + U_4^-, X_1 + X_2, Y_1 + Y_2, Z_1 + Z_2]$ |

2nd minimal solution:  $\mu_2^T = 8$  (10 symmetry vectors)

Space group 63 ( $\mathbb{Z}_1$ )

1st minimal solution:  $\mu_1^T = 4$  (10 symmetry vectors)

| $\mathbf{n}^T$                                                                                                                              |
|---------------------------------------------------------------------------------------------------------------------------------------------|
| $[(\blacksquare)^{2T} + \Gamma_1^+ + \Gamma_2^+, T_1 + T_2, Y_2^+ + Y_2^- + Y_3^- + Y_4^-, Z_1 + Z_2, 2R_1, 2S_1^+ + S_2^+ + S_2^-]$        |
| $[(\blacksquare)^{2T} + \Gamma_1^+ + \Gamma_1^-, T_1 + T_2, Y_1^- + Y_2^- + Y_3^- + Y_4^-, Z_1 + Z_2, 2R_1, S_1^+ + S_1^- + S_2^+ + S_2^-]$ |
| $[(\blacksquare)^{2T} + \Gamma_1^+ + \Gamma_1^-, T_1 + T_2, Y_1^- + Y_2^- + Y_3^- + Y_4^-, Z_1 + Z_2, 2R_1, 2S_1^+ + 2S_2^+]$               |
| $[(\blacksquare)^{2T} + \Gamma_1^- + \Gamma_2^-, T_1 + T_2, Y_2^+ + Y_2^- + Y_3^+ + Y_4^+, Z_1 + Z_2, 2R_1, 2S_1^- + S_2^+ + S_2^-]$        |
| $[(\blacksquare)^{2T} + \Gamma_1^- + \Gamma_2^-, T_1 + T_2, Y_2^+ + Y_2^- + Y_3^+ + Y_4^+, Z_1 + Z_2, 2R_1, S_1^+ + S_1^- + 2S_2^+]$        |
| $[(\blacksquare)^{2T} + \Gamma_1^+ + \Gamma_2^+, T_1 + T_2, Y_2^+ + Y_2^- + Y_3^- + Y_4^-, Z_1 + Z_2, 2R_1, S_1^+ + S_1^- + 2S_2^-]$        |
| $[(\blacksquare)^{2T} + \Gamma_1^+ + \Gamma_1^-, T_1 + T_2, Y_1^- + Y_2^- + Y_3^- + Y_4^-, Z_1 + Z_2, 2R_1, 2S_1^- + 2S_2^-]$               |
| $[(\blacksquare)^{2T} + \Gamma_1^+ + \Gamma_1^-, T_1 + T_2, Y_1^+ + Y_2^+ + Y_3^+ + Y_4^+, Z_1 + Z_2, 2R_1, 2S_1^- + 2S_2^-]$               |
| $[(\blacksquare)^{2T} + \Gamma_1^+ + \Gamma_1^-, T_1 + T_2, Y_1^+ + Y_2^+ + Y_3^+ + Y_4^+, Z_1 + Z_2, 2R_1, S_1^+ + S_1^- + S_2^+ + S_2^-]$ |
| $[(\blacksquare)^{2T} + \Gamma_1^+ + \Gamma_1^-, T_1 + T_2, Y_1^+ + Y_2^+ + Y_3^+ + Y_4^+, Z_1 + Z_2, 2R_1, 2S_1^+ + 2S_2^+]$               |

2nd minimal solution:  $\mu_2^T = 6$  (90 symmetry vectors)

Space group 64 ( $\mathbb{Z}_1$ )

1st minimal solution:  $\mu_1^T = 4$  (6 symmetry vectors)

| $\mathbf{n}^T$                                                                                                                         |
|----------------------------------------------------------------------------------------------------------------------------------------|
| $[(\bullet)^{2T} + \Gamma_1^+ + \Gamma_1^-, T_1 + T_2, Y_1^- + Y_2^- + Y_3^- + Y_4^-, Z_1 + Z_2, 2R_1^- + 2R_2^-, 2S_1]$               |
| $[(\bullet)^{2T} + \Gamma_1^+ + \Gamma_1^-, T_1 + T_2, Y_1^- + Y_2^- + Y_3^- + Y_4^-, Z_1 + Z_2, R_1^+ + R_1^- + R_2^+ + R_2^-, 2S_1]$ |
| $[(\bullet)^{2T} + \Gamma_1^+ + \Gamma_1^-, T_1 + T_2, Y_1^- + Y_2^- + Y_3^- + Y_4^-, Z_1 + Z_2, 2R_1^+ + 2R_2^+, 2S_1]$               |
| $[(\bullet)^{2T} + \Gamma_1^+ + \Gamma_1^-, T_1 + T_2, Y_1^+ + Y_2^+ + Y_3^+ + Y_4^+, Z_1 + Z_2, 2R_1^- + 2R_2^-, 2S_1]$               |
| $[(\bullet)^{2T} + \Gamma_1^+ + \Gamma_1^-, T_1 + T_2, Y_1^+ + Y_2^+ + Y_3^+ + Y_4^+, Z_1 + Z_2, R_1^+ + R_1^- + R_2^+ + R_2^-, 2S_1]$ |
| $[(\bullet)^{2T} + \Gamma_1^+ + \Gamma_1^-, T_1 + T_2, Y_1^+ + Y_2^+ + Y_3^+ + Y_4^+, Z_1 + Z_2, 2R_1^+ + 2R_2^+, 2S_1]$               |

2nd minimal solution:  $\mu_2^T = 6$  (40 symmetry vectors)

Space group 65 ( $\mathbb{Z}_1$ )

1st minimal solution:  $\mu_1^T = 2$  (8 symmetry vectors)

| $\mathbf{n}^T$                                                                                |
|-----------------------------------------------------------------------------------------------|
| $[(\bullet)^{2T}, T_1^- + T_2^-, Y_2^+ + Y_2^-, Z_3^+ + Z_4^+, 2R_2^+, S_2^+ + S_2^-]$        |
| $[(\bullet)^{2T}, T_1^- + T_2^-, Y_2^+ + Y_2^-, Z_3^+ + Z_4^+, R_1^- + R_2^+, S_1^- + S_2^-]$ |
| $[(\bullet)^{2T}, T_1^+ + T_2^+, Y_2^+ + Y_2^-, Z_3^- + Z_4^-, 2R_2^-, S_2^+ + S_2^-]$        |
| $[(\bullet)^{2T}, T_1^- + T_2^-, Y_2^+ + Y_2^-, Z_3^+ + Z_4^+, R_1^- + R_2^+, S_1^+ + S_2^+]$ |
| $[(\bullet)^{2T}, T_1^- + T_2^-, Y_2^+ + Y_2^-, Z_3^+ + Z_4^+, 2R_1^-, S_1^+ + S_1^-]$        |
| $[(\bullet)^{2T}, T_1^+ + T_2^+, Y_2^+ + Y_2^-, Z_3^- + Z_4^-, R_1^+ + R_2^-, S_1^+ + S_2^+]$ |
| $[(\bullet)^{2T}, T_1^+ + T_2^+, Y_2^+ + Y_2^-, Z_3^- + Z_4^-, R_1^+ + R_2^-, S_1^- + S_2^-]$ |
| $[(\bullet)^{2T}, T_1^+ + T_2^+, Y_2^+ + Y_2^-, Z_3^- + Z_4^-, 2R_1^+, S_1^+ + S_1^-]$        |

2nd minimal solution:  $\mu_2^T = 3$  (400 symmetry vectors)

Space group 66 ( $\mathbb{Z}_2$ )

1st minimal solution:  $\mu_1^T = 2$  (6 symmetry vectors)

| $\mathbf{n}^T$                                                            | $\mathbf{v}^T \in \mathbb{Z}_2$ |
|---------------------------------------------------------------------------|---------------------------------|
| $[(\bullet)^{2T}, T_1, Y_2^+ + Y_2^-, Z_2, R_2^+ + R_2^-, S_2^+ + S_2^-]$ | 1                               |
| $[(\bullet)^{2T}, T_1, Y_2^+ + Y_2^-, Z_2, R_1^+ + R_2^+, S_1^- + S_2^-]$ | trivial                         |
| $[(\bullet)^{2T}, T_1, Y_2^+ + Y_2^-, Z_2, R_1^- + R_2^-, S_1^+ + S_2^+]$ | trivial                         |
| $[(\bullet)^{2T}, T_1, Y_2^+ + Y_2^-, Z_2, R_1^+ + R_2^+, S_1^+ + S_2^+]$ | trivial                         |
| $[(\bullet)^{2T}, T_1, Y_2^+ + Y_2^-, Z_2, R_1^+ + R_1^-, S_1^+ + S_1^-]$ | 1                               |
| $[(\bullet)^{2T}, T_1, Y_2^+ + Y_2^-, Z_2, R_1^- + R_2^-, S_1^- + S_2^-]$ | trivial                         |

2nd minimal solution:  $\mu_2^T = 4$  (261 symmetry vectors)

Space group 67 ( $\mathbb{Z}_1$ )

1st minimal solution:  $\mu_1^T = 4$  (70 symmetry vectors)

$$\overline{n^T}$$

$$\begin{aligned}
& [(\mathbf{u})^{2T} + \Gamma_1^+ + \Gamma_1^-, T_1^+ + T_2^+ + T_3^+ + T_4^-, Y_1^+ + Y_2^+ + Y_3^+ + Y_4^-, Z_1^- + Z_2^- + Z_3^- + Z_4^-, 2R_1, 2S_1] \\
& [(\mathbf{u})^{2T} + \Gamma_1^- + \Gamma_3^-, T_2^+ + T_3^+ + T_3^- + T_4^-, Y_2^+ + Y_3^+ + Y_3^- + Y_4^-, Z_2^+ + Z_3^+ + Z_3^- + Z_4^-, 2R_1, 2S_1] \\
& [(\mathbf{u})^{2T} + \Gamma_3^+ + \Gamma_3^-, T_1^+ + T_2^+ + T_3^+ + T_4^-, Y_2^+ + Y_2^- + Y_3^+ + Y_3^-, Z_3^+ + Z_3^- + Z_4^+ + Z_4^-, 2R_1, 2S_1] \\
& [(\mathbf{u})^{2T} + \Gamma_1^+ + \Gamma_2^-, T_2^+ + T_2^- + T_3^+ + T_4^-, Y_2^+ + Y_2^- + Y_3^+ + Y_4^-, 2Z_2^- + Z_3^- + Z_4^- + Z_4^-, 2R_1, 2S_1] \\
& [(\mathbf{u})^{2T} + \Gamma_1^- + \Gamma_3^-, T_1^- + T_3^+ + 2T_3^-, Y_2^+ + Y_3^+ + Y_3^- + Y_4^-, Z_1^- + Z_3^+ + 2Z_3^-, 2R_1, 2S_1] \\
& [(\mathbf{u})^{2T} + \Gamma_3^- + \Gamma_4^+, T_1^- + T_2^+ + T_3^+ + T_3^-, 2Y_2^+ + Y_3^+ + Y_4^-, Z_3^+ + 2Z_3^- + Z_4^-, 2R_1, 2S_1] \\
& [(\mathbf{u})^{2T} + \Gamma_1^+ + \Gamma_1^-, T_2^+ + T_2^- + T_3^+ + T_3^-, Y_1^+ + Y_2^+ + Y_2^- + Y_3^+ + Y_4^-, Z_2^+ + Z_2^- + Z_3^+ + Z_3^-, 2R_1, 2S_1] \\
& [(\mathbf{u})^{2T} + \Gamma_1^+ + \Gamma_1^-, T_1^+ + T_1^- + T_3^+ + T_3^-, Y_1^+ + Y_2^+ + Y_3^+ + Y_4^-, Z_1^+ + Z_1^- + Z_3^+ + Z_3^-, 2R_1, 2S_1] \\
& [(\mathbf{u})^{2T} + \Gamma_1^+ + \Gamma_4^+, T_2^+ + 2T_3^+ + T_3^-, Y_2^+ + Y_3^+ + Y_4^+ + Y_4^-, Z_2^- + Z_3^+ + 2Z_3^-, 2R_1, 2S_1] \\
& [(\mathbf{u})^{2T} + \Gamma_1^+ + \Gamma_4^+, T_1^- + T_3^+ + T_3^- + T_4^-, Y_2^+ + Y_3^+ + Y_3^- + Y_4^-, Z_1^+ + Z_3^+ + Z_3^- + Z_4^-, 2R_1, 2S_1] \\
& [(\mathbf{u})^{2T} + \Gamma_1^+ + \Gamma_2^-, T_1^+ + T_2^+ + 2T_3^-, Y_2^+ + Y_2^- + Y_3^+ + Y_4^-, Z_1^+ + Z_2^- + Z_3^+ + Z_3^-, 2R_1, 2S_1] \\
& [(\mathbf{u})^{2T} + \Gamma_2^- + \Gamma_3^-, T_1^+ + T_1^- + T_2^+ + T_3^-, 2Y_2^+ + Y_2^- + Y_3^+, Z_1^+ + Z_3^+ + Z_3^- + Z_4^-, 2R_1, 2S_1] \\
& [(\mathbf{u})^{2T} + \Gamma_1^+ + \Gamma_3^+, T_1^+ + T_2^+ + T_2^- + T_3^-, Y_1^+ + Y_2^+ + Y_2^- + Y_3^+, Z_2^- + Z_3^+ + Z_3^- + Z_4^-, 2R_1, 2S_1] \\
& [(\mathbf{u})^{2T} + \Gamma_1^+ + \Gamma_4^+, T_2^+ + T_3^+ + T_4^+ + T_4^-, Y_2^+ + Y_3^+ + Y_4^+ + Y_4^-, Z_2^- + Z_3^- + Z_4^+ + Z_4^-, 2R_1, 2S_1] \\
& [(\mathbf{u})^{2T} + \Gamma_1^- + \Gamma_4^-, T_1^+ + 2T_4^+ + T_4^-, Y_2^- + Y_3^- + Y_4^+ + Y_4^-, Z_1^- + Z_4^+ + 2Z_4^-, 2R_1, 2S_1] \\
& [(\mathbf{u})^{2T} + \Gamma_1^- + \Gamma_2^+, T_1^+ + T_2^+ + 2T_4^-, Y_2^+ + Y_2^- + Y_3^- + Y_4^+, Z_1^- + Z_2^+ + Z_4^+ + Z_4^-, 2R_1, 2S_1] \\
& [(\mathbf{u})^{2T} + \Gamma_1^- + \Gamma_2^+, T_1^+ + T_1^- + T_3^- + T_4^-, Y_2^+ + Y_2^- + Y_3^- + Y_4^+, 2Z_1^- + Z_3^- + Z_4^- + Z_4^-, 2R_1, 2S_1] \\
& [(\mathbf{u})^{2T} + \Gamma_1^- + \Gamma_4^-, T_1^+ + T_3^+ + T_3^- + T_4^-, Y_2^- + Y_3^- + Y_4^+ + Y_4^-, Z_1^- + Z_3^+ + Z_3^- + Z_4^- + Z_4^-, 2R_1, 2S_1] \\
& [(\mathbf{u})^{2T} + \Gamma_1^+ + \Gamma_1^-, T_1^+ + T_1^- + T_4^+ + T_4^-, Y_1^+ + Y_2^+ + Y_3^+ + Y_4^+, Z_1^+ + Z_1^- + Z_4^+ + Z_4^-, 2R_1, 2S_1] \\
& [(\mathbf{u})^{2T} + \Gamma_2^+ + \Gamma_4^+, T_1^+ + T_1^- + T_2^+ + T_4^-, 2Y_2^+ + Y_2^- + Y_4^+, Z_1^- + Z_3^- + Z_4^+ + Z_4^-, 2R_1, 2S_1] \\
& [(\mathbf{u})^{2T} + \Gamma_1^+ + \Gamma_1^-, T_3^+ + T_3^- + T_4^+ + T_4^-, Y_3^+ + Y_3^- + Y_4^+ + Y_4^-, Z_1^- + Z_2^- + Z_3^- + Z_4^- + Z_4^-, 2R_1, 2S_1] \\
& [(\mathbf{u})^{2T} + \Gamma_1^- + \Gamma_3^-, T_2^+ + 2T_4^+ + T_4^-, Y_2^+ + Y_3^+ + Y_3^- + Y_4^+, Z_2^+ + 2Z_4^+ + Z_4^-, 2R_1, 2S_1] \\
& [(\mathbf{u})^{2T} + \Gamma_1^- + \Gamma_3^-, T_1^- + T_3^- + T_4^+ + T_4^-, Y_2^+ + Y_3^+ + Y_3^- + Y_4^+, Z_1^- + Z_3^- + Z_4^+ + Z_4^-, 2R_1, 2S_1] \\
& [(\mathbf{u})^{2T} + \Gamma_3^- + \Gamma_4^+, T_1^- + T_2^+ + T_4^+ + T_4^-, 2Y_2^+ + Y_3^+ + Y_4^+, Z_3^- + 2Z_4^+ + Z_4^-, 2R_1, 2S_1] \\
& [(\mathbf{u})^{2T} + \Gamma_1^+ + \Gamma_1^-, T_2^+ + T_2^- + T_4^+ + T_4^-, Y_1^+ + Y_2^+ + Y_3^+ + Y_4^+, Z_2^+ + Z_2^- + Z_4^+ + Z_4^-, 2R_1, 2S_1] \\
& [(\mathbf{u})^{2T} + \Gamma_1^+ + \Gamma_4^+, T_1^- + T_4^+ + 2T_4^-, Y_2^+ + Y_3^+ + Y_4^+ + Y_4^-, Z_1^+ + 2Z_4^+ + Z_4^-, 2R_1, 2S_1] \\
& [(\mathbf{u})^{2T} + \Gamma_1^- + \Gamma_4^-, T_2^- + T_3^- + T_4^+ + T_4^-, Y_2^- + Y_3^- + Y_4^+ + Y_4^-, Z_2^+ + Z_3^- + Z_4^+ + Z_4^-, 2R_1, 2S_1] \\
& [(\mathbf{u})^{2T} + \Gamma_3^- + \Gamma_4^-, T_1^+ + T_2^- + T_4^+ + T_4^-, 2Y_2^- + Y_3^- + Y_4^-, Z_3^+ + Z_4^+ + 2Z_4^-, 2R_1, 2S_1] \\
& [(\mathbf{u})^{2T} + \Gamma_1^+ + \Gamma_1^-, T_2^+ + T_2^- + T_4^+ + T_4^-, Y_1^+ + Y_2^- + Y_3^- + Y_4^-, Z_2^+ + Z_2^- + Z_4^+ + Z_4^-, 2R_1, 2S_1] \\
& [(\mathbf{u})^{2T} + \Gamma_1^+ + \Gamma_1^-, T_1^+ + T_1^- + T_4^+ + T_4^-, Y_1^+ + Y_2^- + Y_3^- + Y_4^-, Z_1^+ + Z_1^- + Z_4^+ + Z_4^-, 2R_1, 2S_1] \\
& [(\mathbf{u})^{2T} + \Gamma_1^+ + \Gamma_3^+, T_2^- + T_4^+ + 2T_4^-, Y_2^- + Y_3^+ + Y_3^- + Y_4^-, Z_2^- + Z_4^+ + 2Z_4^-, 2R_1, 2S_1] \\
& [(\mathbf{u})^{2T} + \Gamma_1^+ + \Gamma_3^+, T_1^+ + T_3^+ + T_4^+ + T_4^-, Y_2^- + Y_3^+ + Y_3^- + Y_4^-, Z_1^+ + Z_3^+ + Z_4^+ + Z_4^-, 2R_1, 2S_1] \\
& [(\mathbf{u})^{2T} + \Gamma_1^- + \Gamma_3^-, T_1^+ + T_1^- + T_2^+ + T_4^-, Y_1^- + Y_2^+ + Y_2^- + Y_3^-, Z_1^- + Z_3^- + Z_4^+ + Z_4^-, 2R_1, 2S_1] \\
& [(\mathbf{u})^{2T} + \Gamma_1^- + \Gamma_2^+, T_2^+ + T_2^- + T_3^- + T_4^-, Y_2^+ + Y_2^- + Y_3^- + Y_4^+, 2Z_2^+ + Z_3^+ + Z_4^+, 2R_1, 2S_1] \\
& [(\mathbf{u})^{2T} + \Gamma_1^+ + \Gamma_1^-, T_3^+ + T_3^- + T_4^+ + T_4^-, Y_3^+ + Y_3^- + Y_4^+ + Y_4^-, Z_1^+ + Z_2^+ + Z_3^+ + Z_4^+, 2R_1, 2S_1] \\
& [(\mathbf{u})^{2T} + \Gamma_1^+ + \Gamma_1^-, T_1^+ + T_2^+ + T_3^+ + T_4^-, Y_1^- + Y_2^- + Y_3^- + Y_4^-, Z_1^+ + Z_2^+ + Z_3^+ + Z_4^+, 2R_1, 2S_1] \\
& [(\mathbf{u})^{2T} + \Gamma_2^+ + \Gamma_3^+, T_1^+ + T_2^+ + T_2^- + T_4^-, Y_2^+ + 2Y_2^- + Y_3^-, Z_2^+ + Z_3^+ + Z_4^+ + Z_4^-, 2R_1, 2S_1] \\
& [(\mathbf{u})^{2T} + \Gamma_1^+ + \Gamma_1^-, T_1^- + T_2^- + T_3^- + T_4^-, Y_1^- + Y_2^- + Y_3^- + Y_4^-, Z_1^- + Z_2^- + Z_3^- + Z_4^- + Z_4^-, 2R_1, 2S_1] \\
& [(\mathbf{u})^{2T} + \Gamma_4^+ + \Gamma_4^-, T_1^- + T_2^- + T_3^- + T_4^-, Y_2^+ + Y_2^- + Y_4^+ + Y_4^-, Z_3^+ + Z_3^- + Z_4^+ + Z_4^-, 2R_1, 2S_1] \\
& [(\mathbf{u})^{$$

... continued on next page



... continued from previous page

---

|                                                                                                                                                            |
|------------------------------------------------------------------------------------------------------------------------------------------------------------|
| $[(\blacksquare)^{2T} + \Gamma_1^+ + \Gamma_1^-, T_1^- + T_2^- + T_3^- + T_4^-, Y_1^+ + Y_2^+ + Y_3^+ + Y_4^+, Z_1^+ + Z_2^+ + Z_3^+ + Z_4^-, 2R_1, 2S_1]$ |
| $[(\blacksquare)^{2T} + \Gamma_2^+ + \Gamma_4^-, T_1^- + T_2^+ + T_2^- + T_3^-, 2Y_2^+ + Y_2^- + Y_4^+, Z_2^+ + Z_3^+ + Z_3^- + Z_4^-, 2R_1, 2S_1]$        |
| $[(\blacksquare)^{2T} + \Gamma_3^+ + \Gamma_4^-, T_1^+ + T_2^- + T_3^+ + T_3^-, 2Y_2^- + Y_3^- + Y_4^-, 2Z_3^+ + Z_3^- + Z_4^-, 2R_1, 2S_1]$               |
| $[(\blacksquare)^{2T} + \Gamma_1^+ + \Gamma_1^-, T_2^+ + T_2^- + T_3^+ + T_3^-, Y_1^- + Y_2^- + Y_3^- + Y_4^-, Z_2^+ + Z_2^- + Z_3^+ + Z_3^-, 2R_1, 2S_1]$ |
| $[(\blacksquare)^{2T} + \Gamma_1^+ + \Gamma_3^+, T_1^+ + 2T_3^+ + T_3^-, Y_2^- + Y_3^+ + Y_3^- + Y_4^-, Z_1^+ + 2Z_3^+ + Z_3^-, 2R_1, 2S_1]$               |
| $[(\blacksquare)^{2T} + \Gamma_1^- + \Gamma_4^-, T_1^+ + T_2^+ + T_2^- + T_4^-, Y_1^+ + Y_2^+ + Y_2^- + Y_4^+, Z_2^+ + Z_3^+ + Z_4^+ + Z_4^-, 2R_1, 2S_1]$ |
| $[(\blacksquare)^{2T} + \Gamma_2^- + \Gamma_4^-, T_1^+ + T_2^+ + T_2^- + T_3^-, Y_2^+ + 2Y_2^- + Y_4^-, Z_2^- + Z_3^+ + Z_3^- + Z_4^-, 2R_1, 2S_1]$        |
| $[(\blacksquare)^{2T} + \Gamma_1^- + \Gamma_3^-, T_1^- + T_2^+ + T_2^- + T_3^-, Y_1^- + Y_2^+ + Y_2^- + Y_3^-, Z_2^+ + Z_3^+ + Z_3^- + Z_4^-, 2R_1, 2S_1]$ |
| $[(\blacksquare)^{2T} + \Gamma_1^+ + \Gamma_2^-, T_1^+ + T_1^- + T_3^+ + T_4^-, Y_2^+ + Y_2^- + Y_3^+ + Y_4^-, 2Z_1^+ + Z_3^+ + Z_4^+, 2R_1, 2S_1]$        |
| $[(\blacksquare)^{2T} + \Gamma_1^+ + \Gamma_3^+, T_1^+ + T_1^- + T_2^- + T_4^-, Y_1^+ + Y_2^+ + Y_2^- + Y_3^+, Z_1^+ + Z_3^+ + Z_4^+ + Z_4^-, 2R_1, 2S_1]$ |
| $[(\blacksquare)^{2T} + \Gamma_1^+ + \Gamma_1^-, T_1^+ + T_2^+ + T_3^+ + T_4^-, Y_1^+ + Y_2^+ + Y_3^+ + Y_4^+, Z_1^+ + Z_2^+ + Z_3^+ + Z_4^+, 2R_1, 2S_1]$ |
| $[(\blacksquare)^{2T} + \Gamma_1^+ + \Gamma_4^-, T_1^+ + T_1^- + T_2^+ + T_3^+, Y_1^- + Y_2^+ + Y_2^- + Y_4^-, Z_1^+ + Z_3^+ + Z_3^- + Z_4^+, 2R_1, 2S_1]$ |
| $[(\blacksquare)^{2T} + \Gamma_1^+ + \Gamma_1^-, T_1^- + T_2^- + T_3^- + T_4^-, Y_1^- + Y_2^- + Y_3^- + Y_4^-, Z_1^+ + Z_2^+ + Z_3^+ + Z_4^+, 2R_1, 2S_1]$ |
| $[(\blacksquare)^{2T} + \Gamma_2^+ + \Gamma_2^-, T_1^+ + T_1^- + T_2^+ + T_2^-, 2Y_2^+ + 2Y_2^-, Z_1^+ + Z_2^+ + Z_3^+ + Z_4^+, 2R_1, 2S_1]$               |
| $[(\blacksquare)^{2T} + \Gamma_1^+ + \Gamma_1^-, T_1^+ + T_1^- + T_2^+ + T_2^-, Y_1^+ + Y_1^- + Y_2^+ + Y_2^-, Z_1^+ + Z_2^+ + Z_3^+ + Z_4^+, 2R_1, 2S_1]$ |
| $[(\blacksquare)^{2T} + \Gamma_3^+ + \Gamma_3^-, T_1^- + T_2^- + T_3^- + T_4^-, Y_2^+ + Y_2^- + Y_3^+ + Y_3^-, Z_3^+ + Z_3^- + Z_4^+ + Z_4^-, 2R_1, 2S_1]$ |
| $[(\blacksquare)^{2T} + \Gamma_4^+ + \Gamma_4^-, T_1^+ + T_2^+ + T_3^+ + T_4^-, Y_2^+ + Y_2^- + Y_4^+ + Y_4^-, Z_3^+ + Z_3^- + Z_4^+ + Z_4^-, 2R_1, 2S_1]$ |

---

2nd minimal solution:  $\mu_2^T = 6$  (1422 symmetry vectors)

Space group 68 ( $\mathbb{Z}_2$ )

1st minimal solution:  $\mu_1^T = 2$  (1 symmetry vector & filling-enforced topology)

| $\mathbf{n}^T$                                             | $\mathbf{v}^T \in \mathbb{Z}_2$ |
|------------------------------------------------------------|---------------------------------|
| $[(\blacksquare)^{2T}, T_1, Y_2^+ + Y_2^-, Z_2, R_1, S_1]$ | 1                               |

2nd minimal solution:  $\mu_2^T = 4$  (7 symmetry vectors)

Space group 69 ( $\mathbb{Z}_1$ )

1st minimal solution:  $\mu_1^T = 3$  (56 symmetry vectors)

| $\mathbf{n}^T$                                                                                                            |
|---------------------------------------------------------------------------------------------------------------------------|
| $[(\blacksquare)^{2T} + \Gamma_1^+, T_2^- + T_3^- + T_4^-, Y_2^- + Y_3^- + Y_4^-, Z_2^- + Z_3^- + Z_4^-, 3L_1^-]$         |
| $[(\blacksquare)^{2T} + \Gamma_1^+, T_2^- + T_3^- + T_4^-, Y_2^- + Y_3^- + Y_4^-, Z_2^- + Z_3^- + Z_4^-, L_1^+ + 2L_1^-]$ |
| $[(\blacksquare)^{2T} + \Gamma_1^+, T_2^- + T_3^- + T_4^-, Y_2^- + Y_3^- + Y_4^-, Z_2^- + Z_3^- + Z_4^-, 2L_1^+ + L_1^-]$ |
| $[(\blacksquare)^{2T} + \Gamma_1^+, T_2^- + T_3^- + T_4^-, Y_2^- + Y_3^- + Y_4^-, Z_2^- + Z_3^- + Z_4^-, 3L_1^+]$         |
| $[(\blacksquare)^{2T} + \Gamma_1^+, T_2^- + T_3^- + T_4^-, Y_1^+ + Y_3^+ + Y_3^-, Z_1^+ + Z_3^+ + Z_3^-, 3L_1^-]$         |
| $[(\blacksquare)^{2T} + \Gamma_1^+, T_2^- + T_3^- + T_4^-, Y_1^+ + Y_3^+ + Y_3^-, Z_1^+ + Z_3^+ + Z_3^-, L_1^+ + 2L_1^-]$ |
| $[(\blacksquare)^{2T} + \Gamma_1^+, T_2^- + T_3^- + T_4^-, Y_1^+ + Y_3^+ + Y_3^-, Z_1^+ + Z_3^+ + Z_3^-, 2L_1^+ + L_1^-]$ |
| $[(\blacksquare)^{2T} + \Gamma_1^+, T_2^- + T_3^- + T_4^-, Y_1^+ + Y_3^+ + Y_3^-, Z_1^+ + Z_3^+ + Z_3^-, 3L_1^+]$         |
| $[(\blacksquare)^{2T} + \Gamma_3^+, T_1^- + T_2^- + T_4^-, Y_2^+ + Y_2^- + Y_3^+, Z_3^+ + Z_4^+ + Z_4^-, 3L_1^-]$         |
| $[(\blacksquare)^{2T} + \Gamma_3^+, T_1^- + T_2^- + T_4^-, Y_2^+ + Y_2^- + Y_3^+, Z_3^+ + Z_4^+ + Z_4^-, L_1^+ + 2L_1^-]$ |
| $[(\blacksquare)^{2T} + \Gamma_3^+, T_1^- + T_2^- + T_4^-, Y_2^+ + Y_2^- + Y_3^+, Z_3^+ + Z_4^+ + Z_4^-, 2L_1^+ + L_1^-]$ |
| $[(\blacksquare)^{2T} + \Gamma_3^+, T_1^- + T_2^- + T_4^-, Y_2^+ + Y_2^- + Y_3^+, Z_3^+ + Z_4^+ + Z_4^-, 3L_1^+]$         |
| $[(\blacksquare)^{2T} + \Gamma_1^+, T_1^+ + T_4^+ + T_4^-, Y_2^- + Y_3^- + Y_4^-, Z_1^+ + Z_4^+ + Z_4^-, 3L_1^-]$         |

... continued on next page

[illegible]

Space group 70 ( $\mathbb{Z}_2$ )

1st minimal solution:  $\mu_1^T = 2$  (3 symmetry vectors)

| $\mathbf{n}^T$                                   | $\mathbf{v}^T \in \mathbb{Z}_2$ |
|--------------------------------------------------|---------------------------------|
| $[(\bullet)^{2T}, T_2, Y_2, Z_2, 2L_1^-]$        | trivial                         |
| $[(\bullet)^{2T}, T_2, Y_2, Z_2, L_1^+ + L_1^-]$ | 1                               |
| $[(\bullet)^{2T}, T_2, Y_2, Z_2, 2L_1^+]$        | trivial                         |

2nd minimal solution:  $\mu_2^T = 4$  (20 symmetry vectors)

Space group 71 ( $\mathbb{Z}_1$ )

1st minimal solution:  $\mu_1^T = 3$  (168 symmetry vectors)

| $\mathbf{n}^T$                                                                                                                               |
|----------------------------------------------------------------------------------------------------------------------------------------------|
| $[(\bullet)^{2T} + \Gamma_1^+, X_2^- + X_3^- + X_4^-, R_2^+ + 2R_2^-, 2S_1^+ + S_1^-, T_2^+ + 2T_2^-, 3W_3]$                                 |
| $[(\bullet)^{2T} + \Gamma_1^+, X_2^- + X_3^- + X_4^-, R_2^+ + 2R_2^-, S_1^+ + S_1^- + S_2^-, T_1^+ + T_2^+ + T_2^-, W_2 + 2W_3]$             |
| $[(\bullet)^{2T} + \Gamma_1^+, X_2^- + X_3^- + X_4^-, R_1^+ + R_2^+ + R_2^-, S_1^+ + S_1^- + S_2^-, T_2^+ + 2T_2^-, 2W_3 + W_4]$             |
| $[(\bullet)^{2T} + \Gamma_1^+, X_2^- + X_3^- + X_4^-, R_1^+ + R_2^+ + R_2^-, 2S_1^+ + S_1^-, T_1^+ + T_2^+ + T_2^-, W_1 + 2W_3]$             |
| $[(\bullet)^{2T} + \Gamma_1^+, X_2^- + X_3^- + X_4^-, R_2^+ + 2R_2^-, S_1^+ + S_1^- + S_2^-, T_1^- + 2T_2^-, W_2 + 2W_3]$                    |
| $[(\bullet)^{2T} + \Gamma_1^+, X_2^- + X_3^- + X_4^-, R_2^+ + 2R_2^-, S_1^- + 2S_2^-, T_1^+ + T_1^- + T_2^-, 2W_2 + W_3]$                    |
| $[(\bullet)^{2T} + \Gamma_1^+, X_2^- + X_3^- + X_4^-, R_1^+ + R_2^+ + R_2^-, S_1^- + 2S_2^-, T_1^- + 2T_2^-, W_2 + W_3 + W_4]$               |
| $[(\bullet)^{2T} + \Gamma_1^+, X_2^- + X_3^- + X_4^-, R_1^+ + R_2^+ + R_2^-, S_1^+ + S_1^- + S_2^-, T_1^+ + T_1^- + T_2^-, W_1 + W_2 + W_3]$ |
| $[(\bullet)^{2T} + \Gamma_1^+, X_2^- + X_3^- + X_4^-, R_1^+ + R_2^+ + R_2^-, S_1^- + 2S_2^-, T_1^+ + T_2^+ + T_2^-, W_2 + W_3 + W_4]$        |
| $[(\bullet)^{2T} + \Gamma_1^+, X_2^- + X_3^- + X_4^-, 2R_1^+ + R_2^+, S_1^- + 2S_2^-, T_2^+ + 2T_2^-, W_3 + 2W_4]$                           |
| $[(\bullet)^{2T} + \Gamma_1^+, X_2^- + X_3^- + X_4^-, 2R_1^+ + R_2^+, S_1^+ + S_1^- + S_2^-, T_1^+ + T_2^+ + T_2^-, W_1 + W_3 + W_4]$        |
| $[(\bullet)^{2T} + \Gamma_1^+, X_2^- + X_3^- + X_4^-, R_1^+ + R_2^+ + R_2^-, 2S_1^+ + S_1^-, T_1^- + 2T_2^-, W_1 + 2W_3]$                    |
| $[(\bullet)^{2T} + \Gamma_1^+, X_2^- + X_3^- + X_4^-, 2R_1^+ + R_2^+, S_1^+ + S_1^- + S_2^-, T_1^- + 2T_2^-, W_1 + W_3 + W_4]$               |
| $[(\bullet)^{2T} + \Gamma_1^+, X_2^- + X_3^- + X_4^-, 2R_1^+ + R_2^+, 2S_1^+ + S_1^-, T_1^+ + T_1^- + T_2^-, 2W_1 + W_3]$                    |
| $[(\bullet)^{2T} + \Gamma_1^+, X_2^- + X_3^- + X_4^-, R_2^+ + 2R_2^-, S_1^- + 2S_2^-, 2T_1^+ + T_2^+, 2W_2 + W_3]$                           |
| $[(\bullet)^{2T} + \Gamma_1^+, X_2^- + X_3^- + X_4^-, R_1^+ + R_2^+ + R_2^-, S_1^+ + S_1^- + S_2^-, 2T_1^+ + T_2^+, W_1 + W_2 + W_3]$        |
| $[(\bullet)^{2T} + \Gamma_1^+, X_2^- + X_3^- + X_4^-, R_1^+ + R_2^+ + R_2^-, S_1^- + 2S_2^-, 2T_1^+ + T_1^-, W_1 + 2W_2]$                    |
| $[(\bullet)^{2T} + \Gamma_1^+, X_2^- + X_3^- + X_4^-, 2R_1^+ + R_2^+, S_1^- + 2S_2^-, 2T_1^+ + T_2^+, W_1 + W_2 + W_4]$                      |
| $[(\bullet)^{2T} + \Gamma_1^+, X_2^- + X_3^- + X_4^-, 2R_1^+ + R_2^+, S_1^- + 2S_2^-, T_1^+ + T_1^- + T_2^-, W_1 + W_2 + W_4]$               |
| $[(\bullet)^{2T} + \Gamma_1^+, X_2^- + X_3^- + X_4^-, R_1^- + 2R_2^-, S_1^+ + S_1^- + S_2^-, T_2^+ + 2T_2^-, 2W_3 + W_4]$                    |
| $[(\bullet)^{2T} + \Gamma_1^+, X_2^- + X_3^- + X_4^-, R_1^- + 2R_2^-, S_1^- + 2S_2^-, T_1^+ + T_2^+ + T_2^-, W_2 + W_3 + W_4]$               |
| $[(\bullet)^{2T} + \Gamma_1^+, X_2^- + X_3^- + X_4^-, R_1^+ + R_1^- + R_2^-, S_1^- + 2S_2^-, T_2^+ + 2T_2^-, W_3 + 2W_4]$                    |
| $[(\bullet)^{2T} + \Gamma_1^+, X_2^- + X_3^- + X_4^-, R_1^+ + R_1^- + R_2^-, S_1^+ + S_1^- + S_2^-, T_1^+ + T_2^+ + T_2^-, W_1 + W_3 + W_4]$ |
| $[(\bullet)^{2T} + \Gamma_1^+, X_2^- + X_3^- + X_4^-, R_1^- + 2R_2^-, S_1^- + 2S_2^-, T_1^- + 2T_2^-, W_2 + W_3 + W_4]$                      |
| $[(\bullet)^{2T} + \Gamma_1^+, X_2^- + X_3^- + X_4^-, R_1^+ + R_1^- + R_2^-, S_1^- + 2S_2^-, T_1^+ + T_1^- + T_2^-, W_1 + W_2 + W_4]$        |
| $[(\bullet)^{2T} + \Gamma_1^+, X_2^- + X_3^- + X_4^-, 2R_1^+ + R_1^-, S_1^- + 2S_2^-, T_1^+ + T_2^+ + T_2^-, W_1 + 2W_4]$                    |
| $[(\bullet)^{2T} + \Gamma_1^+, X_2^- + X_3^- + X_4^-, R_1^+ + R_1^- + R_2^-, S_1^+ + S_1^- + S_2^-, T_1^- + 2T_2^-, W_1 + W_3 + W_4]$        |
| $[(\bullet)^{2T} + \Gamma_1^+, X_2^- + X_3^- + X_4^-, 2R_1^+ + R_1^-, S_1^- + 2S_2^-, T_1^- + 2T_2^-, W_1 + 2W_4]$                           |
| $[(\bullet)^{2T} + \Gamma_1^+, X_2^- + X_3^- + X_4^-, 2R_1^+ + R_1^-, S_1^+ + S_1^- + S_2^-, T_1^+ + T_1^- + T_2^-, 2W_1 + W_4]$             |
| $[(\bullet)^{2T} + \Gamma_1^+, X_2^- + X_3^- + X_4^-, R_1^- + 2R_2^-, 2S_1^+ + S_1^-, T_1^+ + T_2^+ + T_2^-, W_1 + 2W_3]$                    |
| $[(\bullet)^{2T} + \Gamma_1^+, X_2^- + X_3^- + X_4^-, R_1^- + 2R_2^-, S_1^+ + S_1^- + S_2^-, 2T_1^+ + T_2^+, W_1 + W_2 + W_3]$               |
| $[(\bullet)^{2T} + \Gamma_1^+, X_2^- + X_3^- + X_4^-, R_1^+ + R_1^- + R_2^-, 2S_1^+ + S_1^-, 2T_1^+ + T_2^+, 2W_1 + W_3]$                    |
| $[(\bullet)^{2T} + \Gamma_1^+, X_2^- + X_3^- + X_4^-, R_1^- + 2R_2^-, S_1^+ + S_1^- + S_2^-, T_1^+ + T_1^- + T_2^-, W_1 + W_2 + W_3]$        |
| $[(\bullet)^{2T} + \Gamma_1^+, X_2^- + X_3^- + X_4^-, R_1^- + 2R_2^-, S_1^- + 2S_2^-, 2T_1^+ + T_1^-, W_1 + 2W_2]$                           |
| $[(\bullet)^{2T} + \Gamma_1^+, X_2^- + X_3^- + X_4^-, R_1^+ + R_1^- + R_2^-, S_1^+ + S_1^- + S_2^-, 2T_1^+ + T_1^-, 2W_1 + W_2]$             |
| $[(\bullet)^{2T} + \Gamma_1^+, X_2^- + X_3^- + X_4^-, 2R_1^+ + R_1^-, S_1^+ + S_1^- + S_2^-, 2T_1^+ + T_2^+, W_1 + W_2 + W_4]$               |

... continued on next page

... continued on next page

... continued on next page

... continued from previous page

---

|                                                                                                                                              |
|----------------------------------------------------------------------------------------------------------------------------------------------|
| $[(\bullet)^{2T} + \Gamma_1^-, X_2^+ + X_3^+ + X_4^+, R_1^+ + R_1^- + R_2^+, S_1^- + S_2^+ + S_2^-, 2T_1^- + T_2^-, W_1 + W_2 + W_4]$        |
| $[(\bullet)^{2T} + \Gamma_1^-, X_2^+ + X_3^+ + X_4^+, R_1^+ + R_1^- + R_2^+, S_1^+ + 2S_2^+, 2T_1^- + T_2^-, W_1 + W_2 + W_4]$               |
| $[(\bullet)^{2T} + \Gamma_1^-, X_2^+ + X_3^+ + X_4^+, R_1^+ + R_1^- + R_2^+, S_1^+ + 2S_1^-, 2T_1^- + T_2^-, 2W_1 + W_3]$                    |
| $[(\bullet)^{2T} + \Gamma_1^-, X_2^+ + X_3^+ + X_4^+, R_1^+ + R_1^- + R_2^+, 2S_2^+ + S_2^-, T_1^+ + 2T_2^+, W_2 + 2W_4]$                    |
| $[(\bullet)^{2T} + \Gamma_1^-, X_2^+ + X_3^+ + X_4^+, R_1^+ + R_1^- + R_2^+, 2S_1^- + S_2^-, T_1^+ + 2T_2^+, W_1 + W_3 + W_4]$               |
| $[(\bullet)^{2T} + \Gamma_1^-, X_2^+ + X_3^+ + X_4^+, R_1^+ + R_1^- + R_2^+, S_1^+ + S_1^- + S_2^+, T_1^+ + 2T_2^+, W_1 + W_3 + W_4]$        |
| $[(\bullet)^{2T} + \Gamma_1^-, X_2^+ + X_3^+ + X_4^+, R_1^+ + R_1^- + R_2^+, S_1^- + S_2^+ + S_2^-, T_1^+ + T_1^- + T_2^+, W_1 + W_2 + W_4]$ |
| $[(\bullet)^{2T} + \Gamma_1^-, X_2^+ + X_3^+ + X_4^+, R_1^+ + R_1^- + R_2^+, S_1^+ + 2S_2^+, T_1^+ + T_1^- + T_2^+, W_1 + W_2 + W_4]$        |
| $[(\bullet)^{2T} + \Gamma_1^-, X_2^+ + X_3^+ + X_4^+, R_1^+ + R_1^- + R_2^+, S_1^+ + 2S_1^-, T_1^+ + T_1^- + T_2^+, 2W_1 + W_3]$             |
| $[(\bullet)^{2T} + \Gamma_1^-, X_2^+ + X_3^+ + X_4^+, R_1^+ + R_1^- + R_2^+, 2S_1^- + S_2^-, T_1^+ + 2T_1^-, 2W_1 + W_2]$                    |
| $[(\bullet)^{2T} + \Gamma_1^-, X_2^+ + X_3^+ + X_4^+, R_1^+ + R_1^- + R_2^+, S_1^+ + S_1^- + S_2^+, T_1^+ + 2T_1^-, 2W_1 + W_2]$             |
| $[(\bullet)^{2T} + \Gamma_1^-, X_2^+ + X_3^+ + X_4^+, R_1^+ + 2R_1^-, 2S_2^+ + S_2^-, 2T_2^+ + T_2^-, 3W_4]$                                 |
| $[(\bullet)^{2T} + \Gamma_1^-, X_2^+ + X_3^+ + X_4^+, R_1^+ + 2R_1^-, S_1^- + S_2^+ + S_2^-, T_1^- + T_2^+ + T_2^-, W_1 + 2W_4]$             |
| $[(\bullet)^{2T} + \Gamma_1^-, X_2^+ + X_3^+ + X_4^+, R_1^+ + 2R_1^-, S_1^+ + 2S_2^+, T_1^- + T_2^+ + T_2^-, W_1 + 2W_4]$                    |
| $[(\bullet)^{2T} + \Gamma_1^-, X_2^+ + X_3^+ + X_4^+, R_1^+ + 2R_1^-, 2S_1^- + S_2^-, 2T_1^- + T_2^-, 2W_1 + W_4]$                           |
| $[(\bullet)^{2T} + \Gamma_1^-, X_2^+ + X_3^+ + X_4^+, R_1^+ + 2R_1^-, S_1^+ + S_1^- + S_2^+, 2T_1^- + T_2^-, 2W_1 + W_4]$                    |
| $[(\bullet)^{2T} + \Gamma_1^-, X_2^+ + X_3^+ + X_4^+, R_1^+ + 2R_1^-, S_1^- + S_2^+ + S_2^-, T_1^+ + 2T_2^+, W_1 + 2W_4]$                    |
| $[(\bullet)^{2T} + \Gamma_1^-, X_2^+ + X_3^+ + X_4^+, R_1^+ + 2R_1^-, S_1^+ + 2S_2^+, T_1^+ + 2T_2^+, W_1 + 2W_4]$                           |
| $[(\bullet)^{2T} + \Gamma_1^-, X_2^+ + X_3^+ + X_4^+, R_1^+ + 2R_1^-, 2S_1^- + S_2^-, T_1^+ + T_1^- + T_2^+, 2W_1 + W_4]$                    |
| $[(\bullet)^{2T} + \Gamma_1^-, X_2^+ + X_3^+ + X_4^+, R_1^+ + 2R_1^-, S_1^+ + S_1^- + S_2^+, T_1^+ + T_1^- + T_2^+, 2W_1 + W_4]$             |
| $[(\bullet)^{2T} + \Gamma_1^-, X_2^+ + X_3^+ + X_4^+, R_1^+ + 2R_1^-, S_1^+ + 2S_1^-, T_1^+ + 2T_1^-, 3W_1]$                                 |

---

2nd minimal solution:  $\mu_2^T = 4$  (3602 symmetry vectors)

Space group 72 ( $\mathbb{Z}_1$ )

1st minimal solution:  $\mu_1^T = 4$  (18 symmetry vectors)

---

| $n^T$                                                                                                                                         |
|-----------------------------------------------------------------------------------------------------------------------------------------------|
| $[(\bullet)^{2T} + \Gamma_1^- + \Gamma_2^-, X_2^+ + X_2^- + X_3^+ + X_4^+, 2R_1, 2S_1, 3T_2^+ + T_2^-, 2W_3 + 2W_4]$                          |
| $[(\bullet)^{2T} + \Gamma_1^- + \Gamma_2^-, X_2^+ + X_2^- + X_3^+ + X_4^+, 2R_1, 2S_1, 2T_1^- + T_2^+ + T_2^-, W_1 + W_2 + W_3 + W_4]$        |
| $[(\bullet)^{2T} + \Gamma_1^+ + \Gamma_1^-, X_1^+ + X_2^+ + X_3^+ + X_4^+, 2R_1, 2S_1, 2T_2^+ + 2T_2^-, 2W_3 + 2W_4]$                         |
| $[(\bullet)^{2T} + \Gamma_1^+ + \Gamma_1^-, X_1^+ + X_2^+ + X_3^+ + X_4^+, 2R_1, 2S_1, T_1^+ + T_1^- + T_2^+ + T_2^-, W_1 + W_2 + W_3 + W_4]$ |
| $[(\bullet)^{2T} + \Gamma_1^+ + \Gamma_1^-, X_1^+ + X_2^+ + X_3^+ + X_4^+, 2R_1, 2S_1, 2T_1^- + 2T_2^-, W_1 + W_2 + W_3 + W_4]$               |
| $[(\bullet)^{2T} + \Gamma_1^+ + \Gamma_1^-, X_1^+ + X_2^+ + X_3^+ + X_4^+, 2R_1, 2S_1, 2T_2^+ + 2T_2^-, 2W_3 + 2W_4]$                         |
| $[(\bullet)^{2T} + \Gamma_1^+ + \Gamma_1^-, X_1^+ + X_2^+ + X_3^+ + X_4^+, 2R_1, 2S_1, T_1^+ + T_1^- + T_2^+ + T_2^-, W_1 + W_2 + W_3 + W_4]$ |
| $[(\bullet)^{2T} + \Gamma_1^+ + \Gamma_2^+, X_2^+ + X_2^- + X_3^- + X_4^-, 2R_1, 2S_1, T_2^+ + 3T_2^-, 2W_3 + 2W_4]$                          |
| $[(\bullet)^{2T} + \Gamma_1^+ + \Gamma_2^+, X_2^+ + X_2^- + X_3^- + X_4^-, 2R_1, 2S_1, 2T_1^+ + T_2^+ + T_2^-, W_1 + W_2 + W_3 + W_4]$        |
| $[(\bullet)^{2T} + \Gamma_1^+ + \Gamma_1^-, X_1^+ + X_2^- + X_3^- + X_4^-, 2R_1, 2S_1, 2T_1^- + 2T_2^-, W_1 + W_2 + W_3 + W_4]$               |
| $[(\bullet)^{2T} + \Gamma_1^+ + \Gamma_2^+, X_2^+ + X_2^- + X_3^- + X_4^-, 2R_1, 2S_1, T_1^+ + T_1^- + 2T_2^-, W_1 + W_2 + W_3 + W_4]$        |
| $[(\bullet)^{2T} + \Gamma_1^- + \Gamma_2^-, X_2^+ + X_2^- + X_3^+ + X_4^+, 2R_1, 2S_1, T_1^+ + T_1^- + 2T_2^+, W_1 + W_2 + W_3 + W_4]$        |
| $[(\bullet)^{2T} + \Gamma_1^+ + \Gamma_1^-, X_1^+ + X_2^- + X_3^- + X_4^-, 2R_1, 2S_1, 2T_1^+ + 2T_2^+, W_1 + W_2 + W_3 + W_4]$               |
| $[(\bullet)^{2T} + \Gamma_1^- + \Gamma_2^-, X_2^+ + X_2^- + X_3^+ + X_4^+, 2R_1, 2S_1, T_1^+ + 3T_1^-, 2W_1 + 2W_2]$                          |
| $[(\bullet)^{2T} + \Gamma_1^+ + \Gamma_1^-, X_1^+ + X_2^- + X_3^- + X_4^-, 2R_1, 2S_1, 2T_1^+ + 2T_1^-, 2W_1 + 2W_2]$                         |
| $[(\bullet)^{2T} + \Gamma_1^+ + \Gamma_1^-, X_1^+ + X_2^+ + X_3^+ + X_4^+, 2R_1, 2S_1, 2T_1^+ + 2T_1^-, 2W_1 + 2W_2]$                         |
| $[(\bullet)^{2T} + \Gamma_1^+ + \Gamma_2^+, X_2^+ + X_2^- + X_3^- + X_4^-, 2R_1, 2S_1, 3T_1^+ + T_1^-, 2W_1 + 2W_2]$                          |
| $[(\bullet)^{2T} + \Gamma_1^+ + \Gamma_1^-, X_1^+ + X_2^+ + X_3^+ + X_4^+, 2R_1, 2S_1, 2T_1^+ + 2T_2^+, W_1 + W_2 + W_3 + W_4]$               |

---

2nd minimal solution:  $\mu_2^T = 6$  (216 symmetry vectors)

Space group 73 ( $\mathbb{Z}_2$ )

1st minimal solution:  $\mu_1^T = 2$  (1 symmetry vector & filling-enforced topology)

| $\mathbf{n}^T$                                             | $\mathbf{v}^T \in \mathbb{Z}_2$ |
|------------------------------------------------------------|---------------------------------|
| $[(\blacksquare)^{2T}, X_4^+ + X_4^-, R_1, S_1, T_1, W_1]$ | 1                               |

2nd minimal solution:  $\mu_2^T = 4$  (2 symmetry vectors)

Space group 74 ( $\mathbb{Z}_1$ )

1st minimal solution:  $\mu_1^T = 2$  (4 symmetry vectors)

| $\mathbf{n}^T$                                                                 |
|--------------------------------------------------------------------------------|
| $[(\blacksquare)^{2T}, X_4^+ + X_4^-, R_1^+ + R_2^-, S_1^- + S_2^-, T_1, W_1]$ |
| $[(\blacksquare)^{2T}, X_4^+ + X_4^-, R_1^+ + R_2^-, S_1^+ + S_2^+, T_1, W_1]$ |
| $[(\blacksquare)^{2T}, X_4^+ + X_4^-, R_1^- + R_2^-, S_1^- + S_2^-, T_1, W_1]$ |
| $[(\blacksquare)^{2T}, X_4^+ + X_4^-, R_1^- + R_2^-, S_1^+ + S_2^+, T_1, W_1]$ |

2nd minimal solution:  $\mu_2^T = 4$  (82 symmetry vectors)

Space group 75 ( $\mathbb{Z}_4$ )

1st minimal solution:  $\mu_1^T = 2$  (30 symmetry vectors)

| $\mathbf{n}^T$                                                                 | $\mathbf{v}^T \in \mathbb{Z}_4$ |
|--------------------------------------------------------------------------------|---------------------------------|
| $[(\blacksquare)^{2T}, 2A_4, 2M_4, Z_3 + Z_4, 2R_2, 2X_2]$                     | 2                               |
| $[(\blacksquare)^{2T}, 2A_4, 2M_4, Z_3 + Z_4, R_1 + R_2, X_1 + X_2]$           | trivial                         |
| $[(\blacksquare)^{2T}, A_3 + A_4, M_3 + M_4, Z_3 + Z_4, 2R_2, 2X_2]$           | trivial                         |
| $[(\blacksquare)^{2T}, A_3 + A_4, M_3 + M_4, Z_3 + Z_4, R_1 + R_2, X_1 + X_2]$ | 2                               |
| $[(\blacksquare)^{2T}, A_2 + A_4, M_2 + M_4, Z_3 + Z_4, 2R_2, 2X_2]$           | 1                               |
| $[(\blacksquare)^{2T}, A_2 + A_4, M_2 + M_4, Z_3 + Z_4, R_1 + R_2, X_1 + X_2]$ | 3                               |
| $[(\blacksquare)^{2T}, A_1 + A_4, M_1 + M_4, Z_3 + Z_4, 2R_2, 2X_2]$           | 3                               |
| $[(\blacksquare)^{2T}, A_1 + A_4, M_1 + M_4, Z_3 + Z_4, R_1 + R_2, X_1 + X_2]$ | 1                               |
| $[(\blacksquare)^{2T}, 2A_4, 2M_4, Z_3 + Z_4, 2R_1, 2X_1]$                     | 2                               |
| $[(\blacksquare)^{2T}, A_3 + A_4, M_3 + M_4, Z_3 + Z_4, 2R_1, 2X_1]$           | trivial                         |
| $[(\blacksquare)^{2T}, A_2 + A_4, M_2 + M_4, Z_3 + Z_4, 2R_1, 2X_1]$           | 1                               |
| $[(\blacksquare)^{2T}, A_1 + A_4, M_1 + M_4, Z_3 + Z_4, 2R_1, 2X_1]$           | 3                               |
| $[(\blacksquare)^{2T}, 2A_3, 2M_3, Z_3 + Z_4, 2R_2, 2X_2]$                     | 2                               |
| $[(\blacksquare)^{2T}, 2A_3, 2M_3, Z_3 + Z_4, R_1 + R_2, X_1 + X_2]$           | trivial                         |
| $[(\blacksquare)^{2T}, A_2 + A_3, M_2 + M_3, Z_3 + Z_4, 2R_2, 2X_2]$           | 3                               |
| $[(\blacksquare)^{2T}, A_2 + A_3, M_2 + M_3, Z_3 + Z_4, R_1 + R_2, X_1 + X_2]$ | 1                               |
| $[(\blacksquare)^{2T}, A_1 + A_3, M_1 + M_3, Z_3 + Z_4, 2R_2, 2X_2]$           | 1                               |
| $[(\blacksquare)^{2T}, A_1 + A_3, M_1 + M_3, Z_3 + Z_4, R_1 + R_2, X_1 + X_2]$ | 3                               |
| $[(\blacksquare)^{2T}, 2A_3, 2M_3, Z_3 + Z_4, 2R_1, 2X_1]$                     | 2                               |
| $[(\blacksquare)^{2T}, A_2 + A_3, M_2 + M_3, Z_3 + Z_4, 2R_1, 2X_1]$           | 3                               |

... continued on next page

... continued from previous page

|                                                                                |         |
|--------------------------------------------------------------------------------|---------|
| $[(\blacksquare)^{2T}, A_1 + A_3, M_1 + M_3, Z_3 + Z_4, 2R_1, 2X_1]$           | 1       |
| $[(\blacksquare)^{2T}, 2A_2, 2M_2, Z_3 + Z_4, 2R_2, 2X_2]$                     | trivial |
| $[(\blacksquare)^{2T}, 2A_2, 2M_2, Z_3 + Z_4, R_1 + R_2, X_1 + X_2]$           | 2       |
| $[(\blacksquare)^{2T}, A_1 + A_2, M_1 + M_2, Z_3 + Z_4, 2R_2, 2X_2]$           | 2       |
| $[(\blacksquare)^{2T}, A_1 + A_2, M_1 + M_2, Z_3 + Z_4, R_1 + R_2, X_1 + X_2]$ | trivial |
| $[(\blacksquare)^{2T}, 2A_2, 2M_2, Z_3 + Z_4, 2R_1, 2X_1]$                     | trivial |
| $[(\blacksquare)^{2T}, A_1 + A_2, M_1 + M_2, Z_3 + Z_4, 2R_1, 2X_1]$           | 2       |
| $[(\blacksquare)^{2T}, 2A_1, 2M_1, Z_3 + Z_4, 2R_2, 2X_2]$                     | trivial |
| $[(\blacksquare)^{2T}, 2A_1, 2M_1, Z_3 + Z_4, R_1 + R_2, X_1 + X_2]$           | 2       |
| $[(\blacksquare)^{2T}, 2A_1, 2M_1, Z_3 + Z_4, 2R_1, 2X_1]$                     | trivial |

2nd minimal solution:  $\mu_2^T = 3$  (320 symmetry vectors)

Space group 76 ( $\mathbb{Z}_1$ )

1st minimal solution:  $\mu_1^T = 4$  (1 symmetry vector)

| $\mathbf{n}^T$                                                                                                                               |
|----------------------------------------------------------------------------------------------------------------------------------------------|
| $[(\blacksquare)^{2T} + \Gamma_1 + \Gamma_2, A_1 + A_2 + A_3 + A_4, M_1 + M_2 + M_3 + M_4, Z_1 + Z_2 + Z_3 + Z_4, 2R_1 + 2R_2, 2X_1 + 2X_2]$ |

2nd minimal solution:  $\mu_2^T = 8$  (1 symmetry vector)

Space group 77 ( $\mathbb{Z}_2$ )

1st minimal solution:  $\mu_1^T = 2$  (6 symmetry vectors)

| $\mathbf{n}^T$                                                                 | $\mathbf{v}^T \in \mathbb{Z}_2$ |
|--------------------------------------------------------------------------------|---------------------------------|
| $[(\blacksquare)^{2T}, A_3 + A_4, M_3 + M_4, Z_3 + Z_4, 2R_2, 2X_2]$           | trivial                         |
| $[(\blacksquare)^{2T}, A_3 + A_4, M_3 + M_4, Z_3 + Z_4, R_1 + R_2, X_1 + X_2]$ | 1                               |
| $[(\blacksquare)^{2T}, A_3 + A_4, M_3 + M_4, Z_3 + Z_4, 2R_1, 2X_1]$           | trivial                         |
| $[(\blacksquare)^{2T}, A_1 + A_2, M_1 + M_2, Z_3 + Z_4, 2R_2, 2X_2]$           | 1                               |
| $[(\blacksquare)^{2T}, A_1 + A_2, M_1 + M_2, Z_3 + Z_4, R_1 + R_2, X_1 + X_2]$ | trivial                         |
| $[(\blacksquare)^{2T}, A_1 + A_2, M_1 + M_2, Z_3 + Z_4, 2R_1, 2X_1]$           | 1                               |

2nd minimal solution:  $\mu_2^T = 4$  (30 symmetry vectors)

Space group 78 ( $\mathbb{Z}_1$ )

1st minimal solution:  $\mu_1^T = 4$  (1 symmetry vector)

| $\mathbf{n}^T$                                                                                                                               |
|----------------------------------------------------------------------------------------------------------------------------------------------|
| $[(\blacksquare)^{2T} + \Gamma_1 + \Gamma_2, A_1 + A_2 + A_3 + A_4, M_1 + M_2 + M_3 + M_4, Z_1 + Z_2 + Z_3 + Z_4, 2R_1 + 2R_2, 2X_1 + 2X_2]$ |

2nd minimal solution:  $\mu_2^T = 8$  (1 symmetry vector)



Space group 79 ( $\mathbb{Z}_2$ )

1st minimal solution:  $\mu_1^T = 2$  (3 symmetry vectors)

| $\mathbf{n}^T$                                                 | $\mathbf{v}^T \in \mathbb{Z}_2$ |
|----------------------------------------------------------------|---------------------------------|
| $[(\blacksquare)^{2T}, M_3 + M_4, 2P_2, 2X_2, 2N_1]$           | trivial                         |
| $[(\blacksquare)^{2T}, M_3 + M_4, P_1 + P_2, X_1 + X_2, 2N_1]$ | 1                               |
| $[(\blacksquare)^{2T}, M_3 + M_4, 2P_1, 2X_1, 2N_1]$           | trivial                         |

2nd minimal solution:  $\mu_2^T = 3$  (16 symmetry vectors)

Space group 80 ( $\mathbb{Z}_1$ )

1st minimal solution:  $\mu_1^T = 2$  (1 symmetry vector)

| $\mathbf{n}^T$                                                 |
|----------------------------------------------------------------|
| $[(\blacksquare)^{2T}, M_3 + M_4, P_1 + P_2, X_1 + X_2, 2N_1]$ |

2nd minimal solution:  $\mu_2^T = 4$  (2 symmetry vectors)

Space group 81 ( $\mathbb{Z}_2 \times \mathbb{Z}_2 \times \mathbb{Z}_4$ )

1st minimal solution:  $\mu_1^T = 2$  (306 symmetry vectors)

| $\mathbf{n}^T$                                                                 | $\mathbf{v}^T \in \mathbb{Z}_2 \times \mathbb{Z}_2 \times \mathbb{Z}_4$ |
|--------------------------------------------------------------------------------|-------------------------------------------------------------------------|
| $[(\blacksquare)^{2T}, 2A_4, 2M_4, 2Z_3, 2R_2, 2X_2]$                          | (1, 1, 0)                                                               |
| $[(\blacksquare)^{2T}, 2A_4, 2M_4, Z_3 + Z_4, 2R_2, 2X_2]$                     | (0, 1, 0)                                                               |
| $[(\blacksquare)^{2T}, 2A_4, 2M_4, 2Z_3, R_1 + R_2, X_1 + X_2]$                | (1, 1, 2)                                                               |
| $[(\blacksquare)^{2T}, 2A_4, 2M_4, Z_3 + Z_4, R_1 + R_2, X_1 + X_2]$           | (0, 1, 2)                                                               |
| $[(\blacksquare)^{2T}, 2A_4, M_3 + M_4, 2Z_3, 2R_2, 2X_2]$                     | (0, 1, 2)                                                               |
| $[(\blacksquare)^{2T}, 2A_4, M_3 + M_4, Z_3 + Z_4, 2R_2, 2X_2]$                | (1, 1, 2)                                                               |
| $[(\blacksquare)^{2T}, 2A_4, M_3 + M_4, 2Z_3, R_1 + R_2, X_1 + X_2]$           | (0, 1, 0)                                                               |
| $[(\blacksquare)^{2T}, 2A_4, M_3 + M_4, Z_3 + Z_4, R_1 + R_2, X_1 + X_2]$      | (1, 1, 0)                                                               |
| $[(\blacksquare)^{2T}, A_3 + A_4, 2M_4, 2Z_3, 2R_2, 2X_2]$                     | (0, 1, 0)                                                               |
| $[(\blacksquare)^{2T}, A_3 + A_4, 2M_4, Z_3 + Z_4, 2R_2, 2X_2]$                | (1, 1, 0)                                                               |
| $[(\blacksquare)^{2T}, A_3 + A_4, 2M_4, 2Z_3, R_1 + R_2, X_1 + X_2]$           | (0, 1, 2)                                                               |
| $[(\blacksquare)^{2T}, A_3 + A_4, 2M_4, Z_3 + Z_4, R_1 + R_2, X_1 + X_2]$      | (1, 1, 2)                                                               |
| $[(\blacksquare)^{2T}, A_3 + A_4, M_3 + M_4, 2Z_3, 2R_2, 2X_2]$                | (1, 1, 2)                                                               |
| $[(\blacksquare)^{2T}, A_3 + A_4, M_3 + M_4, Z_3 + Z_4, 2R_2, 2X_2]$           | (0, 1, 2)                                                               |
| $[(\blacksquare)^{2T}, A_3 + A_4, M_3 + M_4, 2Z_3, R_1 + R_2, X_1 + X_2]$      | (1, 1, 0)                                                               |
| $[(\blacksquare)^{2T}, A_3 + A_4, M_3 + M_4, Z_3 + Z_4, R_1 + R_2, X_1 + X_2]$ | (0, 1, 0)                                                               |
| $[(\blacksquare)^{2T}, A_2 + A_4, M_2 + M_4, 2Z_3, 2R_2, 2X_2]$                | (0, 1, 1)                                                               |
| $[(\blacksquare)^{2T}, A_2 + A_4, M_2 + M_4, Z_3 + Z_4, 2R_2, 2X_2]$           | (1, 1, 1)                                                               |
| $[(\blacksquare)^{2T}, A_2 + A_4, M_2 + M_4, 2Z_3, R_1 + R_2, X_1 + X_2]$      | (0, 1, 3)                                                               |
| $[(\blacksquare)^{2T}, A_2 + A_4, M_2 + M_4, Z_3 + Z_4, R_1 + R_2, X_1 + X_2]$ | (1, 1, 3)                                                               |

... continued on next page

... continued from previous page

|                                                                                |           |
|--------------------------------------------------------------------------------|-----------|
| $[(\blacksquare)^{2T}, A_2 + A_4, M_1 + M_4, 2Z_3, 2R_2, 2X_2]$                | (0, 0, 3) |
| $[(\blacksquare)^{2T}, A_2 + A_4, M_1 + M_4, Z_3 + Z_4, 2R_2, 2X_2]$           | (1, 0, 3) |
| $[(\blacksquare)^{2T}, A_2 + A_4, M_1 + M_4, 2Z_3, R_1 + R_2, X_1 + X_2]$      | (0, 0, 1) |
| $[(\blacksquare)^{2T}, A_2 + A_4, M_1 + M_4, Z_3 + Z_4, R_1 + R_2, X_1 + X_2]$ | (1, 0, 1) |
| $[(\blacksquare)^{2T}, A_1 + A_4, M_2 + M_4, 2Z_3, 2R_2, 2X_2]$                | (0, 0, 1) |
| $[(\blacksquare)^{2T}, A_1 + A_4, M_2 + M_4, Z_3 + Z_4, 2R_2, 2X_2]$           | (1, 0, 1) |
| $[(\blacksquare)^{2T}, A_1 + A_4, M_2 + M_4, 2Z_3, R_1 + R_2, X_1 + X_2]$      | (0, 0, 3) |
| $[(\blacksquare)^{2T}, A_1 + A_4, M_2 + M_4, Z_3 + Z_4, R_1 + R_2, X_1 + X_2]$ | (1, 0, 3) |
| $[(\blacksquare)^{2T}, A_1 + A_4, M_1 + M_4, 2Z_3, 2R_2, 2X_2]$                | (0, 1, 3) |
| $[(\blacksquare)^{2T}, A_1 + A_4, M_1 + M_4, Z_3 + Z_4, 2R_2, 2X_2]$           | (1, 1, 3) |
| $[(\blacksquare)^{2T}, A_1 + A_4, M_1 + M_4, 2Z_3, R_1 + R_2, X_1 + X_2]$      | (0, 1, 1) |
| $[(\blacksquare)^{2T}, A_1 + A_4, M_1 + M_4, Z_3 + Z_4, R_1 + R_2, X_1 + X_2]$ | (1, 1, 1) |
| $[(\blacksquare)^{2T}, 2A_4, 2M_4, 2Z_3, 2R_1, 2X_1]$                          | (1, 1, 0) |
| $[(\blacksquare)^{2T}, 2A_4, 2M_4, Z_3 + Z_4, 2R_1, 2X_1]$                     | (0, 1, 0) |
| $[(\blacksquare)^{2T}, 2A_4, M_3 + M_4, 2Z_3, 2R_1, 2X_1]$                     | (0, 1, 2) |
| $[(\blacksquare)^{2T}, 2A_4, M_3 + M_4, Z_3 + Z_4, 2R_1, 2X_1]$                | (1, 1, 2) |
| $[(\blacksquare)^{2T}, A_3 + A_4, 2M_4, 2Z_3, 2R_1, 2X_1]$                     | (0, 1, 0) |
| $[(\blacksquare)^{2T}, A_3 + A_4, 2M_4, Z_3 + Z_4, 2R_1, 2X_1]$                | (1, 1, 0) |
| $[(\blacksquare)^{2T}, A_3 + A_4, M_3 + M_4, 2Z_3, 2R_1, 2X_1]$                | (1, 1, 2) |
| $[(\blacksquare)^{2T}, A_3 + A_4, M_3 + M_4, Z_3 + Z_4, 2R_1, 2X_1]$           | (0, 1, 2) |
| $[(\blacksquare)^{2T}, A_2 + A_4, M_2 + M_4, 2Z_3, 2R_1, 2X_1]$                | (0, 1, 1) |
| $[(\blacksquare)^{2T}, A_2 + A_4, M_2 + M_4, Z_3 + Z_4, 2R_1, 2X_1]$           | (1, 1, 1) |
| $[(\blacksquare)^{2T}, A_2 + A_4, M_1 + M_4, 2Z_3, 2R_1, 2X_1]$                | (0, 0, 3) |
| $[(\blacksquare)^{2T}, A_2 + A_4, M_1 + M_4, Z_3 + Z_4, 2R_1, 2X_1]$           | (1, 0, 3) |
| $[(\blacksquare)^{2T}, A_1 + A_4, M_2 + M_4, 2Z_3, 2R_1, 2X_1]$                | (0, 0, 1) |
| $[(\blacksquare)^{2T}, A_1 + A_4, M_2 + M_4, Z_3 + Z_4, 2R_1, 2X_1]$           | (1, 0, 1) |
| $[(\blacksquare)^{2T}, A_1 + A_4, M_1 + M_4, 2Z_3, 2R_1, 2X_1]$                | (0, 1, 3) |
| $[(\blacksquare)^{2T}, A_1 + A_4, M_1 + M_4, Z_3 + Z_4, 2R_1, 2X_1]$           | (1, 1, 3) |
| $[(\blacksquare)^{2T}, 2A_4, 2M_3, 2Z_3, 2R_2, 2X_2]$                          | (1, 1, 0) |
| $[(\blacksquare)^{2T}, 2A_4, 2M_3, Z_3 + Z_4, 2R_2, 2X_2]$                     | (0, 1, 0) |
| $[(\blacksquare)^{2T}, 2A_4, 2M_3, 2Z_3, R_1 + R_2, X_1 + X_2]$                | (1, 1, 2) |
| $[(\blacksquare)^{2T}, 2A_4, 2M_3, Z_3 + Z_4, R_1 + R_2, X_1 + X_2]$           | (0, 1, 2) |
| $[(\blacksquare)^{2T}, A_3 + A_4, 2M_3, 2Z_3, 2R_2, 2X_2]$                     | (0, 1, 0) |
| $[(\blacksquare)^{2T}, A_3 + A_4, 2M_3, Z_3 + Z_4, 2R_2, 2X_2]$                | (1, 1, 0) |
| $[(\blacksquare)^{2T}, A_3 + A_4, 2M_3, 2Z_3, R_1 + R_2, X_1 + X_2]$           | (0, 1, 2) |
| $[(\blacksquare)^{2T}, A_3 + A_4, 2M_3, Z_3 + Z_4, R_1 + R_2, X_1 + X_2]$      | (1, 1, 2) |
| $[(\blacksquare)^{2T}, A_2 + A_4, M_2 + M_3, 2Z_3, 2R_2, 2X_2]$                | (1, 1, 3) |
| $[(\blacksquare)^{2T}, A_2 + A_4, M_2 + M_3, Z_3 + Z_4, 2R_2, 2X_2]$           | (0, 1, 3) |
| $[(\blacksquare)^{2T}, A_2 + A_4, M_2 + M_3, 2Z_3, R_1 + R_2, X_1 + X_2]$      | (1, 1, 1) |
| $[(\blacksquare)^{2T}, A_2 + A_4, M_2 + M_3, Z_3 + Z_4, R_1 + R_2, X_1 + X_2]$ | (0, 1, 1) |
| $[(\blacksquare)^{2T}, A_2 + A_4, M_1 + M_3, 2Z_3, 2R_2, 2X_2]$                | (1, 0, 1) |
| $[(\blacksquare)^{2T}, A_2 + A_4, M_1 + M_3, Z_3 + Z_4, 2R_2, 2X_2]$           | (0, 0, 1) |
| $[(\blacksquare)^{2T}, A_2 + A_4, M_1 + M_3, 2Z_3, R_1 + R_2, X_1 + X_2]$      | (1, 0, 3) |
| $[(\blacksquare)^{2T}, A_2 + A_4, M_1 + M_3, Z_3 + Z_4, R_1 + R_2, X_1 + X_2]$ | (0, 0, 3) |
| $[(\blacksquare)^{2T}, A_1 + A_4, M_2 + M_3, 2Z_3, 2R_2, 2X_2]$                | (1, 0, 3) |
| $[(\blacksquare)^{2T}, A_1 + A_4, M_2 + M_3, Z_3 + Z_4, 2R_2, 2X_2]$           | (0, 0, 3) |
| $[(\blacksquare)^{2T}, A_1 + A_4, M_2 + M_3, 2Z_3, R_1 + R_2, X_1 + X_2]$      | (1, 0, 1) |
| $[(\blacksquare)^{2T}, A_1 + A_4, M_2 + M_3, Z_3 + Z_4, R_1 + R_2, X_1 + X_2]$ | (0, 0, 1) |
| $[(\blacksquare)^{2T}, A_1 + A_4, M_1 + M_3, 2Z_3, 2R_2, 2X_2]$                | (1, 1, 1) |
| $[(\blacksquare)^{2T}, A_1 + A_4, M_1 + M_3, Z_3 + Z_4, 2R_2, 2X_2]$           | (0, 1, 1) |
| $[(\blacksquare)^{2T}, A_1 + A_4, M_1 + M_3, 2Z_3, R_1 + R_2, X_1 + X_2]$      | (1, 1, 3) |
| $[(\blacksquare)^{2T}, A_1 + A_4, M_1 + M_3, Z_3 + Z_4, R_1 + R_2, X_1 + X_2]$ | (0, 1, 3) |
| $[(\blacksquare)^{2T}, 2A_4, 2M_3, 2Z_3, 2R_1, 2X_1]$                          | (1, 1, 0) |
| $[(\blacksquare)^{2T}, 2A_4, 2M_3, Z_3 + Z_4, 2R_1, 2X_1]$                     | (0, 1, 0) |

... continued on next page

... continued from previous page

|                                                                           |           |
|---------------------------------------------------------------------------|-----------|
| $[(\bullet)^{2T}, A_3 + A_4, 2M_3, 2Z_3, 2R_1, 2X_1]$                     | (0, 1, 0) |
| $[(\bullet)^{2T}, A_3 + A_4, 2M_3, Z_3 + Z_4, 2R_1, 2X_1]$                | (1, 1, 0) |
| $[(\bullet)^{2T}, A_2 + A_4, M_2 + M_3, 2Z_3, 2R_1, 2X_1]$                | (1, 1, 3) |
| $[(\bullet)^{2T}, A_2 + A_4, M_2 + M_3, Z_3 + Z_4, 2R_1, 2X_1]$           | (0, 1, 3) |
| $[(\bullet)^{2T}, A_2 + A_4, M_1 + M_3, 2Z_3, 2R_1, 2X_1]$                | (1, 0, 1) |
| $[(\bullet)^{2T}, A_2 + A_4, M_1 + M_3, Z_3 + Z_4, 2R_1, 2X_1]$           | (0, 0, 1) |
| $[(\bullet)^{2T}, A_1 + A_4, M_2 + M_3, 2Z_3, 2R_1, 2X_1]$                | (1, 0, 3) |
| $[(\bullet)^{2T}, A_1 + A_4, M_2 + M_3, Z_3 + Z_4, 2R_1, 2X_1]$           | (0, 0, 3) |
| $[(\bullet)^{2T}, A_1 + A_4, M_1 + M_3, 2Z_3, 2R_1, 2X_1]$                | (1, 1, 1) |
| $[(\bullet)^{2T}, A_1 + A_4, M_1 + M_3, Z_3 + Z_4, 2R_1, 2X_1]$           | (0, 1, 1) |
| $[(\bullet)^{2T}, 2A_3, 2M_4, 2Z_3, 2R_2, 2X_2]$                          | (1, 1, 0) |
| $[(\bullet)^{2T}, 2A_3, 2M_4, Z_3 + Z_4, 2R_2, 2X_2]$                     | (0, 1, 0) |
| $[(\bullet)^{2T}, 2A_3, 2M_4, 2Z_3, R_1 + R_2, X_1 + X_2]$                | (1, 1, 2) |
| $[(\bullet)^{2T}, 2A_3, 2M_4, Z_3 + Z_4, R_1 + R_2, X_1 + X_2]$           | (0, 1, 2) |
| $[(\bullet)^{2T}, 2A_3, M_3 + M_4, 2Z_3, 2R_2, 2X_2]$                     | (0, 1, 2) |
| $[(\bullet)^{2T}, 2A_3, M_3 + M_4, Z_3 + Z_4, 2R_2, 2X_2]$                | (1, 1, 2) |
| $[(\bullet)^{2T}, 2A_3, M_3 + M_4, 2Z_3, R_1 + R_2, X_1 + X_2]$           | (0, 1, 0) |
| $[(\bullet)^{2T}, 2A_3, M_3 + M_4, Z_3 + Z_4, R_1 + R_2, X_1 + X_2]$      | (1, 1, 0) |
| $[(\bullet)^{2T}, A_2 + A_3, M_2 + M_4, 2Z_3, 2R_2, 2X_2]$                | (1, 1, 1) |
| $[(\bullet)^{2T}, A_2 + A_3, M_2 + M_4, Z_3 + Z_4, 2R_2, 2X_2]$           | (0, 1, 1) |
| $[(\bullet)^{2T}, A_2 + A_3, M_2 + M_4, 2Z_3, R_1 + R_2, X_1 + X_2]$      | (1, 1, 3) |
| $[(\bullet)^{2T}, A_2 + A_3, M_2 + M_4, Z_3 + Z_4, R_1 + R_2, X_1 + X_2]$ | (0, 1, 3) |
| $[(\bullet)^{2T}, A_2 + A_3, M_1 + M_4, 2Z_3, 2R_2, 2X_2]$                | (1, 0, 3) |
| $[(\bullet)^{2T}, A_2 + A_3, M_1 + M_4, Z_3 + Z_4, 2R_2, 2X_2]$           | (0, 0, 3) |
| $[(\bullet)^{2T}, A_2 + A_3, M_1 + M_4, 2Z_3, R_1 + R_2, X_1 + X_2]$      | (1, 0, 1) |
| $[(\bullet)^{2T}, A_2 + A_3, M_1 + M_4, Z_3 + Z_4, R_1 + R_2, X_1 + X_2]$ | (0, 0, 1) |
| $[(\bullet)^{2T}, A_1 + A_3, M_2 + M_4, 2Z_3, 2R_2, 2X_2]$                | (1, 0, 1) |
| $[(\bullet)^{2T}, A_1 + A_3, M_2 + M_4, Z_3 + Z_4, 2R_2, 2X_2]$           | (0, 0, 1) |
| $[(\bullet)^{2T}, A_1 + A_3, M_2 + M_4, 2Z_3, R_1 + R_2, X_1 + X_2]$      | (1, 0, 3) |
| $[(\bullet)^{2T}, A_1 + A_3, M_2 + M_4, Z_3 + Z_4, R_1 + R_2, X_1 + X_2]$ | (0, 0, 3) |
| $[(\bullet)^{2T}, A_1 + A_3, M_1 + M_4, 2Z_3, 2R_2, 2X_2]$                | (1, 1, 3) |
| $[(\bullet)^{2T}, A_1 + A_3, M_1 + M_4, Z_3 + Z_4, 2R_2, 2X_2]$           | (0, 1, 3) |
| $[(\bullet)^{2T}, A_1 + A_3, M_1 + M_4, 2Z_3, R_1 + R_2, X_1 + X_2]$      | (1, 1, 1) |
| $[(\bullet)^{2T}, A_1 + A_3, M_1 + M_4, Z_3 + Z_4, R_1 + R_2, X_1 + X_2]$ | (0, 1, 1) |
| $[(\bullet)^{2T}, 2A_3, 2M_4, 2Z_3, 2R_1, 2X_1]$                          | (1, 1, 0) |
| $[(\bullet)^{2T}, 2A_3, 2M_4, Z_3 + Z_4, 2R_1, 2X_1]$                     | (0, 1, 0) |
| $[(\bullet)^{2T}, 2A_3, M_3 + M_4, 2Z_3, 2R_1, 2X_1]$                     | (0, 1, 2) |
| $[(\bullet)^{2T}, 2A_3, M_3 + M_4, Z_3 + Z_4, 2R_1, 2X_1]$                | (1, 1, 2) |
| $[(\bullet)^{2T}, A_2 + A_3, M_2 + M_4, 2Z_3, 2R_1, 2X_1]$                | (1, 1, 1) |
| $[(\bullet)^{2T}, A_2 + A_3, M_2 + M_4, Z_3 + Z_4, 2R_1, 2X_1]$           | (0, 1, 1) |
| $[(\bullet)^{2T}, A_2 + A_3, M_1 + M_4, 2Z_3, 2R_1, 2X_1]$                | (1, 0, 3) |
| $[(\bullet)^{2T}, A_2 + A_3, M_1 + M_4, Z_3 + Z_4, 2R_1, 2X_1]$           | (0, 0, 3) |
| $[(\bullet)^{2T}, A_1 + A_3, M_2 + M_4, 2Z_3, 2R_1, 2X_1]$                | (1, 0, 1) |
| $[(\bullet)^{2T}, A_1 + A_3, M_2 + M_4, Z_3 + Z_4, 2R_1, 2X_1]$           | (0, 0, 1) |
| $[(\bullet)^{2T}, A_1 + A_3, M_1 + M_4, 2Z_3, 2R_1, 2X_1]$                | (1, 1, 3) |
| $[(\bullet)^{2T}, A_1 + A_3, M_1 + M_4, Z_3 + Z_4, 2R_1, 2X_1]$           | (0, 1, 3) |
| $[(\bullet)^{2T}, 2A_3, 2M_3, 2Z_3, 2R_2, 2X_2]$                          | (1, 1, 0) |
| $[(\bullet)^{2T}, 2A_3, 2M_3, Z_3 + Z_4, 2R_2, 2X_2]$                     | (0, 1, 0) |
| $[(\bullet)^{2T}, 2A_3, 2M_3, 2Z_3, R_1 + R_2, X_1 + X_2]$                | (1, 1, 2) |
| $[(\bullet)^{2T}, 2A_3, 2M_3, Z_3 + Z_4, R_1 + R_2, X_1 + X_2]$           | (0, 1, 2) |
| $[(\bullet)^{2T}, A_2 + A_3, M_2 + M_3, 2Z_3, 2R_2, 2X_2]$                | (0, 1, 3) |
| $[(\bullet)^{2T}, A_2 + A_3, M_2 + M_3, Z_3 + Z_4, 2R_2, 2X_2]$           | (1, 1, 3) |
| $[(\bullet)^{2T}, A_2 + A_3, M_2 + M_3, 2Z_3, R_1 + R_2, X_1 + X_2]$      | (0, 1, 1) |
| $[(\bullet)^{2T}, A_2 + A_3, M_2 + M_3, Z_3 + Z_4, R_1 + R_2, X_1 + X_2]$ | (1, 1, 1) |

... continued on next page

... continued from previous page

|                                                                           |           |
|---------------------------------------------------------------------------|-----------|
| $[(\bullet)^{2T}, A_2 + A_3, M_1 + M_3, 2Z_3, 2R_2, 2X_2]$                | (0, 0, 1) |
| $[(\bullet)^{2T}, A_2 + A_3, M_1 + M_3, Z_3 + Z_4, 2R_2, 2X_2]$           | (1, 0, 1) |
| $[(\bullet)^{2T}, A_2 + A_3, M_1 + M_3, 2Z_3, R_1 + R_2, X_1 + X_2]$      | (0, 0, 3) |
| $[(\bullet)^{2T}, A_2 + A_3, M_1 + M_3, Z_3 + Z_4, R_1 + R_2, X_1 + X_2]$ | (1, 0, 3) |
| $[(\bullet)^{2T}, A_1 + A_3, M_2 + M_3, 2Z_3, 2R_2, 2X_2]$                | (0, 0, 3) |
| $[(\bullet)^{2T}, A_1 + A_3, M_2 + M_3, Z_3 + Z_4, 2R_2, 2X_2]$           | (1, 0, 3) |
| $[(\bullet)^{2T}, A_1 + A_3, M_2 + M_3, 2Z_3, R_1 + R_2, X_1 + X_2]$      | (0, 0, 1) |
| $[(\bullet)^{2T}, A_1 + A_3, M_2 + M_3, Z_3 + Z_4, R_1 + R_2, X_1 + X_2]$ | (1, 0, 1) |
| $[(\bullet)^{2T}, A_1 + A_3, M_1 + M_3, 2Z_3, 2R_2, 2X_2]$                | (0, 1, 1) |
| $[(\bullet)^{2T}, A_1 + A_3, M_1 + M_3, Z_3 + Z_4, 2R_2, 2X_2]$           | (1, 1, 1) |
| $[(\bullet)^{2T}, A_1 + A_3, M_1 + M_3, 2Z_3, R_1 + R_2, X_1 + X_2]$      | (0, 1, 3) |
| $[(\bullet)^{2T}, A_1 + A_3, M_1 + M_3, Z_3 + Z_4, R_1 + R_2, X_1 + X_2]$ | (1, 1, 3) |
| $[(\bullet)^{2T}, 2A_3, 2M_3, 2Z_3, 2R_1, 2X_1]$                          | (1, 1, 0) |
| $[(\bullet)^{2T}, 2A_3, 2M_3, Z_3 + Z_4, 2R_1, 2X_1]$                     | (0, 1, 0) |
| $[(\bullet)^{2T}, A_2 + A_3, M_2 + M_3, 2Z_3, 2R_1, 2X_1]$                | (0, 1, 3) |
| $[(\bullet)^{2T}, A_2 + A_3, M_2 + M_3, Z_3 + Z_4, 2R_1, 2X_1]$           | (1, 1, 3) |
| $[(\bullet)^{2T}, A_2 + A_3, M_1 + M_3, 2Z_3, 2R_1, 2X_1]$                | (0, 0, 1) |
| $[(\bullet)^{2T}, A_2 + A_3, M_1 + M_3, Z_3 + Z_4, 2R_1, 2X_1]$           | (1, 0, 1) |
| $[(\bullet)^{2T}, A_1 + A_3, M_2 + M_3, 2Z_3, 2R_1, 2X_1]$                | (0, 0, 3) |
| $[(\bullet)^{2T}, A_1 + A_3, M_2 + M_3, Z_3 + Z_4, 2R_1, 2X_1]$           | (1, 0, 3) |
| $[(\bullet)^{2T}, A_1 + A_3, M_1 + M_3, 2Z_3, 2R_1, 2X_1]$                | (0, 1, 1) |
| $[(\bullet)^{2T}, A_1 + A_3, M_1 + M_3, Z_3 + Z_4, 2R_1, 2X_1]$           | (1, 1, 1) |
| $[(\bullet)^{2T}, 2A_2, 2M_2, 2Z_3, 2R_2, 2X_2]$                          | (1, 1, 2) |
| $[(\bullet)^{2T}, 2A_2, 2M_2, Z_3 + Z_4, 2R_2, 2X_2]$                     | (0, 1, 2) |
| $[(\bullet)^{2T}, 2A_2, 2M_2, 2Z_3, R_1 + R_2, X_1 + X_2]$                | (1, 1, 0) |
| $[(\bullet)^{2T}, 2A_2, 2M_2, Z_3 + Z_4, R_1 + R_2, X_1 + X_2]$           | (0, 1, 0) |
| $[(\bullet)^{2T}, 2A_2, M_1 + M_2, 2Z_3, 2R_2, 2X_2]$                     | (1, 0, 0) |
| $[(\bullet)^{2T}, 2A_2, M_1 + M_2, Z_3 + Z_4, 2R_2, 2X_2]$                | trivial   |
| $[(\bullet)^{2T}, 2A_2, M_1 + M_2, 2Z_3, R_1 + R_2, X_1 + X_2]$           | (1, 0, 2) |
| $[(\bullet)^{2T}, 2A_2, M_1 + M_2, Z_3 + Z_4, R_1 + R_2, X_1 + X_2]$      | (0, 0, 2) |
| $[(\bullet)^{2T}, A_1 + A_2, 2M_2, 2Z_3, 2R_2, 2X_2]$                     | (1, 0, 2) |
| $[(\bullet)^{2T}, A_1 + A_2, 2M_2, Z_3 + Z_4, 2R_2, 2X_2]$                | (0, 0, 2) |
| $[(\bullet)^{2T}, A_1 + A_2, 2M_2, 2Z_3, R_1 + R_2, X_1 + X_2]$           | (1, 0, 0) |
| $[(\bullet)^{2T}, A_1 + A_2, 2M_2, Z_3 + Z_4, R_1 + R_2, X_1 + X_2]$      | trivial   |
| $[(\bullet)^{2T}, A_1 + A_2, M_1 + M_2, 2Z_3, 2R_2, 2X_2]$                | (1, 1, 0) |
| $[(\bullet)^{2T}, A_1 + A_2, M_1 + M_2, Z_3 + Z_4, 2R_2, 2X_2]$           | (0, 1, 0) |
| $[(\bullet)^{2T}, A_1 + A_2, M_1 + M_2, 2Z_3, R_1 + R_2, X_1 + X_2]$      | (1, 1, 2) |
| $[(\bullet)^{2T}, A_1 + A_2, M_1 + M_2, Z_3 + Z_4, R_1 + R_2, X_1 + X_2]$ | (0, 1, 2) |
| $[(\bullet)^{2T}, 2A_2, 2M_2, 2Z_3, 2R_1, 2X_1]$                          | (1, 1, 2) |
| $[(\bullet)^{2T}, 2A_2, 2M_2, Z_3 + Z_4, 2R_1, 2X_1]$                     | (0, 1, 2) |
| $[(\bullet)^{2T}, 2A_2, M_1 + M_2, 2Z_3, 2R_1, 2X_1]$                     | (1, 0, 0) |
| $[(\bullet)^{2T}, 2A_2, M_1 + M_2, Z_3 + Z_4, 2R_1, 2X_1]$                | trivial   |
| $[(\bullet)^{2T}, A_1 + A_2, 2M_2, 2Z_3, 2R_1, 2X_1]$                     | (1, 0, 2) |
| $[(\bullet)^{2T}, A_1 + A_2, 2M_2, Z_3 + Z_4, 2R_1, 2X_1]$                | (0, 0, 2) |
| $[(\bullet)^{2T}, A_1 + A_2, M_1 + M_2, 2Z_3, 2R_1, 2X_1]$                | (1, 1, 0) |
| $[(\bullet)^{2T}, A_1 + A_2, M_1 + M_2, Z_3 + Z_4, 2R_1, 2X_1]$           | (0, 1, 0) |
| $[(\bullet)^{2T}, 2A_2, 2M_1, 2Z_3, 2R_2, 2X_2]$                          | (1, 1, 2) |
| $[(\bullet)^{2T}, 2A_2, 2M_1, Z_3 + Z_4, 2R_2, 2X_2]$                     | (0, 1, 2) |
| $[(\bullet)^{2T}, 2A_2, 2M_1, 2Z_3, R_1 + R_2, X_1 + X_2]$                | (1, 1, 0) |
| $[(\bullet)^{2T}, 2A_2, 2M_1, Z_3 + Z_4, R_1 + R_2, X_1 + X_2]$           | (0, 1, 0) |
| $[(\bullet)^{2T}, A_1 + A_2, 2M_1, 2Z_3, 2R_2, 2X_2]$                     | (1, 0, 2) |
| $[(\bullet)^{2T}, A_1 + A_2, 2M_1, Z_3 + Z_4, 2R_2, 2X_2]$                | (0, 0, 2) |
| $[(\bullet)^{2T}, A_1 + A_2, 2M_1, 2Z_3, R_1 + R_2, X_1 + X_2]$           | (1, 0, 0) |
| $[(\bullet)^{2T}, A_1 + A_2, 2M_1, Z_3 + Z_4, R_1 + R_2, X_1 + X_2]$      | trivial   |

... continued on next page

... continued from previous page

|                                                                      |           |
|----------------------------------------------------------------------|-----------|
| $[(\bullet)^{2T}, 2A_2, 2M_1, 2Z_3, 2R_1, 2X_1]$                     | (1, 1, 2) |
| $[(\bullet)^{2T}, 2A_2, 2M_1, Z_3 + Z_4, 2R_1, 2X_1]$                | (0, 1, 2) |
| $[(\bullet)^{2T}, A_1 + A_2, 2M_1, 2Z_3, 2R_1, 2X_1]$                | (1, 0, 2) |
| $[(\bullet)^{2T}, A_1 + A_2, 2M_1, Z_3 + Z_4, 2R_1, 2X_1]$           | (0, 0, 2) |
| $[(\bullet)^{2T}, 2A_1, 2M_2, 2Z_3, 2R_2, 2X_2]$                     | (1, 1, 2) |
| $[(\bullet)^{2T}, 2A_1, 2M_2, Z_3 + Z_4, 2R_2, 2X_2]$                | (0, 1, 2) |
| $[(\bullet)^{2T}, 2A_1, 2M_2, 2Z_3, R_1 + R_2, X_1 + X_2]$           | (1, 1, 0) |
| $[(\bullet)^{2T}, 2A_1, 2M_2, Z_3 + Z_4, R_1 + R_2, X_1 + X_2]$      | (0, 1, 0) |
| $[(\bullet)^{2T}, 2A_1, M_1 + M_2, 2Z_3, 2R_2, 2X_2]$                | (1, 0, 0) |
| $[(\bullet)^{2T}, 2A_1, M_1 + M_2, Z_3 + Z_4, 2R_2, 2X_2]$           | trivial   |
| $[(\bullet)^{2T}, 2A_1, M_1 + M_2, 2Z_3, R_1 + R_2, X_1 + X_2]$      | (1, 0, 2) |
| $[(\bullet)^{2T}, 2A_1, M_1 + M_2, Z_3 + Z_4, R_1 + R_2, X_1 + X_2]$ | (0, 0, 2) |
| $[(\bullet)^{2T}, 2A_1, 2M_2, 2Z_3, 2R_1, 2X_1]$                     | (1, 1, 2) |
| $[(\bullet)^{2T}, 2A_1, 2M_2, Z_3 + Z_4, 2R_1, 2X_1]$                | (0, 1, 2) |
| $[(\bullet)^{2T}, 2A_1, M_1 + M_2, 2Z_3, 2R_1, 2X_1]$                | (1, 0, 0) |
| $[(\bullet)^{2T}, 2A_1, M_1 + M_2, Z_3 + Z_4, 2R_1, 2X_1]$           | trivial   |
| $[(\bullet)^{2T}, 2A_1, 2M_1, 2Z_3, 2R_2, 2X_2]$                     | (1, 1, 2) |
| $[(\bullet)^{2T}, 2A_1, 2M_1, Z_3 + Z_4, 2R_2, 2X_2]$                | (0, 1, 2) |
| $[(\bullet)^{2T}, 2A_1, 2M_1, 2Z_3, R_1 + R_2, X_1 + X_2]$           | (1, 1, 0) |
| $[(\bullet)^{2T}, 2A_1, 2M_1, Z_3 + Z_4, R_1 + R_2, X_1 + X_2]$      | (0, 1, 0) |
| $[(\bullet)^{2T}, 2A_1, 2M_1, 2Z_3, 2R_1, 2X_1]$                     | (1, 1, 2) |
| $[(\bullet)^{2T}, 2A_1, 2M_1, Z_3 + Z_4, 2R_1, 2X_1]$                | (0, 1, 2) |
| $[(\bullet)^{2T}, 2A_4, 2M_4, 2Z_4, 2R_2, 2X_2]$                     | (1, 1, 0) |
| $[(\bullet)^{2T}, 2A_4, 2M_4, 2Z_4, R_1 + R_2, X_1 + X_2]$           | (1, 1, 2) |
| $[(\bullet)^{2T}, 2A_4, M_3 + M_4, 2Z_4, 2R_2, 2X_2]$                | (0, 1, 2) |
| $[(\bullet)^{2T}, 2A_4, M_3 + M_4, 2Z_4, R_1 + R_2, X_1 + X_2]$      | (0, 1, 0) |
| $[(\bullet)^{2T}, A_3 + A_4, 2M_4, 2Z_4, 2R_2, 2X_2]$                | (0, 1, 0) |
| $[(\bullet)^{2T}, A_3 + A_4, 2M_4, 2Z_4, R_1 + R_2, X_1 + X_2]$      | (0, 1, 2) |
| $[(\bullet)^{2T}, A_3 + A_4, M_3 + M_4, 2Z_4, 2R_2, 2X_2]$           | (1, 1, 2) |
| $[(\bullet)^{2T}, A_3 + A_4, M_3 + M_4, 2Z_4, R_1 + R_2, X_1 + X_2]$ | (1, 1, 0) |
| $[(\bullet)^{2T}, A_2 + A_4, M_2 + M_4, 2Z_4, 2R_2, 2X_2]$           | (0, 1, 1) |
| $[(\bullet)^{2T}, A_2 + A_4, M_2 + M_4, 2Z_4, R_1 + R_2, X_1 + X_2]$ | (0, 1, 3) |
| $[(\bullet)^{2T}, A_2 + A_4, M_1 + M_4, 2Z_4, 2R_2, 2X_2]$           | (0, 0, 3) |
| $[(\bullet)^{2T}, A_2 + A_4, M_1 + M_4, 2Z_4, R_1 + R_2, X_1 + X_2]$ | (0, 0, 1) |
| $[(\bullet)^{2T}, A_1 + A_4, M_2 + M_4, 2Z_4, 2R_2, 2X_2]$           | (0, 0, 1) |
| $[(\bullet)^{2T}, A_1 + A_4, M_2 + M_4, 2Z_4, R_1 + R_2, X_1 + X_2]$ | (0, 0, 3) |
| $[(\bullet)^{2T}, A_1 + A_4, M_1 + M_4, 2Z_4, 2R_2, 2X_2]$           | (0, 1, 3) |
| $[(\bullet)^{2T}, A_1 + A_4, M_1 + M_4, 2Z_4, R_1 + R_2, X_1 + X_2]$ | (0, 1, 1) |
| $[(\bullet)^{2T}, 2A_4, 2M_4, 2Z_4, 2R_1, 2X_1]$                     | (1, 1, 0) |
| $[(\bullet)^{2T}, 2A_4, M_3 + M_4, 2Z_4, 2R_1, 2X_1]$                | (0, 1, 2) |
| $[(\bullet)^{2T}, A_3 + A_4, 2M_4, 2Z_4, 2R_1, 2X_1]$                | (0, 1, 0) |
| $[(\bullet)^{2T}, A_3 + A_4, M_3 + M_4, 2Z_4, 2R_1, 2X_1]$           | (1, 1, 2) |
| $[(\bullet)^{2T}, A_2 + A_4, M_2 + M_4, 2Z_4, 2R_1, 2X_1]$           | (0, 1, 1) |
| $[(\bullet)^{2T}, A_2 + A_4, M_1 + M_4, 2Z_4, 2R_1, 2X_1]$           | (0, 0, 3) |
| $[(\bullet)^{2T}, A_1 + A_4, M_2 + M_4, 2Z_4, 2R_1, 2X_1]$           | (0, 0, 1) |
| $[(\bullet)^{2T}, A_1 + A_4, M_1 + M_4, 2Z_4, 2R_1, 2X_1]$           | (0, 1, 3) |
| $[(\bullet)^{2T}, 2A_4, 2M_3, 2Z_4, 2R_2, 2X_2]$                     | (1, 1, 0) |
| $[(\bullet)^{2T}, 2A_4, 2M_3, 2Z_4, R_1 + R_2, X_1 + X_2]$           | (1, 1, 2) |
| $[(\bullet)^{2T}, A_3 + A_4, 2M_3, 2Z_4, 2R_2, 2X_2]$                | (0, 1, 0) |
| $[(\bullet)^{2T}, A_3 + A_4, 2M_3, 2Z_4, R_1 + R_2, X_1 + X_2]$      | (0, 1, 2) |
| $[(\bullet)^{2T}, A_2 + A_4, M_2 + M_3, 2Z_4, 2R_2, 2X_2]$           | (1, 1, 3) |
| $[(\bullet)^{2T}, A_2 + A_4, M_2 + M_3, 2Z_4, R_1 + R_2, X_1 + X_2]$ | (1, 1, 1) |
| $[(\bullet)^{2T}, A_2 + A_4, M_1 + M_3, 2Z_4, 2R_2, 2X_2]$           | (1, 0, 1) |
| $[(\bullet)^{2T}, A_2 + A_4, M_1 + M_3, 2Z_4, R_1 + R_2, X_1 + X_2]$ | (1, 0, 3) |

... continued on next page

... continued from previous page

|                                                                           |           |
|---------------------------------------------------------------------------|-----------|
| $[(\blacksquare)^{2T}, A_1 + A_4, M_2 + M_3, 2Z_4, 2R_2, 2X_2]$           | (1, 0, 3) |
| $[(\blacksquare)^{2T}, A_1 + A_4, M_2 + M_3, 2Z_4, R_1 + R_2, X_1 + X_2]$ | (1, 0, 1) |
| $[(\blacksquare)^{2T}, A_1 + A_4, M_1 + M_3, 2Z_4, 2R_2, 2X_2]$           | (1, 1, 1) |
| $[(\blacksquare)^{2T}, A_1 + A_4, M_1 + M_3, 2Z_4, R_1 + R_2, X_1 + X_2]$ | (1, 1, 3) |
| $[(\blacksquare)^{2T}, 2A_4, 2M_3, 2Z_4, 2R_1, 2X_1]$                     | (1, 1, 0) |
| $[(\blacksquare)^{2T}, A_3 + A_4, 2M_3, 2Z_4, 2R_1, 2X_1]$                | (0, 1, 0) |
| $[(\blacksquare)^{2T}, A_2 + A_4, M_2 + M_3, 2Z_4, 2R_1, 2X_1]$           | (1, 1, 3) |
| $[(\blacksquare)^{2T}, A_2 + A_4, M_1 + M_3, 2Z_4, 2R_1, 2X_1]$           | (1, 0, 1) |
| $[(\blacksquare)^{2T}, A_1 + A_4, M_2 + M_3, 2Z_4, 2R_1, 2X_1]$           | (1, 0, 3) |
| $[(\blacksquare)^{2T}, A_1 + A_4, M_1 + M_3, 2Z_4, 2R_1, 2X_1]$           | (1, 1, 1) |
| $[(\blacksquare)^{2T}, 2A_3, 2M_4, 2Z_4, 2R_2, 2X_2]$                     | (1, 1, 0) |
| $[(\blacksquare)^{2T}, 2A_3, 2M_4, 2Z_4, R_1 + R_2, X_1 + X_2]$           | (1, 1, 2) |
| $[(\blacksquare)^{2T}, 2A_3, M_3 + M_4, 2Z_4, 2R_2, 2X_2]$                | (0, 1, 2) |
| $[(\blacksquare)^{2T}, 2A_3, M_3 + M_4, 2Z_4, R_1 + R_2, X_1 + X_2]$      | (0, 1, 0) |
| $[(\blacksquare)^{2T}, A_2 + A_3, M_2 + M_4, 2Z_4, 2R_2, 2X_2]$           | (1, 1, 1) |
| $[(\blacksquare)^{2T}, A_2 + A_3, M_2 + M_4, 2Z_4, R_1 + R_2, X_1 + X_2]$ | (1, 1, 3) |
| $[(\blacksquare)^{2T}, A_2 + A_3, M_1 + M_4, 2Z_4, 2R_2, 2X_2]$           | (1, 0, 3) |
| $[(\blacksquare)^{2T}, A_2 + A_3, M_1 + M_4, 2Z_4, R_1 + R_2, X_1 + X_2]$ | (1, 0, 1) |
| $[(\blacksquare)^{2T}, A_1 + A_3, M_2 + M_4, 2Z_4, 2R_2, 2X_2]$           | (1, 0, 1) |
| $[(\blacksquare)^{2T}, A_1 + A_3, M_2 + M_4, 2Z_4, R_1 + R_2, X_1 + X_2]$ | (1, 0, 3) |
| $[(\blacksquare)^{2T}, A_1 + A_3, M_1 + M_4, 2Z_4, 2R_2, 2X_2]$           | (1, 1, 3) |
| $[(\blacksquare)^{2T}, A_1 + A_3, M_1 + M_4, 2Z_4, R_1 + R_2, X_1 + X_2]$ | (1, 1, 1) |
| $[(\blacksquare)^{2T}, 2A_3, 2M_4, 2Z_4, 2R_1, 2X_1]$                     | (1, 1, 0) |
| $[(\blacksquare)^{2T}, 2A_3, M_3 + M_4, 2Z_4, 2R_1, 2X_1]$                | (0, 1, 2) |
| $[(\blacksquare)^{2T}, A_2 + A_3, M_2 + M_4, 2Z_4, 2R_1, 2X_1]$           | (1, 1, 1) |
| $[(\blacksquare)^{2T}, A_2 + A_3, M_1 + M_4, 2Z_4, 2R_1, 2X_1]$           | (1, 0, 3) |
| $[(\blacksquare)^{2T}, A_1 + A_3, M_2 + M_4, 2Z_4, 2R_1, 2X_1]$           | (1, 0, 1) |
| $[(\blacksquare)^{2T}, A_1 + A_3, M_1 + M_4, 2Z_4, 2R_1, 2X_1]$           | (1, 1, 3) |
| $[(\blacksquare)^{2T}, 2A_3, 2M_3, 2Z_4, 2R_2, 2X_2]$                     | (1, 1, 0) |
| $[(\blacksquare)^{2T}, 2A_3, 2M_3, 2Z_4, R_1 + R_2, X_1 + X_2]$           | (1, 1, 2) |
| $[(\blacksquare)^{2T}, A_2 + A_3, M_2 + M_3, 2Z_4, 2R_2, 2X_2]$           | (0, 1, 3) |
| $[(\blacksquare)^{2T}, A_2 + A_3, M_2 + M_3, 2Z_4, R_1 + R_2, X_1 + X_2]$ | (0, 1, 1) |
| $[(\blacksquare)^{2T}, A_2 + A_3, M_1 + M_3, 2Z_4, 2R_2, 2X_2]$           | (0, 0, 1) |
| $[(\blacksquare)^{2T}, A_2 + A_3, M_1 + M_3, 2Z_4, R_1 + R_2, X_1 + X_2]$ | (0, 0, 3) |
| $[(\blacksquare)^{2T}, A_1 + A_3, M_2 + M_3, 2Z_4, 2R_2, 2X_2]$           | (0, 0, 3) |
| $[(\blacksquare)^{2T}, A_1 + A_3, M_2 + M_3, 2Z_4, R_1 + R_2, X_1 + X_2]$ | (0, 0, 1) |
| $[(\blacksquare)^{2T}, A_1 + A_3, M_1 + M_3, 2Z_4, 2R_2, 2X_2]$           | (0, 1, 1) |
| $[(\blacksquare)^{2T}, A_1 + A_3, M_1 + M_3, 2Z_4, R_1 + R_2, X_1 + X_2]$ | (0, 1, 3) |
| $[(\blacksquare)^{2T}, 2A_3, 2M_3, 2Z_4, 2R_1, 2X_1]$                     | (1, 1, 0) |
| $[(\blacksquare)^{2T}, A_2 + A_3, M_2 + M_3, 2Z_4, 2R_1, 2X_1]$           | (0, 1, 3) |
| $[(\blacksquare)^{2T}, A_2 + A_3, M_1 + M_3, 2Z_4, 2R_1, 2X_1]$           | (0, 0, 1) |
| $[(\blacksquare)^{2T}, A_1 + A_3, M_2 + M_3, 2Z_4, 2R_1, 2X_1]$           | (0, 0, 3) |
| $[(\blacksquare)^{2T}, A_1 + A_3, M_1 + M_3, 2Z_4, 2R_1, 2X_1]$           | (0, 1, 1) |
| $[(\blacksquare)^{2T}, 2A_2, 2M_2, 2Z_4, 2R_2, 2X_2]$                     | (1, 1, 2) |
| $[(\blacksquare)^{2T}, 2A_2, 2M_2, 2Z_4, R_1 + R_2, X_1 + X_2]$           | (1, 1, 0) |
| $[(\blacksquare)^{2T}, 2A_2, M_1 + M_2, 2Z_4, 2R_2, 2X_2]$                | (1, 0, 0) |
| $[(\blacksquare)^{2T}, 2A_2, M_1 + M_2, 2Z_4, R_1 + R_2, X_1 + X_2]$      | (1, 0, 2) |
| $[(\blacksquare)^{2T}, A_1 + A_2, 2M_2, 2Z_4, 2R_2, 2X_2]$                | (1, 0, 2) |
| $[(\blacksquare)^{2T}, A_1 + A_2, 2M_2, 2Z_4, R_1 + R_2, X_1 + X_2]$      | (1, 0, 0) |
| $[(\blacksquare)^{2T}, A_1 + A_2, M_1 + M_2, 2Z_4, 2R_2, 2X_2]$           | (1, 1, 0) |
| $[(\blacksquare)^{2T}, A_1 + A_2, M_1 + M_2, 2Z_4, R_1 + R_2, X_1 + X_2]$ | (1, 1, 2) |
| $[(\blacksquare)^{2T}, 2A_2, 2M_2, 2Z_4, 2R_1, 2X_1]$                     | (1, 1, 2) |
| $[(\blacksquare)^{2T}, 2A_2, M_1 + M_2, 2Z_4, 2R_1, 2X_1]$                | (1, 0, 0) |
| $[(\blacksquare)^{2T}, A_1 + A_2, 2M_2, 2Z_4, 2R_1, 2X_1]$                | (1, 0, 2) |

... continued on next page

... continued from previous page

|                                                                      |           |
|----------------------------------------------------------------------|-----------|
| $[(\blacksquare)^{2T}, A_1 + A_2, M_1 + M_2, 2Z_4, 2R_1, 2X_1]$      | (1, 1, 0) |
| $[(\blacksquare)^{2T}, 2A_2, 2M_1, 2Z_4, 2R_2, 2X_2]$                | (1, 1, 2) |
| $[(\blacksquare)^{2T}, 2A_2, 2M_1, 2Z_4, R_1 + R_2, X_1 + X_2]$      | (1, 1, 0) |
| $[(\blacksquare)^{2T}, A_1 + A_2, 2M_1, 2Z_4, 2R_2, 2X_2]$           | (1, 0, 2) |
| $[(\blacksquare)^{2T}, A_1 + A_2, 2M_1, 2Z_4, R_1 + R_2, X_1 + X_2]$ | (1, 0, 0) |
| $[(\blacksquare)^{2T}, 2A_2, 2M_1, 2Z_4, 2R_1, 2X_1]$                | (1, 1, 2) |
| $[(\blacksquare)^{2T}, A_1 + A_2, 2M_1, 2Z_4, 2R_1, 2X_1]$           | (1, 0, 2) |
| $[(\blacksquare)^{2T}, 2A_1, 2M_2, 2Z_4, 2R_2, 2X_2]$                | (1, 1, 2) |
| $[(\blacksquare)^{2T}, 2A_1, 2M_2, 2Z_4, R_1 + R_2, X_1 + X_2]$      | (1, 1, 0) |
| $[(\blacksquare)^{2T}, 2A_1, M_1 + M_2, 2Z_4, 2R_2, 2X_2]$           | (1, 0, 0) |
| $[(\blacksquare)^{2T}, 2A_1, M_1 + M_2, 2Z_4, R_1 + R_2, X_1 + X_2]$ | (1, 0, 2) |
| $[(\blacksquare)^{2T}, 2A_1, 2M_2, 2Z_4, 2R_1, 2X_1]$                | (1, 1, 2) |
| $[(\blacksquare)^{2T}, 2A_1, M_1 + M_2, 2Z_4, 2R_1, 2X_1]$           | (1, 0, 0) |
| $[(\blacksquare)^{2T}, 2A_1, 2M_1, 2Z_4, 2R_2, 2X_2]$                | (1, 1, 2) |
| $[(\blacksquare)^{2T}, 2A_1, 2M_1, 2Z_4, R_1 + R_2, X_1 + X_2]$      | (1, 1, 0) |
| $[(\blacksquare)^{2T}, 2A_1, 2M_1, 2Z_4, 2R_1, 2X_1]$                | (1, 1, 2) |

2nd minimal solution:  $\mu_2^T = 3$  (8320 symmetry vectors)

Space group 82 ( $\mathbb{Z}_2 \times \mathbb{Z}_2 \times \mathbb{Z}_2$ )

1st minimal solution:  $\mu_1^T = 2$  (102 symmetry vectors)

| $\mathbf{n}^T$                                                              | $\mathbf{v}^T \in \mathbb{Z}_2 \times \mathbb{Z}_2 \times \mathbb{Z}_2$ |
|-----------------------------------------------------------------------------|-------------------------------------------------------------------------|
| $[(\blacksquare)^{2T}, 2M_4, 2P_2, 2PA_2, 2X_1, 2N_1]$                      | (1, 1, 1)                                                               |
| $[(\blacksquare)^{2T}, 2M_4, P_2 + P_4, PA_2 + PA_3, X_1 + X_2, 2N_1]$      | (0, 1, 1)                                                               |
| $[(\blacksquare)^{2T}, 2M_4, 2P_2, PA_1 + PA_2, 2X_1, 2N_1]$                | (0, 1, 0)                                                               |
| $[(\blacksquare)^{2T}, 2M_4, P_2 + P_4, PA_2 + PA_4, X_1 + X_2, 2N_1]$      | (0, 0, 1)                                                               |
| $[(\blacksquare)^{2T}, 2M_4, P_2 + P_3, PA_2 + PA_3, X_1 + X_2, 2N_1]$      | (0, 0, 1)                                                               |
| $[(\blacksquare)^{2T}, 2M_4, P_2 + P_3, PA_2 + PA_4, X_1 + X_2, 2N_1]$      | (0, 1, 1)                                                               |
| $[(\blacksquare)^{2T}, 2M_4, P_1 + P_2, 2PA_2, 2X_1, 2N_1]$                 | (0, 1, 0)                                                               |
| $[(\blacksquare)^{2T}, 2M_4, P_1 + P_2, PA_1 + PA_2, 2X_1, 2N_1]$           | (1, 1, 1)                                                               |
| $[(\blacksquare)^{2T}, 2M_4, 2P_4, 2PA_3, 2X_2, 2N_1]$                      | (1, 1, 1)                                                               |
| $[(\blacksquare)^{2T}, 2M_4, P_2 + P_4, PA_1 + PA_3, X_1 + X_2, 2N_1]$      | (1, 1, 0)                                                               |
| $[(\blacksquare)^{2T}, 2M_4, 2P_4, PA_3 + PA_4, 2X_2, 2N_1]$                | (1, 0, 1)                                                               |
| $[(\blacksquare)^{2T}, 2M_4, P_3 + P_4, 2PA_3, 2X_2, 2N_1]$                 | (1, 0, 1)                                                               |
| $[(\blacksquare)^{2T}, 2M_4, P_3 + P_4, PA_3 + PA_4, 2X_2, 2N_1]$           | (1, 1, 1)                                                               |
| $[(\blacksquare)^{2T}, 2M_4, P_1 + P_4, PA_2 + PA_3, X_1 + X_2, 2N_1]$      | (1, 1, 0)                                                               |
| $[(\blacksquare)^{2T}, 2M_4, P_1 + P_4, PA_1 + PA_3, X_1 + X_2, 2N_1]$      | (0, 1, 1)                                                               |
| $[(\blacksquare)^{2T}, 2M_4, 2P_2, 2PA_1, 2X_1, 2N_1]$                      | (1, 1, 1)                                                               |
| $[(\blacksquare)^{2T}, 2M_4, P_2 + P_4, PA_1 + PA_4, X_1 + X_2, 2N_1]$      | (1, 0, 0)                                                               |
| $[(\blacksquare)^{2T}, 2M_4, P_2 + P_3, PA_1 + PA_3, X_1 + X_2, 2N_1]$      | (1, 0, 0)                                                               |
| $[(\blacksquare)^{2T}, 2M_4, P_2 + P_3, PA_1 + PA_4, X_1 + X_2, 2N_1]$      | (1, 1, 0)                                                               |
| $[(\blacksquare)^{2T}, 2M_4, P_1 + P_2, 2PA_1, 2X_1, 2N_1]$                 | (0, 1, 0)                                                               |
| $[(\blacksquare)^{2T}, 2M_4, 2P_4, 2PA_4, 2X_2, 2N_1]$                      | (1, 1, 1)                                                               |
| $[(\blacksquare)^{2T}, 2M_4, P_3 + P_4, 2PA_4, 2X_2, 2N_1]$                 | (1, 0, 1)                                                               |
| $[(\blacksquare)^{2T}, 2M_4, P_1 + P_4, PA_2 + PA_4, X_1 + X_2, 2N_1]$      | (1, 0, 0)                                                               |
| $[(\blacksquare)^{2T}, 2M_4, P_1 + P_4, PA_1 + PA_4, X_1 + X_2, 2N_1]$      | (0, 0, 1)                                                               |
| $[(\blacksquare)^{2T}, M_3 + M_4, 2P_2, 2PA_2, 2X_1, 2N_1]$                 | (1, 1, 0)                                                               |
| $[(\blacksquare)^{2T}, M_3 + M_4, P_2 + P_4, PA_2 + PA_3, X_1 + X_2, 2N_1]$ | (0, 1, 0)                                                               |
| $[(\blacksquare)^{2T}, M_3 + M_4, 2P_2, PA_1 + PA_2, 2X_1, 2N_1]$           | (0, 1, 1)                                                               |

... continued on next page

... continued from previous page

|                                                                             |           |
|-----------------------------------------------------------------------------|-----------|
| $[(\blacksquare)^{2T}, M_3 + M_4, P_2 + P_4, PA_2 + PA_4, X_1 + X_2, 2N_1]$ | trivial   |
| $[(\blacksquare)^{2T}, M_3 + M_4, P_2 + P_3, PA_2 + PA_3, X_1 + X_2, 2N_1]$ | trivial   |
| $[(\blacksquare)^{2T}, M_3 + M_4, P_2 + P_3, PA_2 + PA_4, X_1 + X_2, 2N_1]$ | (0, 1, 0) |
| $[(\blacksquare)^{2T}, M_3 + M_4, P_1 + P_2, 2PA_2, 2X_1, 2N_1]$            | (0, 1, 1) |
| $[(\blacksquare)^{2T}, M_3 + M_4, P_1 + P_2, PA_1 + PA_2, 2X_1, 2N_1]$      | (1, 1, 0) |
| $[(\blacksquare)^{2T}, M_3 + M_4, 2P_4, 2PA_3, 2X_2, 2N_1]$                 | (1, 1, 0) |
| $[(\blacksquare)^{2T}, M_3 + M_4, P_2 + P_4, PA_1 + PA_3, X_1 + X_2, 2N_1]$ | (1, 1, 1) |
| $[(\blacksquare)^{2T}, M_3 + M_4, 2P_4, PA_3 + PA_4, 2X_2, 2N_1]$           | (1, 0, 0) |
| $[(\blacksquare)^{2T}, M_3 + M_4, P_3 + P_4, 2PA_3, 2X_2, 2N_1]$            | (1, 0, 0) |
| $[(\blacksquare)^{2T}, M_3 + M_4, P_3 + P_4, PA_3 + PA_4, 2X_2, 2N_1]$      | (1, 1, 0) |
| $[(\blacksquare)^{2T}, M_3 + M_4, P_1 + P_4, PA_2 + PA_3, X_1 + X_2, 2N_1]$ | (1, 1, 1) |
| $[(\blacksquare)^{2T}, M_3 + M_4, P_1 + P_4, PA_1 + PA_3, X_1 + X_2, 2N_1]$ | (0, 1, 0) |
| $[(\blacksquare)^{2T}, M_3 + M_4, 2P_2, 2PA_1, 2X_1, 2N_1]$                 | (1, 1, 0) |
| $[(\blacksquare)^{2T}, M_3 + M_4, P_2 + P_4, PA_1 + PA_4, X_1 + X_2, 2N_1]$ | (1, 0, 1) |
| $[(\blacksquare)^{2T}, M_3 + M_4, P_2 + P_3, PA_1 + PA_3, X_1 + X_2, 2N_1]$ | (1, 0, 1) |
| $[(\blacksquare)^{2T}, M_3 + M_4, P_2 + P_3, PA_1 + PA_4, X_1 + X_2, 2N_1]$ | (1, 1, 1) |
| $[(\blacksquare)^{2T}, M_3 + M_4, P_1 + P_2, 2PA_1, 2X_1, 2N_1]$            | (0, 1, 1) |
| $[(\blacksquare)^{2T}, M_3 + M_4, 2P_4, 2PA_4, 2X_2, 2N_1]$                 | (1, 1, 0) |
| $[(\blacksquare)^{2T}, M_3 + M_4, P_3 + P_4, 2PA_4, 2X_2, 2N_1]$            | (1, 0, 0) |
| $[(\blacksquare)^{2T}, M_3 + M_4, P_1 + P_4, PA_2 + PA_4, X_1 + X_2, 2N_1]$ | (1, 0, 1) |
| $[(\blacksquare)^{2T}, M_3 + M_4, P_1 + P_4, PA_1 + PA_4, X_1 + X_2, 2N_1]$ | trivial   |
| $[(\blacksquare)^{2T}, 2M_4, 2P_3, 2PA_3, 2X_2, 2N_1]$                      | (1, 1, 1) |
| $[(\blacksquare)^{2T}, 2M_4, 2P_3, PA_3 + PA_4, 2X_2, 2N_1]$                | (1, 0, 1) |
| $[(\blacksquare)^{2T}, 2M_4, P_1 + P_3, PA_2 + PA_3, X_1 + X_2, 2N_1]$      | (1, 0, 0) |
| $[(\blacksquare)^{2T}, 2M_4, P_1 + P_3, PA_1 + PA_3, X_1 + X_2, 2N_1]$      | (0, 0, 1) |
| $[(\blacksquare)^{2T}, 2M_4, 2P_3, 2PA_4, 2X_2, 2N_1]$                      | (1, 1, 1) |
| $[(\blacksquare)^{2T}, 2M_4, P_1 + P_3, PA_2 + PA_4, X_1 + X_2, 2N_1]$      | (1, 1, 0) |
| $[(\blacksquare)^{2T}, 2M_4, P_1 + P_3, PA_1 + PA_4, X_1 + X_2, 2N_1]$      | (0, 1, 1) |
| $[(\blacksquare)^{2T}, M_3 + M_4, 2P_3, 2PA_3, 2X_2, 2N_1]$                 | (1, 1, 0) |
| $[(\blacksquare)^{2T}, M_3 + M_4, 2P_3, PA_3 + PA_4, 2X_2, 2N_1]$           | (1, 0, 0) |
| $[(\blacksquare)^{2T}, M_3 + M_4, P_1 + P_3, PA_2 + PA_3, X_1 + X_2, 2N_1]$ | (1, 0, 1) |
| $[(\blacksquare)^{2T}, M_3 + M_4, P_1 + P_3, PA_1 + PA_3, X_1 + X_2, 2N_1]$ | trivial   |
| $[(\blacksquare)^{2T}, M_3 + M_4, 2P_3, 2PA_4, 2X_2, 2N_1]$                 | (1, 1, 0) |
| $[(\blacksquare)^{2T}, M_3 + M_4, P_1 + P_3, PA_2 + PA_4, X_1 + X_2, 2N_1]$ | (1, 1, 1) |
| $[(\blacksquare)^{2T}, M_3 + M_4, P_1 + P_3, PA_1 + PA_4, X_1 + X_2, 2N_1]$ | (0, 1, 0) |
| $[(\blacksquare)^{2T}, 2M_4, 2P_1, 2PA_2, 2X_1, 2N_1]$                      | (1, 1, 1) |
| $[(\blacksquare)^{2T}, 2M_4, 2P_1, PA_1 + PA_2, 2X_1, 2N_1]$                | (0, 1, 0) |
| $[(\blacksquare)^{2T}, 2M_4, 2P_1, 2PA_1, 2X_1, 2N_1]$                      | (1, 1, 1) |
| $[(\blacksquare)^{2T}, M_3 + M_4, 2P_1, 2PA_2, 2X_1, 2N_1]$                 | (1, 1, 0) |
| $[(\blacksquare)^{2T}, M_3 + M_4, 2P_1, PA_1 + PA_2, 2X_1, 2N_1]$           | (0, 1, 1) |
| $[(\blacksquare)^{2T}, M_3 + M_4, 2P_1, 2PA_1, 2X_1, 2N_1]$                 | (1, 1, 0) |
| $[(\blacksquare)^{2T}, 2M_3, 2P_2, 2PA_2, 2X_1, 2N_1]$                      | (1, 1, 1) |
| $[(\blacksquare)^{2T}, 2M_3, P_2 + P_4, PA_2 + PA_3, X_1 + X_2, 2N_1]$      | (0, 1, 1) |
| $[(\blacksquare)^{2T}, 2M_3, 2P_2, PA_1 + PA_2, 2X_1, 2N_1]$                | (0, 1, 0) |
| $[(\blacksquare)^{2T}, 2M_3, P_2 + P_4, PA_2 + PA_4, X_1 + X_2, 2N_1]$      | (0, 0, 1) |
| $[(\blacksquare)^{2T}, 2M_3, P_2 + P_3, PA_2 + PA_3, X_1 + X_2, 2N_1]$      | (0, 0, 1) |
| $[(\blacksquare)^{2T}, 2M_3, P_2 + P_3, PA_2 + PA_4, X_1 + X_2, 2N_1]$      | (0, 1, 1) |
| $[(\blacksquare)^{2T}, 2M_3, P_1 + P_2, 2PA_2, 2X_1, 2N_1]$                 | (0, 1, 0) |
| $[(\blacksquare)^{2T}, 2M_3, P_1 + P_2, PA_1 + PA_2, 2X_1, 2N_1]$           | (1, 1, 1) |
| $[(\blacksquare)^{2T}, 2M_3, 2P_4, 2PA_3, 2X_2, 2N_1]$                      | (1, 1, 1) |
| $[(\blacksquare)^{2T}, 2M_3, P_2 + P_4, PA_1 + PA_3, X_1 + X_2, 2N_1]$      | (1, 1, 0) |
| $[(\blacksquare)^{2T}, 2M_3, 2P_4, PA_3 + PA_4, 2X_2, 2N_1]$                | (1, 0, 1) |
| $[(\blacksquare)^{2T}, 2M_3, P_3 + P_4, 2PA_3, 2X_2, 2N_1]$                 | (1, 0, 1) |
| $[(\blacksquare)^{2T}, 2M_3, P_3 + P_4, PA_3 + PA_4, 2X_2, 2N_1]$           | (1, 1, 1) |

... continued on next page



... continued from previous page

|                                                                        |           |
|------------------------------------------------------------------------|-----------|
| $[(\blacksquare)^{2T}, 2M_3, P_1 + P_4, PA_2 + PA_3, X_1 + X_2, 2N_1]$ | (1, 1, 0) |
| $[(\blacksquare)^{2T}, 2M_3, P_1 + P_4, PA_1 + PA_3, X_1 + X_2, 2N_1]$ | (0, 1, 1) |
| $[(\blacksquare)^{2T}, 2M_3, 2P_2, 2PA_1, 2X_1, 2N_1]$                 | (1, 1, 1) |
| $[(\blacksquare)^{2T}, 2M_3, P_2 + P_4, PA_1 + PA_4, X_1 + X_2, 2N_1]$ | (1, 0, 0) |
| $[(\blacksquare)^{2T}, 2M_3, P_2 + P_3, PA_1 + PA_3, X_1 + X_2, 2N_1]$ | (1, 0, 0) |
| $[(\blacksquare)^{2T}, 2M_3, P_2 + P_3, PA_1 + PA_4, X_1 + X_2, 2N_1]$ | (1, 1, 0) |
| $[(\blacksquare)^{2T}, 2M_3, P_1 + P_2, 2PA_1, 2X_1, 2N_1]$            | (0, 1, 0) |
| $[(\blacksquare)^{2T}, 2M_3, 2P_4, 2PA_4, 2X_2, 2N_1]$                 | (1, 1, 1) |
| $[(\blacksquare)^{2T}, 2M_3, P_3 + P_4, 2PA_4, 2X_2, 2N_1]$            | (1, 0, 1) |
| $[(\blacksquare)^{2T}, 2M_3, P_1 + P_4, PA_2 + PA_4, X_1 + X_2, 2N_1]$ | (1, 0, 0) |
| $[(\blacksquare)^{2T}, 2M_3, P_1 + P_4, PA_1 + PA_4, X_1 + X_2, 2N_1]$ | (0, 0, 1) |
| $[(\blacksquare)^{2T}, 2M_3, 2P_3, 2PA_3, 2X_2, 2N_1]$                 | (1, 1, 1) |
| $[(\blacksquare)^{2T}, 2M_3, 2P_3, PA_3 + PA_4, 2X_2, 2N_1]$           | (1, 0, 1) |
| $[(\blacksquare)^{2T}, 2M_3, P_1 + P_3, PA_2 + PA_3, X_1 + X_2, 2N_1]$ | (1, 0, 0) |
| $[(\blacksquare)^{2T}, 2M_3, P_1 + P_3, PA_1 + PA_3, X_1 + X_2, 2N_1]$ | (0, 0, 1) |
| $[(\blacksquare)^{2T}, 2M_3, 2P_3, 2PA_4, 2X_2, 2N_1]$                 | (1, 1, 1) |
| $[(\blacksquare)^{2T}, 2M_3, P_1 + P_3, PA_2 + PA_4, X_1 + X_2, 2N_1]$ | (1, 1, 0) |
| $[(\blacksquare)^{2T}, 2M_3, P_1 + P_3, PA_1 + PA_4, X_1 + X_2, 2N_1]$ | (0, 1, 1) |
| $[(\blacksquare)^{2T}, 2M_3, 2P_1, 2PA_2, 2X_1, 2N_1]$                 | (1, 1, 1) |
| $[(\blacksquare)^{2T}, 2M_3, 2P_1, PA_1 + PA_2, 2X_1, 2N_1]$           | (0, 1, 0) |
| $[(\blacksquare)^{2T}, 2M_3, 2P_1, 2PA_1, 2X_1, 2N_1]$                 | (1, 1, 1) |

2nd minimal solution:  $\mu_2^T = 3$  (2080 symmetry vectors)

Space group 83 ( $\mathbb{Z}_4 \times \mathbb{Z}_4 \times \mathbb{Z}_4$ )

1st minimal solution:  $\mu_1^T = 2$  (464 symmetry vectors)

| $\mathbf{n}^T$                                                                                     | $\mathbf{v}^T \in \mathbb{Z}_4 \times \mathbb{Z}_4 \times \mathbb{Z}_4$ |
|----------------------------------------------------------------------------------------------------|-------------------------------------------------------------------------|
| $[(\blacksquare)^{2T}, 2A_4^-, M_4^+ + M_4^-, Z_3^- + Z_4^-, 2R_2^-, X_2^+ + X_2^-]$               | (0, 1, 3)                                                               |
| $[(\blacksquare)^{2T}, 2A_4^-, M_4^+ + M_4^-, Z_3^- + Z_4^-, R_1^+ + R_2^-, X_1^- + X_2^-]$        | (0, 3, 3)                                                               |
| $[(\blacksquare)^{2T}, A_3^- + A_4^-, M_3^+ + M_4^-, Z_3^- + Z_4^-, 2R_2^-, X_2^+ + X_2^-]$        | (0, 3, 3)                                                               |
| $[(\blacksquare)^{2T}, A_3^- + A_4^-, M_3^+ + M_4^-, Z_3^- + Z_4^-, R_1^+ + R_2^-, X_1^- + X_2^-]$ | (0, 1, 3)                                                               |
| $[(\blacksquare)^{2T}, A_2^+ + A_4^-, M_2^- + M_4^-, Z_3^- + Z_4^-, 2R_2^-, X_2^+ + X_2^-]$        | (0, 0, 3)                                                               |
| $[(\blacksquare)^{2T}, A_2^+ + A_4^-, M_2^- + M_4^-, Z_3^- + Z_4^-, R_1^+ + R_2^-, X_1^- + X_2^-]$ | (0, 2, 3)                                                               |
| $[(\blacksquare)^{2T}, A_1^+ + A_4^-, M_1^- + M_4^-, Z_3^- + Z_4^-, 2R_2^-, X_2^+ + X_2^-]$        | (0, 2, 3)                                                               |
| $[(\blacksquare)^{2T}, A_1^+ + A_4^-, M_1^- + M_4^-, Z_3^- + Z_4^-, R_1^+ + R_2^-, X_1^- + X_2^-]$ | (0, 0, 3)                                                               |
| $[(\blacksquare)^{2T}, 2A_4^-, M_4^+ + M_4^-, Z_3^- + Z_4^-, R_1^+ + R_2^-, X_1^+ + X_2^+]$        | (0, 1, 1)                                                               |
| $[(\blacksquare)^{2T}, 2A_4^-, M_4^+ + M_4^-, Z_3^- + Z_4^-, 2R_1^+, X_1^+ + X_1^-]$               | (0, 3, 1)                                                               |
| $[(\blacksquare)^{2T}, A_3^- + A_4^-, M_3^+ + M_4^-, Z_3^- + Z_4^-, R_1^+ + R_2^-, X_1^+ + X_2^+]$ | (0, 3, 1)                                                               |
| $[(\blacksquare)^{2T}, A_3^- + A_4^-, M_3^+ + M_4^-, Z_3^- + Z_4^-, 2R_1^+, X_1^+ + X_1^-]$        | (0, 1, 1)                                                               |
| $[(\blacksquare)^{2T}, A_2^+ + A_4^-, M_2^- + M_4^-, Z_3^- + Z_4^-, R_1^+ + R_2^-, X_1^+ + X_2^+]$ | (0, 0, 1)                                                               |
| $[(\blacksquare)^{2T}, A_2^+ + A_4^-, M_2^- + M_4^-, Z_3^- + Z_4^-, 2R_1^+, X_1^+ + X_1^-]$        | (0, 2, 1)                                                               |
| $[(\blacksquare)^{2T}, A_1^+ + A_4^-, M_1^- + M_4^-, Z_3^- + Z_4^-, R_1^+ + R_2^-, X_1^+ + X_2^+]$ | (0, 2, 1)                                                               |
| $[(\blacksquare)^{2T}, A_1^+ + A_4^-, M_1^- + M_4^-, Z_3^- + Z_4^-, 2R_1^+, X_1^+ + X_1^-]$        | (0, 0, 1)                                                               |
| $[(\blacksquare)^{2T}, A_4^+ + A_4^-, M_4^+ + M_4^-, Z_3^+ + Z_4^-, R_2^+ + R_2^-, X_2^+ + X_2^-]$ | (2, 1, 3)                                                               |
| $[(\blacksquare)^{2T}, A_4^+ + A_4^-, M_4^+ + M_4^-, Z_3^+ + Z_4^-, R_1^- + R_2^-, X_1^+ + X_2^+]$ | (0, 1, 1)                                                               |
| $[(\blacksquare)^{2T}, A_3^- + A_4^-, M_3^- + M_4^+, Z_3^- + Z_4^-, 2R_2^-, X_2^+ + X_2^-]$        | (0, 1, 1)                                                               |
| $[(\blacksquare)^{2T}, A_3^- + A_4^-, M_3^- + M_4^+, Z_3^- + Z_4^-, R_1^+ + R_2^-, X_1^+ + X_2^+]$ | (0, 1, 3)                                                               |
| $[(\blacksquare)^{2T}, A_3^+ + A_4^-, M_3^+ + M_4^+, Z_3^+ + Z_4^-, R_2^+ + R_2^-, X_2^+ + X_2^-]$ | (0, 1, 1)                                                               |
| $[(\blacksquare)^{2T}, A_3^+ + A_4^-, M_3^+ + M_4^+, Z_3^+ + Z_4^-, R_1^- + R_2^-, X_1^+ + X_2^+]$ | (2, 1, 3)                                                               |

... continued on next page



... continued from previous page

[illegible]

... continued on next page

... continued from previous page

|                                                                                               |           |
|-----------------------------------------------------------------------------------------------|-----------|
| $[(\bullet)^{2T}, A_2^- + A_4^-, M_2^+ + M_4^+, Z_3^+ + Z_4^-, R_1^- + R_2^-, X_1^- + X_2^-]$ | (3, 3, 0) |
| $[(\bullet)^{2T}, A_2^- + A_4^-, M_2^+ + M_4^+, Z_3^+ + Z_4^-, R_1^+ + R_2^+, X_1^+ + X_2^+]$ | (1, 1, 2) |
| $[(\bullet)^{2T}, A_2^- + A_3^-, M_2^- + M_3^-, Z_3^+ + Z_4^-, R_2^+ + R_2^-, X_2^+ + X_2^-]$ | (1, 0, 1) |
| $[(\bullet)^{2T}, A_2^- + A_3^-, M_2^- + M_3^-, Z_3^+ + Z_4^-, R_1^+ + R_2^+, X_1^- + X_2^-]$ | (1, 2, 1) |
| $[(\bullet)^{2T}, A_2^- + A_3^-, M_2^- + M_3^-, Z_3^+ + Z_4^-, R_1^- + R_2^-, X_1^- + X_2^-]$ | (3, 2, 1) |
| $[(\bullet)^{2T}, A_2^- + A_3^-, M_2^- + M_3^-, Z_3^+ + Z_4^-, R_1^+ + R_2^+, X_1^+ + X_2^+]$ | (1, 0, 3) |
| $[(\bullet)^{2T}, A_2^- + A_3^-, M_2^- + M_3^-, Z_3^+ + Z_4^-, R_1^- + R_2^-, X_1^+ + X_2^+]$ | (3, 0, 3) |
| $[(\bullet)^{2T}, A_2^- + A_3^-, M_2^- + M_3^-, Z_3^+ + Z_4^-, R_1^+ + R_1^-, X_1^+ + X_1^-]$ | (3, 2, 3) |
| $[(\bullet)^{2T}, A_2^- + A_3^-, M_2^+ + M_3^+, Z_3^+ + Z_4^-, R_1^- + R_2^-, X_1^- + X_2^-]$ | (3, 1, 0) |
| $[(\bullet)^{2T}, A_2^- + A_3^-, M_2^+ + M_3^+, Z_3^+ + Z_4^-, R_1^+ + R_2^+, X_1^+ + X_2^+]$ | (1, 3, 2) |
| $[(\bullet)^{2T}, 2A_2^+, M_2^+ + M_2^-, Z_3^- + Z_4^-, 2R_2^-, X_2^+ + X_2^-]$               | trivial   |
| $[(\bullet)^{2T}, 2A_2^+, M_2^+ + M_2^-, Z_3^- + Z_4^-, R_1^+ + R_2^-, X_1^+ + X_2^+]$        | (0, 0, 2) |
| $[(\bullet)^{2T}, A_1^- + A_2^+, M_1^+ + M_2^-, Z_3^+ + Z_4^-, R_2^+ + R_2^-, X_2^+ + X_2^-]$ | (3, 0, 2) |
| $[(\bullet)^{2T}, A_1^- + A_2^+, M_1^+ + M_2^-, Z_3^+ + Z_4^-, R_1^- + R_2^-, X_1^+ + X_2^+]$ | (1, 0, 0) |
| $[(\bullet)^{2T}, A_1^+ + A_2^+, M_1^+ + M_2^-, Z_3^- + Z_4^-, 2R_2^-, X_2^+ + X_2^-]$        | (0, 0, 2) |
| $[(\bullet)^{2T}, A_1^+ + A_2^+, M_1^+ + M_2^-, Z_3^- + Z_4^-, R_1^+ + R_2^-, X_1^+ + X_2^+]$ | trivial   |
| $[(\bullet)^{2T}, 2A_2^+, M_2^+ + M_2^-, Z_3^- + Z_4^-, R_1^+ + R_2^-, X_1^- + X_2^-]$        | (0, 2, 0) |
| $[(\bullet)^{2T}, 2A_2^+, M_2^+ + M_2^-, Z_3^- + Z_4^-, 2R_1^+, X_1^+ + X_1^-]$               | (0, 2, 2) |
| $[(\bullet)^{2T}, A_1^- + A_2^+, M_1^+ + M_2^-, Z_3^+ + Z_4^-, R_1^+ + R_2^+, X_1^- + X_2^-]$ | (3, 2, 2) |
| $[(\bullet)^{2T}, A_1^- + A_2^+, M_1^+ + M_2^-, Z_3^+ + Z_4^-, R_1^+ + R_1^-, X_1^+ + X_1^-]$ | (1, 2, 0) |
| $[(\bullet)^{2T}, A_1^+ + A_2^+, M_1^+ + M_2^-, Z_3^- + Z_4^-, R_1^+ + R_2^-, X_1^- + X_2^-]$ | (0, 2, 2) |
| $[(\bullet)^{2T}, A_1^+ + A_2^+, M_1^+ + M_2^-, Z_3^- + Z_4^-, 2R_1^+, X_1^+ + X_1^-]$        | (0, 2, 0) |
| $[(\bullet)^{2T}, A_1^+ + A_2^+, M_1^- + M_2^+, Z_3^- + Z_4^-, 2R_2^-, X_2^+ + X_2^-]$        | (0, 2, 0) |
| $[(\bullet)^{2T}, A_1^+ + A_2^+, M_1^- + M_2^+, Z_3^- + Z_4^-, R_1^+ + R_2^-, X_1^- + X_2^-]$ | trivial   |
| $[(\bullet)^{2T}, A_1^+ + A_2^+, M_1^- + M_2^+, Z_3^- + Z_4^-, R_1^+ + R_2^-, X_1^+ + X_2^+]$ | (0, 2, 2) |
| $[(\bullet)^{2T}, A_1^+ + A_2^+, M_1^- + M_2^+, Z_3^- + Z_4^-, 2R_1^+, X_1^+ + X_1^-]$        | (0, 0, 2) |
| $[(\bullet)^{2T}, A_2^+ + A_4^+, M_2^- + M_4^-, Z_3^+ + Z_4^-, R_1^- + R_2^-, X_1^- + X_2^-]$ | (0, 2, 3) |
| $[(\bullet)^{2T}, A_2^+ + A_4^+, M_2^- + M_4^-, Z_3^+ + Z_4^-, R_1^+ + R_2^+, X_1^+ + X_2^+]$ | (2, 0, 1) |
| $[(\bullet)^{2T}, A_2^+ + A_4^+, M_2^+ + M_4^+, Z_3^+ + Z_4^-, R_2^+ + R_2^-, X_2^+ + X_2^-]$ | (2, 1, 0) |
| $[(\bullet)^{2T}, A_2^+ + A_4^+, M_2^+ + M_4^+, Z_3^+ + Z_4^-, R_1^+ + R_2^+, X_1^- + X_2^-]$ | (2, 3, 0) |
| $[(\bullet)^{2T}, A_2^+ + A_4^+, M_2^+ + M_4^+, Z_3^+ + Z_4^-, R_1^- + R_2^-, X_1^- + X_2^-]$ | (0, 3, 0) |
| $[(\bullet)^{2T}, A_2^+ + A_4^+, M_2^+ + M_4^+, Z_3^+ + Z_4^-, R_1^+ + R_2^+, X_1^+ + X_2^+]$ | (2, 1, 2) |
| $[(\bullet)^{2T}, A_2^+ + A_4^+, M_2^+ + M_4^+, Z_3^+ + Z_4^-, R_1^- + R_2^-, X_1^+ + X_2^+]$ | (0, 1, 2) |
| $[(\bullet)^{2T}, A_2^+ + A_4^+, M_2^+ + M_4^+, Z_3^+ + Z_4^-, R_1^+ + R_1^-, X_1^+ + X_1^-]$ | (0, 3, 2) |
| $[(\bullet)^{2T}, A_2^+ + A_3^+, M_2^- + M_3^-, Z_3^+ + Z_4^-, R_1^- + R_2^-, X_1^- + X_2^-]$ | (2, 2, 1) |
| $[(\bullet)^{2T}, A_2^+ + A_3^+, M_2^- + M_3^-, Z_3^+ + Z_4^-, R_1^+ + R_2^+, X_1^+ + X_2^+]$ | (0, 0, 3) |
| $[(\bullet)^{2T}, A_2^+ + A_3^+, M_2^+ + M_3^+, Z_3^+ + Z_4^-, R_2^+ + R_2^-, X_2^+ + X_2^-]$ | (0, 3, 0) |
| $[(\bullet)^{2T}, A_2^+ + A_3^+, M_2^+ + M_3^+, Z_3^+ + Z_4^-, R_1^+ + R_2^+, X_1^- + X_2^-]$ | (0, 1, 0) |
| $[(\bullet)^{2T}, A_2^+ + A_3^+, M_2^+ + M_3^+, Z_3^+ + Z_4^-, R_1^- + R_2^-, X_1^- + X_2^-]$ | (2, 1, 0) |
| $[(\bullet)^{2T}, A_2^+ + A_3^+, M_2^+ + M_3^+, Z_3^+ + Z_4^-, R_1^+ + R_2^+, X_1^+ + X_2^+]$ | (0, 3, 2) |
| $[(\bullet)^{2T}, A_2^+ + A_3^+, M_2^+ + M_3^+, Z_3^+ + Z_4^-, R_1^- + R_2^-, X_1^+ + X_2^+]$ | (2, 3, 2) |
| $[(\bullet)^{2T}, A_2^+ + A_3^+, M_2^+ + M_3^+, Z_3^+ + Z_4^-, R_1^+ + R_1^-, X_1^+ + X_1^-]$ | (2, 1, 2) |
| $[(\bullet)^{2T}, A_2^+ + A_2^+, M_2^+ + M_2^-, Z_3^+ + Z_4^-, R_1^- + R_2^-, X_1^- + X_2^-]$ | (3, 2, 0) |
| $[(\bullet)^{2T}, A_2^+ + A_2^+, M_2^+ + M_2^-, Z_3^+ + Z_4^-, R_1^+ + R_2^+, X_1^+ + X_2^+]$ | (1, 0, 2) |
| $[(\bullet)^{2T}, A_1^+ + A_1^-, M_1^+ + M_1^-, Z_3^+ + Z_4^-, R_2^+ + R_2^-, X_2^+ + X_2^-]$ | (3, 2, 2) |
| $[(\bullet)^{2T}, A_1^+ + A_1^-, M_1^+ + M_1^-, Z_3^+ + Z_4^-, R_1^+ + R_2^+, X_1^- + X_2^-]$ | (3, 0, 2) |
| $[(\bullet)^{2T}, A_1^+ + A_1^-, M_1^+ + M_1^-, Z_3^+ + Z_4^-, R_1^- + R_2^-, X_1^+ + X_2^+]$ | (1, 2, 0) |
| $[(\bullet)^{2T}, A_1^+ + A_1^-, M_1^+ + M_1^-, Z_3^+ + Z_4^-, R_1^+ + R_1^-, X_1^+ + X_1^-]$ | (1, 0, 0) |
| $[(\bullet)^{2T}, A_1^- + A_4^-, M_1^- + M_4^-, Z_3^+ + Z_4^-, R_2^+ + R_2^-, X_2^+ + X_2^-]$ | (3, 2, 3) |
| $[(\bullet)^{2T}, A_1^- + A_4^-, M_1^- + M_4^-, Z_3^+ + Z_4^-, R_1^+ + R_2^+, X_1^- + X_2^-]$ | (3, 0, 3) |
| $[(\bullet)^{2T}, A_1^- + A_4^-, M_1^- + M_4^-, Z_3^+ + Z_4^-, R_1^- + R_2^-, X_1^- + X_2^-]$ | (1, 0, 3) |
| $[(\bullet)^{2T}, A_1^- + A_4^-, M_1^- + M_4^-, Z_3^+ + Z_4^-, R_1^+ + R_2^+, X_1^+ + X_2^+]$ | (3, 2, 1) |
| $[(\bullet)^{2T}, A_1^- + A_4^-, M_1^- + M_4^-, Z_3^+ + Z_4^-, R_1^- + R_2^-, X_1^+ + X_2^+]$ | (1, 2, 1) |
| $[(\bullet)^{2T}, A_1^- + A_4^-, M_1^- + M_4^-, Z_3^+ + Z_4^-, R_1^+ + R_1^-, X_1^+ + X_1^-]$ | (1, 0, 1) |

... continued on next page

... continued from previous page

[illegible]

... continued on next page





... continued on next page



... continued from previous page

|                                                                                               |           |
|-----------------------------------------------------------------------------------------------|-----------|
| $[(\bullet)^{2T}, 2A_4^+, M_4^+ + M_4^-, Z_3^+ + Z_4^+, 2R_2^+, X_2^+ + X_2^-]$               | (2, 1, 3) |
| $[(\bullet)^{2T}, 2A_4^+, M_4^+ + M_4^-, Z_3^+ + Z_4^+, R_1^- + R_2^+, X_1^+ + X_2^+]$        | (0, 1, 1) |
| $[(\bullet)^{2T}, A_3^+ + A_4^+, M_3^- + M_4^+, Z_3^+ + Z_4^+, 2R_2^+, X_2^+ + X_2^-]$        | (0, 1, 1) |
| $[(\bullet)^{2T}, A_3^+ + A_4^+, M_3^- + M_4^+, Z_3^+ + Z_4^+, R_1^- + R_2^+, X_1^+ + X_2^+]$ | (2, 1, 3) |
| $[(\bullet)^{2T}, A_2^- + A_4^+, M_2^+ + M_4^+, Z_3^+ + Z_4^+, 2R_2^+, X_2^+ + X_2^-]$        | (1, 1, 0) |
| $[(\bullet)^{2T}, A_2^- + A_4^+, M_2^+ + M_4^+, Z_3^+ + Z_4^+, R_1^- + R_2^+, X_1^+ + X_2^+]$ | (3, 1, 2) |
| $[(\bullet)^{2T}, A_1^- + A_4^+, M_1^+ + M_4^+, Z_3^+ + Z_4^+, 2R_2^+, X_2^+ + X_2^-]$        | (3, 1, 2) |
| $[(\bullet)^{2T}, A_1^- + A_4^+, M_1^+ + M_4^+, Z_3^+ + Z_4^+, R_1^- + R_2^+, X_1^+ + X_2^+]$ | (1, 1, 0) |
| $[(\bullet)^{2T}, 2A_4^+, M_4^+ + M_4^-, Z_3^+ + Z_4^+, R_1^- + R_2^+, X_1^- + X_2^-]$        | (0, 3, 3) |
| $[(\bullet)^{2T}, A_3^+ + A_4^+, M_3^- + M_4^+, Z_3^+ + Z_4^+, R_1^- + R_2^+, X_1^- + X_2^-]$ | (2, 3, 1) |
| $[(\bullet)^{2T}, A_3^+ + A_4^+, M_3^+ + M_4^-, Z_3^+ + Z_4^+, 2R_2^+, X_2^+ + X_2^-]$        | (0, 3, 3) |
| $[(\bullet)^{2T}, A_3^+ + A_4^+, M_3^+ + M_4^-, Z_3^+ + Z_4^+, R_1^- + R_2^+, X_1^- + X_2^-]$ | (2, 1, 3) |
| $[(\bullet)^{2T}, A_3^+ + A_4^+, M_3^+ + M_4^-, Z_3^+ + Z_4^+, R_1^- + R_2^+, X_1^+ + X_2^+]$ | (2, 3, 1) |
| $[(\bullet)^{2T}, A_2^- + A_4^+, M_2^- + M_4^-, Z_3^+ + Z_4^+, 2R_2^+, X_2^+ + X_2^-]$        | (1, 0, 3) |
| $[(\bullet)^{2T}, A_2^- + A_4^+, M_2^- + M_4^-, Z_3^+ + Z_4^+, R_1^- + R_2^+, X_1^- + X_2^-]$ | (3, 2, 3) |
| $[(\bullet)^{2T}, A_2^- + A_4^+, M_2^- + M_4^-, Z_3^+ + Z_4^+, R_1^- + R_2^+, X_1^+ + X_2^+]$ | (3, 0, 1) |
| $[(\bullet)^{2T}, A_2^- + A_4^+, M_2^+ + M_4^+, Z_3^+ + Z_4^+, R_1^- + R_2^+, X_1^- + X_2^-]$ | (3, 3, 0) |
| $[(\bullet)^{2T}, A_1^- + A_4^+, M_1^- + M_4^-, Z_3^+ + Z_4^+, 2R_2^+, X_2^+ + X_2^-]$        | (3, 2, 3) |
| $[(\bullet)^{2T}, A_1^- + A_4^+, M_1^- + M_4^-, Z_3^+ + Z_4^+, R_1^- + R_2^+, X_1^- + X_2^-]$ | (1, 0, 3) |
| $[(\bullet)^{2T}, A_1^- + A_4^+, M_1^- + M_4^-, Z_3^+ + Z_4^+, R_1^- + R_2^+, X_1^+ + X_2^+]$ | (1, 2, 1) |
| $[(\bullet)^{2T}, A_1^- + A_4^+, M_1^+ + M_4^+, Z_3^+ + Z_4^+, R_1^- + R_2^+, X_1^- + X_2^-]$ | (1, 3, 2) |
| $[(\bullet)^{2T}, 2A_4^+, M_4^+ + M_4^-, Z_3^+ + Z_4^+, 2R_1^-, X_1^+ + X_1^-]$               | (2, 3, 1) |
| $[(\bullet)^{2T}, A_3^+ + A_4^+, M_3^- + M_4^-, Z_3^+ + Z_4^+, 2R_1^-, X_1^+ + X_1^-]$        | (0, 3, 3) |
| $[(\bullet)^{2T}, A_3^+ + A_4^+, M_3^+ + M_4^-, Z_3^+ + Z_4^+, 2R_1^-, X_1^+ + X_1^-]$        | (0, 1, 1) |
| $[(\bullet)^{2T}, A_2^- + A_4^+, M_2^- + M_4^-, Z_3^+ + Z_4^+, 2R_1^-, X_1^+ + X_1^-]$        | (1, 2, 1) |
| $[(\bullet)^{2T}, A_2^- + A_4^+, M_2^+ + M_4^-, Z_3^+ + Z_4^+, 2R_1^-, X_1^+ + X_1^-]$        | (1, 3, 2) |
| $[(\bullet)^{2T}, A_1^- + A_4^+, M_1^- + M_4^-, Z_3^+ + Z_4^+, 2R_1^-, X_1^+ + X_1^-]$        | (3, 0, 1) |
| $[(\bullet)^{2T}, A_1^- + A_4^+, M_1^+ + M_4^+, Z_3^+ + Z_4^+, 2R_1^-, X_1^+ + X_1^-]$        | (3, 3, 0) |
| $[(\bullet)^{2T}, 2A_3^+, M_3^+ + M_3^-, Z_3^+ + Z_4^+, 2R_2^+, X_2^+ + X_2^-]$               | (2, 3, 1) |
| $[(\bullet)^{2T}, 2A_3^+, M_3^+ + M_3^-, Z_3^+ + Z_4^+, R_1^- + R_2^+, X_1^- + X_2^-]$        | (0, 1, 1) |
| $[(\bullet)^{2T}, 2A_3^+, M_3^+ + M_3^-, Z_3^+ + Z_4^+, R_1^- + R_2^+, X_1^+ + X_2^+]$        | (0, 3, 3) |
| $[(\bullet)^{2T}, A_2^- + A_3^+, M_2^- + M_3^-, Z_3^+ + Z_4^+, 2R_2^+, X_2^+ + X_2^-]$        | (3, 0, 1) |
| $[(\bullet)^{2T}, A_2^- + A_3^+, M_2^- + M_3^-, Z_3^+ + Z_4^+, R_1^- + R_2^+, X_1^- + X_2^-]$ | (1, 2, 1) |
| $[(\bullet)^{2T}, A_2^- + A_3^+, M_2^- + M_3^-, Z_3^+ + Z_4^+, R_1^- + R_2^+, X_1^+ + X_2^+]$ | (1, 0, 3) |
| $[(\bullet)^{2T}, A_1^- + A_3^+, M_1^- + M_3^-, Z_3^+ + Z_4^+, 2R_2^+, X_2^+ + X_2^-]$        | (1, 2, 1) |
| $[(\bullet)^{2T}, A_1^- + A_3^+, M_1^- + M_3^-, Z_3^+ + Z_4^+, R_1^- + R_2^+, X_1^- + X_2^-]$ | (3, 0, 1) |
| $[(\bullet)^{2T}, A_1^- + A_3^+, M_1^- + M_3^-, Z_3^+ + Z_4^+, R_1^- + R_2^+, X_1^+ + X_2^+]$ | (3, 2, 3) |
| $[(\bullet)^{2T}, 2A_3^+, M_3^+ + M_3^-, Z_3^+ + Z_4^+, 2R_1^-, X_1^+ + X_1^-]$               | (2, 1, 3) |
| $[(\bullet)^{2T}, A_2^- + A_3^+, M_2^- + M_3^-, Z_3^+ + Z_4^+, 2R_1^-, X_1^+ + X_1^-]$        | (3, 2, 3) |
| $[(\bullet)^{2T}, A_1^- + A_3^+, M_1^- + M_3^-, Z_3^+ + Z_4^+, 2R_1^-, X_1^+ + X_1^-]$        | (1, 0, 3) |
| $[(\bullet)^{2T}, A_2^- + A_3^+, M_2^+ + M_3^+, Z_3^+ + Z_4^+, 2R_2^+, X_2^+ + X_2^-]$        | (3, 3, 0) |
| $[(\bullet)^{2T}, A_2^- + A_3^+, M_2^+ + M_3^+, Z_3^+ + Z_4^+, R_1^- + R_2^+, X_1^+ + X_2^+]$ | (1, 3, 2) |
| $[(\bullet)^{2T}, A_1^- + A_3^+, M_1^+ + M_3^+, Z_3^+ + Z_4^+, 2R_2^+, X_2^+ + X_2^-]$        | (1, 3, 2) |
| $[(\bullet)^{2T}, A_1^- + A_3^+, M_1^+ + M_3^+, Z_3^+ + Z_4^+, R_1^- + R_2^+, X_1^+ + X_2^+]$ | (3, 3, 0) |
| $[(\bullet)^{2T}, A_2^- + A_3^+, M_2^+ + M_3^+, Z_3^+ + Z_4^+, R_1^- + R_2^+, X_1^- + X_2^-]$ | (1, 1, 0) |
| $[(\bullet)^{2T}, A_2^- + A_3^+, M_2^+ + M_3^+, Z_3^+ + Z_4^+, 2R_1^-, X_1^+ + X_1^-]$        | (3, 1, 2) |
| $[(\bullet)^{2T}, A_1^- + A_3^+, M_1^+ + M_3^+, Z_3^+ + Z_4^+, R_1^- + R_2^+, X_1^- + X_2^-]$ | (3, 1, 2) |
| $[(\bullet)^{2T}, A_1^- + A_3^+, M_1^+ + M_3^+, Z_3^+ + Z_4^+, 2R_1^-, X_1^+ + X_1^-]$        | (1, 1, 0) |
| $[(\bullet)^{2T}, 2A_2^-, M_2^+ + M_2^-, Z_3^+ + Z_4^+, 2R_2^+, X_2^+ + X_2^-]$               | trivial   |
| $[(\bullet)^{2T}, 2A_2^-, M_2^+ + M_2^-, Z_3^+ + Z_4^+, R_1^- + R_2^+, X_1^- + X_2^-]$        | (2, 2, 0) |
| $[(\bullet)^{2T}, 2A_2^-, M_2^+ + M_2^-, Z_3^+ + Z_4^+, R_1^- + R_2^+, X_1^+ + X_2^+]$        | (2, 0, 2) |
| $[(\bullet)^{2T}, A_1^- + A_2^-, M_1^- + M_2^-, Z_3^+ + Z_4^+, 2R_2^+, X_2^+ + X_2^-]$        | (2, 2, 0) |
| $[(\bullet)^{2T}, A_1^- + A_2^-, M_1^- + M_2^-, Z_3^+ + Z_4^+, R_1^- + R_2^+, X_1^- + X_2^-]$ | trivial   |
| $[(\bullet)^{2T}, A_1^- + A_2^-, M_1^- + M_2^-, Z_3^+ + Z_4^+, R_1^- + R_2^+, X_1^+ + X_2^+]$ | (0, 2, 2) |

... continued on next page

... continued from previous page

|                                                                                                    |           |
|----------------------------------------------------------------------------------------------------|-----------|
| $[(\blacksquare)^{2T}, 2A_2^-, M_2^+ + M_2^-, Z_3^+ + Z_4^+, 2R_1^-, X_1^+ + X_1^-]$               | (0, 2, 2) |
| $[(\blacksquare)^{2T}, A_1^- + A_2^-, M_1^- + M_2^+, Z_3^+ + Z_4^+, 2R_1^-, X_1^+ + X_1^-]$        | (2, 0, 2) |
| $[(\blacksquare)^{2T}, A_1^- + A_2^-, M_1^+ + M_2^-, Z_3^+ + Z_4^+, 2R_2^+, X_2^+ + X_2^-]$        | (2, 0, 2) |
| $[(\blacksquare)^{2T}, A_1^- + A_2^-, M_1^+ + M_2^-, Z_3^+ + Z_4^+, R_1^- + R_2^+, X_1^+ + X_2^-]$ | trivial   |
| $[(\blacksquare)^{2T}, A_1^- + A_2^-, M_1^+ + M_2^-, Z_3^+ + Z_4^+, R_1^- + R_2^+, X_1^- + X_2^-]$ | (0, 2, 2) |
| $[(\blacksquare)^{2T}, A_1^- + A_2^-, M_1^+ + M_2^-, Z_3^+ + Z_4^+, 2R_1^-, X_1^+ + X_1^-]$        | (2, 2, 0) |
| $[(\blacksquare)^{2T}, 2A_1^-, M_1^+ + M_1^-, Z_3^+ + Z_4^+, 2R_2^+, X_2^+ + X_2^-]$               | (0, 2, 2) |
| $[(\blacksquare)^{2T}, 2A_1^-, M_1^+ + M_1^-, Z_3^+ + Z_4^+, R_1^- + R_2^+, X_1^- + X_2^-]$        | (2, 0, 2) |
| $[(\blacksquare)^{2T}, 2A_1^-, M_1^+ + M_1^-, Z_3^+ + Z_4^+, R_1^- + R_2^+, X_1^+ + X_2^+]$        | (2, 2, 0) |
| $[(\blacksquare)^{2T}, 2A_1^-, M_1^+ + M_1^-, Z_3^+ + Z_4^+, 2R_1^-, X_1^+ + X_1^-]$               | trivial   |

2nd minimal solution:  $\mu_2^T = 3$  (39040 symmetry vectors)

Space group 84 ( $\mathbb{Z}_2 \times \mathbb{Z}_4$ )

1st minimal solution:  $\mu_1^T = 2$  (24 symmetry vectors)

| $\mathbf{n}^T$                                                                 | $\mathbf{v}^T \in \mathbb{Z}_2 \times \mathbb{Z}_4$ |
|--------------------------------------------------------------------------------|-----------------------------------------------------|
| $[(\blacksquare)^{2T}, A_2, M_3^+ + M_4^-, Z_2, R_2^+ + R_2^-, X_2^+ + X_2^-]$ | (1, 3)                                              |
| $[(\blacksquare)^{2T}, A_2, M_3^+ + M_4^-, Z_2, R_1^- + R_2^-, X_1^- + X_2^-]$ | (0, 1)                                              |
| $[(\blacksquare)^{2T}, A_2, M_3^+ + M_4^-, Z_2, R_1^+ + R_2^+, X_1^- + X_2^-]$ | (0, 1)                                              |
| $[(\blacksquare)^{2T}, A_2, M_3^+ + M_4^-, Z_2, R_1^+ + R_2^+, X_1^+ + X_2^+]$ | (0, 3)                                              |
| $[(\blacksquare)^{2T}, A_2, M_3^+ + M_4^-, Z_2, R_1^+ + R_1^-, X_1^+ + X_1^-]$ | (1, 1)                                              |
| $[(\blacksquare)^{2T}, A_2, M_3^- + M_4^+, Z_2, R_1^- + R_2^-, X_1^+ + X_2^+]$ | (0, 1)                                              |
| $[(\blacksquare)^{2T}, A_2, M_3^- + M_4^+, Z_2, R_2^+ + R_2^-, X_2^+ + X_2^-]$ | (1, 1)                                              |
| $[(\blacksquare)^{2T}, A_2, M_3^- + M_4^+, Z_2, R_1^- + R_2^-, X_1^+ + X_2^+]$ | (0, 3)                                              |
| $[(\blacksquare)^{2T}, A_2, M_3^- + M_4^+, Z_2, R_1^- + R_2^-, X_1^- + X_2^-]$ | (0, 3)                                              |
| $[(\blacksquare)^{2T}, A_2, M_3^- + M_4^+, Z_2, R_1^+ + R_2^+, X_1^+ + X_2^+]$ | (0, 1)                                              |
| $[(\blacksquare)^{2T}, A_2, M_3^- + M_4^+, Z_2, R_1^+ + R_1^-, X_1^+ + X_1^-]$ | (1, 3)                                              |
| $[(\blacksquare)^{2T}, A_2, M_3^- + M_4^+, Z_2, R_1^+ + R_2^+, X_1^- + X_2^-]$ | (0, 3)                                              |
| $[(\blacksquare)^{2T}, A_1, M_1^+ + M_2^-, Z_2, R_1^- + R_2^-, X_1^+ + X_2^+]$ | trivial                                             |
| $[(\blacksquare)^{2T}, A_1, M_1^+ + M_2^-, Z_2, R_2^+ + R_2^-, X_2^+ + X_2^-]$ | (1, 0)                                              |
| $[(\blacksquare)^{2T}, A_1, M_1^- + M_2^+, Z_2, R_1^- + R_2^-, X_1^+ + X_2^+]$ | (0, 2)                                              |
| $[(\blacksquare)^{2T}, A_1, M_1^- + M_2^+, Z_2, R_2^+ + R_2^-, X_2^+ + X_2^-]$ | (1, 2)                                              |
| $[(\blacksquare)^{2T}, A_1, M_1^- + M_2^+, Z_2, R_1^- + R_2^-, X_1^- + X_2^-]$ | (0, 2)                                              |
| $[(\blacksquare)^{2T}, A_1, M_1^- + M_2^+, Z_2, R_1^- + R_2^-, X_1^- + X_2^-]$ | trivial                                             |
| $[(\blacksquare)^{2T}, A_1, M_1^+ + M_2^-, Z_2, R_1^+ + R_2^+, X_1^+ + X_2^+]$ | trivial                                             |
| $[(\blacksquare)^{2T}, A_1, M_1^- + M_2^+, Z_2, R_1^+ + R_2^+, X_1^+ + X_2^+]$ | (0, 2)                                              |
| $[(\blacksquare)^{2T}, A_1, M_1^+ + M_2^-, Z_2, R_1^+ + R_1^-, X_1^+ + X_1^-]$ | (1, 2)                                              |
| $[(\blacksquare)^{2T}, A_1, M_1^+ + M_2^-, Z_2, R_1^+ + R_2^+, X_1^- + X_2^-]$ | (0, 2)                                              |
| $[(\blacksquare)^{2T}, A_1, M_1^- + M_2^+, Z_2, R_1^+ + R_1^-, X_1^+ + X_1^-]$ | (1, 0)                                              |
| $[(\blacksquare)^{2T}, A_1, M_1^- + M_2^+, Z_2, R_1^+ + R_2^+, X_1^- + X_2^-]$ | trivial                                             |

2nd minimal solution:  $\mu_2^T = 4$  (1424 symmetry vectors)

Space group 85 ( $\mathbb{Z}_2 \times \mathbb{Z}_4$ )

1st minimal solution:  $\mu_1^T = 2$  (4 symmetry vectors & filling-enforced topology)

| $\mathbf{n}^T$                                             | $\mathbf{v}^T \in \mathbb{Z}_2 \times \mathbb{Z}_4$ |
|------------------------------------------------------------|-----------------------------------------------------|
| $[(\blacksquare)^{2T}, A_2, M_2, Z_3^+ + Z_4^-, R_1, X_1]$ | (1, 2)                                              |
| $[(\blacksquare)^{2T}, A_1, M_1, Z_3^+ + Z_4^-, R_1, X_1]$ | (1, 0)                                              |
| $[(\blacksquare)^{2T}, A_2, M_2, Z_3^- + Z_4^+, R_1, X_1]$ | (1, 2)                                              |
| $[(\blacksquare)^{2T}, A_1, M_1, Z_3^- + Z_4^+, R_1, X_1]$ | (1, 0)                                              |

2nd minimal solution:  $\mu_2^T = 4$  (186 symmetry vectors)

Space group 86 ( $\mathbb{Z}_2 \times \mathbb{Z}_2$ )

1st minimal solution:  $\mu_1^T = 2$  (4 symmetry vectors & filling-enforced topology)

| $\mathbf{n}^T$                                             | $\mathbf{v}^T \in \mathbb{Z}_2 \times \mathbb{Z}_2$ |
|------------------------------------------------------------|-----------------------------------------------------|
| $[(\blacksquare)^{2T}, A_3^- + A_4^+, M_2, Z_2, R_1, X_1]$ | (1, 0)                                              |
| $[(\blacksquare)^{2T}, A_3^+ + A_4^-, M_2, Z_2, R_1, X_1]$ | (1, 0)                                              |
| $[(\blacksquare)^{2T}, A_1^- + A_2^+, M_1, Z_2, R_1, X_1]$ | (1, 1)                                              |
| $[(\blacksquare)^{2T}, A_1^+ + A_2^-, M_1, Z_2, R_1, X_1]$ | (1, 1)                                              |

2nd minimal solution:  $\mu_2^T = 4$  (48 symmetry vectors)

Space group 87 ( $\mathbb{Z}_4 \times \mathbb{Z}_4$ )

1st minimal solution:  $\mu_1^T = 2$  (84 symmetry vectors & filling-enforced topology)

| $\mathbf{n}^T$                                                                  | $\mathbf{v}^T \in \mathbb{Z}_4 \times \mathbb{Z}_4$ |
|---------------------------------------------------------------------------------|-----------------------------------------------------|
| $[(\blacksquare)^{2T}, M_3^+ + M_4^-, P_2 + P_4, X_1^+ + X_2^+, 2N_1^-]$        | (0, 1)                                              |
| $[(\blacksquare)^{2T}, M_3^+ + M_4^-, 2P_4, X_2^+ + X_2^-, 2N_1^-]$             | (1, 2)                                              |
| $[(\blacksquare)^{2T}, M_3^+ + M_4^-, P_2 + P_3, X_1^+ + X_2^+, 2N_1^-]$        | (2, 3)                                              |
| $[(\blacksquare)^{2T}, M_3^+ + M_4^-, P_3 + P_4, X_2^+ + X_2^-, 2N_1^-]$        | (3, 0)                                              |
| $[(\blacksquare)^{2T}, M_3^+ + M_4^-, 2P_3, X_2^+ + X_2^-, 2N_1^-]$             | (1, 2)                                              |
| $[(\blacksquare)^{2T}, M_3^+ + M_4^-, 2P_2, X_1^+ + X_1^-, 2N_1^-]$             | (1, 0)                                              |
| $[(\blacksquare)^{2T}, M_3^+ + M_4^-, P_2 + P_4, X_1^- + X_2^-, 2N_1^-]$        | (2, 1)                                              |
| $[(\blacksquare)^{2T}, M_3^+ + M_4^-, P_2 + P_3, X_1^- + X_2^-, 2N_1^-]$        | (0, 3)                                              |
| $[(\blacksquare)^{2T}, M_3^+ + M_4^-, P_2 + P_4, X_1^+ + X_2^-, N_1^+ + N_1^-]$ | (2, 3)                                              |
| $[(\blacksquare)^{2T}, M_3^+ + M_4^-, 2P_4, X_2^+ + X_2^-, N_1^+ + N_1^-]$      | (3, 0)                                              |
| $[(\blacksquare)^{2T}, M_3^+ + M_4^-, P_2 + P_3, X_1^+ + X_2^-, N_1^+ + N_1^-]$ | (0, 1)                                              |
| $[(\blacksquare)^{2T}, M_3^+ + M_4^-, P_3 + P_4, X_2^+ + X_2^-, N_1^+ + N_1^-]$ | (1, 2)                                              |
| $[(\blacksquare)^{2T}, M_3^+ + M_4^-, 2P_3, X_2^+ + X_2^-, N_1^+ + N_1^-]$      | (3, 0)                                              |
| $[(\blacksquare)^{2T}, M_3^+ + M_4^-, 2P_2, X_1^+ + X_1^-, N_1^+ + N_1^-]$      | (3, 2)                                              |
| $[(\blacksquare)^{2T}, M_3^+ + M_4^-, P_2 + P_4, X_1^- + X_2^-, N_1^+ + N_1^-]$ | (0, 3)                                              |
| $[(\blacksquare)^{2T}, M_3^+ + M_4^-, P_2 + P_3, X_1^- + X_2^-, N_1^+ + N_1^-]$ | (2, 1)                                              |
| $[(\blacksquare)^{2T}, M_3^+ + M_4^-, P_2 + P_4, X_1^+ + X_2^-, 2N_1^+]$        | (0, 1)                                              |
| $[(\blacksquare)^{2T}, M_3^+ + M_4^-, 2P_4, X_2^+ + X_2^-, 2N_1^+]$             | (1, 2)                                              |
| $[(\blacksquare)^{2T}, M_3^+ + M_4^-, P_2 + P_3, X_1^+ + X_2^-, 2N_1^+]$        | (2, 3)                                              |
| $[(\blacksquare)^{2T}, M_3^+ + M_4^-, P_3 + P_4, X_2^+ + X_2^-, 2N_1^+]$        | (3, 0)                                              |
| $[(\blacksquare)^{2T}, M_3^+ + M_4^-, 2P_3, X_2^+ + X_2^-, 2N_1^+]$             | (1, 2)                                              |
| $[(\blacksquare)^{2T}, M_3^+ + M_4^-, 2P_2, X_1^+ + X_1^-, 2N_1^+]$             | (1, 0)                                              |
| $[(\blacksquare)^{2T}, M_3^+ + M_4^-, P_2 + P_4, X_1^- + X_2^-, 2N_1^+]$        | (2, 1)                                              |

... continued on next page

... continued from previous page

|                                                                                 |        |
|---------------------------------------------------------------------------------|--------|
| $[(\blacksquare)^{2T}, M_3^+ + M_4^-, P_2 + P_3, X_1^- + X_2^-, 2N_1^+]$        | (0, 3) |
| $[(\blacksquare)^{2T}, M_3^+ + M_4^-, P_1 + P_4, X_1^+ + X_2^+, 2N_1^-]$        | (2, 3) |
| $[(\blacksquare)^{2T}, M_3^+ + M_4^-, P_1 + P_3, X_1^+ + X_2^+, 2N_1^-]$        | (0, 1) |
| $[(\blacksquare)^{2T}, M_3^+ + M_4^-, P_1 + P_2, X_1^+ + X_1^-, 2N_1^-]$        | (3, 2) |
| $[(\blacksquare)^{2T}, M_3^+ + M_4^-, P_1 + P_4, X_1^- + X_2^-, 2N_1^-]$        | (0, 3) |
| $[(\blacksquare)^{2T}, M_3^+ + M_4^-, P_1 + P_3, X_1^- + X_2^-, 2N_1^-]$        | (2, 1) |
| $[(\blacksquare)^{2T}, M_3^+ + M_4^-, P_1 + P_4, X_1^+ + X_2^+, N_1^+ + N_1^-]$ | (0, 1) |
| $[(\blacksquare)^{2T}, M_3^+ + M_4^-, P_1 + P_3, X_1^+ + X_2^+, N_1^+ + N_1^-]$ | (2, 3) |
| $[(\blacksquare)^{2T}, M_3^+ + M_4^-, P_1 + P_2, X_1^+ + X_1^-, N_1^+ + N_1^-]$ | (1, 0) |
| $[(\blacksquare)^{2T}, M_3^+ + M_4^-, P_1 + P_4, X_1^- + X_2^-, N_1^+ + N_1^-]$ | (2, 1) |
| $[(\blacksquare)^{2T}, M_3^+ + M_4^-, P_1 + P_3, X_1^- + X_2^-, N_1^+ + N_1^-]$ | (0, 3) |
| $[(\blacksquare)^{2T}, M_3^+ + M_4^-, P_1 + P_4, X_1^+ + X_2^+, 2N_1^+]$        | (2, 3) |
| $[(\blacksquare)^{2T}, M_3^+ + M_4^-, P_1 + P_3, X_1^+ + X_2^+, 2N_1^+]$        | (0, 1) |
| $[(\blacksquare)^{2T}, M_3^+ + M_4^-, P_1 + P_2, X_1^+ + X_1^-, 2N_1^+]$        | (3, 2) |
| $[(\blacksquare)^{2T}, M_3^+ + M_4^-, P_1 + P_4, X_1^- + X_2^-, 2N_1^+]$        | (0, 3) |
| $[(\blacksquare)^{2T}, M_3^+ + M_4^-, P_1 + P_3, X_1^- + X_2^-, 2N_1^+]$        | (2, 1) |
| $[(\blacksquare)^{2T}, M_3^+ + M_4^-, 2P_1, X_1^+ + X_1^-, 2N_1^-]$             | (1, 0) |
| $[(\blacksquare)^{2T}, M_3^+ + M_4^-, 2P_1, X_1^+ + X_1^-, N_1^+ + N_1^-]$      | (3, 2) |
| $[(\blacksquare)^{2T}, M_3^+ + M_4^-, 2P_1, X_1^+ + X_1^-, 2N_1^+]$             | (1, 0) |
| $[(\blacksquare)^{2T}, M_3^- + M_4^+, P_2 + P_4, X_1^+ + X_2^+, 2N_1^-]$        | (2, 1) |
| $[(\blacksquare)^{2T}, M_3^- + M_4^+, 2P_4, X_2^+ + X_2^-, 2N_1^-]$             | (3, 2) |
| $[(\blacksquare)^{2T}, M_3^- + M_4^+, P_2 + P_3, X_1^+ + X_2^+, 2N_1^-]$        | (0, 3) |
| $[(\blacksquare)^{2T}, M_3^- + M_4^+, P_3 + P_4, X_2^+ + X_2^-, 2N_1^-]$        | (1, 0) |
| $[(\blacksquare)^{2T}, M_3^- + M_4^+, 2P_3, X_2^+ + X_2^-, 2N_1^-]$             | (3, 2) |
| $[(\blacksquare)^{2T}, M_3^- + M_4^+, 2P_2, X_1^+ + X_1^-, 2N_1^-]$             | (3, 0) |
| $[(\blacksquare)^{2T}, M_3^- + M_4^+, P_2 + P_4, X_1^- + X_2^-, 2N_1^-]$        | (0, 1) |
| $[(\blacksquare)^{2T}, M_3^- + M_4^+, P_2 + P_3, X_1^- + X_2^-, 2N_1^-]$        | (2, 3) |
| $[(\blacksquare)^{2T}, M_3^- + M_4^+, P_2 + P_4, X_1^+ + X_2^+, N_1^+ + N_1^-]$ | (0, 3) |
| $[(\blacksquare)^{2T}, M_3^- + M_4^+, 2P_4, X_2^+ + X_2^-, N_1^+ + N_1^-]$      | (1, 0) |
| $[(\blacksquare)^{2T}, M_3^- + M_4^+, P_2 + P_3, X_1^+ + X_2^+, N_1^+ + N_1^-]$ | (2, 1) |
| $[(\blacksquare)^{2T}, M_3^- + M_4^+, P_3 + P_4, X_2^+ + X_2^-, N_1^+ + N_1^-]$ | (3, 2) |
| $[(\blacksquare)^{2T}, M_3^- + M_4^+, 2P_3, X_2^+ + X_2^-, N_1^+ + N_1^-]$      | (1, 0) |
| $[(\blacksquare)^{2T}, M_3^- + M_4^+, 2P_2, X_1^+ + X_1^-, N_1^+ + N_1^-]$      | (1, 2) |
| $[(\blacksquare)^{2T}, M_3^- + M_4^+, P_2 + P_4, X_1^- + X_2^-, N_1^+ + N_1^-]$ | (2, 3) |
| $[(\blacksquare)^{2T}, M_3^- + M_4^+, P_2 + P_3, X_1^- + X_2^-, N_1^+ + N_1^-]$ | (0, 1) |
| $[(\blacksquare)^{2T}, M_3^- + M_4^+, P_2 + P_4, X_1^+ + X_2^+, 2N_1^+]$        | (2, 1) |
| $[(\blacksquare)^{2T}, M_3^- + M_4^+, 2P_4, X_2^+ + X_2^-, 2N_1^+]$             | (3, 2) |
| $[(\blacksquare)^{2T}, M_3^- + M_4^+, P_2 + P_3, X_1^+ + X_2^+, 2N_1^+]$        | (0, 3) |
| $[(\blacksquare)^{2T}, M_3^- + M_4^+, P_3 + P_4, X_2^+ + X_2^-, 2N_1^+]$        | (1, 0) |
| $[(\blacksquare)^{2T}, M_3^- + M_4^+, 2P_3, X_2^+ + X_2^-, 2N_1^+]$             | (3, 2) |
| $[(\blacksquare)^{2T}, M_3^- + M_4^+, 2P_2, X_1^+ + X_1^-, 2N_1^+]$             | (3, 0) |
| $[(\blacksquare)^{2T}, M_3^- + M_4^+, P_2 + P_4, X_1^- + X_2^-, 2N_1^+]$        | (0, 1) |
| $[(\blacksquare)^{2T}, M_3^- + M_4^+, P_2 + P_3, X_1^- + X_2^-, 2N_1^+]$        | (2, 3) |
| $[(\blacksquare)^{2T}, M_3^- + M_4^+, P_1 + P_4, X_1^+ + X_2^+, 2N_1^-]$        | (0, 3) |
| $[(\blacksquare)^{2T}, M_3^- + M_4^+, P_1 + P_3, X_1^+ + X_2^+, 2N_1^-]$        | (2, 1) |
| $[(\blacksquare)^{2T}, M_3^- + M_4^+, P_1 + P_2, X_1^+ + X_1^-, 2N_1^-]$        | (1, 2) |
| $[(\blacksquare)^{2T}, M_3^- + M_4^+, P_1 + P_4, X_1^- + X_2^-, 2N_1^-]$        | (2, 3) |
| $[(\blacksquare)^{2T}, M_3^- + M_4^+, P_1 + P_3, X_1^- + X_2^-, 2N_1^-]$        | (0, 1) |
| $[(\blacksquare)^{2T}, M_3^- + M_4^+, P_1 + P_4, X_1^+ + X_2^+, N_1^+ + N_1^-]$ | (2, 1) |
| $[(\blacksquare)^{2T}, M_3^- + M_4^+, P_1 + P_3, X_1^+ + X_2^+, N_1^+ + N_1^-]$ | (0, 3) |
| $[(\blacksquare)^{2T}, M_3^- + M_4^+, P_1 + P_2, X_1^+ + X_1^-, N_1^+ + N_1^-]$ | (3, 0) |
| $[(\blacksquare)^{2T}, M_3^- + M_4^+, P_1 + P_4, X_1^- + X_2^-, N_1^+ + N_1^-]$ | (0, 1) |
| $[(\blacksquare)^{2T}, M_3^- + M_4^+, P_1 + P_3, X_1^- + X_2^-, N_1^+ + N_1^-]$ | (2, 3) |
| $[(\blacksquare)^{2T}, M_3^- + M_4^+, P_1 + P_4, X_1^+ + X_2^+, 2N_1^+]$        | (0, 3) |

... continued on next page

... continued from previous page

|                                                                            |        |
|----------------------------------------------------------------------------|--------|
| $[(\blacksquare)^{2T}, M_3^- + M_4^+, P_1 + P_3, X_1^+ + X_2^+, 2N_1^+]$   | (2, 1) |
| $[(\blacksquare)^{2T}, M_3^- + M_4^+, P_1 + P_2, X_1^+ + X_1^-, 2N_1^+]$   | (1, 2) |
| $[(\blacksquare)^{2T}, M_3^- + M_4^+, P_1 + P_4, X_1^- + X_2^-, 2N_1^+]$   | (2, 3) |
| $[(\blacksquare)^{2T}, M_3^- + M_4^+, P_1 + P_3, X_1^- + X_2^-, 2N_1^+]$   | (0, 1) |
| $[(\blacksquare)^{2T}, M_3^- + M_4^+, 2P_1, X_1^+ + X_1^-, 2N_1^-]$        | (3, 0) |
| $[(\blacksquare)^{2T}, M_3^- + M_4^+, 2P_1, X_1^+ + X_1^-, N_1^+ + N_1^-]$ | (1, 2) |
| $[(\blacksquare)^{2T}, M_3^- + M_4^+, 2P_1, X_1^+ + X_1^-, 2N_1^+]$        | (3, 0) |

2nd minimal solution:  $\mu_2^T = 3$  (2560 symmetry vectors)

Space group 88 ( $\mathbb{Z}_2 \times \mathbb{Z}_2$ )

1st minimal solution:  $\mu_1^T = 2$  (12 symmetry vectors)

| $\mathbf{n}^T$                                              | $\mathbf{v}^T \in \mathbb{Z}_2 \times \mathbb{Z}_2$ |
|-------------------------------------------------------------|-----------------------------------------------------|
| $[(\blacksquare)^{2T}, M_2, P_2 + P_4, X_1, 2N_1^-]$        | (1, 0)                                              |
| $[(\blacksquare)^{2T}, M_2, P_2 + P_4, X_1, N_1^+ + N_1^-]$ | (1, 1)                                              |
| $[(\blacksquare)^{2T}, M_2, P_2 + P_4, X_1, 2N_1^+]$        | (1, 0)                                              |
| $[(\blacksquare)^{2T}, M_2, P_1 + P_4, X_1, 2N_1^-]$        | trivial                                             |
| $[(\blacksquare)^{2T}, M_2, P_1 + P_4, X_1, N_1^+ + N_1^-]$ | (0, 1)                                              |
| $[(\blacksquare)^{2T}, M_2, P_1 + P_4, X_1, 2N_1^+]$        | trivial                                             |
| $[(\blacksquare)^{2T}, M_2, P_2 + P_3, X_1, 2N_1^-]$        | trivial                                             |
| $[(\blacksquare)^{2T}, M_2, P_2 + P_3, X_1, N_1^+ + N_1^-]$ | (0, 1)                                              |
| $[(\blacksquare)^{2T}, M_2, P_2 + P_3, X_1, 2N_1^+]$        | trivial                                             |
| $[(\blacksquare)^{2T}, M_2, P_1 + P_3, X_1, 2N_1^-]$        | (1, 0)                                              |
| $[(\blacksquare)^{2T}, M_2, P_1 + P_3, X_1, N_1^+ + N_1^-]$ | (1, 1)                                              |
| $[(\blacksquare)^{2T}, M_2, P_1 + P_3, X_1, 2N_1^+]$        | (1, 0)                                              |

2nd minimal solution:  $\mu_2^T = 4$  (180 symmetry vectors)

Space group 89 ( $\mathbb{Z}_1$ )

1st minimal solution:  $\mu_1^T = 2$  (4 symmetry vectors)

| $\mathbf{n}^T$                                                           |
|--------------------------------------------------------------------------|
| $[(\blacksquare)^{2T}, A_2 + A_4, 2M_2, Z_5, R_3 + R_4, 2X_3]$           |
| $[(\blacksquare)^{2T}, A_3 + A_4, M_2 + M_3, Z_5, R_2 + R_4, X_2 + X_3]$ |
| $[(\blacksquare)^{2T}, A_1 + A_2, M_2 + M_3, Z_5, R_1 + R_3, X_2 + X_3]$ |
| $[(\blacksquare)^{2T}, A_1 + A_3, 2M_3, Z_5, R_1 + R_2, 2X_2]$           |

2nd minimal solution:  $\mu_2^T = 3$  (84 symmetry vectors)

Space group 90 ( $\mathbb{Z}_1$ )

1st minimal solution:  $\mu_1^T = 4$  (13 symmetry vectors)

| $\mathbf{n}^T$                                                                                                 |
|----------------------------------------------------------------------------------------------------------------|
| $[(\blacksquare)^{2T} + 2\Gamma_1, 2A_5, 2M_5, Z_1 + Z_3 + Z_5, 2R_1, 2X_1]$                                   |
| $[(\blacksquare)^{2T} + \Gamma_1 + \Gamma_2, A_2 + A_3 + A_5, M_2 + M_3 + M_5, Z_2 + Z_3 + Z_5, 2R_1, 2X_1]$   |
| $[(\blacksquare)^{2T} + 2\Gamma_1, A_2 + A_4 + A_5, M_2 + M_4 + M_5, Z_1 + Z_3 + Z_5, 2R_1, 2X_1]$             |
| $[(\blacksquare)^{2T} + \Gamma_1 + \Gamma_2, A_1 + A_4 + A_5, M_2 + M_3 + M_5, Z_1 + Z_4 + Z_5, 2R_1, 2X_1]$   |
| $[(\blacksquare)^{2T} + 2\Gamma_1, A_1 + A_3 + A_5, M_1 + M_3 + M_5, Z_1 + Z_3 + Z_5, 2R_1, 2X_1]$             |
| $[(\blacksquare)^{2T} + \Gamma_1 + \Gamma_2, 2A_2 + A_3 + A_4, 2M_2 + M_3 + M_4, Z_2 + Z_3 + Z_5, 2R_1, 2X_1]$ |
| $[(\blacksquare)^{2T} + 2\Gamma_2, A_1 + A_2 + A_3 + A_4, 2M_2 + 2M_3, Z_2 + Z_4 + Z_5, 2R_1, 2X_1]$           |
| $[(\blacksquare)^{2T} + \Gamma_1 + \Gamma_2, A_1 + A_2 + 2A_3, M_1 + M_2 + 2M_3, Z_2 + Z_3 + Z_5, 2R_1, 2X_1]$ |
| $[(\blacksquare)^{2T} + 2\Gamma_1, 2A_2 + 2A_4, 2M_2 + 2M_4, Z_1 + Z_3 + Z_5, 2R_1, 2X_1]$                     |
| $[(\blacksquare)^{2T} + \Gamma_1 + \Gamma_2, A_1 + A_2 + 2A_4, 2M_2 + M_3 + M_4, Z_1 + Z_4 + Z_5, 2R_1, 2X_1]$ |
| $[(\blacksquare)^{2T} + 2\Gamma_1, A_1 + A_2 + A_3 + A_4, M_1 + M_2 + M_3 + M_4, Z_1 + Z_3 + Z_5, 2R_1, 2X_1]$ |
| $[(\blacksquare)^{2T} + \Gamma_1 + \Gamma_2, 2A_1 + A_3 + A_4, M_1 + M_2 + 2M_3, Z_1 + Z_4 + Z_5, 2R_1, 2X_1]$ |
| $[(\blacksquare)^{2T} + 2\Gamma_1, 2A_1 + 2A_3, 2M_1 + 2M_3, Z_1 + Z_3 + Z_5, 2R_1, 2X_1]$                     |

2nd minimal solution:  $\mu_2^T = 6$  (101 symmetry vectors)

Space group 91 ( $\mathbb{Z}_1$ )

1st minimal solution:  $\mu_1^T = 4$  (4 symmetry vectors)

| $\mathbf{n}^T$                                                                                                    |
|-------------------------------------------------------------------------------------------------------------------|
| $[(\blacksquare)^{2T} + \Gamma_1 + \Gamma_4, A_1 + A_2, M_3 + M_4 + M_5, Z_1 + Z_2, 2R_1, 2X_2 + X_3 + X_4]$      |
| $[(\blacksquare)^{2T} + \Gamma_1 + \Gamma_2, A_1 + A_2, M_2 + M_3 + M_5, Z_1 + Z_2, 2R_1, X_1 + X_2 + X_3 + X_4]$ |
| $[(\blacksquare)^{2T} + \Gamma_1 + \Gamma_4, A_1 + A_2, M_1 + M_2 + M_5, Z_1 + Z_2, 2R_1, X_1 + X_2 + 2X_3]$      |
| $[(\blacksquare)^{2T} + \Gamma_3 + \Gamma_4, A_1 + A_2, M_2 + M_3 + M_5, Z_1 + Z_2, 2R_1, 2X_2 + 2X_3]$           |

2nd minimal solution:  $\mu_2^T = 8$  (16 symmetry vectors)

Space group 92 ( $\mathbb{Z}_1$ )

1st minimal solution:  $\mu_1^T = 4$  (1 symmetry vector)

| $\mathbf{n}^T$                                                                                                    |
|-------------------------------------------------------------------------------------------------------------------|
| $[(\blacksquare)^{2T} + \Gamma_1 + \Gamma_2, A_1 + A_2, M_2 + M_3 + M_5, Z_1 + Z_2, R_1 + R_2 + R_3 + R_4, 2X_1]$ |

2nd minimal solution:  $\mu_2^T = 8$  (2 symmetry vectors)

Space group 93 ( $\mathbb{Z}_1$ )

1st minimal solution:  $\mu_1^T = 2$  (2 symmetry vectors)

| $\mathbf{n}^T$                                                           |
|--------------------------------------------------------------------------|
| $[(\blacksquare)^{2T}, A_5, M_2 + M_3, Z_1 + Z_2, R_2 + R_3, X_2 + X_3]$ |
| $[(\blacksquare)^{2T}, A_5, M_2 + M_3, Z_3 + Z_4, R_1 + R_4, X_2 + X_3]$ |

2nd minimal solution:  $\mu_2^T = 4$  (104 symmetry vectors)

Space group 94 ( $\mathbb{Z}_1$ )

1st minimal solution:  $\mu_1^T = 4$  (2 symmetry vectors)

| $\mathbf{n}^T$                                                                                               |
|--------------------------------------------------------------------------------------------------------------|
| $[(\blacksquare)^{2T} + \Gamma_1 + \Gamma_2, A_2 + A_3 + A_5, M_2 + M_3 + M_5, Z_2 + Z_3 + Z_5, 2R_1, 2X_1]$ |
| $[(\blacksquare)^{2T} + \Gamma_1 + \Gamma_2, A_1 + A_4 + A_5, M_2 + M_3 + M_5, Z_1 + Z_4 + Z_5, 2R_1, 2X_1]$ |

2nd minimal solution:  $\mu_2^T = 6$  (10 symmetry vectors)

Space group 95 ( $\mathbb{Z}_1$ )

1st minimal solution:  $\mu_1^T = 4$  (4 symmetry vectors)

| $\mathbf{n}^T$                                                                                                    |
|-------------------------------------------------------------------------------------------------------------------|
| $[(\blacksquare)^{2T} + \Gamma_1 + \Gamma_4, A_1 + A_2, M_3 + M_4 + M_5, Z_1 + Z_2, 2R_1, 2X_2 + X_3 + X_4]$      |
| $[(\blacksquare)^{2T} + \Gamma_1 + \Gamma_2, A_1 + A_2, M_2 + M_3 + M_5, Z_1 + Z_2, 2R_1, X_1 + X_2 + X_3 + X_4]$ |
| $[(\blacksquare)^{2T} + \Gamma_1 + \Gamma_4, A_1 + A_2, M_1 + M_2 + M_5, Z_1 + Z_2, 2R_1, X_1 + X_2 + 2X_3]$      |
| $[(\blacksquare)^{2T} + \Gamma_3 + \Gamma_4, A_1 + A_2, M_2 + M_3 + M_5, Z_1 + Z_2, 2R_1, 2X_2 + 2X_3]$           |

2nd minimal solution:  $\mu_2^T = 8$  (16 symmetry vectors)

Space group 96 ( $\mathbb{Z}_1$ )

1st minimal solution:  $\mu_1^T = 4$  (1 symmetry vector)

| $\mathbf{n}^T$                                                                                                    |
|-------------------------------------------------------------------------------------------------------------------|
| $[(\blacksquare)^{2T} + \Gamma_1 + \Gamma_2, A_1 + A_2, M_2 + M_3 + M_5, Z_1 + Z_2, R_1 + R_2 + R_3 + R_4, 2X_1]$ |

2nd minimal solution:  $\mu_2^T = 8$  (2 symmetry vectors)

Space group 97 ( $\mathbb{Z}_1$ )

1st minimal solution:  $\mu_1^T = 3$  (8 symmetry vectors)

| $\mathbf{n}^T$                                                                              |
|---------------------------------------------------------------------------------------------|
| $[(\blacksquare)^{2T} + \Gamma_1, M_3 + M_5, 3P_2, X_1 + 2X_2, 3N_2]$                       |
| $[(\blacksquare)^{2T} + \Gamma_1, M_3 + M_5, P_1 + 2P_2, X_1 + 2X_2, N_1 + 2N_2]$           |
| $[(\blacksquare)^{2T} + \Gamma_1, M_3 + M_5, 2P_1 + P_2, X_1 + 2X_2, 2N_1 + N_2]$           |
| $[(\blacksquare)^{2T} + \Gamma_2, M_4 + M_5, P_2 + P_3 + P_4, X_2 + 2X_4, N_1 + 2N_2]$      |
| $[(\blacksquare)^{2T} + \Gamma_1, M_3 + M_5, P_2 + P_3 + P_4, X_2 + X_3 + X_4, N_1 + 2N_2]$ |

... continued on next page

... continued from previous page

$$\begin{array}{l} [(\blacksquare)^{2T}, \Gamma_1, M_3 + M_5, P_1 + P_3 + P_4, X_2 + X_3 + X_4, 2N_1 + N_2] \\ [(\blacksquare)^{2T}, \Gamma_1, M_3 + M_5, 3P_1, X_1 + 2X_2, 3N_1] \\ [(\blacksquare)^{2T}, \Gamma_2, M_4 + M_5, P_1 + P_3 + P_4, X_2 + 2X_4, 2N_1 + N_2] \end{array}$$

2nd minimal solution:  $\mu_2^T = 4$  (48 symmetry vectors)

Space group 98 ( $\mathbb{Z}_1$ )

1st minimal solution:  $\mu_1^T = 2$  (1 symmetry vector)

$$\begin{array}{l} \mathbf{n}^T \\ [(\blacksquare)^{2T}, M_3 + M_4, P_1, X_2 + X_4, N_1 + N_2] \end{array}$$

2nd minimal solution:  $\mu_2^T = 4$  (6 symmetry vectors)

Space group 99 ( $\mathbb{Z}_1$ )

1st minimal solution:  $\mu_1^T = 2$  (8 symmetry vectors)

$$\begin{array}{l} \mathbf{n}^T \\ [(\blacksquare)^{2T}, A_5, M_5, Z_5, R_3 + R_4, X_3 + X_4] \\ [(\blacksquare)^{2T}, A_5, M_5, Z_5, R_1 + R_2, X_1 + X_2] \\ [(\blacksquare)^{2T}, A_2 + A_3, M_2 + M_3, Z_5, R_3 + R_4, X_3 + X_4] \\ [(\blacksquare)^{2T}, A_2 + A_3, M_2 + M_3, Z_5, R_1 + R_2, X_1 + X_2] \\ [(\blacksquare)^{2T}, A_3 + A_4, M_3 + M_4, Z_5, R_2 + R_3, X_2 + X_3] \\ [(\blacksquare)^{2T}, A_1 + A_2, M_1 + M_2, Z_5, R_1 + R_4, X_1 + X_4] \\ [(\blacksquare)^{2T}, A_1 + A_4, M_1 + M_4, Z_5, R_3 + R_4, X_3 + X_4] \\ [(\blacksquare)^{2T}, A_1 + A_4, M_1 + M_4, Z_5, R_1 + R_2, X_1 + X_2] \end{array}$$

2nd minimal solution:  $\mu_2^T = 3$  (56 symmetry vectors)

Space group 100 ( $\mathbb{Z}_1$ )

1st minimal solution:  $\mu_1^T = 2$  (3 symmetry vectors)

$$\begin{array}{l} \mathbf{n}^T \\ [(\blacksquare)^{2T}, A_5, M_5, Z_5, R_1, X_1] \\ [(\blacksquare)^{2T}, A_2 + A_3, M_2 + M_3, Z_5, R_1, X_1] \\ [(\blacksquare)^{2T}, A_1 + A_4, M_1 + M_4, Z_5, R_1, X_1] \end{array}$$

2nd minimal solution:  $\mu_2^T = 4$  (24 symmetry vectors)



Space group 101 ( $\mathbb{Z}_1$ )

1st minimal solution:  $\mu_1^T = 2$  (2 symmetry vectors)

| $\mathbf{n}^T$                                               |
|--------------------------------------------------------------|
| $[(\blacksquare)^{2T}, A_5, M_5, Z_5, R_3 + R_4, X_3 + X_4]$ |
| $[(\blacksquare)^{2T}, A_5, M_5, Z_5, R_1 + R_2, X_1 + X_2]$ |

2nd minimal solution:  $\mu_2^T = 4$  (12 symmetry vectors)

Space group 102 ( $\mathbb{Z}_1$ )

1st minimal solution:  $\mu_1^T = 2$  (1 symmetry vector)

| $\mathbf{n}^T$                                   |
|--------------------------------------------------|
| $[(\blacksquare)^{2T}, A_5, M_5, Z_5, R_1, X_1]$ |

2nd minimal solution:  $\mu_2^T = 4$  (4 symmetry vectors)

Space group 103 ( $\mathbb{Z}_2$ )

1st minimal solution:  $\mu_1^T = 2$  (6 symmetry vectors)

| $\mathbf{n}^T$                                                           | $\mathbf{v}^T \in \mathbb{Z}_2$ |
|--------------------------------------------------------------------------|---------------------------------|
| $[(\blacksquare)^{2T}, A_5, M_5, Z_5, R_3 + R_4, X_3 + X_4]$             | trivial                         |
| $[(\blacksquare)^{2T}, A_5, M_5, Z_5, R_1 + R_2, X_1 + X_2]$             | trivial                         |
| $[(\blacksquare)^{2T}, A_2 + A_3, M_2 + M_3, Z_5, R_3 + R_4, X_3 + X_4]$ | 1                               |
| $[(\blacksquare)^{2T}, A_2 + A_3, M_2 + M_3, Z_5, R_1 + R_2, X_1 + X_2]$ | 1                               |
| $[(\blacksquare)^{2T}, A_1 + A_4, M_1 + M_4, Z_5, R_3 + R_4, X_3 + X_4]$ | 1                               |
| $[(\blacksquare)^{2T}, A_1 + A_4, M_1 + M_4, Z_5, R_1 + R_2, X_1 + X_2]$ | 1                               |

2nd minimal solution:  $\mu_2^T = 4$  (54 symmetry vectors)

Space group 104 ( $\mathbb{Z}_2$ )

1st minimal solution:  $\mu_1^T = 2$  (3 symmetry vectors)

| $\mathbf{n}^T$                                               | $\mathbf{v}^T \in \mathbb{Z}_2$ |
|--------------------------------------------------------------|---------------------------------|
| $[(\blacksquare)^{2T}, A_5, M_5, Z_5, R_1, X_1]$             | 1                               |
| $[(\blacksquare)^{2T}, A_1 + A_4, M_2 + M_3, Z_5, R_1, X_1]$ | trivial                         |
| $[(\blacksquare)^{2T}, A_2 + A_3, M_1 + M_4, Z_5, R_1, X_1]$ | trivial                         |

2nd minimal solution:  $\mu_2^T = 4$  (18 symmetry vectors)

Space group 105 ( $\mathbb{Z}_1$ )

1st minimal solution:  $\mu_1^T = 2$  (4 symmetry vectors)

| $\mathbf{n}^T$                                                           |
|--------------------------------------------------------------------------|
| $[(\blacksquare)^{2T}, A_5, M_5, Z_5, R_1 + R_2, X_1 + X_2]$             |
| $[(\blacksquare)^{2T}, A_3 + A_4, M_3 + M_4, Z_5, R_2 + R_3, X_2 + X_3]$ |
| $[(\blacksquare)^{2T}, A_5, M_5, Z_5, R_3 + R_4, X_3 + X_4]$             |
| $[(\blacksquare)^{2T}, A_1 + A_2, M_1 + M_2, Z_5, R_1 + R_4, X_1 + X_4]$ |

2nd minimal solution:  $\mu_2^T = 4$  (32 symmetry vectors)

Space group 106 ( $\mathbb{Z}_2$ )

1st minimal solution:  $\mu_1^T = 2$  (1 symmetry vector & filling-enforced topology)

| $\mathbf{n}^T$                                   | $\mathbf{v}^T \in \mathbb{Z}_2$ |
|--------------------------------------------------|---------------------------------|
| $[(\blacksquare)^{2T}, A_5, M_5, Z_5, R_1, X_1]$ | 1                               |

2nd minimal solution:  $\mu_2^T = 4$  (2 symmetry vectors)

Space group 107 ( $\mathbb{Z}_1$ )

1st minimal solution:  $\mu_1^T = 2$  (2 symmetry vectors)

| $\mathbf{n}^T$                                                |
|---------------------------------------------------------------|
| $[(\blacksquare)^{2T}, M_5, P_3 + P_4, X_3 + X_4, N_1 + N_2]$ |
| $[(\blacksquare)^{2T}, M_5, P_1 + P_2, X_1 + X_2, N_1 + N_2]$ |

2nd minimal solution:  $\mu_2^T = 3$  (8 symmetry vectors)

Space group 108 ( $\mathbb{Z}_1$ )

1st minimal solution:  $\mu_1^T = 2$  (2 symmetry vectors)

| $\mathbf{n}^T$                                                |
|---------------------------------------------------------------|
| $[(\blacksquare)^{2T}, M_5, P_1 + P_2, X_1 + X_2, N_1 + N_2]$ |
| $[(\blacksquare)^{2T}, M_5, P_3 + P_4, X_3 + X_4, N_1 + N_2]$ |

2nd minimal solution:  $\mu_2^T = 4$  (13 symmetry vectors)

Space group 109 ( $\mathbb{Z}_1$ )

1st minimal solution:  $\mu_1^T = 2$  (1 symmetry vector)

| $\mathbf{n}^T$                                    |
|---------------------------------------------------|
| $[(\blacksquare)^{2T}, M_5, P_1, X_1, N_1 + N_2]$ |

2nd minimal solution:  $\mu_2^T = 4$  (3 symmetry vectors)

Space group 110 ( $\mathbb{Z}_2$ )

1st minimal solution:  $\mu_1^T = 2$  (1 symmetry vector & filling-enforced topology)

| $\mathbf{n}^T$                                    | $\mathbf{v}^T \in \mathbb{Z}_2$ |
|---------------------------------------------------|---------------------------------|
| $[(\blacksquare)^{2T}, M_5, P_1, X_1, N_1 + N_2]$ | 1                               |

2nd minimal solution:  $\mu_2^T = 4$  (1 symmetry vector)

Space group 111 ( $\mathbb{Z}_1$ )

1st minimal solution:  $\mu_1^T = 2$  (8 symmetry vectors)

| $\mathbf{n}^T$                                                           |
|--------------------------------------------------------------------------|
| $[(\blacksquare)^{2T}, A_2 + A_3, M_1 + M_2, Z_5, R_3 + R_4, 2X_3]$      |
| $[(\blacksquare)^{2T}, A_3 + A_4, M_1 + M_4, Z_5, R_2 + R_4, X_2 + X_3]$ |
| $[(\blacksquare)^{2T}, A_1 + A_2, M_1 + M_4, Z_5, R_1 + R_3, X_2 + X_3]$ |
| $[(\blacksquare)^{2T}, A_1 + A_4, M_1 + M_2, Z_5, R_3 + R_4, 2X_3]$      |
| $[(\blacksquare)^{2T}, A_1 + A_2, M_2 + M_3, Z_5, R_1 + R_3, X_2 + X_3]$ |
| $[(\blacksquare)^{2T}, A_2 + A_3, M_3 + M_4, Z_5, R_1 + R_2, 2X_2]$      |
| $[(\blacksquare)^{2T}, A_1 + A_4, M_3 + M_4, Z_5, R_1 + R_2, 2X_2]$      |
| $[(\blacksquare)^{2T}, A_3 + A_4, M_2 + M_3, Z_5, R_2 + R_4, X_2 + X_3]$ |

2nd minimal solution:  $\mu_2^T = 3$  (192 symmetry vectors)

Space group 112 ( $\mathbb{Z}_2$ )

1st minimal solution:  $\mu_1^T = 2$  (16 symmetry vectors)

| $\mathbf{n}^T$                                                           | $\mathbf{v}^T \in \mathbb{Z}_2$ |
|--------------------------------------------------------------------------|---------------------------------|
| $[(\blacksquare)^{2T}, A_5, M_2 + M_3, Z_3 + Z_4, R_1 + R_4, X_2 + X_3]$ | trivial                         |
| $[(\blacksquare)^{2T}, A_5, M_1 + M_4, Z_3 + Z_4, R_1 + R_4, X_2 + X_3]$ | trivial                         |
| $[(\blacksquare)^{2T}, A_1 + A_4, M_5, Z_3 + Z_4, R_1 + R_4, X_2 + X_3]$ | 1                               |
| $[(\blacksquare)^{2T}, A_2 + A_3, M_5, Z_3 + Z_4, R_1 + R_4, X_2 + X_3]$ | 1                               |
| $[(\blacksquare)^{2T}, A_5, M_2 + M_3, Z_1 + Z_2, R_2 + R_3, X_2 + X_3]$ | trivial                         |

... continued on next page

... continued from previous page

|                                                                          |         |
|--------------------------------------------------------------------------|---------|
| $[(\blacksquare)^{2T}, A_5, M_1 + M_4, Z_1 + Z_2, R_2 + R_3, X_2 + X_3]$ | trivial |
| $[(\blacksquare)^{2T}, A_1 + A_4, M_5, Z_1 + Z_2, R_2 + R_3, X_2 + X_3]$ | 1       |
| $[(\blacksquare)^{2T}, A_2 + A_3, M_5, Z_1 + Z_2, R_2 + R_3, X_2 + X_3]$ | 1       |
| $[(\blacksquare)^{2T}, A_5, M_1 + M_2, Z_2 + Z_3, R_3 + R_4, 2X_3]$      | 1       |
| $[(\blacksquare)^{2T}, A_5, M_1 + M_2, Z_1 + Z_4, R_3 + R_4, 2X_3]$      | 1       |
| $[(\blacksquare)^{2T}, A_5, M_3 + M_4, Z_2 + Z_3, R_1 + R_2, 2X_2]$      | 1       |
| $[(\blacksquare)^{2T}, A_5, M_3 + M_4, Z_1 + Z_4, R_1 + R_2, 2X_2]$      | 1       |
| $[(\blacksquare)^{2T}, A_1 + A_2, M_5, Z_2 + Z_3, R_1 + R_3, X_2 + X_3]$ | 1       |
| $[(\blacksquare)^{2T}, A_1 + A_2, M_5, Z_1 + Z_4, R_1 + R_3, X_2 + X_3]$ | 1       |
| $[(\blacksquare)^{2T}, A_3 + A_4, M_5, Z_2 + Z_3, R_2 + R_4, X_2 + X_3]$ | 1       |
| $[(\blacksquare)^{2T}, A_3 + A_4, M_5, Z_1 + Z_4, R_2 + R_4, X_2 + X_3]$ | 1       |

2nd minimal solution:  $\mu_2^T = 4$  (712 symmetry vectors)

Space group 113 ( $Z_1$ )

1st minimal solution:  $\mu_1^T = 4$  (38 symmetry vectors)

| $n^T$                                                                                                                    |
|--------------------------------------------------------------------------------------------------------------------------|
| $[(\blacksquare)^{2T} + 2\Gamma_2, A_2 + A_4 + A_5, M_2 + M_4 + M_5, Z_2 + Z_4 + Z_5, 2R_1, 2X_1]$                       |
| $[(\blacksquare)^{2T} + \Gamma_1 + \Gamma_2, 2A_5, 2M_5, Z_2 + Z_3 + Z_5, 2R_1, 2X_1]$                                   |
| $[(\blacksquare)^{2T} + \Gamma_1 + \Gamma_2, 2A_5, 2M_5, Z_1 + Z_4 + Z_5, 2R_1, 2X_1]$                                   |
| $[(\blacksquare)^{2T} + \Gamma_1 + \Gamma_2, A_2 + A_3 + A_5, M_1 + M_4 + M_5, Z_2 + Z_3 + Z_5, 2R_1, 2X_1]$             |
| $[(\blacksquare)^{2T} + \Gamma_1 + \Gamma_2, A_2 + A_3 + A_5, M_2 + M_3 + M_5, Z_2 + Z_3 + Z_5, 2R_1, 2X_1]$             |
| $[(\blacksquare)^{2T} + \Gamma_1 + \Gamma_2, A_2 + A_3 + A_5, M_1 + M_4 + M_5, Z_1 + Z_4 + Z_5, 2R_1, 2X_1]$             |
| $[(\blacksquare)^{2T} + \Gamma_1 + \Gamma_2, A_2 + A_3 + A_5, M_2 + M_3 + M_5, Z_1 + Z_4 + Z_5, 2R_1, 2X_1]$             |
| $[(\blacksquare)^{2T} + \Gamma_1 + \Gamma_2, A_1 + A_4 + A_5, M_1 + M_4 + M_5, Z_2 + Z_3 + Z_5, 2R_1, 2X_1]$             |
| $[(\blacksquare)^{2T} + \Gamma_1 + \Gamma_2, A_1 + A_4 + A_5, M_2 + M_3 + M_5, Z_2 + Z_3 + Z_5, 2R_1, 2X_1]$             |
| $[(\blacksquare)^{2T} + \Gamma_1 + \Gamma_2, A_1 + A_4 + A_5, M_1 + M_4 + M_5, Z_1 + Z_4 + Z_5, 2R_1, 2X_1]$             |
| $[(\blacksquare)^{2T} + \Gamma_1 + \Gamma_2, A_1 + A_4 + A_5, M_2 + M_3 + M_5, Z_1 + Z_4 + Z_5, 2R_1, 2X_1]$             |
| $[(\blacksquare)^{2T} + 2\Gamma_2, 2A_2 + A_3 + A_4, M_1 + M_2 + 2M_4, Z_2 + Z_4 + Z_5, 2R_1, 2X_1]$                     |
| $[(\blacksquare)^{2T} + \Gamma_1 + \Gamma_2, 2A_2 + 2A_3, 2M_1 + 2M_4, Z_2 + Z_3 + Z_5, 2R_1, 2X_1]$                     |
| $[(\blacksquare)^{2T} + \Gamma_1 + \Gamma_2, 2A_2 + 2A_3, M_1 + M_2 + M_3 + M_4, Z_2 + Z_3 + Z_5, 2R_1, 2X_1]$           |
| $[(\blacksquare)^{2T} + \Gamma_1 + \Gamma_2, 2A_2 + 2A_3, 2M_1 + 2M_4, Z_1 + Z_4 + Z_5, 2R_1, 2X_1]$                     |
| $[(\blacksquare)^{2T} + \Gamma_1 + \Gamma_2, 2A_2 + 2A_3, M_1 + M_2 + M_3 + M_4, Z_1 + Z_4 + Z_5, 2R_1, 2X_1]$           |
| $[(\blacksquare)^{2T} + \Gamma_1 + \Gamma_2, A_1 + A_2 + A_3 + A_4, 2M_1 + 2M_4, Z_2 + Z_3 + Z_5, 2R_1, 2X_1]$           |
| $[(\blacksquare)^{2T} + \Gamma_1 + \Gamma_2, A_1 + A_2 + A_3 + A_4, M_1 + M_2 + M_3 + M_4, Z_2 + Z_3 + Z_5, 2R_1, 2X_1]$ |
| $[(\blacksquare)^{2T} + \Gamma_1 + \Gamma_2, A_1 + A_2 + A_3 + A_4, 2M_1 + 2M_4, Z_1 + Z_4 + Z_5, 2R_1, 2X_1]$           |
| $[(\blacksquare)^{2T} + \Gamma_1 + \Gamma_2, A_1 + A_2 + A_3 + A_4, M_1 + M_2 + M_3 + M_4, Z_1 + Z_4 + Z_5, 2R_1, 2X_1]$ |
| $[(\blacksquare)^{2T} + 2\Gamma_2, 2A_2 + A_3 + A_4, 2M_2 + M_3 + M_4, Z_2 + Z_4 + Z_5, 2R_1, 2X_1]$                     |
| $[(\blacksquare)^{2T} + \Gamma_1 + \Gamma_2, 2A_2 + 2A_3, 2M_2 + 2M_3, Z_2 + Z_3 + Z_5, 2R_1, 2X_1]$                     |
| $[(\blacksquare)^{2T} + \Gamma_1 + \Gamma_2, 2A_2 + 2A_3, 2M_2 + 2M_3, Z_1 + Z_4 + Z_5, 2R_1, 2X_1]$                     |
| $[(\blacksquare)^{2T} + \Gamma_1 + \Gamma_2, A_1 + A_2 + A_3 + A_4, 2M_2 + 2M_3, Z_2 + Z_3 + Z_5, 2R_1, 2X_1]$           |
| $[(\blacksquare)^{2T} + \Gamma_1 + \Gamma_2, A_1 + A_2 + A_3 + A_4, 2M_2 + 2M_3, Z_1 + Z_4 + Z_5, 2R_1, 2X_1]$           |
| $[(\blacksquare)^{2T} + 2\Gamma_2, A_1 + A_2 + 2A_4, M_1 + M_2 + 2M_4, Z_2 + Z_4 + Z_5, 2R_1, 2X_1]$                     |
| $[(\blacksquare)^{2T} + \Gamma_1 + \Gamma_2, 2A_1 + 2A_4, 2M_1 + 2M_4, Z_2 + Z_3 + Z_5, 2R_1, 2X_1]$                     |
| $[(\blacksquare)^{2T} + \Gamma_1 + \Gamma_2, 2A_1 + 2A_4, M_1 + M_2 + M_3 + M_4, Z_2 + Z_3 + Z_5, 2R_1, 2X_1]$           |
| $[(\blacksquare)^{2T} + \Gamma_1 + \Gamma_2, 2A_1 + 2A_4, 2M_1 + 2M_4, Z_1 + Z_4 + Z_5, 2R_1, 2X_1]$                     |
| $[(\blacksquare)^{2T} + \Gamma_1 + \Gamma_2, 2A_1 + 2A_4, M_1 + M_2 + M_3 + M_4, Z_1 + Z_4 + Z_5, 2R_1, 2X_1]$           |
| $[(\blacksquare)^{2T} + 2\Gamma_2, A_1 + A_2 + 2A_4, 2M_2 + M_3 + M_4, Z_2 + Z_4 + Z_5, 2R_1, 2X_1]$                     |
| $[(\blacksquare)^{2T} + \Gamma_1 + \Gamma_2, 2A_1 + 2A_4, 2M_2 + 2M_3, Z_2 + Z_3 + Z_5, 2R_1, 2X_1]$                     |

... continued on next page

... continued from previous page

---

|                                                                                                      |
|------------------------------------------------------------------------------------------------------|
| $[(\blacksquare)^{2T} + \Gamma_1 + \Gamma_2, 2A_1 + 2A_4, 2M_2 + 2M_3, Z_1 + Z_4 + Z_5, 2R_1, 2X_1]$ |
| $[(\blacksquare)^{2T} + 2\Gamma_1, A_1 + A_3 + A_5, M_1 + M_3 + M_5, Z_1 + Z_3 + Z_5, 2R_1, 2X_1]$   |
| $[(\blacksquare)^{2T} + 2\Gamma_1, A_1 + A_2 + 2A_3, 2M_1 + M_3 + M_4, Z_1 + Z_3 + Z_5, 2R_1, 2X_1]$ |
| $[(\blacksquare)^{2T} + 2\Gamma_1, A_1 + A_2 + 2A_3, M_1 + M_2 + 2M_3, Z_1 + Z_3 + Z_5, 2R_1, 2X_1]$ |
| $[(\blacksquare)^{2T} + 2\Gamma_1, 2A_1 + A_3 + A_4, 2M_1 + M_3 + M_4, Z_1 + Z_3 + Z_5, 2R_1, 2X_1]$ |
| $[(\blacksquare)^{2T} + 2\Gamma_1, 2A_1 + A_3 + A_4, M_1 + M_2 + 2M_3, Z_1 + Z_3 + Z_5, 2R_1, 2X_1]$ |

---

2nd minimal solution:  $\mu_2^T = 6$  (390 symmetry vectors)

Space group 114 ( $\mathbb{Z}_2$ )

1st minimal solution:  $\mu_1^T = 4$  (20 symmetry vectors)

| $\mathbf{n}^T$                                                                                               | $\mathbf{v}^T \in \mathbb{Z}_2$ |
|--------------------------------------------------------------------------------------------------------------|---------------------------------|
| $[(\blacksquare)^{2T} + \Gamma_1 + \Gamma_2, 2A_5, 2M_2 + 2M_3, Z_2 + Z_3 + Z_5, 2R_1, 2X_1]$                | 1                               |
| $[(\blacksquare)^{2T} + \Gamma_1 + \Gamma_2, 2A_5, M_1 + M_2 + M_3 + M_4, Z_2 + Z_3 + Z_5, 2R_1, 2X_1]$      | 1                               |
| $[(\blacksquare)^{2T} + \Gamma_1 + \Gamma_2, A_2 + A_3 + A_5, M_2 + M_3 + M_5, Z_2 + Z_3 + Z_5, 2R_1, 2X_1]$ | trivial                         |
| $[(\blacksquare)^{2T} + \Gamma_1 + \Gamma_2, A_1 + A_4 + A_5, M_2 + M_3 + M_5, Z_2 + Z_3 + Z_5, 2R_1, 2X_1]$ | trivial                         |
| $[(\blacksquare)^{2T} + \Gamma_1 + \Gamma_2, 2A_5, 2M_1 + 2M_4, Z_2 + Z_3 + Z_5, 2R_1, 2X_1]$                | 1                               |
| $[(\blacksquare)^{2T} + \Gamma_1 + \Gamma_2, A_2 + A_3 + A_5, M_1 + M_4 + M_5, Z_2 + Z_3 + Z_5, 2R_1, 2X_1]$ | trivial                         |
| $[(\blacksquare)^{2T} + \Gamma_1 + \Gamma_2, A_1 + A_4 + A_5, M_1 + M_4 + M_5, Z_2 + Z_3 + Z_5, 2R_1, 2X_1]$ | trivial                         |
| $[(\blacksquare)^{2T} + \Gamma_1 + \Gamma_2, 2A_2 + 2A_3, 2M_5, Z_2 + Z_3 + Z_5, 2R_1, 2X_1]$                | 1                               |
| $[(\blacksquare)^{2T} + \Gamma_1 + \Gamma_2, A_1 + A_2 + A_3 + A_4, 2M_5, Z_2 + Z_3 + Z_5, 2R_1, 2X_1]$      | 1                               |
| $[(\blacksquare)^{2T} + \Gamma_1 + \Gamma_2, 2A_1 + 2A_4, 2M_5, Z_2 + Z_3 + Z_5, 2R_1, 2X_1]$                | 1                               |
| $[(\blacksquare)^{2T} + \Gamma_1 + \Gamma_2, 2A_5, 2M_2 + 2M_3, Z_1 + Z_4 + Z_5, 2R_1, 2X_1]$                | 1                               |
| $[(\blacksquare)^{2T} + \Gamma_1 + \Gamma_2, 2A_5, M_1 + M_2 + M_3 + M_4, Z_1 + Z_4 + Z_5, 2R_1, 2X_1]$      | 1                               |
| $[(\blacksquare)^{2T} + \Gamma_1 + \Gamma_2, A_2 + A_3 + A_5, M_2 + M_3 + M_5, Z_1 + Z_4 + Z_5, 2R_1, 2X_1]$ | trivial                         |
| $[(\blacksquare)^{2T} + \Gamma_1 + \Gamma_2, A_1 + A_4 + A_5, M_2 + M_3 + M_5, Z_1 + Z_4 + Z_5, 2R_1, 2X_1]$ | trivial                         |
| $[(\blacksquare)^{2T} + \Gamma_1 + \Gamma_2, 2A_5, 2M_1 + 2M_4, Z_1 + Z_4 + Z_5, 2R_1, 2X_1]$                | 1                               |
| $[(\blacksquare)^{2T} + \Gamma_1 + \Gamma_2, A_2 + A_3 + A_5, M_1 + M_4 + M_5, Z_1 + Z_4 + Z_5, 2R_1, 2X_1]$ | trivial                         |
| $[(\blacksquare)^{2T} + \Gamma_1 + \Gamma_2, A_1 + A_4 + A_5, M_1 + M_4 + M_5, Z_1 + Z_4 + Z_5, 2R_1, 2X_1]$ | trivial                         |
| $[(\blacksquare)^{2T} + \Gamma_1 + \Gamma_2, 2A_2 + 2A_3, 2M_5, Z_1 + Z_4 + Z_5, 2R_1, 2X_1]$                | 1                               |
| $[(\blacksquare)^{2T} + \Gamma_1 + \Gamma_2, A_1 + A_2 + A_3 + A_4, 2M_5, Z_1 + Z_4 + Z_5, 2R_1, 2X_1]$      | 1                               |
| $[(\blacksquare)^{2T} + \Gamma_1 + \Gamma_2, 2A_1 + 2A_4, 2M_5, Z_1 + Z_4 + Z_5, 2R_1, 2X_1]$                | 1                               |

---

2nd minimal solution:  $\mu_2^T = 6$  (140 symmetry vectors)

Space group 115 ( $\mathbb{Z}_1$ )

1st minimal solution:  $\mu_1^T = 2$  (6 symmetry vectors)

| $\mathbf{n}^T$                                                           |
|--------------------------------------------------------------------------|
| $[(\blacksquare)^{2T}, A_3 + A_4, 2M_3, Z_5, R_2 + R_3, X_2 + X_3]$      |
| $[(\blacksquare)^{2T}, A_2 + A_4, M_2 + M_3, Z_5, R_3 + R_4, X_3 + X_4]$ |
| $[(\blacksquare)^{2T}, A_2 + A_4, M_2 + M_3, Z_5, R_1 + R_2, X_1 + X_2]$ |
| $[(\blacksquare)^{2T}, A_1 + A_3, M_2 + M_3, Z_5, R_3 + R_4, X_3 + X_4]$ |
| $[(\blacksquare)^{2T}, A_1 + A_3, M_2 + M_3, Z_5, R_1 + R_2, X_1 + X_2]$ |
| $[(\blacksquare)^{2T}, A_1 + A_2, 2M_2, Z_5, R_1 + R_4, X_1 + X_4]$      |

---

2nd minimal solution:  $\mu_2^T = 3$  (128 symmetry vectors)

Space group 116 ( $\mathbb{Z}_2$ )

1st minimal solution:  $\mu_1^T = 2$  (4 symmetry vectors & filling-enforced topology)

| $\mathbf{n}^T$                                                           | $\mathbf{v}^T \in \mathbb{Z}_2$ |
|--------------------------------------------------------------------------|---------------------------------|
| $[(\blacksquare)^{2T}, A_5, M_2 + M_3, Z_1 + Z_3, R_3 + R_4, X_3 + X_4]$ | 1                               |
| $[(\blacksquare)^{2T}, A_5, M_2 + M_3, Z_1 + Z_3, R_1 + R_2, X_1 + X_2]$ | 1                               |
| $[(\blacksquare)^{2T}, A_5, M_2 + M_3, Z_2 + Z_4, R_3 + R_4, X_3 + X_4]$ | 1                               |
| $[(\blacksquare)^{2T}, A_5, M_2 + M_3, Z_2 + Z_4, R_1 + R_2, X_1 + X_2]$ | 1                               |

2nd minimal solution:  $\mu_2^T = 4$  (198 symmetry vectors)

Space group 117 ( $\mathbb{Z}_2$ )

1st minimal solution:  $\mu_1^T = 2$  (2 symmetry vectors & filling-enforced topology)

| $\mathbf{n}^T$                                               | $\mathbf{v}^T \in \mathbb{Z}_2$ |
|--------------------------------------------------------------|---------------------------------|
| $[(\blacksquare)^{2T}, A_2 + A_4, M_1 + M_4, Z_5, R_1, X_1]$ | 1                               |
| $[(\blacksquare)^{2T}, A_1 + A_3, M_1 + M_4, Z_5, R_1, X_1]$ | 1                               |

2nd minimal solution:  $\mu_2^T = 4$  (114 symmetry vectors)

Space group 118 ( $\mathbb{Z}_2$ )

1st minimal solution:  $\mu_1^T = 2$  (2 symmetry vectors & filling-enforced topology)

| $\mathbf{n}^T$                                               | $\mathbf{v}^T \in \mathbb{Z}_2$ |
|--------------------------------------------------------------|---------------------------------|
| $[(\blacksquare)^{2T}, A_5, M_1 + M_4, Z_2 + Z_4, R_1, X_1]$ | 1                               |
| $[(\blacksquare)^{2T}, A_5, M_1 + M_4, Z_1 + Z_3, R_1, X_1]$ | 1                               |

2nd minimal solution:  $\mu_2^T = 4$  (66 symmetry vectors)

Space group 119 ( $\mathbb{Z}_1$ )

1st minimal solution:  $\mu_1^T = 2$  (4 symmetry vectors)

| $\mathbf{n}^T$                                                |
|---------------------------------------------------------------|
| $[(\blacksquare)^{2T}, M_5, P_2 + P_4, X_2 + X_4, N_1 + N_2]$ |
| $[(\blacksquare)^{2T}, M_5, P_2 + P_3, X_2 + X_4, N_1 + N_2]$ |
| $[(\blacksquare)^{2T}, M_5, P_1 + P_4, X_2 + X_4, N_1 + N_2]$ |
| $[(\blacksquare)^{2T}, M_5, P_1 + P_3, X_2 + X_4, N_1 + N_2]$ |

2nd minimal solution:  $\mu_2^T = 3$  (64 symmetry vectors)

Space group 120 ( $\mathbb{Z}_2$ )

1st minimal solution:  $\mu_1^T = 2$  (4 symmetry vectors & filling-enforced topology)

| $\mathbf{n}^T$                                                | $\mathbf{v}^T \in \mathbb{Z}_2$ |
|---------------------------------------------------------------|---------------------------------|
| $[(\blacksquare)^{2T}, M_5, P_2 + P_4, X_2 + X_4, N_1 + N_2]$ | 1                               |
| $[(\blacksquare)^{2T}, M_5, P_1 + P_4, X_2 + X_4, N_1 + N_2]$ | 1                               |
| $[(\blacksquare)^{2T}, M_5, P_2 + P_3, X_2 + X_4, N_1 + N_2]$ | 1                               |
| $[(\blacksquare)^{2T}, M_5, P_1 + P_3, X_2 + X_4, N_1 + N_2]$ | 1                               |

2nd minimal solution:  $\mu_2^T = 4$  (240 symmetry vectors)

Space group 121 ( $\mathbb{Z}_1$ )

1st minimal solution:  $\mu_1^T = 3$  (24 symmetry vectors)

| $\mathbf{n}^T$                                                                                             |
|------------------------------------------------------------------------------------------------------------|
| $[(\blacksquare)^{2T} + \Gamma_1, M_3 + M_5, P_3 + P_5, PA_3 + PA_5, X_1 + X_3 + X_4, N_1 + 2N_2]$         |
| $[(\blacksquare)^{2T} + \Gamma_1, M_3 + M_5, P_1 + P_5, PA_1 + PA_5, X_1 + X_3 + X_4, 2N_1 + N_2]$         |
| $[(\blacksquare)^{2T} + \Gamma_2, M_4 + M_5, P_4 + P_5, PA_4 + PA_5, X_2 + X_3 + X_4, N_1 + 2N_2]$         |
| $[(\blacksquare)^{2T} + \Gamma_2, M_4 + M_5, P_2 + P_5, PA_2 + PA_5, X_2 + X_3 + X_4, 2N_1 + N_2]$         |
| $[(\blacksquare)^{2T} + \Gamma_1, M_3 + M_5, 2P_3 + P_4, 2PA_3 + PA_4, 2X_1 + X_2, 3N_2]$                  |
| $[(\blacksquare)^{2T} + \Gamma_1, M_3 + M_5, P_1 + P_3 + P_4, PA_1 + PA_3 + PA_4, 2X_1 + X_2, N_1 + 2N_2]$ |
| $[(\blacksquare)^{2T} + \Gamma_1, M_3 + M_5, 2P_1 + P_4, 2PA_1 + PA_4, 2X_1 + X_2, 2N_1 + N_2]$            |
| $[(\blacksquare)^{2T} + \Gamma_2, M_4 + M_5, P_3 + 2P_4, PA_3 + 2PA_4, X_1 + 2X_2, 3N_2]$                  |
| $[(\blacksquare)^{2T} + \Gamma_2, M_4 + M_5, P_2 + P_3 + P_4, PA_1 + 2PA_4, X_1 + 2X_2, N_1 + 2N_2]$       |
| $[(\blacksquare)^{2T} + \Gamma_2, M_4 + M_5, P_2 + P_3 + P_4, PA_2 + PA_3 + PA_4, X_1 + 2X_2, N_1 + 2N_2]$ |
| $[(\blacksquare)^{2T} + \Gamma_2, M_4 + M_5, P_1 + 2P_4, PA_1 + 2PA_4, X_1 + 2X_2, N_1 + 2N_2]$            |
| $[(\blacksquare)^{2T} + \Gamma_2, M_4 + M_5, P_1 + 2P_4, PA_2 + PA_3 + PA_4, X_1 + 2X_2, N_1 + 2N_2]$      |
| $[(\blacksquare)^{2T} + \Gamma_2, M_4 + M_5, P_1 + P_2 + P_4, PA_1 + PA_2 + PA_4, X_1 + 2X_2, 2N_1 + N_2]$ |
| $[(\blacksquare)^{2T} + \Gamma_1, M_3 + M_5, P_2 + 2P_3, PA_1 + PA_3 + PA_4, 2X_1 + X_2, N_1 + 2N_2]$      |
| $[(\blacksquare)^{2T} + \Gamma_1, M_3 + M_5, P_1 + P_2 + P_3, 2PA_1 + PA_4, 2X_1 + X_2, 2N_1 + N_2]$       |
| $[(\blacksquare)^{2T} + \Gamma_2, M_4 + M_5, 2P_2 + P_3, PA_1 + PA_2 + PA_4, X_1 + 2X_2, 2N_1 + N_2]$      |
| $[(\blacksquare)^{2T} + \Gamma_1, M_3 + M_5, P_2 + 2P_3, PA_2 + 2PA_3, 2X_1 + X_2, N_1 + 2N_2]$            |
| $[(\blacksquare)^{2T} + \Gamma_1, M_3 + M_5, P_1 + P_2 + P_3, PA_1 + PA_2 + PA_3, 2X_1 + X_2, 2N_1 + N_2]$ |
| $[(\blacksquare)^{2T} + \Gamma_1, M_3 + M_5, 2P_1 + P_2, 2PA_1 + PA_2, 2X_1 + X_2, 3N_1]$                  |
| $[(\blacksquare)^{2T} + \Gamma_2, M_4 + M_5, 2P_2 + P_3, 2PA_2 + PA_3, X_1 + 2X_2, 2N_1 + N_2]$            |
| $[(\blacksquare)^{2T} + \Gamma_2, M_4 + M_5, P_1 + P_2 + P_4, 2PA_2 + PA_3, X_1 + 2X_2, 2N_1 + N_2]$       |
| $[(\blacksquare)^{2T} + \Gamma_2, M_4 + M_5, P_1 + 2P_2, PA_1 + 2PA_2, X_1 + 2X_2, 3N_1]$                  |
| $[(\blacksquare)^{2T} + \Gamma_1, M_3 + M_5, P_1 + P_3 + P_4, PA_2 + 2PA_3, 2X_1 + X_2, N_1 + 2N_2]$       |
| $[(\blacksquare)^{2T} + \Gamma_1, M_3 + M_5, 2P_1 + P_4, PA_1 + PA_2 + PA_3, 2X_1 + X_2, 2N_1 + N_2]$      |

2nd minimal solution:  $\mu_2^T = 4$  (172 symmetry vectors)

Space group 122 ( $\mathbb{Z}_2$ )

1st minimal solution:  $\mu_1^T = 2$  (4 symmetry vectors)

| $\mathbf{n}^T$                                                | $\mathbf{v}^T \in \mathbb{Z}_2$ |
|---------------------------------------------------------------|---------------------------------|
| $[(\blacksquare)^{2T}, M_3 + M_4, P_2, PA_1, X_1, N_1 + N_2]$ | 1                               |
| $[(\blacksquare)^{2T}, M_3 + M_4, P_2, PA_2, X_1, N_1 + N_2]$ | trivial                         |
| $[(\blacksquare)^{2T}, M_3 + M_4, P_1, PA_1, X_1, N_1 + N_2]$ | trivial                         |
| $[(\blacksquare)^{2T}, M_3 + M_4, P_1, PA_2, X_1, N_1 + N_2]$ | 1                               |

2nd minimal solution:  $\mu_2^T = 4$  (54 symmetry vectors)

Space group 123 ( $\mathbb{Z}_1$ )

1st minimal solution:  $\mu_1^T = 2$  (8 symmetry vectors)

| $\mathbf{n}^T$                                                                             |
|--------------------------------------------------------------------------------------------|
| $[(\blacksquare)^{2T}, A_2^- + A_4^-, M_2^+ + M_2^-, Z_5^+, R_3^+ + R_4^+, X_3^+ + X_3^-]$ |
| $[(\blacksquare)^{2T}, A_2^+ + A_4^+, M_2^+ + M_2^-, Z_5^-, R_3^- + R_4^-, X_3^+ + X_3^-]$ |
| $[(\blacksquare)^{2T}, A_3^+ + A_4^+, M_2^- + M_3^+, Z_5^-, R_2^+ + R_4^-, X_2^+ + X_3^+]$ |
| $[(\blacksquare)^{2T}, A_1^- + A_2^-, M_2^- + M_3^+, Z_5^+, R_1^- + R_3^+, X_2^+ + X_3^+]$ |
| $[(\blacksquare)^{2T}, A_1^+ + A_2^+, M_2^+ + M_3^-, Z_5^-, R_1^+ + R_3^-, X_2^- + X_3^-]$ |
| $[(\blacksquare)^{2T}, A_3^- + A_4^-, M_2^+ + M_3^-, Z_5^+, R_2^- + R_4^+, X_2^- + X_3^-]$ |
| $[(\blacksquare)^{2T}, A_1^+ + A_3^+, M_3^+ + M_3^-, Z_5^-, R_1^+ + R_2^+, X_2^+ + X_2^-]$ |
| $[(\blacksquare)^{2T}, A_1^- + A_3^-, M_3^+ + M_3^-, Z_5^+, R_1^- + R_2^-, X_2^+ + X_2^-]$ |

2nd minimal solution:  $\mu_2^T = 3$  (360 symmetry vectors)

Space group 124 ( $\mathbb{Z}_4$ )

1st minimal solution:  $\mu_1^T = 2$  (4 symmetry vectors & filling-enforced topology)

| $\mathbf{n}^T$                                                       | $\mathbf{v}^T \in \mathbb{Z}_4$ |
|----------------------------------------------------------------------|---------------------------------|
| $[(\blacksquare)^{2T}, A_1, M_2^+ + M_2^-, Z_4, R_2, X_3^+ + X_3^-]$ | 3                               |
| $[(\blacksquare)^{2T}, A_1, M_2^+ + M_2^-, Z_3, R_2, X_3^+ + X_3^-]$ | 1                               |
| $[(\blacksquare)^{2T}, A_2, M_3^+ + M_3^-, Z_4, R_1, X_2^+ + X_2^-]$ | 3                               |
| $[(\blacksquare)^{2T}, A_2, M_3^+ + M_3^-, Z_3, R_1, X_2^+ + X_2^-]$ | 1                               |

2nd minimal solution:  $\mu_2^T = 4$  (400 symmetry vectors)

Space group 125 ( $\mathbb{Z}_1$ )

1st minimal solution:  $\mu_1^T = 4$  (20 symmetry vectors)

| $\mathbf{n}^T$                                                                                                       |
|----------------------------------------------------------------------------------------------------------------------|
| $[(\blacksquare)^{2T} + \Gamma_1^+ + \Gamma_1^-, A_3 + A_4, M_3 + M_4, Z_1^- + Z_3^- + Z_5^-, R_1 + R_2, X_1 + X_2]$ |
| $[(\blacksquare)^{2T} + \Gamma_1^+ + \Gamma_1^-, A_3 + A_4, M_3 + M_4, Z_1^+ + Z_3^+ + Z_5^+, R_1 + R_2, X_1 + X_2]$ |
| $[(\blacksquare)^{2T} + \Gamma_1^+ + \Gamma_2^-, A_2 + A_3, M_2 + M_3, Z_2^- + Z_3^- + Z_5^-, R_1 + R_2, X_1 + X_2]$ |
| $[(\blacksquare)^{2T} + \Gamma_1^+ + \Gamma_2^-, A_1 + A_3, M_2 + M_3, Z_1^+ + Z_4^+ + Z_5^+, R_1 + R_2, X_1 + X_2]$ |

... continued on next page



... continued from previous page

---

|                                                                                                                      |
|----------------------------------------------------------------------------------------------------------------------|
| $[(\blacksquare)^{2T} + \Gamma_1^+ + \Gamma_1^-, A_1 + A_2, M_1 + M_2, Z_1^- + Z_3^- + Z_5^-, R_1 + R_2, X_1 + X_2]$ |
| $[(\blacksquare)^{2T} + \Gamma_1^+ + \Gamma_1^-, A_1 + A_2, M_1 + M_2, Z_1^+ + Z_3^+ + Z_5^+, R_1 + R_2, X_1 + X_2]$ |
| $[(\blacksquare)^{2T} + \Gamma_4^+ + \Gamma_4^-, A_3 + A_4, M_3 + M_4, Z_2^- + Z_4^- + Z_5^-, R_1 + R_2, 2X_2]$      |
| $[(\blacksquare)^{2T} + \Gamma_3^+ + \Gamma_4^-, A_1 + A_4, M_2 + M_4, Z_1^- + Z_4^- + Z_5^-, R_1 + R_2, 2X_2]$      |
| $[(\blacksquare)^{2T} + \Gamma_4^+ + \Gamma_4^-, A_3 + A_4, M_3 + M_4, Z_2^+ + Z_4^+ + Z_5^+, R_1 + R_2, 2X_2]$      |
| $[(\blacksquare)^{2T} + \Gamma_1^- + \Gamma_2^+, A_2 + A_4, M_2 + M_4, Z_2^+ + Z_3^+ + Z_5^+, R_1 + R_2, X_1 + X_2]$ |
| $[(\blacksquare)^{2T} + \Gamma_3^- + \Gamma_4^+, A_2 + A_3, M_2 + M_3, Z_2^- + Z_3^- + Z_5^-, R_1 + R_2, 2X_2]$      |
| $[(\blacksquare)^{2T} + \Gamma_3^- + \Gamma_4^+, A_1 + A_3, M_2 + M_3, Z_1^+ + Z_4^+ + Z_5^+, R_1 + R_2, 2X_2]$      |
| $[(\blacksquare)^{2T} + \Gamma_4^+ + \Gamma_4^-, A_1 + A_2, M_1 + M_2, Z_2^- + Z_4^- + Z_5^-, R_1 + R_2, 2X_2]$      |
| $[(\blacksquare)^{2T} + \Gamma_4^+ + \Gamma_4^-, A_1 + A_2, M_1 + M_2, Z_2^+ + Z_4^+ + Z_5^+, R_1 + R_2, 2X_2]$      |
| $[(\blacksquare)^{2T} + \Gamma_3^+ + \Gamma_3^-, A_1 + A_2, 2M_2, Z_1^- + Z_3^- + Z_5^-, R_1 + R_2, 2X_2]$           |
| $[(\blacksquare)^{2T} + \Gamma_3^+ + \Gamma_4^-, A_2 + A_4, M_2 + M_4, Z_2^+ + Z_3^+ + Z_5^+, R_1 + R_2, 2X_2]$      |
| $[(\blacksquare)^{2T} + \Gamma_2^+ + \Gamma_2^-, A_1 + A_2, 2M_2, Z_2^+ + Z_4^+ + Z_5^+, R_1 + R_2, X_1 + X_2]$      |
| $[(\blacksquare)^{2T} + \Gamma_1^- + \Gamma_2^+, A_1 + A_4, M_2 + M_4, Z_1^- + Z_4^- + Z_5^-, R_1 + R_2, X_1 + X_2]$ |
| $[(\blacksquare)^{2T} + \Gamma_3^+ + \Gamma_3^-, A_1 + A_2, 2M_2, Z_1^+ + Z_3^+ + Z_5^+, R_1 + R_2, 2X_2]$           |
| $[(\blacksquare)^{2T} + \Gamma_2^+ + \Gamma_2^-, A_1 + A_2, 2M_2, Z_2^- + Z_4^- + Z_5^-, R_1 + R_2, X_1 + X_2]$      |

---

2nd minimal solution:  $\mu_2^T = 6$  (308 symmetry vectors)

Space group 126 ( $\mathbb{Z}_2$ )

1st minimal solution:  $\mu_1^T = 2$  (4 symmetry vectors & filling-enforced topology)

| $\mathbf{n}^T$                                   | $\mathbf{v}^T \in \mathbb{Z}_2$ |
|--------------------------------------------------|---------------------------------|
| $[(\blacksquare)^{2T}, A_2, M_2, Z_4, R_2, X_2]$ | 1                               |
| $[(\blacksquare)^{2T}, A_2, M_2, Z_3, R_2, X_2]$ | 1                               |
| $[(\blacksquare)^{2T}, A_1, M_2, Z_4, R_1, X_2]$ | 1                               |
| $[(\blacksquare)^{2T}, A_1, M_2, Z_3, R_1, X_2]$ | 1                               |

2nd minimal solution:  $\mu_2^T = 4$  (28 symmetry vectors)

Space group 127 ( $\mathbb{Z}_1$ )

1st minimal solution:  $\mu_1^T = 4$  (78 symmetry vectors)

---

| $\mathbf{n}^T$                                                                                                                                               |
|--------------------------------------------------------------------------------------------------------------------------------------------------------------|
| $[(\blacksquare)^{2T} + \Gamma_2^+ + \Gamma_2^-, A_1^+ + A_2^+ + A_3^+ + A_4^+, M_1^+ + M_1^- + M_4^+ + M_4^-, Z_2^- + Z_4^- + Z_5^+, 2R_1, X_1 + X_2]$      |
| $[(\blacksquare)^{2T} + \Gamma_1^+ + \Gamma_2^-, A_1^+ + A_4^+ + A_5^-, M_1^+ + M_4^+ + M_5^+, Z_2^- + Z_3^- + Z_5^+, 2R_1, X_1 + X_2]$                      |
| $[(\blacksquare)^{2T} + \Gamma_1^+ + \Gamma_2^-, A_1^+ + A_2^+ + 2A_4^+, M_1^+ + M_2^- + M_4^+ + M_4^-, Z_2^- + Z_3^- + Z_5^+, 2R_1, X_1 + X_2]$             |
| $[(\blacksquare)^{2T} + \Gamma_1^+ + \Gamma_2^-, 2A_1^+ + A_3^+ + A_4^+, M_1^+ + M_1^- + M_3^- + M_4^+, Z_2^- + Z_3^- + Z_5^+, 2R_1, X_1 + X_2]$             |
| $[(\blacksquare)^{2T} + \Gamma_1^+ + \Gamma_2^-, A_2^- + A_3^- + A_5^-, M_1^+ + M_4^+ + M_5^+, Z_1^+ + Z_4^+ + Z_5^+, R_1 + R_2, X_1 + X_2]$                 |
| $[(\blacksquare)^{2T} + \Gamma_1^+ + \Gamma_2^-, A_2^+ + A_2^- + A_3^- + A_4^+, M_1^+ + M_2^- + M_4^+ + M_4^-, Z_1^+ + Z_4^+ + Z_5^+, R_1 + R_2, X_1 + X_2]$ |
| $[(\blacksquare)^{2T} + \Gamma_1^+ + \Gamma_2^-, A_1^+ + A_2^- + A_3^+ + A_3^-, M_1^+ + M_1^- + M_3^- + M_4^+, Z_1^+ + Z_4^+ + Z_5^+, R_1 + R_2, X_1 + X_2]$ |
| $[(\blacksquare)^{2T} + \Gamma_1^- + \Gamma_2^+, A_1^- + A_4^- + A_5^-, M_1^- + M_4^- + M_5^-, Z_2^+ + Z_3^+ + Z_5^+, R_1 + R_2, X_1 + X_2]$                 |
| $[(\blacksquare)^{2T} + \Gamma_1^- + \Gamma_2^+, A_1^- + A_2^+ + A_4^+ + A_4^-, M_1^- + M_2^+ + M_4^+ + M_4^-, Z_2^+ + Z_3^+ + Z_5^+, R_1 + R_2, X_1 + X_2]$ |
| $[(\blacksquare)^{2T} + \Gamma_1^- + \Gamma_2^+, A_1^+ + A_1^- + A_3^+ + A_4^-, M_1^+ + M_1^- + M_3^+ + M_4^-, Z_2^+ + Z_3^+ + Z_5^+, R_1 + R_2, X_1 + X_2]$ |
| $[(\blacksquare)^{2T} + \Gamma_1^- + \Gamma_2^+, A_2^+ + A_3^+ + A_5^-, M_1^- + M_4^- + M_5^-, Z_1^- + Z_4^- + Z_5^+, 2R_1, X_1 + X_2]$                      |

---

... continued on next page

... continued on next page

... continued from previous page

---

|                                                                                                                                                              |
|--------------------------------------------------------------------------------------------------------------------------------------------------------------|
| $[(\blacksquare)^{2T} + \Gamma_1^+ + \Gamma_1^-, 2A_1^- + 2A_3^-, M_1^+ + M_1^- + M_3^+ + M_3^-, Z_1^+ + Z_3^+ + Z_5^-, 2R_2, X_1 + X_2]$                    |
| $[(\blacksquare)^{2T} + \Gamma_1^+ + \Gamma_1^-, A_1^+ + A_1^- + A_3^+ + A_3^-, M_1^+ + M_1^- + M_3^+ + M_3^-, Z_1^- + Z_3^- + Z_5^-, R_1 + R_2, X_1 + X_2]$ |
| $[(\blacksquare)^{2T} + \Gamma_1^- + \Gamma_2^+, A_1^- + A_2^- + 2A_4^-, M_1^- + M_2^+ + M_4^+ + M_4^-, Z_2^+ + Z_3^+ + Z_5^-, 2R_2, X_1 + X_2]$             |
| $[(\blacksquare)^{2T} + \Gamma_1^- + \Gamma_2^+, 2A_1^- + A_3^- + A_4^-, M_1^+ + M_1^- + M_3^+ + M_4^-, Z_2^+ + Z_3^+ + Z_5^-, 2R_2, X_1 + X_2]$             |
| $[(\blacksquare)^{2T} + \Gamma_1^- + \Gamma_2^+, A_2^+ + A_2^- + A_3^+ + A_4^-, M_1^- + M_2^+ + M_4^+ + M_4^-, Z_1^- + Z_4^- + Z_5^-, R_1 + R_2, X_1 + X_2]$ |
| $[(\blacksquare)^{2T} + \Gamma_1^- + \Gamma_2^+, A_1^- + A_2^+ + A_3^+ + A_3^-, M_1^+ + M_1^- + M_3^+ + M_4^-, Z_1^- + Z_4^- + Z_5^-, R_1 + R_2, X_1 + X_2]$ |
| $[(\blacksquare)^{2T} + \Gamma_2^+ + \Gamma_2^-, A_1^- + A_2^- + A_3^- + A_4^-, M_1^+ + M_1^- + M_4^+ + M_4^-, Z_2^+ + Z_4^+ + Z_5^-, 2R_2, X_1 + X_2]$      |
| $[(\blacksquare)^{2T} + \Gamma_2^+ + \Gamma_2^-, A_1^- + A_2^+ + A_3^- + A_4^+, M_1^+ + M_1^- + M_4^+ + M_4^-, Z_2^- + Z_4^- + Z_5^-, R_1 + R_2, X_1 + X_2]$ |
| $[(\blacksquare)^{2T} + \Gamma_2^+ + \Gamma_2^-, A_1^+ + A_2^- + A_3^+ + A_4^-, M_1^+ + M_1^- + M_4^+ + M_4^-, Z_2^- + Z_4^- + Z_5^-, R_1 + R_2, X_1 + X_2]$ |
| $[(\blacksquare)^{2T} + \Gamma_1^+ + \Gamma_1^-, A_2^- + A_4^- + A_5^-, M_2^+ + M_4^+ + M_5^+, Z_1^- + Z_3^- + Z_5^-, R_1 + R_2, X_1 + X_2]$                 |
| $[(\blacksquare)^{2T} + \Gamma_1^+ + \Gamma_1^-, A_1^+ + A_2^- + A_3^+ + A_4^-, M_1^- + M_2^+ + M_3^- + M_4^+, Z_1^- + Z_3^- + Z_5^-, R_1 + R_2, X_1 + X_2]$ |
| $[(\blacksquare)^{2T} + \Gamma_1^+ + \Gamma_1^-, A_1^- + A_3^- + A_5^-, M_1^+ + M_3^+ + M_5^+, Z_1^- + Z_3^- + Z_5^-, R_1 + R_2, X_1 + X_2]$                 |
| $[(\blacksquare)^{2T} + \Gamma_1^+ + \Gamma_1^-, A_1^- + A_2^+ + A_3^- + A_4^+, M_1^+ + M_2^- + M_3^+ + M_4^-, Z_1^- + Z_3^- + Z_5^-, R_1 + R_2, X_1 + X_2]$ |

---

2nd minimal solution:  $\mu_2^T = 6$  (2664 symmetry vectors)

Space group 128 ( $\mathbb{Z}_4$ )

1st minimal solution:  $\mu_1^T = 4$  (96 symmetry vectors)

| $\mathbf{n}^T$                                                                                                                   | $\mathbf{v}^T \in \mathbb{Z}_4$ |
|----------------------------------------------------------------------------------------------------------------------------------|---------------------------------|
| $[(\blacksquare)^{2T} + \Gamma_1^+ + \Gamma_1^-, 2A_3, M_2^+ + M_2^- + M_4^+ + M_4^-, Z_2 + Z_4, 2R_1^-, X_1 + X_2]$             | 1                               |
| $[(\blacksquare)^{2T} + \Gamma_1^+ + \Gamma_1^-, 2A_3, M_2^+ + M_2^- + M_4^+ + M_4^-, Z_2 + Z_4, R_1^+ + R_1^-, X_1 + X_2]$      | 3                               |
| $[(\blacksquare)^{2T} + \Gamma_1^+ + \Gamma_1^-, A_3 + A_4, M_1^- + M_2^+ + M_3^- + M_4^+, Z_2 + Z_4, 2R_1^-, X_1 + X_2]$        | 3                               |
| $[(\blacksquare)^{2T} + \Gamma_1^+ + \Gamma_1^-, A_3 + A_4, M_1^- + M_2^+ + M_3^- + M_4^+, Z_2 + Z_4, R_1^+ + R_1^-, X_1 + X_2]$ | 1                               |
| $[(\blacksquare)^{2T} + \Gamma_1^+ + \Gamma_1^-, A_2 + A_3, M_2^+ + M_4^+ + M_5^+, Z_2 + Z_4, 2R_1^-, X_1 + X_2]$                | trivial                         |
| $[(\blacksquare)^{2T} + \Gamma_1^+ + \Gamma_1^-, A_2 + A_3, M_2^+ + M_4^+ + M_5^+, Z_2 + Z_4, R_1^+ + R_1^-, X_1 + X_2]$         | 2                               |
| $[(\blacksquare)^{2T} + \Gamma_1^+ + \Gamma_1^-, A_1 + A_3, M_2^+ + M_4^+ + M_5^+, Z_2 + Z_4, 2R_1^-, X_1 + X_2]$                | 2                               |
| $[(\blacksquare)^{2T} + \Gamma_1^+ + \Gamma_1^-, A_1 + A_3, M_2^+ + M_4^+ + M_5^+, Z_2 + Z_4, R_1^+ + R_1^-, X_1 + X_2]$         | trivial                         |
| $[(\blacksquare)^{2T} + \Gamma_1^+ + \Gamma_1^-, 2A_3, M_2^+ + M_2^- + M_4^+ + M_4^-, Z_2 + Z_3, 2R_1^-, X_1 + X_2]$             | 3                               |
| $[(\blacksquare)^{2T} + \Gamma_1^+ + \Gamma_1^-, 2A_3, M_2^+ + M_2^- + M_4^+ + M_4^-, Z_2 + Z_3, R_1^+ + R_1^-, X_1 + X_2]$      | 1                               |
| $[(\blacksquare)^{2T} + \Gamma_1^+ + \Gamma_1^-, A_3 + A_4, M_1^- + M_2^+ + M_3^- + M_4^+, Z_2 + Z_3, 2R_1^-, X_1 + X_2]$        | 1                               |
| $[(\blacksquare)^{2T} + \Gamma_1^+ + \Gamma_1^-, A_3 + A_4, M_1^- + M_2^+ + M_3^- + M_4^+, Z_2 + Z_3, R_1^+ + R_1^-, X_1 + X_2]$ | 3                               |
| $[(\blacksquare)^{2T} + \Gamma_1^+ + \Gamma_1^-, A_2 + A_3, M_2^+ + M_4^+ + M_5^+, Z_2 + Z_3, 2R_1^-, X_1 + X_2]$                | 2                               |
| $[(\blacksquare)^{2T} + \Gamma_1^+ + \Gamma_1^-, A_2 + A_3, M_2^+ + M_4^+ + M_5^+, Z_2 + Z_3, R_1^+ + R_1^-, X_1 + X_2]$         | trivial                         |
| $[(\blacksquare)^{2T} + \Gamma_1^+ + \Gamma_1^-, A_1 + A_3, M_2^+ + M_4^+ + M_5^+, Z_2 + Z_3, 2R_1^-, X_1 + X_2]$                | trivial                         |
| $[(\blacksquare)^{2T} + \Gamma_1^+ + \Gamma_1^-, A_1 + A_3, M_2^+ + M_4^+ + M_5^+, Z_2 + Z_3, R_1^+ + R_1^-, X_1 + X_2]$         | 2                               |
| $[(\blacksquare)^{2T} + \Gamma_1^+ + \Gamma_1^-, 2A_3, M_2^+ + M_2^- + M_4^+ + M_4^-, Z_2 + Z_4, 2R_1^+, X_1 + X_2]$             | 1                               |
| $[(\blacksquare)^{2T} + \Gamma_1^+ + \Gamma_1^-, A_3 + A_4, M_1^- + M_2^+ + M_3^- + M_4^+, Z_2 + Z_4, 2R_1^+, X_1 + X_2]$        | 3                               |
| $[(\blacksquare)^{2T} + \Gamma_1^+ + \Gamma_1^-, A_2 + A_3, M_2^+ + M_4^+ + M_5^+, Z_2 + Z_4, 2R_1^+, X_1 + X_2]$                | trivial                         |
| $[(\blacksquare)^{2T} + \Gamma_1^+ + \Gamma_1^-, A_1 + A_3, M_2^+ + M_4^+ + M_5^+, Z_2 + Z_4, 2R_1^+, X_1 + X_2]$                | 2                               |
| $[(\blacksquare)^{2T} + \Gamma_1^+ + \Gamma_1^-, 2A_3, M_2^+ + M_2^- + M_4^+ + M_4^-, Z_2 + Z_3, 2R_1^+, X_1 + X_2]$             | 3                               |
| $[(\blacksquare)^{2T} + \Gamma_1^+ + \Gamma_1^-, A_3 + A_4, M_1^- + M_2^+ + M_3^- + M_4^+, Z_2 + Z_3, 2R_1^+, X_1 + X_2]$        | 1                               |
| $[(\blacksquare)^{2T} + \Gamma_1^+ + \Gamma_1^-, A_2 + A_3, M_2^+ + M_4^+ + M_5^+, Z_2 + Z_3, 2R_1^+, X_1 + X_2]$                | 2                               |
| $[(\blacksquare)^{2T} + \Gamma_1^+ + \Gamma_1^-, A_1 + A_3, M_2^+ + M_4^+ + M_5^+, Z_2 + Z_3, 2R_1^+, X_1 + X_2]$                | trivial                         |
| $[(\blacksquare)^{2T} + \Gamma_1^+ + \Gamma_1^-, A_3 + A_4, M_1^- + M_2^- + M_3^+ + M_4^-, Z_2 + Z_4, 2R_1^-, X_1 + X_2]$        | 3                               |
| $[(\blacksquare)^{2T} + \Gamma_1^+ + \Gamma_1^-, A_3 + A_4, M_1^- + M_2^- + M_3^+ + M_4^-, Z_2 + Z_4, R_1^+ + R_1^-, X_1 + X_2]$ | 1                               |
| $[(\blacksquare)^{2T} + \Gamma_1^+ + \Gamma_1^-, A_2 + A_3, M_2^- + M_4^- + M_5^-, Z_2 + Z_4, 2R_1^-, X_1 + X_2]$                | trivial                         |
| $[(\blacksquare)^{2T} + \Gamma_1^+ + \Gamma_1^-, A_2 + A_3, M_2^- + M_4^- + M_5^-, Z_2 + Z_4, R_1^+ + R_1^-, X_1 + X_2]$         | 2                               |
| $[(\blacksquare)^{2T} + \Gamma_1^+ + \Gamma_1^-, A_1 + A_3, M_2^- + M_4^- + M_5^-, Z_2 + Z_4, 2R_1^-, X_1 + X_2]$                | 2                               |
| $[(\blacksquare)^{2T} + \Gamma_1^+ + \Gamma_1^-, A_1 + A_3, M_2^- + M_4^- + M_5^-, Z_2 + Z_4, R_1^+ + R_1^-, X_1 + X_2]$         | trivial                         |

... continued on next page



... continued from previous page

|                                                                                                                                  |   |
|----------------------------------------------------------------------------------------------------------------------------------|---|
| $[(\blacksquare)^{2T} + \Gamma_2^+ + \Gamma_2^-, A_3 + A_4, M_1^+ + M_1^- + M_4^+ + M_4^-, Z_1 + Z_3, 2R_1^-, X_1 + X_2]$        | 3 |
| $[(\blacksquare)^{2T} + \Gamma_2^+ + \Gamma_2^-, A_3 + A_4, M_1^+ + M_1^- + M_4^+ + M_4^-, Z_1 + Z_3, R_1^+ + R_1^-, X_1 + X_2]$ | 1 |
| $[(\blacksquare)^{2T} + \Gamma_2^+ + \Gamma_2^-, A_3 + A_4, M_1^+ + M_1^- + M_4^+ + M_4^-, Z_1 + Z_3, 2R_1^+, X_1 + X_2]$        | 3 |
| $[(\blacksquare)^{2T} + \Gamma_1^+ + \Gamma_1^-, 2A_2, M_5^+ + M_5^-, Z_2 + Z_3, 2R_1^-, X_1 + X_2]$                             | 1 |
| $[(\blacksquare)^{2T} + \Gamma_1^+ + \Gamma_1^-, 2A_2, M_5^+ + M_5^-, Z_2 + Z_3, R_1^+ + R_1^-, X_1 + X_2]$                      | 3 |
| $[(\blacksquare)^{2T} + \Gamma_1^+ + \Gamma_1^-, A_1 + A_2, M_5^+ + M_5^-, Z_2 + Z_3, 2R_1^-, X_1 + X_2]$                        | 3 |
| $[(\blacksquare)^{2T} + \Gamma_1^+ + \Gamma_1^-, A_1 + A_2, M_5^+ + M_5^-, Z_2 + Z_3, R_1^+ + R_1^-, X_1 + X_2]$                 | 1 |
| $[(\blacksquare)^{2T} + \Gamma_1^+ + \Gamma_1^-, 2A_2, M_5^+ + M_5^-, Z_2 + Z_3, 2R_1^+, X_1 + X_2]$                             | 1 |
| $[(\blacksquare)^{2T} + \Gamma_1^+ + \Gamma_1^-, A_1 + A_2, M_5^+ + M_5^-, Z_2 + Z_3, 2R_1^+, X_1 + X_2]$                        | 3 |
| $[(\blacksquare)^{2T} + \Gamma_1^+ + \Gamma_1^-, 2A_1, M_5^+ + M_5^-, Z_2 + Z_3, 2R_1^-, X_1 + X_2]$                             | 1 |
| $[(\blacksquare)^{2T} + \Gamma_1^+ + \Gamma_1^-, 2A_1, M_5^+ + M_5^-, Z_2 + Z_3, R_1^+ + R_1^-, X_1 + X_2]$                      | 3 |
| $[(\blacksquare)^{2T} + \Gamma_1^+ + \Gamma_1^-, 2A_1, M_5^+ + M_5^-, Z_2 + Z_3, 2R_1^+, X_1 + X_2]$                             | 1 |

2nd minimal solution:  $\mu_2^T = 6$  (2240 symmetry vectors)

Space group 129 ( $\mathbb{Z}_1$ )

1st minimal solution:  $\mu_1^T = 4$  (10 symmetry vectors)

| $\mathbf{n}^T$                                                                                                       |
|----------------------------------------------------------------------------------------------------------------------|
| $[(\blacksquare)^{2T} + \Gamma_1^- + \Gamma_2^+, A_1 + A_4, M_1 + M_4, Z_2^+ + Z_3^+ + Z_5^+, R_1 + R_2, X_1 + X_2]$ |
| $[(\blacksquare)^{2T} + \Gamma_1^+ + \Gamma_1^-, A_3 + A_4, M_3 + M_4, Z_1^+ + Z_3^+ + Z_5^+, R_1 + R_2, X_1 + X_2]$ |
| $[(\blacksquare)^{2T} + \Gamma_1^- + \Gamma_2^+, A_2 + A_4, M_1 + M_4, Z_1^- + Z_4^- + Z_5^-, R_1 + R_2, X_1 + X_2]$ |
| $[(\blacksquare)^{2T} + \Gamma_1^+ + \Gamma_1^-, A_3 + A_4, M_3 + M_4, Z_1^- + Z_3^- + Z_5^-, R_1 + R_2, X_1 + X_2]$ |
| $[(\blacksquare)^{2T} + \Gamma_2^+ + \Gamma_2^-, A_1 + A_2, 2M_1, Z_2^- + Z_4^- + Z_5^-, R_1 + R_2, X_1 + X_2]$      |
| $[(\blacksquare)^{2T} + \Gamma_1^+ + \Gamma_2^-, A_1 + A_3, M_1 + M_3, Z_2^- + Z_3^- + Z_5^-, R_1 + R_2, X_1 + X_2]$ |
| $[(\blacksquare)^{2T} + \Gamma_2^+ + \Gamma_2^-, A_1 + A_2, 2M_1, Z_2^+ + Z_4^+ + Z_5^+, R_1 + R_2, X_1 + X_2]$      |
| $[(\blacksquare)^{2T} + \Gamma_1^+ + \Gamma_1^-, A_1 + A_2, M_1 + M_2, Z_1^+ + Z_3^+ + Z_5^+, R_1 + R_2, X_1 + X_2]$ |
| $[(\blacksquare)^{2T} + \Gamma_1^+ + \Gamma_1^-, A_1 + A_2, M_1 + M_2, Z_1^- + Z_3^- + Z_5^-, R_1 + R_2, X_1 + X_2]$ |
| $[(\blacksquare)^{2T} + \Gamma_1^+ + \Gamma_2^-, A_2 + A_3, M_1 + M_3, Z_1^+ + Z_4^+ + Z_5^+, R_1 + R_2, X_1 + X_2]$ |

2nd minimal solution:  $\mu_2^T = 6$  (130 symmetry vectors)

Space group 130 ( $\mathbb{Z}_2$ )

1st minimal solution:  $\mu_1^T = 4$  (6 symmetry vectors & filling-enforced topology)

| $\mathbf{n}^T$                                                                                           | $\mathbf{v}^T \in \mathbb{Z}_2$ |
|----------------------------------------------------------------------------------------------------------|---------------------------------|
| $[(\blacksquare)^{2T} + \Gamma_1^+ + \Gamma_1^-, A_3 + A_4, M_3 + M_4, Z_2 + Z_4, R_1 + R_2, X_1 + X_2]$ | 1                               |
| $[(\blacksquare)^{2T} + \Gamma_1^+ + \Gamma_1^-, A_1 + A_2, M_1 + M_2, Z_2 + Z_4, R_1 + R_2, X_1 + X_2]$ | 1                               |
| $[(\blacksquare)^{2T} + \Gamma_2^+ + \Gamma_2^-, A_1 + A_2, 2M_1, Z_1 + Z_4, R_1 + R_2, X_1 + X_2]$      | 1                               |
| $[(\blacksquare)^{2T} + \Gamma_1^+ + \Gamma_1^-, A_3 + A_4, M_3 + M_4, Z_2 + Z_3, R_1 + R_2, X_1 + X_2]$ | 1                               |
| $[(\blacksquare)^{2T} + \Gamma_1^+ + \Gamma_1^-, A_1 + A_2, M_1 + M_2, Z_2 + Z_3, R_1 + R_2, X_1 + X_2]$ | 1                               |
| $[(\blacksquare)^{2T} + \Gamma_2^+ + \Gamma_2^-, A_1 + A_2, 2M_1, Z_1 + Z_3, R_1 + R_2, X_1 + X_2]$      | 1                               |

2nd minimal solution:  $\mu_2^T = 8$  (126 symmetry vectors)

Space group 131 ( $\mathbb{Z}_1$ )

1st minimal solution:  $\mu_1^T = 2$  (4 symmetry vectors)

| $\mathbf{n}^T$                                                                 |
|--------------------------------------------------------------------------------|
| $[(\blacksquare)^{2T}, A_2, M_2^- + M_3^+, Z_4, R_1^- + R_4^-, X_2^+ + X_3^-]$ |
| $[(\blacksquare)^{2T}, A_1, M_2^+ + M_3^-, Z_3, R_2^- + R_3^-, X_2^- + X_3^-]$ |
| $[(\blacksquare)^{2T}, A_2, M_2^- + M_3^+, Z_3, R_2^+ + R_3^+, X_2^+ + X_3^+]$ |
| $[(\blacksquare)^{2T}, A_1, M_2^+ + M_3^-, Z_4, R_1^+ + R_4^+, X_2^- + X_3^-]$ |

2nd minimal solution:  $\mu_2^T = 4$  (248 symmetry vectors)

Space group 132 ( $\mathbb{Z}_1$ )

1st minimal solution:  $\mu_1^T = 4$  (44 symmetry vectors)

| $\mathbf{n}^T$                                                                                                                           |
|------------------------------------------------------------------------------------------------------------------------------------------|
| $[(\blacksquare)^{2T} + \Gamma_1^+ + \Gamma_4^+, A_1 + A_4, M_1^+ + M_2^- + M_5^-, Z_1 + Z_4, 2R_2, X_3^+ + 2X_3^- + X_4^-]$             |
| $[(\blacksquare)^{2T} + \Gamma_1^+ + \Gamma_4^+, A_1 + A_4, M_3^- + M_4^+ + M_5^-, Z_1 + Z_4, R_1 + R_2, X_2^+ + X_2^- + X_3^- + X_4^-]$ |
| $[(\blacksquare)^{2T} + \Gamma_1^+ + \Gamma_2^-, A_1 + A_4, M_2^- + M_3^- + M_5^-, Z_1 + Z_4, 2R_2, X_3^+ + X_3^- + X_4^+ + X_4^-]$      |
| $[(\blacksquare)^{2T} + \Gamma_1^+ + \Gamma_2^-, A_1 + A_4, M_2^- + M_3^- + M_5^-, Z_1 + Z_4, R_1 + R_2, X_1^- + X_2^- + X_3^- + X_4^-]$ |
| $[(\blacksquare)^{2T} + \Gamma_1^+ + \Gamma_4^+, A_1 + A_4, M_1^+ + M_2^- + M_5^-, Z_1 + Z_4, R_1 + R_2, X_1^+ + X_2^+ + X_3^+ + X_3^-]$ |
| $[(\blacksquare)^{2T} + \Gamma_1^+ + \Gamma_4^+, A_1 + A_4, M_3^- + M_4^+ + M_5^-, Z_1 + Z_4, 2R_1, X_1^+ + 2X_2^+ + X_2^-]$             |
| $[(\blacksquare)^{2T} + \Gamma_1^+ + \Gamma_2^-, A_1 + A_4, M_2^- + M_3^- + M_5^-, Z_1 + Z_4, R_1 + R_2, X_1^+ + X_2^+ + X_3^+ + X_4^+]$ |
| $[(\blacksquare)^{2T} + \Gamma_1^+ + \Gamma_2^-, A_1 + A_4, M_2^- + M_3^- + M_5^-, Z_1 + Z_4, 2R_1, X_1^+ + X_1^- + X_2^+ + X_2^-]$      |
| $[(\blacksquare)^{2T} + \Gamma_3^- + \Gamma_4^+, A_1 + A_4, M_2^- + M_3^- + M_5^-, Z_1 + Z_4, R_1 + R_2, X_2^+ + X_2^- + X_3^+ + X_3^-]$ |
| $[(\blacksquare)^{2T} + \Gamma_1^+ + \Gamma_4^+, A_1 + A_3, M_1^+ + M_2^- + M_5^-, Z_1 + Z_3, 2R_2, X_3^+ + 2X_3^- + X_4^-]$             |
| $[(\blacksquare)^{2T} + \Gamma_1^+ + \Gamma_4^+, A_1 + A_3, M_3^- + M_4^+ + M_5^-, Z_1 + Z_3, R_1 + R_2, X_2^+ + X_2^- + X_3^- + X_4^-]$ |
| $[(\blacksquare)^{2T} + \Gamma_1^+ + \Gamma_2^-, A_1 + A_3, M_2^- + M_3^- + M_5^-, Z_1 + Z_3, 2R_2, X_3^+ + X_3^- + X_4^+ + X_4^-]$      |
| $[(\blacksquare)^{2T} + \Gamma_1^+ + \Gamma_2^-, A_1 + A_3, M_2^- + M_3^- + M_5^-, Z_1 + Z_3, R_1 + R_2, X_1^- + X_2^- + X_3^- + X_4^-]$ |
| $[(\blacksquare)^{2T} + \Gamma_1^+ + \Gamma_4^+, A_1 + A_3, M_1^+ + M_2^- + M_5^-, Z_1 + Z_3, R_1 + R_2, X_1^+ + X_2^+ + X_3^+ + X_3^-]$ |
| $[(\blacksquare)^{2T} + \Gamma_1^+ + \Gamma_4^+, A_1 + A_3, M_3^- + M_4^+ + M_5^-, Z_1 + Z_3, 2R_1, X_1^+ + 2X_2^+ + X_2^-]$             |
| $[(\blacksquare)^{2T} + \Gamma_1^+ + \Gamma_2^-, A_1 + A_3, M_2^- + M_3^- + M_5^-, Z_1 + Z_3, R_1 + R_2, X_1^+ + X_2^+ + X_3^+ + X_4^+]$ |
| $[(\blacksquare)^{2T} + \Gamma_1^+ + \Gamma_2^-, A_1 + A_3, M_2^- + M_3^- + M_5^-, Z_1 + Z_3, 2R_1, X_1^+ + X_1^- + X_2^+ + X_2^-]$      |
| $[(\blacksquare)^{2T} + \Gamma_3^- + \Gamma_4^+, A_1 + A_3, M_2^- + M_3^- + M_5^-, Z_1 + Z_3, R_1 + R_2, X_2^+ + X_2^- + X_3^+ + X_3^-]$ |
| $[(\blacksquare)^{2T} + \Gamma_5^-, A_1 + A_2, M_1^+ + M_2^+ + M_2^- + M_3^+, Z_3 + Z_4, 2R_2, X_3^+ + 2X_3^- + X_4^-]$                  |
| $[(\blacksquare)^{2T} + \Gamma_5^-, A_1 + A_2, M_1^+ + M_2^+ + M_2^- + M_3^+, Z_3 + Z_4, R_1 + R_2, X_1^+ + X_2^+ + X_3^+ + X_3^-]$      |
| $[(\blacksquare)^{2T} + \Gamma_5^-, A_1 + A_2, M_1^- + M_2^+ + M_2^- + M_3^-, Z_3 + Z_4, 2R_2, 2X_3^+ + X_3^- + X_4^+]$                  |
| $[(\blacksquare)^{2T} + \Gamma_5^-, A_1 + A_2, M_2^- + M_3^+ + M_3^- + M_4^-, Z_3 + Z_4, R_1 + R_2, X_2^+ + X_2^- + X_3^+ + X_4^+]$      |
| $[(\blacksquare)^{2T} + \Gamma_5^-, A_1 + A_2, M_1^- + M_2^+ + M_2^- + M_3^-, Z_3 + Z_4, R_1 + R_2, X_1^- + X_2^- + X_3^+ + X_3^-]$      |
| $[(\blacksquare)^{2T} + \Gamma_5^-, A_1 + A_2, M_2^+ + M_3^+ + M_3^- + M_4^+, Z_3 + Z_4, R_1 + R_2, X_2^+ + X_2^- + X_3^- + X_4^-]$      |
| $[(\blacksquare)^{2T} + \Gamma_5^-, A_1 + A_2, M_2^+ + M_3^+ + M_3^- + M_4^+, Z_3 + Z_4, 2R_1, X_1^+ + 2X_2^+ + X_2^-]$                  |
| $[(\blacksquare)^{2T} + \Gamma_5^-, A_1 + A_2, M_2^- + M_3^+ + M_3^- + M_4^-, Z_3 + Z_4, 2R_1, X_1^- + X_2^+ + 2X_2^-]$                  |
| $[(\blacksquare)^{2T} + \Gamma_1^- + \Gamma_4^-, A_2 + A_4, M_1^- + M_2^+ + M_5^+, Z_2 + Z_4, 2R_2, 2X_3^+ + X_3^- + X_4^+]$             |
| $[(\blacksquare)^{2T} + \Gamma_1^- + \Gamma_4^-, A_2 + A_4, M_3^+ + M_4^- + M_5^+, Z_2 + Z_4, R_1 + R_2, X_2^+ + X_2^- + X_3^+ + X_4^+]$ |
| $[(\blacksquare)^{2T} + \Gamma_1^- + \Gamma_4^-, A_2 + A_4, M_1^- + M_2^+ + M_5^+, Z_2 + Z_4, R_1 + R_2, X_1^- + X_2^- + X_3^+ + X_3^-]$ |
| $[(\blacksquare)^{2T} + \Gamma_1^- + \Gamma_4^-, A_2 + A_4, M_3^+ + M_4^- + M_5^+, Z_2 + Z_4, 2R_1, X_1^- + X_2^+ + 2X_2^-]$             |
| $[(\blacksquare)^{2T} + \Gamma_3^+ + \Gamma_4^-, A_2 + A_4, M_2^+ + M_3^+ + M_5^+, Z_2 + Z_4, R_1 + R_2, X_2^+ + X_2^- + X_3^+ + X_3^-]$ |
| $[(\blacksquare)^{2T} + \Gamma_1^- + \Gamma_4^-, A_2 + A_3, M_1^- + M_2^+ + M_5^+, Z_2 + Z_3, 2R_2, 2X_3^+ + X_3^- + X_4^+]$             |
| $[(\blacksquare)^{2T} + \Gamma_1^- + \Gamma_4^-, A_2 + A_3, M_3^+ + M_4^- + M_5^+, Z_2 + Z_3, R_1 + R_2, X_2^+ + X_2^- + X_3^+ + X_4^+]$ |
| $[(\blacksquare)^{2T} + \Gamma_1^- + \Gamma_4^-, A_2 + A_3, M_1^- + M_2^+ + M_5^+, Z_2 + Z_3, R_1 + R_2, X_1^- + X_2^- + X_3^+ + X_3^-]$ |

... continued on next page

... continued from previous page

---

|                                                                                                                                          |
|------------------------------------------------------------------------------------------------------------------------------------------|
| $[(\blacksquare)^{2T} + \Gamma_1^- + \Gamma_4^-, A_2 + A_3, M_3^+ + M_4^- + M_5^+, Z_2 + Z_3, 2R_1, X_1^- + X_2^+ + 2X_2^-]$             |
| $[(\blacksquare)^{2T} + \Gamma_3^+ + \Gamma_4^-, A_2 + A_3, M_2^+ + M_3^+ + M_5^+, Z_2 + Z_3, R_1 + R_2, X_2^+ + X_2^- + X_3^+ + X_3^-]$ |
| $[(\blacksquare)^{2T} + \Gamma_1^- + \Gamma_2^+, A_2 + A_4, M_2^+ + M_3^+ + M_5^+, Z_2 + Z_4, 2R_2, X_3^+ + X_3^- + X_4^+ + X_4^-]$      |
| $[(\blacksquare)^{2T} + \Gamma_1^- + \Gamma_2^+, A_2 + A_4, M_2^+ + M_3^+ + M_5^+, Z_2 + Z_4, R_1 + R_2, X_1^- + X_2^- + X_3^- + X_4^-]$ |
| $[(\blacksquare)^{2T} + \Gamma_1^- + \Gamma_2^+, A_2 + A_4, M_2^+ + M_3^+ + M_5^+, Z_2 + Z_4, R_1 + R_2, X_1^+ + X_2^+ + X_3^+ + X_4^+]$ |
| $[(\blacksquare)^{2T} + \Gamma_1^- + \Gamma_2^+, A_2 + A_4, M_2^+ + M_3^+ + M_5^+, Z_2 + Z_4, 2R_1, X_1^+ + X_1^- + X_2^+ + X_2^-]$      |
| $[(\blacksquare)^{2T} + \Gamma_1^- + \Gamma_2^+, A_2 + A_3, M_2^+ + M_3^+ + M_5^+, Z_2 + Z_3, 2R_2, X_3^+ + X_3^- + X_4^+ + X_4^-]$      |
| $[(\blacksquare)^{2T} + \Gamma_1^- + \Gamma_2^+, A_2 + A_3, M_2^+ + M_3^+ + M_5^+, Z_2 + Z_3, R_1 + R_2, X_1^- + X_2^- + X_3^- + X_4^-]$ |
| $[(\blacksquare)^{2T} + \Gamma_1^- + \Gamma_2^+, A_2 + A_3, M_2^+ + M_3^+ + M_5^+, Z_2 + Z_3, R_1 + R_2, X_1^+ + X_2^+ + X_3^+ + X_4^+]$ |
| $[(\blacksquare)^{2T} + \Gamma_1^- + \Gamma_2^+, A_2 + A_3, M_2^+ + M_3^+ + M_5^+, Z_2 + Z_3, 2R_1, X_1^+ + X_1^- + X_2^+ + X_2^-]$      |

---

2nd minimal solution:  $\mu_2^T = 6$  (936 symmetry vectors)

Space group 133 ( $\mathbb{Z}_2$ )

1st minimal solution:  $\mu_1^T = 2$  (4 symmetry vectors & filling-enforced topology)

| $\mathbf{n}^T$                                   | $\mathbf{v}^T \in \mathbb{Z}_2$ |
|--------------------------------------------------|---------------------------------|
| $[(\blacksquare)^{2T}, A_4, M_3, Z_3, R_2, X_2]$ | 1                               |
| $[(\blacksquare)^{2T}, A_3, M_3, Z_3, R_2, X_2]$ | 1                               |
| $[(\blacksquare)^{2T}, A_4, M_3, Z_4, R_1, X_2]$ | 1                               |
| $[(\blacksquare)^{2T}, A_3, M_3, Z_4, R_1, X_2]$ | 1                               |

2nd minimal solution:  $\mu_2^T = 6$  (92 symmetry vectors)

Space group 134 ( $\mathbb{Z}_1$ )

1st minimal solution:  $\mu_1^T = 4$  (8 symmetry vectors)

| $\mathbf{n}^T$                                                                                                       |
|----------------------------------------------------------------------------------------------------------------------|
| $[(\blacksquare)^{2T} + \Gamma_3^- + \Gamma_4^+, A_2^- + A_3^- + A_5^-, M_1 + M_3, Z_1 + Z_3, R_1 + R_2, 2X_2]$      |
| $[(\blacksquare)^{2T} + \Gamma_3^- + \Gamma_4^+, A_1^+ + A_4^+ + A_5^+, M_1 + M_3, Z_1 + Z_4, R_1 + R_2, 2X_2]$      |
| $[(\blacksquare)^{2T} + \Gamma_1^+ + \Gamma_2^-, A_2^- + A_3^- + A_5^-, M_1 + M_3, Z_1 + Z_3, R_1 + R_2, X_1 + X_2]$ |
| $[(\blacksquare)^{2T} + \Gamma_1^+ + \Gamma_2^-, A_1^+ + A_4^+ + A_5^+, M_1 + M_3, Z_1 + Z_4, R_1 + R_2, X_1 + X_2]$ |
| $[(\blacksquare)^{2T} + \Gamma_3^+ + \Gamma_4^-, A_1^- + A_4^- + A_5^-, M_2 + M_3, Z_2 + Z_4, R_1 + R_2, 2X_2]$      |
| $[(\blacksquare)^{2T} + \Gamma_1^- + \Gamma_2^+, A_1^- + A_4^- + A_5^-, M_2 + M_3, Z_2 + Z_4, R_1 + R_2, X_1 + X_2]$ |
| $[(\blacksquare)^{2T} + \Gamma_3^+ + \Gamma_4^-, A_2^+ + A_3^+ + A_5^+, M_2 + M_3, Z_2 + Z_3, R_1 + R_2, 2X_2]$      |
| $[(\blacksquare)^{2T} + \Gamma_1^- + \Gamma_2^+, A_2^+ + A_3^+ + A_5^+, M_2 + M_3, Z_2 + Z_3, R_1 + R_2, X_1 + X_2]$ |

2nd minimal solution:  $\mu_2^T = 6$  (100 symmetry vectors)

Space group 135 ( $\mathbb{Z}_1$ )

1st minimal solution:  $\mu_1^T = 8$  (38 symmetry vectors)

2nd minimal solution:  $\mu_2^T = 12$  (430 symmetry vectors)

Space group 136 ( $Z_1$ )

1st minimal solution:  $\mu_1^T = 4$  (12 symmetry vectors)

| $\mathbf{n}^\top$                                                                                                           |
|-----------------------------------------------------------------------------------------------------------------------------|
| $[(\blacksquare)^{2\top} + \Gamma_1^+ + \Gamma_2^-, A_1 + A_4, M_2^- + M_3^- + M_5^-, Z_1 + Z_4, 2R_1^-, X_1 + X_2]$        |
| $[(\blacksquare)^{2\top} + \Gamma_1^+ + \Gamma_2^-, A_1 + A_4, M_2^- + M_3^- + M_5^-, Z_1 + Z_4, R_1^+ + R_1^-, X_1 + X_2]$ |
| $[(\blacksquare)^{2\top} + \Gamma_1^+ + \Gamma_2^-, A_1 + A_4, M_2^- + M_3^- + M_5^-, Z_1 + Z_4, 2R_1^+, X_1 + X_2]$        |
| $[(\blacksquare)^{2\top} + \Gamma_1^+ + \Gamma_2^-, A_1 + A_3, M_2^- + M_3^- + M_5^-, Z_1 + Z_3, 2R_1^-, X_1 + X_2]$        |

... continued on next page



... continued from previous page

---

|                                                                                                                          |
|--------------------------------------------------------------------------------------------------------------------------|
| $[(\blacksquare)^{2T} + \Gamma_1^+ + \Gamma_2^-, A_1 + A_3, M_2^- + M_3^- + M_5^-, Z_1 + Z_3, R_1^+ + R_1^-, X_1 + X_2]$ |
| $[(\blacksquare)^{2T} + \Gamma_1^+ + \Gamma_2^-, A_1 + A_3, M_2^- + M_3^- + M_5^-, Z_1 + Z_3, 2R_1^+, X_1 + X_2]$        |
| $[(\blacksquare)^{2T} + \Gamma_1^- + \Gamma_2^+, A_2 + A_4, M_2^+ + M_3^+ + M_5^+, Z_2 + Z_4, 2R_1^-, X_1 + X_2]$        |
| $[(\blacksquare)^{2T} + \Gamma_1^- + \Gamma_2^+, A_2 + A_4, M_2^+ + M_3^+ + M_5^+, Z_2 + Z_4, R_1^+ + R_1^-, X_1 + X_2]$ |
| $[(\blacksquare)^{2T} + \Gamma_1^- + \Gamma_2^+, A_2 + A_4, M_2^+ + M_3^+ + M_5^+, Z_2 + Z_4, 2R_1^+, X_1 + X_2]$        |
| $[(\blacksquare)^{2T} + \Gamma_1^- + \Gamma_2^+, A_2 + A_3, M_2^+ + M_3^+ + M_5^+, Z_2 + Z_3, 2R_1^-, X_1 + X_2]$        |
| $[(\blacksquare)^{2T} + \Gamma_1^- + \Gamma_2^+, A_2 + A_3, M_2^+ + M_3^+ + M_5^+, Z_2 + Z_3, R_1^+ + R_1^-, X_1 + X_2]$ |
| $[(\blacksquare)^{2T} + \Gamma_1^- + \Gamma_2^+, A_2 + A_3, M_2^+ + M_3^+ + M_5^+, Z_2 + Z_3, 2R_1^+, X_1 + X_2]$        |

---

2nd minimal solution:  $\mu_2^T = 6$  (184 symmetry vectors)

Space group 137 ( $\mathbb{Z}_1$ )

1st minimal solution:  $\mu_1^T = 6$  (12 symmetry vectors)

---

| $\mathbf{n}^T$                                                                                                                            |
|-------------------------------------------------------------------------------------------------------------------------------------------|
| $[(\blacksquare)^{2T} + \Gamma_1^+ + \Gamma_2^+ + \Gamma_5^+, A_2 + A_3 + A_4, M_1 + M_3 + M_4, Z_1 + Z_3 + Z_4, 2R_1 + R_2, 2X_1 + X_2]$ |
| $[(\blacksquare)^{2T} + \Gamma_1^+ + \Gamma_2^+ + \Gamma_5^+, A_1 + A_3 + A_4, M_1 + M_3 + M_4, Z_1 + Z_3 + Z_4, 2R_1 + R_2, 2X_1 + X_2]$ |
| $[(\blacksquare)^{2T} + \Gamma_1^+ + \Gamma_2^+ + \Gamma_5^+, 3A_2, 2M_1 + M_2, Z_1 + Z_3 + Z_4, 2R_1 + R_2, 2X_1 + X_2]$                 |
| $[(\blacksquare)^{2T} + \Gamma_1^+ + \Gamma_2^+ + \Gamma_5^+, A_1 + 2A_2, 2M_1 + M_2, Z_1 + Z_3 + Z_4, 2R_1 + R_2, 2X_1 + X_2]$           |
| $[(\blacksquare)^{2T} + \Gamma_1^+ + \Gamma_2^+ + \Gamma_5^+, 2A_1 + A_2, 2M_1 + M_2, Z_1 + Z_3 + Z_4, 2R_1 + R_2, 2X_1 + X_2]$           |
| $[(\blacksquare)^{2T} + \Gamma_1^+ + \Gamma_2^+ + \Gamma_5^+, 3A_1, 2M_1 + M_2, Z_1 + Z_3 + Z_4, 2R_1 + R_2, 2X_1 + X_2]$                 |
| $[(\blacksquare)^{2T} + \Gamma_1^- + \Gamma_2^- + \Gamma_5^-, A_2 + A_3 + A_4, M_1 + M_3 + M_4, Z_2 + Z_3 + Z_4, R_1 + 2R_2, X_1 + 2X_2]$ |
| $[(\blacksquare)^{2T} + \Gamma_1^- + \Gamma_2^- + \Gamma_5^-, 3A_2, 2M_1 + M_2, Z_2 + Z_3 + Z_4, R_1 + 2R_2, X_1 + 2X_2]$                 |
| $[(\blacksquare)^{2T} + \Gamma_1^- + \Gamma_2^- + \Gamma_5^-, A_1 + A_3 + A_4, M_1 + M_3 + M_4, Z_2 + Z_3 + Z_4, R_1 + 2R_2, X_1 + 2X_2]$ |
| $[(\blacksquare)^{2T} + \Gamma_1^- + \Gamma_2^- + \Gamma_5^-, A_1 + 2A_2, 2M_1 + M_2, Z_2 + Z_3 + Z_4, R_1 + 2R_2, X_1 + 2X_2]$           |
| $[(\blacksquare)^{2T} + \Gamma_1^- + \Gamma_2^- + \Gamma_5^-, 2A_1 + A_2, 2M_1 + M_2, Z_2 + Z_3 + Z_4, R_1 + 2R_2, X_1 + 2X_2]$           |
| $[(\blacksquare)^{2T} + \Gamma_1^- + \Gamma_2^- + \Gamma_5^-, 3A_1, 2M_1 + M_2, Z_2 + Z_3 + Z_4, R_1 + 2R_2, X_1 + 2X_2]$                 |

---

2nd minimal solution:  $\mu_2^T = 8$  (68 symmetry vectors)

Space group 138 ( $\mathbb{Z}_1$ )

1st minimal solution:  $\mu_1^T = 4$  (4 symmetry vectors)

---

| $\mathbf{n}^T$                                                                                                       |
|----------------------------------------------------------------------------------------------------------------------|
| $[(\blacksquare)^{2T} + \Gamma_1^+ + \Gamma_2^-, A_2^- + A_3^- + A_5^-, M_1 + M_3, Z_1 + Z_4, R_1 + R_2, X_1 + X_2]$ |
| $[(\blacksquare)^{2T} + \Gamma_1^- + \Gamma_2^+, A_1^- + A_4^- + A_5^-, M_1 + M_4, Z_2 + Z_3, R_1 + R_2, X_1 + X_2]$ |
| $[(\blacksquare)^{2T} + \Gamma_1^+ + \Gamma_2^-, A_1^+ + A_4^+ + A_5^+, M_1 + M_3, Z_1 + Z_3, R_1 + R_2, X_1 + X_2]$ |
| $[(\blacksquare)^{2T} + \Gamma_1^- + \Gamma_2^+, A_2^+ + A_3^+ + A_5^+, M_1 + M_4, Z_2 + Z_4, R_1 + R_2, X_1 + X_2]$ |

---

2nd minimal solution:  $\mu_2^T = 8$  (138 symmetry vectors)

Space group 139 ( $\mathbb{Z}_1$ )

1st minimal solution:  $\mu_1^T = 3$  (36 symmetry vectors)

| $\mathbf{n}^T$                                                                                                     |
|--------------------------------------------------------------------------------------------------------------------|
| $[(\blacksquare)^{2T} + \Gamma_1^+, M_3^- + M_5^-, P_3 + P_5, X_2^- + X_3^- + X_4^-, N_1^- + 2N_2^-]$              |
| $[(\blacksquare)^{2T} + \Gamma_1^+, M_3^- + M_5^-, P_1 + P_5, X_2^- + X_3^- + X_4^-, N_1^+ + N_1^- + N_2^-]$       |
| $[(\blacksquare)^{2T} + \Gamma_1^+, M_3^- + M_5^-, 2P_3 + P_4, X_1^+ + X_2^+ + X_2^-, N_2^+ + 2N_2^-]$             |
| $[(\blacksquare)^{2T} + \Gamma_1^+, M_3^- + M_5^-, P_1 + P_3 + P_4, X_1^+ + X_2^+ + X_2^-, N_1^+ + N_2^+ + N_2^-]$ |
| $[(\blacksquare)^{2T} + \Gamma_1^+, M_3^- + M_5^-, 2P_1 + P_4, X_1^+ + X_2^+ + X_2^-, 2N_1^+ + N_2^+]$             |
| $[(\blacksquare)^{2T} + \Gamma_2^+, M_4^- + M_5^-, P_4 + P_5, X_2^+ + X_3^+ + X_3^-, N_1^+ + N_2^+ + N_2^-]$       |
| $[(\blacksquare)^{2T} + \Gamma_1^+, M_3^- + M_5^-, P_3 + P_5, X_2^- + X_3^- + X_4^-, N_1^+ + N_2^+ + N_2^-]$       |
| $[(\blacksquare)^{2T} + \Gamma_1^+, M_3^- + M_5^-, P_1 + P_5, X_2^- + X_3^- + X_4^-, 2N_1^+ + N_2^+]$              |
| $[(\blacksquare)^{2T} + \Gamma_1^+, M_3^- + M_5^-, P_2 + 2P_3, X_1^+ + X_2^+ + X_2^-, N_1^- + 2N_2^-]$             |
| $[(\blacksquare)^{2T} + \Gamma_1^+, M_3^- + M_5^-, P_1 + P_2 + P_3, X_1^+ + X_2^+ + X_2^-, N_1^+ + N_1^- + N_2^-]$ |
| $[(\blacksquare)^{2T} + \Gamma_1^+, M_3^- + M_5^-, 2P_1 + P_2, X_1^+ + X_2^+ + X_2^-, 2N_1^+ + N_1^-]$             |
| $[(\blacksquare)^{2T} + \Gamma_2^+, M_4^- + M_5^-, P_2 + P_5, X_2^+ + X_3^+ + X_3^-, N_1^+ + N_1^- + N_2^-]$       |
| $[(\blacksquare)^{2T} + \Gamma_1^+, M_3^- + M_5^-, P_2 + 2P_3, X_1^+ + X_2^+ + X_2^-, N_1^+ + N_2^+ + N_2^-]$      |
| $[(\blacksquare)^{2T} + \Gamma_1^+, M_3^- + M_5^-, P_1 + P_2 + P_3, X_1^+ + X_2^+ + X_2^-, 2N_1^+ + N_2^+]$        |
| $[(\blacksquare)^{2T} + \Gamma_2^+, M_4^- + M_5^-, P_2 + P_5, X_2^+ + X_3^+ + X_3^-, 2N_1^+ + N_2^+]$              |
| $[(\blacksquare)^{2T} + \Gamma_1^+, M_3^- + M_5^-, P_1 + P_3 + P_4, X_1^+ + X_2^+ + X_2^-, N_1^- + 2N_2^-]$        |
| $[(\blacksquare)^{2T} + \Gamma_1^+, M_3^- + M_5^-, 2P_1 + P_4, X_1^+ + X_2^+ + X_2^-, N_1^+ + N_1^- + N_2^-]$      |
| $[(\blacksquare)^{2T} + \Gamma_2^-, M_4^+ + M_5^+, P_3 + P_5, X_2^- + X_3^- + X_3^-, N_1^- + N_2^+ + N_2^-]$       |
| $[(\blacksquare)^{2T} + \Gamma_2^-, M_4^+ + M_5^+, P_3 + P_5, X_2^- + X_3^- + X_3^-, N_1^+ + 2N_2^+]$              |
| $[(\blacksquare)^{2T} + \Gamma_2^-, M_4^+ + M_5^+, P_1 + P_5, X_2^- + X_3^- + X_3^-, 2N_1^- + N_2^-]$              |
| $[(\blacksquare)^{2T} + \Gamma_2^-, M_4^+ + M_5^+, P_1 + P_5, X_2^- + X_3^- + X_3^-, N_1^+ + N_1^- + N_2^+]$       |
| $[(\blacksquare)^{2T} + \Gamma_2^+, M_4^- + M_5^-, P_4 + P_5, X_2^+ + X_3^+ + X_3^-, N_1^- + 2N_2^-]$              |
| $[(\blacksquare)^{2T} + \Gamma_1^-, M_3^+ + M_5^+, P_4 + P_5, X_2^+ + X_3^+ + X_4^+, N_1^- + N_2^+ + N_2^-]$       |
| $[(\blacksquare)^{2T} + \Gamma_1^-, M_3^+ + M_5^+, P_3 + 2P_4, X_1^- + X_2^+ + X_2^-, 2N_2^+ + N_2^-]$             |
| $[(\blacksquare)^{2T} + \Gamma_1^-, M_3^+ + M_5^+, P_4 + P_5, X_2^+ + X_3^+ + X_4^+, N_1^+ + 2N_2^+]$              |
| $[(\blacksquare)^{2T} + \Gamma_1^-, M_3^+ + M_5^+, P_2 + P_5, X_2^+ + X_3^+ + X_4^+, 2N_1^- + N_2^-]$              |
| $[(\blacksquare)^{2T} + \Gamma_1^-, M_3^+ + M_5^+, P_2 + P_3 + P_4, X_1^- + X_2^+ + X_2^-, N_1^- + N_2^+ + N_2^-]$ |
| $[(\blacksquare)^{2T} + \Gamma_1^-, M_3^+ + M_5^+, P_2 + P_5, X_2^+ + X_3^+ + X_4^+, N_1^+ + N_1^- + N_2^+]$       |
| $[(\blacksquare)^{2T} + \Gamma_1^-, M_3^+ + M_5^+, P_2 + P_3 + P_4, X_1^- + X_2^+ + X_2^-, N_1^+ + 2N_2^+]$        |
| $[(\blacksquare)^{2T} + \Gamma_1^-, M_3^+ + M_5^+, 2P_2 + P_3, X_1^- + X_2^+ + X_2^-, 2N_1^- + N_2^-]$             |
| $[(\blacksquare)^{2T} + \Gamma_1^-, M_3^+ + M_5^+, 2P_2 + P_3, X_1^- + X_2^+ + X_2^-, N_1^+ + N_1^- + N_2^+]$      |
| $[(\blacksquare)^{2T} + \Gamma_1^-, M_3^+ + M_5^+, P_1 + 2P_4, X_1^- + X_2^+ + X_2^-, N_1^- + N_2^+ + N_2^-]$      |
| $[(\blacksquare)^{2T} + \Gamma_1^-, M_3^+ + M_5^+, P_1 + 2P_4, X_1^- + X_2^+ + X_2^-, N_1^+ + 2N_2^+]$             |
| $[(\blacksquare)^{2T} + \Gamma_1^-, M_3^+ + M_5^+, P_1 + P_2 + P_4, X_1^- + X_2^+ + X_2^-, 2N_1^- + N_2^-]$        |
| $[(\blacksquare)^{2T} + \Gamma_1^-, M_3^+ + M_5^+, P_1 + P_2 + P_4, X_1^- + X_2^+ + X_2^-, N_1^+ + N_1^- + N_2^+]$ |
| $[(\blacksquare)^{2T} + \Gamma_1^-, M_3^+ + M_5^+, P_1 + 2P_2, X_1^- + X_2^+ + X_2^-, N_1^+ + 2N_1^-]$             |

2nd minimal solution:  $\mu_2^T = 4$  (564 symmetry vectors)

Space group 140 ( $\mathbb{Z}_4$ )

1st minimal solution:  $\mu_1^T = 4$  (52 symmetry vectors)

| $\mathbf{n}^T$                                                                                                                 |
|--------------------------------------------------------------------------------------------------------------------------------|
| $[(\blacksquare)^{2T} + \Gamma_2^- + \Gamma_4^-, M_4^+ + M_4^- + M_5^+, 2P_2 + 2P_3, 2X_3^+ + X_3^- + X_4^+, 2N_1]$            |
| $[(\blacksquare)^{2T} + \Gamma_1^- + \Gamma_4^-, M_3^- + M_4^+ + M_5^+, P_1 + P_2 + 2P_3, X_3^+ + X_3^- + 2X_4^+, 2N_1]$       |
| $[(\blacksquare)^{2T} + \Gamma_2^+ + \Gamma_2^-, M_2^- + M_4^- + M_5^-, P_2 + P_3 + P_5, X_2^+ + X_2^- + X_3^+ + X_3^-, 2N_1]$ |
| $[(\blacksquare)^{2T} + \Gamma_2^+ + \Gamma_4^+, M_4^+ + M_4^- + M_5^-, 2P_2 + 2P_3, X_3^+ + 2X_3^- + X_4^-, 2N_1]$            |
| $[(\blacksquare)^{2T} + \Gamma_2^+ + \Gamma_4^+, M_4^+ + M_4^- + M_5^-, P_1 + P_2 + P_3 + P_4, X_3^+ + 2X_3^- + X_4^-, 2N_1]$  |
| $[(\blacksquare)^{2T} + \Gamma_2^+ + \Gamma_4^+, M_4^+ + M_4^- + M_5^-, P_2 + P_3 + P_5, X_1^+ + X_2^+ + X_3^+ + X_3^-, 2N_1]$ |

... continued on next page

... continued from previous page

$$\begin{aligned}
&[(\blacksquare)^{2T} + \Gamma_1^+ + \Gamma_2^-, M_1^- + M_4^- + M_5^-, 2P_2 + P_3 + P_4, 2X_3^+ + X_3^- + X_4^-, 2N_1] \\
&[(\blacksquare)^{2T} + \Gamma_1^+ + \Gamma_4^+, M_3^+ + M_4^- + M_5^-, 2P_2 + P_3 + P_4, X_3^+ + X_3^- + 2X_4^-, 2N_1] \\
&[(\blacksquare)^{2T} + \Gamma_1^+ + \Gamma_1^-, M_1^- + M_3^- + M_5^-, 2P_2 + 2P_3, X_3^+ + X_3^- + X_4^+ + X_4^-, 2N_1] \\
&[(\blacksquare)^{2T} + \Gamma_1^+ + \Gamma_1^-, M_1^- + M_3^- + M_5^-, P_2 + P_3 + P_5, X_1^- + X_2^- + X_3^- + X_4^-, 2N_1] \\
&[(\blacksquare)^{2T} + \Gamma_1^- + \Gamma_2^+, M_2^- + M_3^- + M_5^-, P_1 + P_3 + P_5, X_2^+ + X_2^- + X_3^- + X_4^+, 2N_1] \\
&[(\blacksquare)^{2T} + \Gamma_1^+ + \Gamma_1^-, M_1^- + M_3^- + M_5^-, P_1 + P_2 + P_3 + P_4, X_3^+ + X_3^- + X_4^+ + X_4^-, 2N_1] \\
&[(\blacksquare)^{2T} + \Gamma_1^+ + \Gamma_3^+, M_3^+ + M_3^- + M_5^-, P_2 + P_3 + P_5, X_2^+ + X_2^- + X_3^- + X_4^-, 2N_1] \\
&[(\blacksquare)^{2T} + \Gamma_2^+ + \Gamma_3^+, M_3^+ + M_4^+ + M_5^-, P_1 + P_3 + P_5, X_2^+ + X_2^- + 2X_3^-, 2N_1] \\
&[(\blacksquare)^{2T} + \Gamma_2^- + \Gamma_4^-, M_4^+ + M_4^- + M_5^+, P_2 + P_3 + P_5, X_1^- + X_2^- + X_3^+ + X_3^-, 2N_1] \\
&[(\blacksquare)^{2T} + \Gamma_1^- + \Gamma_4^-, M_3^- + M_4^+ + M_5^+, P_1 + P_3 + P_5, X_1^- + X_2^- + X_3^- + X_4^+, 2N_1] \\
&[(\blacksquare)^{2T} + \Gamma_2^- + \Gamma_4^-, M_4^+ + M_4^- + M_5^+, P_1 + P_2 + P_3 + P_4, 2X_3^+ + X_3^- + X_4^+, 2N_1] \\
&[(\blacksquare)^{2T} + \Gamma_1^- + \Gamma_4^-, M_3^- + M_4^+ + M_5^+, 2P_1 + P_3 + P_4, X_3^+ + X_3^- + 2X_4^+, 2N_1] \\
&[(\blacksquare)^{2T} + \Gamma_2^+ + \Gamma_2^-, M_2^- + M_4^- + M_5^-, P_1 + P_4 + P_5, X_2^+ + X_2^- + X_3^+ + X_3^-, 2N_1] \\
&[(\blacksquare)^{2T} + \Gamma_2^+ + \Gamma_4^+, M_4^+ + M_4^- + M_5^-, 2P_1 + 2P_4, X_3^+ + 2X_3^- + X_4^-, 2N_1] \\
&[(\blacksquare)^{2T} + \Gamma_2^+ + \Gamma_4^+, M_4^+ + M_4^- + M_5^-, P_1 + P_4 + P_5, X_1^+ + X_2^+ + X_3^+ + X_3^-, 2N_1] \\
&[(\blacksquare)^{2T} + \Gamma_1^+ + \Gamma_2^-, M_1^- + M_4^- + M_5^-, P_1 + P_2 + 2P_4, 2X_3^+ + X_3^- + X_4^-, 2N_1] \\
&[(\blacksquare)^{2T} + \Gamma_1^+ + \Gamma_4^+, M_3^+ + M_4^- + M_5^-, P_1 + P_2 + 2P_4, X_3^+ + X_3^- + 2X_4^-, 2N_1] \\
&[(\blacksquare)^{2T} + \Gamma_1^+ + \Gamma_1^-, M_1^- + M_3^- + M_5^-, P_1 + P_4 + P_5, X_1^- + X_2^- + X_3^- + X_4^-, 2N_1] \\
&[(\blacksquare)^{2T} + \Gamma_1^+ + \Gamma_1^-, M_1^- + M_3^- + M_5^-, 2P_1 + 2P_4, X_3^+ + X_3^- + X_4^+ + X_4^-, 2N_1] \\
&[(\blacksquare)^{2T} + \Gamma_1^+ + \Gamma_3^+, M_3^+ + M_3^- + M_5^-, P_1 + P_4 + P_5, X_2^+ + X_2^- + X_3^- + X_4^-, 2N_1] \\
&[(\blacksquare)^{2T} + \Gamma_2^- + \Gamma_4^-, M_4^+ + M_4^- + M_5^+, P_1 + P_4 + P_5, X_1^- + X_2^- + X_3^+ + X_3^-, 2N_1] \\
&[(\blacksquare)^{2T} + \Gamma_2^- + \Gamma_4^-, M_4^+ + M_4^- + M_5^+, 2P_1 + 2P_4, 2X_3^+ + X_3^- + X_4^+, 2N_1] \\
&[(\blacksquare)^{2T} + \Gamma_1^+ + \Gamma_2^-, M_1^- + M_4^- + M_5^-, P_2 + P_4 + P_5, X_1^+ + X_2^+ + 2X_3^-, 2N_1] \\
&[(\blacksquare)^{2T} + \Gamma_1^+ + \Gamma_4^+, M_3^+ + M_4^- + M_5^-, P_2 + P_4 + P_5, X_1^+ + X_2^+ + X_3^+ + X_4^-, 2N_1] \\
&[(\blacksquare)^{2T} + \Gamma_1^+ + \Gamma_1^-, M_1^- + M_3^- + M_5^-, P_2 + P_3 + P_5, X_1^+ + X_2^+ + X_3^+ + X_4^+, 2N_1] \\
&[(\blacksquare)^{2T} + \Gamma_1^+ + \Gamma_1^-, M_1^- + M_3^- + M_5^-, 2P_5, X_1^+ + X_1^- + X_2^+ + X_2^-, 2N_1] \\
&[(\blacksquare)^{2T} + \Gamma_1^+ + \Gamma_1^-, M_1^- + M_3^- + M_5^-, P_1 + P_4 + P_5, X_1^+ + X_2^+ + X_3^+ + X_4^+, 2N_1] \\
&[(\blacksquare)^{2T} + \Gamma_1^+ + \Gamma_3^+, M_3^+ + M_3^- + M_5^-, 2P_5, X_1^+ + 2X_2^+ + X_2^-, 2N_1] \\
&[(\blacksquare)^{2T} + \Gamma_2^- + \Gamma_3^-, M_3^- + M_4^- + M_5^+, P_2 + P_4 + P_5, X_2^+ + X_2^- + 2X_3^+, 2N_1] \\
&[(\blacksquare)^{2T} + \Gamma_1^- + \Gamma_3^-, M_3^- + M_3^- + M_5^+, P_2 + P_3 + P_5, X_2^+ + X_2^- + X_3^- + X_4^+, 2N_1] \\
&[(\blacksquare)^{2T} + \Gamma_1^- + \Gamma_3^-, M_3^- + M_3^- + M_5^+, 2P_5, X_1^- + X_2^+ + 2X_2^-, 2N_1] \\
&[(\blacksquare)^{2T} + \Gamma_1^- + \Gamma_3^-, M_3^- + M_3^- + M_5^+, P_1 + P_4 + P_5, X_2^+ + X_2^- + X_3^- + X_4^+, 2N_1] \\
&[(\blacksquare)^{2T} + \Gamma_1^+ + \Gamma_2^-, M_2^+ + M_3^+ + M_5^+, P_2 + P_4 + P_5, X_2^+ + X_2^- + X_3^+ + X_4^-, 2N_1] \\
&[(\blacksquare)^{2T} + \Gamma_1^+ + \Gamma_1^-, M_1^+ + M_3^+ + M_5^+, 2P_5, X_1^+ + X_1^- + X_2^+ + X_2^-, 2N_1] \\
&[(\blacksquare)^{2T} + \Gamma_1^+ + \Gamma_1^-, M_1^+ + M_3^+ + M_5^+, 2P_2 + 2P_3, X_3^+ + X_3^- + X_4^+ + X_4^-, 2N_1] \\
&[(\blacksquare)^{2T} + \Gamma_1^+ + \Gamma_1^-, M_1^+ + M_3^+ + M_5^+, P_2 + P_3 + P_5, X_1^- + X_2^- + X_3^- + X_4^-, 2N_1] \\
&[(\blacksquare)^{2T} + \Gamma_1^+ + \Gamma_1^-, M_1^+ + M_3^+ + M_5^+, P_1 + P_2 + P_3 + P_4, X_3^+ + X_3^- + X_4^+ + X_4^-, 2N_1] \\
&[(\blacksquare)^{2T} + \Gamma_1^+ + \Gamma_1^-, M_1^+ + M_3^+ + M_5^+, P_1 + P_4 + P_5, X_1^- + X_2^- + X_3^- + X_4^-, 2N_1] \\
&[(\blacksquare)^{2T} + \Gamma_1^+ + \Gamma_1^-, M_1^+ + M_3^+ + M_5^+, 2P_1 + 2P_4, X_3^+ + X_3^- + X_4^+ + X_4^-, 2N_1] \\
&[(\blacksquare)^{2T} + \Gamma_1^+ + \Gamma_1^-, M_1^+ + M_3^+ + M_5^+, P_2 + P_3 + P_5, X_1^+ + X_2^+ + X_3^+ + X_4^+, 2N_1] \\
&[(\blacksquare)^{2T} + \Gamma_2^+ + \Gamma_2^-, M_2^+ + M_4^+ + M_5^+, P_2 + P_3 + P_5, X_2^+ + X_2^- + X_3^+ + X_3^-, 2N_1] \\
&[(\blacksquare)^{2T} + \Gamma_2^+ + \Gamma_2^-, M_2^+ + M_4^+ + M_5^+, P_1 + P_4 + P_5, X_2^+ + X_2^- + X_3^+ + X_3^-, 2N_1] \\
&[(\blacksquare)^{2T} + \Gamma_1^+ + \Gamma_2^+, M_1^+ + M_4^+ + M_5^+, P_1 + P_2 + 2P_3, X_3^+ + 2X_3^- + X_4^+, 2N_1] \\
&[(\blacksquare)^{2T} + \Gamma_1^- + \Gamma_2^+, M_1^+ + M_4^+ + M_5^+, P_1 + P_3 + P_5, X_1^- + X_2^- + 2X_3^-, 2N_1] \\
&[(\blacksquare)^{2T} + \Gamma_1^- + \Gamma_2^+, M_1^+ + M_4^+ + M_5^+, 2P_1 + P_3 + P_4, X_3^+ + 2X_3^- + X_4^+, 2N_1]
\end{aligned}$$

2nd minimal solution:  $\mu_2^T = 6$  (1300 symmetry vectors)

Space group 141 ( $\mathbb{Z}_1$ )

1st minimal solution:  $\mu_1^T = 2$  (4 symmetry vectors)

| $\mathbf{n}^T$                                        |
|-------------------------------------------------------|
| $[(\blacksquare)^{2T}, M_4, P_2, X_2, N_1^- + N_2^-]$ |
| $[(\blacksquare)^{2T}, M_4, P_2, X_2, N_1^+ + N_2^+]$ |
| $[(\blacksquare)^{2T}, M_4, P_1, X_2, N_1^- + N_2^-]$ |
| $[(\blacksquare)^{2T}, M_4, P_1, X_2, N_1^+ + N_2^+]$ |

2nd minimal solution:  $\mu_2^T = 4$  (24 symmetry vectors)

Space group 142 ( $\mathbb{Z}_2$ )

1st minimal solution:  $\mu_1^T = 2$  (2 symmetry vectors & filling-enforced topology)

| $\mathbf{n}^T$                              | $\mathbf{v}^T \in \mathbb{Z}_2$ |
|---------------------------------------------|---------------------------------|
| $[(\blacksquare)^{2T}, M_3, P_2, X_2, N_1]$ | 1                               |
| $[(\blacksquare)^{2T}, M_3, P_1, X_2, N_1]$ | 1                               |

2nd minimal solution:  $\mu_2^T = 6$  (24 symmetry vectors)

Space group 143 ( $\mathbb{Z}_3$ )

1st minimal solution:  $\mu_1^T = 2$  (36 symmetry vectors)

| $\mathbf{n}^T$                                                                                 | $\mathbf{v}^T \in \mathbb{Z}_3$ |
|------------------------------------------------------------------------------------------------|---------------------------------|
| $[(\blacksquare)^{2T}, A_2 + A_3, 2H_3, 2HA_3, 2K_3, 2KA_3, 2L_1, 2M_1]$                       | trivial                         |
| $[(\blacksquare)^{2T}, A_2 + A_3, 2H_3, HA_2 + HA_3, 2K_3, KA_2 + KA_3, 2L_1, 2M_1]$           | 1                               |
| $[(\blacksquare)^{2T}, A_2 + A_3, 2H_3, HA_1 + HA_3, 2K_3, KA_1 + KA_3, 2L_1, 2M_1]$           | 2                               |
| $[(\blacksquare)^{2T}, A_2 + A_3, H_2 + H_3, 2HA_3, K_2 + K_3, 2KA_3, 2L_1, 2M_1]$             | 2                               |
| $[(\blacksquare)^{2T}, A_2 + A_3, H_2 + H_3, HA_2 + HA_3, K_2 + K_3, KA_2 + KA_3, 2L_1, 2M_1]$ | trivial                         |
| $[(\blacksquare)^{2T}, A_2 + A_3, H_2 + H_3, HA_1 + HA_3, K_2 + K_3, KA_1 + KA_3, 2L_1, 2M_1]$ | 1                               |
| $[(\blacksquare)^{2T}, A_2 + A_3, H_1 + H_3, 2HA_3, K_1 + K_3, 2KA_3, 2L_1, 2M_1]$             | 1                               |
| $[(\blacksquare)^{2T}, A_2 + A_3, H_1 + H_3, HA_2 + HA_3, K_1 + K_3, KA_2 + KA_3, 2L_1, 2M_1]$ | 2                               |
| $[(\blacksquare)^{2T}, A_2 + A_3, H_1 + H_3, HA_1 + HA_3, K_1 + K_3, KA_1 + KA_3, 2L_1, 2M_1]$ | trivial                         |
| $[(\blacksquare)^{2T}, A_2 + A_3, 2H_3, 2HA_2, 2K_3, 2KA_2, 2L_1, 2M_1]$                       | 2                               |
| $[(\blacksquare)^{2T}, A_2 + A_3, 2H_3, HA_1 + HA_2, 2K_3, KA_1 + KA_2, 2L_1, 2M_1]$           | trivial                         |
| $[(\blacksquare)^{2T}, A_2 + A_3, H_2 + H_3, 2HA_2, K_2 + K_3, 2KA_2, 2L_1, 2M_1]$             | 1                               |
| $[(\blacksquare)^{2T}, A_2 + A_3, H_2 + H_3, HA_1 + HA_2, K_2 + K_3, KA_1 + KA_2, 2L_1, 2M_1]$ | 2                               |
| $[(\blacksquare)^{2T}, A_2 + A_3, H_1 + H_3, 2HA_2, K_1 + K_3, 2KA_2, 2L_1, 2M_1]$             | trivial                         |
| $[(\blacksquare)^{2T}, A_2 + A_3, H_1 + H_3, HA_1 + HA_2, K_1 + K_3, KA_1 + KA_2, 2L_1, 2M_1]$ | 1                               |
| $[(\blacksquare)^{2T}, A_2 + A_3, 2H_3, 2HA_1, 2K_3, 2KA_1, 2L_1, 2M_1]$                       | 1                               |
| $[(\blacksquare)^{2T}, A_2 + A_3, H_2 + H_3, 2HA_1, K_2 + K_3, 2KA_1, 2L_1, 2M_1]$             | trivial                         |
| $[(\blacksquare)^{2T}, A_2 + A_3, H_1 + H_3, 2HA_1, K_1 + K_3, 2KA_1, 2L_1, 2M_1]$             | 2                               |
| $[(\blacksquare)^{2T}, A_2 + A_3, 2H_2, 2HA_3, 2K_2, 2KA_3, 2L_1, 2M_1]$                       | 1                               |
| $[(\blacksquare)^{2T}, A_2 + A_3, 2H_2, HA_2 + HA_3, 2K_2, KA_2 + KA_3, 2L_1, 2M_1]$           | 2                               |
| $[(\blacksquare)^{2T}, A_2 + A_3, 2H_2, HA_1 + HA_3, 2K_2, KA_1 + KA_3, 2L_1, 2M_1]$           | trivial                         |
| $[(\blacksquare)^{2T}, A_2 + A_3, H_1 + H_2, 2HA_3, K_1 + K_2, 2KA_3, 2L_1, 2M_1]$             | trivial                         |
| $[(\blacksquare)^{2T}, A_2 + A_3, H_1 + H_2, HA_2 + HA_3, K_1 + K_2, KA_2 + KA_3, 2L_1, 2M_1]$ | 1                               |
| $[(\blacksquare)^{2T}, A_2 + A_3, H_1 + H_2, HA_1 + HA_3, K_1 + K_2, KA_1 + KA_3, 2L_1, 2M_1]$ | 2                               |
| $[(\blacksquare)^{2T}, A_2 + A_3, 2H_2, 2HA_2, 2K_2, 2KA_2, 2L_1, 2M_1]$                       | trivial                         |

... continued on next page

... continued from previous page

|                                                                                                |         |
|------------------------------------------------------------------------------------------------|---------|
| $[(\blacksquare)^{2T}, A_2 + A_3, 2H_2, HA_1 + HA_2, 2K_2, KA_1 + KA_2, 2L_1, 2M_1]$           | 1       |
| $[(\blacksquare)^{2T}, A_2 + A_3, H_1 + H_2, 2HA_2, K_1 + K_2, 2KA_2, 2L_1, 2M_1]$             | 2       |
| $[(\blacksquare)^{2T}, A_2 + A_3, H_1 + H_2, HA_1 + HA_2, K_1 + K_2, KA_1 + KA_2, 2L_1, 2M_1]$ | trivial |
| $[(\blacksquare)^{2T}, A_2 + A_3, 2H_2, 2HA_1, 2K_2, 2KA_1, 2L_1, 2M_1]$                       | 2       |
| $[(\blacksquare)^{2T}, A_2 + A_3, H_1 + H_2, 2HA_1, K_1 + K_2, 2KA_1, 2L_1, 2M_1]$             | 1       |
| $[(\blacksquare)^{2T}, A_2 + A_3, 2H_1, 2HA_3, 2K_1, 2KA_3, 2L_1, 2M_1]$                       | 2       |
| $[(\blacksquare)^{2T}, A_2 + A_3, 2H_1, HA_2 + HA_3, 2K_1, KA_2 + KA_3, 2L_1, 2M_1]$           | trivial |
| $[(\blacksquare)^{2T}, A_2 + A_3, 2H_1, HA_1 + HA_3, 2K_1, KA_1 + KA_3, 2L_1, 2M_1]$           | 1       |
| $[(\blacksquare)^{2T}, A_2 + A_3, 2H_1, 2HA_2, 2K_1, 2KA_2, 2L_1, 2M_1]$                       | 1       |
| $[(\blacksquare)^{2T}, A_2 + A_3, 2H_1, HA_1 + HA_2, 2K_1, KA_1 + KA_2, 2L_1, 2M_1]$           | 2       |
| $[(\blacksquare)^{2T}, A_2 + A_3, 2H_1, 2HA_1, 2K_1, 2KA_1, 2L_1, 2M_1]$                       | trivial |

2nd minimal solution:  $\mu_2^T = 3$  (300 symmetry vectors)

Space group 144 ( $\mathbb{Z}_1$ )

1st minimal solution:  $\mu_1^T = 3$  (1 symmetry vector)

| $\mathbf{n}^T$                                                                                                                            |
|-------------------------------------------------------------------------------------------------------------------------------------------|
| $[(\blacksquare)^{2T} + \Gamma_1, A_1 + A_2 + A_3, H_1 + H_2 + H_3, HA_1 + HA_2 + HA_3, K_1 + K_2 + K_3, KA_1 + KA_2 + KA_3, 3L_1, 3M_1]$ |

2nd minimal solution:  $\mu_2^T = 6$  (1 symmetry vector)

Space group 145 ( $\mathbb{Z}_1$ )

1st minimal solution:  $\mu_1^T = 3$  (1 symmetry vector)

| $\mathbf{n}^T$                                                                                                                            |
|-------------------------------------------------------------------------------------------------------------------------------------------|
| $[(\blacksquare)^{2T} + \Gamma_1, A_1 + A_2 + A_3, H_1 + H_2 + H_3, HA_1 + HA_2 + HA_3, K_1 + K_2 + K_3, KA_1 + KA_2 + KA_3, 3L_1, 3M_1]$ |

2nd minimal solution:  $\mu_2^T = 6$  (1 symmetry vector)

Space group 146 ( $\mathbb{Z}_1$ )

1st minimal solution:  $\mu_1^T = 2$  (1 symmetry vector)

| $\mathbf{n}^T$                                 |
|------------------------------------------------|
| $[(\blacksquare)^{2T}, T_2 + T_3, 2F_1, 2L_1]$ |

2nd minimal solution:  $\mu_2^T = 3$  (3 symmetry vectors)

Space group 147 ( $\mathbb{Z}_2 \times \mathbb{Z}_{12}$ )1st minimal solution:  $\mu_1^T = 2$  (216 symmetry vectors)

| $\mathbf{n}^T$                                                                             | $\mathbf{v}^T \in \mathbb{Z}_2 \times \mathbb{Z}_{12}$ |
|--------------------------------------------------------------------------------------------|--------------------------------------------------------|
| $[(\blacksquare)^{2T}, A_2^- + A_3^-, 2H_2, 2K_2, 2L_1^+, 2M_1^+]$                         | (1, 11)                                                |
| $[(\blacksquare)^{2T}, A_2^- + A_3^-, 2H_2, 2K_2, 2L_1^+, M_1^+ + M_1^-]$                  | (0, 8)                                                 |
| $[(\blacksquare)^{2T}, A_2^- + A_3^-, 2H_2, 2K_2, L_1^+ + L_1^-, 2M_1^+]$                  | (1, 8)                                                 |
| $[(\blacksquare)^{2T}, A_2^- + A_3^-, 2H_2, 2K_2, L_1^+ + L_1^-, M_1^+ + M_1^-]$           | (0, 5)                                                 |
| $[(\blacksquare)^{2T}, A_2^- + A_3^-, H_2 + H_3, K_2 + K_3, 2L_1^+, 2M_1^+]$               | (1, 3)                                                 |
| $[(\blacksquare)^{2T}, A_2^- + A_3^-, H_2 + H_3, K_2 + K_3, 2L_1^+, M_1^+ + M_1^-]$        | trivial                                                |
| $[(\blacksquare)^{2T}, A_2^- + A_3^-, H_2 + H_3, K_2 + K_3, L_1^+ + L_1^-, 2M_1^+]$        | (1, 0)                                                 |
| $[(\blacksquare)^{2T}, A_2^- + A_3^-, H_2 + H_3, K_2 + K_3, L_1^+ + L_1^-, M_1^+ + M_1^-]$ | (0, 9)                                                 |
| $[(\blacksquare)^{2T}, A_2^- + A_3^-, H_1 + H_2, K_1 + K_2, 2L_1^+, 2M_1^+]$               | (1, 7)                                                 |
| $[(\blacksquare)^{2T}, A_2^- + A_3^-, H_1 + H_2, K_1 + K_2, 2L_1^+, M_1^+ + M_1^-]$        | (0, 4)                                                 |
| $[(\blacksquare)^{2T}, A_2^- + A_3^-, H_1 + H_2, K_1 + K_2, L_1^+ + L_1^-, 2M_1^+]$        | (1, 4)                                                 |
| $[(\blacksquare)^{2T}, A_2^- + A_3^-, H_1 + H_2, K_1 + K_2, L_1^+ + L_1^-, M_1^+ + M_1^-]$ | (0, 1)                                                 |
| $[(\blacksquare)^{2T}, A_2^- + A_3^-, 2H_2, 2K_2, 2L_1^+, 2M_1^-]$                         | (1, 5)                                                 |
| $[(\blacksquare)^{2T}, A_2^- + A_3^-, 2H_2, 2K_2, L_1^+ + L_1^-, 2M_1^-]$                  | (1, 2)                                                 |
| $[(\blacksquare)^{2T}, A_2^- + A_3^-, H_2 + H_3, K_2 + K_3, 2L_1^+, 2M_1^-]$               | (1, 9)                                                 |
| $[(\blacksquare)^{2T}, A_2^- + A_3^-, H_2 + H_3, K_2 + K_3, L_1^+ + L_1^-, 2M_1^-]$        | (1, 6)                                                 |
| $[(\blacksquare)^{2T}, A_2^- + A_3^-, H_1 + H_2, K_1 + K_2, 2L_1^+, 2M_1^-]$               | (1, 1)                                                 |
| $[(\blacksquare)^{2T}, A_2^- + A_3^-, H_1 + H_2, K_1 + K_2, L_1^+ + L_1^-, 2M_1^-]$        | (1, 10)                                                |
| $[(\blacksquare)^{2T}, A_2^- + A_3^-, 2H_2, 2K_2, 2L_1^-, 2M_1^+]$                         | (1, 5)                                                 |
| $[(\blacksquare)^{2T}, A_2^- + A_3^-, 2H_2, 2K_2, 2L_1^-, M_1^+ + M_1^-]$                  | (0, 2)                                                 |
| $[(\blacksquare)^{2T}, A_2^- + A_3^-, H_2 + H_3, K_2 + K_3, 2L_1^-, 2M_1^+]$               | (1, 9)                                                 |
| $[(\blacksquare)^{2T}, A_2^- + A_3^-, H_2 + H_3, K_2 + K_3, 2L_1^-, M_1^+ + M_1^-]$        | (0, 6)                                                 |
| $[(\blacksquare)^{2T}, A_2^- + A_3^-, H_1 + H_2, K_1 + K_2, 2L_1^-, 2M_1^+]$               | (1, 1)                                                 |
| $[(\blacksquare)^{2T}, A_2^- + A_3^-, H_1 + H_2, K_1 + K_2, 2L_1^-, M_1^+ + M_1^-]$        | (0, 10)                                                |
| $[(\blacksquare)^{2T}, A_2^- + A_3^-, 2H_2, 2K_2, 2L_1^-, 2M_1^-]$                         | (1, 11)                                                |
| $[(\blacksquare)^{2T}, A_2^- + A_3^-, H_2 + H_3, K_2 + K_3, 2L_1^-, 2M_1^-]$               | (1, 3)                                                 |
| $[(\blacksquare)^{2T}, A_2^- + A_3^-, H_1 + H_2, K_1 + K_2, 2L_1^-, 2M_1^-]$               | (1, 7)                                                 |
| $[(\blacksquare)^{2T}, A_2^- + A_3^-, 2H_3, 2K_3, 2L_1^+, 2M_1^+]$                         | (1, 7)                                                 |
| $[(\blacksquare)^{2T}, A_2^- + A_3^-, 2H_3, 2K_3, 2L_1^+, M_1^+ + M_1^-]$                  | (0, 4)                                                 |
| $[(\blacksquare)^{2T}, A_2^- + A_3^-, 2H_3, 2K_3, L_1^+ + L_1^-, 2M_1^+]$                  | (1, 4)                                                 |
| $[(\blacksquare)^{2T}, A_2^- + A_3^-, 2H_3, 2K_3, L_1^+ + L_1^-, M_1^+ + M_1^-]$           | (0, 1)                                                 |
| $[(\blacksquare)^{2T}, A_2^- + A_3^-, H_1 + H_3, K_1 + K_3, 2L_1^+, 2M_1^+]$               | (1, 11)                                                |
| $[(\blacksquare)^{2T}, A_2^- + A_3^-, H_1 + H_3, K_1 + K_3, 2L_1^+, M_1^+ + M_1^-]$        | (0, 8)                                                 |
| $[(\blacksquare)^{2T}, A_2^- + A_3^-, H_1 + H_3, K_1 + K_3, L_1^+ + L_1^-, 2M_1^+]$        | (1, 8)                                                 |
| $[(\blacksquare)^{2T}, A_2^- + A_3^-, H_1 + H_3, K_1 + K_3, L_1^+ + L_1^-, M_1^+ + M_1^-]$ | (0, 5)                                                 |
| $[(\blacksquare)^{2T}, A_2^- + A_3^-, 2H_3, 2K_3, 2L_1^+, 2M_1^-]$                         | (1, 1)                                                 |
| $[(\blacksquare)^{2T}, A_2^- + A_3^-, 2H_3, 2K_3, L_1^+ + L_1^-, 2M_1^-]$                  | (1, 10)                                                |
| $[(\blacksquare)^{2T}, A_2^- + A_3^-, H_1 + H_3, K_1 + K_3, 2L_1^+, 2M_1^-]$               | (1, 5)                                                 |
| $[(\blacksquare)^{2T}, A_2^- + A_3^-, H_1 + H_3, K_1 + K_3, L_1^+ + L_1^-, 2M_1^-]$        | (1, 2)                                                 |
| $[(\blacksquare)^{2T}, A_2^- + A_3^-, 2H_3, 2K_3, 2L_1^-, 2M_1^+]$                         | (1, 1)                                                 |
| $[(\blacksquare)^{2T}, A_2^- + A_3^-, 2H_3, 2K_3, 2L_1^-, M_1^+ + M_1^-]$                  | (0, 10)                                                |
| $[(\blacksquare)^{2T}, A_2^- + A_3^-, H_1 + H_3, K_1 + K_3, 2L_1^-, 2M_1^+]$               | (1, 5)                                                 |
| $[(\blacksquare)^{2T}, A_2^- + A_3^-, H_1 + H_3, K_1 + K_3, 2L_1^-, M_1^+ + M_1^-]$        | (0, 2)                                                 |
| $[(\blacksquare)^{2T}, A_2^- + A_3^-, 2H_3, 2K_3, 2L_1^-, 2M_1^-]$                         | (1, 7)                                                 |
| $[(\blacksquare)^{2T}, A_2^- + A_3^-, H_1 + H_3, K_1 + K_3, 2L_1^-, 2M_1^-]$               | (1, 11)                                                |
| $[(\blacksquare)^{2T}, A_2^- + A_3^-, 2H_1, 2K_1, 2L_1^+, 2M_1^+]$                         | (1, 3)                                                 |
| $[(\blacksquare)^{2T}, A_2^- + A_3^-, 2H_1, 2K_1, 2L_1^+, M_1^+ + M_1^-]$                  | trivial                                                |
| $[(\blacksquare)^{2T}, A_2^- + A_3^-, 2H_1, 2K_1, L_1^+ + L_1^-, 2M_1^+]$                  | (1, 0)                                                 |
| $[(\blacksquare)^{2T}, A_2^- + A_3^-, 2H_1, 2K_1, L_1^+ + L_1^-, M_1^+ + M_1^-]$           | (0, 9)                                                 |

... continued on next page

... continued from previous page

|                                                                                            |         |
|--------------------------------------------------------------------------------------------|---------|
| $[(\blacksquare)^{2T}, A_2^- + A_3^-, 2H_1, 2K_1, 2L_1^+, 2M_1^-]$                         | (1, 9)  |
| $[(\blacksquare)^{2T}, A_2^- + A_3^-, 2H_1, 2K_1, L_1^+ + L_1^-, 2M_1^-]$                  | (1, 6)  |
| $[(\blacksquare)^{2T}, A_2^- + A_3^-, 2H_1, 2K_1, 2L_1^-, 2M_1^+]$                         | (1, 9)  |
| $[(\blacksquare)^{2T}, A_2^- + A_3^-, 2H_1, 2K_1, 2L_1^-, M_1^+ + M_1^-]$                  | (0, 6)  |
| $[(\blacksquare)^{2T}, A_2^- + A_3^-, 2H_1, 2K_1, 2L_1^-, 2M_1^-]$                         | (1, 3)  |
| $[(\blacksquare)^{2T}, A_2^+ + A_3^-, 2H_2, 2K_2, 2L_1^+, 2M_1^+]$                         | (1, 8)  |
| $[(\blacksquare)^{2T}, A_2^+ + A_3^-, 2H_2, 2K_2, 2L_1^+, M_1^+ + M_1^-]$                  | (0, 5)  |
| $[(\blacksquare)^{2T}, A_2^+ + A_3^-, 2H_2, 2K_2, L_1^+ + L_1^-, 2M_1^+]$                  | (1, 5)  |
| $[(\blacksquare)^{2T}, A_2^+ + A_3^-, 2H_2, 2K_2, L_1^+ + L_1^-, M_1^+ + M_1^-]$           | (0, 2)  |
| $[(\blacksquare)^{2T}, A_2^+ + A_3^-, H_2 + H_3, K_2 + K_3, 2L_1^+, 2M_1^+]$               | (1, 0)  |
| $[(\blacksquare)^{2T}, A_2^+ + A_3^-, H_2 + H_3, K_2 + K_3, 2L_1^+, M_1^+ + M_1^-]$        | (0, 9)  |
| $[(\blacksquare)^{2T}, A_2^+ + A_3^-, H_2 + H_3, K_2 + K_3, L_1^+ + L_1^-, 2M_1^+]$        | (1, 9)  |
| $[(\blacksquare)^{2T}, A_2^+ + A_3^-, H_2 + H_3, K_2 + K_3, L_1^+ + L_1^-, M_1^+ + M_1^-]$ | (0, 6)  |
| $[(\blacksquare)^{2T}, A_2^+ + A_3^-, H_1 + H_2, K_1 + K_2, 2L_1^+, 2M_1^+]$               | (1, 4)  |
| $[(\blacksquare)^{2T}, A_2^+ + A_3^-, H_1 + H_2, K_1 + K_2, 2L_1^+, M_1^+ + M_1^-]$        | (0, 1)  |
| $[(\blacksquare)^{2T}, A_2^+ + A_3^-, H_1 + H_2, K_1 + K_2, L_1^+ + L_1^-, 2M_1^+]$        | (1, 1)  |
| $[(\blacksquare)^{2T}, A_2^+ + A_3^-, H_1 + H_2, K_1 + K_2, L_1^+ + L_1^-, M_1^+ + M_1^-]$ | (0, 10) |
| $[(\blacksquare)^{2T}, A_2^+ + A_3^-, 2H_2, 2K_2, 2L_1^+, 2M_1^-]$                         | (1, 2)  |
| $[(\blacksquare)^{2T}, A_2^+ + A_3^-, 2H_2, 2K_2, L_1^+ + L_1^-, 2M_1^-]$                  | (1, 11) |
| $[(\blacksquare)^{2T}, A_2^+ + A_3^-, H_2 + H_3, K_2 + K_3, 2L_1^+, 2M_1^-]$               | (1, 6)  |
| $[(\blacksquare)^{2T}, A_2^+ + A_3^-, H_2 + H_3, K_2 + K_3, L_1^+ + L_1^-, 2M_1^-]$        | (1, 3)  |
| $[(\blacksquare)^{2T}, A_2^+ + A_3^-, H_1 + H_2, K_1 + K_2, 2L_1^+, 2M_1^-]$               | (1, 10) |
| $[(\blacksquare)^{2T}, A_2^+ + A_3^-, H_1 + H_2, K_1 + K_2, L_1^+ + L_1^-, 2M_1^-]$        | (1, 7)  |
| $[(\blacksquare)^{2T}, A_2^+ + A_3^-, 2H_2, 2K_2, 2L_1^-, 2M_1^+]$                         | (1, 2)  |
| $[(\blacksquare)^{2T}, A_2^+ + A_3^-, 2H_2, 2K_2, 2L_1^-, M_1^+ + M_1^-]$                  | (0, 11) |
| $[(\blacksquare)^{2T}, A_2^+ + A_3^-, H_2 + H_3, K_2 + K_3, 2L_1^-, 2M_1^+]$               | (1, 6)  |
| $[(\blacksquare)^{2T}, A_2^+ + A_3^-, H_2 + H_3, K_2 + K_3, 2L_1^-, M_1^+ + M_1^-]$        | (0, 3)  |
| $[(\blacksquare)^{2T}, A_2^+ + A_3^-, H_1 + H_2, K_1 + K_2, 2L_1^-, 2M_1^+]$               | (1, 10) |
| $[(\blacksquare)^{2T}, A_2^+ + A_3^-, H_1 + H_2, K_1 + K_2, 2L_1^-, M_1^+ + M_1^-]$        | (0, 7)  |
| $[(\blacksquare)^{2T}, A_2^+ + A_3^-, 2H_2, 2K_2, 2L_1^-, 2M_1^-]$                         | (1, 8)  |
| $[(\blacksquare)^{2T}, A_2^+ + A_3^-, H_2 + H_3, K_2 + K_3, 2L_1^-, 2M_1^-]$               | (1, 0)  |
| $[(\blacksquare)^{2T}, A_2^+ + A_3^-, H_1 + H_2, K_1 + K_2, 2L_1^-, 2M_1^-]$               | (1, 4)  |
| $[(\blacksquare)^{2T}, A_2^+ + A_3^-, 2H_3, 2K_3, 2L_1^+, 2M_1^+]$                         | (1, 4)  |
| $[(\blacksquare)^{2T}, A_2^+ + A_3^-, 2H_3, 2K_3, 2L_1^+, M_1^+ + M_1^-]$                  | (0, 1)  |
| $[(\blacksquare)^{2T}, A_2^+ + A_3^-, 2H_3, 2K_3, L_1^+ + L_1^-, 2M_1^+]$                  | (1, 1)  |
| $[(\blacksquare)^{2T}, A_2^+ + A_3^-, 2H_3, 2K_3, L_1^+ + L_1^-, M_1^+ + M_1^-]$           | (0, 10) |
| $[(\blacksquare)^{2T}, A_2^+ + A_3^-, H_1 + H_3, K_1 + K_3, 2L_1^+, 2M_1^+]$               | (1, 8)  |
| $[(\blacksquare)^{2T}, A_2^+ + A_3^-, H_1 + H_3, K_1 + K_3, 2L_1^+, M_1^+ + M_1^-]$        | (0, 5)  |
| $[(\blacksquare)^{2T}, A_2^+ + A_3^-, H_1 + H_3, K_1 + K_3, L_1^+ + L_1^-, 2M_1^+]$        | (1, 5)  |
| $[(\blacksquare)^{2T}, A_2^+ + A_3^-, H_1 + H_3, K_1 + K_3, L_1^+ + L_1^-, M_1^+ + M_1^-]$ | (0, 2)  |
| $[(\blacksquare)^{2T}, A_2^+ + A_3^-, 2H_3, 2K_3, 2L_1^+, 2M_1^-]$                         | (1, 10) |
| $[(\blacksquare)^{2T}, A_2^+ + A_3^-, 2H_3, 2K_3, L_1^+ + L_1^-, 2M_1^-]$                  | (1, 7)  |
| $[(\blacksquare)^{2T}, A_2^+ + A_3^-, H_1 + H_3, K_1 + K_3, 2L_1^+, 2M_1^-]$               | (1, 2)  |
| $[(\blacksquare)^{2T}, A_2^+ + A_3^-, H_1 + H_3, K_1 + K_3, L_1^+ + L_1^-, 2M_1^-]$        | (1, 11) |
| $[(\blacksquare)^{2T}, A_2^+ + A_3^-, 2H_3, 2K_3, 2L_1^-, 2M_1^+]$                         | (1, 10) |
| $[(\blacksquare)^{2T}, A_2^+ + A_3^-, 2H_3, 2K_3, 2L_1^-, M_1^+ + M_1^-]$                  | (0, 7)  |
| $[(\blacksquare)^{2T}, A_2^+ + A_3^-, H_1 + H_3, K_1 + K_3, 2L_1^-, 2M_1^+]$               | (1, 2)  |
| $[(\blacksquare)^{2T}, A_2^+ + A_3^-, H_1 + H_3, K_1 + K_3, 2L_1^-, M_1^+ + M_1^-]$        | (0, 11) |
| $[(\blacksquare)^{2T}, A_2^+ + A_3^-, 2H_3, 2K_3, 2L_1^-, 2M_1^-]$                         | (1, 4)  |
| $[(\blacksquare)^{2T}, A_2^+ + A_3^-, H_1 + H_3, K_1 + K_3, 2L_1^-, 2M_1^-]$               | (1, 8)  |
| $[(\blacksquare)^{2T}, A_2^+ + A_3^-, 2H_1, 2K_1, 2L_1^+, 2M_1^+]$                         | (1, 0)  |
| $[(\blacksquare)^{2T}, A_2^+ + A_3^-, 2H_1, 2K_1, 2L_1^+, M_1^+ + M_1^-]$                  | (0, 9)  |
| $[(\blacksquare)^{2T}, A_2^+ + A_3^-, 2H_1, 2K_1, L_1^+ + L_1^-, 2M_1^+]$                  | (1, 9)  |
| $[(\blacksquare)^{2T}, A_2^+ + A_3^-, 2H_1, 2K_1, L_1^+ + L_1^-, M_1^+ + M_1^-]$           | (0, 6)  |

... continued on next page

... continued from previous page

|                                                                                            |         |
|--------------------------------------------------------------------------------------------|---------|
| $[(\blacksquare)^{2T}, A_2^+ + A_3^-, 2H_1, 2K_1, 2L_1^+, 2M_1^-]$                         | (1, 6)  |
| $[(\blacksquare)^{2T}, A_2^+ + A_3^-, 2H_1, 2K_1, L_1^+ + L_1^-, 2M_1^-]$                  | (1, 3)  |
| $[(\blacksquare)^{2T}, A_2^+ + A_3^-, 2H_1, 2K_1, 2L_1^-, 2M_1^+]$                         | (1, 6)  |
| $[(\blacksquare)^{2T}, A_2^+ + A_3^-, 2H_1, 2K_1, 2L_1^-, M_1^+ + M_1^-]$                  | (0, 3)  |
| $[(\blacksquare)^{2T}, A_2^+ + A_3^-, 2H_1, 2K_1, 2L_1^-, 2M_1^-]$                         | (1, 0)  |
| $[(\blacksquare)^{2T}, A_2^- + A_3^+, 2H_2, 2K_2, 2L_1^+, 2M_1^+]$                         | (1, 8)  |
| $[(\blacksquare)^{2T}, A_2^- + A_3^+, 2H_2, 2K_2, 2L_1^+, M_1^+ + M_1^-]$                  | (0, 5)  |
| $[(\blacksquare)^{2T}, A_2^- + A_3^+, 2H_2, 2K_2, L_1^+ + L_1^-, 2M_1^+]$                  | (1, 5)  |
| $[(\blacksquare)^{2T}, A_2^- + A_3^+, 2H_2, 2K_2, L_1^+ + L_1^-, M_1^+ + M_1^-]$           | (0, 2)  |
| $[(\blacksquare)^{2T}, A_2^- + A_3^+, H_2 + H_3, K_2 + K_3, 2L_1^+, 2M_1^+]$               | (1, 0)  |
| $[(\blacksquare)^{2T}, A_2^- + A_3^+, H_2 + H_3, K_2 + K_3, 2L_1^+, M_1^+ + M_1^-]$        | (0, 9)  |
| $[(\blacksquare)^{2T}, A_2^- + A_3^+, H_2 + H_3, K_2 + K_3, L_1^+ + L_1^-, 2M_1^+]$        | (1, 9)  |
| $[(\blacksquare)^{2T}, A_2^- + A_3^+, H_2 + H_3, K_2 + K_3, L_1^+ + L_1^-, M_1^+ + M_1^-]$ | (0, 6)  |
| $[(\blacksquare)^{2T}, A_2^- + A_3^+, H_1 + H_2, K_1 + K_2, 2L_1^+, 2M_1^+]$               | (1, 4)  |
| $[(\blacksquare)^{2T}, A_2^- + A_3^+, H_1 + H_2, K_1 + K_2, 2L_1^+, M_1^+ + M_1^-]$        | (0, 1)  |
| $[(\blacksquare)^{2T}, A_2^- + A_3^+, H_1 + H_2, K_1 + K_2, L_1^+ + L_1^-, 2M_1^+]$        | (1, 1)  |
| $[(\blacksquare)^{2T}, A_2^- + A_3^+, H_1 + H_2, K_1 + K_2, L_1^+ + L_1^-, M_1^+ + M_1^-]$ | (0, 10) |
| $[(\blacksquare)^{2T}, A_2^- + A_3^+, 2H_2, 2K_2, 2L_1^+, 2M_1^-]$                         | (1, 2)  |
| $[(\blacksquare)^{2T}, A_2^- + A_3^+, 2H_2, 2K_2, L_1^+ + L_1^-, 2M_1^-]$                  | (1, 11) |
| $[(\blacksquare)^{2T}, A_2^- + A_3^+, H_2 + H_3, K_2 + K_3, 2L_1^+, 2M_1^-]$               | (1, 6)  |
| $[(\blacksquare)^{2T}, A_2^- + A_3^+, H_2 + H_3, K_2 + K_3, L_1^+ + L_1^-, 2M_1^-]$        | (1, 3)  |
| $[(\blacksquare)^{2T}, A_2^- + A_3^+, H_1 + H_2, K_1 + K_2, 2L_1^+, 2M_1^-]$               | (1, 10) |
| $[(\blacksquare)^{2T}, A_2^- + A_3^+, H_1 + H_2, K_1 + K_2, L_1^+ + L_1^-, 2M_1^-]$        | (1, 7)  |
| $[(\blacksquare)^{2T}, A_2^- + A_3^+, 2H_2, 2K_2, 2L_1^-, 2M_1^+]$                         | (1, 2)  |
| $[(\blacksquare)^{2T}, A_2^- + A_3^+, 2H_2, 2K_2, 2L_1^-, M_1^+ + M_1^-]$                  | (0, 11) |
| $[(\blacksquare)^{2T}, A_2^- + A_3^+, H_2 + H_3, K_2 + K_3, 2L_1^-, 2M_1^+]$               | (1, 6)  |
| $[(\blacksquare)^{2T}, A_2^- + A_3^+, H_2 + H_3, K_2 + K_3, 2L_1^-, M_1^+ + M_1^-]$        | (0, 3)  |
| $[(\blacksquare)^{2T}, A_2^- + A_3^+, H_1 + H_2, K_1 + K_2, 2L_1^-, 2M_1^+]$               | (1, 10) |
| $[(\blacksquare)^{2T}, A_2^- + A_3^+, H_1 + H_2, K_1 + K_2, 2L_1^-, M_1^+ + M_1^-]$        | (0, 7)  |
| $[(\blacksquare)^{2T}, A_2^- + A_3^+, 2H_2, 2K_2, 2L_1^-, 2M_1^-]$                         | (1, 8)  |
| $[(\blacksquare)^{2T}, A_2^- + A_3^+, H_2 + H_3, K_2 + K_3, 2L_1^-, 2M_1^-]$               | (1, 0)  |
| $[(\blacksquare)^{2T}, A_2^- + A_3^+, H_1 + H_2, K_1 + K_2, 2L_1^-, 2M_1^-]$               | (1, 4)  |
| $[(\blacksquare)^{2T}, A_2^- + A_3^+, 2H_3, 2K_3, 2L_1^+, 2M_1^+]$                         | (1, 4)  |
| $[(\blacksquare)^{2T}, A_2^- + A_3^+, 2H_3, 2K_3, 2L_1^+, M_1^+ + M_1^-]$                  | (0, 1)  |
| $[(\blacksquare)^{2T}, A_2^- + A_3^+, 2H_3, 2K_3, L_1^+ + L_1^-, 2M_1^+]$                  | (1, 1)  |
| $[(\blacksquare)^{2T}, A_2^- + A_3^+, 2H_3, 2K_3, L_1^+ + L_1^-, M_1^+ + M_1^-]$           | (0, 10) |
| $[(\blacksquare)^{2T}, A_2^- + A_3^+, H_1 + H_3, K_1 + K_3, 2L_1^+, 2M_1^+]$               | (1, 8)  |
| $[(\blacksquare)^{2T}, A_2^- + A_3^+, H_1 + H_3, K_1 + K_3, 2L_1^+, M_1^+ + M_1^-]$        | (0, 5)  |
| $[(\blacksquare)^{2T}, A_2^- + A_3^+, H_1 + H_3, K_1 + K_3, L_1^+ + L_1^-, 2M_1^+]$        | (1, 5)  |
| $[(\blacksquare)^{2T}, A_2^- + A_3^+, H_1 + H_3, K_1 + K_3, L_1^+ + L_1^-, M_1^+ + M_1^-]$ | (0, 2)  |
| $[(\blacksquare)^{2T}, A_2^- + A_3^+, 2H_3, 2K_3, 2L_1^+, 2M_1^-]$                         | (1, 10) |
| $[(\blacksquare)^{2T}, A_2^- + A_3^+, 2H_3, 2K_3, L_1^+ + L_1^-, 2M_1^-]$                  | (1, 7)  |
| $[(\blacksquare)^{2T}, A_2^- + A_3^+, H_1 + H_3, K_1 + K_3, 2L_1^+, 2M_1^-]$               | (1, 2)  |
| $[(\blacksquare)^{2T}, A_2^- + A_3^+, H_1 + H_3, K_1 + K_3, L_1^+ + L_1^-, 2M_1^-]$        | (1, 11) |
| $[(\blacksquare)^{2T}, A_2^- + A_3^+, 2H_3, 2K_3, 2L_1^-, 2M_1^+]$                         | (1, 10) |
| $[(\blacksquare)^{2T}, A_2^- + A_3^+, 2H_3, 2K_3, 2L_1^-, M_1^+ + M_1^-]$                  | (0, 7)  |
| $[(\blacksquare)^{2T}, A_2^- + A_3^+, H_1 + H_3, K_1 + K_3, 2L_1^-, 2M_1^+]$               | (1, 2)  |
| $[(\blacksquare)^{2T}, A_2^- + A_3^+, H_1 + H_3, K_1 + K_3, 2L_1^-, M_1^+ + M_1^-]$        | (0, 11) |
| $[(\blacksquare)^{2T}, A_2^- + A_3^+, 2H_3, 2K_3, 2L_1^-, 2M_1^-]$                         | (1, 4)  |
| $[(\blacksquare)^{2T}, A_2^- + A_3^+, H_1 + H_3, K_1 + K_3, 2L_1^-, 2M_1^-]$               | (1, 8)  |
| $[(\blacksquare)^{2T}, A_2^- + A_3^+, 2H_1, 2K_1, 2L_1^+, 2M_1^+]$                         | (1, 0)  |
| $[(\blacksquare)^{2T}, A_2^- + A_3^+, 2H_1, 2K_1, 2L_1^+, M_1^+ + M_1^-]$                  | (0, 9)  |
| $[(\blacksquare)^{2T}, A_2^- + A_3^+, 2H_1, 2K_1, L_1^+ + L_1^-, 2M_1^+]$                  | (1, 9)  |
| $[(\blacksquare)^{2T}, A_2^- + A_3^+, 2H_1, 2K_1, L_1^+ + L_1^-, M_1^+ + M_1^-]$           | (0, 6)  |

... continued on next page



... continued from previous page

|                                                                                            |         |
|--------------------------------------------------------------------------------------------|---------|
| $[(\blacksquare)^{2T}, A_2^- + A_3^+, 2H_1, 2K_1, 2L_1^+, 2M_1^-]$                         | (1, 6)  |
| $[(\blacksquare)^{2T}, A_2^- + A_3^+, 2H_1, 2K_1, L_1^+ + L_1^-, 2M_1^-]$                  | (1, 3)  |
| $[(\blacksquare)^{2T}, A_2^- + A_3^+, 2H_1, 2K_1, 2L_1^-, 2M_1^+]$                         | (1, 6)  |
| $[(\blacksquare)^{2T}, A_2^- + A_3^+, 2H_1, 2K_1, 2L_1^-, M_1^+ + M_1^-]$                  | (0, 3)  |
| $[(\blacksquare)^{2T}, A_2^- + A_3^+, 2H_1, 2K_1, 2L_1^-, 2M_1^-]$                         | (1, 0)  |
| $[(\blacksquare)^{2T}, A_2^+ + A_3^+, 2H_2, 2K_2, 2L_1^+, 2M_1^+]$                         | (1, 5)  |
| $[(\blacksquare)^{2T}, A_2^+ + A_3^+, 2H_2, 2K_2, 2L_1^+, M_1^+ + M_1^-]$                  | (0, 2)  |
| $[(\blacksquare)^{2T}, A_2^+ + A_3^+, 2H_2, 2K_2, L_1^+ + L_1^-, 2M_1^+]$                  | (1, 2)  |
| $[(\blacksquare)^{2T}, A_2^+ + A_3^+, 2H_2, 2K_2, L_1^+ + L_1^-, M_1^+ + M_1^-]$           | (0, 11) |
| $[(\blacksquare)^{2T}, A_2^+ + A_3^+, H_2 + H_3, K_2 + K_3, 2L_1^+, 2M_1^+]$               | (1, 9)  |
| $[(\blacksquare)^{2T}, A_2^+ + A_3^+, H_2 + H_3, K_2 + K_3, 2L_1^+, M_1^+ + M_1^-]$        | (0, 6)  |
| $[(\blacksquare)^{2T}, A_2^+ + A_3^+, H_2 + H_3, K_2 + K_3, L_1^+ + L_1^-, 2M_1^+]$        | (1, 6)  |
| $[(\blacksquare)^{2T}, A_2^+ + A_3^+, H_2 + H_3, K_2 + K_3, L_1^+ + L_1^-, M_1^+ + M_1^-]$ | (0, 3)  |
| $[(\blacksquare)^{2T}, A_2^+ + A_3^+, H_1 + H_2, K_1 + K_2, 2L_1^+, 2M_1^+]$               | (1, 1)  |
| $[(\blacksquare)^{2T}, A_2^+ + A_3^+, H_1 + H_2, K_1 + K_2, 2L_1^+, M_1^+ + M_1^-]$        | (0, 10) |
| $[(\blacksquare)^{2T}, A_2^+ + A_3^+, H_1 + H_2, K_1 + K_2, L_1^+ + L_1^-, 2M_1^+]$        | (1, 10) |
| $[(\blacksquare)^{2T}, A_2^+ + A_3^+, H_1 + H_2, K_1 + K_2, L_1^+ + L_1^-, M_1^+ + M_1^-]$ | (0, 7)  |
| $[(\blacksquare)^{2T}, A_2^+ + A_3^+, 2H_2, 2K_2, 2L_1^+, 2M_1^-]$                         | (1, 11) |
| $[(\blacksquare)^{2T}, A_2^+ + A_3^+, 2H_2, 2K_2, L_1^+ + L_1^-, 2M_1^-]$                  | (1, 8)  |
| $[(\blacksquare)^{2T}, A_2^+ + A_3^+, H_2 + H_3, K_2 + K_3, 2L_1^+, 2M_1^-]$               | (1, 3)  |
| $[(\blacksquare)^{2T}, A_2^+ + A_3^+, H_2 + H_3, K_2 + K_3, L_1^+ + L_1^-, 2M_1^-]$        | (1, 0)  |
| $[(\blacksquare)^{2T}, A_2^+ + A_3^+, H_1 + H_2, K_1 + K_2, 2L_1^+, 2M_1^-]$               | (1, 7)  |
| $[(\blacksquare)^{2T}, A_2^+ + A_3^+, H_1 + H_2, K_1 + K_2, L_1^+ + L_1^-, 2M_1^-]$        | (1, 4)  |
| $[(\blacksquare)^{2T}, A_2^+ + A_3^+, 2H_2, 2K_2, 2L_1^-, 2M_1^+]$                         | (1, 11) |
| $[(\blacksquare)^{2T}, A_2^+ + A_3^+, 2H_2, 2K_2, 2L_1^-, M_1^+ + M_1^-]$                  | (0, 8)  |
| $[(\blacksquare)^{2T}, A_2^+ + A_3^+, H_2 + H_3, K_2 + K_3, 2L_1^-, 2M_1^+]$               | (1, 3)  |
| $[(\blacksquare)^{2T}, A_2^+ + A_3^+, H_2 + H_3, K_2 + K_3, 2L_1^-, M_1^+ + M_1^-]$        | trivial |
| $[(\blacksquare)^{2T}, A_2^+ + A_3^+, H_1 + H_2, K_1 + K_2, 2L_1^-, 2M_1^+]$               | (1, 7)  |
| $[(\blacksquare)^{2T}, A_2^+ + A_3^+, H_1 + H_2, K_1 + K_2, 2L_1^-, M_1^+ + M_1^-]$        | (0, 4)  |
| $[(\blacksquare)^{2T}, A_2^+ + A_3^+, 2H_2, 2K_2, 2L_1^-, 2M_1^-]$                         | (1, 5)  |
| $[(\blacksquare)^{2T}, A_2^+ + A_3^+, H_2 + H_3, K_2 + K_3, 2L_1^-, 2M_1^-]$               | (1, 9)  |
| $[(\blacksquare)^{2T}, A_2^+ + A_3^+, H_1 + H_2, K_1 + K_2, 2L_1^-, 2M_1^-]$               | (1, 1)  |
| $[(\blacksquare)^{2T}, A_2^+ + A_3^+, 2H_3, 2K_3, 2L_1^+, 2M_1^+]$                         | (1, 1)  |
| $[(\blacksquare)^{2T}, A_2^+ + A_3^+, 2H_3, 2K_3, 2L_1^+, M_1^+ + M_1^-]$                  | (0, 10) |
| $[(\blacksquare)^{2T}, A_2^+ + A_3^+, 2H_3, 2K_3, L_1^+ + L_1^-, 2M_1^+]$                  | (1, 10) |
| $[(\blacksquare)^{2T}, A_2^+ + A_3^+, 2H_3, 2K_3, L_1^+ + L_1^-, M_1^+ + M_1^-]$           | (0, 7)  |
| $[(\blacksquare)^{2T}, A_2^+ + A_3^+, H_1 + H_3, K_1 + K_3, 2L_1^+, 2M_1^+]$               | (1, 5)  |
| $[(\blacksquare)^{2T}, A_2^+ + A_3^+, H_1 + H_3, K_1 + K_3, 2L_1^+, M_1^+ + M_1^-]$        | (0, 2)  |
| $[(\blacksquare)^{2T}, A_2^+ + A_3^+, H_1 + H_3, K_1 + K_3, L_1^+ + L_1^-, 2M_1^+]$        | (1, 2)  |
| $[(\blacksquare)^{2T}, A_2^+ + A_3^+, H_1 + H_3, K_1 + K_3, L_1^+ + L_1^-, M_1^+ + M_1^-]$ | (0, 11) |
| $[(\blacksquare)^{2T}, A_2^+ + A_3^+, 2H_3, 2K_3, 2L_1^+, 2M_1^-]$                         | (1, 7)  |
| $[(\blacksquare)^{2T}, A_2^+ + A_3^+, 2H_3, 2K_3, L_1^+ + L_1^-, 2M_1^-]$                  | (1, 4)  |
| $[(\blacksquare)^{2T}, A_2^+ + A_3^+, H_1 + H_3, K_1 + K_3, 2L_1^+, 2M_1^-]$               | (1, 11) |
| $[(\blacksquare)^{2T}, A_2^+ + A_3^+, H_1 + H_3, K_1 + K_3, L_1^+ + L_1^-, 2M_1^-]$        | (1, 8)  |
| $[(\blacksquare)^{2T}, A_2^+ + A_3^+, 2H_3, 2K_3, 2L_1^-, 2M_1^+]$                         | (1, 7)  |
| $[(\blacksquare)^{2T}, A_2^+ + A_3^+, 2H_3, 2K_3, 2L_1^-, M_1^+ + M_1^-]$                  | (0, 4)  |
| $[(\blacksquare)^{2T}, A_2^+ + A_3^+, H_1 + H_3, K_1 + K_3, 2L_1^-, 2M_1^+]$               | (1, 11) |
| $[(\blacksquare)^{2T}, A_2^+ + A_3^+, H_1 + H_3, K_1 + K_3, 2L_1^-, M_1^+ + M_1^-]$        | (0, 8)  |
| $[(\blacksquare)^{2T}, A_2^+ + A_3^+, 2H_3, 2K_3, 2L_1^-, 2M_1^-]$                         | (1, 1)  |
| $[(\blacksquare)^{2T}, A_2^+ + A_3^+, H_1 + H_3, K_1 + K_3, 2L_1^-, 2M_1^-]$               | (1, 5)  |
| $[(\blacksquare)^{2T}, A_2^+ + A_3^+, 2H_1, 2K_1, 2L_1^+, 2M_1^+]$                         | (1, 9)  |
| $[(\blacksquare)^{2T}, A_2^+ + A_3^+, 2H_1, 2K_1, 2L_1^+, M_1^+ + M_1^-]$                  | (0, 6)  |
| $[(\blacksquare)^{2T}, A_2^+ + A_3^+, 2H_1, 2K_1, L_1^+ + L_1^-, 2M_1^+]$                  | (1, 6)  |
| $[(\blacksquare)^{2T}, A_2^+ + A_3^+, 2H_1, 2K_1, L_1^+ + L_1^-, M_1^+ + M_1^-]$           | (0, 3)  |

... continued on next page

... continued from previous page

|                                                                           |         |
|---------------------------------------------------------------------------|---------|
| $[(\blacksquare)^{2T}, A_2^+ + A_3^+, 2H_1, 2K_1, 2L_1^+, 2M_1^-]$        | (1, 3)  |
| $[(\blacksquare)^{2T}, A_2^+ + A_3^+, 2H_1, 2K_1, L_1^+ + L_1^-, 2M_1^-]$ | (1, 0)  |
| $[(\blacksquare)^{2T}, A_2^+ + A_3^+, 2H_1, 2K_1, 2L_1^-, 2M_1^+]$        | (1, 3)  |
| $[(\blacksquare)^{2T}, A_2^+ + A_3^+, 2H_1, 2K_1, 2L_1^-, M_1^+ + M_1^-]$ | trivial |
| $[(\blacksquare)^{2T}, A_2^+ + A_3^+, 2H_1, 2K_1, 2L_1^-, 2M_1^-]$        | (1, 9)  |

2nd minimal solution:  $\mu_2^T = 3$  (6400 symmetry vectors)

Space group 148 ( $\mathbb{Z}_2 \times \mathbb{Z}_4$ )

1st minimal solution:  $\mu_1^T = 2$  (36 symmetry vectors)

| $\mathbf{n}^T$                                                       | $\mathbf{v}^T \in \mathbb{Z}_2 \times \mathbb{Z}_4$ |
|----------------------------------------------------------------------|-----------------------------------------------------|
| $[(\blacksquare)^{2T}, T_2^- + T_3^-, 2F_1^-, 2L_1^+]$               | (1, 1)                                              |
| $[(\blacksquare)^{2T}, T_2^- + T_3^-, 2F_1^-, L_1^+ + L_1^-]$        | (1, 2)                                              |
| $[(\blacksquare)^{2T}, T_2^- + T_3^-, F_1^+ + F_1^-, 2L_1^+]$        | trivial                                             |
| $[(\blacksquare)^{2T}, T_2^- + T_3^-, F_1^+ + F_1^-, L_1^+ + L_1^-]$ | (0, 1)                                              |
| $[(\blacksquare)^{2T}, T_2^- + T_3^-, 2F_1^-, 2L_1^-]$               | (1, 3)                                              |
| $[(\blacksquare)^{2T}, T_2^- + T_3^-, F_1^+ + F_1^-, 2L_1^-]$        | (0, 2)                                              |
| $[(\blacksquare)^{2T}, T_2^- + T_3^-, 2F_1^+, 2L_1^+]$               | (1, 3)                                              |
| $[(\blacksquare)^{2T}, T_2^- + T_3^-, 2F_1^+, L_1^+ + L_1^-]$        | (1, 0)                                              |
| $[(\blacksquare)^{2T}, T_2^- + T_3^-, 2F_1^+, 2L_1^-]$               | (1, 1)                                              |
| $[(\blacksquare)^{2T}, T_2^+ + T_3^-, 2F_1^-, 2L_1^+]$               | (1, 2)                                              |
| $[(\blacksquare)^{2T}, T_2^+ + T_3^-, 2F_1^-, L_1^+ + L_1^-]$        | (1, 3)                                              |
| $[(\blacksquare)^{2T}, T_2^+ + T_3^-, F_1^+ + F_1^-, 2L_1^+]$        | (0, 1)                                              |
| $[(\blacksquare)^{2T}, T_2^+ + T_3^-, F_1^+ + F_1^-, L_1^+ + L_1^-]$ | (0, 2)                                              |
| $[(\blacksquare)^{2T}, T_2^+ + T_3^-, 2F_1^-, 2L_1^-]$               | (1, 0)                                              |
| $[(\blacksquare)^{2T}, T_2^+ + T_3^-, F_1^+ + F_1^-, 2L_1^-]$        | (0, 3)                                              |
| $[(\blacksquare)^{2T}, T_2^+ + T_3^-, 2F_1^+, 2L_1^+]$               | (1, 0)                                              |
| $[(\blacksquare)^{2T}, T_2^+ + T_3^-, 2F_1^+, L_1^+ + L_1^-]$        | (1, 1)                                              |
| $[(\blacksquare)^{2T}, T_2^+ + T_3^-, 2F_1^+, 2L_1^-]$               | (1, 2)                                              |
| $[(\blacksquare)^{2T}, T_2^- + T_3^+, 2F_1^-, 2L_1^+]$               | (1, 2)                                              |
| $[(\blacksquare)^{2T}, T_2^- + T_3^+, 2F_1^-, L_1^+ + L_1^-]$        | (1, 3)                                              |
| $[(\blacksquare)^{2T}, T_2^- + T_3^+, F_1^+ + F_1^-, 2L_1^+]$        | (0, 1)                                              |
| $[(\blacksquare)^{2T}, T_2^- + T_3^+, F_1^+ + F_1^-, L_1^+ + L_1^-]$ | (0, 2)                                              |
| $[(\blacksquare)^{2T}, T_2^- + T_3^+, 2F_1^-, 2L_1^-]$               | (1, 0)                                              |
| $[(\blacksquare)^{2T}, T_2^- + T_3^+, F_1^+ + F_1^-, 2L_1^-]$        | (0, 3)                                              |
| $[(\blacksquare)^{2T}, T_2^- + T_3^+, 2F_1^+, 2L_1^+]$               | (1, 0)                                              |
| $[(\blacksquare)^{2T}, T_2^- + T_3^+, 2F_1^+, L_1^+ + L_1^-]$        | (1, 1)                                              |
| $[(\blacksquare)^{2T}, T_2^- + T_3^+, 2F_1^+, 2L_1^-]$               | (1, 2)                                              |
| $[(\blacksquare)^{2T}, T_2^+ + T_3^-, 2F_1^-, 2L_1^+]$               | (1, 2)                                              |
| $[(\blacksquare)^{2T}, T_2^+ + T_3^-, 2F_1^-, L_1^+ + L_1^-]$        | (1, 3)                                              |
| $[(\blacksquare)^{2T}, T_2^+ + T_3^-, F_1^+ + F_1^-, 2L_1^+]$        | (0, 1)                                              |
| $[(\blacksquare)^{2T}, T_2^+ + T_3^-, F_1^+ + F_1^-, L_1^+ + L_1^-]$ | (0, 2)                                              |
| $[(\blacksquare)^{2T}, T_2^+ + T_3^-, 2F_1^-, 2L_1^-]$               | (1, 0)                                              |
| $[(\blacksquare)^{2T}, T_2^+ + T_3^-, F_1^+ + F_1^-, 2L_1^-]$        | (0, 3)                                              |
| $[(\blacksquare)^{2T}, T_2^+ + T_3^-, 2F_1^+, 2L_1^+]$               | (1, 0)                                              |
| $[(\blacksquare)^{2T}, T_2^+ + T_3^-, 2F_1^+, L_1^+ + L_1^-]$        | (1, 1)                                              |
| $[(\blacksquare)^{2T}, T_2^+ + T_3^-, 2F_1^+, 2L_1^-]$               | (1, 2)                                              |
| $[(\blacksquare)^{2T}, T_2^+ + T_3^+, 2F_1^-, 2L_1^+]$               | (1, 3)                                              |
| $[(\blacksquare)^{2T}, T_2^+ + T_3^+, 2F_1^-, L_1^+ + L_1^-]$        | (1, 0)                                              |
| $[(\blacksquare)^{2T}, T_2^+ + T_3^+, F_1^+ + F_1^-, 2L_1^+]$        | (0, 2)                                              |
| $[(\blacksquare)^{2T}, T_2^+ + T_3^+, F_1^+ + F_1^-, L_1^+ + L_1^-]$ | (0, 3)                                              |
| $[(\blacksquare)^{2T}, T_2^+ + T_3^+, 2F_1^-, 2L_1^-]$               | (1, 1)                                              |
| $[(\blacksquare)^{2T}, T_2^+ + T_3^+, F_1^+ + F_1^-, 2L_1^-]$        | trivial                                             |
| $[(\blacksquare)^{2T}, T_2^+ + T_3^+, 2F_1^+, 2L_1^+]$               | (1, 1)                                              |
| $[(\blacksquare)^{2T}, T_2^+ + T_3^+, 2F_1^+, L_1^+ + L_1^-]$        | (1, 2)                                              |
| $[(\blacksquare)^{2T}, T_2^+ + T_3^+, 2F_1^+, 2L_1^-]$               | (1, 3)                                              |

2nd minimal solution:  $\mu_2^T = 3$  (640 symmetry vectors)

Space group 149 ( $\mathbb{Z}_1$ )

1st minimal solution:  $\mu_1^T = 2$  (6 symmetry vectors)

| $\mathbf{n}^T$                                                      |
|---------------------------------------------------------------------|
| $[(\blacksquare)^{2T}, A_3, 2H_3, 2K_3, L_1 + L_2, 2M_2]$           |
| $[(\blacksquare)^{2T}, A_3, H_1 + H_3, K_1 + K_3, L_1 + L_2, 2M_2]$ |
| $[(\blacksquare)^{2T}, A_3, H_2 + H_3, K_2 + K_3, L_1 + L_2, 2M_2]$ |
| $[(\blacksquare)^{2T}, A_3, 2H_1, 2K_1, L_1 + L_2, 2M_2]$           |
| $[(\blacksquare)^{2T}, A_3, H_1 + H_2, K_1 + K_2, L_1 + L_2, 2M_2]$ |
| $[(\blacksquare)^{2T}, A_3, 2H_2, 2K_2, L_1 + L_2, 2M_2]$           |

2nd minimal solution:  $\mu_2^T = 3$  (40 symmetry vectors)

Space group 150 ( $\mathbb{Z}_1$ )

1st minimal solution:  $\mu_1^T = 2$  (1 symmetry vector)

| $\mathbf{n}^T$                                                                     |
|------------------------------------------------------------------------------------|
| $[(\blacksquare)^{2T}, A_3, H_1 + H_2, HA_1 + HA_2, 2K_2, 2KA_2, L_1 + L_2, 2M_2]$ |

2nd minimal solution:  $\mu_2^T = 3$  (10 symmetry vectors)

Space group 151 ( $\mathbb{Z}_1$ )

1st minimal solution:  $\mu_1^T = 3$  (4 symmetry vectors)

| $\mathbf{n}^T$                                                                                          |
|---------------------------------------------------------------------------------------------------------|
| $[(\blacksquare)^{2T} + \Gamma_2, A_1 + A_3, H_1 + H_2 + H_3, K_1 + K_2 + K_3, 2L_1 + L_2, 3M_2]$       |
| $[(\blacksquare)^{2T} + \Gamma_1, A_1 + A_3, H_1 + H_2 + H_3, K_1 + K_2 + K_3, 2L_1 + L_2, M_1 + 2M_2]$ |
| $[(\blacksquare)^{2T} + \Gamma_2, A_2 + A_3, H_1 + H_2 + H_3, K_1 + K_2 + K_3, L_1 + 2L_2, 3M_2]$       |
| $[(\blacksquare)^{2T} + \Gamma_1, A_2 + A_3, H_1 + H_2 + H_3, K_1 + K_2 + K_3, L_1 + 2L_2, M_1 + 2M_2]$ |

2nd minimal solution:  $\mu_2^T = 6$  (9 symmetry vectors)

Space group 152 ( $\mathbb{Z}_1$ )

1st minimal solution:  $\mu_1^T = 3$  (2 symmetry vectors)

| $\mathbf{n}^T$                                                                                                        |
|-----------------------------------------------------------------------------------------------------------------------|
| $[(\blacksquare)^{2T} + \Gamma_1, A_2 + A_3, H_2 + H_3, HA_2 + HA_3, K_2 + K_3, KA_2 + KA_3, 2L_1 + L_2, M_1 + 2M_2]$ |
| $[(\blacksquare)^{2T} + \Gamma_1, A_1 + A_3, H_1 + H_3, HA_1 + HA_3, K_2 + K_3, KA_2 + KA_3, L_1 + 2L_2, M_1 + 2M_2]$ |

2nd minimal solution:  $\mu_2^T = 6$  (6 symmetry vectors)

Space group 153 ( $\mathbb{Z}_1$ )

1st minimal solution:  $\mu_1^T = 3$  (4 symmetry vectors)

| $\mathbf{n}^T$                                                                                          |
|---------------------------------------------------------------------------------------------------------|
| $[(\blacksquare)^{2T} + \Gamma_2, A_1 + A_3, H_1 + H_2 + H_3, K_1 + K_2 + K_3, L_1 + 2L_2, 3M_2]$       |
| $[(\blacksquare)^{2T} + \Gamma_1, A_1 + A_3, H_1 + H_2 + H_3, K_1 + K_2 + K_3, L_1 + 2L_2, M_1 + 2M_2]$ |
| $[(\blacksquare)^{2T} + \Gamma_2, A_2 + A_3, H_1 + H_2 + H_3, K_1 + K_2 + K_3, 2L_1 + L_2, 3M_2]$       |
| $[(\blacksquare)^{2T} + \Gamma_1, A_2 + A_3, H_1 + H_2 + H_3, K_1 + K_2 + K_3, 2L_1 + L_2, M_1 + 2M_2]$ |

2nd minimal solution:  $\mu_2^T = 6$  (9 symmetry vectors)

Space group 154 ( $\mathbb{Z}_1$ )

1st minimal solution:  $\mu_1^T = 3$  (2 symmetry vectors)

| $\mathbf{n}^T$                                                                                                        |
|-----------------------------------------------------------------------------------------------------------------------|
| $[(\blacksquare)^{2T} + \Gamma_1, A_1 + A_3, H_1 + H_3, HA_1 + HA_3, K_2 + K_3, KA_2 + KA_3, L_1 + 2L_2, M_1 + 2M_2]$ |
| $[(\blacksquare)^{2T} + \Gamma_1, A_2 + A_3, H_2 + H_3, HA_2 + HA_3, K_2 + K_3, KA_2 + KA_3, 2L_1 + L_2, M_1 + 2M_2]$ |

2nd minimal solution:  $\mu_2^T = 6$  (6 symmetry vectors)

Space group 155 ( $\mathbb{Z}_1$ )

1st minimal solution:  $\mu_1^T = 2$  (1 symmetry vector)

| $\mathbf{n}^T$                                |
|-----------------------------------------------|
| $[(\blacksquare)^{2T}, T_3, 2F_2, L_1 + L_2]$ |

2nd minimal solution:  $\mu_2^T = 3$  (4 symmetry vectors)

Space group 156 ( $\mathbb{Z}_1$ )

1st minimal solution:  $\mu_1^T = 2$  (6 symmetry vectors)

| $\mathbf{n}^T$                                                           |
|--------------------------------------------------------------------------|
| $[(\blacksquare)^{2T}, A_3, 2H_3, 2K_3, L_1 + L_2, M_1 + M_2]$           |
| $[(\blacksquare)^{2T}, A_3, H_1 + H_3, K_1 + K_3, L_1 + L_2, M_1 + M_2]$ |
| $[(\blacksquare)^{2T}, A_3, H_2 + H_3, K_2 + K_3, L_1 + L_2, M_1 + M_2]$ |
| $[(\blacksquare)^{2T}, A_3, 2H_1, 2K_1, L_1 + L_2, M_1 + M_2]$           |
| $[(\blacksquare)^{2T}, A_3, H_1 + H_2, K_1 + K_2, L_1 + L_2, M_1 + M_2]$ |
| $[(\blacksquare)^{2T}, A_3, 2H_2, 2K_2, L_1 + L_2, M_1 + M_2]$           |

2nd minimal solution:  $\mu_2^T = 3$  (20 symmetry vectors)

Space group 157 ( $\mathbb{Z}_1$ )

1st minimal solution:  $\mu_1^T = 2$  (4 symmetry vectors)

| $\mathbf{n}^T$                                                                                     |
|----------------------------------------------------------------------------------------------------|
| $[(\blacksquare)^{2T}, A_3, H_3, HA_3, K_3, KA_3, L_1 + L_2, M_1 + M_2]$                           |
| $[(\blacksquare)^{2T}, A_3, H_3, HA_1 + HA_2, K_3, KA_1 + KA_2, L_1 + L_2, M_1 + M_2]$             |
| $[(\blacksquare)^{2T}, A_3, H_1 + H_2, HA_3, K_1 + K_2, KA_3, L_1 + L_2, M_1 + M_2]$               |
| $[(\blacksquare)^{2T}, A_3, H_1 + H_2, HA_1 + HA_2, K_1 + K_2, KA_1 + KA_2, L_1 + L_2, M_1 + M_2]$ |

2nd minimal solution:  $\mu_2^T = 3$  (8 symmetry vectors)

Space group 158 ( $\mathbb{Z}_1$ )

1st minimal solution:  $\mu_1^T = 2$  (6 symmetry vectors)

| $\mathbf{n}^T$                                                           |
|--------------------------------------------------------------------------|
| $[(\blacksquare)^{2T}, A_3, 2H_3, 2K_3, L_1 + L_2, M_1 + M_2]$           |
| $[(\blacksquare)^{2T}, A_3, H_1 + H_3, K_1 + K_3, L_1 + L_2, M_1 + M_2]$ |
| $[(\blacksquare)^{2T}, A_3, 2H_1, 2K_1, L_1 + L_2, M_1 + M_2]$           |
| $[(\blacksquare)^{2T}, A_3, H_2 + H_3, K_2 + K_3, L_1 + L_2, M_1 + M_2]$ |
| $[(\blacksquare)^{2T}, A_3, H_1 + H_2, K_1 + K_2, L_1 + L_2, M_1 + M_2]$ |
| $[(\blacksquare)^{2T}, A_3, 2H_2, 2K_2, L_1 + L_2, M_1 + M_2]$           |

2nd minimal solution:  $\mu_2^T = 4$  (30 symmetry vectors)

Space group 159 ( $\mathbb{Z}_1$ )

1st minimal solution:  $\mu_1^T = 2$  (4 symmetry vectors)

| $\mathbf{n}^T$                                                                                     |
|----------------------------------------------------------------------------------------------------|
| $[(\blacksquare)^{2T}, A_3, H_3, HA_3, K_3, KA_3, L_1 + L_2, M_1 + M_2]$                           |
| $[(\blacksquare)^{2T}, A_3, H_3, HA_1 + HA_2, K_3, KA_1 + KA_2, L_1 + L_2, M_1 + M_2]$             |
| $[(\blacksquare)^{2T}, A_3, H_1 + H_2, HA_3, K_1 + K_2, KA_3, L_1 + L_2, M_1 + M_2]$               |
| $[(\blacksquare)^{2T}, A_3, H_1 + H_2, HA_1 + HA_2, K_1 + K_2, KA_1 + KA_2, L_1 + L_2, M_1 + M_2]$ |

2nd minimal solution:  $\mu_2^T = 4$  (18 symmetry vectors)

Space group 160 ( $\mathbb{Z}_1$ )

1st minimal solution:  $\mu_1^T = 2$  (1 symmetry vector)

| $\mathbf{n}^T$                                     |
|----------------------------------------------------|
| $[(\blacksquare)^{2T}, T_3, F_1 + F_2, L_1 + L_2]$ |

2nd minimal solution:  $\mu_2^T = 3$  (2 symmetry vectors)

Space group 161 ( $\mathbb{Z}_1$ )

1st minimal solution:  $\mu_1^T = 2$  (1 symmetry vector)

| $\mathbf{n}^T$                                     |
|----------------------------------------------------|
| $[(\blacksquare)^{2T}, T_3, F_1 + F_2, L_1 + L_2]$ |

2nd minimal solution:  $\mu_2^T = 4$  (2 symmetry vectors)

Space group 162 ( $\mathbb{Z}_2$ )

1st minimal solution:  $\mu_1^T = 2$  (8 symmetry vectors)

| $\mathbf{n}^T$                                                                     | $\mathbf{v}^T \in \mathbb{Z}_2$ |
|------------------------------------------------------------------------------------|---------------------------------|
| $[(\blacksquare)^{2T}, A_3^-, H_3, K_3, L_1^- + L_2^-, M_2^+ + M_2^-]$             | 1                               |
| $[(\blacksquare)^{2T}, A_3^-, H_3, K_3, L_1^+ + L_2^+, M_2^+ + M_2^-]$             | trivial                         |
| $[(\blacksquare)^{2T}, A_3^-, H_1 + H_2, K_1 + K_2, L_1^- + L_2^-, M_2^+ + M_2^-]$ | 1                               |
| $[(\blacksquare)^{2T}, A_3^-, H_1 + H_2, K_1 + K_2, L_1^+ + L_2^+, M_2^+ + M_2^-]$ | trivial                         |
| $[(\blacksquare)^{2T}, A_3^+, H_3, K_3, L_1^- + L_2^-, M_2^+ + M_2^-]$             | trivial                         |
| $[(\blacksquare)^{2T}, A_3^+, H_3, K_3, L_1^+ + L_2^+, M_2^+ + M_2^-]$             | 1                               |
| $[(\blacksquare)^{2T}, A_3^+, H_1 + H_2, K_1 + K_2, L_1^- + L_2^-, M_2^+ + M_2^-]$ | trivial                         |
| $[(\blacksquare)^{2T}, A_3^+, H_1 + H_2, K_1 + K_2, L_1^+ + L_2^+, M_2^+ + M_2^-]$ | 1                               |

2nd minimal solution:  $\mu_2^T = 3$  (96 symmetry vectors)

Space group 163 ( $\mathbb{Z}_2$ )

1st minimal solution:  $\mu_1^T = 2$  (4 symmetry vectors & filling-enforced topology)

| $\mathbf{n}^T$                                                         | $\mathbf{v}^T \in \mathbb{Z}_2$ |
|------------------------------------------------------------------------|---------------------------------|
| $[(\blacksquare)^{2T}, A_2, H_3, K_3, L_1, M_2^+ + M_2^-]$             | 1                               |
| $[(\blacksquare)^{2T}, A_2, H_1 + H_2, K_1 + K_2, L_1, M_2^+ + M_2^-]$ | 1                               |
| $[(\blacksquare)^{2T}, A_1, H_3, K_3, L_1, M_2^+ + M_2^-]$             | 1                               |
| $[(\blacksquare)^{2T}, A_1, H_1 + H_2, K_1 + K_2, L_1, M_2^+ + M_2^-]$ | 1                               |

2nd minimal solution:  $\mu_2^T = 4$  (84 symmetry vectors)

Space group 164 ( $\mathbb{Z}_2$ )

1st minimal solution:  $\mu_1^T = 2$  (4 symmetry vectors)

| $\mathbf{n}^T$                                                                | $\mathbf{v}^T \in \mathbb{Z}_2$ |
|-------------------------------------------------------------------------------|---------------------------------|
| $[(\blacksquare)^{2T}, A_3^-, H_1 + H_2, 2K_2, L_1^- + L_2^-, M_2^+ + M_2^-]$ | 1                               |
| $[(\blacksquare)^{2T}, A_3^-, H_1 + H_2, 2K_2, L_1^+ + L_2^+, M_2^+ + M_2^-]$ | trivial                         |
| $[(\blacksquare)^{2T}, A_3^+, H_1 + H_2, 2K_2, L_1^- + L_2^-, M_2^+ + M_2^-]$ | trivial                         |
| $[(\blacksquare)^{2T}, A_3^+, H_1 + H_2, 2K_2, L_1^+ + L_2^+, M_2^+ + M_2^-]$ | 1                               |

2nd minimal solution:  $\mu_2^T = 3$  (80 symmetry vectors)

Space group 165 ( $\mathbb{Z}_2$ )

1st minimal solution:  $\mu_1^T = 2$  (2 symmetry vectors & filling-enforced topology)

| $\mathbf{n}^T$                                                    | $\mathbf{v}^T \in \mathbb{Z}_2$ |
|-------------------------------------------------------------------|---------------------------------|
| $[(\blacksquare)^{2T}, A_1, H_1 + H_2, 2K_2, L_1, M_2^+ + M_2^-]$ | 1                               |
| $[(\blacksquare)^{2T}, A_2, H_1 + H_2, 2K_2, L_1, M_2^+ + M_2^-]$ | 1                               |

2nd minimal solution:  $\mu_2^T = 4$  (60 symmetry vectors)

Space group 166 ( $\mathbb{Z}_2$ )

1st minimal solution:  $\mu_1^T = 2$  (4 symmetry vectors)

| $\mathbf{n}^T$                                               | $\mathbf{v}^T \in \mathbb{Z}_2$ |
|--------------------------------------------------------------|---------------------------------|
| $[(\blacksquare)^{2T}, T_3^-, F_2^+ + F_2^-, L_1^- + L_2^-]$ | 1                               |
| $[(\blacksquare)^{2T}, T_3^-, F_2^+ + F_2^-, L_1^+ + L_2^+]$ | trivial                         |
| $[(\blacksquare)^{2T}, T_3^+, F_2^+ + F_2^-, L_1^- + L_2^-]$ | trivial                         |
| $[(\blacksquare)^{2T}, T_3^+, F_2^+ + F_2^-, L_1^+ + L_2^+]$ | 1                               |

2nd minimal solution:  $\mu_2^T = 3$  (48 symmetry vectors)

Space group 167 ( $\mathbb{Z}_2$ )

1st minimal solution:  $\mu_1^T = 2$  (2 symmetry vectors & filling-enforced topology)

| $\mathbf{n}^T$                                   | $\mathbf{v}^T \in \mathbb{Z}_2$ |
|--------------------------------------------------|---------------------------------|
| $[(\blacksquare)^{2T}, T_2, F_2^+ + F_2^-, L_1]$ | 1                               |
| $[(\blacksquare)^{2T}, T_1, F_2^+ + F_2^-, L_1]$ | 1                               |

2nd minimal solution:  $\mu_2^T = 4$  (28 symmetry vectors)

Space group 168 ( $\mathbb{Z}_6$ )

1st minimal solution:  $\mu_1^T = 2$  (18 symmetry vectors)

| $\mathbf{n}^T$                                                                 | $\mathbf{v}^T \in \mathbb{Z}_6$ |
|--------------------------------------------------------------------------------|---------------------------------|
| $[(\blacksquare)^{2T}, A_4 + A_6, 2H_2, 2K_2, 2L_1, 2M_1]$                     | 2                               |
| $[(\blacksquare)^{2T}, A_4 + A_6, 2H_2, 2K_2, L_1 + L_2, M_1 + M_2]$           | 5                               |
| $[(\blacksquare)^{2T}, A_4 + A_6, H_2 + H_3, K_2 + K_3, 2L_1, 2M_1]$           | trivial                         |
| $[(\blacksquare)^{2T}, A_4 + A_6, H_2 + H_3, K_2 + K_3, L_1 + L_2, M_1 + M_2]$ | 3                               |
| $[(\blacksquare)^{2T}, A_4 + A_6, H_1 + H_2, K_1 + K_2, 2L_1, 2M_1]$           | 4                               |
| $[(\blacksquare)^{2T}, A_4 + A_6, H_1 + H_2, K_1 + K_2, L_1 + L_2, M_1 + M_2]$ | 1                               |
| $[(\blacksquare)^{2T}, A_4 + A_6, 2H_2, 2K_2, 2L_2, 2M_2]$                     | 2                               |
| $[(\blacksquare)^{2T}, A_4 + A_6, H_2 + H_3, K_2 + K_3, 2L_2, 2M_2]$           | trivial                         |
| $[(\blacksquare)^{2T}, A_4 + A_6, H_1 + H_2, K_1 + K_2, 2L_2, 2M_2]$           | 4                               |
| $[(\blacksquare)^{2T}, A_4 + A_6, 2H_3, 2K_3, 2L_1, 2M_1]$                     | 4                               |
| $[(\blacksquare)^{2T}, A_4 + A_6, 2H_3, 2K_3, L_1 + L_2, M_1 + M_2]$           | 1                               |
| $[(\blacksquare)^{2T}, A_4 + A_6, H_1 + H_3, K_1 + K_3, 2L_1, 2M_1]$           | 2                               |
| $[(\blacksquare)^{2T}, A_4 + A_6, H_1 + H_3, K_1 + K_3, L_1 + L_2, M_1 + M_2]$ | 5                               |
| $[(\blacksquare)^{2T}, A_4 + A_6, 2H_3, 2K_3, 2L_2, 2M_2]$                     | 4                               |
| $[(\blacksquare)^{2T}, A_4 + A_6, H_1 + H_3, K_1 + K_3, 2L_2, 2M_2]$           | 2                               |
| $[(\blacksquare)^{2T}, A_4 + A_6, 2H_1, 2K_1, 2L_1, 2M_1]$                     | trivial                         |
| $[(\blacksquare)^{2T}, A_4 + A_6, 2H_1, 2K_1, L_1 + L_2, M_1 + M_2]$           | 3                               |
| $[(\blacksquare)^{2T}, A_4 + A_6, 2H_1, 2K_1, 2L_2, 2M_2]$                     | trivial                         |

2nd minimal solution:  $\mu_2^T = 3$  (240 symmetry vectors)

Space group 169 ( $\mathbb{Z}_1$ )

1st minimal solution:  $\mu_1^T = 6$  (1 symmetry vector)

| $\mathbf{n}^T$                                                                                                                                                           |
|--------------------------------------------------------------------------------------------------------------------------------------------------------------------------|
| $[(\blacksquare)^{2T} + \Gamma_1 + \Gamma_2 + \Gamma_3 + \Gamma_5, A_1 + A_2 + A_3 + A_4 + A_5 + A_6, 2H_1 + 2H_2 + 2H_3, 2K_1 + 2K_2 + 2K_3, 3L_1 + 3L_2, 3M_1 + 3M_2]$ |

2nd minimal solution:  $\mu_2^T = 12$  (1 symmetry vector)

Space group 170 ( $\mathbb{Z}_1$ )

1st minimal solution:  $\mu_1^T = 6$  (1 symmetry vector)

| $\mathbf{n}^T$                                                                                                                                                           |
|--------------------------------------------------------------------------------------------------------------------------------------------------------------------------|
| $[(\blacksquare)^{2T} + \Gamma_1 + \Gamma_2 + \Gamma_3 + \Gamma_5, A_1 + A_2 + A_3 + A_4 + A_5 + A_6, 2H_1 + 2H_2 + 2H_3, 2K_1 + 2K_2 + 2K_3, 3L_1 + 3L_2, 3M_1 + 3M_2]$ |

2nd minimal solution:  $\mu_2^T = 12$  (1 symmetry vector)

Space group 171 ( $\mathbb{Z}_2$ )

1st minimal solution:  $\mu_1^T = 3$  (4 symmetry vectors)



| $\mathbf{n}^T$                                                                                                | $\mathbf{v}^T \in \mathbb{Z}_2$ |
|---------------------------------------------------------------------------------------------------------------|---------------------------------|
| $[(\blacksquare)^{2T} + \Gamma_2, A_2 + A_4 + A_6, H_1 + H_2 + H_3, K_1 + K_2 + K_3, 3L_2, 3M_2]$             | trivial                         |
| $[(\blacksquare)^{2T} + \Gamma_2, A_2 + A_4 + A_6, H_1 + H_2 + H_3, K_1 + K_2 + K_3, L_1 + 2L_2, M_1 + 2M_2]$ | 1                               |
| $[(\blacksquare)^{2T} + \Gamma_2, A_2 + A_4 + A_6, H_1 + H_2 + H_3, K_1 + K_2 + K_3, 2L_1 + L_2, 2M_1 + M_2]$ | trivial                         |
| $[(\blacksquare)^{2T} + \Gamma_2, A_2 + A_4 + A_6, H_1 + H_2 + H_3, K_1 + K_2 + K_3, 3L_1, 3M_1]$             | 1                               |

2nd minimal solution:  $\mu_2^T = 6$  (14 symmetry vectors)

Space group 172 ( $\mathbb{Z}_2$ )

1st minimal solution:  $\mu_1^T = 3$  (4 symmetry vectors)

| $\mathbf{n}^T$                                                                                                | $\mathbf{v}^T \in \mathbb{Z}_2$ |
|---------------------------------------------------------------------------------------------------------------|---------------------------------|
| $[(\blacksquare)^{2T} + \Gamma_2, A_2 + A_4 + A_6, H_1 + H_2 + H_3, K_1 + K_2 + K_3, 3L_2, 3M_2]$             | trivial                         |
| $[(\blacksquare)^{2T} + \Gamma_2, A_2 + A_4 + A_6, H_1 + H_2 + H_3, K_1 + K_2 + K_3, L_1 + 2L_2, M_1 + 2M_2]$ | 1                               |
| $[(\blacksquare)^{2T} + \Gamma_2, A_2 + A_4 + A_6, H_1 + H_2 + H_3, K_1 + K_2 + K_3, 2L_1 + L_2, 2M_1 + M_2]$ | trivial                         |
| $[(\blacksquare)^{2T} + \Gamma_2, A_2 + A_4 + A_6, H_1 + H_2 + H_3, K_1 + K_2 + K_3, 3L_1, 3M_1]$             | 1                               |

2nd minimal solution:  $\mu_2^T = 6$  (14 symmetry vectors)

Space group 173 ( $\mathbb{Z}_3$ )

1st minimal solution:  $\mu_1^T = 4$  (15 symmetry vectors)

| $\mathbf{n}^T$                                                                                                                     | $\mathbf{v}^T \in \mathbb{Z}_3$ |
|------------------------------------------------------------------------------------------------------------------------------------|---------------------------------|
| $[(\blacksquare)^{2T} + \Gamma_3 + \Gamma_5, A_3 + A_4 + A_5 + A_6, 4H_2, 4K_2, 2L_1 + 2L_2, 2M_1 + 2M_2]$                         | 1                               |
| $[(\blacksquare)^{2T} + \Gamma_3 + \Gamma_5, A_3 + A_4 + A_5 + A_6, 3H_2 + H_3, 3K_2 + K_3, 2L_1 + 2L_2, 2M_1 + 2M_2]$             | 2                               |
| $[(\blacksquare)^{2T} + \Gamma_3 + \Gamma_5, A_3 + A_4 + A_5 + A_6, 2H_2 + 2H_3, 2K_2 + 2K_3, 2L_1 + 2L_2, 2M_1 + 2M_2]$           | trivial                         |
| $[(\blacksquare)^{2T} + \Gamma_3 + \Gamma_5, A_3 + A_4 + A_5 + A_6, H_1 + 3H_2, K_1 + 3K_2, 2L_1 + 2L_2, 2M_1 + 2M_2]$             | trivial                         |
| $[(\blacksquare)^{2T} + \Gamma_3 + \Gamma_5, A_3 + A_4 + A_5 + A_6, H_1 + 2H_2 + H_3, K_1 + 2K_2 + K_3, 2L_1 + 2L_2, 2M_1 + 2M_2]$ | 1                               |
| $[(\blacksquare)^{2T} + \Gamma_3 + \Gamma_5, A_3 + A_4 + A_5 + A_6, 2H_1 + 2H_2, 2K_1 + 2K_2, 2L_1 + 2L_2, 2M_1 + 2M_2]$           | 2                               |
| $[(\blacksquare)^{2T} + \Gamma_3 + \Gamma_5, A_3 + A_4 + A_5 + A_6, H_2 + 3H_3, K_2 + 3K_3, 2L_1 + 2L_2, 2M_1 + 2M_2]$             | 1                               |
| $[(\blacksquare)^{2T} + \Gamma_3 + \Gamma_5, A_3 + A_4 + A_5 + A_6, H_1 + H_2 + 2H_3, K_1 + K_2 + 2K_3, 2L_1 + 2L_2, 2M_1 + 2M_2]$ | 2                               |
| $[(\blacksquare)^{2T} + \Gamma_3 + \Gamma_5, A_3 + A_4 + A_5 + A_6, 2H_1 + H_2 + H_3, 2K_1 + K_2 + K_3, 2L_1 + 2L_2, 2M_1 + 2M_2]$ | trivial                         |
| $[(\blacksquare)^{2T} + \Gamma_3 + \Gamma_5, A_3 + A_4 + A_5 + A_6, 4H_3, 4K_3, 2L_1 + 2L_2, 2M_1 + 2M_2]$                         | 2                               |
| $[(\blacksquare)^{2T} + \Gamma_3 + \Gamma_5, A_3 + A_4 + A_5 + A_6, H_1 + 3H_3, K_1 + 3K_3, 2L_1 + 2L_2, 2M_1 + 2M_2]$             | trivial                         |
| $[(\blacksquare)^{2T} + \Gamma_3 + \Gamma_5, A_3 + A_4 + A_5 + A_6, 2H_1 + 2H_3, 2K_1 + 2K_3, 2L_1 + 2L_2, 2M_1 + 2M_2]$           | 1                               |
| $[(\blacksquare)^{2T} + \Gamma_3 + \Gamma_5, A_3 + A_4 + A_5 + A_6, 3H_1 + H_2, 3K_1 + K_2, 2L_1 + 2L_2, 2M_1 + 2M_2]$             | 1                               |
| $[(\blacksquare)^{2T} + \Gamma_3 + \Gamma_5, A_3 + A_4 + A_5 + A_6, 3H_1 + H_3, 3K_1 + K_3, 2L_1 + 2L_2, 2M_1 + 2M_2]$             | 2                               |
| $[(\blacksquare)^{2T} + \Gamma_3 + \Gamma_5, A_3 + A_4 + A_5 + A_6, 4H_1, 4K_1, 2L_1 + 2L_2, 2M_1 + 2M_2]$                         | trivial                         |

2nd minimal solution:  $\mu_2^T = 6$  (84 symmetry vectors)

Space group 174 ( $\mathbb{Z}_3 \times \mathbb{Z}_3 \times \mathbb{Z}_3$ )

1st minimal solution:  $\mu_1^T = 2$  (612 symmetry vectors)

| $n^T$                                                                                               | $v^T \in \mathbb{Z}_3 \times \mathbb{Z}_3 \times \mathbb{Z}_3$ |
|-----------------------------------------------------------------------------------------------------|----------------------------------------------------------------|
| $[(\blacksquare)^{2T}, A_4 + A_6, 2H_6, 2HA_4, K_5 + K_6, KA_3 + KA_4, 2L_2, M_1 + M_2]$            | (0, 1, 1)                                                      |
| $[(\blacksquare)^{2T}, A_4 + A_6, 2H_6, HA_4 + HA_6, K_5 + K_6, KA_3 + KA_6, 2L_2, M_1 + M_2]$      | (0, 2, 1)                                                      |
| $[(\blacksquare)^{2T}, A_4 + A_6, 2H_6, HA_2 + HA_4, K_5 + K_6, KA_2 + KA_3, 2L_2, M_1 + M_2]$      | (0, 0, 1)                                                      |
| $[(\blacksquare)^{2T}, A_4 + A_6, H_4 + H_6, 2HA_4, K_4 + K_5, KA_3 + KA_4, 2L_2, M_1 + M_2]$       | (0, 2, 1)                                                      |
| $[(\blacksquare)^{2T}, A_4 + A_6, H_4 + H_6, HA_4 + HA_6, K_4 + K_5, KA_3 + KA_6, 2L_2, M_1 + M_2]$ | (0, 0, 1)                                                      |
| $[(\blacksquare)^{2T}, A_4 + A_6, H_4 + H_6, HA_2 + HA_4, K_4 + K_5, KA_2 + KA_3, 2L_2, M_1 + M_2]$ | (0, 1, 1)                                                      |
| $[(\blacksquare)^{2T}, A_4 + A_6, H_2 + H_6, 2HA_4, K_2 + K_5, KA_3 + KA_4, 2L_2, M_1 + M_2]$       | (0, 0, 1)                                                      |
| $[(\blacksquare)^{2T}, A_4 + A_6, H_2 + H_6, HA_4 + HA_6, K_2 + K_5, KA_3 + KA_6, 2L_2, M_1 + M_2]$ | (0, 1, 1)                                                      |
| $[(\blacksquare)^{2T}, A_4 + A_6, H_2 + H_6, HA_2 + HA_4, K_2 + K_5, KA_2 + KA_3, 2L_2, M_1 + M_2]$ | (0, 2, 1)                                                      |
| $[(\blacksquare)^{2T}, A_4 + A_6, 2H_6, HA_4 + HA_6, K_5 + K_6, KA_4 + KA_5, 2L_2, M_1 + M_2]$      | (0, 2, 0)                                                      |
| $[(\blacksquare)^{2T}, A_4 + A_6, 2H_6, 2HA_6, K_5 + K_6, KA_5 + KA_6, 2L_2, M_1 + M_2]$            | trivial                                                        |
| $[(\blacksquare)^{2T}, A_4 + A_6, 2H_6, HA_2 + HA_6, K_5 + K_6, KA_2 + KA_5, 2L_2, M_1 + M_2]$      | (0, 1, 0)                                                      |
| $[(\blacksquare)^{2T}, A_4 + A_6, H_4 + H_6, HA_4 + HA_6, K_4 + K_5, KA_4 + KA_5, 2L_2, M_1 + M_2]$ | trivial                                                        |
| $[(\blacksquare)^{2T}, A_4 + A_6, H_4 + H_6, 2HA_6, K_4 + K_5, KA_5 + KA_6, 2L_2, M_1 + M_2]$       | (0, 1, 0)                                                      |
| $[(\blacksquare)^{2T}, A_4 + A_6, H_4 + H_6, HA_2 + HA_6, K_4 + K_5, KA_2 + KA_5, 2L_2, M_1 + M_2]$ | (0, 2, 0)                                                      |
| $[(\blacksquare)^{2T}, A_4 + A_6, H_2 + H_6, HA_4 + HA_6, K_2 + K_5, KA_4 + KA_5, 2L_2, M_1 + M_2]$ | (0, 1, 0)                                                      |
| $[(\blacksquare)^{2T}, A_4 + A_6, H_2 + H_6, 2HA_6, K_2 + K_5, KA_5 + KA_6, 2L_2, M_1 + M_2]$       | (0, 2, 0)                                                      |
| $[(\blacksquare)^{2T}, A_4 + A_6, H_2 + H_6, HA_2 + HA_6, K_2 + K_5, KA_2 + KA_5, 2L_2, M_1 + M_2]$ | trivial                                                        |
| $[(\blacksquare)^{2T}, A_4 + A_6, 2H_6, HA_2 + HA_4, K_5 + K_6, KA_1 + KA_4, 2L_2, M_1 + M_2]$      | (0, 0, 2)                                                      |
| $[(\blacksquare)^{2T}, A_4 + A_6, 2H_6, HA_2 + HA_6, K_5 + K_6, KA_1 + KA_6, 2L_2, M_1 + M_2]$      | (0, 1, 2)                                                      |
| $[(\blacksquare)^{2T}, A_4 + A_6, 2H_6, 2HA_2, K_5 + K_6, KA_1 + KA_2, 2L_2, M_1 + M_2]$            | (0, 2, 2)                                                      |
| $[(\blacksquare)^{2T}, A_4 + A_6, H_4 + H_6, HA_2 + HA_4, K_4 + K_5, KA_1 + KA_4, 2L_2, M_1 + M_2]$ | (0, 1, 2)                                                      |
| $[(\blacksquare)^{2T}, A_4 + A_6, H_4 + H_6, HA_2 + HA_6, K_4 + K_5, KA_1 + KA_6, 2L_2, M_1 + M_2]$ | (0, 2, 2)                                                      |
| $[(\blacksquare)^{2T}, A_4 + A_6, H_4 + H_6, 2HA_2, K_4 + K_5, KA_1 + KA_2, 2L_2, M_1 + M_2]$       | (0, 0, 2)                                                      |
| $[(\blacksquare)^{2T}, A_4 + A_6, H_2 + H_6, HA_2 + HA_4, K_2 + K_5, KA_1 + KA_4, 2L_2, M_1 + M_2]$ | (0, 2, 2)                                                      |
| $[(\blacksquare)^{2T}, A_4 + A_6, H_2 + H_6, HA_2 + HA_6, K_2 + K_5, KA_1 + KA_6, 2L_2, M_1 + M_2]$ | (0, 0, 2)                                                      |
| $[(\blacksquare)^{2T}, A_4 + A_6, H_2 + H_6, 2HA_2, K_2 + K_5, KA_1 + KA_2, 2L_2, M_1 + M_2]$       | (0, 1, 2)                                                      |
| $[(\blacksquare)^{2T}, A_4 + A_6, H_4 + H_6, 2HA_4, K_3 + K_6, KA_3 + KA_4, 2L_2, M_1 + M_2]$       | (0, 2, 0)                                                      |
| $[(\blacksquare)^{2T}, A_4 + A_6, H_4 + H_6, HA_4 + HA_6, K_3 + K_6, KA_3 + KA_6, 2L_2, M_1 + M_2]$ | trivial                                                        |
| $[(\blacksquare)^{2T}, A_4 + A_6, H_4 + H_6, HA_2 + HA_4, K_3 + K_6, KA_2 + KA_3, 2L_2, M_1 + M_2]$ | (0, 1, 0)                                                      |
| $[(\blacksquare)^{2T}, A_4 + A_6, 2H_4, 2HA_4, K_3 + K_4, KA_3 + KA_4, 2L_2, M_1 + M_2]$            | trivial                                                        |
| $[(\blacksquare)^{2T}, A_4 + A_6, 2H_4, HA_4 + HA_6, K_3 + K_4, KA_3 + KA_6, 2L_2, M_1 + M_2]$      | (0, 1, 0)                                                      |
| $[(\blacksquare)^{2T}, A_4 + A_6, 2H_4, HA_2 + HA_4, K_3 + K_4, KA_2 + KA_3, 2L_2, M_1 + M_2]$      | (0, 2, 0)                                                      |
| $[(\blacksquare)^{2T}, A_4 + A_6, H_2 + H_4, 2HA_4, K_2 + K_3, KA_3 + KA_4, 2L_2, M_1 + M_2]$       | (0, 1, 0)                                                      |
| $[(\blacksquare)^{2T}, A_4 + A_6, H_2 + H_4, HA_4 + HA_6, K_2 + K_3, KA_3 + KA_6, 2L_2, M_1 + M_2]$ | (0, 2, 0)                                                      |
| $[(\blacksquare)^{2T}, A_4 + A_6, H_2 + H_4, HA_2 + HA_4, K_2 + K_3, KA_2 + KA_3, 2L_2, M_1 + M_2]$ | trivial                                                        |
| $[(\blacksquare)^{2T}, A_4 + A_6, H_4 + H_6, HA_4 + HA_6, K_3 + K_6, KA_4 + KA_5, 2L_2, M_1 + M_2]$ | (0, 0, 2)                                                      |
| $[(\blacksquare)^{2T}, A_4 + A_6, H_4 + H_6, 2HA_6, K_3 + K_6, KA_5 + KA_6, 2L_2, M_1 + M_2]$       | (0, 1, 2)                                                      |
| $[(\blacksquare)^{2T}, A_4 + A_6, H_4 + H_6, HA_2 + HA_6, K_3 + K_6, KA_2 + KA_5, 2L_2, M_1 + M_2]$ | (0, 2, 2)                                                      |
| $[(\blacksquare)^{2T}, A_4 + A_6, 2H_4, HA_4 + HA_6, K_3 + K_4, KA_4 + KA_5, 2L_2, M_1 + M_2]$      | (0, 1, 2)                                                      |
| $[(\blacksquare)^{2T}, A_4 + A_6, 2H_4, 2HA_6, K_3 + K_4, KA_5 + KA_6, 2L_2, M_1 + M_2]$            | (0, 2, 2)                                                      |
| $[(\blacksquare)^{2T}, A_4 + A_6, 2H_4, HA_2 + HA_6, K_3 + K_4, KA_2 + KA_5, 2L_2, M_1 + M_2]$      | (0, 0, 2)                                                      |
| $[(\blacksquare)^{2T}, A_4 + A_6, H_2 + H_4, HA_4 + HA_6, K_2 + K_3, KA_4 + KA_5, 2L_2, M_1 + M_2]$ | (0, 2, 2)                                                      |
| $[(\blacksquare)^{2T}, A_4 + A_6, H_2 + H_4, 2HA_6, K_2 + K_3, KA_5 + KA_6, 2L_2, M_1 + M_2]$       | (0, 0, 2)                                                      |
| $[(\blacksquare)^{2T}, A_4 + A_6, H_2 + H_4, HA_2 + HA_6, K_2 + K_3, KA_2 + KA_5, 2L_2, M_1 + M_2]$ | (0, 1, 2)                                                      |
| $[(\blacksquare)^{2T}, A_4 + A_6, H_4 + H_6, HA_2 + HA_4, K_3 + K_6, KA_1 + KA_4, 2L_2, M_1 + M_2]$ | (0, 1, 1)                                                      |
| $[(\blacksquare)^{2T}, A_4 + A_6, H_4 + H_6, HA_2 + HA_6, K_3 + K_6, KA_1 + KA_6, 2L_2, M_1 + M_2]$ | (0, 2, 1)                                                      |
| $[(\blacksquare)^{2T}, A_4 + A_6, H_4 + H_6, 2HA_2, K_3 + K_6, KA_1 + KA_2, 2L_2, M_1 + M_2]$       | (0, 0, 1)                                                      |
| $[(\blacksquare)^{2T}, A_4 + A_6, 2H_4, HA_2 + HA_4, K_3 + K_4, KA_1 + KA_4, 2L_2, M_1 + M_2]$      | (0, 2, 1)                                                      |
| $[(\blacksquare)^{2T}, A_4 + A_6, 2H_4, HA_2 + HA_6, K_3 + K_4, KA_1 + KA_6, 2L_2, M_1 + M_2]$      | (0, 0, 1)                                                      |
| $[(\blacksquare)^{2T}, A_4 + A_6, 2H_4, 2HA_2, K_3 + K_4, KA_1 + KA_2, 2L_2, M_1 + M_2]$            | (0, 1, 1)                                                      |
| $[(\blacksquare)^{2T}, A_4 + A_6, H_2 + H_4, HA_2 + HA_4, K_2 + K_3, KA_1 + KA_4, 2L_2, M_1 + M_2]$ | (0, 0, 1)                                                      |
| $[(\blacksquare)^{2T}, A_4 + A_6, H_2 + H_4, HA_2 + HA_6, K_2 + K_3, KA_1 + KA_6, 2L_2, M_1 + M_2]$ | (0, 1, 1)                                                      |

... continued on next page





... continued from previous page

[illegible]

... continued on next page



... continued from previous page

[illegible]

... continued on next page

... continued on next page



... continued from previous page

|                                                                                                          |           |
|----------------------------------------------------------------------------------------------------------|-----------|
| $[(\blacksquare)^{2T}, A_3 + A_5, H_1 + H_5, 2HA_5, K_2 + K_5, KA_5 + KA_6, 2L_1, M_1 + M_2]$            | (2, 0, 2) |
| $[(\blacksquare)^{2T}, A_3 + A_5, H_1 + H_5, HA_1 + HA_5, K_2 + K_5, KA_2 + KA_5, 2L_1, M_1 + M_2]$      | trivial   |
| $[(\blacksquare)^{2T}, A_3 + A_5, H_1 + H_5, 2HA_5, K_1 + K_6, KA_5 + KA_6, 2L_1, M_1 + M_2]$            | (2, 0, 0) |
| $[(\blacksquare)^{2T}, A_3 + A_5, H_1 + H_5, HA_1 + HA_5, K_1 + K_6, KA_2 + KA_5, 2L_1, M_1 + M_2]$      | (0, 0, 1) |
| $[(\blacksquare)^{2T}, A_4 + A_5, H_5 + H_6, HA_1 + HA_4, K_5 + K_6, KA_1 + KA_4, L_1 + L_2, M_1 + M_2]$ | (2, 1, 1) |
| $[(\blacksquare)^{2T}, A_4 + A_5, H_5 + H_6, HA_1 + HA_6, K_5 + K_6, KA_1 + KA_6, L_1 + L_2, M_1 + M_2]$ | (2, 2, 1) |
| $[(\blacksquare)^{2T}, A_4 + A_5, H_5 + H_6, HA_1 + HA_2, K_5 + K_6, KA_1 + KA_2, L_1 + L_2, M_1 + M_2]$ | (2, 0, 1) |
| $[(\blacksquare)^{2T}, A_4 + A_5, H_4 + H_5, HA_1 + HA_4, K_4 + K_5, KA_1 + KA_4, L_1 + L_2, M_1 + M_2]$ | (2, 2, 1) |
| $[(\blacksquare)^{2T}, A_4 + A_5, H_4 + H_5, HA_1 + HA_6, K_4 + K_5, KA_1 + KA_6, L_1 + L_2, M_1 + M_2]$ | (2, 0, 1) |
| $[(\blacksquare)^{2T}, A_4 + A_5, H_4 + H_5, HA_1 + HA_2, K_4 + K_5, KA_1 + KA_2, L_1 + L_2, M_1 + M_2]$ | (2, 1, 1) |
| $[(\blacksquare)^{2T}, A_4 + A_5, H_2 + H_5, HA_1 + HA_4, K_2 + K_5, KA_1 + KA_4, L_1 + L_2, M_1 + M_2]$ | (2, 0, 1) |
| $[(\blacksquare)^{2T}, A_4 + A_5, H_2 + H_5, HA_1 + HA_6, K_2 + K_5, KA_1 + KA_6, L_1 + L_2, M_1 + M_2]$ | (2, 1, 1) |
| $[(\blacksquare)^{2T}, A_4 + A_5, H_2 + H_5, HA_1 + HA_2, K_2 + K_5, KA_1 + KA_2, L_1 + L_2, M_1 + M_2]$ | (2, 2, 1) |
| $[(\blacksquare)^{2T}, A_4 + A_5, H_4 + H_5, HA_1 + HA_4, K_3 + K_6, KA_1 + KA_4, L_1 + L_2, M_1 + M_2]$ | (2, 2, 0) |
| $[(\blacksquare)^{2T}, A_4 + A_5, H_4 + H_5, HA_1 + HA_6, K_3 + K_6, KA_1 + KA_6, L_1 + L_2, M_1 + M_2]$ | (2, 0, 0) |
| $[(\blacksquare)^{2T}, A_4 + A_5, H_4 + H_5, HA_1 + HA_2, K_3 + K_6, KA_1 + KA_2, L_1 + L_2, M_1 + M_2]$ | (2, 1, 0) |
| $[(\blacksquare)^{2T}, A_4 + A_5, H_2 + H_5, HA_1 + HA_4, K_1 + K_6, KA_1 + KA_4, L_1 + L_2, M_1 + M_2]$ | (2, 0, 2) |
| $[(\blacksquare)^{2T}, A_4 + A_5, H_2 + H_5, HA_1 + HA_6, K_1 + K_6, KA_1 + KA_6, L_1 + L_2, M_1 + M_2]$ | (2, 1, 2) |
| $[(\blacksquare)^{2T}, A_4 + A_5, H_2 + H_5, HA_1 + HA_2, K_1 + K_6, KA_1 + KA_2, L_1 + L_2, M_1 + M_2]$ | (2, 2, 2) |
| $[(\blacksquare)^{2T}, A_3 + A_5, 2H_5, HA_1 + HA_5, K_5 + K_6, KA_1 + KA_6, 2L_1, M_1 + M_2]$           | (1, 0, 0) |
| $[(\blacksquare)^{2T}, A_3 + A_5, 2H_5, 2HA_1, K_5 + K_6, KA_1 + KA_2, 2L_1, M_1 + M_2]$                 | (2, 0, 1) |
| $[(\blacksquare)^{2T}, A_3 + A_5, H_3 + H_5, HA_1 + HA_5, K_4 + K_5, KA_1 + KA_6, 2L_1, M_1 + M_2]$      | (2, 0, 1) |
| $[(\blacksquare)^{2T}, A_3 + A_5, H_3 + H_5, 2HA_1, K_4 + K_5, KA_1 + KA_2, 2L_1, M_1 + M_2]$            | (0, 0, 2) |
| $[(\blacksquare)^{2T}, A_3 + A_5, H_3 + H_5, HA_1 + HA_5, K_3 + K_6, KA_1 + KA_6, 2L_1, M_1 + M_2]$      | (2, 0, 0) |
| $[(\blacksquare)^{2T}, A_3 + A_5, H_3 + H_5, 2HA_1, K_3 + K_6, KA_1 + KA_2, 2L_1, M_1 + M_2]$            | (0, 0, 1) |
| $[(\blacksquare)^{2T}, A_3 + A_5, H_1 + H_5, HA_1 + HA_5, K_2 + K_5, KA_1 + KA_6, 2L_1, M_1 + M_2]$      | (0, 0, 2) |
| $[(\blacksquare)^{2T}, A_3 + A_5, H_1 + H_5, 2HA_1, K_2 + K_5, KA_1 + KA_2, 2L_1, M_1 + M_2]$            | (1, 0, 0) |
| $[(\blacksquare)^{2T}, A_3 + A_5, H_1 + H_5, HA_1 + HA_5, K_1 + K_6, KA_1 + KA_6, 2L_1, M_1 + M_2]$      | trivial   |
| $[(\blacksquare)^{2T}, A_3 + A_5, H_1 + H_5, 2HA_1, K_1 + K_6, KA_1 + KA_2, 2L_1, M_1 + M_2]$            | (1, 0, 1) |
| $[(\blacksquare)^{2T}, A_4 + A_5, H_3 + H_6, HA_3 + HA_4, K_3 + K_6, KA_3 + KA_4, L_1 + L_2, M_1 + M_2]$ | (1, 1, 1) |
| $[(\blacksquare)^{2T}, A_4 + A_5, H_3 + H_6, HA_3 + HA_6, K_3 + K_6, KA_3 + KA_6, L_1 + L_2, M_1 + M_2]$ | (1, 2, 1) |
| $[(\blacksquare)^{2T}, A_4 + A_5, H_3 + H_6, HA_2 + HA_3, K_3 + K_6, KA_2 + KA_3, L_1 + L_2, M_1 + M_2]$ | (1, 0, 1) |
| $[(\blacksquare)^{2T}, A_4 + A_5, H_3 + H_4, HA_3 + HA_4, K_3 + K_4, KA_3 + KA_4, L_1 + L_2, M_1 + M_2]$ | (1, 2, 1) |
| $[(\blacksquare)^{2T}, A_4 + A_5, H_3 + H_4, HA_3 + HA_6, K_3 + K_4, KA_3 + KA_6, L_1 + L_2, M_1 + M_2]$ | (1, 0, 1) |
| $[(\blacksquare)^{2T}, A_4 + A_5, H_3 + H_4, HA_2 + HA_3, K_3 + K_4, KA_2 + KA_3, L_1 + L_2, M_1 + M_2]$ | (1, 1, 1) |
| $[(\blacksquare)^{2T}, A_4 + A_5, H_2 + H_3, HA_3 + HA_4, K_2 + K_3, KA_3 + KA_4, L_1 + L_2, M_1 + M_2]$ | (1, 0, 1) |
| $[(\blacksquare)^{2T}, A_4 + A_5, H_2 + H_3, HA_3 + HA_6, K_2 + K_3, KA_3 + KA_6, L_1 + L_2, M_1 + M_2]$ | (1, 1, 1) |
| $[(\blacksquare)^{2T}, A_4 + A_5, H_2 + H_3, HA_2 + HA_3, K_2 + K_3, KA_2 + KA_3, L_1 + L_2, M_1 + M_2]$ | (1, 2, 1) |
| $[(\blacksquare)^{2T}, A_4 + A_5, H_3 + H_6, HA_3 + HA_6, K_3 + K_6, KA_4 + KA_5, L_1 + L_2, M_1 + M_2]$ | (1, 2, 0) |
| $[(\blacksquare)^{2T}, A_4 + A_5, H_3 + H_4, HA_3 + HA_6, K_3 + K_4, KA_4 + KA_5, L_1 + L_2, M_1 + M_2]$ | (1, 0, 0) |
| $[(\blacksquare)^{2T}, A_4 + A_5, H_2 + H_3, HA_3 + HA_6, K_2 + K_3, KA_4 + KA_5, L_1 + L_2, M_1 + M_2]$ | (1, 1, 0) |
| $[(\blacksquare)^{2T}, A_4 + A_5, H_3 + H_6, HA_2 + HA_3, K_3 + K_6, KA_1 + KA_4, L_1 + L_2, M_1 + M_2]$ | (1, 0, 2) |
| $[(\blacksquare)^{2T}, A_4 + A_5, H_3 + H_4, HA_2 + HA_3, K_3 + K_4, KA_1 + KA_4, L_1 + L_2, M_1 + M_2]$ | (1, 1, 2) |
| $[(\blacksquare)^{2T}, A_4 + A_5, H_2 + H_3, HA_2 + HA_3, K_2 + K_3, KA_1 + KA_4, L_1 + L_2, M_1 + M_2]$ | (1, 2, 2) |
| $[(\blacksquare)^{2T}, A_3 + A_5, 2H_3, 2HA_3, K_3 + K_4, KA_3 + KA_4, 2L_1, M_1 + M_2]$                 | trivial   |
| $[(\blacksquare)^{2T}, A_3 + A_5, 2H_3, HA_3 + HA_5, K_3 + K_4, KA_4 + KA_5, 2L_1, M_1 + M_2]$           | (1, 0, 0) |
| $[(\blacksquare)^{2T}, A_3 + A_5, 2H_3, HA_3 + HA_5, K_3 + K_4, KA_3 + KA_6, 2L_1, M_1 + M_2]$           | (1, 0, 1) |
| $[(\blacksquare)^{2T}, A_3 + A_5, 2H_3, HA_1 + HA_3, K_3 + K_4, KA_2 + KA_3, 2L_1, M_1 + M_2]$           | (2, 0, 2) |
| $[(\blacksquare)^{2T}, A_3 + A_5, 2H_3, HA_1 + HA_3, K_3 + K_4, KA_1 + KA_4, 2L_1, M_1 + M_2]$           | (2, 0, 0) |
| $[(\blacksquare)^{2T}, A_3 + A_5, H_1 + H_3, 2HA_3, K_2 + K_3, KA_3 + KA_4, 2L_1, M_1 + M_2]$            | (1, 0, 1) |
| $[(\blacksquare)^{2T}, A_3 + A_5, H_1 + H_3, HA_3 + HA_5, K_2 + K_3, KA_4 + KA_5, 2L_1, M_1 + M_2]$      | (2, 0, 1) |
| $[(\blacksquare)^{2T}, A_3 + A_5, H_1 + H_3, HA_3 + HA_5, K_2 + K_3, KA_3 + KA_6, 2L_1, M_1 + M_2]$      | (2, 0, 2) |
| $[(\blacksquare)^{2T}, A_3 + A_5, H_1 + H_3, HA_1 + HA_3, K_2 + K_3, KA_2 + KA_3, 2L_1, M_1 + M_2]$      | trivial   |
| $[(\blacksquare)^{2T}, A_3 + A_5, H_1 + H_3, HA_1 + HA_3, K_2 + K_3, KA_1 + KA_4, 2L_1, M_1 + M_2]$      | (0, 0, 1) |

... continued on next page

... continued on next page



... continued on next page

... continued from previous page

|                                                                                                          |           |
|----------------------------------------------------------------------------------------------------------|-----------|
| $[(\blacksquare)^{2T}, A_4 + A_5, H_1 + H_4, HA_4 + HA_5, K_2 + K_3, KA_3 + KA_6, L_1 + L_2, M_1 + M_2]$ | (0, 2, 0) |
| $[(\blacksquare)^{2T}, A_4 + A_5, H_1 + H_4, HA_5 + HA_6, K_2 + K_3, KA_5 + KA_6, L_1 + L_2, M_1 + M_2]$ | (0, 0, 2) |
| $[(\blacksquare)^{2T}, A_4 + A_5, H_1 + H_4, HA_2 + HA_3, K_2 + K_3, KA_2 + KA_3, L_1 + L_2, M_1 + M_2]$ | (2, 1, 2) |
| $[(\blacksquare)^{2T}, A_4 + A_5, H_1 + H_4, HA_2 + HA_5, K_2 + K_3, KA_2 + KA_5, L_1 + L_2, M_1 + M_2]$ | (0, 1, 2) |
| $[(\blacksquare)^{2T}, A_4 + A_5, H_1 + H_4, HA_2 + HA_3, K_2 + K_3, KA_1 + KA_4, L_1 + L_2, M_1 + M_2]$ | (2, 1, 0) |
| $[(\blacksquare)^{2T}, A_4 + A_5, H_1 + H_4, HA_2 + HA_5, K_2 + K_3, KA_1 + KA_6, L_1 + L_2, M_1 + M_2]$ | (0, 1, 1) |
| $[(\blacksquare)^{2T}, A_4 + A_5, H_1 + H_4, HA_1 + HA_4, K_2 + K_3, KA_2 + KA_3, L_1 + L_2, M_1 + M_2]$ | (1, 2, 1) |
| $[(\blacksquare)^{2T}, A_4 + A_5, H_1 + H_4, HA_1 + HA_6, K_2 + K_3, KA_2 + KA_5, L_1 + L_2, M_1 + M_2]$ | (1, 0, 0) |
| $[(\blacksquare)^{2T}, A_4 + A_5, H_1 + H_4, HA_1 + HA_4, K_2 + K_3, KA_1 + KA_4, L_1 + L_2, M_1 + M_2]$ | (1, 2, 2) |
| $[(\blacksquare)^{2T}, A_4 + A_5, H_1 + H_4, HA_1 + HA_6, K_2 + K_3, KA_1 + KA_6, L_1 + L_2, M_1 + M_2]$ | (1, 0, 2) |
| $[(\blacksquare)^{2T}, A_4 + A_5, H_1 + H_4, HA_1 + HA_2, K_2 + K_3, KA_1 + KA_2, L_1 + L_2, M_1 + M_2]$ | (1, 1, 2) |
| $[(\blacksquare)^{2T}, A_4 + A_5, H_1 + H_4, HA_4 + HA_5, K_1 + K_4, KA_3 + KA_6, L_1 + L_2, M_1 + M_2]$ | (0, 2, 2) |
| $[(\blacksquare)^{2T}, A_4 + A_5, H_1 + H_4, HA_2 + HA_5, K_1 + K_4, KA_1 + KA_6, L_1 + L_2, M_1 + M_2]$ | (0, 1, 0) |
| $[(\blacksquare)^{2T}, A_4 + A_5, H_1 + H_4, HA_1 + HA_4, K_1 + K_4, KA_2 + KA_3, L_1 + L_2, M_1 + M_2]$ | (1, 2, 0) |
| $[(\blacksquare)^{2T}, A_4 + A_5, H_1 + H_4, HA_1 + HA_6, K_1 + K_4, KA_2 + KA_5, L_1 + L_2, M_1 + M_2]$ | (1, 0, 2) |
| $[(\blacksquare)^{2T}, A_4 + A_5, H_1 + H_2, HA_4 + HA_5, K_1 + K_2, KA_3 + KA_6, L_1 + L_2, M_1 + M_2]$ | (0, 0, 2) |
| $[(\blacksquare)^{2T}, A_4 + A_5, H_1 + H_2, HA_2 + HA_5, K_1 + K_2, KA_1 + KA_6, L_1 + L_2, M_1 + M_2]$ | (0, 2, 0) |
| $[(\blacksquare)^{2T}, A_4 + A_5, H_1 + H_2, HA_1 + HA_4, K_1 + K_2, KA_2 + KA_3, L_1 + L_2, M_1 + M_2]$ | (1, 0, 0) |
| $[(\blacksquare)^{2T}, A_4 + A_5, H_1 + H_2, HA_1 + HA_6, K_1 + K_2, KA_2 + KA_5, L_1 + L_2, M_1 + M_2]$ | (1, 1, 2) |

2nd minimal solution:  $\mu_2^T = 3$  (40176 symmetry vectors)Space group 175 ( $\mathbb{Z}_6 \times \mathbb{Z}_6 \times \mathbb{Z}_6$ )1st minimal solution:  $\mu_1^T = 2$  (252 symmetry vectors)

| $\mathbf{n}^T$                                                                             | $\mathbf{v}^T \in \mathbb{Z}_6 \times \mathbb{Z}_6 \times \mathbb{Z}_6$ |
|--------------------------------------------------------------------------------------------|-------------------------------------------------------------------------|
| $[(\blacksquare)^{2T}, A_4^- + A_6^-, 2H_5, K_5 + K_6, 2L_1^+, M_1^+ + M_1^-]$             | (0, 4, 2)                                                               |
| $[(\blacksquare)^{2T}, A_4^- + A_6^-, 2H_5, K_5 + K_6, L_1^+ + L_2^-, M_1^- + M_2^-]$      | (0, 4, 5)                                                               |
| $[(\blacksquare)^{2T}, A_4^- + A_6^-, H_3 + H_5, K_3 + K_6, 2L_1^+, M_1^+ + M_1^-]$        | (0, 2, 2)                                                               |
| $[(\blacksquare)^{2T}, A_4^- + A_6^-, H_3 + H_5, K_3 + K_6, L_1^+ + L_2^-, M_1^- + M_2^-]$ | (0, 2, 5)                                                               |
| $[(\blacksquare)^{2T}, A_4^- + A_6^-, H_1 + H_5, K_1 + K_6, 2L_1^+, M_1^+ + M_1^-]$        | (0, 0, 2)                                                               |
| $[(\blacksquare)^{2T}, A_4^- + A_6^-, H_1 + H_5, K_1 + K_6, L_1^+ + L_2^-, M_1^- + M_2^-]$ | (0, 0, 5)                                                               |
| $[(\blacksquare)^{2T}, A_4^+ + A_6^-, H_4 + H_5, K_4 + K_5, L_1^+ + L_1^-, M_1^+ + M_1^-]$ | (3, 4, 1)                                                               |
| $[(\blacksquare)^{2T}, A_4^+ + A_6^-, H_4 + H_5, K_4 + K_5, L_1^+ + L_2^+, M_1^+ + M_2^+]$ | (3, 1, 4)                                                               |
| $[(\blacksquare)^{2T}, A_4^+ + A_6^-, H_5 + H_6, K_5 + K_6, L_1^+ + L_1^-, M_1^+ + M_1^-]$ | (5, 2, 1)                                                               |
| $[(\blacksquare)^{2T}, A_4^+ + A_6^-, H_5 + H_6, K_5 + K_6, L_1^+ + L_2^+, M_1^+ + M_2^+]$ | (5, 5, 4)                                                               |
| $[(\blacksquare)^{2T}, A_4^+ + A_6^-, H_2 + H_5, K_2 + K_5, L_1^+ + L_1^-, M_1^+ + M_1^-]$ | (1, 0, 1)                                                               |
| $[(\blacksquare)^{2T}, A_4^+ + A_6^-, H_2 + H_5, K_2 + K_5, L_1^+ + L_2^+, M_1^+ + M_2^+]$ | (1, 3, 4)                                                               |
| $[(\blacksquare)^{2T}, A_4^+ + A_6^-, H_4 + H_5, K_4 + K_5, L_1^+ + L_2^+, M_1^- + M_2^-]$ | (0, 4, 1)                                                               |
| $[(\blacksquare)^{2T}, A_4^+ + A_6^-, H_5 + H_6, K_5 + K_6, L_1^+ + L_2^+, M_1^- + M_2^-]$ | (2, 2, 1)                                                               |
| $[(\blacksquare)^{2T}, A_4^+ + A_6^-, H_2 + H_5, K_2 + K_5, L_1^+ + L_2^+, M_1^- + M_2^-]$ | (4, 0, 1)                                                               |
| $[(\blacksquare)^{2T}, A_4^+ + A_6^-, H_4 + H_5, K_3 + K_6, L_1^+ + L_1^-, M_1^+ + M_1^-]$ | (3, 2, 5)                                                               |
| $[(\blacksquare)^{2T}, A_4^+ + A_6^-, H_4 + H_5, K_3 + K_6, L_1^+ + L_2^+, M_1^+ + M_2^+]$ | (3, 5, 2)                                                               |
| $[(\blacksquare)^{2T}, A_4^+ + A_6^-, H_4 + H_5, K_3 + K_6, L_1^+ + L_2^+, M_1^- + M_2^-]$ | (0, 2, 5)                                                               |
| $[(\blacksquare)^{2T}, A_4^+ + A_6^-, H_2 + H_5, K_1 + K_6, L_1^+ + L_1^-, M_1^+ + M_1^-]$ | (1, 2, 3)                                                               |
| $[(\blacksquare)^{2T}, A_4^+ + A_6^-, H_2 + H_5, K_1 + K_6, L_1^+ + L_2^+, M_1^+ + M_2^+]$ | (1, 5, 0)                                                               |
| $[(\blacksquare)^{2T}, A_4^+ + A_6^-, H_2 + H_5, K_1 + K_6, L_1^+ + L_2^+, M_1^- + M_2^-]$ | (4, 2, 3)                                                               |
| $[(\blacksquare)^{2T}, A_4^- + A_6^-, H_3 + H_5, K_4 + K_5, 2L_1^+, M_1^+ + M_1^-]$        | (0, 4, 4)                                                               |
| $[(\blacksquare)^{2T}, A_4^- + A_6^-, H_3 + H_5, K_4 + K_5, L_1^+ + L_2^-, M_1^+ + M_2^+]$ | (3, 1, 4)                                                               |
| $[(\blacksquare)^{2T}, A_4^- + A_6^-, H_3 + H_5, K_4 + K_5, L_1^+ + L_2^-, M_1^- + M_2^-]$ | (0, 4, 1)                                                               |

... continued on next page

... continued from previous page

|                                                                                       |           |
|---------------------------------------------------------------------------------------|-----------|
| $[(\bullet)^{2T}, A_4^- + A_6^-, 2H_5, K_5 + K_6, L_1^+ + L_2^-, M_1^+ + M_2^+]$      | (3, 1, 2) |
| $[(\bullet)^{2T}, A_4^- + A_6^-, H_3 + H_5, K_3 + K_6, L_1^+ + L_2^-, M_1^+ + M_2^+]$ | (3, 5, 2) |
| $[(\bullet)^{2T}, A_4^- + A_6^-, H_1 + H_5, K_2 + K_5, 2L_1^+, M_1^+ + M_1^-]$        | (0, 4, 0) |
| $[(\bullet)^{2T}, A_4^- + A_6^-, H_1 + H_5, K_2 + K_5, L_1^+ + L_2^-, M_1^+ + M_2^+]$ | (3, 1, 0) |
| $[(\bullet)^{2T}, A_4^- + A_6^-, H_1 + H_5, K_2 + K_5, L_1^+ + L_2^-, M_1^- + M_2^-]$ | (0, 4, 3) |
| $[(\bullet)^{2T}, A_4^- + A_6^-, H_1 + H_5, K_1 + K_6, L_1^+ + L_2^-, M_1^+ + M_2^+]$ | (3, 3, 2) |
| $[(\bullet)^{2T}, A_4^+ + A_6^-, H_4 + H_5, K_4 + K_5, L_1^- + L_2^-, M_1^- + M_2^-]$ | (3, 4, 4) |
| $[(\bullet)^{2T}, A_4^+ + A_6^-, H_4 + H_5, K_4 + K_5, L_2^+ + L_2^-, M_2^+ + M_2^-]$ | (3, 1, 1) |
| $[(\bullet)^{2T}, A_4^+ + A_6^-, H_5 + H_6, K_5 + K_6, L_1^- + L_2^-, M_1^- + M_2^-]$ | (5, 2, 4) |
| $[(\bullet)^{2T}, A_4^+ + A_6^-, H_5 + H_6, K_5 + K_6, L_2^+ + L_2^-, M_2^+ + M_2^-]$ | (5, 5, 1) |
| $[(\bullet)^{2T}, A_4^+ + A_6^-, H_2 + H_5, K_2 + K_5, L_1^- + L_2^-, M_1^- + M_2^-]$ | (1, 0, 4) |
| $[(\bullet)^{2T}, A_4^+ + A_6^-, H_2 + H_5, K_2 + K_5, L_2^+ + L_2^-, M_2^+ + M_2^-]$ | (1, 3, 1) |
| $[(\bullet)^{2T}, A_4^+ + A_6^-, H_4 + H_5, K_3 + K_6, L_1^- + L_2^-, M_1^- + M_2^-]$ | (3, 2, 2) |
| $[(\bullet)^{2T}, A_4^+ + A_6^-, H_4 + H_5, K_3 + K_6, L_2^+ + L_2^-, M_2^+ + M_2^-]$ | (3, 5, 5) |
| $[(\bullet)^{2T}, A_4^+ + A_6^-, H_2 + H_5, K_1 + K_6, L_1^- + L_2^-, M_1^- + M_2^-]$ | (1, 2, 0) |
| $[(\bullet)^{2T}, A_4^+ + A_6^-, H_2 + H_5, K_1 + K_6, L_2^+ + L_2^-, M_2^+ + M_2^-]$ | (1, 5, 3) |
| $[(\bullet)^{2T}, A_4^- + A_6^-, H_3 + H_5, K_4 + K_5, 2L_2^-, M_2^+ + M_2^-]$        | (3, 1, 1) |
| $[(\bullet)^{2T}, A_4^- + A_6^-, 2H_5, K_5 + K_6, 2L_2^-, M_2^+ + M_2^-]$             | (3, 1, 5) |
| $[(\bullet)^{2T}, A_4^- + A_6^-, H_3 + H_5, K_3 + K_6, 2L_2^-, M_2^+ + M_2^-]$        | (3, 5, 5) |
| $[(\bullet)^{2T}, A_4^- + A_6^-, H_1 + H_5, K_2 + K_5, 2L_2^-, M_2^+ + M_2^-]$        | (3, 1, 3) |
| $[(\bullet)^{2T}, A_4^- + A_6^-, H_1 + H_5, K_1 + K_6, 2L_2^-, M_2^+ + M_2^-]$        | (3, 3, 5) |
| $[(\bullet)^{2T}, A_4^+ + A_6^-, H_3 + H_4, K_3 + K_4, L_1^+ + L_1^-, M_1^+ + M_1^-]$ | (3, 2, 1) |
| $[(\bullet)^{2T}, A_4^+ + A_6^-, H_3 + H_4, K_3 + K_4, L_1^+ + L_2^+, M_1^+ + M_2^+]$ | (3, 5, 4) |
| $[(\bullet)^{2T}, A_4^+ + A_6^-, H_3 + H_6, K_3 + K_6, L_1^+ + L_1^-, M_1^+ + M_1^-]$ | (5, 0, 1) |
| $[(\bullet)^{2T}, A_4^+ + A_6^-, H_3 + H_6, K_3 + K_6, L_1^+ + L_2^+, M_1^+ + M_2^+]$ | (5, 3, 4) |
| $[(\bullet)^{2T}, A_4^+ + A_6^-, H_2 + H_3, K_2 + K_3, L_1^+ + L_1^-, M_1^+ + M_1^-]$ | (1, 4, 1) |
| $[(\bullet)^{2T}, A_4^+ + A_6^-, H_2 + H_3, K_2 + K_3, L_1^+ + L_2^+, M_1^+ + M_2^+]$ | (1, 1, 4) |
| $[(\bullet)^{2T}, A_4^+ + A_6^-, H_3 + H_4, K_3 + K_4, L_1^+ + L_2^+, M_1^- + M_2^-]$ | (0, 2, 1) |
| $[(\bullet)^{2T}, A_4^+ + A_6^-, H_3 + H_6, K_3 + K_6, L_1^+ + L_2^+, M_1^- + M_2^-]$ | (2, 0, 1) |
| $[(\bullet)^{2T}, A_4^+ + A_6^-, H_2 + H_3, K_2 + K_3, L_1^+ + L_2^+, M_1^- + M_2^-]$ | (4, 4, 1) |
| $[(\bullet)^{2T}, A_4^- + A_6^-, 2H_3, K_3 + K_4, 2L_1^+, M_1^+ + M_1^-]$             | (0, 2, 4) |
| $[(\bullet)^{2T}, A_4^- + A_6^-, 2H_3, K_3 + K_4, L_1^+ + L_2^-, M_1^+ + M_2^+]$      | (3, 5, 4) |
| $[(\bullet)^{2T}, A_4^- + A_6^-, 2H_3, K_3 + K_4, L_1^+ + L_2^-, M_1^- + M_2^-]$      | (0, 2, 1) |
| $[(\bullet)^{2T}, A_4^- + A_6^-, H_1 + H_3, K_2 + K_3, 2L_1^+, M_1^+ + M_1^-]$        | (0, 2, 0) |
| $[(\bullet)^{2T}, A_4^- + A_6^-, H_1 + H_3, K_2 + K_3, L_1^+ + L_2^-, M_1^+ + M_2^+]$ | (3, 5, 0) |
| $[(\bullet)^{2T}, A_4^- + A_6^-, H_1 + H_3, K_2 + K_3, L_1^+ + L_2^-, M_1^- + M_2^-]$ | (0, 2, 3) |
| $[(\bullet)^{2T}, A_4^+ + A_6^-, H_3 + H_4, K_3 + K_4, L_1^- + L_2^-, M_1^- + M_2^-]$ | (3, 2, 4) |
| $[(\bullet)^{2T}, A_4^+ + A_6^-, H_3 + H_4, K_3 + K_4, L_2^+ + L_2^-, M_2^+ + M_2^-]$ | (3, 5, 1) |
| $[(\bullet)^{2T}, A_4^+ + A_6^-, H_3 + H_6, K_3 + K_6, L_1^- + L_2^-, M_1^- + M_2^-]$ | (5, 0, 4) |
| $[(\bullet)^{2T}, A_4^+ + A_6^-, H_3 + H_6, K_3 + K_6, L_2^+ + L_2^-, M_2^+ + M_2^-]$ | (5, 3, 1) |
| $[(\bullet)^{2T}, A_4^+ + A_6^-, H_2 + H_3, K_2 + K_3, L_1^- + L_2^-, M_1^- + M_2^-]$ | (1, 4, 4) |
| $[(\bullet)^{2T}, A_4^+ + A_6^-, H_2 + H_3, K_2 + K_3, L_2^+ + L_2^-, M_2^+ + M_2^-]$ | (1, 1, 1) |
| $[(\bullet)^{2T}, A_4^- + A_6^-, 2H_3, K_3 + K_4, 2L_2^-, M_2^+ + M_2^-]$             | (3, 5, 1) |
| $[(\bullet)^{2T}, A_4^- + A_6^-, H_1 + H_3, K_2 + K_3, 2L_2^-, M_2^+ + M_2^-]$        | (3, 5, 3) |
| $[(\bullet)^{2T}, A_4^+ + A_6^-, H_1 + H_4, K_1 + K_4, L_1^+ + L_1^-, M_1^+ + M_1^-]$ | (3, 0, 1) |
| $[(\bullet)^{2T}, A_4^+ + A_6^-, H_1 + H_4, K_1 + K_4, L_1^+ + L_2^+, M_1^+ + M_2^+]$ | (3, 3, 4) |
| $[(\bullet)^{2T}, A_4^+ + A_6^-, H_1 + H_6, K_1 + K_6, L_1^+ + L_1^-, M_1^+ + M_1^-]$ | (5, 4, 1) |
| $[(\bullet)^{2T}, A_4^+ + A_6^-, H_1 + H_6, K_1 + K_6, L_1^+ + L_2^+, M_1^+ + M_2^+]$ | (5, 1, 4) |
| $[(\bullet)^{2T}, A_4^+ + A_6^-, H_1 + H_2, K_1 + K_2, L_1^+ + L_1^-, M_1^+ + M_1^-]$ | (1, 2, 1) |
| $[(\bullet)^{2T}, A_4^+ + A_6^-, H_1 + H_2, K_1 + K_2, L_1^+ + L_2^+, M_1^+ + M_2^+]$ | (1, 5, 4) |
| $[(\bullet)^{2T}, A_4^+ + A_6^-, H_1 + H_4, K_1 + K_4, L_1^+ + L_2^+, M_1^- + M_2^-]$ | (0, 0, 1) |
| $[(\bullet)^{2T}, A_4^+ + A_6^-, H_1 + H_6, K_1 + K_6, L_1^+ + L_2^+, M_1^- + M_2^-]$ | (2, 4, 1) |
| $[(\bullet)^{2T}, A_4^+ + A_6^-, H_1 + H_2, K_1 + K_2, L_1^+ + L_2^+, M_1^- + M_2^-]$ | (4, 2, 1) |
| $[(\bullet)^{2T}, A_4^- + A_6^-, H_1 + H_3, K_1 + K_4, 2L_1^+, M_1^+ + M_1^-]$        | (0, 0, 4) |

... continued on next page

... continued from previous page

|                                                                                       |           |
|---------------------------------------------------------------------------------------|-----------|
| $[(\bullet)^{2T}, A_4^- + A_6^-, H_1 + H_3, K_1 + K_4, L_1^+ + L_2^-, M_1^+ + M_2^+]$ | (3, 3, 4) |
| $[(\bullet)^{2T}, A_4^- + A_6^-, H_1 + H_3, K_1 + K_4, L_1^+ + L_2^-, M_1^- + M_2^-]$ | (0, 0, 1) |
| $[(\bullet)^{2T}, A_4^- + A_6^-, 2H_1, K_1 + K_2, 2L_1^+, M_1^+ + M_1^-]$             | trivial   |
| $[(\bullet)^{2T}, A_4^- + A_6^-, 2H_1, K_1 + K_2, L_1^+ + L_2^-, M_1^+ + M_2^+]$      | (3, 3, 0) |
| $[(\bullet)^{2T}, A_4^- + A_6^-, 2H_1, K_1 + K_2, L_1^+ + L_2^-, M_1^- + M_2^-]$      | (0, 0, 3) |
| $[(\bullet)^{2T}, A_4^+ + A_6^-, H_1 + H_4, K_1 + K_4, L_1^- + L_2^-, M_1^- + M_2^-]$ | (3, 0, 4) |
| $[(\bullet)^{2T}, A_4^+ + A_6^-, H_1 + H_4, K_1 + K_4, L_2^+ + L_2^-, M_2^+ + M_2^-]$ | (3, 3, 1) |
| $[(\bullet)^{2T}, A_4^+ + A_6^-, H_1 + H_6, K_1 + K_6, L_1^- + L_2^-, M_1^- + M_2^-]$ | (5, 4, 4) |
| $[(\bullet)^{2T}, A_4^+ + A_6^-, H_1 + H_6, K_1 + K_6, L_2^+ + L_2^-, M_2^+ + M_2^-]$ | (5, 1, 1) |
| $[(\bullet)^{2T}, A_4^+ + A_6^-, H_1 + H_2, K_1 + K_2, L_1^- + L_2^-, M_1^- + M_2^-]$ | (1, 2, 4) |
| $[(\bullet)^{2T}, A_4^+ + A_6^-, H_1 + H_2, K_1 + K_2, L_2^+ + L_2^-, M_2^+ + M_2^-]$ | (1, 5, 1) |
| $[(\bullet)^{2T}, A_4^- + A_6^-, H_1 + H_3, K_1 + K_4, 2L_2^-, M_2^+ + M_2^-]$        | (3, 3, 1) |
| $[(\bullet)^{2T}, A_4^- + A_6^-, 2H_1, K_1 + K_2, 2L_2^-, M_2^+ + M_2^-]$             | (3, 3, 3) |
| $[(\bullet)^{2T}, A_4^- + A_6^+, H_4 + H_5, K_4 + K_5, L_1^+ + L_1^-, M_1^+ + M_1^-]$ | (1, 0, 5) |
| $[(\bullet)^{2T}, A_4^- + A_6^+, H_4 + H_5, K_4 + K_5, L_1^+ + L_2^+, M_1^+ + M_2^+]$ | (1, 3, 2) |
| $[(\bullet)^{2T}, A_4^- + A_6^+, H_5 + H_6, K_5 + K_6, L_1^+ + L_1^-, M_1^+ + M_1^-]$ | (3, 4, 5) |
| $[(\bullet)^{2T}, A_4^- + A_6^+, H_5 + H_6, K_5 + K_6, L_1^+ + L_2^+, M_1^+ + M_2^+]$ | (3, 1, 2) |
| $[(\bullet)^{2T}, A_4^- + A_6^+, H_2 + H_5, K_2 + K_5, L_1^+ + L_1^-, M_1^+ + M_1^-]$ | (5, 2, 5) |
| $[(\bullet)^{2T}, A_4^- + A_6^+, H_2 + H_5, K_2 + K_5, L_1^+ + L_2^+, M_1^+ + M_2^+]$ | (5, 5, 2) |
| $[(\bullet)^{2T}, A_4^- + A_6^+, H_4 + H_5, K_4 + K_5, L_1^- + L_2^-, M_1^- + M_2^-]$ | (1, 0, 2) |
| $[(\bullet)^{2T}, A_4^- + A_6^+, H_4 + H_5, K_4 + K_5, L_2^+ + L_2^-, M_2^+ + M_2^-]$ | (1, 3, 5) |
| $[(\bullet)^{2T}, A_4^- + A_6^+, H_5 + H_6, K_5 + K_6, L_1^- + L_2^-, M_1^- + M_2^-]$ | (3, 4, 2) |
| $[(\bullet)^{2T}, A_4^- + A_6^+, H_5 + H_6, K_5 + K_6, L_2^+ + L_2^-, M_2^+ + M_2^-]$ | (3, 1, 5) |
| $[(\bullet)^{2T}, A_4^- + A_6^+, H_2 + H_5, K_2 + K_5, L_1^- + L_2^-, M_1^- + M_2^-]$ | (5, 2, 2) |
| $[(\bullet)^{2T}, A_4^- + A_6^+, H_2 + H_5, K_2 + K_5, L_2^+ + L_2^-, M_2^+ + M_2^-]$ | (5, 5, 5) |
| $[(\bullet)^{2T}, A_4^- + A_6^+, H_3 + H_4, K_3 + K_4, L_1^+ + L_1^-, M_1^+ + M_1^-]$ | (1, 4, 5) |
| $[(\bullet)^{2T}, A_4^- + A_6^+, H_3 + H_4, K_3 + K_4, L_1^+ + L_2^+, M_1^+ + M_2^+]$ | (1, 1, 2) |
| $[(\bullet)^{2T}, A_4^- + A_6^+, H_3 + H_6, K_3 + K_6, L_1^+ + L_1^-, M_1^+ + M_1^-]$ | (3, 2, 5) |
| $[(\bullet)^{2T}, A_4^- + A_6^+, H_3 + H_6, K_3 + K_6, L_1^+ + L_2^+, M_1^+ + M_2^+]$ | (3, 5, 2) |
| $[(\bullet)^{2T}, A_4^- + A_6^+, H_2 + H_3, K_2 + K_3, L_1^+ + L_1^-, M_1^+ + M_1^-]$ | (5, 0, 5) |
| $[(\bullet)^{2T}, A_4^- + A_6^+, H_2 + H_3, K_2 + K_3, L_1^+ + L_2^+, M_1^+ + M_2^+]$ | (5, 3, 2) |
| $[(\bullet)^{2T}, A_4^- + A_6^+, H_3 + H_4, K_3 + K_4, L_1^- + L_2^-, M_1^- + M_2^-]$ | (1, 4, 2) |
| $[(\bullet)^{2T}, A_4^- + A_6^+, H_3 + H_4, K_3 + K_4, L_2^+ + L_2^-, M_2^+ + M_2^-]$ | (1, 1, 5) |
| $[(\bullet)^{2T}, A_4^- + A_6^+, H_3 + H_6, K_3 + K_6, L_1^- + L_2^-, M_1^- + M_2^-]$ | (3, 2, 2) |
| $[(\bullet)^{2T}, A_4^- + A_6^+, H_3 + H_6, K_3 + K_6, L_2^+ + L_2^-, M_2^+ + M_2^-]$ | (3, 5, 5) |
| $[(\bullet)^{2T}, A_4^- + A_6^+, H_2 + H_3, K_2 + K_3, L_1^- + L_2^-, M_1^- + M_2^-]$ | (5, 0, 2) |
| $[(\bullet)^{2T}, A_4^- + A_6^+, H_2 + H_3, K_2 + K_3, L_2^+ + L_2^-, M_2^+ + M_2^-]$ | (5, 3, 5) |
| $[(\bullet)^{2T}, A_4^- + A_6^+, H_1 + H_4, K_1 + K_4, L_1^+ + L_1^-, M_1^+ + M_1^-]$ | (1, 2, 5) |
| $[(\bullet)^{2T}, A_4^- + A_6^+, H_1 + H_4, K_1 + K_4, L_1^+ + L_2^+, M_1^+ + M_2^+]$ | (1, 5, 2) |
| $[(\bullet)^{2T}, A_4^- + A_6^+, H_1 + H_6, K_1 + K_6, L_1^+ + L_1^-, M_1^+ + M_1^-]$ | (3, 0, 5) |
| $[(\bullet)^{2T}, A_4^- + A_6^+, H_1 + H_6, K_1 + K_6, L_1^+ + L_2^+, M_1^+ + M_2^+]$ | (3, 3, 2) |
| $[(\bullet)^{2T}, A_4^- + A_6^+, H_1 + H_2, K_1 + K_2, L_1^+ + L_1^-, M_1^+ + M_1^-]$ | (5, 4, 5) |
| $[(\bullet)^{2T}, A_4^- + A_6^+, H_1 + H_2, K_1 + K_2, L_1^+ + L_2^+, M_1^+ + M_2^+]$ | (5, 1, 2) |
| $[(\bullet)^{2T}, A_4^- + A_6^+, H_1 + H_4, K_1 + K_4, L_1^- + L_2^-, M_1^- + M_2^-]$ | (1, 2, 2) |
| $[(\bullet)^{2T}, A_4^- + A_6^+, H_1 + H_4, K_1 + K_4, L_2^+ + L_2^-, M_2^+ + M_2^-]$ | (1, 5, 5) |
| $[(\bullet)^{2T}, A_4^- + A_6^+, H_1 + H_6, K_1 + K_6, L_1^- + L_2^-, M_1^- + M_2^-]$ | (3, 0, 2) |
| $[(\bullet)^{2T}, A_4^- + A_6^+, H_1 + H_6, K_1 + K_6, L_2^+ + L_2^-, M_2^+ + M_2^-]$ | (3, 3, 5) |
| $[(\bullet)^{2T}, A_4^- + A_6^+, H_1 + H_2, K_1 + K_2, L_1^- + L_2^-, M_1^- + M_2^-]$ | (5, 4, 2) |
| $[(\bullet)^{2T}, A_4^- + A_6^+, H_1 + H_2, K_1 + K_2, L_2^+ + L_2^-, M_2^+ + M_2^-]$ | (5, 1, 5) |
| $[(\bullet)^{2T}, A_4^+ + A_6^+, H_4 + H_6, K_4 + K_5, 2L_1^-, M_1^+ + M_1^-]$        | (0, 4, 4) |
| $[(\bullet)^{2T}, A_4^+ + A_6^+, H_4 + H_6, K_4 + K_5, L_1^- + L_2^+, M_1^- + M_2^+]$ | (0, 1, 1) |
| $[(\bullet)^{2T}, A_4^+ + A_6^+, 2H_6, K_5 + K_6, 2L_1^-, M_1^+ + M_1^-]$             | (2, 2, 4) |
| $[(\bullet)^{2T}, A_4^+ + A_6^+, 2H_6, K_5 + K_6, L_1^- + L_2^+, M_1^- + M_2^+]$      | (2, 5, 1) |
| $[(\bullet)^{2T}, A_4^+ + A_6^+, H_2 + H_6, K_2 + K_5, 2L_1^-, M_1^+ + M_1^-]$        | (4, 0, 4) |

... continued on next page

... continued from previous page

|                                                                                       |           |
|---------------------------------------------------------------------------------------|-----------|
| $[(\bullet)^{2T}, A_4^+ + A_6^+, H_2 + H_6, K_2 + K_5, L_1^- + L_2^+, M_1^+ + M_2^+]$ | (4, 3, 1) |
| $[(\bullet)^{2T}, A_4^+ + A_6^+, H_4 + H_6, K_4 + K_5, L_1^- + L_2^+, M_1^- + M_2^-]$ | (3, 4, 4) |
| $[(\bullet)^{2T}, A_4^+ + A_6^+, H_4 + H_6, K_4 + K_5, 2L_2^+, M_2^+ + M_2^-]$        | (3, 1, 1) |
| $[(\bullet)^{2T}, A_4^+ + A_6^+, 2H_6, K_5 + K_6, L_1^- + L_2^+, M_1^- + M_2^-]$      | (5, 2, 4) |
| $[(\bullet)^{2T}, A_4^+ + A_6^+, 2H_6, K_5 + K_6, 2L_2^+, M_2^+ + M_2^-]$             | (5, 5, 1) |
| $[(\bullet)^{2T}, A_4^+ + A_6^+, H_2 + H_6, K_2 + K_5, L_1^- + L_2^+, M_1^- + M_2^-]$ | (1, 0, 4) |
| $[(\bullet)^{2T}, A_4^+ + A_6^+, H_2 + H_6, K_2 + K_5, 2L_2^+, M_2^+ + M_2^-]$        | (1, 3, 1) |
| $[(\bullet)^{2T}, A_4^+ + A_6^+, 2H_4, K_3 + K_4, 2L_1^-, M_1^+ + M_1^-]$             | (4, 4, 2) |
| $[(\bullet)^{2T}, A_4^+ + A_6^+, 2H_4, K_3 + K_4, L_1^- + L_2^+, M_1^+ + M_2^+]$      | (4, 1, 5) |
| $[(\bullet)^{2T}, A_4^+ + A_6^+, H_4 + H_6, K_3 + K_6, 2L_1^-, M_1^+ + M_1^-]$        | (0, 2, 2) |
| $[(\bullet)^{2T}, A_4^+ + A_6^+, H_4 + H_6, K_3 + K_6, L_1^- + L_2^+, M_1^+ + M_2^+]$ | (0, 5, 5) |
| $[(\bullet)^{2T}, A_4^+ + A_6^+, H_2 + H_4, K_2 + K_3, 2L_1^-, M_1^+ + M_1^-]$        | (2, 0, 2) |
| $[(\bullet)^{2T}, A_4^+ + A_6^+, H_2 + H_4, K_2 + K_3, L_1^- + L_2^+, M_1^+ + M_2^+]$ | (2, 3, 5) |
| $[(\bullet)^{2T}, A_4^+ + A_6^+, 2H_4, K_3 + K_4, L_1^- + L_2^+, M_1^- + M_2^-]$      | (1, 4, 2) |
| $[(\bullet)^{2T}, A_4^+ + A_6^+, 2H_4, K_3 + K_4, 2L_2^+, M_2^+ + M_2^-]$             | (1, 1, 5) |
| $[(\bullet)^{2T}, A_4^+ + A_6^+, H_4 + H_6, K_3 + K_6, L_1^- + L_2^+, M_1^- + M_2^-]$ | (3, 2, 2) |
| $[(\bullet)^{2T}, A_4^+ + A_6^+, H_4 + H_6, K_3 + K_6, 2L_2^+, M_2^+ + M_2^-]$        | (3, 5, 5) |
| $[(\bullet)^{2T}, A_4^+ + A_6^+, H_2 + H_4, K_2 + K_3, L_1^- + L_2^+, M_1^- + M_2^-]$ | (5, 0, 2) |
| $[(\bullet)^{2T}, A_4^+ + A_6^+, H_2 + H_4, K_2 + K_3, 2L_2^+, M_2^+ + M_2^-]$        | (5, 3, 5) |
| $[(\bullet)^{2T}, A_4^+ + A_6^+, H_2 + H_4, K_1 + K_4, 2L_1^-, M_1^+ + M_1^-]$        | (2, 4, 0) |
| $[(\bullet)^{2T}, A_4^+ + A_6^+, H_2 + H_4, K_1 + K_4, L_1^- + L_2^+, M_1^+ + M_2^+]$ | (2, 1, 3) |
| $[(\bullet)^{2T}, A_4^+ + A_6^+, H_2 + H_6, K_1 + K_6, 2L_1^-, M_1^+ + M_1^-]$        | (4, 2, 0) |
| $[(\bullet)^{2T}, A_4^+ + A_6^+, H_2 + H_6, K_1 + K_6, L_1^- + L_2^+, M_1^+ + M_2^+]$ | (4, 5, 3) |
| $[(\bullet)^{2T}, A_4^+ + A_6^+, 2H_2, K_1 + K_2, 2L_1^-, M_1^+ + M_1^-]$             | trivial   |
| $[(\bullet)^{2T}, A_4^+ + A_6^+, 2H_2, K_1 + K_2, L_1^- + L_2^+, M_1^+ + M_2^+]$      | (0, 3, 3) |
| $[(\bullet)^{2T}, A_4^+ + A_6^+, H_2 + H_4, K_1 + K_4, L_1^- + L_2^+, M_1^- + M_2^-]$ | (5, 4, 0) |
| $[(\bullet)^{2T}, A_4^+ + A_6^+, H_2 + H_4, K_1 + K_4, 2L_2^+, M_2^+ + M_2^-]$        | (5, 1, 3) |
| $[(\bullet)^{2T}, A_4^+ + A_6^+, H_2 + H_6, K_1 + K_6, L_1^- + L_2^+, M_1^- + M_2^-]$ | (1, 2, 0) |
| $[(\bullet)^{2T}, A_4^+ + A_6^+, H_2 + H_6, K_1 + K_6, 2L_2^+, M_2^+ + M_2^-]$        | (1, 5, 3) |
| $[(\bullet)^{2T}, A_4^+ + A_6^+, 2H_2, K_1 + K_2, L_1^- + L_2^+, M_1^- + M_2^-]$      | (3, 0, 0) |
| $[(\bullet)^{2T}, A_4^+ + A_6^+, 2H_2, K_1 + K_2, 2L_2^+, M_2^+ + M_2^-]$             | (3, 3, 3) |
| $[(\bullet)^{2T}, A_4^- + A_6^+, H_4 + H_5, K_4 + K_5, L_1^+ + L_2^+, M_1^- + M_2^-]$ | (4, 0, 5) |
| $[(\bullet)^{2T}, A_4^- + A_6^+, H_4 + H_5, K_4 + K_5, L_1^- + L_2^-, M_1^+ + M_2^+]$ | (4, 3, 5) |
| $[(\bullet)^{2T}, A_4^- + A_6^+, H_3 + H_6, K_4 + K_5, L_1^+ + L_1^-, M_1^+ + M_1^-]$ | (3, 4, 1) |
| $[(\bullet)^{2T}, A_4^- + A_6^+, H_3 + H_6, K_4 + K_5, L_1^+ + L_2^+, M_1^+ + M_2^+]$ | (3, 1, 4) |
| $[(\bullet)^{2T}, A_4^- + A_6^+, H_3 + H_6, K_4 + K_5, L_1^+ + L_2^-, M_1^- + M_2^-]$ | (0, 4, 1) |
| $[(\bullet)^{2T}, A_4^- + A_6^+, H_3 + H_6, K_4 + K_5, L_1^- + L_2^-, M_1^+ + M_2^+]$ | (0, 1, 1) |
| $[(\bullet)^{2T}, A_4^- + A_6^+, H_3 + H_6, K_4 + K_5, L_1^- + L_2^-, M_1^- + M_2^-]$ | (3, 4, 4) |
| $[(\bullet)^{2T}, A_4^- + A_6^+, H_3 + H_6, K_4 + K_5, L_2^+ + L_2^-, M_2^+ + M_2^-]$ | (3, 1, 1) |
| $[(\bullet)^{2T}, A_4^- + A_6^+, H_5 + H_6, K_5 + K_6, L_1^+ + L_2^+, M_1^- + M_2^-]$ | (0, 4, 5) |
| $[(\bullet)^{2T}, A_4^- + A_6^+, H_3 + H_4, K_3 + K_4, L_1^+ + L_2^+, M_1^- + M_2^-]$ | (4, 4, 5) |
| $[(\bullet)^{2T}, A_4^- + A_6^+, H_5 + H_6, K_5 + K_6, L_1^- + L_2^-, M_1^+ + M_2^+]$ | (0, 1, 5) |
| $[(\bullet)^{2T}, A_4^- + A_6^+, H_3 + H_4, K_3 + K_4, L_1^- + L_2^-, M_1^+ + M_2^+]$ | (4, 1, 5) |
| $[(\bullet)^{2T}, A_4^- + A_6^+, H_4 + H_5, K_3 + K_6, L_1^+ + L_1^-, M_1^+ + M_1^-]$ | (1, 4, 3) |
| $[(\bullet)^{2T}, A_4^- + A_6^+, H_4 + H_5, K_3 + K_6, L_1^+ + L_2^+, M_1^+ + M_2^+]$ | (1, 1, 0) |
| $[(\bullet)^{2T}, A_4^- + A_6^+, H_4 + H_5, K_3 + K_6, L_1^+ + L_2^-, M_1^- + M_2^-]$ | (4, 4, 3) |
| $[(\bullet)^{2T}, A_4^- + A_6^+, H_4 + H_5, K_3 + K_6, L_1^- + L_2^-, M_1^+ + M_2^+]$ | (4, 1, 3) |
| $[(\bullet)^{2T}, A_4^- + A_6^+, H_4 + H_5, K_3 + K_6, L_1^- + L_2^-, M_1^- + M_2^-]$ | (1, 4, 0) |
| $[(\bullet)^{2T}, A_4^- + A_6^+, H_4 + H_5, K_3 + K_6, L_2^+ + L_2^-, M_2^+ + M_2^-]$ | (1, 1, 3) |
| $[(\bullet)^{2T}, A_4^- + A_6^+, H_3 + H_6, K_3 + K_6, L_1^+ + L_2^+, M_1^- + M_2^-]$ | (0, 2, 5) |
| $[(\bullet)^{2T}, A_4^- + A_6^+, H_3 + H_6, K_3 + K_6, L_1^- + L_2^-, M_1^+ + M_2^+]$ | (0, 5, 5) |
| $[(\bullet)^{2T}, A_4^- + A_6^+, H_2 + H_5, K_2 + K_5, L_1^+ + L_2^+, M_1^- + M_2^-]$ | (2, 2, 5) |
| $[(\bullet)^{2T}, A_4^- + A_6^+, H_2 + H_5, K_2 + K_5, L_1^- + L_2^-, M_1^+ + M_2^+]$ | (2, 5, 5) |
| $[(\bullet)^{2T}, A_4^- + A_6^+, H_2 + H_3, K_1 + K_4, L_1^+ + L_1^-, M_1^+ + M_1^-]$ | (5, 4, 3) |

... continued on next page



... continued on next page

... continued from previous page

|                                                                                       |           |
|---------------------------------------------------------------------------------------|-----------|
| $[(\bullet)^{2T}, A_4^+ + A_6^-, H_1 + H_6, K_2 + K_5, L_1^+ + L_2^+, M_1^- + M_2^-]$ | (2, 2, 5) |
| $[(\bullet)^{2T}, A_4^+ + A_6^-, H_1 + H_6, K_2 + K_5, L_1^- + L_2^-, M_1^+ + M_2^+]$ | (2, 5, 5) |
| $[(\bullet)^{2T}, A_4^+ + A_6^-, H_1 + H_6, K_2 + K_5, L_1^- + L_2^-, M_1^- + M_2^-]$ | (5, 2, 2) |
| $[(\bullet)^{2T}, A_4^+ + A_6^-, H_1 + H_4, K_2 + K_3, L_1^+ + L_1^-, M_1^+ + M_1^-]$ | (3, 2, 3) |
| $[(\bullet)^{2T}, A_4^+ + A_6^-, H_1 + H_6, K_2 + K_5, L_2^+ + L_2^-, M_2^+ + M_2^-]$ | (5, 5, 5) |
| $[(\bullet)^{2T}, A_4^+ + A_6^-, H_1 + H_4, K_2 + K_3, L_1^+ + L_2^+, M_1^+ + M_2^+]$ | (3, 5, 0) |
| $[(\bullet)^{2T}, A_4^+ + A_6^-, H_1 + H_4, K_2 + K_3, L_1^+ + L_2^+, M_1^- + M_2^-]$ | (0, 2, 3) |
| $[(\bullet)^{2T}, A_4^+ + A_6^-, H_1 + H_4, K_2 + K_3, L_1^- + L_2^-, M_1^+ + M_2^+]$ | (0, 5, 3) |
| $[(\bullet)^{2T}, A_4^+ + A_6^-, H_1 + H_4, K_2 + K_3, L_1^- + L_2^-, M_1^- + M_2^-]$ | (3, 2, 0) |
| $[(\bullet)^{2T}, A_4^+ + A_6^-, H_1 + H_4, K_2 + K_3, L_2^+ + L_2^-, M_2^+ + M_2^-]$ | (3, 5, 3) |
| $[(\bullet)^{2T}, A_4^+ + A_6^-, H_1 + H_6, K_1 + K_6, L_1^- + L_2^-, M_1^+ + M_2^+]$ | (2, 1, 1) |
| $[(\bullet)^{2T}, A_4^+ + A_6^-, H_1 + H_2, K_1 + K_2, L_1^- + L_2^-, M_1^+ + M_2^+]$ | (4, 5, 1) |

2nd minimal solution:  $\mu_2^T = 3$  (25632 symmetry vectors)

Space group 176 ( $\mathbb{Z}_3 \times \mathbb{Z}_6$ )

1st minimal solution:  $\mu_1^T = 4$  (936 symmetry vectors)

| $\mathbf{n}^T$                                                                                                                      | $\mathbf{v}^T \in \mathbb{Z}_3 \times \mathbb{Z}_6$ |
|-------------------------------------------------------------------------------------------------------------------------------------|-----------------------------------------------------|
| $[(\bullet)^{2T} + \Gamma_3^- + \Gamma_5^-, A_2 + A_3, 2H_5 + 2H_6, K_5 + 3K_6, 2L_1, 2M_1^- + M_2^+ + M_2^-]$                      | (1, 1)                                              |
| $[(\bullet)^{2T} + \Gamma_3^- + \Gamma_5^-, A_2 + A_3, H_3 + H_5 + 2H_6, K_4 + K_5 + 2K_6, 2L_1, 2M_1^- + M_2^+ + M_2^-]$           | (2, 3)                                              |
| $[(\bullet)^{2T} + \Gamma_3^- + \Gamma_5^-, A_2 + A_3, H_4 + 2H_5 + H_6, K_4 + K_5 + 2K_6, 2L_1, 2M_1^- + M_2^+ + M_2^-]$           | (2, 3)                                              |
| $[(\bullet)^{2T} + \Gamma_3^- + \Gamma_5^-, A_2 + A_3, H_3 + H_4 + H_5 + H_6, 2K_4 + K_5 + K_6, 2L_1, 2M_1^- + M_2^+ + M_2^-]$      | (0, 5)                                              |
| $[(\bullet)^{2T} + \Gamma_3^- + \Gamma_5^-, A_2 + A_3, H_1 + H_5 + 2H_6, K_2 + K_5 + 2K_6, 2L_1, 2M_1^- + M_2^+ + M_2^-]$           | (0, 5)                                              |
| $[(\bullet)^{2T} + \Gamma_3^- + \Gamma_5^-, A_2 + A_3, H_2 + 2H_5 + H_6, K_2 + K_5 + 2K_6, 2L_1, 2M_1^- + M_2^+ + M_2^-]$           | (0, 5)                                              |
| $[(\bullet)^{2T} + \Gamma_3^- + \Gamma_5^-, A_2 + A_3, H_2 + H_3 + H_5 + H_6, K_2 + K_4 + K_5 + K_6, 2L_1, 2M_1^- + M_2^+ + M_2^-]$ | (1, 1)                                              |
| $[(\bullet)^{2T} + \Gamma_3^- + \Gamma_5^-, A_2 + A_3, H_1 + H_4 + H_5 + H_6, K_2 + K_4 + K_5 + K_6, 2L_1, 2M_1^- + M_2^+ + M_2^-]$ | (1, 1)                                              |
| $[(\bullet)^{2T} + \Gamma_3^- + \Gamma_5^-, A_2 + A_3, H_1 + H_2 + H_5 + H_6, 2K_2 + K_5 + K_6, 2L_1, 2M_1^- + M_2^+ + M_2^-]$      | (2, 3)                                              |
| $[(\bullet)^{2T} + \Gamma_3^- + \Gamma_5^-, A_2 + A_3, 2H_5 + 2H_6, K_5 + 3K_6, 2L_1, M_1^+ + M_1^- + 2M_2^+]$                      | (1, 4)                                              |
| $[(\bullet)^{2T} + \Gamma_3^- + \Gamma_5^-, A_2 + A_3, H_3 + H_5 + 2H_6, K_4 + K_5 + 2K_6, 2L_1, M_1^+ + M_1^- + 2M_2^+]$           | (2, 0)                                              |
| $[(\bullet)^{2T} + \Gamma_3^- + \Gamma_5^-, A_2 + A_3, H_4 + 2H_5 + H_6, K_4 + K_5 + 2K_6, 2L_1, M_1^+ + M_1^- + 2M_2^+]$           | (2, 0)                                              |
| $[(\bullet)^{2T} + \Gamma_3^- + \Gamma_5^-, A_2 + A_3, H_3 + H_4 + H_5 + H_6, 2K_4 + K_5 + K_6, 2L_1, M_1^+ + M_1^- + 2M_2^+]$      | (0, 2)                                              |
| $[(\bullet)^{2T} + \Gamma_3^- + \Gamma_5^-, A_2 + A_3, H_1 + H_5 + 2H_6, K_2 + K_5 + 2K_6, 2L_1, M_1^+ + M_1^- + 2M_2^+]$           | (0, 2)                                              |
| $[(\bullet)^{2T} + \Gamma_3^- + \Gamma_5^-, A_2 + A_3, H_2 + 2H_5 + H_6, K_2 + K_5 + 2K_6, 2L_1, M_1^+ + M_1^- + 2M_2^+]$           | (0, 2)                                              |
| $[(\bullet)^{2T} + \Gamma_3^- + \Gamma_5^-, A_2 + A_3, H_2 + H_3 + H_5 + H_6, K_2 + K_4 + K_5 + K_6, 2L_1, M_1^+ + M_1^- + 2M_2^+]$ | (1, 4)                                              |
| $[(\bullet)^{2T} + \Gamma_3^- + \Gamma_5^-, A_2 + A_3, H_1 + H_4 + H_5 + H_6, K_2 + K_4 + K_5 + K_6, 2L_1, M_1^+ + M_1^- + 2M_2^+]$ | (1, 4)                                              |
| $[(\bullet)^{2T} + \Gamma_3^- + \Gamma_5^-, A_2 + A_3, H_1 + H_2 + H_5 + H_6, 2K_2 + K_5 + K_6, 2L_1, M_1^+ + M_1^- + 2M_2^+]$      | (2, 0)                                              |
| $[(\bullet)^{2T} + \Gamma_3^- + \Gamma_5^-, A_2 + A_3, H_3 + H_5 + 2H_6, K_3 + 3K_6, 2L_1, 2M_1^- + M_2^+ + M_2^-]$                 | (2, 5)                                              |
| $[(\bullet)^{2T} + \Gamma_3^- + \Gamma_5^-, A_2 + A_3, 2H_3 + 2H_6, K_3 + K_4 + 2K_6, 2L_1, 2M_1^- + M_2^+ + M_2^-]$                | (0, 1)                                              |
| $[(\bullet)^{2T} + \Gamma_3^- + \Gamma_5^-, A_2 + A_3, H_3 + H_4 + H_5 + H_6, K_3 + K_4 + 2K_6, 2L_1, 2M_1^- + M_2^+ + M_2^-]$      | (0, 1)                                              |
| $[(\bullet)^{2T} + \Gamma_3^- + \Gamma_5^-, A_2 + A_3, 2H_3 + H_4 + H_6, K_3 + 2K_4 + K_6, 2L_1, 2M_1^- + M_2^+ + M_2^-]$           | (1, 3)                                              |
| $[(\bullet)^{2T} + \Gamma_3^- + \Gamma_5^-, A_2 + A_3, H_1 + H_3 + 2H_6, K_2 + K_3 + 2K_6, 2L_1, 2M_1^- + M_2^+ + M_2^-]$           | (1, 3)                                              |
| $[(\bullet)^{2T} + \Gamma_3^- + \Gamma_5^-, A_2 + A_3, H_2 + H_3 + H_5 + H_6, K_2 + K_3 + 2K_6, 2L_1, 2M_1^- + M_2^+ + M_2^-]$      | (1, 3)                                              |
| $[(\bullet)^{2T} + \Gamma_3^- + \Gamma_5^-, A_2 + A_3, H_2 + 2H_3 + H_6, K_2 + K_3 + K_4 + K_6, 2L_1, 2M_1^- + M_2^+ + M_2^-]$      | (2, 5)                                              |
| $[(\bullet)^{2T} + \Gamma_3^- + \Gamma_5^-, A_2 + A_3, H_1 + H_3 + H_4 + H_6, K_2 + K_3 + K_4 + K_6, 2L_1, 2M_1^- + M_2^+ + M_2^-]$ | (2, 5)                                              |
| $[(\bullet)^{2T} + \Gamma_3^- + \Gamma_5^-, A_2 + A_3, H_1 + H_2 + H_3 + H_6, 2K_2 + K_3 + K_6, 2L_1, 2M_1^- + M_2^+ + M_2^-]$      | (0, 1)                                              |
| $[(\bullet)^{2T} + \Gamma_3^- + \Gamma_5^-, A_2 + A_3, H_3 + H_5 + 2H_6, K_3 + 3K_6, 2L_1, M_1^+ + M_1^- + 2M_2^+]$                 | (2, 2)                                              |
| $[(\bullet)^{2T} + \Gamma_3^- + \Gamma_5^-, A_2 + A_3, 2H_3 + 2H_6, K_3 + K_4 + 2K_6, 2L_1, M_1^+ + M_1^- + 2M_2^+]$                | (0, 4)                                              |
| $[(\bullet)^{2T} + \Gamma_3^- + \Gamma_5^-, A_2 + A_3, H_3 + H_4 + H_5 + H_6, K_3 + K_4 + 2K_6, 2L_1, M_1^+ + M_1^- + 2M_2^+]$      | (0, 4)                                              |
| $[(\bullet)^{2T} + \Gamma_3^- + \Gamma_5^-, A_2 + A_3, 2H_3 + H_4 + H_6, K_3 + 2K_4 + K_6, 2L_1, M_1^+ + M_1^- + 2M_2^+]$           | (1, 0)                                              |

... continued on next page

... continued on next page

... continued on next page

... continued on next page

... continued on next page

... continued on next page

... continued on next page



... continued on next page

... continued on next page

... continued on next page

... continued on next page

... continued on next page

... continued on next page

... continued on next page

... continued on next page



... continued on next page

... continued on next page

... continued from previous page

|                                                                                                                                   |         |
|-----------------------------------------------------------------------------------------------------------------------------------|---------|
| $[(\blacksquare)^{2T} + \Gamma_3^- + \Gamma_5^+, A_2 + A_3, H_2 + H_4 + 2H_5, K_1 + K_3 + 2K_6, 2L_1, 2M_1^- + 2M_2^-]$           | (1, 4)  |
| $[(\blacksquare)^{2T} + \Gamma_3^- + \Gamma_5^+, A_2 + A_3, H_2 + H_4 + 2H_5, K_1 + K_4 + K_5 + K_6, 2L_1, 2M_1^- + 2M_2^-]$      | (1, 2)  |
| $[(\blacksquare)^{2T} + \Gamma_3^- + \Gamma_5^+, A_2 + A_3, H_2 + H_3 + H_4 + H_5, K_1 + K_3 + K_4 + K_6, 2L_1, 2M_1^- + 2M_2^-]$ | (2, 0)  |
| $[(\blacksquare)^{2T} + \Gamma_3^- + \Gamma_5^+, A_2 + A_3, H_2 + H_3 + H_4 + H_5, K_1 + 2K_4 + K_5, 2L_1, 2M_1^- + 2M_2^-]$      | (2, 4)  |
| $[(\blacksquare)^{2T} + \Gamma_3^- + \Gamma_5^+, A_2 + A_3, H_2 + 2H_3 + H_4, K_1 + K_3 + 2K_4, 2L_1, 2M_1^- + 2M_2^-]$           | (0, 2)  |
| $[(\blacksquare)^{2T} + \Gamma_3^- + \Gamma_5^+, A_2 + A_3, H_1 + 2H_4 + H_5, K_1 + K_3 + K_4 + K_6, 2L_1, 2M_1^- + 2M_2^-]$      | (2, 0)  |
| $[(\blacksquare)^{2T} + \Gamma_3^- + \Gamma_5^+, A_2 + A_3, H_1 + 2H_4 + H_5, K_1 + 2K_4 + K_5, 2L_1, 2M_1^- + 2M_2^-]$           | (2, 4)  |
| $[(\blacksquare)^{2T} + \Gamma_3^- + \Gamma_5^+, A_2 + A_3, H_1 + H_3 + 2H_4, K_1 + K_3 + 2K_4, 2L_1, 2M_1^- + 2M_2^-]$           | (0, 2)  |
| $[(\blacksquare)^{2T} + \Gamma_3^- + \Gamma_5^+, A_2 + A_3, 2H_1 + 2H_6, K_1 + K_2 + K_5 + K_6, 2L_1, 2M_1^- + 2M_2^-]$           | (2, 4)  |
| $[(\blacksquare)^{2T} + \Gamma_3^- + \Gamma_5^+, A_2 + A_3, H_1 + H_2 + H_5 + H_6, K_1 + K_2 + K_5 + K_6, 2L_1, 2M_1^- + 2M_2^-]$ | (2, 4)  |
| $[(\blacksquare)^{2T} + \Gamma_3^- + \Gamma_5^+, A_2 + A_3, H_1 + H_2 + H_3 + H_6, K_1 + K_2 + K_3 + K_6, 2L_1, 2M_1^- + 2M_2^-]$ | (0, 2)  |
| $[(\blacksquare)^{2T} + \Gamma_3^- + \Gamma_5^+, A_2 + A_3, H_1 + H_2 + H_3 + H_6, K_1 + K_2 + K_4 + K_5, 2L_1, 2M_1^- + 2M_2^-]$ | trivial |
| $[(\blacksquare)^{2T} + \Gamma_3^- + \Gamma_5^+, A_2 + A_3, 2H_1 + H_4 + H_6, K_1 + K_2 + K_3 + K_6, 2L_1, 2M_1^- + 2M_2^-]$      | (0, 2)  |
| $[(\blacksquare)^{2T} + \Gamma_3^- + \Gamma_5^+, A_2 + A_3, 2H_1 + H_4 + H_6, K_1 + K_2 + K_4 + K_5, 2L_1, 2M_1^- + 2M_2^-]$      | trivial |
| $[(\blacksquare)^{2T} + \Gamma_3^- + \Gamma_5^+, A_2 + A_3, 2H_2 + 2H_5, K_1 + K_2 + K_5 + K_6, 2L_1, 2M_1^- + 2M_2^-]$           | (2, 4)  |
| $[(\blacksquare)^{2T} + \Gamma_3^- + \Gamma_5^+, A_2 + A_3, 2H_2 + H_3 + H_5, K_1 + K_2 + K_3 + K_6, 2L_1, 2M_1^- + 2M_2^-]$      | (0, 2)  |
| $[(\blacksquare)^{2T} + \Gamma_3^- + \Gamma_5^+, A_2 + A_3, 2H_2 + H_3 + H_5, K_1 + K_2 + K_4 + K_5, 2L_1, 2M_1^- + 2M_2^-]$      | trivial |
| $[(\blacksquare)^{2T} + \Gamma_3^- + \Gamma_5^+, A_2 + A_3, 2H_2 + 2H_3, K_1 + K_2 + K_3 + K_4, 2L_1, 2M_1^- + 2M_2^-]$           | (1, 4)  |
| $[(\blacksquare)^{2T} + \Gamma_3^- + \Gamma_5^+, A_2 + A_3, H_1 + H_2 + H_4 + H_5, K_1 + K_2 + K_3 + K_6, 2L_1, 2M_1^- + 2M_2^-]$ | (0, 2)  |
| $[(\blacksquare)^{2T} + \Gamma_3^- + \Gamma_5^+, A_2 + A_3, H_1 + H_2 + H_4 + H_5, K_1 + K_2 + K_4 + K_5, 2L_1, 2M_1^- + 2M_2^-]$ | trivial |
| $[(\blacksquare)^{2T} + \Gamma_3^- + \Gamma_5^+, A_2 + A_3, H_1 + H_2 + H_3 + H_4, K_1 + K_2 + K_3 + K_4, 2L_1, 2M_1^- + 2M_2^-]$ | (1, 4)  |
| $[(\blacksquare)^{2T} + \Gamma_3^- + \Gamma_5^+, A_2 + A_3, 2H_1 + 2H_4, K_1 + K_2 + K_3 + K_4, 2L_1, 2M_1^- + 2M_2^-]$           | (1, 4)  |
| $[(\blacksquare)^{2T} + \Gamma_3^- + \Gamma_5^+, A_2 + A_3, 2H_1 + H_2 + H_6, K_1 + 2K_2 + K_5, 2L_1, 2M_1^- + 2M_2^-]$           | (1, 2)  |
| $[(\blacksquare)^{2T} + \Gamma_3^- + \Gamma_5^+, A_2 + A_3, H_1 + 2H_2 + H_5, K_1 + 2K_2 + K_5, 2L_1, 2M_1^- + 2M_2^-]$           | (1, 2)  |
| $[(\blacksquare)^{2T} + \Gamma_3^- + \Gamma_5^+, A_2 + A_3, H_1 + 2H_2 + H_3, K_1 + 2K_2 + K_3, 2L_1, 2M_1^- + 2M_2^-]$           | (2, 0)  |
| $[(\blacksquare)^{2T} + \Gamma_3^- + \Gamma_5^+, A_2 + A_3, 2H_1 + H_2 + H_4, K_1 + 2K_2 + K_3, 2L_1, 2M_1^- + 2M_2^-]$           | (2, 0)  |
| $[(\blacksquare)^{2T} + \Gamma_3^- + \Gamma_5^+, A_2 + A_3, 2H_1 + 2H_6, 2K_1 + 2K_6, 2L_1, 2M_1^- + 2M_2^-]$                     | (2, 2)  |
| $[(\blacksquare)^{2T} + \Gamma_3^- + \Gamma_5^+, A_2 + A_3, H_1 + H_2 + H_5 + H_6, 2K_1 + 2K_6, 2L_1, 2M_1^- + 2M_2^-]$           | (2, 2)  |
| $[(\blacksquare)^{2T} + \Gamma_3^- + \Gamma_5^+, A_2 + A_3, H_1 + H_2 + H_3 + H_6, 2K_1 + K_4 + K_6, 2L_1, 2M_1^- + 2M_2^-]$      | (0, 4)  |
| $[(\blacksquare)^{2T} + \Gamma_3^- + \Gamma_5^+, A_2 + A_3, 2H_1 + H_4 + H_6, 2K_1 + K_4 + K_6, 2L_1, 2M_1^- + 2M_2^-]$           | (0, 4)  |
| $[(\blacksquare)^{2T} + \Gamma_3^- + \Gamma_5^+, A_2 + A_3, 2H_2 + 2H_5, 2K_1 + 2K_6, 2L_1, 2M_1^- + 2M_2^-]$                     | (2, 2)  |
| $[(\blacksquare)^{2T} + \Gamma_3^- + \Gamma_5^+, A_2 + A_3, 2H_2 + H_3 + H_5, 2K_1 + K_4 + K_6, 2L_1, 2M_1^- + 2M_2^-]$           | (0, 4)  |
| $[(\blacksquare)^{2T} + \Gamma_3^- + \Gamma_5^+, A_2 + A_3, 2H_2 + 2H_3, 2K_1 + 2K_4, 2L_1, 2M_1^- + 2M_2^-]$                     | (1, 0)  |
| $[(\blacksquare)^{2T} + \Gamma_3^- + \Gamma_5^+, A_2 + A_3, H_1 + H_2 + H_4 + H_5, 2K_1 + K_4 + K_6, 2L_1, 2M_1^- + 2M_2^-]$      | (0, 4)  |
| $[(\blacksquare)^{2T} + \Gamma_3^- + \Gamma_5^+, A_2 + A_3, H_1 + H_2 + H_3 + H_4, 2K_1 + 2K_4, 2L_1, 2M_1^- + 2M_2^-]$           | (1, 0)  |
| $[(\blacksquare)^{2T} + \Gamma_3^- + \Gamma_5^+, A_2 + A_3, 2H_1 + 2H_4, 2K_1 + 2K_4, 2L_1, 2M_1^- + 2M_2^-]$                     | (1, 0)  |
| $[(\blacksquare)^{2T} + \Gamma_3^- + \Gamma_5^+, A_2 + A_3, 2H_1 + H_2 + H_6, 2K_1 + K_2 + K_6, 2L_1, 2M_1^- + 2M_2^-]$           | (1, 0)  |
| $[(\blacksquare)^{2T} + \Gamma_3^- + \Gamma_5^+, A_2 + A_3, H_1 + 2H_2 + H_5, 2K_1 + K_2 + K_6, 2L_1, 2M_1^- + 2M_2^-]$           | (1, 0)  |
| $[(\blacksquare)^{2T} + \Gamma_3^- + \Gamma_5^+, A_2 + A_3, H_1 + 2H_2 + H_3, 2K_1 + K_2 + K_4, 2L_1, 2M_1^- + 2M_2^-]$           | (2, 2)  |
| $[(\blacksquare)^{2T} + \Gamma_3^- + \Gamma_5^+, A_2 + A_3, 2H_1 + H_2 + H_4, 2K_1 + K_2 + K_4, 2L_1, 2M_1^- + 2M_2^-]$           | (2, 2)  |
| $[(\blacksquare)^{2T} + \Gamma_3^- + \Gamma_5^+, A_2 + A_3, 2H_1 + 2H_2, 2K_1 + 2K_2, 2L_1, 2M_1^- + 2M_2^-]$                     | (0, 4)  |

2nd minimal solution:  $\mu_2^T = 6$  (50996 symmetry vectors)

Space group 177 ( $\mathbb{Z}_1$ )

1st minimal solution:  $\mu_1^T = 2$  (1 symmetry vector)

$$\overline{\mathbf{n}^T} \\ \overline{[(\blacksquare)^{2T}, A_6, H_1 + H_2, 2K_2, L_1 + L_2, 2M_2]}$$

2nd minimal solution:  $\mu_2^T = 3$  (16 symmetry vectors)

Space group 178 ( $\mathbb{Z}_1$ )

1st minimal solution:  $\mu_1^T = 6$  (3 symmetry vectors)

| $\mathbf{n}^T$                                                                                                                               |
|----------------------------------------------------------------------------------------------------------------------------------------------|
| $[(\blacksquare)^{2T} + \Gamma_1 + \Gamma_4 + \Gamma_5, A_1 + A_2 + A_3, H_1 + H_2 + 2H_3, 2K_2 + 2K_3, 3L_1, M_1 + 2M_2 + M_3 + 2M_4]$      |
| $[(\blacksquare)^{2T} + \Gamma_1 + \Gamma_3 + \Gamma_5, A_1 + A_2 + A_3, H_1 + H_2 + 2H_3, K_1 + K_2 + 2K_3, 3L_1, M_1 + 2M_2 + 2M_3 + M_4]$ |
| $[(\blacksquare)^{2T} + \Gamma_2 + \Gamma_3 + \Gamma_5, A_1 + A_2 + A_3, H_1 + H_2 + 2H_3, 2K_2 + 2K_3, 3L_1, 3M_2 + 2M_3 + M_4]$            |

2nd minimal solution:  $\mu_2^T = 12$  (8 symmetry vectors)

Space group 179 ( $\mathbb{Z}_1$ )

1st minimal solution:  $\mu_1^T = 6$  (3 symmetry vectors)

| $\mathbf{n}^T$                                                                                                                               |
|----------------------------------------------------------------------------------------------------------------------------------------------|
| $[(\blacksquare)^{2T} + \Gamma_1 + \Gamma_4 + \Gamma_5, A_1 + A_2 + A_3, H_1 + H_2 + 2H_3, 2K_2 + 2K_3, 3L_1, M_1 + 2M_2 + M_3 + 2M_4]$      |
| $[(\blacksquare)^{2T} + \Gamma_1 + \Gamma_3 + \Gamma_5, A_1 + A_2 + A_3, H_1 + H_2 + 2H_3, K_1 + K_2 + 2K_3, 3L_1, M_1 + 2M_2 + 2M_3 + M_4]$ |
| $[(\blacksquare)^{2T} + \Gamma_2 + \Gamma_3 + \Gamma_5, A_1 + A_2 + A_3, H_1 + H_2 + 2H_3, 2K_2 + 2K_3, 3L_1, 3M_2 + 2M_3 + M_4]$            |

2nd minimal solution:  $\mu_2^T = 12$  (8 symmetry vectors)

Space group 180 ( $\mathbb{Z}_1$ )

1st minimal solution:  $\mu_1^T = 3$  (2 symmetry vectors)

| $\mathbf{n}^T$                                                                                   |
|--------------------------------------------------------------------------------------------------|
| $[(\blacksquare)^{2T} + \Gamma_3, A_3 + A_6, H_1 + H_3, K_2 + K_3, L_1 + L_2 + L_4, 2M_2 + M_3]$ |
| $[(\blacksquare)^{2T} + \Gamma_3, A_4 + A_6, H_2 + H_3, K_2 + K_3, L_1 + L_2 + L_3, 2M_2 + M_3]$ |

2nd minimal solution:  $\mu_2^T = 6$  (45 symmetry vectors)

Space group 181 ( $\mathbb{Z}_1$ )

1st minimal solution:  $\mu_1^T = 3$  (2 symmetry vectors)

| $\mathbf{n}^T$                                                                                   |
|--------------------------------------------------------------------------------------------------|
| $[(\blacksquare)^{2T} + \Gamma_3, A_3 + A_6, H_1 + H_3, K_2 + K_3, L_1 + L_2 + L_3, 2M_2 + M_3]$ |
| $[(\blacksquare)^{2T} + \Gamma_3, A_4 + A_6, H_2 + H_3, K_2 + K_3, L_1 + L_2 + L_4, 2M_2 + M_3]$ |

2nd minimal solution:  $\mu_2^T = 6$  (45 symmetry vectors)

Space group 182 ( $\mathbb{Z}_1$ )

1st minimal solution:  $\mu_1^T = 4$  (2 symmetry vectors)

| $\mathbf{n}^T$                                                                                     |
|----------------------------------------------------------------------------------------------------|
| $[(\blacksquare)^{2T} + \Gamma_5, A_2 + A_3, H_1 + H_2 + H_3, 2K_2 + K_3, 2L_1, 2M_2 + M_3 + M_4]$ |
| $[(\blacksquare)^{2T} + \Gamma_5, A_2 + A_3, 2H_1 + 2H_2, K_1 + 3K_2, 2L_1, 2M_2 + M_3 + M_4]$     |

2nd minimal solution:  $\mu_2^T = 6$  (12 symmetry vectors)

Space group 183 ( $\mathbb{Z}_1$ )

1st minimal solution:  $\mu_1^T = 2$  (4 symmetry vectors)

| $\mathbf{n}^T$                                                           |
|--------------------------------------------------------------------------|
| $[(\blacksquare)^{2T}, A_6, H_3, K_3, L_3 + L_4, M_3 + M_4]$             |
| $[(\blacksquare)^{2T}, A_6, H_3, K_3, L_1 + L_2, M_1 + M_2]$             |
| $[(\blacksquare)^{2T}, A_6, H_1 + H_2, K_1 + K_2, L_3 + L_4, M_3 + M_4]$ |
| $[(\blacksquare)^{2T}, A_6, H_1 + H_2, K_1 + K_2, L_1 + L_2, M_1 + M_2]$ |

2nd minimal solution:  $\mu_2^T = 3$  (16 symmetry vectors)

Space group 184 ( $\mathbb{Z}_2$ )

1st minimal solution:  $\mu_1^T = 2$  (4 symmetry vectors)

| $\mathbf{n}^T$                                                           | $\mathbf{v}^T \in \mathbb{Z}_2$ |
|--------------------------------------------------------------------------|---------------------------------|
| $[(\blacksquare)^{2T}, A_6, H_1 + H_2, K_1 + K_2, L_3 + L_4, M_3 + M_4]$ | trivial                         |
| $[(\blacksquare)^{2T}, A_6, H_1 + H_2, K_1 + K_2, L_1 + L_2, M_1 + M_2]$ | 1                               |
| $[(\blacksquare)^{2T}, A_6, H_3, K_3, L_3 + L_4, M_3 + M_4]$             | trivial                         |
| $[(\blacksquare)^{2T}, A_6, H_3, K_3, L_1 + L_2, M_1 + M_2]$             | 1                               |

2nd minimal solution:  $\mu_2^T = 4$  (36 symmetry vectors)

Space group 185 ( $\mathbb{Z}_1$ )

1st minimal solution:  $\mu_1^T = 4$  (3 symmetry vectors)

| $\mathbf{n}^T$                                                                                                                |
|-------------------------------------------------------------------------------------------------------------------------------|
| $[(\blacksquare)^{2T} + \Gamma_5, A_5 + A_6, 2H_3, 2K_3, L_1 + L_2 + L_3 + L_4, M_1 + M_2 + M_3 + M_4]$                       |
| $[(\blacksquare)^{2T} + \Gamma_5, A_5 + A_6, H_1 + H_2 + H_3, K_1 + K_2 + K_3, L_1 + L_2 + L_3 + L_4, M_1 + M_2 + M_3 + M_4]$ |
| $[(\blacksquare)^{2T} + \Gamma_5, A_5 + A_6, 2H_1 + 2H_2, 2K_1 + 2K_2, L_1 + L_2 + L_3 + L_4, M_1 + M_2 + M_3 + M_4]$         |

2nd minimal solution:  $\mu_2^T = 6$  (6 symmetry vectors)

Space group 186 ( $\mathbb{Z}_1$ )

1st minimal solution:  $\mu_1^T = 4$  (3 symmetry vectors)

| $\mathbf{n}^T$                                                                                                               |
|------------------------------------------------------------------------------------------------------------------------------|
| $[(\blacksquare)^{2T}, \Gamma_5, A_5 + A_6, 2H_3, 2K_3, L_1 + L_2 + L_3 + L_4, M_1 + M_2 + M_3 + M_4]$                       |
| $[(\blacksquare)^{2T}, \Gamma_5, A_5 + A_6, H_1 + H_2 + H_3, K_1 + K_2 + K_3, L_1 + L_2 + L_3 + L_4, M_1 + M_2 + M_3 + M_4]$ |
| $[(\blacksquare)^{2T}, \Gamma_5, A_5 + A_6, 2H_1 + 2H_2, 2K_1 + 2K_2, L_1 + L_2 + L_3 + L_4, M_1 + M_2 + M_3 + M_4]$         |

2nd minimal solution:  $\mu_2^T = 6$  (8 symmetry vectors)

Space group 187 ( $\mathbb{Z}_1$ )

1st minimal solution:  $\mu_1^T = 2$  (18 symmetry vectors)

| $\mathbf{n}^T$                                                           |
|--------------------------------------------------------------------------|
| $[(\blacksquare)^{2T}, A_6, 2H_6, K_5 + K_6, L_3 + L_4, M_2 + M_3]$      |
| $[(\blacksquare)^{2T}, A_6, H_2 + H_6, K_2 + K_5, L_3 + L_4, M_2 + M_3]$ |
| $[(\blacksquare)^{2T}, A_6, H_4 + H_6, K_4 + K_5, L_3 + L_4, M_2 + M_3]$ |
| $[(\blacksquare)^{2T}, A_6, H_2 + H_6, K_1 + K_6, L_3 + L_4, M_2 + M_3]$ |
| $[(\blacksquare)^{2T}, A_6, 2H_2, K_1 + K_2, L_3 + L_4, M_2 + M_3]$      |
| $[(\blacksquare)^{2T}, A_6, H_2 + H_4, K_1 + K_4, L_3 + L_4, M_2 + M_3]$ |
| $[(\blacksquare)^{2T}, A_6, H_4 + H_6, K_3 + K_6, L_3 + L_4, M_2 + M_3]$ |
| $[(\blacksquare)^{2T}, A_6, H_2 + H_4, K_2 + K_3, L_3 + L_4, M_2 + M_3]$ |
| $[(\blacksquare)^{2T}, A_6, 2H_4, K_3 + K_4, L_3 + L_4, M_2 + M_3]$      |
| $[(\blacksquare)^{2T}, A_5, 2H_5, K_5 + K_6, L_1 + L_2, M_2 + M_3]$      |
| $[(\blacksquare)^{2T}, A_5, H_1 + H_5, K_1 + K_6, L_1 + L_2, M_2 + M_3]$ |
| $[(\blacksquare)^{2T}, A_5, H_3 + H_5, K_3 + K_6, L_1 + L_2, M_2 + M_3]$ |
| $[(\blacksquare)^{2T}, A_5, H_1 + H_5, K_2 + K_5, L_1 + L_2, M_2 + M_3]$ |
| $[(\blacksquare)^{2T}, A_5, 2H_1, K_1 + K_2, L_1 + L_2, M_2 + M_3]$      |
| $[(\blacksquare)^{2T}, A_5, H_3 + H_5, K_4 + K_5, L_1 + L_2, M_2 + M_3]$ |
| $[(\blacksquare)^{2T}, A_5, H_1 + H_3, K_1 + K_4, L_1 + L_2, M_2 + M_3]$ |
| $[(\blacksquare)^{2T}, A_5, H_1 + H_3, K_2 + K_3, L_1 + L_2, M_2 + M_3]$ |
| $[(\blacksquare)^{2T}, A_5, 2H_3, K_3 + K_4, L_1 + L_2, M_2 + M_3]$      |

2nd minimal solution:  $\mu_2^T = 3$  (432 symmetry vectors)

Space group 188 ( $\mathbb{Z}_3$ )

1st minimal solution:  $\mu_1^T = 2$  (30 symmetry vectors)

| $\mathbf{n}^T$                                                     | $\mathbf{v}^T \in \mathbb{Z}_3$ |
|--------------------------------------------------------------------|---------------------------------|
| $[(\blacksquare)^{2T}, A_3, H_5 + H_6, K_5 + K_6, L_1, M_2 + M_3]$ | 1                               |
| $[(\blacksquare)^{2T}, A_3, H_2 + H_5, K_2 + K_5, L_1, M_2 + M_3]$ | 2                               |
| $[(\blacksquare)^{2T}, A_3, H_4 + H_5, K_4 + K_5, L_1, M_2 + M_3]$ | trivial                         |
| $[(\blacksquare)^{2T}, A_3, H_1 + H_6, K_1 + K_6, L_1, M_2 + M_3]$ | trivial                         |
| $[(\blacksquare)^{2T}, A_3, H_1 + H_2, K_1 + K_2, L_1, M_2 + M_3]$ | 1                               |

... continued on next page

... continued from previous page

|                                                                    |         |
|--------------------------------------------------------------------|---------|
| $[(\blacksquare)^{2T}, A_3, H_2 + H_5, K_1 + K_6, L_1, M_2 + M_3]$ | 2       |
| $[(\blacksquare)^{2T}, A_3, H_1 + H_4, K_1 + K_4, L_1, M_2 + M_3]$ | 2       |
| $[(\blacksquare)^{2T}, A_3, H_2 + H_3, K_1 + K_4, L_1, M_2 + M_3]$ | trivial |
| $[(\blacksquare)^{2T}, A_3, H_4 + H_5, K_3 + K_6, L_1, M_2 + M_3]$ | trivial |
| $[(\blacksquare)^{2T}, A_3, H_3 + H_6, K_3 + K_6, L_1, M_2 + M_3]$ | 2       |
| $[(\blacksquare)^{2T}, A_3, H_2 + H_3, K_2 + K_3, L_1, M_2 + M_3]$ | trivial |
| $[(\blacksquare)^{2T}, A_3, H_3 + H_4, K_3 + K_4, L_1, M_2 + M_3]$ | 1       |
| $[(\blacksquare)^{2T}, A_2, H_5 + H_6, K_5 + K_6, L_1, M_2 + M_3]$ | 2       |
| $[(\blacksquare)^{2T}, A_2, H_2 + H_5, K_2 + K_5, L_1, M_2 + M_3]$ | trivial |
| $[(\blacksquare)^{2T}, A_2, H_4 + H_5, K_4 + K_5, L_1, M_2 + M_3]$ | 1       |
| $[(\blacksquare)^{2T}, A_2, H_1 + H_6, K_1 + K_6, L_1, M_2 + M_3]$ | 1       |
| $[(\blacksquare)^{2T}, A_2, H_1 + H_2, K_1 + K_2, L_1, M_2 + M_3]$ | 2       |
| $[(\blacksquare)^{2T}, A_2, H_2 + H_5, K_1 + K_6, L_1, M_2 + M_3]$ | trivial |
| $[(\blacksquare)^{2T}, A_2, H_1 + H_4, K_1 + K_4, L_1, M_2 + M_3]$ | trivial |
| $[(\blacksquare)^{2T}, A_2, H_2 + H_3, K_1 + K_4, L_1, M_2 + M_3]$ | 1       |
| $[(\blacksquare)^{2T}, A_2, H_4 + H_5, K_3 + K_6, L_1, M_2 + M_3]$ | 1       |
| $[(\blacksquare)^{2T}, A_2, H_3 + H_6, K_3 + K_6, L_1, M_2 + M_3]$ | trivial |
| $[(\blacksquare)^{2T}, A_2, H_2 + H_3, K_2 + K_3, L_1, M_2 + M_3]$ | 1       |
| $[(\blacksquare)^{2T}, A_2, H_3 + H_4, K_3 + K_4, L_1, M_2 + M_3]$ | 2       |
| $[(\blacksquare)^{2T}, A_3, H_1 + H_6, K_2 + K_5, L_1, M_2 + M_3]$ | trivial |
| $[(\blacksquare)^{2T}, A_3, H_3 + H_6, K_4 + K_5, L_1, M_2 + M_3]$ | 2       |
| $[(\blacksquare)^{2T}, A_3, H_1 + H_4, K_2 + K_3, L_1, M_2 + M_3]$ | 2       |
| $[(\blacksquare)^{2T}, A_2, H_1 + H_6, K_2 + K_5, L_1, M_2 + M_3]$ | 1       |
| $[(\blacksquare)^{2T}, A_2, H_3 + H_6, K_4 + K_5, L_1, M_2 + M_3]$ | trivial |
| $[(\blacksquare)^{2T}, A_2, H_1 + H_4, K_2 + K_3, L_1, M_2 + M_3]$ | trivial |

2nd minimal solution:  $\mu_2^T = 4$  (1218 symmetry vectors)

Space group 189 ( $\mathbb{Z}_1$ )

1st minimal solution:  $\mu_1^T = 2$  (2 symmetry vectors)

| $\mathbf{n}^T$                                                                                     |
|----------------------------------------------------------------------------------------------------|
| $[(\blacksquare)^{2T}, A_6, H_2 + H_3, HA_2 + HA_3, K_3 + K_4, KA_3 + KA_4, L_2 + L_3, M_3 + M_4]$ |
| $[(\blacksquare)^{2T}, A_5, H_1 + H_4, HA_1 + HA_4, K_3 + K_4, KA_3 + KA_4, L_1 + L_4, M_3 + M_4]$ |

2nd minimal solution:  $\mu_2^T = 3$  (40 symmetry vectors)

Space group 190 ( $\mathbb{Z}_3$ )

1st minimal solution:  $\mu_1^T = 2$  (2 symmetry vectors & filling-enforced topology)

| $\mathbf{n}^T$                                                                  | $\mathbf{v}^T \in \mathbb{Z}_3$ |
|---------------------------------------------------------------------------------|---------------------------------|
| $[(\blacksquare)^{2T}, A_2, H_3, HA_3, K_3 + K_4, KA_3 + KA_4, L_1, M_3 + M_4]$ | 2                               |
| $[(\blacksquare)^{2T}, A_1, H_3, HA_3, K_3 + K_4, KA_3 + KA_4, L_1, M_3 + M_4]$ | 1                               |

2nd minimal solution:  $\mu_2^T = 4$  (220 symmetry vectors)

Space group 191 ( $\mathbb{Z}_1$ )

1st minimal solution:  $\mu_1^T = 2$  (2 symmetry vectors)

| $\mathbf{n}^T$                                                                     |
|------------------------------------------------------------------------------------|
| $[(\blacksquare)^{2T}, A_6^-, H_1 + H_4, K_3 + K_4, L_1^+ + L_2^+, M_2^+ + M_2^-]$ |
| $[(\blacksquare)^{2T}, A_6^+, H_2 + H_3, K_3 + K_4, L_1^- + L_2^-, M_2^+ + M_2^-]$ |

2nd minimal solution:  $\mu_2^T = 3$  (64 symmetry vectors)

Space group 192 ( $\mathbb{Z}_6$ )

1st minimal solution:  $\mu_1^T = 2$  (2 symmetry vectors & filling-enforced topology)

| $\mathbf{n}^T$                                                   | $\mathbf{v}^T \in \mathbb{Z}_6$ |
|------------------------------------------------------------------|---------------------------------|
| $[(\blacksquare)^{2T}, A_4, H_3, K_3 + K_4, L_1, M_2^+ + M_2^-]$ | 1                               |
| $[(\blacksquare)^{2T}, A_3, H_3, K_3 + K_4, L_1, M_2^+ + M_2^-]$ | 5                               |

2nd minimal solution:  $\mu_2^T = 4$  (216 symmetry vectors)

Space group 193 ( $\mathbb{Z}_1$ )

1st minimal solution:  $\mu_1^T = 4$  (6 symmetry vectors)

| $\mathbf{n}^T$                                                                                                               |
|------------------------------------------------------------------------------------------------------------------------------|
| $[(\blacksquare)^{2T} + \Gamma_5^+, A_3, H_2 + H_3 + H_5, K_3 + K_4 + K_5, L_1 + L_2, M_2^+ + M_2^- + M_3^- + M_4^-]$        |
| $[(\blacksquare)^{2T} + \Gamma_5^+, A_3, H_1 + H_4 + H_6, K_3 + K_4 + K_5, L_1 + L_2, M_2^+ + M_2^- + M_3^- + M_4^-]$        |
| $[(\blacksquare)^{2T} + \Gamma_5^+, A_3, H_1 + H_2 + H_3 + H_4, K_1 + K_3 + 2K_4, L_1 + L_2, M_2^+ + M_2^- + M_3^- + M_4^-]$ |
| $[(\blacksquare)^{2T} + \Gamma_5^-, A_3, H_2 + H_3 + H_5, K_3 + K_4 + K_6, L_1 + L_2, M_2^+ + M_2^- + M_3^+ + M_4^+]$        |
| $[(\blacksquare)^{2T} + \Gamma_5^-, A_3, H_1 + H_4 + H_6, K_3 + K_4 + K_6, L_1 + L_2, M_2^+ + M_2^- + M_3^+ + M_4^+]$        |
| $[(\blacksquare)^{2T} + \Gamma_5^-, A_3, H_1 + H_2 + H_3 + H_4, K_2 + 2K_3 + K_4, L_1 + L_2, M_2^+ + M_2^- + M_3^+ + M_4^+]$ |

2nd minimal solution:  $\mu_2^T = 6$  (96 symmetry vectors)

Space group 194 ( $\mathbb{Z}_1$ )

1st minimal solution:  $\mu_1^T = 4$  (6 symmetry vectors)

| $\mathbf{n}^T$                                                                                                  |
|-----------------------------------------------------------------------------------------------------------------|
| $[(\blacksquare)^{2T} + \Gamma_5^+, A_3, 2H_3, K_1 + K_3 + 2K_4, L_1 + L_2, M_2^+ + M_2^- + M_3^- + M_4^-]$     |
| $[(\blacksquare)^{2T} + \Gamma_5^+, A_3, H_2 + H_3, K_3 + K_4 + K_5, L_1 + L_2, M_2^+ + M_2^- + M_3^- + M_4^-]$ |
| $[(\blacksquare)^{2T} + \Gamma_5^+, A_3, H_1 + H_3, K_3 + K_4 + K_5, L_1 + L_2, M_2^+ + M_2^- + M_3^- + M_4^-]$ |
| $[(\blacksquare)^{2T} + \Gamma_5^-, A_3, 2H_3, K_2 + 2K_3 + K_4, L_1 + L_2, M_2^+ + M_2^- + M_3^+ + M_4^+]$     |
| $[(\blacksquare)^{2T} + \Gamma_5^-, A_3, H_2 + H_3, K_3 + K_4 + K_6, L_1 + L_2, M_2^+ + M_2^- + M_3^+ + M_4^+]$ |
| $[(\blacksquare)^{2T} + \Gamma_5^-, A_3, H_1 + H_3, K_3 + K_4 + K_6, L_1 + L_2, M_2^+ + M_2^- + M_3^+ + M_4^+]$ |



2nd minimal solution:  $\mu_2^T = 6$  (174 symmetry vectors)

Space group 195 ( $\mathbb{Z}_1$ )

1st minimal solution:  $\mu_1^T = 2$  (1 symmetry vector)

$$\frac{\mathbf{n}^T}{[(\blacksquare)^{2T}, R_2 + R_3, M_1 + M_2, X_2 + X_3]}$$

2nd minimal solution:  $\mu_2^T = 3$  (12 symmetry vectors)

Space group 196 ( $\mathbb{Z}_1$ )

1st minimal solution:  $\mu_1^T = 2$  (1 symmetry vector)

$$\frac{\mathbf{n}^T}{[(\blacksquare)^{2T}, X_2 + X_3, L_2 + L_3, W_1 + W_2]}$$

2nd minimal solution:  $\mu_2^T = 3$  (6 symmetry vectors)

Space group 197 ( $\mathbb{Z}_1$ )

1st minimal solution:  $\mu_1^T = 3$  (2 symmetry vectors)

$$\frac{\mathbf{n}^T}{[(\blacksquare)^{2T} + \Gamma_1, H_4, P_4, PA_4, N_1 + 2N_2] \\ [(\blacksquare)^{2T} + \Gamma_1, H_4, P_1 + P_2 + P_3, PA_1 + PA_2 + PA_3, 3N_1]}$$

2nd minimal solution:  $\mu_2^T = 4$  (6 symmetry vectors)

Space group 198 ( $\mathbb{Z}_1$ )

1st minimal solution:  $\mu_1^T = 4$  (4 symmetry vectors)

$$\frac{\mathbf{n}^T}{[(\blacksquare)^{2T} + \Gamma_2 + \Gamma_3, 2R_2, M_1 + M_2 + M_3 + M_4, 2X_1] \\ [(\blacksquare)^{2T} + \Gamma_1 + \Gamma_3, R_2 + R_3, M_1 + M_2 + M_3 + M_4, 2X_1] \\ [(\blacksquare)^{2T} + \Gamma_1 + \Gamma_2, R_1 + R_2, M_1 + M_2 + M_3 + M_4, 2X_1] \\ [(\blacksquare)^{2T} + 2\Gamma_1, R_1 + R_3, M_1 + M_2 + M_3 + M_4, 2X_1]}$$

2nd minimal solution:  $\mu_2^T = 8$  (8 symmetry vectors)

Space group 199 ( $\mathbb{Z}_1$ )

1st minimal solution:  $\mu_1^T = 2$  (1 symmetry vector)

| $\mathbf{n}^T$                                      |
|-----------------------------------------------------|
| $[(\bullet)^{2T}, H_2 + H_3, P_2, PA_2, N_1 + N_2]$ |

2nd minimal solution:  $\mu_2^T = 4$  (3 symmetry vectors)

Space group 200 ( $\mathbb{Z}_1$ )

1st minimal solution:  $\mu_1^T = 2$  (2 symmetry vectors)

| $\mathbf{n}^T$                                                  |
|-----------------------------------------------------------------|
| $[(\bullet)^{2T}, R_2^- + R_3^-, M_1^- + M_2^+, X_2^+ + X_3^+]$ |
| $[(\bullet)^{2T}, R_2^+ + R_3^+, M_1^+ + M_2^-, X_2^- + X_3^-]$ |

2nd minimal solution:  $\mu_2^T = 3$  (52 symmetry vectors)

Space group 201 ( $\mathbb{Z}_2$ )

1st minimal solution:  $\mu_1^T = 2$  (2 symmetry vectors & filling-enforced topology)

| $\mathbf{n}^T$                              | $\mathbf{v}^T \in \mathbb{Z}_2$ |
|---------------------------------------------|---------------------------------|
| $[(\bullet)^{2T}, R_2^+ + R_3^-, M_1, X_2]$ | 1                               |
| $[(\bullet)^{2T}, R_2^- + R_3^+, M_1, X_2]$ | 1                               |

2nd minimal solution:  $\mu_2^T = 4$  (40 symmetry vectors)

Space group 202 ( $\mathbb{Z}_1$ )

1st minimal solution:  $\mu_1^T = 3$  (40 symmetry vectors)

| $\mathbf{n}^T$                                                                                 |
|------------------------------------------------------------------------------------------------|
| $[(\bullet)^{2T} + \Gamma_2^+, X_2^- + X_3^- + X_4^-, 2L_2^- + L_3^-, W_1 + W_3 + W_4]$        |
| $[(\bullet)^{2T} + \Gamma_2^+, X_2^- + X_3^- + X_4^-, L_2^+ + L_2^- + L_3^-, W_1 + W_3 + W_4]$ |
| $[(\bullet)^{2T} + \Gamma_3^+, X_2^- + X_3^- + X_4^-, L_2^- + 2L_3^-, W_1 + W_3 + W_4]$        |
| $[(\bullet)^{2T} + \Gamma_3^+, X_2^- + X_3^- + X_4^-, L_2^- + L_3^+ + L_3^-, W_1 + W_3 + W_4]$ |
| $[(\bullet)^{2T} + \Gamma_1^+, X_2^- + X_3^- + X_4^-, L_1^- + L_2^- + L_3^-, W_1 + W_3 + W_4]$ |
| $[(\bullet)^{2T} + \Gamma_1^+, X_2^- + X_3^- + X_4^-, L_1^+ + L_2^- + L_3^-, W_1 + W_3 + W_4]$ |
| $[(\bullet)^{2T} + \Gamma_2^+, X_2^- + X_3^- + X_4^-, 2L_2^+ + L_3^-, W_1 + W_3 + W_4]$        |
| $[(\bullet)^{2T} + \Gamma_3^+, X_2^- + X_3^- + X_4^-, L_2^+ + 2L_3^-, W_1 + W_3 + W_4]$        |
| $[(\bullet)^{2T} + \Gamma_3^+, X_2^- + X_3^- + X_4^-, L_2^+ + L_3^+ + L_3^-, W_1 + W_3 + W_4]$ |
| $[(\bullet)^{2T} + \Gamma_1^+, X_2^- + X_3^- + X_4^-, L_1^- + L_2^+ + L_3^-, W_1 + W_3 + W_4]$ |

... continued on next page

... continued from previous page

---

|                                                                                              |
|----------------------------------------------------------------------------------------------|
| $[(\bullet)^{2T} + \Gamma_1^+, X_2^-, X_3^-, X_4^-, L_1^+ + L_2^+ + L_3^-, W_1 + W_3 + W_4]$ |
| $[(\bullet)^{2T} + \Gamma_2^+, X_2^-, X_3^-, X_4^-, 2L_2^- + L_3^+, W_1 + W_3 + W_4]$        |
| $[(\bullet)^{2T} + \Gamma_2^+, X_2^-, X_3^-, X_4^-, L_2^+ + L_2^- + L_3^+, W_1 + W_3 + W_4]$ |
| $[(\bullet)^{2T} + \Gamma_3^+, X_2^-, X_3^-, X_4^-, L_2^- + 2L_3^+, W_1 + W_3 + W_4]$        |
| $[(\bullet)^{2T} + \Gamma_1^+, X_2^-, X_3^-, X_4^-, L_1^- + L_2^- + L_3^+, W_1 + W_3 + W_4]$ |
| $[(\bullet)^{2T} + \Gamma_1^+, X_2^-, X_3^-, X_4^-, L_1^+ + L_2^- + L_3^+, W_1 + W_3 + W_4]$ |
| $[(\bullet)^{2T} + \Gamma_2^+, X_2^-, X_3^-, X_4^-, 2L_2^+ + L_3^+, W_1 + W_3 + W_4]$        |
| $[(\bullet)^{2T} + \Gamma_3^+, X_2^-, X_3^-, X_4^-, L_2^+ + 2L_3^+, W_1 + W_3 + W_4]$        |
| $[(\bullet)^{2T} + \Gamma_1^+, X_2^-, X_3^-, X_4^-, L_1^- + L_2^+ + L_3^+, W_1 + W_3 + W_4]$ |
| $[(\bullet)^{2T} + \Gamma_1^+, X_2^-, X_3^-, X_4^-, L_1^+ + L_2^+ + L_3^+, W_1 + W_3 + W_4]$ |
| $[(\bullet)^{2T} + \Gamma_2^-, X_2^+, X_3^+, X_4^+, 2L_2^- + L_3^-, W_2 + W_3 + W_4]$        |
| $[(\bullet)^{2T} + \Gamma_2^-, X_2^+, X_3^+, X_4^+, L_2^+ + L_2^- + L_3^-, W_2 + W_3 + W_4]$ |
| $[(\bullet)^{2T} + \Gamma_2^-, X_2^+, X_3^+, X_4^+, 2L_2^+ + L_3^-, W_2 + W_3 + W_4]$        |
| $[(\bullet)^{2T} + \Gamma_2^-, X_2^+, X_3^+, X_4^+, 2L_2^- + L_3^+, W_2 + W_3 + W_4]$        |
| $[(\bullet)^{2T} + \Gamma_2^-, X_2^+, X_3^+, X_4^+, L_2^+ + L_2^- + L_3^+, W_2 + W_3 + W_4]$ |
| $[(\bullet)^{2T} + \Gamma_2^-, X_2^+, X_3^+, X_4^+, 2L_2^+ + L_3^+, W_2 + W_3 + W_4]$        |
| $[(\bullet)^{2T} + \Gamma_3^-, X_2^+, X_3^+, X_4^+, L_2^- + 2L_3^-, W_2 + W_3 + W_4]$        |
| $[(\bullet)^{2T} + \Gamma_3^-, X_2^+, X_3^+, X_4^+, L_2^+ + 2L_3^-, W_2 + W_3 + W_4]$        |
| $[(\bullet)^{2T} + \Gamma_3^-, X_2^+, X_3^+, X_4^+, L_2^- + L_3^+ + L_3^-, W_2 + W_3 + W_4]$ |
| $[(\bullet)^{2T} + \Gamma_3^-, X_2^+, X_3^+, X_4^+, L_2^+ + L_3^+ + L_3^-, W_2 + W_3 + W_4]$ |
| $[(\bullet)^{2T} + \Gamma_3^-, X_2^+, X_3^+, X_4^+, L_2^- + 2L_3^+, W_2 + W_3 + W_4]$        |
| $[(\bullet)^{2T} + \Gamma_3^-, X_2^+, X_3^+, X_4^+, L_2^+ + 2L_3^+, W_2 + W_3 + W_4]$        |
| $[(\bullet)^{2T} + \Gamma_1^-, X_2^+, X_3^+, X_4^+, L_1^- + L_2^- + L_3^-, W_2 + W_3 + W_4]$ |
| $[(\bullet)^{2T} + \Gamma_1^-, X_2^+, X_3^+, X_4^+, L_1^- + L_2^+ + L_3^-, W_2 + W_3 + W_4]$ |
| $[(\bullet)^{2T} + \Gamma_1^-, X_2^+, X_3^+, X_4^+, L_1^- + L_2^- + L_3^+, W_2 + W_3 + W_4]$ |
| $[(\bullet)^{2T} + \Gamma_1^-, X_2^+, X_3^+, X_4^+, L_1^- + L_2^+ + L_3^+, W_2 + W_3 + W_4]$ |
| $[(\bullet)^{2T} + \Gamma_1^-, X_2^+, X_3^+, X_4^+, L_1^+ + L_2^- + L_3^-, W_2 + W_3 + W_4]$ |
| $[(\bullet)^{2T} + \Gamma_1^-, X_2^+, X_3^+, X_4^+, L_1^+ + L_2^+ + L_3^-, W_2 + W_3 + W_4]$ |
| $[(\bullet)^{2T} + \Gamma_1^-, X_2^+, X_3^+, X_4^+, L_1^+ + L_2^- + L_3^+, W_2 + W_3 + W_4]$ |
| $[(\bullet)^{2T} + \Gamma_1^-, X_2^+, X_3^+, X_4^+, L_1^+ + L_2^+ + L_3^+, W_2 + W_3 + W_4]$ |

---

2nd minimal solution:  $\mu_2^T = 4$  (310 symmetry vectors)

Space group 203 ( $\mathbb{Z}_2$ )

1st minimal solution:  $\mu_1^T = 2$  (4 symmetry vectors)

| $\mathbf{n}^T$                              | $\mathbf{v}^T \in \mathbb{Z}_2$ |
|---------------------------------------------|---------------------------------|
| $[(\bullet)^{2T}, X_2, L_2^- + L_3^+, W_1]$ | 1                               |
| $[(\bullet)^{2T}, X_2, L_2^- + L_3^-, W_1]$ | trivial                         |
| $[(\bullet)^{2T}, X_2, L_2^+ + L_3^+, W_1]$ | trivial                         |
| $[(\bullet)^{2T}, X_2, L_2^+ + L_3^-, W_1]$ | 1                               |

2nd minimal solution:  $\mu_2^T = 4$  (94 symmetry vectors)

Space group 204 ( $\mathbb{Z}_1$ )

1st minimal solution:  $\mu_1^T = 3$  (6 symmetry vectors)

| $\mathbf{n}^T$                                                               |
|------------------------------------------------------------------------------|
| $[(\blacksquare)^{2T} + \Gamma_1^+, H_4^-, P_4, N_1^- + 2N_2^-]$             |
| $[(\blacksquare)^{2T} + \Gamma_1^+, H_4^-, P_4, N_1^+ + N_2^+ + N_2^-]$      |
| $[(\blacksquare)^{2T} + \Gamma_1^+, H_4^-, P_1 + P_2 + P_3, 2N_1^+ + N_1^-]$ |
| $[(\blacksquare)^{2T} + \Gamma_1^-, H_4^+, P_4, N_1^- + N_2^+ + N_2^-]$      |
| $[(\blacksquare)^{2T} + \Gamma_1^-, H_4^+, P_4, N_1^+ + 2N_2^+]$             |
| $[(\blacksquare)^{2T} + \Gamma_1^-, H_4^+, P_1 + P_2 + P_3, N_1^+ + 2N_1^-]$ |

2nd minimal solution:  $\mu_2^T = 4$  (58 symmetry vectors)

Space group 205 ( $\mathbb{Z}_2$ )

1st minimal solution:  $\mu_1^T = 4$  (26 symmetry vectors)

| $\mathbf{n}^T$                                                                         | $\mathbf{v}^T \in \mathbb{Z}_2$ |
|----------------------------------------------------------------------------------------|---------------------------------|
| $[(\blacksquare)^{2T} + \Gamma_2^+ + \Gamma_3^-, 2R_2^-, M_1 + M_2, X_1 + X_2]$        | trivial                         |
| $[(\blacksquare)^{2T} + \Gamma_2^+ + \Gamma_3^-, R_2^+ + R_2^-, M_1 + M_2, X_1 + X_2]$ | 1                               |
| $[(\blacksquare)^{2T} + \Gamma_1^+ + \Gamma_3^-, R_2^- + R_3^+, M_1 + M_2, X_1 + X_2]$ | 1                               |
| $[(\blacksquare)^{2T} + \Gamma_1^+ + \Gamma_3^-, R_2^- + R_3^-, M_1 + M_2, X_1 + X_2]$ | trivial                         |
| $[(\blacksquare)^{2T} + \Gamma_2^+ + \Gamma_3^-, 2R_2^+, M_1 + M_2, X_1 + X_2]$        | trivial                         |
| $[(\blacksquare)^{2T} + \Gamma_1^+ + \Gamma_3^-, R_2^+ + R_3^+, M_1 + M_2, X_1 + X_2]$ | trivial                         |
| $[(\blacksquare)^{2T} + \Gamma_1^+ + \Gamma_3^-, R_2^+ + R_3^-, M_1 + M_2, X_1 + X_2]$ | 1                               |
| $[(\blacksquare)^{2T} + \Gamma_2^- + \Gamma_3^+, 2R_2^-, M_1 + M_2, X_1 + X_2]$        | trivial                         |
| $[(\blacksquare)^{2T} + \Gamma_2^- + \Gamma_3^+, R_2^+ + R_2^-, M_1 + M_2, X_1 + X_2]$ | 1                               |
| $[(\blacksquare)^{2T} + \Gamma_1^- + \Gamma_3^+, R_2^- + R_3^+, M_1 + M_2, X_1 + X_2]$ | 1                               |
| $[(\blacksquare)^{2T} + \Gamma_1^- + \Gamma_3^+, R_2^- + R_3^-, M_1 + M_2, X_1 + X_2]$ | trivial                         |
| $[(\blacksquare)^{2T} + \Gamma_2^- + \Gamma_3^+, 2R_2^+, M_1 + M_2, X_1 + X_2]$        | trivial                         |
| $[(\blacksquare)^{2T} + \Gamma_1^- + \Gamma_3^+, R_2^+ + R_3^+, M_1 + M_2, X_1 + X_2]$ | trivial                         |
| $[(\blacksquare)^{2T} + \Gamma_1^- + \Gamma_3^+, R_2^+ + R_3^-, M_1 + M_2, X_1 + X_2]$ | 1                               |
| $[(\blacksquare)^{2T} + \Gamma_1^+ + \Gamma_2^-, R_1^- + R_2^-, M_1 + M_2, X_1 + X_2]$ | trivial                         |
| $[(\blacksquare)^{2T} + \Gamma_1^+ + \Gamma_2^-, R_1^+ + R_2^-, M_1 + M_2, X_1 + X_2]$ | 1                               |
| $[(\blacksquare)^{2T} + \Gamma_1^+ + \Gamma_2^-, R_1^- + R_2^+, M_1 + M_2, X_1 + X_2]$ | 1                               |
| $[(\blacksquare)^{2T} + \Gamma_1^+ + \Gamma_2^-, R_1^+ + R_2^+, M_1 + M_2, X_1 + X_2]$ | trivial                         |
| $[(\blacksquare)^{2T} + \Gamma_1^- + \Gamma_2^+, R_1^- + R_2^-, M_1 + M_2, X_1 + X_2]$ | trivial                         |
| $[(\blacksquare)^{2T} + \Gamma_1^- + \Gamma_2^+, R_1^+ + R_2^-, M_1 + M_2, X_1 + X_2]$ | 1                               |
| $[(\blacksquare)^{2T} + \Gamma_1^- + \Gamma_2^+, R_1^- + R_2^+, M_1 + M_2, X_1 + X_2]$ | 1                               |
| $[(\blacksquare)^{2T} + \Gamma_1^- + \Gamma_2^+, R_1^+ + R_2^+, M_1 + M_2, X_1 + X_2]$ | trivial                         |
| $[(\blacksquare)^{2T} + \Gamma_1^+ + \Gamma_1^-, R_1^- + R_3^+, M_1 + M_2, X_1 + X_2]$ | 1                               |
| $[(\blacksquare)^{2T} + \Gamma_1^+ + \Gamma_1^-, R_1^- + R_3^-, M_1 + M_2, X_1 + X_2]$ | trivial                         |
| $[(\blacksquare)^{2T} + \Gamma_1^+ + \Gamma_1^-, R_1^+ + R_3^+, M_1 + M_2, X_1 + X_2]$ | trivial                         |
| $[(\blacksquare)^{2T} + \Gamma_1^+ + \Gamma_1^-, R_1^+ + R_3^-, M_1 + M_2, X_1 + X_2]$ | 1                               |

2nd minimal solution:  $\mu_2^T = 8$  (322 symmetry vectors)

Space group 206 ( $\mathbb{Z}_2$ )

1st minimal solution:  $\mu_1^T = 2$  (2 symmetry vectors & filling-enforced topology)

| $\mathbf{n}^T$                                  | $\mathbf{v}^T \in \mathbb{Z}_2$ |
|-------------------------------------------------|---------------------------------|
| $[(\blacksquare)^{2T}, H_2^-, H_3^+, P_2, N_1]$ | 1                               |
| $[(\blacksquare)^{2T}, H_2^+, H_3^-, P_2, N_1]$ | 1                               |

2nd minimal solution:  $\mu_2^T = 4$  (10 symmetry vectors)

Space group 207 ( $\mathbb{Z}_1$ )

1st minimal solution:  $\mu_1^T = 2$  (1 symmetry vector)

| $\mathbf{n}^T$                               |
|----------------------------------------------|
| $[(\blacksquare)^{2T}, R_3, M_2 + M_3, X_5]$ |

2nd minimal solution:  $\mu_2^T = 3$  (6 symmetry vectors)

Space group 208 ( $\mathbb{Z}_1$ )

1st minimal solution:  $\mu_1^T = 4$  (2 symmetry vectors)

| $\mathbf{n}^T$                                                                             |
|--------------------------------------------------------------------------------------------|
| $[(\blacksquare)^{2T} + \Gamma_1 + \Gamma_2, R_1 + R_5, M_1 + M_4 + M_5, X_2 + X_3 + X_5]$ |
| $[(\blacksquare)^{2T} + \Gamma_1 + \Gamma_2, R_2 + R_4, M_1 + M_4 + M_5, X_1 + X_4 + X_5]$ |

2nd minimal solution:  $\mu_2^T = 6$  (15 symmetry vectors)

Space group 209 ( $\mathbb{Z}_1$ )

1st minimal solution:  $\mu_1^T = 3$  (2 symmetry vectors)

| $\mathbf{n}^T$                                                            |
|---------------------------------------------------------------------------|
| $[(\blacksquare)^{2T} + \Gamma_1, X_3 + X_5, L_2 + L_3, W_2 + W_3 + W_4]$ |
| $[(\blacksquare)^{2T} + \Gamma_1, X_3 + X_5, L_1 + L_3, W_1 + W_3 + W_4]$ |

2nd minimal solution:  $\mu_2^T = 4$  (7 symmetry vectors)

Space group 210 ( $\mathbb{Z}_1$ )

1st minimal solution:  $\mu_1^T = 2$  (1 symmetry vector)

| $\mathbf{n}^T$                               |
|----------------------------------------------|
| $[(\blacksquare)^{2T}, X_1 + X_4, L_3, W_1]$ |

2nd minimal solution:  $\mu_2^T = 4$  (2 symmetry vectors)

Space group 211 ( $\mathbb{Z}_1$ )

1st minimal solution:  $\mu_1^T = 3$  (3 symmetry vectors)

| $\mathbf{n}^T$                                                       |
|----------------------------------------------------------------------|
| $[(\blacksquare)^{2T} + \Gamma_1, H_4, P_4, N_2 + N_3 + N_4]$        |
| $[(\blacksquare)^{2T} + \Gamma_1, H_4, P_1 + P_2 + P_3, N_1 + 2N_2]$ |
| $[(\blacksquare)^{2T} + \Gamma_2, H_5, P_4, N_2 + 2N_4]$             |

2nd minimal solution:  $\mu_2^T = 4$  (6 symmetry vectors)

Space group 212 ( $\mathbb{Z}_1$ )

1st minimal solution:  $\mu_1^T = 4$  (2 symmetry vectors)

| $\mathbf{n}^T$                                                                 |
|--------------------------------------------------------------------------------|
| $[(\blacksquare)^{2T} + \Gamma_3, R_1 + R_2, M_2 + M_3 + M_5, X_1 + X_2]$      |
| $[(\blacksquare)^{2T} + \Gamma_1 + \Gamma_2, R_3, M_2 + M_3 + M_5, X_1 + X_2]$ |

2nd minimal solution:  $\mu_2^T = 8$  (4 symmetry vectors)

Space group 213 ( $\mathbb{Z}_1$ )

1st minimal solution:  $\mu_1^T = 4$  (2 symmetry vectors)

| $\mathbf{n}^T$                                                                 |
|--------------------------------------------------------------------------------|
| $[(\blacksquare)^{2T} + \Gamma_3, R_1 + R_2, M_2 + M_3 + M_5, X_1 + X_2]$      |
| $[(\blacksquare)^{2T} + \Gamma_1 + \Gamma_2, R_3, M_2 + M_3 + M_5, X_1 + X_2]$ |

2nd minimal solution:  $\mu_2^T = 8$  (4 symmetry vectors)

Space group 214 ( $\mathbb{Z}_1$ )

1st minimal solution:  $\mu_1^T = 2$  (1 symmetry vector)

| $\mathbf{n}^T$                               |
|----------------------------------------------|
| $[(\blacksquare)^{2T}, H_3, P_2, N_2 + N_4]$ |

2nd minimal solution:  $\mu_2^T = 4$  (2 symmetry vectors)

Space group 215 ( $\mathbb{Z}_1$ )

1st minimal solution:  $\mu_1^T = 2$  (2 symmetry vectors)

| $\mathbf{n}^T$                               |
|----------------------------------------------|
| $[(\blacksquare)^{2T}, R_3, M_1 + M_4, X_5]$ |
| $[(\blacksquare)^{2T}, R_3, M_2 + M_3, X_5]$ |

2nd minimal solution:  $\mu_2^T = 3$  (12 symmetry vectors)

Space group 216 ( $\mathbb{Z}_1$ )

1st minimal solution:  $\mu_1^T = 2$  (4 symmetry vectors)

| $\mathbf{n}^T$                               |
|----------------------------------------------|
| $[(\blacksquare)^{2T}, X_5, L_3, W_2 + W_4]$ |
| $[(\blacksquare)^{2T}, X_5, L_3, W_2 + W_3]$ |
| $[(\blacksquare)^{2T}, X_5, L_3, W_1 + W_4]$ |
| $[(\blacksquare)^{2T}, X_5, L_3, W_1 + W_3]$ |

2nd minimal solution:  $\mu_2^T = 3$  (24 symmetry vectors)

Space group 217 ( $\mathbb{Z}_1$ )

1st minimal solution:  $\mu_1^T = 3$  (4 symmetry vectors)

| $\mathbf{n}^T$                                                              |
|-----------------------------------------------------------------------------|
| $[(\blacksquare)^{2T} + \Gamma_1, H_4, P_4, PA_4, N_1 + N_3 + N_4]$         |
| $[(\blacksquare)^{2T} + \Gamma_1, H_4, P_1 + P_3, PA_1 + PA_3, 2N_1 + N_2]$ |
| $[(\blacksquare)^{2T} + \Gamma_2, H_5, P_5, PA_5, N_2 + N_3 + N_4]$         |
| $[(\blacksquare)^{2T} + \Gamma_2, H_5, P_2 + P_3, PA_2 + PA_3, N_1 + 2N_2]$ |

2nd minimal solution:  $\mu_2^T = 4$  (14 symmetry vectors)

Space group 218 ( $\mathbb{Z}_2$ )

1st minimal solution:  $\mu_1^T = 2$  (2 symmetry vectors & filling-enforced topology)

| $\mathbf{n}^T$                               | $\mathbf{v}^T \in \mathbb{Z}_2$ |
|----------------------------------------------|---------------------------------|
| $[(\blacksquare)^{2T}, R_3, M_5, X_2 + X_3]$ | 1                               |
| $[(\blacksquare)^{2T}, R_3, M_5, X_1 + X_4]$ | 1                               |

2nd minimal solution:  $\mu_2^T = 4$  (16 symmetry vectors)

Space group 219 ( $\mathbb{Z}_2$ )

1st minimal solution:  $\mu_1^T = 2$  (4 symmetry vectors & filling-enforced topology)

| $\mathbf{n}^T$                               | $\mathbf{v}^T \in \mathbb{Z}_2$ |
|----------------------------------------------|---------------------------------|
| $[(\blacksquare)^{2T}, X_5, L_3, W_2 + W_3]$ | 1                               |
| $[(\blacksquare)^{2T}, X_5, L_3, W_2 + W_4]$ | 1                               |
| $[(\blacksquare)^{2T}, X_5, L_3, W_1 + W_3]$ | 1                               |
| $[(\blacksquare)^{2T}, X_5, L_3, W_1 + W_4]$ | 1                               |

2nd minimal solution:  $\mu_2^T = 4$  (68 symmetry vectors)

Space group 220 ( $\mathbb{Z}_2$ )

1st minimal solution:  $\mu_1^T = 2$  (4 symmetry vectors)

| $\mathbf{n}^T$                               | $\mathbf{v}^T \in \mathbb{Z}_2$ |
|----------------------------------------------|---------------------------------|
| $[(\blacksquare)^{2T}, H_3, P_1, PA_1, N_1]$ | trivial                         |
| $[(\blacksquare)^{2T}, H_3, P_1, PA_2, N_1]$ | 1                               |
| $[(\blacksquare)^{2T}, H_3, P_2, PA_1, N_1]$ | 1                               |
| $[(\blacksquare)^{2T}, H_3, P_2, PA_2, N_1]$ | trivial                         |

2nd minimal solution:  $\mu_2^T = 4$  (2 symmetry vectors)

Space group 221 ( $\mathbb{Z}_1$ )

1st minimal solution:  $\mu_1^T = 2$  (2 symmetry vectors)

| $\mathbf{n}^T$                                       |
|------------------------------------------------------|
| $[(\blacksquare)^{2T}, R_3^-, M_2^- + M_3^+, X_5^+]$ |
| $[(\blacksquare)^{2T}, R_3^+, M_2^+ + M_3^-, X_5^-]$ |

2nd minimal solution:  $\mu_2^T = 3$  (20 symmetry vectors)

Space group 222 ( $\mathbb{Z}_2$ )

1st minimal solution:  $\mu_1^T = 2$  (4 symmetry vectors & filling-enforced topology)

| $\mathbf{n}^T$                         | $\mathbf{v}^T \in \mathbb{Z}_2$ |
|----------------------------------------|---------------------------------|
| $[(\blacksquare)^{2T}, R_2, M_2, X_4]$ | 1                               |
| $[(\blacksquare)^{2T}, R_3, M_2, X_4]$ | 1                               |
| $[(\blacksquare)^{2T}, R_2, M_2, X_3]$ | 1                               |
| $[(\blacksquare)^{2T}, R_3, M_2, X_3]$ | 1                               |



2nd minimal solution:  $\mu_2^T = 4$  (8 symmetry vectors)

Space group 223 ( $\mathbb{Z}_1$ )

1st minimal solution:  $\mu_1^T = 6$  (30 symmetry vectors)

| $\mathbf{n}^T$                                                                                                              |
|-----------------------------------------------------------------------------------------------------------------------------|
| $[(\blacksquare)^{2T} + \Gamma_1^+ + \Gamma_5^-, R_4, M_3^+ + M_3^- + M_4^+ + M_4^- + M_5^+, X_1 + 2X_3]$                   |
| $[(\blacksquare)^{2T} + \Gamma_1^+ + \Gamma_5^-, R_4, M_1^- + M_2^+ + M_3^- + M_4^+ + M_5^+, X_1 + X_3 + X_4]$              |
| $[(\blacksquare)^{2T} + \Gamma_1^+ + \Gamma_2^+ + \Gamma_3^-, R_4, M_2^+ + M_3^+ + M_3^- + M_4^+ + M_5^+, X_1 + X_2 + X_3]$ |
| $[(\blacksquare)^{2T} + \Gamma_1^- + \Gamma_2^- + \Gamma_3^-, R_4, M_2^+ + M_3^+ + M_3^- + M_4^+ + M_5^-, 2X_2 + X_3]$      |
| $[(\blacksquare)^{2T} + \Gamma_1^+ + \Gamma_5^-, R_4, M_1^- + M_2^- + M_3^- + M_4^- + M_5^-, X_1 + X_3 + X_4]$              |
| $[(\blacksquare)^{2T} + \Gamma_1^+ + \Gamma_5^-, R_4, M_1^+ + M_2^- + M_3^+ + M_4^- + M_5^+, X_1 + X_3 + X_4]$              |
| $[(\blacksquare)^{2T} + \Gamma_1^+ + \Gamma_2^+ + \Gamma_3^-, R_4, M_2^- + M_3^+ + M_3^- + M_4^- + M_5^-, X_1 + X_2 + X_3]$ |
| $[(\blacksquare)^{2T} + \Gamma_1^+ + \Gamma_5^-, R_4, M_1^+ + M_1^- + M_2^+ + M_2^- + M_5^+, X_1 + 2X_4]$                   |
| $[(\blacksquare)^{2T} + \Gamma_1^+ + \Gamma_2^+ + \Gamma_3^-, R_4, M_1^- + M_2^+ + M_2^- + M_3^- + M_5^-, X_1 + X_2 + X_4]$ |
| $[(\blacksquare)^{2T} + \Gamma_1^+ + \Gamma_2^+ + \Gamma_3^-, R_4, M_1^+ + M_2^+ + M_2^- + M_3^+ + M_5^+, X_1 + X_2 + X_4]$ |
| $[(\blacksquare)^{2T} + \Gamma_1^- + \Gamma_2^- + \Gamma_3^-, R_4, M_1^+ + M_2^+ + M_2^- + M_3^+ + M_5^-, 2X_2 + X_4]$      |
| $[(\blacksquare)^{2T} + \Gamma_2^+ + \Gamma_4^-, R_4, M_2^+ + M_2^- + M_3^+ + M_3^- + M_5^+, X_1 + X_3 + X_4]$              |
| $[(\blacksquare)^{2T} + \Gamma_2^- + \Gamma_4^+, R_4, M_2^+ + M_2^- + M_3^+ + M_3^- + M_5^-, X_2 + X_3 + X_4]$              |
| $[(\blacksquare)^{2T} + \Gamma_1^+ + \Gamma_2^+ + \Gamma_3^+, R_4, M_2^- + M_3^+ + M_3^- + M_4^- + M_5^+, 2X_1 + X_3]$      |
| $[(\blacksquare)^{2T} + \Gamma_1^- + \Gamma_2^- + \Gamma_3^+, R_4, M_2^- + M_3^+ + M_3^- + M_4^- + M_5^-, X_1 + X_2 + X_3]$ |
| $[(\blacksquare)^{2T} + \Gamma_1^+ + \Gamma_2^+ + \Gamma_3^+, R_4, M_1^- + M_2^+ + M_2^- + M_3^- + M_5^+, 2X_1 + X_4]$      |
| $[(\blacksquare)^{2T} + \Gamma_1^- + \Gamma_2^- + \Gamma_3^+, R_4, M_1^- + M_2^+ + M_2^- + M_3^- + M_5^-, X_1 + X_2 + X_4]$ |
| $[(\blacksquare)^{2T} + \Gamma_1^+ + \Gamma_5^-, R_1 + 2R_2, 2M_5^+ + M_5^-, X_1 + X_3 + X_4]$                              |
| $[(\blacksquare)^{2T} + \Gamma_1^+ + \Gamma_5^-, R_1 + R_2 + R_3, 2M_5^+ + M_5^-, X_1 + X_3 + X_4]$                         |
| $[(\blacksquare)^{2T} + \Gamma_1^+ + \Gamma_5^-, R_1 + 2R_3, 2M_5^+ + M_5^-, X_1 + X_3 + X_4]$                              |
| $[(\blacksquare)^{2T} + \Gamma_1^- + \Gamma_5^+, R_4, M_3^+ + M_3^- + M_4^+ + M_4^- + M_5^-, X_2 + 2X_3]$                   |
| $[(\blacksquare)^{2T} + \Gamma_1^- + \Gamma_5^+, R_4, M_1^- + M_2^+ + M_3^- + M_4^+ + M_5^-, X_2 + X_3 + X_4]$              |
| $[(\blacksquare)^{2T} + \Gamma_1^- + \Gamma_5^+, R_4, M_1^+ + M_2^+ + M_3^+ + M_4^+ + M_5^+, X_2 + X_3 + X_4]$              |
| $[(\blacksquare)^{2T} + \Gamma_1^- + \Gamma_5^+, R_4, M_1^+ + M_2^- + M_3^+ + M_4^- + M_5^-, X_2 + X_3 + X_4]$              |
| $[(\blacksquare)^{2T} + \Gamma_1^- + \Gamma_5^+, R_4, M_1^+ + M_1^- + M_2^+ + M_2^- + M_5^-, X_2 + 2X_4]$                   |
| $[(\blacksquare)^{2T} + \Gamma_1^- + \Gamma_2^- + \Gamma_3^+, R_4, M_2^+ + M_3^+ + M_3^- + M_4^+ + M_5^+, X_1 + X_2 + X_3]$ |
| $[(\blacksquare)^{2T} + \Gamma_1^- + \Gamma_2^- + \Gamma_3^+, R_4, M_1^+ + M_2^+ + M_2^- + M_3^+ + M_5^+, X_1 + X_2 + X_4]$ |
| $[(\blacksquare)^{2T} + \Gamma_1^- + \Gamma_5^+, R_1 + 2R_2, M_5^+ + 2M_5^-, X_2 + X_3 + X_4]$                              |
| $[(\blacksquare)^{2T} + \Gamma_1^- + \Gamma_5^+, R_1 + R_2 + R_3, M_5^+ + 2M_5^-, X_2 + X_3 + X_4]$                         |
| $[(\blacksquare)^{2T} + \Gamma_1^- + \Gamma_5^+, R_1 + 2R_3, M_5^+ + 2M_5^-, X_2 + X_3 + X_4]$                              |

2nd minimal solution:  $\mu_2^T = 8$  (182 symmetry vectors)

Space group 224 ( $\mathbb{Z}_1$ )

1st minimal solution:  $\mu_1^T = 4$  (4 symmetry vectors)

| $\mathbf{n}^T$                                                                         |
|----------------------------------------------------------------------------------------|
| $[(\blacksquare)^{2T} + \Gamma_1^+ + \Gamma_2^-, R_2^- + R_4^-, M_1 + M_4, X_1 + X_3]$ |
| $[(\blacksquare)^{2T} + \Gamma_1^+ + \Gamma_2^-, R_1^+ + R_5^+, M_1 + M_4, X_1 + X_4]$ |
| $[(\blacksquare)^{2T} + \Gamma_1^- + \Gamma_2^+, R_2^+ + R_4^+, M_2 + M_4, X_2 + X_3]$ |
| $[(\blacksquare)^{2T} + \Gamma_1^- + \Gamma_2^+, R_1^- + R_5^-, M_2 + M_4, X_2 + X_4]$ |

2nd minimal solution:  $\mu_2^T = 6$  (22 symmetry vectors)

Space group 225 ( $\mathbb{Z}_1$ )

1st minimal solution:  $\mu_1^T = 3$  (8 symmetry vectors)

| $\mathbf{n}^T$                                                                |
|-------------------------------------------------------------------------------|
| $[(\blacksquare)^{2T} + \Gamma_1^+, X_3^- + X_5^-, L_2^- + L_3^-, W_2 + W_5]$ |
| $[(\blacksquare)^{2T} + \Gamma_1^+, X_3^- + X_5^-, L_1^+ + L_3^-, W_1 + W_5]$ |
| $[(\blacksquare)^{2T} + \Gamma_1^+, X_3^- + X_5^-, L_2^- + L_3^+, W_2 + W_5]$ |
| $[(\blacksquare)^{2T} + \Gamma_1^+, X_3^- + X_5^-, L_1^+ + L_3^+, W_1 + W_5]$ |
| $[(\blacksquare)^{2T} + \Gamma_1^-, X_3^+ + X_5^+, L_2^+ + L_3^-, W_3 + W_5]$ |
| $[(\blacksquare)^{2T} + \Gamma_1^-, X_3^+ + X_5^+, L_2^+ + L_3^+, W_3 + W_5]$ |
| $[(\blacksquare)^{2T} + \Gamma_1^-, X_3^+ + X_5^+, L_1^- + L_3^-, W_4 + W_5]$ |
| $[(\blacksquare)^{2T} + \Gamma_1^-, X_3^+ + X_5^+, L_1^- + L_3^+, W_4 + W_5]$ |

2nd minimal solution:  $\mu_2^T = 4$  (74 symmetry vectors)

Space group 226 ( $\mathbb{Z}_1$ )

1st minimal solution:  $\mu_1^T = 4$  (18 symmetry vectors)

| $\mathbf{n}^T$                                                                                       |
|------------------------------------------------------------------------------------------------------|
| $[(\blacksquare)^{2T} + \Gamma_1^+ + \Gamma_1^-, X_2^- + X_4^- + X_5^-, L_2 + L_3, W_2 + W_4 + W_5]$ |
| $[(\blacksquare)^{2T} + \Gamma_1^+ + \Gamma_1^-, X_2^- + X_4^- + X_5^-, L_2 + L_3, W_1 + W_3 + W_5]$ |
| $[(\blacksquare)^{2T} + \Gamma_1^+ + \Gamma_1^-, X_2^+ + X_4^+ + X_5^+, L_2 + L_3, W_2 + W_4 + W_5]$ |
| $[(\blacksquare)^{2T} + \Gamma_1^+ + \Gamma_1^-, X_2^+ + X_4^+ + X_5^+, L_2 + L_3, W_1 + W_3 + W_5]$ |
| $[(\blacksquare)^{2T} + \Gamma_1^+ + \Gamma_1^-, X_2^- + X_4^- + X_5^-, L_1 + L_3, W_2 + W_4 + W_5]$ |
| $[(\blacksquare)^{2T} + \Gamma_1^+ + \Gamma_1^-, X_2^- + X_4^- + X_5^-, L_1 + L_3, W_1 + W_3 + W_5]$ |
| $[(\blacksquare)^{2T} + \Gamma_1^+ + \Gamma_1^-, X_2^+ + X_4^+ + X_5^+, L_1 + L_3, W_2 + W_4 + W_5]$ |
| $[(\blacksquare)^{2T} + \Gamma_1^+ + \Gamma_1^-, X_2^+ + X_4^+ + X_5^+, L_1 + L_3, W_1 + W_3 + W_5]$ |
| $[(\blacksquare)^{2T} + \Gamma_3^-, X_2^- + X_3^+ + X_5^+, 2L_2, W_3 + W_4 + W_5]$                   |
| $[(\blacksquare)^{2T} + \Gamma_3^-, X_2^- + X_3^+ + X_5^+, L_1 + L_2, W_3 + W_4 + W_5]$              |
| $[(\blacksquare)^{2T} + \Gamma_3^-, X_2^- + X_3^+ + X_5^+, 2L_1, W_3 + W_4 + W_5]$                   |
| $[(\blacksquare)^{2T} + \Gamma_1^- + \Gamma_2^-, X_2^- + X_3^+ + X_5^+, L_2 + L_3, W_3 + W_4 + W_5]$ |
| $[(\blacksquare)^{2T} + \Gamma_1^- + \Gamma_2^-, X_2^- + X_3^+ + X_5^+, L_1 + L_3, W_3 + W_4 + W_5]$ |
| $[(\blacksquare)^{2T} + \Gamma_3^+, X_2^+ + X_3^- + X_5^-, 2L_2, W_1 + W_2 + W_5]$                   |
| $[(\blacksquare)^{2T} + \Gamma_3^+, X_2^+ + X_3^- + X_5^-, L_1 + L_2, W_1 + W_2 + W_5]$              |
| $[(\blacksquare)^{2T} + \Gamma_3^+, X_2^+ + X_3^- + X_5^-, 2L_1, W_1 + W_2 + W_5]$                   |
| $[(\blacksquare)^{2T} + \Gamma_1^+ + \Gamma_2^+, X_2^+ + X_3^- + X_5^-, L_2 + L_3, W_1 + W_2 + W_5]$ |
| $[(\blacksquare)^{2T} + \Gamma_1^+ + \Gamma_2^+, X_2^+ + X_3^- + X_5^-, L_1 + L_3, W_1 + W_2 + W_5]$ |

2nd minimal solution:  $\mu_2^T = 6$  (254 symmetry vectors)

Space group 227 ( $\mathbb{Z}_1$ )

1st minimal solution:  $\mu_1^T = 2$  (4 symmetry vectors)

| $\mathbf{n}^T$                           |
|------------------------------------------|
| $[(\blacksquare)^{2T}, X_4, L_3^-, W_1]$ |
| $[(\blacksquare)^{2T}, X_4, L_3^+, W_1]$ |
| $[(\blacksquare)^{2T}, X_4, L_3^-, W_2]$ |
| $[(\blacksquare)^{2T}, X_4, L_3^+, W_2]$ |

2nd minimal solution:  $\mu_2^T = 4$  (12 symmetry vectors)

Space group 228 ( $\mathbb{Z}_2$ )

1st minimal solution:  $\mu_1^T = 2$  (4 symmetry vectors & filling-enforced topology)

| $\mathbf{n}^T$                         | $\mathbf{v}^T \in \mathbb{Z}_2$ |
|----------------------------------------|---------------------------------|
| $[(\blacksquare)^{2T}, X_4, L_2, W_1]$ | 1                               |
| $[(\blacksquare)^{2T}, X_4, L_2, W_2]$ | 1                               |
| $[(\blacksquare)^{2T}, X_4, L_1, W_1]$ | 1                               |
| $[(\blacksquare)^{2T}, X_4, L_1, W_2]$ | 1                               |

2nd minimal solution:  $\mu_2^T = 6$  (48 symmetry vectors)

Space group 229 ( $\mathbb{Z}_1$ )

1st minimal solution:  $\mu_1^T = 3$  (6 symmetry vectors)

| $\mathbf{n}^T$                                                                |
|-------------------------------------------------------------------------------|
| $[(\blacksquare)^{2T} + \Gamma_1^+, H_4^-, P_4, N_2^- + N_3^- + N_4^-]$       |
| $[(\blacksquare)^{2T} + \Gamma_1^+, H_4^-, P_1 + P_3, N_1^+ + N_2^+ + N_2^-]$ |
| $[(\blacksquare)^{2T} + \Gamma_2^-, H_5^+, P_4, N_2^- + N_4^+ + N_4^-]$       |
| $[(\blacksquare)^{2T} + \Gamma_2^+, H_5^-, P_5, N_2^+ + N_4^+ + N_4^-]$       |
| $[(\blacksquare)^{2T} + \Gamma_1^-, H_4^+, P_5, N_2^+ + N_3^+ + N_4^+]$       |
| $[(\blacksquare)^{2T} + \Gamma_1^-, H_4^+, P_2 + P_3, N_1^- + N_2^+ + N_2^-]$ |

2nd minimal solution:  $\mu_2^T = 4$  (36 symmetry vectors)

Space group 230 ( $\mathbb{Z}_2$ )

1st minimal solution:  $\mu_1^T = 2$  (4 symmetry vectors & filling-enforced topology)

| $\mathbf{n}^T$                         | $\mathbf{v}^T \in \mathbb{Z}_2$ |
|----------------------------------------|---------------------------------|
| $[(\blacksquare)^{2T}, H_3, P_2, N_1]$ | 1                               |
| $[(\blacksquare)^{2T}, H_2, P_2, N_1]$ | 1                               |
| $[(\blacksquare)^{2T}, H_3, P_1, N_1]$ | 1                               |
| $[(\blacksquare)^{2T}, H_2, P_1, N_1]$ | 1                               |

2nd minimal solution:  $\mu_2^T = 6$  (4 symmetry vectors)

### C. Phononic $\Gamma$ -enforced topology (without time-reversal symmetry)

Below, we list the minimum-connectivity solutions in space group 218, 219, and 226 in a phononic setting with broken time-reversal symmetry. These space groups exhibit either fragile or mixed stable–fragile phononic  $\Gamma$ -enforced topology in their minimum-connectivity solutions (with  $\mu^{L+T} = 4$ ).

Space group 218 ( $\overline{P43n}$ ): mixed stable–fragile  $\Gamma$ -enforced topology

| <b>n</b>                                                                       | <b>Topology</b> |
|--------------------------------------------------------------------------------|-----------------|
| $[(\Gamma_4)^{2T+1L} + \Gamma_2, R_2 + R_4, M_3 + M_4 + M_5, X_1 + X_2 + X_5]$ | nontrivial      |
| $[(\Gamma_4)^{2T+1L} + \Gamma_2, R_2 + R_4, M_1 + M_2 + M_5, X_3 + X_4 + X_5]$ | nontrivial      |
| $[(\Gamma_4)^{2T+1L} + \Gamma_2, R_1 + R_5, M_3 + M_4 + M_5, X_1 + X_2 + X_5]$ | nontrivial      |
| $[(\Gamma_4)^{2T+1L} + \Gamma_2, R_1 + R_5, M_1 + M_2 + M_5, X_3 + X_4 + X_5]$ | nontrivial      |
| $[(\Gamma_4)^{2T+1L} + \Gamma_2, R_1 + R_2 + R_3, 2M_5, X_2 + X_3 + X_5]$      | nontrivial      |
| $[(\Gamma_4)^{2T+1L} + \Gamma_2, R_1 + R_2 + R_3, 2M_5, X_1 + X_4 + X_5]$      | nontrivial      |
| $[(\Gamma_4)^{2T+1L} + \Gamma_2, R_2 + R_4, M_2 + M_3 + M_5, X_2 + X_3 + X_5]$ | fragile         |
| $[(\Gamma_4)^{2T+1L} + \Gamma_2, R_2 + R_4, M_2 + M_3 + M_5, X_1 + X_4 + X_5]$ | fragile         |
| $[(\Gamma_4)^{2T+1L} + \Gamma_2, R_2 + R_4, M_1 + M_4 + M_5, X_2 + X_3 + X_5]$ | fragile         |
| $[(\Gamma_4)^{2T+1L} + \Gamma_2, R_2 + R_4, M_1 + M_4 + M_5, X_1 + X_4 + X_5]$ | fragile         |
| $[(\Gamma_4)^{2T+1L} + \Gamma_2, R_1 + R_5, M_2 + M_3 + M_5, X_2 + X_3 + X_5]$ | fragile         |
| $[(\Gamma_4)^{2T+1L} + \Gamma_2, R_1 + R_5, M_2 + M_3 + M_5, X_1 + X_4 + X_5]$ | fragile         |
| $[(\Gamma_4)^{2T+1L} + \Gamma_2, R_1 + R_5, M_1 + M_4 + M_5, X_2 + X_3 + X_5]$ | fragile         |
| $[(\Gamma_4)^{2T+1L} + \Gamma_2, R_1 + R_5, M_1 + M_4 + M_5, X_1 + X_4 + X_5]$ | fragile         |

Space group 219 ( $\overline{F43c}$ ): mixed stable–fragile  $\Gamma$ -enforced topology

| <b>n</b>                                                                                   | <b>Topology</b> |
|--------------------------------------------------------------------------------------------|-----------------|
| $[(\Gamma_4)^{2T+1L} + \Gamma_2, X_2 + X_3 + X_5, L_1 + L_2 + L_3, 2W_2 + 2W_4]$           | fragile         |
| $[(\Gamma_4)^{2T+1L} + \Gamma_2, X_2 + X_3 + X_5, L_1 + L_2 + L_3, 2W_2 + W_3 + W_4]$      | fragile         |
| $[(\Gamma_4)^{2T+1L} + \Gamma_2, X_2 + X_3 + X_5, L_1 + L_2 + L_3, 2W_2 + 2W_3]$           | fragile         |
| $[(\Gamma_4)^{2T+1L} + \Gamma_2, X_2 + X_3 + X_5, L_1 + L_2 + L_3, W_1 + W_2 + 2W_4]$      | fragile         |
| $[(\Gamma_4)^{2T+1L} + \Gamma_2, X_2 + X_3 + X_5, L_1 + L_2 + L_3, W_1 + W_2 + W_3 + W_4]$ | fragile         |
| $[(\Gamma_4)^{2T+1L} + \Gamma_2, X_2 + X_3 + X_5, L_1 + L_2 + L_3, W_1 + W_2 + 2W_3]$      | fragile         |
| $[(\Gamma_4)^{2T+1L} + \Gamma_2, X_2 + X_3 + X_5, L_1 + L_2 + L_3, 2W_1 + 2W_4]$           | fragile         |
| $[(\Gamma_4)^{2T+1L} + \Gamma_2, X_2 + X_3 + X_5, L_1 + L_2 + L_3, 2W_1 + W_3 + W_4]$      | fragile         |
| $[(\Gamma_4)^{2T+1L} + \Gamma_2, X_2 + X_3 + X_5, L_1 + L_2 + L_3, 2W_1 + 2W_3]$           | fragile         |
| $[(\Gamma_4)^{2T+1L} + \Gamma_2, X_1 + X_4 + X_5, L_1 + L_2 + L_3, 2W_2 + 2W_4]$           | fragile         |
| $[(\Gamma_4)^{2T+1L} + \Gamma_2, X_1 + X_4 + X_5, L_1 + L_2 + L_3, 2W_2 + W_3 + W_4]$      | fragile         |
| $[(\Gamma_4)^{2T+1L} + \Gamma_2, X_1 + X_4 + X_5, L_1 + L_2 + L_3, 2W_2 + 2W_3]$           | fragile         |
| $[(\Gamma_4)^{2T+1L} + \Gamma_2, X_1 + X_4 + X_5, L_1 + L_2 + L_3, W_1 + W_2 + 2W_4]$      | fragile         |
| $[(\Gamma_4)^{2T+1L} + \Gamma_2, X_1 + X_4 + X_5, L_1 + L_2 + L_3, W_1 + W_2 + W_3 + W_4]$ | fragile         |
| $[(\Gamma_4)^{2T+1L} + \Gamma_2, X_1 + X_4 + X_5, L_1 + L_2 + L_3, W_1 + W_2 + 2W_3]$      | fragile         |
| $[(\Gamma_4)^{2T+1L} + \Gamma_2, X_1 + X_4 + X_5, L_1 + L_2 + L_3, 2W_1 + 2W_4]$           | fragile         |
| $[(\Gamma_4)^{2T+1L} + \Gamma_2, X_1 + X_4 + X_5, L_1 + L_2 + L_3, 2W_1 + W_3 + W_4]$      | fragile         |
| $[(\Gamma_4)^{2T+1L} + \Gamma_2, X_1 + X_4 + X_5, L_1 + L_2 + L_3, 2W_1 + 2W_3]$           | fragile         |
| $[(\Gamma_4)^{2T+1L} + \Gamma_2, X_3 + X_4 + X_5, L_1 + L_2 + L_3, W_2 + 3W_4]$            | nontrivial      |
| $[(\Gamma_4)^{2T+1L} + \Gamma_2, X_3 + X_4 + X_5, L_1 + L_2 + L_3, W_2 + W_3 + 2W_4]$      | nontrivial      |
| $[(\Gamma_4)^{2T+1L} + \Gamma_2, X_3 + X_4 + X_5, L_1 + L_2 + L_3, W_2 + 2W_3 + W_4]$      | nontrivial      |
| $[(\Gamma_4)^{2T+1L} + \Gamma_2, X_3 + X_4 + X_5, L_1 + L_2 + L_3, W_2 + 3W_3]$            | nontrivial      |
| $[(\Gamma_4)^{2T+1L} + \Gamma_2, X_3 + X_4 + X_5, L_1 + L_2 + L_3, W_1 + 3W_4]$            | nontrivial      |

... continued on next page

... continued from previous page

|                                                                                       |            |
|---------------------------------------------------------------------------------------|------------|
| $[(\Gamma_4)^{2T+1L} + \Gamma_2, X_3 + X_4 + X_5, L_1 + L_2 + L_3, W_1 + W_3 + 2W_4]$ | nontrivial |
| $[(\Gamma_4)^{2T+1L} + \Gamma_2, X_3 + X_4 + X_5, L_1 + L_2 + L_3, W_1 + 2W_3 + W_4]$ | nontrivial |
| $[(\Gamma_4)^{2T+1L} + \Gamma_2, X_3 + X_4 + X_5, L_1 + L_2 + L_3, W_1 + 3W_3]$       | nontrivial |
| $[(\Gamma_4)^{2T+1L} + \Gamma_2, X_1 + X_2 + X_5, L_1 + L_2 + L_3, 3W_2 + W_4]$       | nontrivial |
| $[(\Gamma_4)^{2T+1L} + \Gamma_2, X_1 + X_2 + X_5, L_1 + L_2 + L_3, 3W_2 + W_3]$       | nontrivial |
| $[(\Gamma_4)^{2T+1L} + \Gamma_2, X_1 + X_2 + X_5, L_1 + L_2 + L_3, W_1 + 2W_2 + W_4]$ | nontrivial |
| $[(\Gamma_4)^{2T+1L} + \Gamma_2, X_1 + X_2 + X_5, L_1 + L_2 + L_3, W_1 + 2W_2 + W_3]$ | nontrivial |
| $[(\Gamma_4)^{2T+1L} + \Gamma_2, X_1 + X_2 + X_5, L_1 + L_2 + L_3, 2W_1 + W_2 + W_4]$ | nontrivial |
| $[(\Gamma_4)^{2T+1L} + \Gamma_2, X_1 + X_2 + X_5, L_1 + L_2 + L_3, 2W_1 + W_2 + W_3]$ | nontrivial |
| $[(\Gamma_4)^{2T+1L} + \Gamma_2, X_1 + X_2 + X_5, L_1 + L_2 + L_3, 3W_1 + W_4]$       | nontrivial |
| $[(\Gamma_4)^{2T+1L} + \Gamma_2, X_1 + X_2 + X_5, L_1 + L_2 + L_3, 3W_1 + W_3]$       | nontrivial |

Space group 226 ( $Fm\bar{3}c$ ): fragile  $\Gamma$ -enforced topology

| <b>n</b>                                                                                 | <b>Topology</b> |
|------------------------------------------------------------------------------------------|-----------------|
| $[(\Gamma_4^-)^{2T+1L} + \Gamma_2^+, X_2^+ + X_3^- + X_5^-, L_2 + L_3, W_1 + W_2 + W_5]$ | fragile         |
| $[(\Gamma_4^-)^{2T+1L} + \Gamma_2^+, X_2^+ + X_3^- + X_5^-, L_1 + L_3, W_1 + W_2 + W_5]$ | fragile         |
| $[(\Gamma_4^-)^{2T+1L} + \Gamma_1^-, X_2^- + X_4^- + X_5^-, L_2 + L_3, W_2 + W_4 + W_5]$ | fragile         |
| $[(\Gamma_4^-)^{2T+1L} + \Gamma_1^-, X_2^- + X_4^- + X_5^-, L_2 + L_3, W_1 + W_3 + W_5]$ | fragile         |
| $[(\Gamma_4^-)^{2T+1L} + \Gamma_1^-, X_2^- + X_4^- + X_5^-, L_1 + L_3, W_2 + W_4 + W_5]$ | fragile         |
| $[(\Gamma_4^-)^{2T+1L} + \Gamma_1^-, X_2^- + X_4^- + X_5^-, L_1 + L_3, W_1 + W_3 + W_5]$ | fragile         |
| $[(\Gamma_4^-)^{2T+1L} + \Gamma_1^-, X_2^+ + X_4^+ + X_5^+, L_2 + L_3, W_2 + W_4 + W_5]$ | fragile         |
| $[(\Gamma_4^-)^{2T+1L} + \Gamma_1^-, X_2^+ + X_4^+ + X_5^+, L_2 + L_3, W_1 + W_3 + W_5]$ | fragile         |
| $[(\Gamma_4^-)^{2T+1L} + \Gamma_1^-, X_2^+ + X_4^+ + X_5^+, L_1 + L_3, W_2 + W_4 + W_5]$ | fragile         |
| $[(\Gamma_4^-)^{2T+1L} + \Gamma_1^-, X_2^+ + X_4^+ + X_5^+, L_1 + L_3, W_1 + W_3 + W_5]$ | fragile         |
